# Supplementary material for: STREAMLINE: An Automated Machine Learning Pipeline for Biomedicine Applied to Examine the Utility of Photography-Based Phenotypes for OSA Prediction Across International Sleep Centers
Source: arXiv:2312.05461 ancillary file (2023-12-09)
Supplement: Supplementary file 2 [file gametes_exp_STREAMLINE_Report.pdf]

# STREAMLINE Testing Data Evaluation Report: 2023-09-26 12:47:00.811732

## General Pipeline Settings:

CV Partitions: 10  
Partition Method: Stratified  
Categorical Cutoff: 2  
Statistical Significance Cutoff: 0.05  
Random Seed: 42  
Run From Notebook: False

## Feature Importance/Selection Settings:

Use Mutual Information: True  
Use MultiSURF: True  
Use TURF: False  
TURF Cutoff: 0.5  
MultiSURF Instance Subset: 2000  
Max Features to Keep: 2000  
Filter Poor Features: True  
Top Features to Display: 40  
Export Feature Importance Plot: True

## ML Modeling Algorithms:

Artificial Neural Network: True  
Category Gradient Boosting: True  
Decision Tree: True  
Elastic Net: True  
ExSTraCS: True  
Extreme Gradient Boosting: True  
Genetic Programming: True  
Gradient Boosting: True  
K-Nearest Neighbors: True  
Light Gradient Boosting: True  
Logistic Regression: True  
Naive Bayes: True  
Random Forest: True  
Support Vector Machine: True  
XCS: False  
eLCS: False

## Modeling Settings:

Primary Metric: balanced\_accuracy  
Training Subsample for KNN,ANN,SVM,and XGB: 0  
Uniform Feature Importance Estimation (Models): True  
Hyperparameter Sweep Number of Trials: 200  
Hyperparameter Timeout: 900  
Export Hyperparameter Sweep Plots: False

## LCS Settings (eLCS,XCS,ExSTraCS):

Do LCS Hyperparameter Sweep: False  
nu: 1  
Training Iterations: 200000  
N (Rule Population Size): 2000  
LCS Hyperparameter Sweep Timeout: 1200

## Stats and Figure Settings:

Export ROC Plot: True  
Export PRC Plot: True  
Export Metric Boxplots: True  
Export Feature Importance Boxplots: True  
Metric Weighting Composite FI Plots: balanced\_accuracy  
Top Model Features To Display: 40

## EDA and Processing Settings:

Engineering Missingness Cutoff: 0.5  
Cleaning Missingness Cutoff: 0.5  
Correlation Removal Threshold: 1.0  
List of Exploratory Analysis Ran: ['Describe', 'Univariate Analysis', 'Feature Correlation']  
List of Exploratory Plots Saved: ['Describe', 'Univariate Analysis', 'Feature Correlation']  
Use Data Scaling: True  
Use Data Imputation: True  
Use Multivariate Imputation: True  
Overwrite CV Datasets: True

## Target Dataset(s):

D1 = A\_gametes\_univariate\_L\_1\_H\_0  
D2 = B\_gametes\_uni\_4add\_L\_1\_H\_0  
D3 = C\_gametes\_uni\_4het\_L\_1\_H\_0  
D4 = D\_gametes\_2way\_epistasis\_L\_2\_H\_0  
D5 = E\_gametes\_2way\_epi\_2het\_L\_2\_H\_0  
D6 = F\_gametes\_3way\_epistasis\_L\_3\_H\_0

## Target Data Settings:

Data Path: /home/ryanurb/idata/datasets/GAMETES\_set  
Output Path: /home/ryanurb/idata/output  
Experiment Name: gametes\_exp  
Class Label: Class  
Instance Label: None  
Match Label: None  
Ignored Features: None  
Specified Categorical Features: None  
Specified Quantitative Features: None

# Univariate Analysis of Each Dataset (Top 10 Features for Each): Page 1

## D1 = A\_gametes\_univariate\_L\_1\_H\_0

| Feature | p-value                | Test-statistic     | Test-name           |
|---------|------------------------|--------------------|---------------------|
| M0P0    | 1.958445526403697e-142 | 113208.5           | Mann-Whitney U Test |
| N93     | 0.0005869443443839     | 295274.0           | Mann-Whitney U Test |
| N34     | 0.0318727566416838     | 305350.0           | Mann-Whitney U Test |
| N11     | 0.0329670391575441     | 304400.0           | Mann-Whitney U Test |
| N87     | 0.0367714989196929     | 337716.0           | Mann-Whitney U Test |
| N7      | 0.039318187888567      | 303884.5           | Mann-Whitney U Test |
| N67     | 0.0439355371489448     | 329084.5           | Mann-Whitney U Test |
| N26     | 0.0627459103393591     | 335695.0           | Mann-Whitney U Test |
| N18     | 0.0680671826646687     | 3.3290257560610863 | Chi Square Test     |
| N75     | 0.0774530383976894     | 305498.0           | Mann-Whitney U Test |

## D2 = B\_gametes\_uni\_4add\_L\_1\_H\_0

| Feature | p-value                 | Test-statistic | Test-name           |
|---------|-------------------------|----------------|---------------------|
| M0P0    | 1.471380000793489e-150  | 106640.0       | Mann-Whitney U Test |
| M2P0    | 1.6368544175573264e-141 | 113824.5       | Mann-Whitney U Test |
| M1P0    | 6.215433181178304e-136  | 117164.5       | Mann-Whitney U Test |
| M3P0    | 9.925925684541387e-121  | 129140.0       | Mann-Whitney U Test |
| N43     | 0.0265774314170957      | 301812.0       | Mann-Whitney U Test |
| N37     | 0.0423614597785156      | 304896.0       | Mann-Whitney U Test |
| N66     | 0.0460956754762378      | 336579.5       | Mann-Whitney U Test |
| N25     | 0.0637403816827963      | 335357.5       | Mann-Whitney U Test |
| N30     | 0.0664324935378486      | 304545.5       | Mann-Whitney U Test |
| N69     | 0.0724149243714784      | 334900.0       | Mann-Whitney U Test |

## D3 = C\_gametes\_uni\_4het\_L\_1\_H\_0

| Feature | p-value               | Test-statistic | Test-name           |
|---------|-----------------------|----------------|---------------------|
| M2P0    | 4.27370154275195e-13  | 262858.0       | Mann-Whitney U Test |
| M1P0    | 7.193239751163257e-11 | 268436.0       | Mann-Whitney U Test |
| M0P0    | 8.192797422973474e-10 | 271749.0       | Mann-Whitney U Test |
| M3P0    | 3.612194136758094e-07 | 280086.5       | Mann-Whitney U Test |
| N32     | 0.0096959448819325    | 300362.5       | Mann-Whitney U Test |
| N60     | 0.0409333271555459    | 337349.0       | Mann-Whitney U Test |
| N81     | 0.0445570714888509    | 308496.5       | Mann-Whitney U Test |
| N30     | 0.0519049579636733    | 309404.0       | Mann-Whitney U Test |
| N11     | 0.0519844482092975    | 308259.0       | Mann-Whitney U Test |
| N2      | 0.0540101201061311    | 308870.0       | Mann-Whitney U Test |

## D4 = D\_gametes\_2way\_epistasis\_L\_2\_H\_0

| Feature | p-value            | Test-statistic | Test-name           |
|---------|--------------------|----------------|---------------------|
| N39     | 0.0235658209543952 | 337524.5       | Mann-Whitney U Test |
| N94     | 0.0410675952102596 | 302719.5       | Mann-Whitney U Test |
| N53     | 0.0490391377720209 | 312409.5       | Mann-Whitney U Test |
| N41     | 0.0607311281102123 | 326013.0       | Mann-Whitney U Test |
| N10     | 0.0609599842500847 | 304550.0       | Mann-Whitney U Test |
| N49     | 0.0722031977660922 | 334607.0       | Mann-Whitney U Test |
| N51     | 0.0734045452519738 | 304928.0       | Mann-Whitney U Test |
| N17     | 0.0859610449206753 | 309361.0       | Mann-Whitney U Test |
| N21     | 0.087381229983095  | 305565.5       | Mann-Whitney U Test |
| N59     | 0.1085615361646212 | 306517.5       | Mann-Whitney U Test |

## D5 = E\_gametes\_2way\_epi\_2het\_L\_2\_H\_0

| Feature | p-value            | Test-statistic | Test-name           |
|---------|--------------------|----------------|---------------------|
| N8      | 0.0018129531110294 | 346469.0       | Mann-Whitney U Test |
| N16     | 0.0201899721208968 | 306538.5       | Mann-Whitney U Test |
| N51     | 0.0336266435907043 | 301946.5       | Mann-Whitney U Test |
| N67     | 0.0382978809738868 | 306204.0       | Mann-Whitney U Test |
| N49     | 0.0439192709155552 | 302954.0       | Mann-Whitney U Test |
| N45     | 0.0461416535866234 | 305592.0       | Mann-Whitney U Test |
| N10     | 0.0591962576653912 | 333221.5       | Mann-Whitney U Test |
| N85     | 0.0610039429019777 | 309972.5       | Mann-Whitney U Test |
| N1      | 0.0878804063404616 | 305741.0       | Mann-Whitney U Test |
| N62     | 0.1111376714150672 | 306487.0       | Mann-Whitney U Test |

D6 = F\_gametes\_3way\_epistasis\_L\_3\_H\_0

| Feature | p-value            | Test-statistic | Test-name           |
|---------|--------------------|----------------|---------------------|
| N32     | 0.0185514813514058 | 307976.5       | Mann-Whitney U Test |
| N79     | 0.0270732672312567 | 303067.0       | Mann-Whitney U Test |
| N77     | 0.0498828284381861 | 307111.5       | Mann-Whitney U Test |
| N6      | 0.0536032527165466 | 336223.0       | Mann-Whitney U Test |
| N29     | 0.0713730028400286 | 304582.5       | Mann-Whitney U Test |
| N35     | 0.0785710868445943 | 305065.0       | Mann-Whitney U Test |
| N70     | 0.105612608591244  | 329504.0       | Mann-Whitney U Test |
| N18     | 0.1089636461676558 | 307398.0       | Mann-Whitney U Test |
| N73     | 0.1114483736672534 | 333272.0       | Mann-Whitney U Test |
| N3      | 0.1261389109163312 | 329269.5       | Mann-Whitney U Test |

# Dataset and Model Prediction Summary: D1 = A\_gametes\_univariate\_L\_1\_H\_0

## Data Processing/Counts Summary

|           | Instances | Total Features | Categorical Features | Quantitative Features | Missing Values | Missing Percent | Class 0 | Class 1 |
|-----------|-----------|----------------|----------------------|-----------------------|----------------|-----------------|---------|---------|
| Original  | 1600      | 100            | 2                    | 98                    | 0              | 0.0             | 800     | 800     |
| C1        | 1600      | 100            | 2                    | 98                    | 0              | 0.0             | 800     | 800     |
| E1        | 1600      | 100            | 2                    | 98                    | 0              | 0.0             | 800     | 800     |
| C2        | 1600      | 100            | 2                    | 98                    | 0              | 0.0             | 800     | 800     |
| C3        | 1600      | 100            | 2                    | 98                    | 0              | 0.0             | 800     | 800     |
| E2        | 1600      | 100            | 2                    | 98                    | 0              | 0.0             | 800     | 800     |
| C4        | 1600      | 100            | 2                    | 98                    | 0              | 0.0             | 800     | 800     |
| Processed | 1600      | 100            | 2                    | 98                    | 0              | 0.0             | 800     | 800     |

## Cleaning (C) and Engineering (E) Elements

- \* C1 - Remove instances with no outcome and features to ignore
- \* E1 - Add missingness features
- \* C2 - Remove features with invariance or high missingness
- \* C3 - Remove instances with high missingness
- \* E2 - Add one-hot-encoding of categorical features
- \* C4 - Remove highly correlated features

## Class Balance (Processed)

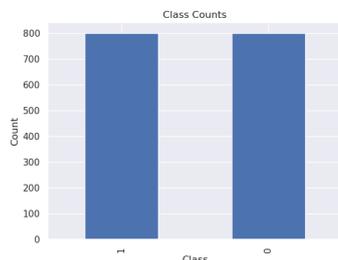

## Feature Correlations (Pearson)

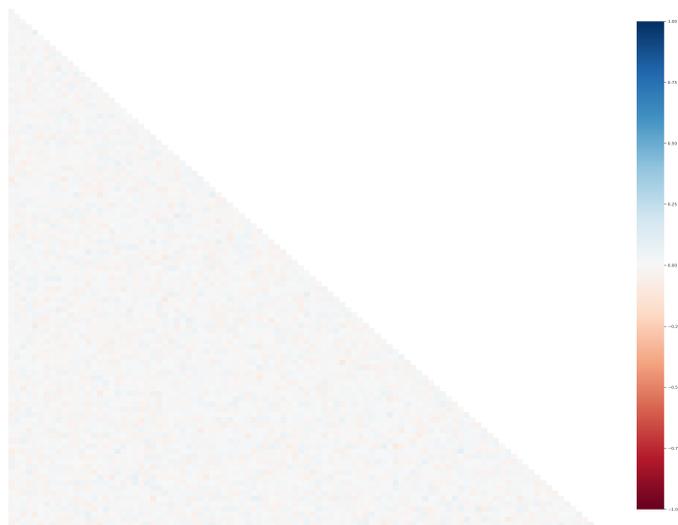

## Top ML Algorithm Results (Averaged Over CV Runs):

|                                                                |
|----------------------------------------------------------------|
| Best (ROC_AUC): Random Forest = 0.852                          |
| Best (Balanced Acc.): Category Gradient Boosting (TIE) = 0.829 |
| Best (F1 Score): Category Gradient Boosting (TIE) = 0.826      |
| Best (PRC AUC): Genetic Programming = 0.875                    |
| Best (PRC APS): Random Forest = 0.826                          |

## ROC

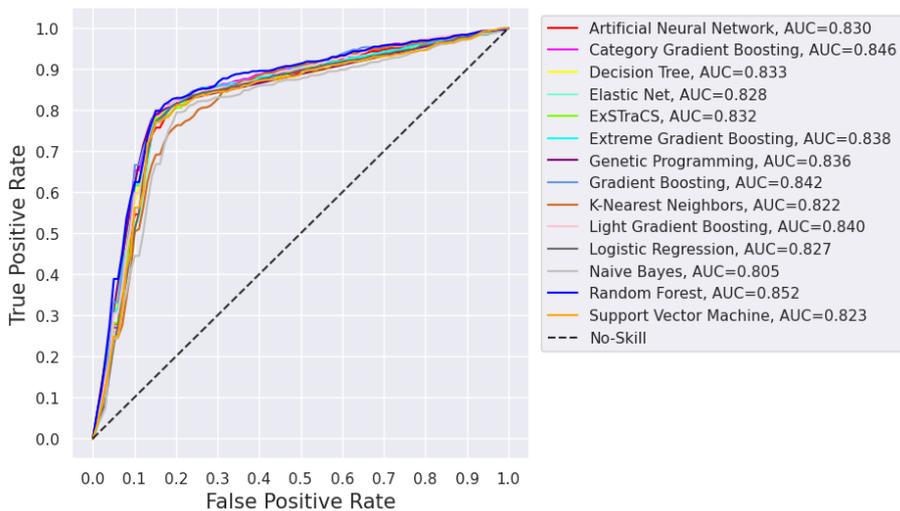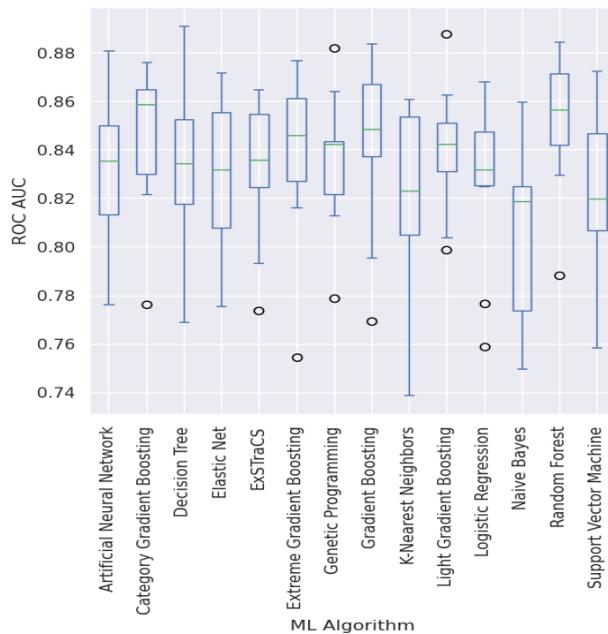

## PRC

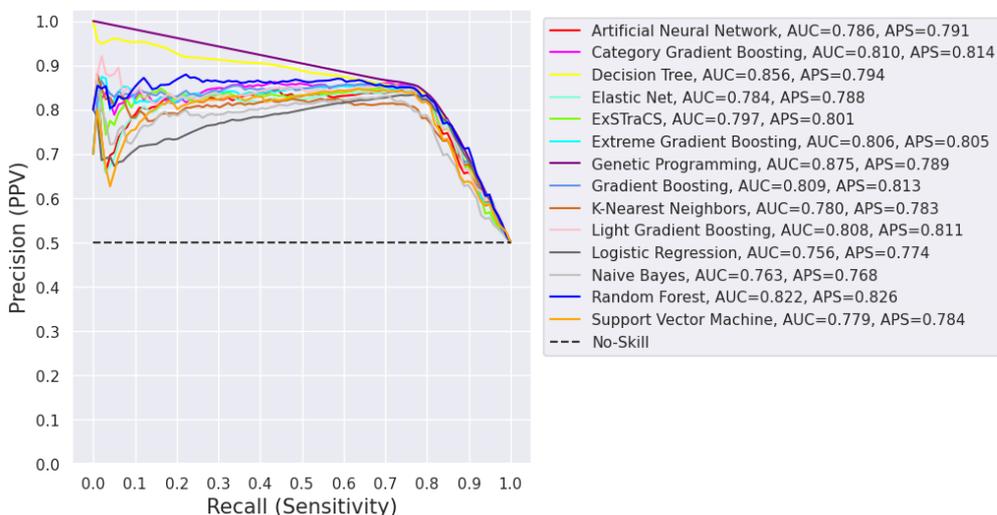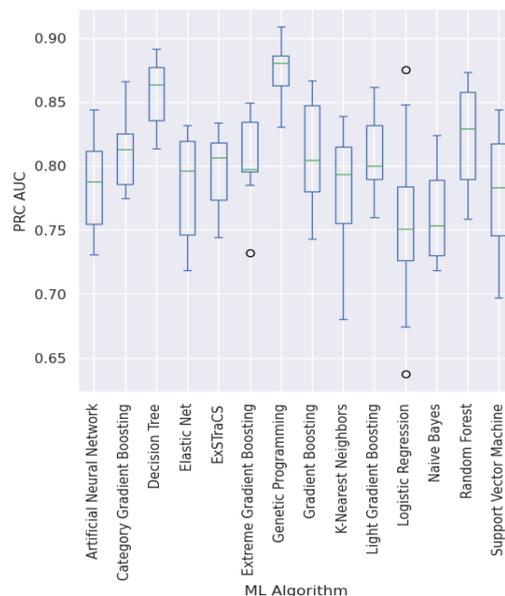

# Dataset and Model Prediction Summary: D2 = B\_gametes\_uni\_4add\_L\_1\_H\_0

## Data Processing/Counts Summary

|           | Instances | Total Features | Categorical Features | Quantitative Features | Missing Values | Missing Percent | Class 0 | Class 1 |
|-----------|-----------|----------------|----------------------|-----------------------|----------------|-----------------|---------|---------|
| Original  | 1600      | 100            | 1                    | 99                    | 0              | 0.0             | 800     | 800     |
| C1        | 1600      | 100            | 1                    | 99                    | 0              | 0.0             | 800     | 800     |
| E1        | 1600      | 100            | 1                    | 99                    | 0              | 0.0             | 800     | 800     |
| C2        | 1600      | 100            | 1                    | 99                    | 0              | 0.0             | 800     | 800     |
| C3        | 1600      | 100            | 1                    | 99                    | 0              | 0.0             | 800     | 800     |
| E2        | 1600      | 100            | 1                    | 99                    | 0              | 0.0             | 800     | 800     |
| C4        | 1600      | 100            | 1                    | 99                    | 0              | 0.0             | 800     | 800     |
| Processed | 1600      | 100            | 1                    | 99                    | 0              | 0.0             | 800     | 800     |

## Cleaning (C) and Engineering (E) Elements

- \* C1 - Remove instances with no outcome and features to ignore
- \* E1 - Add missingness features
- \* C2 - Remove features with invariance or high missingness
- \* C3 - Remove instances with high missingness
- \* E2 - Add one-hot-encoding of categorical features
- \* C4 - Remove highly correlated features

## Class Balance (Processed)

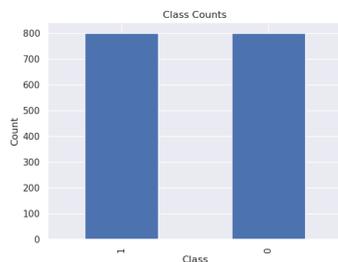

## Feature Correlations (Pearson)

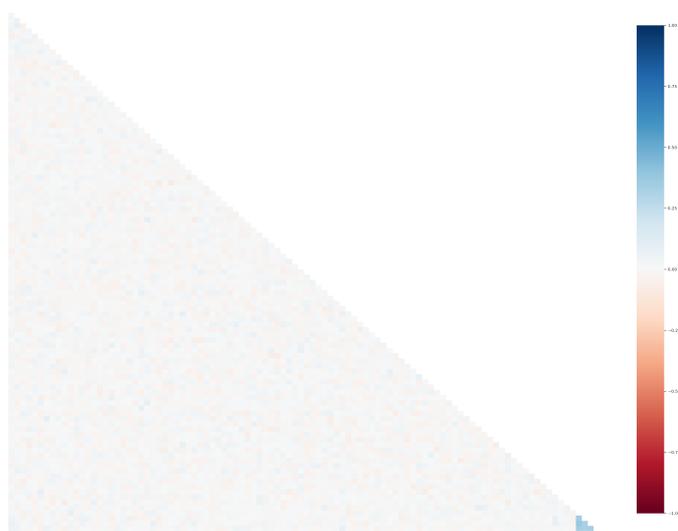

## Top ML Algorithm Results (Averaged Over CV Runs):

|                                                                |
|----------------------------------------------------------------|
| Best (ROC_AUC): ExSTraCS = 0.983                               |
| Best (Balanced Acc.): Category Gradient Boosting (TIE) = 0.931 |
| Best (F1 Score): Extreme Gradient Boosting = 0.932             |
| Best (PRC AUC): ExSTraCS = 0.981                               |
| Best (PRC APS): ExSTraCS = 0.981                               |

## ROC

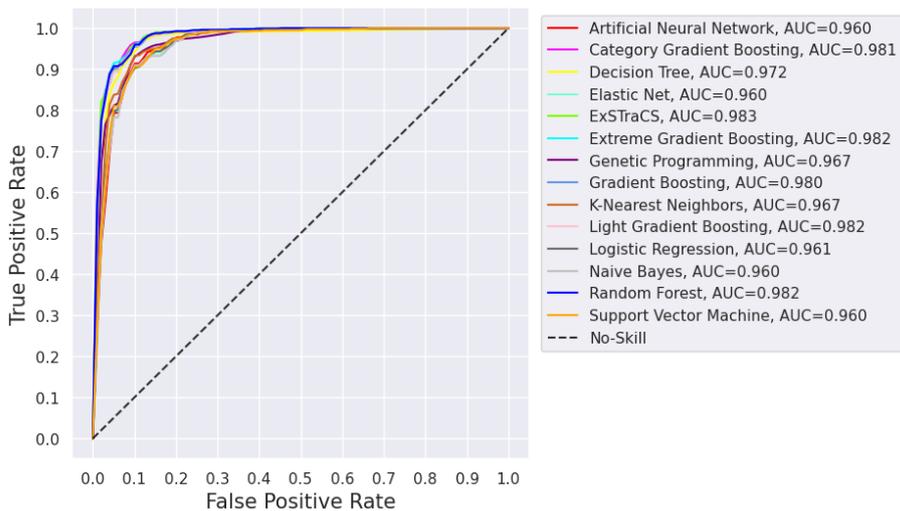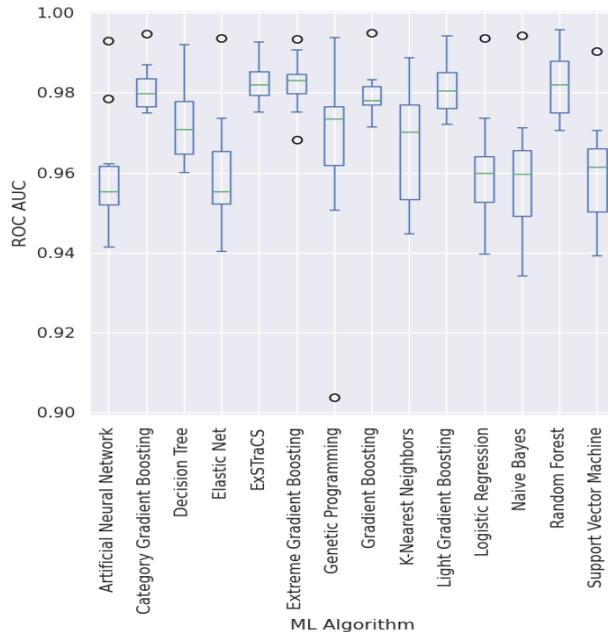

## PRC

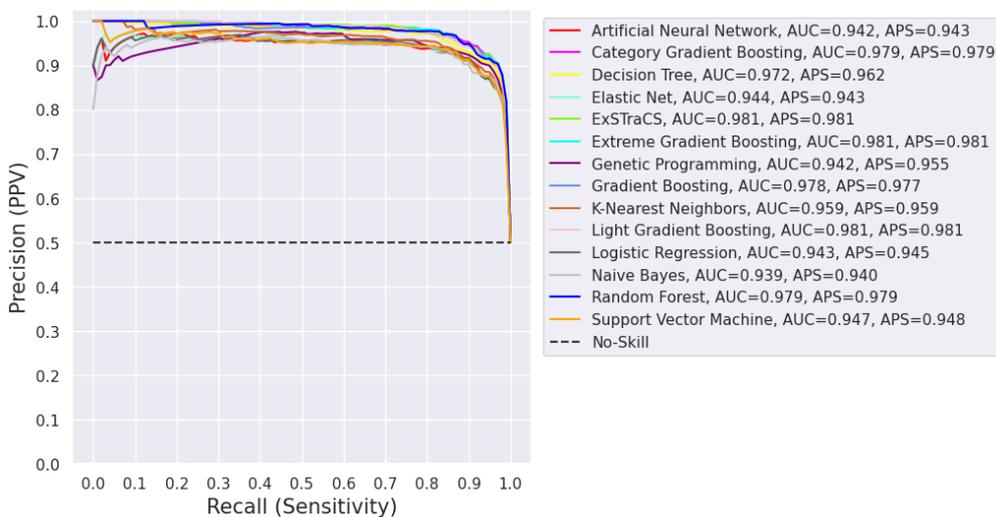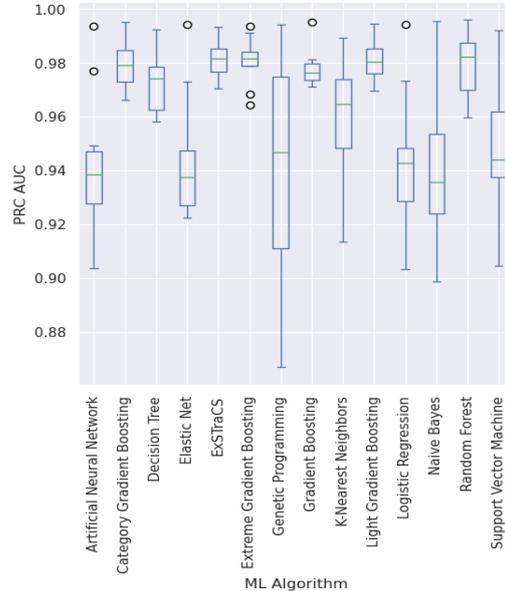

# Dataset and Model Prediction Summary: D3 = C\_gametes\_uni\_4het\_L\_1\_H\_0

## Data Processing/Counts Summary

|           | Instances | Total Features | Categorical Features | Quantitative Features | Missing Values | Missing Percent | Class 0 | Class 1 |
|-----------|-----------|----------------|----------------------|-----------------------|----------------|-----------------|---------|---------|
| Original  | 1600      | 100            | 0                    | 100                   | 0              | 0.0             | 800     | 800     |
| C1        | 1600      | 100            | 0                    | 100                   | 0              | 0.0             | 800     | 800     |
| E1        | 1600      | 100            | 0                    | 100                   | 0              | 0.0             | 800     | 800     |
| C2        | 1600      | 100            | 0                    | 100                   | 0              | 0.0             | 800     | 800     |
| C3        | 1600      | 100            | 0                    | 100                   | 0              | 0.0             | 800     | 800     |
| E2        | 1600      | 100            | 0                    | 100                   | 0              | 0.0             | 800     | 800     |
| C4        | 1600      | 100            | 0                    | 100                   | 0              | 0.0             | 800     | 800     |
| Processed | 1600      | 100            | 0                    | 100                   | 0              | 0.0             | 800     | 800     |

## Cleaning (C) and Engineering (E) Elements

- \* C1 - Remove instances with no outcome and features to ignore
- \* E1 - Add missingness features
- \* C2 - Remove features with invariance or high missingness
- \* C3 - Remove instances with high missingness
- \* E2 - Add one-hot-encoding of categorical features
- \* C4 - Remove highly correlated features

## Class Balance (Processed)

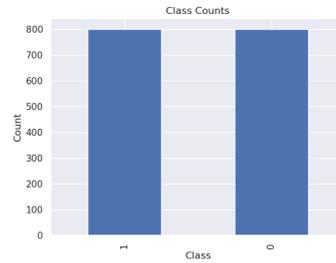

## Feature Correlations (Pearson)

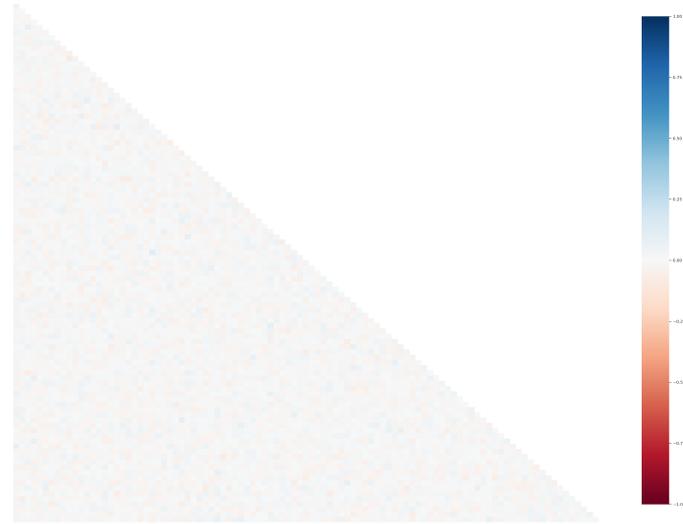

## Top ML Algorithm Results (Averaged Over CV Runs):

Best (ROC\_AUC): Category Gradient Boosting = 0.670

Best (Balanced Acc.): Category Gradient Boosting = 0.622

Best (F1 Score): Gradient Boosting = 0.616

Best (PRC AUC): Category Gradient Boosting = 0.659

Best (PRC APS): Category Gradient Boosting = 0.664

## ROC

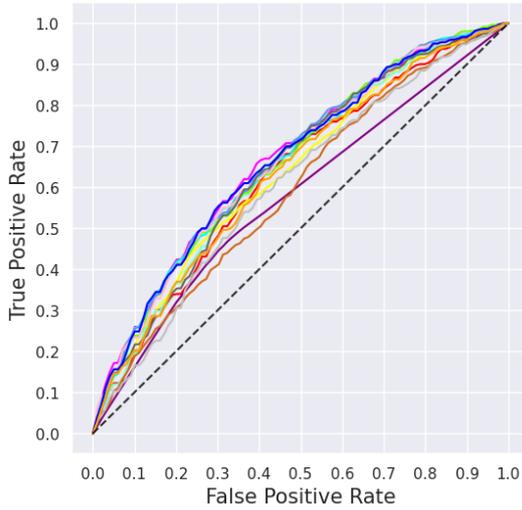

- Artificial Neural Network, AUC=0.633
- Category Gradient Boosting, AUC=0.670
- Decision Tree, AUC=0.639
- Elastic Net, AUC=0.650
- ExSTraCS, AUC=0.661
- Extreme Gradient Boosting, AUC=0.661
- Genetic Programming, AUC=0.578
- Gradient Boosting, AUC=0.667
- K-Nearest Neighbors, AUC=0.594
- Light Gradient Boosting, AUC=0.662
- Logistic Regression, AUC=0.649
- Naive Bayes, AUC=0.606
- Random Forest, AUC=0.666
- Support Vector Machine, AUC=0.635
- No-Skill

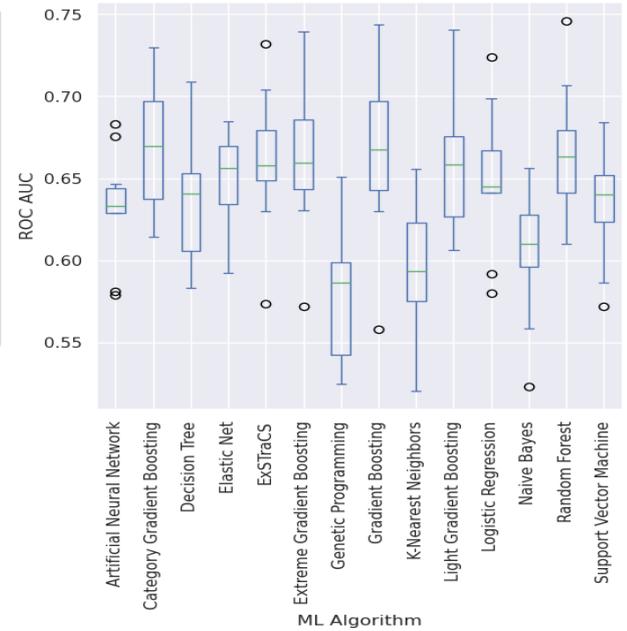

## PRC

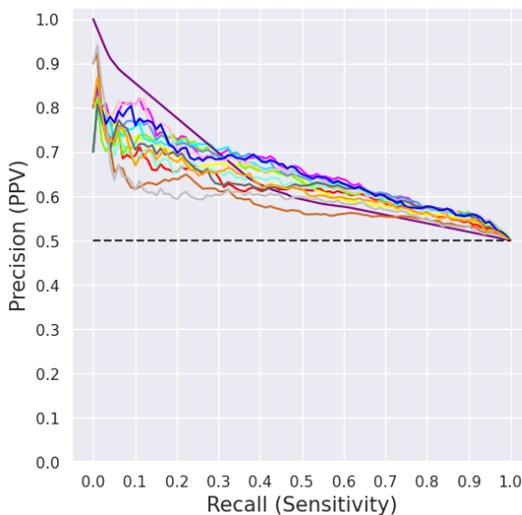

- Artificial Neural Network, AUC=0.616, APS=0.622
- Category Gradient Boosting, AUC=0.659, APS=0.664
- Decision Tree, AUC=0.632, APS=0.622
- Elastic Net, AUC=0.627, APS=0.633
- ExSTraCS, AUC=0.641, APS=0.647
- Extreme Gradient Boosting, AUC=0.647, APS=0.646
- Genetic Programming, AUC=0.647, APS=0.551
- Gradient Boosting, AUC=0.653, APS=0.654
- K-Nearest Neighbors, AUC=0.587, APS=0.589
- Light Gradient Boosting, AUC=0.652, APS=0.657
- Logistic Regression, AUC=0.628, APS=0.633
- Naive Bayes, AUC=0.592, APS=0.598
- Random Forest, AUC=0.652, APS=0.658
- Support Vector Machine, AUC=0.621, APS=0.627
- No-Skill

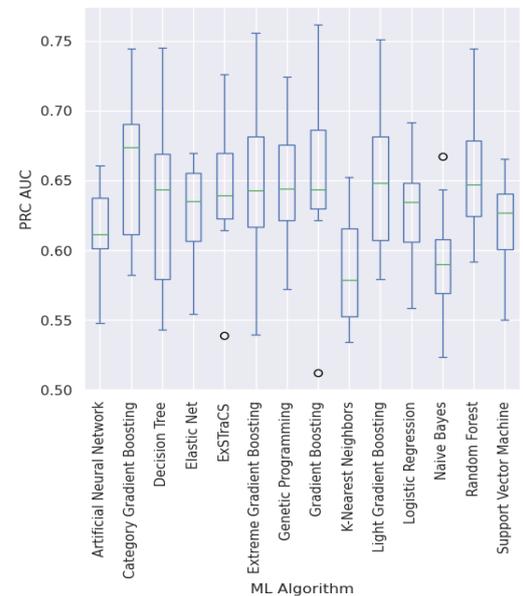

# Dataset and Model Prediction Summary: D4 = D\_gametes\_2way\_epistasis\_L\_2\_H\_0

## Data Processing/Counts Summary

|           | Instances | Total Features | Categorical Features | Quantitative Features | Missing Values | Missing Percent | Class 0 | Class 1 |
|-----------|-----------|----------------|----------------------|-----------------------|----------------|-----------------|---------|---------|
| Original  | 1600      | 100            | 2                    | 98                    | 0              | 0.0             | 800     | 800     |
| C1        | 1600      | 100            | 2                    | 98                    | 0              | 0.0             | 800     | 800     |
| E1        | 1600      | 100            | 2                    | 98                    | 0              | 0.0             | 800     | 800     |
| C2        | 1600      | 100            | 2                    | 98                    | 0              | 0.0             | 800     | 800     |
| C3        | 1600      | 100            | 2                    | 98                    | 0              | 0.0             | 800     | 800     |
| E2        | 1600      | 100            | 2                    | 98                    | 0              | 0.0             | 800     | 800     |
| C4        | 1600      | 100            | 2                    | 98                    | 0              | 0.0             | 800     | 800     |
| Processed | 1600      | 100            | 2                    | 98                    | 0              | 0.0             | 800     | 800     |

## Cleaning (C) and Engineering (E) Elements

- \* C1 - Remove instances with no outcome and features to ignore
- \* E1 - Add missingness features
- \* C2 - Remove features with invariance or high missingness
- \* C3 - Remove instances with high missingness
- \* E2 - Add one-hot-encoding of categorical features
- \* C4 - Remove highly correlated features

## Class Balance (Processed)

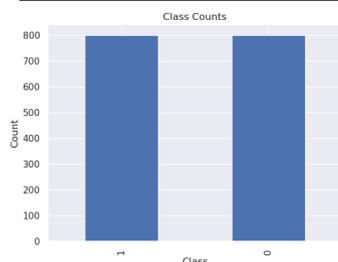

## Feature Correlations (Pearson)

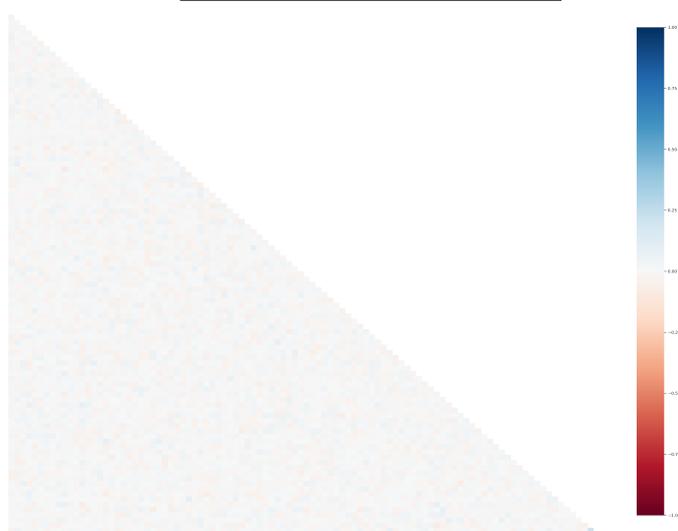

## Top ML Algorithm Results (Averaged Over CV Runs):

|                                                          |
|----------------------------------------------------------|
| Best (ROC_AUC): ExSTraCS = 0.855                         |
| Best (Balanced Acc.): Category Gradient Boosting = 0.799 |
| Best (F1 Score): Category Gradient Boosting = 0.819      |
| Best (PRC AUC): ExSTraCS = 0.822                         |
| Best (PRC APS): ExSTraCS = 0.826                         |

## ROC

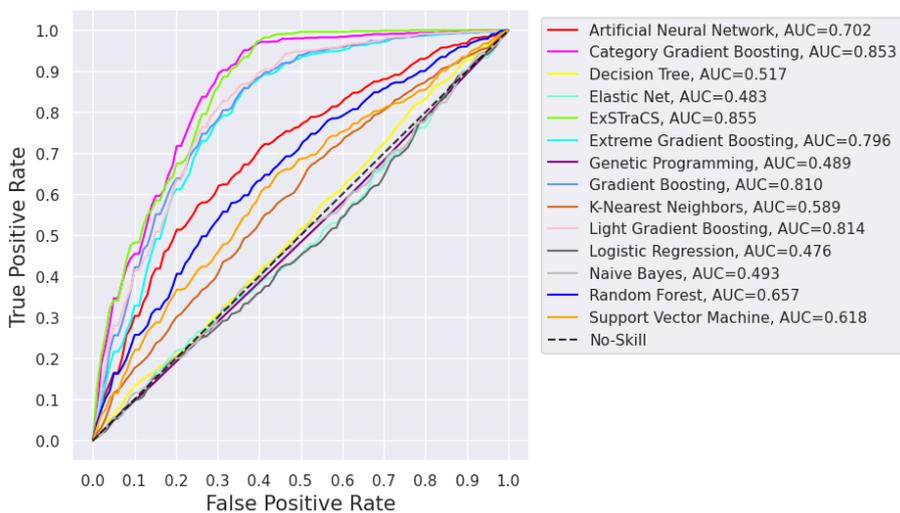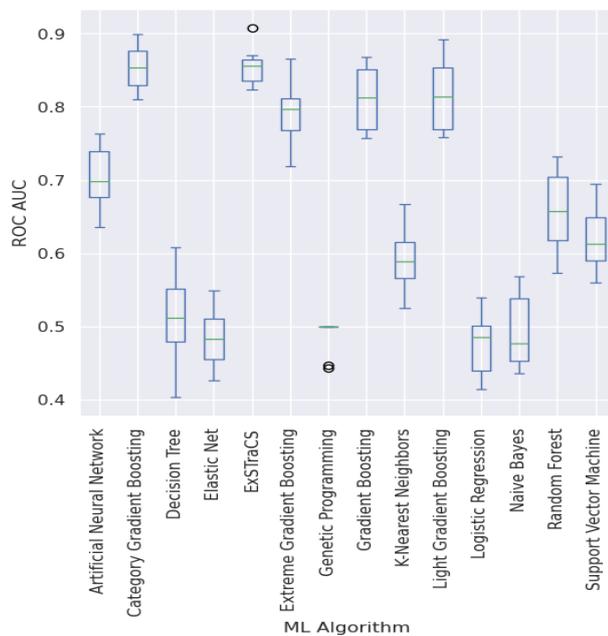

## PRC

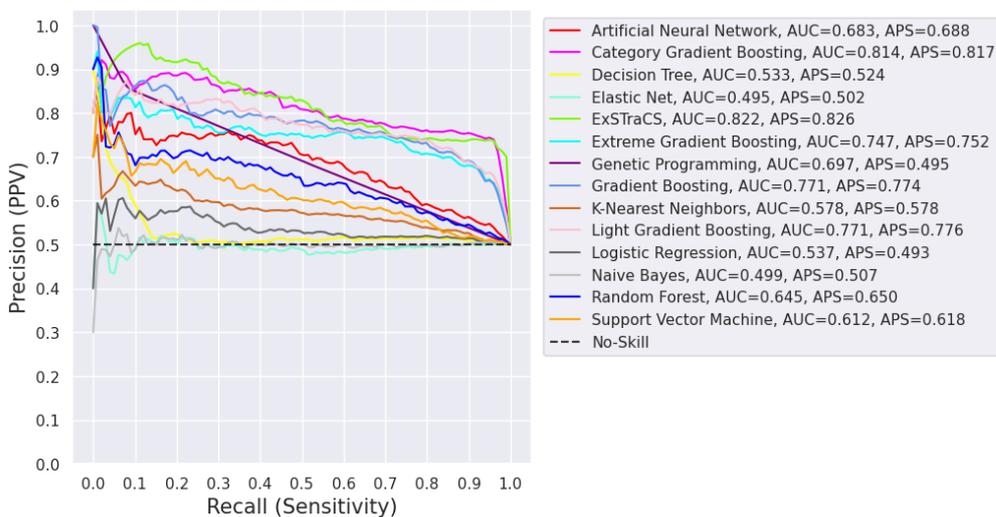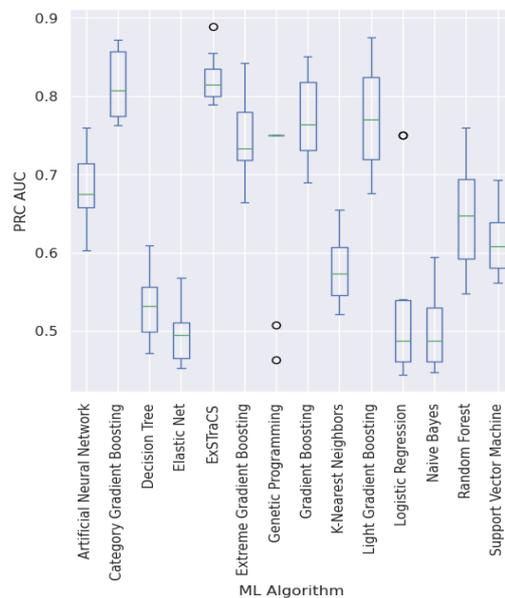

# Dataset and Model Prediction Summary: D5 = E\_gametes\_2way\_epi\_2het\_L\_2\_H\_0

## Data Processing/Counts Summary

|           | Instances | Total Features | Categorical Features | Quantitative Features | Missing Values | Missing Percent | Class 0 | Class 1 |
|-----------|-----------|----------------|----------------------|-----------------------|----------------|-----------------|---------|---------|
| Original  | 1600      | 100            | 1                    | 99                    | 0              | 0.0             | 800     | 800     |
| C1        | 1600      | 100            | 1                    | 99                    | 0              | 0.0             | 800     | 800     |
| E1        | 1600      | 100            | 1                    | 99                    | 0              | 0.0             | 800     | 800     |
| C2        | 1600      | 100            | 1                    | 99                    | 0              | 0.0             | 800     | 800     |
| C3        | 1600      | 100            | 1                    | 99                    | 0              | 0.0             | 800     | 800     |
| E2        | 1600      | 100            | 1                    | 99                    | 0              | 0.0             | 800     | 800     |
| C4        | 1600      | 100            | 1                    | 99                    | 0              | 0.0             | 800     | 800     |
| Processed | 1600      | 100            | 1                    | 99                    | 0              | 0.0             | 800     | 800     |

## Cleaning (C) and Engineering (E) Elements

- \* C1 - Remove instances with no outcome and features to ignore
- \* E1 - Add missingness features
- \* C2 - Remove features with invariance or high missingness
- \* C3 - Remove instances with high missingness
- \* E2 - Add one-hot-encoding of categorical features
- \* C4 - Remove highly correlated features

## Class Balance (Processed)

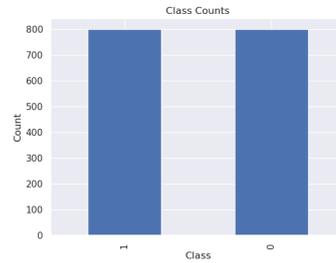

## Feature Correlations (Pearson)

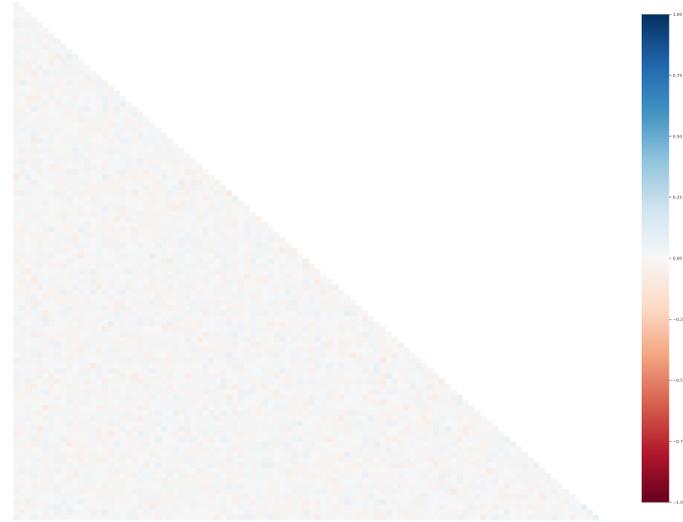

## Top ML Algorithm Results (Averaged Over CV Runs):

Best (ROC\_AUC): ExSTraCS = 0.756

Best (Balanced Acc.): ExSTraCS = 0.682

Best (F1 Score): ExSTraCS = 0.687

Best (PRC AUC): ExSTraCS = 0.730

Best (PRC APS): ExSTraCS = 0.734

## ROC

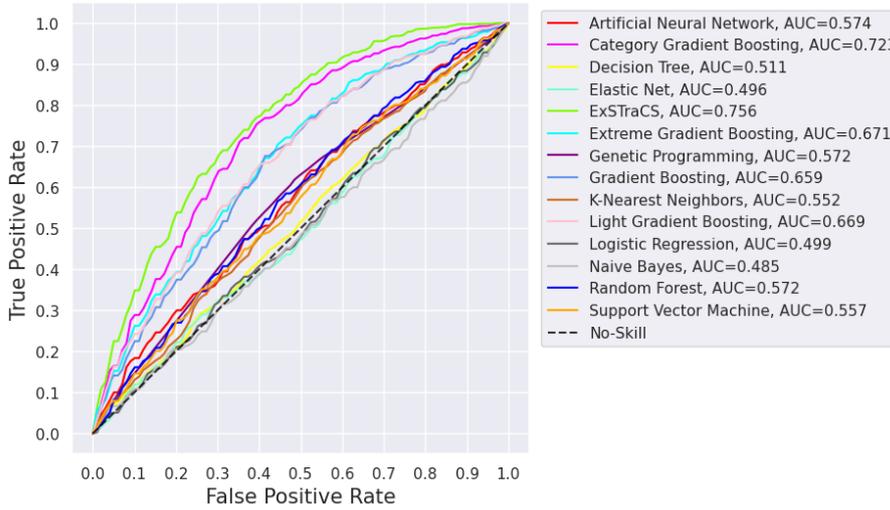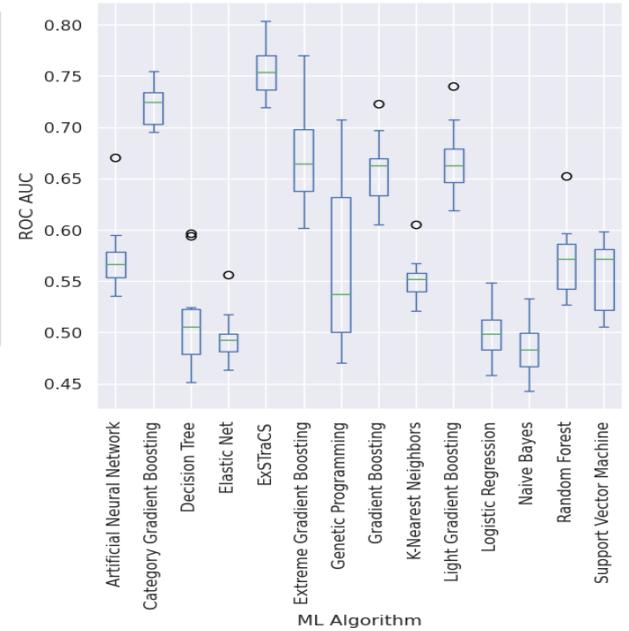

## PRC

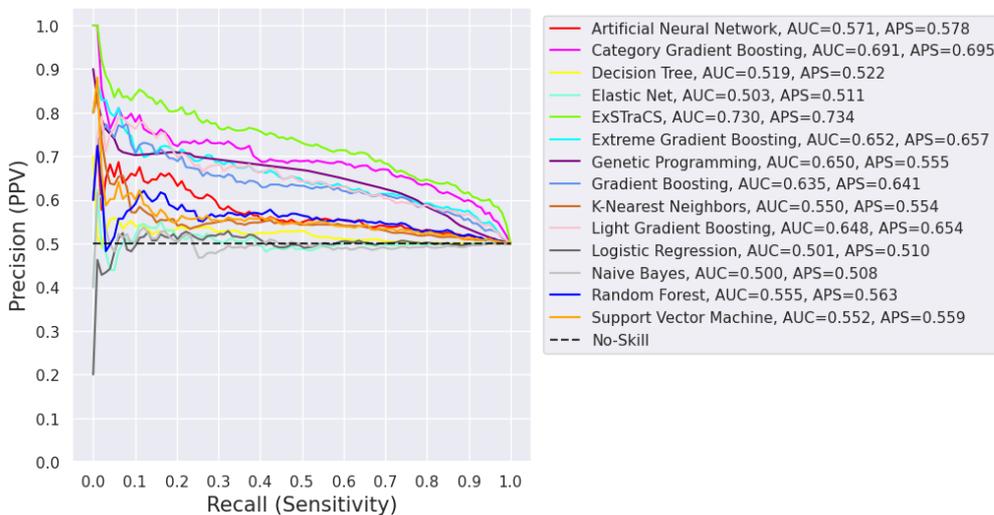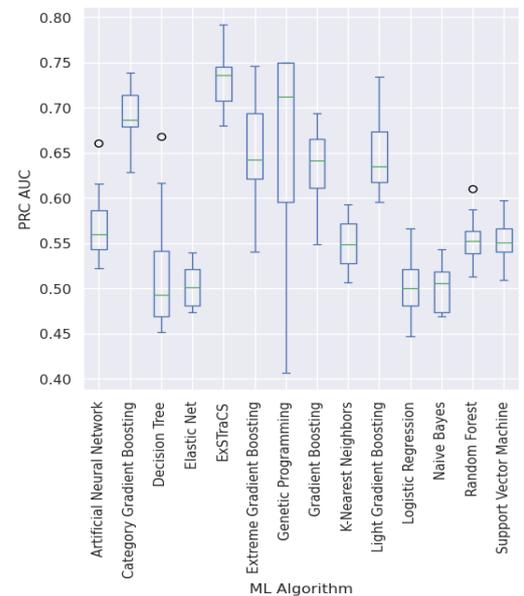

# Dataset and Model Prediction Summary: D6 = F\_gametes\_3way\_epistasis\_L\_3\_H\_0

## Data Processing/Counts Summary

|           | Instances | Total Features | Categorical Features | Quantitative Features | Missing Values | Missing Percent | Class 0 | Class 1 |
|-----------|-----------|----------------|----------------------|-----------------------|----------------|-----------------|---------|---------|
| Original  | 1600      | 100            | 1                    | 99                    | 0              | 0.0             | 800     | 800     |
| C1        | 1600      | 100            | 1                    | 99                    | 0              | 0.0             | 800     | 800     |
| E1        | 1600      | 100            | 1                    | 99                    | 0              | 0.0             | 800     | 800     |
| C2        | 1600      | 100            | 1                    | 99                    | 0              | 0.0             | 800     | 800     |
| C3        | 1600      | 100            | 1                    | 99                    | 0              | 0.0             | 800     | 800     |
| E2        | 1600      | 100            | 1                    | 99                    | 0              | 0.0             | 800     | 800     |
| C4        | 1600      | 100            | 1                    | 99                    | 0              | 0.0             | 800     | 800     |
| Processed | 1600      | 100            | 1                    | 99                    | 0              | 0.0             | 800     | 800     |

## Cleaning (C) and Engineering (E) Elements

- \* C1 - Remove instances with no outcome and features to ignore
- \* E1 - Add missingness features
- \* C2 - Remove features with invariance or high missingness
- \* C3 - Remove instances with high missingness
- \* E2 - Add one-hot-encoding of categorical features
- \* C4 - Remove highly correlated features

## Class Balance (Processed)

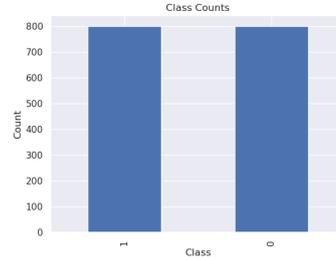

## Feature Correlations (Pearson)

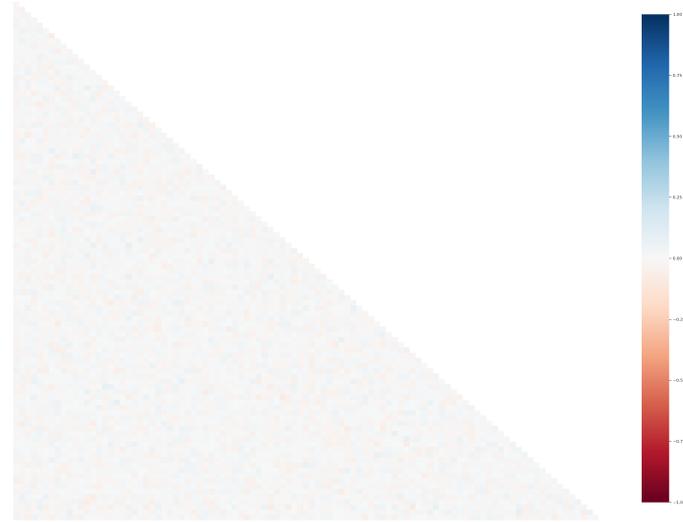

## Top ML Algorithm Results (Averaged Over CV Runs):

|                                                      |
|------------------------------------------------------|
| Best (ROC_AUC): Support Vector Machine = 0.508       |
| Best (Balanced Acc.): Support Vector Machine = 0.516 |
| Best (F1 Score): Support Vector Machine = 0.516      |
| Best (PRC AUC): Genetic Programming = 0.563          |
| Best (PRC APS): Support Vector Machine = 0.512       |

## ROC

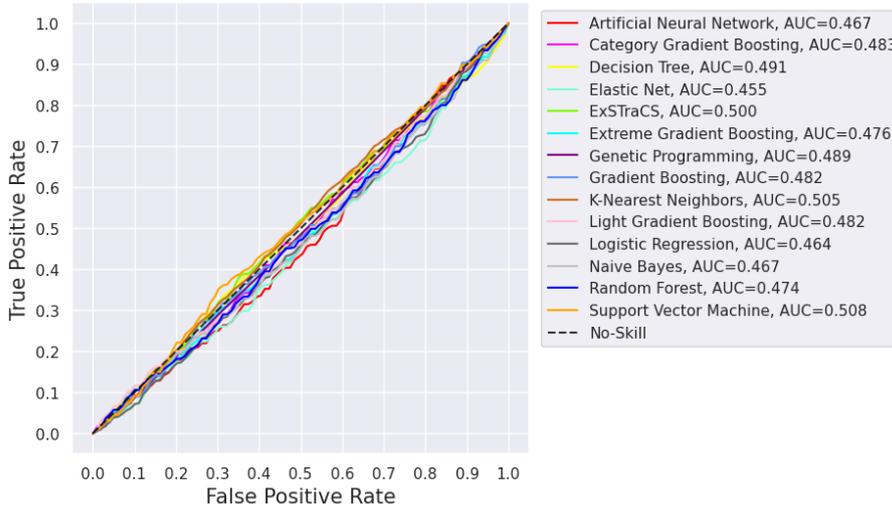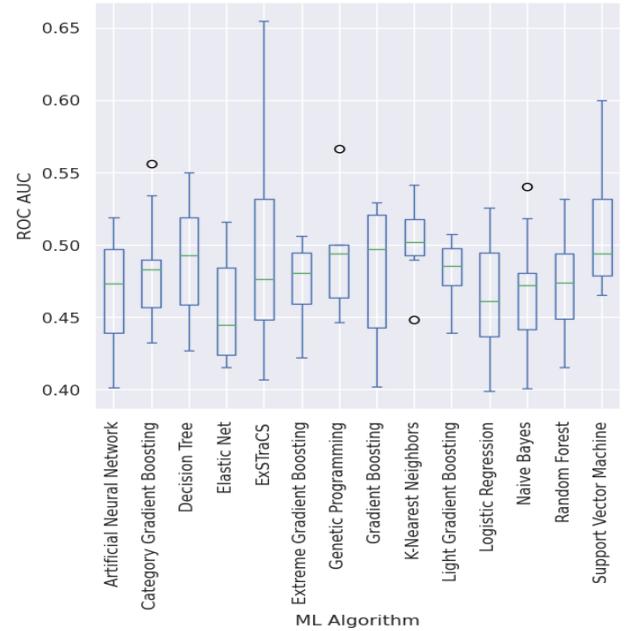

## PRC

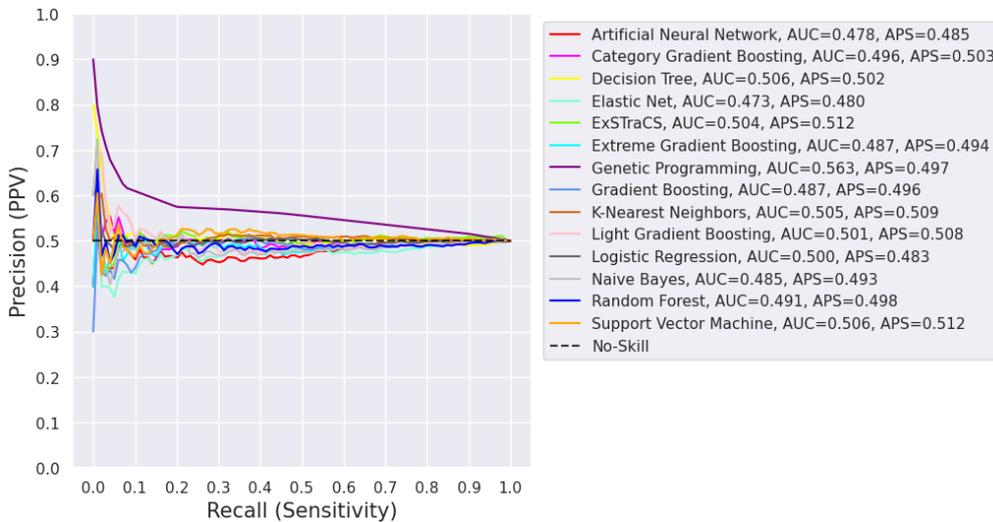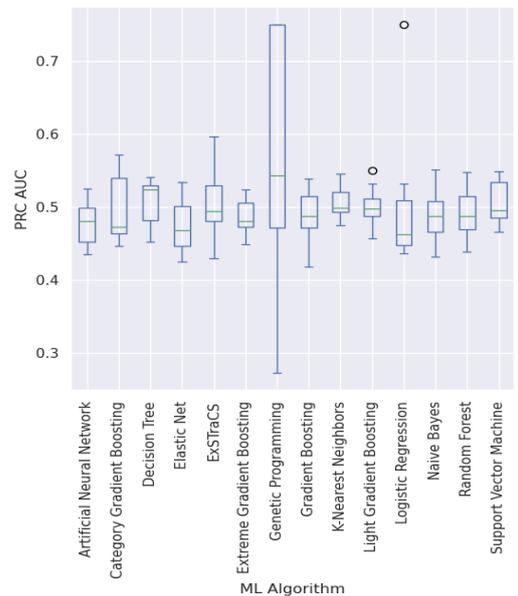

# Average Model Prediction Statistics (Rounded to 3 Decimal Points): Page 1

## D1 = A\_gametes\_univariate\_L\_1\_H\_0

| ML Algorithm               | Balanced Accuracy | Accuracy | F1 Score | Sensitivity (Recall) | Specificity | Precision (PPV) | TP   | TN   | FP   | FN   | NPV   | LR+   | LR-   | ROC AUC | PRC AUC | PRC APS |
|----------------------------|-------------------|----------|----------|----------------------|-------------|-----------------|------|------|------|------|-------|-------|-------|---------|---------|---------|
| Artificial Neural Network  | 0.827             | 0.827    | 0.824    | 0.809                | 0.845       | 0.84            | 64.7 | 67.6 | 12.4 | 15.3 | 0.816 | 5.44  | 0.227 | 0.83    | 0.786   | 0.791   |
| Category Gradient Boosting | 0.829             | 0.829    | 0.826    | 0.811                | 0.848       | 0.842           | 64.9 | 67.8 | 12.2 | 15.1 | 0.818 | 5.518 | 0.224 | 0.846   | 0.81    | 0.814   |
| Decision Tree              | 0.829             | 0.829    | 0.826    | 0.811                | 0.848       | 0.842           | 64.9 | 67.8 | 12.2 | 15.1 | 0.818 | 5.518 | 0.224 | 0.833   | 0.856   | 0.794   |
| Elastic Net                | 0.829             | 0.829    | 0.826    | 0.811                | 0.848       | 0.842           | 64.9 | 67.8 | 12.2 | 15.1 | 0.818 | 5.518 | 0.224 | 0.828   | 0.784   | 0.788   |
| ExSTraCS                   | 0.828             | 0.828    | 0.824    | 0.81                 | 0.845       | 0.84            | 64.8 | 67.6 | 12.4 | 15.2 | 0.817 | 5.422 | 0.226 | 0.832   | 0.797   | 0.801   |
| Extreme Gradient Boosting  | 0.828             | 0.828    | 0.825    | 0.809                | 0.848       | 0.842           | 64.7 | 67.8 | 12.2 | 15.3 | 0.816 | 5.498 | 0.226 | 0.838   | 0.806   | 0.805   |
| Genetic Programming        | 0.829             | 0.829    | 0.826    | 0.811                | 0.848       | 0.842           | 64.9 | 67.8 | 12.2 | 15.1 | 0.818 | 5.518 | 0.224 | 0.836   | 0.875   | 0.789   |
| Gradient Boosting          | 0.826             | 0.826    | 0.823    | 0.806                | 0.846       | 0.841           | 64.5 | 67.7 | 12.3 | 15.5 | 0.814 | 5.522 | 0.23  | 0.842   | 0.809   | 0.813   |
| K-Nearest Neighbors        | 0.784             | 0.784    | 0.772    | 0.734                | 0.835       | 0.816           | 58.7 | 66.8 | 13.2 | 21.3 | 0.759 | 4.772 | 0.322 | 0.822   | 0.78    | 0.783   |
| Light Gradient Boosting    | 0.828             | 0.828    | 0.825    | 0.811                | 0.845       | 0.84            | 64.9 | 67.6 | 12.4 | 15.1 | 0.818 | 5.462 | 0.225 | 0.84    | 0.808   | 0.811   |
| Logistic Regression        | 0.829             | 0.829    | 0.826    | 0.811                | 0.848       | 0.842           | 64.9 | 67.8 | 12.2 | 15.1 | 0.818 | 5.518 | 0.224 | 0.827   | 0.756   | 0.774   |
| Naive Bayes                | 0.799             | 0.799    | 0.798    | 0.796                | 0.801       | 0.801           | 63.7 | 64.1 | 15.9 | 16.3 | 0.798 | 4.081 | 0.255 | 0.805   | 0.763   | 0.768   |
| Random Forest              | 0.829             | 0.829    | 0.825    | 0.81                 | 0.848       | 0.842           | 64.8 | 67.8 | 12.2 | 15.2 | 0.817 | 5.51  | 0.225 | 0.852   | 0.822   | 0.826   |
| Support Vector Machine     | 0.829             | 0.829    | 0.826    | 0.811                | 0.848       | 0.842           | 64.9 | 67.8 | 12.2 | 15.1 | 0.818 | 5.518 | 0.224 | 0.823   | 0.779   | 0.784   |

## D2 = B\_gametes\_uni\_4add\_L\_1\_H\_0

| ML Algorithm               | Balanced Accuracy | Accuracy | F1 Score | Sensitivity (Recall) | Specificity | Precision (PPV) | TP   | TN   | FP  | FN  | NPV   | LR+    | LR-   | ROC AUC | PRC AUC | PRC APS |
|----------------------------|-------------------|----------|----------|----------------------|-------------|-----------------|------|------|-----|-----|-------|--------|-------|---------|---------|---------|
| Artificial Neural Network  | 0.904             | 0.904    | 0.904    | 0.904                | 0.904       | 0.904           | 72.3 | 72.3 | 7.7 | 7.7 | 0.905 | 10.233 | 0.106 | 0.96    | 0.942   | 0.943   |
| Category Gradient Boosting | 0.931             | 0.931    | 0.932    | 0.938                | 0.925       | 0.927           | 75.0 | 74.0 | 6.0 | 5.0 | 0.938 | 13.639 | 0.067 | 0.981   | 0.979   | 0.979   |
| Decision Tree              | 0.918             | 0.918    | 0.918    | 0.93                 | 0.905       | 0.908           | 74.4 | 72.4 | 7.6 | 5.6 | 0.931 | 10.527 | 0.076 | 0.972   | 0.972   | 0.962   |
| Elastic Net                | 0.898             | 0.898    | 0.897    | 0.891                | 0.905       | 0.904           | 71.3 | 72.4 | 7.6 | 8.7 | 0.894 | 10.483 | 0.121 | 0.96    | 0.944   | 0.943   |
| ExSTraCS                   | 0.93              | 0.93     | 0.931    | 0.95                 | 0.91        | 0.914           | 76.0 | 72.8 | 7.2 | 4.0 | 0.949 | 11.264 | 0.055 | 0.983   | 0.981   | 0.981   |
| Extreme Gradient Boosting  | 0.931             | 0.931    | 0.932    | 0.944                | 0.919       | 0.921           | 75.5 | 73.5 | 6.5 | 4.5 | 0.943 | 13.192 | 0.061 | 0.982   | 0.981   | 0.981   |
| Genetic Programming        | 0.916             | 0.916    | 0.918    | 0.932                | 0.9         | 0.904           | 74.6 | 72.0 | 8.0 | 5.4 | 0.931 | 10.748 | 0.077 | 0.967   | 0.942   | 0.955   |
| Gradient Boosting          | 0.924             | 0.924    | 0.925    | 0.936                | 0.912       | 0.916           | 74.9 | 73.0 | 7.0 | 5.1 | 0.936 | 12.059 | 0.069 | 0.98    | 0.978   | 0.977   |
| K-Nearest Neighbors        | 0.91              | 0.91     | 0.91     | 0.911                | 0.909       | 0.911           | 72.9 | 72.7 | 7.3 | 7.1 | 0.912 | 12.731 | 0.098 | 0.967   | 0.959   | 0.959   |
| Light Gradient Boosting    | 0.928             | 0.928    | 0.928    | 0.936                | 0.919       | 0.921           | 74.9 | 73.5 | 6.5 | 5.1 | 0.937 | 12.787 | 0.069 | 0.982   | 0.981   | 0.981   |
| Logistic Regression        | 0.894             | 0.894    | 0.895    | 0.899                | 0.89        | 0.893           | 71.9 | 71.2 | 8.8 | 8.1 | 0.901 | 10.46  | 0.113 | 0.961   | 0.943   | 0.945   |
| Naive Bayes                | 0.901             | 0.901    | 0.901    | 0.901                | 0.9         | 0.901           | 72.1 | 72.0 | 8.0 | 7.9 | 0.902 | 10.877 | 0.11  | 0.96    | 0.939   | 0.94    |
| Random Forest              | 0.92              | 0.92     | 0.921    | 0.931                | 0.909       | 0.912           | 74.5 | 72.7 | 7.3 | 5.5 | 0.931 | 11.079 | 0.075 | 0.982   | 0.979   | 0.979   |
| Support Vector Machine     | 0.905             | 0.905    | 0.905    | 0.905                | 0.905       | 0.907           | 72.4 | 72.4 | 7.6 | 7.6 | 0.906 | 12.638 | 0.105 | 0.96    | 0.947   | 0.948   |

## D3 = C\_gametes\_uni\_4het\_L\_1\_H\_0

| ML Algorithm               | Balanced Accuracy | Accuracy | F1 Score | Sensitivity (Recall) | Specificity | Precision (PPV) | TP   | TN   | FP   | FN   | NPV   | LR+   | LR-   | ROC AUC | PRC AUC | PRC APS |
|----------------------------|-------------------|----------|----------|----------------------|-------------|-----------------|------|------|------|------|-------|-------|-------|---------|---------|---------|
| Artificial Neural Network  | 0.601             | 0.601    | 0.597    | 0.595                | 0.606       | 0.601           | 47.6 | 48.5 | 31.5 | 32.4 | 0.601 | 1.519 | 0.669 | 0.633   | 0.616   | 0.622   |
| Category Gradient Boosting | 0.622             | 0.622    | 0.609    | 0.59                 | 0.654       | 0.63            | 47.2 | 52.3 | 27.7 | 32.8 | 0.616 | 1.715 | 0.628 | 0.67    | 0.659   | 0.664   |
| Decision Tree              | 0.594             | 0.594    | 0.581    | 0.57                 | 0.619       | 0.601           | 45.6 | 49.5 | 30.5 | 34.4 | 0.594 | 1.532 | 0.693 | 0.639   | 0.632   | 0.622   |
| Elastic Net                | 0.606             | 0.606    | 0.594    | 0.578                | 0.635       | 0.612           | 46.2 | 50.8 | 29.2 | 33.8 | 0.602 | 1.596 | 0.667 | 0.65    | 0.627   | 0.633   |
| ExSTraCS                   | 0.598             | 0.598    | 0.578    | 0.556                | 0.64        | 0.608           | 44.5 | 51.2 | 28.8 | 35.5 | 0.593 | 1.575 | 0.696 | 0.661   | 0.641   | 0.647   |
| Extreme Gradient Boosting  | 0.611             | 0.611    | 0.599    | 0.584                | 0.638       | 0.62            | 46.7 | 51.0 | 29.0 | 33.3 | 0.606 | 1.686 | 0.659 | 0.661   | 0.647   | 0.646   |
| Genetic Programming        | 0.568             | 0.568    | 0.478    | 0.425                | 0.71        | 0.595           | 34.0 | 56.8 | 23.2 | 46.0 | 0.556 | 1.509 | 0.808 | 0.578   | 0.647   | 0.551   |
| Gradient Boosting          | 0.619             | 0.619    | 0.616    | 0.612                | 0.626       | 0.621           | 49.0 | 50.1 | 29.9 | 31.0 | 0.619 | 1.656 | 0.621 | 0.667   | 0.653   | 0.654   |
| K-Nearest Neighbors        | 0.551             | 0.551    | 0.505    | 0.461                | 0.64        | 0.566           | 36.9 | 51.2 | 28.8 | 43.1 | 0.542 | 1.332 | 0.848 | 0.594   | 0.587   | 0.589   |
| Light Gradient Boosting    | 0.612             | 0.612    | 0.606    | 0.598                | 0.626       | 0.615           | 47.8 | 50.1 | 29.9 | 32.2 | 0.609 | 1.62  | 0.646 | 0.662   | 0.652   | 0.657   |
| Logistic Regression        | 0.608             | 0.608    | 0.598    | 0.584                | 0.632       | 0.613           | 46.7 | 50.6 | 29.4 | 33.3 | 0.604 | 1.605 | 0.662 | 0.649   | 0.628   | 0.633   |
| Naive Bayes                | 0.574             | 0.574    | 0.557    | 0.538                | 0.611       | 0.581           | 43.0 | 48.9 | 31.1 | 37.0 | 0.57  | 1.41  | 0.764 | 0.606   | 0.592   | 0.598   |
| Random Forest              | 0.621             | 0.621    | 0.614    | 0.602                | 0.64        | 0.626           | 48.2 | 51.2 | 28.8 | 31.8 | 0.617 | 1.703 | 0.626 | 0.666   | 0.652   | 0.658   |
| Support Vector Machine     | 0.596             | 0.596    | 0.586    | 0.576                | 0.616       | 0.599           | 46.1 | 49.3 | 30.7 | 33.9 | 0.595 | 1.505 | 0.687 | 0.635   | 0.621   | 0.627   |

## D4 = D\_gametes\_2way\_epistasis\_L\_2\_H\_0

| ML Algorithm               | Balanced Accuracy | Accuracy | F1 Score | Sensitivity (Recall) | Specificity | Precision (PPV) | TP   | TN   | FP   | FN   | NPV   | LR+   | LR-   | ROC AUC | PRC AUC | PRC APS |
|----------------------------|-------------------|----------|----------|----------------------|-------------|-----------------|------|------|------|------|-------|-------|-------|---------|---------|---------|
| Artificial Neural Network  | 0.652             | 0.652    | 0.645    | 0.634                | 0.67        | 0.659           | 50.7 | 53.6 | 26.4 | 29.3 | 0.647 | 1.969 | 0.549 | 0.702   | 0.683   | 0.688   |
| Category Gradient Boosting | 0.799             | 0.799    | 0.819    | 0.901                | 0.698       | 0.751           | 72.1 | 55.8 | 24.2 | 7.9  | 0.876 | 3.109 | 0.142 | 0.853   | 0.814   | 0.817   |
| Decision Tree              | 0.506             | 0.506    | 0.491    | 0.484                | 0.528       | 0.503           | 38.7 | 42.2 | 37.8 | 41.3 | 0.507 | 1.04  | 0.994 | 0.517   | 0.533   | 0.524   |
| Elastic Net                | 0.478             | 0.478    | 0.477    | 0.478                | 0.478       | 0.478           | 38.2 | 38.2 | 41.8 | 41.8 | 0.476 | 0.923 | 1.111 | 0.483   | 0.495   | 0.502   |
| ExSTraCS                   | 0.784             | 0.784    | 0.804    | 0.884                | 0.684       | 0.739           | 70.7 | 54.7 | 25.3 | 9.3  | 0.857 | 2.893 | 0.169 | 0.855   | 0.822   | 0.826   |
| Extreme Gradient Boosting  | 0.734             | 0.734    | 0.738    | 0.746                | 0.722       | 0.731           | 59.7 | 57.8 | 22.2 | 20.3 | 0.739 | 2.857 | 0.354 | 0.796   | 0.747   | 0.752   |
| Genetic Programming        | 0.498             | 0.498    | 0.161    | 0.216                | 0.779       | 0.189           | 17.3 | 62.3 | 17.7 | 62.7 | 0.399 | 0.371 | 0.806 | 0.489   | 0.697   | 0.495   |
| Gradient Boosting          | 0.739             | 0.739    | 0.744    | 0.756                | 0.721       | 0.733           | 60.5 | 57.7 | 22.3 | 19.5 | 0.747 | 2.874 | 0.342 | 0.81    | 0.771   | 0.774   |
| K-Nearest Neighbors        | 0.565             | 0.565    | 0.544    | 0.522                | 0.608       | 0.573           | 41.8 | 48.6 | 31.4 | 38.2 | 0.56  | 1.36  | 0.791 | 0.589   | 0.578   | 0.578   |
| Light Gradient Boosting    | 0.747             | 0.747    | 0.75     | 0.761                | 0.732       | 0.74            | 60.9 | 58.6 | 21.4 | 19.1 | 0.756 | 2.92  | 0.328 | 0.814   | 0.771   | 0.776   |
| Logistic Regression        | 0.474             | 0.474    | 0.372    | 0.37                 | 0.578       | 0.375           | 29.6 | 46.2 | 33.8 | 50.4 | 0.472 | 0.713 | 1.131 | 0.476   | 0.537   | 0.493   |
| Naive Bayes                | 0.489             | 0.489    | 0.554    | 0.638                | 0.341       | 0.492           | 51.0 | 27.3 | 52.7 | 29.0 | 0.483 | 0.974 | 1.096 | 0.493   | 0.499   | 0.507   |
| Random Forest              | 0.616             | 0.616    | 0.611    | 0.606                | 0.625       | 0.618           | 48.5 | 50.0 | 30.0 | 31.5 | 0.615 | 1.66  | 0.636 | 0.657   | 0.645   | 0.65    |
| Support Vector Machine     | 0.587             | 0.587    | 0.575    | 0.561                | 0.612       | 0.592           | 44.9 | 49.0 | 31.0 | 35.1 | 0.583 | 1.482 | 0.721 | 0.618   | 0.612   | 0.618   |

## D5 = E\_gametes\_2way\_epi\_2het\_L\_2\_H\_0

| ML Algorithm               | Balanced Accuracy | Accuracy | F1 Score | Sensitivity (Recall) | Specificity | Precision (PPV) | TP   | TN   | FP   | FN   | NPV   | LR+   | LR-   | ROC AUC | PRC AUC | PRC APS |
|----------------------------|-------------------|----------|----------|----------------------|-------------|-----------------|------|------|------|------|-------|-------|-------|---------|---------|---------|
| Artificial Neural Network  | 0.554             | 0.554    | 0.558    | 0.565                | 0.542       | 0.553           | 45.2 | 43.4 | 36.6 | 34.8 | 0.555 | 1.259 | 0.809 | 0.574   | 0.571   | 0.578   |
| Category Gradient Boosting | 0.674             | 0.674    | 0.678    | 0.689                | 0.659       | 0.669           | 55.1 | 52.7 | 27.3 | 24.9 | 0.679 | 2.039 | 0.473 | 0.723   | 0.691   | 0.695   |
| Decision Tree              | 0.506             | 0.506    | 0.508    | 0.515                | 0.496       | 0.505           | 41.2 | 39.7 | 40.3 | 38.8 | 0.507 | 1.03  | 0.98  | 0.511   | 0.519   | 0.522   |
| Elastic Net                | 0.483             | 0.483    | 0.478    | 0.475                | 0.491       | 0.483           | 38.0 | 39.3 | 40.7 | 42.0 | 0.483 | 0.941 | 1.079 | 0.496   | 0.503   | 0.511   |
| ExSTraCS                   | 0.682             | 0.682    | 0.687    | 0.696                | 0.669       | 0.679           | 55.7 | 53.5 | 26.5 | 24.3 | 0.688 | 2.141 | 0.455 | 0.756   | 0.73    | 0.734   |
| Extreme Gradient Boosting  | 0.624             | 0.624    | 0.626    | 0.63                 | 0.617       | 0.622           | 50.4 | 49.4 | 30.6 | 29.6 | 0.626 | 1.679 | 0.605 | 0.671   | 0.652   | 0.657   |
| Genetic Programming        | 0.571             | 0.571    | 0.483    | 0.578                | 0.564       | 0.446           | 46.2 | 45.1 | 34.9 | 33.8 | 0.489 | 1.091 | 0.544 | 0.572   | 0.65    | 0.555   |
| Gradient Boosting          | 0.611             | 0.611    | 0.608    | 0.606                | 0.616       | 0.613           | 48.5 | 49.3 | 30.7 | 31.5 | 0.611 | 1.597 | 0.64  | 0.659   | 0.635   | 0.641   |
| K-Nearest Neighbors        | 0.536             | 0.536    | 0.503    | 0.472                | 0.6         | 0.544           | 37.8 | 48.0 | 32.0 | 42.2 | 0.532 | 1.205 | 0.883 | 0.552   | 0.55    | 0.554   |
| Light Gradient Boosting    | 0.621             | 0.621    | 0.619    | 0.62                 | 0.622       | 0.622           | 49.6 | 49.8 | 30.2 | 30.4 | 0.623 | 1.66  | 0.61  | 0.669   | 0.      |         |

## D6 = F\_gametes\_3way\_epistasis\_L\_3\_H\_0

| ML Algorithm               | Balanced Accuracy | Accuracy | F1 Score | Sensitivity (Recall) | Specificity | Precision (PPV) | TP   | TN   | FP   | FN   | NPV   | LR+   | LR-   | ROC AUC | PRC AUC | PRC APS |
|----------------------------|-------------------|----------|----------|----------------------|-------------|-----------------|------|------|------|------|-------|-------|-------|---------|---------|---------|
| Artificial Neural Network  | 0.463             | 0.463    | 0.463    | 0.464                | 0.462       | 0.463           | 37.1 | 37.0 | 43.0 | 42.9 | 0.463 | 0.87  | 1.172 | 0.467   | 0.478   | 0.485   |
| Category Gradient Boosting | 0.492             | 0.492    | 0.501    | 0.511                | 0.474       | 0.493           | 40.9 | 37.9 | 42.1 | 39.1 | 0.492 | 0.974 | 1.035 | 0.483   | 0.496   | 0.503   |
| Decision Tree              | 0.496             | 0.496    | 0.487    | 0.48                 | 0.512       | 0.501           | 38.4 | 41.0 | 39.0 | 41.6 | 0.492 | 1.018 | 1.049 | 0.491   | 0.506   | 0.502   |
| Elastic Net                | 0.475             | 0.475    | 0.467    | 0.464                | 0.486       | 0.473           | 37.1 | 38.9 | 41.1 | 42.9 | 0.477 | 0.903 | 1.104 | 0.455   | 0.473   | 0.48    |
| ExSTraCS                   | 0.494             | 0.494    | 0.475    | 0.456                | 0.532       | 0.498           | 36.5 | 42.6 | 37.4 | 43.5 | 0.492 | 1.016 | 1.056 | 0.5     | 0.504   | 0.512   |
| Extreme Gradient Boosting  | 0.466             | 0.466    | 0.462    | 0.459                | 0.474       | 0.466           | 36.7 | 37.9 | 42.1 | 43.3 | 0.466 | 0.875 | 1.15  | 0.476   | 0.487   | 0.494   |
| Genetic Programming        | 0.495             | 0.495    | 0.373    | 0.451                | 0.539       | 0.345           | 36.1 | 43.1 | 36.9 | 43.9 | 0.392 | 0.693 | 0.838 | 0.489   | 0.563   | 0.497   |
| Gradient Boosting          | 0.486             | 0.486    | 0.488    | 0.492                | 0.48        | 0.485           | 39.4 | 38.4 | 41.6 | 40.6 | 0.488 | 0.949 | 1.06  | 0.482   | 0.487   | 0.496   |
| K-Nearest Neighbors        | 0.502             | 0.502    | 0.451    | 0.411                | 0.594       | 0.505           | 32.9 | 47.5 | 32.5 | 47.1 | 0.501 | 1.03  | 0.999 | 0.505   | 0.505   | 0.509   |
| Light Gradient Boosting    | 0.487             | 0.487    | 0.488    | 0.49                 | 0.484       | 0.486           | 39.2 | 38.7 | 41.3 | 40.8 | 0.487 | 0.951 | 1.057 | 0.482   | 0.501   | 0.508   |
| Logistic Regression        | 0.481             | 0.481    | 0.39     | 0.379                | 0.584       | 0.422           | 30.3 | 46.7 | 33.3 | 49.7 | 0.482 | 0.811 | 1.085 | 0.464   | 0.5     | 0.483   |
| Naive Bayes                | 0.481             | 0.481    | 0.475    | 0.474                | 0.488       | 0.478           | 37.9 | 39.0 | 41.0 | 42.1 | 0.482 | 0.924 | 1.081 | 0.466   | 0.485   | 0.493   |
| Random Forest              | 0.482             | 0.482    | 0.49     | 0.501                | 0.464       | 0.482           | 40.1 | 37.1 | 42.9 | 39.9 | 0.483 | 0.939 | 1.085 | 0.474   | 0.491   | 0.498   |
| Support Vector Machine     | 0.516             | 0.516    | 0.516    | 0.521                | 0.51        | 0.52            | 41.7 | 40.8 | 39.2 | 38.3 | 0.512 | 1.107 | 0.969 | 0.508   | 0.506   | 0.512   |

# Median Model Prediction Statistics (Rounded to 3 Decimal Points): Page 1

## D1 = A\_gametes\_univariate\_L\_1\_H\_0

| ML Algorithm               | Balanced Accuracy | Accuracy | F1 Score | Sensitivity (Recall) | Specificity | Precision (PPV) | TP   | TN   | FP   | FN   | NPV   | LR+   | LR-   | ROC AUC | PRC AUC | PRC APS |
|----------------------------|-------------------|----------|----------|----------------------|-------------|-----------------|------|------|------|------|-------|-------|-------|---------|---------|---------|
| Artificial Neural Network  | 0.828             | 0.828    | 0.822    | 0.8                  | 0.85        | 0.846           | 64.0 | 68.0 | 12.0 | 16.0 | 0.807 | 5.485 | 0.239 | 0.835   | 0.788   | 0.793   |
| Category Gradient Boosting | 0.831             | 0.831    | 0.826    | 0.812                | 0.85        | 0.848           | 65.0 | 68.0 | 12.0 | 15.0 | 0.817 | 5.568 | 0.224 | 0.859   | 0.813   | 0.816   |
| Decision Tree              | 0.831             | 0.831    | 0.826    | 0.812                | 0.85        | 0.848           | 65.0 | 68.0 | 12.0 | 15.0 | 0.817 | 5.568 | 0.224 | 0.834   | 0.864   | 0.795   |
| Elastic Net                | 0.831             | 0.831    | 0.826    | 0.812                | 0.85        | 0.848           | 65.0 | 68.0 | 12.0 | 15.0 | 0.817 | 5.568 | 0.224 | 0.832   | 0.796   | 0.801   |
| ExSTraCS                   | 0.831             | 0.831    | 0.826    | 0.812                | 0.85        | 0.843           | 65.0 | 68.0 | 12.0 | 15.0 | 0.817 | 5.362 | 0.224 | 0.836   | 0.806   | 0.811   |
| Extreme Gradient Boosting  | 0.831             | 0.831    | 0.826    | 0.806                | 0.85        | 0.847           | 64.5 | 68.0 | 12.0 | 15.5 | 0.814 | 5.523 | 0.228 | 0.846   | 0.797   | 0.802   |
| Genetic Programming        | 0.831             | 0.831    | 0.826    | 0.812                | 0.85        | 0.848           | 65.0 | 68.0 | 12.0 | 15.0 | 0.817 | 5.568 | 0.224 | 0.842   | 0.88    | 0.794   |
| Gradient Boosting          | 0.825             | 0.825    | 0.821    | 0.794                | 0.85        | 0.847           | 63.5 | 68.0 | 12.0 | 16.5 | 0.81  | 5.523 | 0.235 | 0.848   | 0.805   | 0.813   |
| K-Nearest Neighbors        | 0.803             | 0.803    | 0.799    | 0.756                | 0.844       | 0.826           | 60.5 | 67.5 | 12.5 | 19.5 | 0.783 | 4.75  | 0.277 | 0.823   | 0.793   | 0.793   |
| Light Gradient Boosting    | 0.831             | 0.831    | 0.826    | 0.812                | 0.85        | 0.848           | 65.0 | 68.0 | 12.0 | 15.0 | 0.817 | 5.568 | 0.224 | 0.842   | 0.8     | 0.803   |
| Logistic Regression        | 0.831             | 0.831    | 0.826    | 0.812                | 0.85        | 0.848           | 65.0 | 68.0 | 12.0 | 15.0 | 0.817 | 5.568 | 0.224 | 0.832   | 0.751   | 0.783   |
| Naive Bayes                | 0.806             | 0.806    | 0.804    | 0.794                | 0.806       | 0.805           | 63.5 | 64.5 | 15.5 | 16.5 | 0.799 | 4.138 | 0.252 | 0.819   | 0.753   | 0.76    |
| Random Forest              | 0.831             | 0.831    | 0.826    | 0.806                | 0.85        | 0.848           | 64.5 | 68.0 | 12.0 | 15.5 | 0.812 | 5.568 | 0.232 | 0.856   | 0.829   | 0.833   |
| Support Vector Machine     | 0.831             | 0.831    | 0.826    | 0.812                | 0.85        | 0.848           | 65.0 | 68.0 | 12.0 | 15.0 | 0.817 | 5.568 | 0.224 | 0.82    | 0.783   | 0.789   |

## D2 = B\_gametes\_uni\_4add\_L\_1\_H\_0

| ML Algorithm               | Balanced Accuracy | Accuracy | F1 Score | Sensitivity (Recall) | Specificity | Precision (PPV) | TP   | TN   | FP  | FN  | NPV   | LR+    | LR-   | ROC AUC | PRC AUC | PRC APS |
|----------------------------|-------------------|----------|----------|----------------------|-------------|-----------------|------|------|-----|-----|-------|--------|-------|---------|---------|---------|
| Artificial Neural Network  | 0.897             | 0.897    | 0.898    | 0.906                | 0.912       | 0.913           | 72.5 | 73.0 | 7.0 | 7.5 | 0.906 | 10.571 | 0.104 | 0.955   | 0.938   | 0.939   |
| Category Gradient Boosting | 0.931             | 0.931    | 0.932    | 0.938                | 0.931       | 0.931           | 75.0 | 74.5 | 5.5 | 5.0 | 0.937 | 13.533 | 0.067 | 0.98    | 0.979   | 0.979   |
| Decision Tree              | 0.919             | 0.919    | 0.919    | 0.931                | 0.912       | 0.914           | 74.5 | 73.0 | 7.0 | 5.5 | 0.929 | 10.571 | 0.076 | 0.971   | 0.974   | 0.965   |
| Elastic Net                | 0.897             | 0.897    | 0.896    | 0.9                  | 0.912       | 0.909           | 72.0 | 73.0 | 7.0 | 8.0 | 0.899 | 10.0   | 0.113 | 0.955   | 0.938   | 0.937   |
| ExSTraCS                   | 0.931             | 0.931    | 0.933    | 0.95                 | 0.912       | 0.916           | 76.0 | 73.0 | 7.0 | 4.0 | 0.948 | 10.857 | 0.055 | 0.982   | 0.982   | 0.982   |
| Extreme Gradient Boosting  | 0.938             | 0.938    | 0.938    | 0.944                | 0.925       | 0.926           | 75.5 | 74.0 | 6.0 | 4.5 | 0.941 | 12.5   | 0.062 | 0.983   | 0.981   | 0.982   |
| Genetic Programming        | 0.931             | 0.931    | 0.93     | 0.944                | 0.906       | 0.911           | 75.5 | 72.5 | 7.5 | 4.5 | 0.943 | 10.312 | 0.061 | 0.974   | 0.947   | 0.963   |
| Gradient Boosting          | 0.925             | 0.925    | 0.925    | 0.931                | 0.925       | 0.924           | 74.5 | 74.0 | 6.0 | 5.5 | 0.932 | 12.083 | 0.073 | 0.978   | 0.976   | 0.976   |
| K-Nearest Neighbors        | 0.912             | 0.912    | 0.913    | 0.912                | 0.925       | 0.921           | 73.0 | 74.0 | 6.0 | 7.0 | 0.91  | 11.943 | 0.099 | 0.97    | 0.965   | 0.964   |
| Light Gradient Boosting    | 0.928             | 0.928    | 0.928    | 0.931                | 0.919       | 0.922           | 74.5 | 73.5 | 6.5 | 5.5 | 0.931 | 11.833 | 0.074 | 0.981   | 0.98    | 0.98    |
| Logistic Regression        | 0.884             | 0.884    | 0.89     | 0.906                | 0.899       | 0.899           | 72.5 | 72.5 | 7.5 | 7.5 | 0.905 | 8.955  | 0.106 | 0.96    | 0.943   | 0.944   |
| Naive Bayes                | 0.903             | 0.903    | 0.901    | 0.9                  | 0.9         | 0.902           | 72.0 | 72.0 | 8.0 | 8.0 | 0.897 | 9.31   | 0.114 | 0.96    | 0.936   | 0.937   |
| Random Forest              | 0.912             | 0.912    | 0.916    | 0.925                | 0.912       | 0.913           | 74.0 | 73.0 | 7.0 | 6.0 | 0.924 | 10.5   | 0.083 | 0.982   | 0.982   | 0.982   |
| Support Vector Machine     | 0.9               | 0.9      | 0.899    | 0.906                | 0.906       | 0.905           | 72.5 | 72.5 | 7.5 | 7.5 | 0.906 | 9.589  | 0.104 | 0.961   | 0.944   | 0.944   |

## D3 = C\_gametes\_uni\_4het\_L\_1\_H\_0

| ML Algorithm               | Balanced Accuracy | Accuracy | F1 Score | Sensitivity (Recall) | Specificity | Precision (PPV) | TP   | TN   | FP   | FN   | NPV   | LR+   | LR-   | ROC AUC | PRC AUC | PRC APS |
|----------------------------|-------------------|----------|----------|----------------------|-------------|-----------------|------|------|------|------|-------|-------|-------|---------|---------|---------|
| Artificial Neural Network  | 0.606             | 0.606    | 0.593    | 0.575                | 0.606       | 0.611           | 46.0 | 48.5 | 31.5 | 34.0 | 0.601 | 1.569 | 0.663 | 0.633   | 0.611   | 0.618   |
| Category Gradient Boosting | 0.622             | 0.622    | 0.612    | 0.594                | 0.656       | 0.633           | 47.5 | 52.5 | 27.5 | 32.5 | 0.613 | 1.725 | 0.63  | 0.67    | 0.674   | 0.678   |
| Decision Tree              | 0.6               | 0.6      | 0.586    | 0.556                | 0.625       | 0.6             | 44.5 | 50.0 | 30.0 | 35.5 | 0.598 | 1.501 | 0.672 | 0.641   | 0.644   | 0.639   |
| Elastic Net                | 0.609             | 0.609    | 0.59     | 0.562                | 0.619       | 0.618           | 45.0 | 49.5 | 30.5 | 35.0 | 0.6   | 1.622 | 0.667 | 0.656   | 0.635   | 0.639   |
| ExSTraCS                   | 0.6               | 0.6      | 0.597    | 0.588                | 0.644       | 0.619           | 47.0 | 51.5 | 28.5 | 33.0 | 0.598 | 1.624 | 0.672 | 0.658   | 0.639   | 0.647   |
| Extreme Gradient Boosting  | 0.603             | 0.603    | 0.579    | 0.562                | 0.669       | 0.614           | 45.0 | 53.5 | 26.5 | 35.0 | 0.591 | 1.589 | 0.692 | 0.659   | 0.643   | 0.645   |
| Genetic Programming        | 0.569             | 0.569    | 0.511    | 0.45                 | 0.694       | 0.605           | 36.0 | 55.5 | 24.5 | 44.0 | 0.555 | 1.53  | 0.802 | 0.587   | 0.644   | 0.553   |
| Gradient Boosting          | 0.606             | 0.606    | 0.604    | 0.619                | 0.625       | 0.614           | 49.5 | 50.0 | 30.0 | 30.5 | 0.605 | 1.593 | 0.653 | 0.668   | 0.643   | 0.649   |
| K-Nearest Neighbors        | 0.547             | 0.547    | 0.512    | 0.475                | 0.619       | 0.558           | 38.0 | 49.5 | 30.5 | 42.0 | 0.54  | 1.261 | 0.853 | 0.594   | 0.579   | 0.58    |
| Light Gradient Boosting    | 0.603             | 0.603    | 0.598    | 0.594                | 0.638       | 0.611           | 47.5 | 51.0 | 29.0 | 32.5 | 0.598 | 1.569 | 0.673 | 0.658   | 0.648   | 0.652   |
| Logistic Regression        | 0.6               | 0.6      | 0.588    | 0.575                | 0.644       | 0.608           | 46.0 | 51.5 | 28.5 | 34.0 | 0.593 | 1.551 | 0.686 | 0.645   | 0.635   | 0.637   |
| Naive Bayes                | 0.581             | 0.581    | 0.572    | 0.544                | 0.619       | 0.586           | 43.5 | 49.5 | 30.5 | 36.5 | 0.579 | 1.418 | 0.727 | 0.61    | 0.59    | 0.595   |
| Random Forest              | 0.619             | 0.619    | 0.599    | 0.594                | 0.65        | 0.634           | 47.5 | 52.0 | 28.0 | 32.5 | 0.607 | 1.731 | 0.648 | 0.663   | 0.647   | 0.652   |
| Support Vector Machine     | 0.606             | 0.606    | 0.599    | 0.588                | 0.625       | 0.608           | 47.0 | 50.0 | 30.0 | 33.0 | 0.602 | 1.551 | 0.66  | 0.64    | 0.627   | 0.63    |

## D4 = D\_gametes\_2way\_epistasis\_L\_2\_H\_0

| ML Algorithm               | Balanced Accuracy | Accuracy | F1 Score | Sensitivity (Recall) | Specificity | Precision (PPV) | TP   | TN   | FP   | FN   | NPV   | LR+   | LR-   | ROC AUC | PRC AUC | PRC APS |
|----------------------------|-------------------|----------|----------|----------------------|-------------|-----------------|------|------|------|------|-------|-------|-------|---------|---------|---------|
| Artificial Neural Network  | 0.656             | 0.656    | 0.654    | 0.638                | 0.675       | 0.652           | 51.0 | 54.0 | 26.0 | 29.0 | 0.655 | 1.877 | 0.528 | 0.698   | 0.675   | 0.681   |
| Category Gradient Boosting | 0.803             | 0.803    | 0.819    | 0.9                  | 0.712       | 0.757           | 72.0 | 57.0 | 23.0 | 8.0  | 0.878 | 3.114 | 0.139 | 0.854   | 0.807   | 0.811   |
| Decision Tree              | 0.497             | 0.497    | 0.497    | 0.488                | 0.531       | 0.497           | 39.0 | 42.5 | 37.5 | 41.0 | 0.498 | 0.987 | 1.01  | 0.511   | 0.532   | 0.515   |
| Elastic Net                | 0.481             | 0.481    | 0.475    | 0.475                | 0.5         | 0.48            | 38.0 | 40.0 | 40.0 | 42.0 | 0.482 | 0.922 | 1.076 | 0.482   | 0.495   | 0.502   |
| ExSTraCS                   | 0.784             | 0.784    | 0.8      | 0.875                | 0.7         | 0.746           | 70.0 | 56.0 | 24.0 | 10.0 | 0.849 | 2.938 | 0.179 | 0.855   | 0.815   | 0.819   |
| Extreme Gradient Boosting  | 0.731             | 0.731    | 0.736    | 0.744                | 0.712       | 0.721           | 59.5 | 57.0 | 23.0 | 20.5 | 0.74  | 2.587 | 0.351 | 0.797   | 0.733   | 0.738   |
| Genetic Programming        | 0.5               | 0.5      | 0.0      | 0.0                  | 1.0         | 0.0             | 0.0  | 80.0 | 0.0  | 80.0 | 0.5   | 0.0   | 1.0   | 0.5     | 0.75    | 0.5     |
| Gradient Boosting          | 0.738             | 0.738    | 0.735    | 0.738                | 0.731       | 0.741           | 59.0 | 58.5 | 21.5 | 21.0 | 0.731 | 2.9   | 0.368 | 0.812   | 0.764   | 0.767   |
| K-Nearest Neighbors        | 0.566             | 0.566    | 0.543    | 0.538                | 0.6         | 0.578           | 43.0 | 48.0 | 32.0 | 37.0 | 0.562 | 1.368 | 0.78  | 0.589   | 0.573   | 0.574   |
| Light Gradient Boosting    | 0.753             | 0.753    | 0.76     | 0.762                | 0.725       | 0.739           | 61.0 | 58.0 | 22.0 | 19.0 | 0.766 | 2.833 | 0.306 | 0.814   | 0.77    | 0.773   |
| Logistic Regression        | 0.475             | 0.475    | 0.447    | 0.456                | 0.512       | 0.444           | 36.5 | 41.0 | 39.0 | 43.5 | 0.478 | 0.8   | 1.093 | 0.486   | 0.488   | 0.489   |
| Naive Bayes                | 0.491             | 0.491    | 0.549    | 0.644                | 0.325       | 0.492           | 51.5 | 26.0 | 54.0 | 28.5 | 0.486 | 0.97  | 1.058 | 0.476   | 0.487   | 0.495   |
| Random Forest              | 0.619             | 0.619    | 0.622    | 0.612                | 0.625       | 0.616           | 49.0 | 50.0 | 30.0 | 31.0 | 0.622 | 1.61  | 0.608 | 0.658   | 0.648   | 0.653   |
| Support Vector Machine     | 0.591             | 0.591    | 0.587    | 0.581                | 0.619       | 0.59            | 46.5 | 49.5 | 30.5 | 33.5 | 0.589 | 1.441 | 0.698 | 0.613   | 0.608   | 0.613   |

## D5 = E\_gametes\_2way\_epi\_2het\_L\_2\_H\_0

| ML Algorithm               | Balanced Accuracy | Accuracy | F1 Score | Sensitivity (Recall) | Specificity | Precision (PPV) | TP   | TN   | FP   | FN   | NPV   | LR+   | LR-   | ROC AUC | PRC AUC | PRC APS |
|----------------------------|-------------------|----------|----------|----------------------|-------------|-----------------|------|------|------|------|-------|-------|-------|---------|---------|---------|
| Artificial Neural Network  | 0.541             | 0.541    | 0.547    | 0.562                | 0.525       | 0.538           | 45.0 | 42.0 | 38.0 | 35.0 | 0.544 | 1.166 | 0.839 | 0.566   | 0.56    | 0.568   |
| Category Gradient Boosting | 0.681             | 0.681    | 0.681    | 0.7                  | 0.662       | 0.673           | 56.0 | 53.0 | 27.0 | 24.0 | 0.682 | 2.055 | 0.466 | 0.725   | 0.686   | 0.69    |
| Decision Tree              | 0.503             | 0.503    | 0.509    | 0.512                | 0.5         | 0.503           | 41.0 | 40.0 | 40.0 | 39.0 | 0.503 | 1.01  | 0.989 | 0.506   | 0.492   | 0.502   |
| Elastic Net                | 0.484             | 0.484    | 0.472    | 0.481                | 0.512       | 0.483           | 38.5 | 41.0 | 39.0 | 41.5 | 0.485 | 0.936 | 1.061 | 0.493   | 0.501   | 0.51    |
| ExSTraCS                   | 0.681             | 0.681    | 0.687    | 0.7                  | 0.662       | 0.673           | 56.0 | 53.0 | 27.0 | 24.0 | 0.688 | 2.054 | 0.453 | 0.754   | 0.736   | 0.739   |
| Extreme Gradient Boosting  | 0.619             | 0.619    | 0.625    | 0.625                | 0.606       | 0.617           | 50.0 | 48.5 | 31.5 | 30.0 | 0.624 | 1.609 | 0.602 | 0.664   | 0.642   | 0.646   |
| Genetic Programming        | 0.547             | 0.547    | 0.667    | 0.731                | 0.569       | 0.539           | 58.5 | 45.5 | 34.5 | 21.5 | 0.56  | 1.183 | 0.5   | 0.538   | 0.712   | 0.523   |
| Gradient Boosting          | 0.603             | 0.603    | 0.601    | 0.612                | 0.631       | 0.613           | 49.0 | 50.5 | 29.5 | 31.0 | 0.605 | 1.586 | 0.654 | 0.663   | 0.641   | 0.645   |
| K-Nearest Neighbors        | 0.534             | 0.534    | 0.509    | 0.494                | 0.606       | 0.535           | 39.5 | 48.5 | 31.5 | 40.5 | 0.535 | 1.149 | 0.871 | 0.552   | 0.548   | 0.559   |
| Light Gradient Boosting    | 0.619             | 0.619    | 0.63     | 0.638                | 0.625       | 0.626           | 51.0 | 50.0 | 30.0 | 29.0 | 0.628 | 1.677 | 0.593 | 0.663   | 0.634   | 0.641   |
| Logistic Regression        | 0.503             | 0.503    | 0.497    | 0.5                  | 0           |                 |      |      |      |      |       |       |       |         |         |         |

## Median Model Prediction Statistics (Rounded to 3 Decimal Points): Page 2

### D6 = F\_gametes\_3way\_epistasis\_L\_3\_H\_0

| ML Algorithm               | Balanced Accuracy | Accuracy | F1 Score | Sensitivity (Recall) | Specificity | Precision (PPV) | TP   | TN   | FP   | FN   | NPV   | LR+   | LR-   | ROC AUC | PRC AUC | PRC APS |
|----------------------------|-------------------|----------|----------|----------------------|-------------|-----------------|------|------|------|------|-------|-------|-------|---------|---------|---------|
| Artificial Neural Network  | 0.472             | 0.472    | 0.464    | 0.469                | 0.475       | 0.47            | 37.5 | 38.0 | 42.0 | 42.5 | 0.47  | 0.888 | 1.128 | 0.473   | 0.481   | 0.489   |
| Category Gradient Boosting | 0.494             | 0.494    | 0.502    | 0.506                | 0.45        | 0.494           | 40.5 | 36.0 | 44.0 | 39.5 | 0.493 | 0.978 | 1.029 | 0.483   | 0.472   | 0.48    |
| Decision Tree              | 0.5               | 0.5      | 0.474    | 0.481                | 0.512       | 0.5             | 38.5 | 41.0 | 39.0 | 41.5 | 0.5   | 1.0   | 1.0   | 0.493   | 0.524   | 0.513   |
| Elastic Net                | 0.475             | 0.475    | 0.459    | 0.45                 | 0.488       | 0.474           | 36.0 | 39.0 | 41.0 | 44.0 | 0.476 | 0.9   | 1.1   | 0.445   | 0.468   | 0.476   |
| ExSTraCS                   | 0.491             | 0.491    | 0.474    | 0.456                | 0.531       | 0.49            | 36.5 | 42.5 | 37.5 | 43.5 | 0.491 | 0.96  | 1.035 | 0.476   | 0.494   | 0.504   |
| Extreme Gradient Boosting  | 0.469             | 0.469    | 0.462    | 0.45                 | 0.488       | 0.467           | 36.0 | 39.0 | 41.0 | 44.0 | 0.47  | 0.877 | 1.129 | 0.481   | 0.481   | 0.487   |
| Genetic Programming        | 0.5               | 0.5      | 0.432    | 0.394                | 0.6         | 0.458           | 31.5 | 48.0 | 32.0 | 48.5 | 0.473 | 0.845 | 1.0   | 0.494   | 0.542   | 0.498   |
| Gradient Boosting          | 0.494             | 0.494    | 0.5      | 0.506                | 0.481       | 0.494           | 40.5 | 38.5 | 41.5 | 39.5 | 0.494 | 0.977 | 1.024 | 0.497   | 0.487   | 0.496   |
| K-Nearest Neighbors        | 0.497             | 0.497    | 0.455    | 0.419                | 0.6         | 0.496           | 33.5 | 48.0 | 32.0 | 46.5 | 0.497 | 0.985 | 1.011 | 0.502   | 0.499   | 0.506   |
| Light Gradient Boosting    | 0.481             | 0.481    | 0.486    | 0.488                | 0.475       | 0.481           | 39.0 | 38.0 | 42.0 | 41.0 | 0.482 | 0.926 | 1.076 | 0.485   | 0.497   | 0.505   |
| Logistic Regression        | 0.484             | 0.484    | 0.458    | 0.45                 | 0.488       | 0.471           | 36.0 | 39.0 | 41.0 | 44.0 | 0.484 | 0.89  | 1.067 | 0.461   | 0.463   | 0.481   |
| Naive Bayes                | 0.484             | 0.484    | 0.484    | 0.488                | 0.481       | 0.485           | 39.0 | 38.5 | 41.5 | 41.0 | 0.485 | 0.942 | 1.061 | 0.472   | 0.487   | 0.494   |
| Random Forest              | 0.491             | 0.491    | 0.483    | 0.5                  | 0.469       | 0.491           | 40.0 | 37.5 | 42.5 | 40.0 | 0.49  | 0.965 | 1.04  | 0.474   | 0.488   | 0.495   |
| Support Vector Machine     | 0.5               | 0.5      | 0.501    | 0.525                | 0.519       | 0.499           | 42.0 | 41.5 | 38.5 | 38.0 | 0.502 | 0.996 | 0.994 | 0.494   | 0.495   | 0.502   |

# Feature Importance Summary: D1 = A\_gametes\_univariate\_L\_1\_H\_0

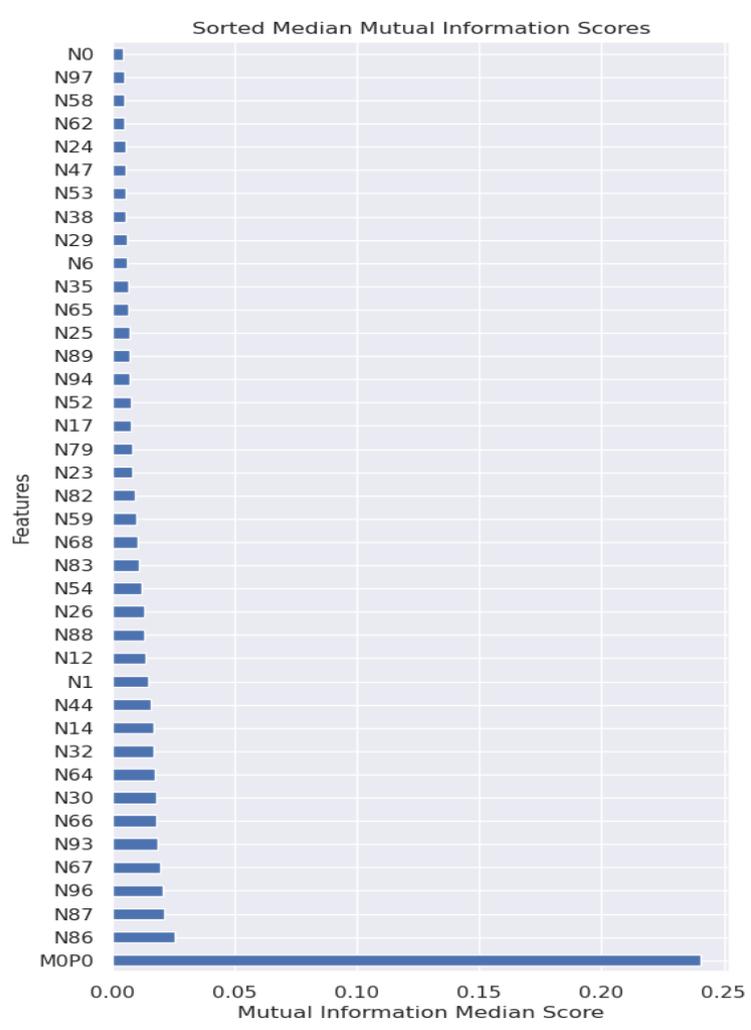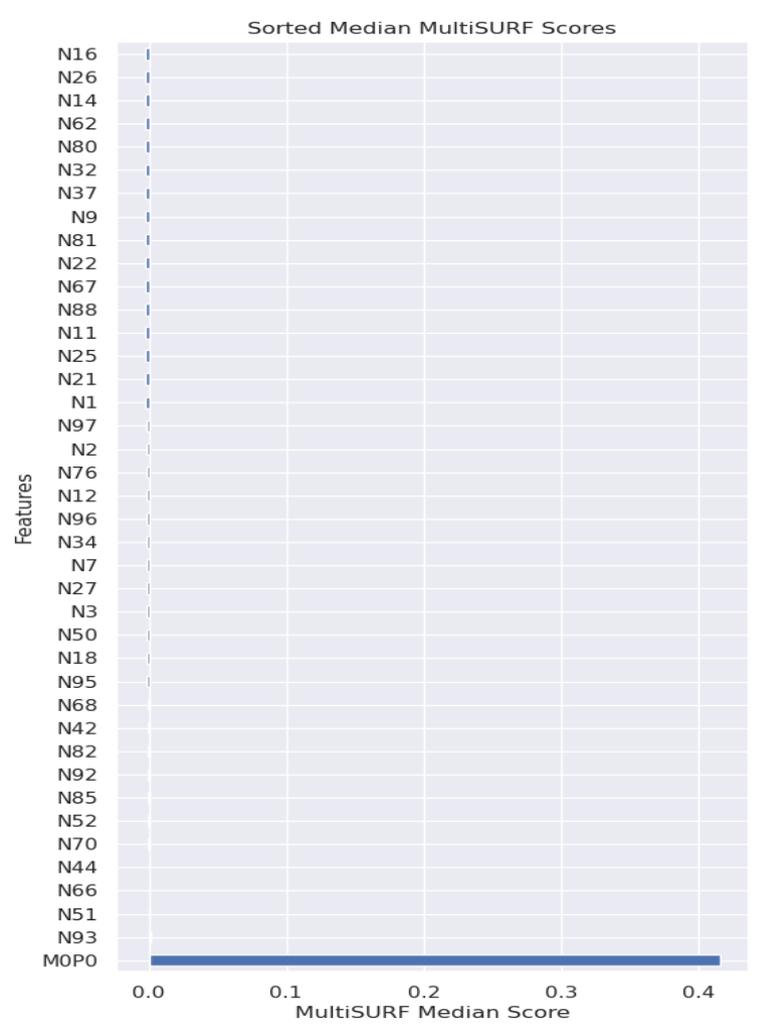

## Composite Feature Importance Plot (Normalized and Performance Weighted)

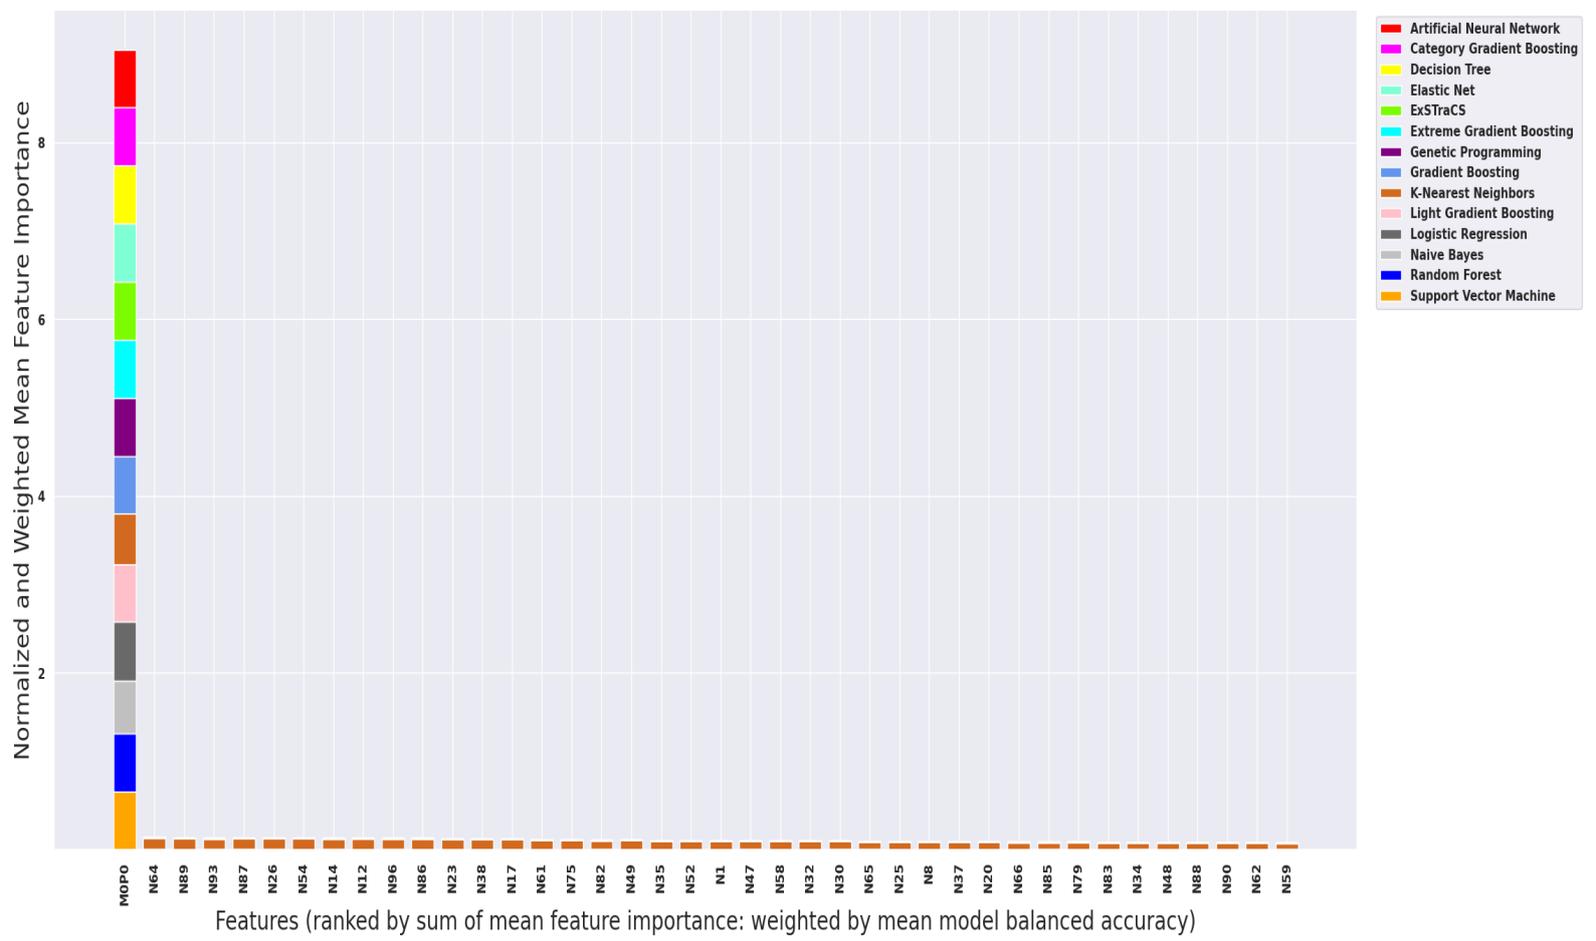

# Feature Importance Summary: D2 = B\_gametes\_uni\_4add\_L\_1\_H\_0

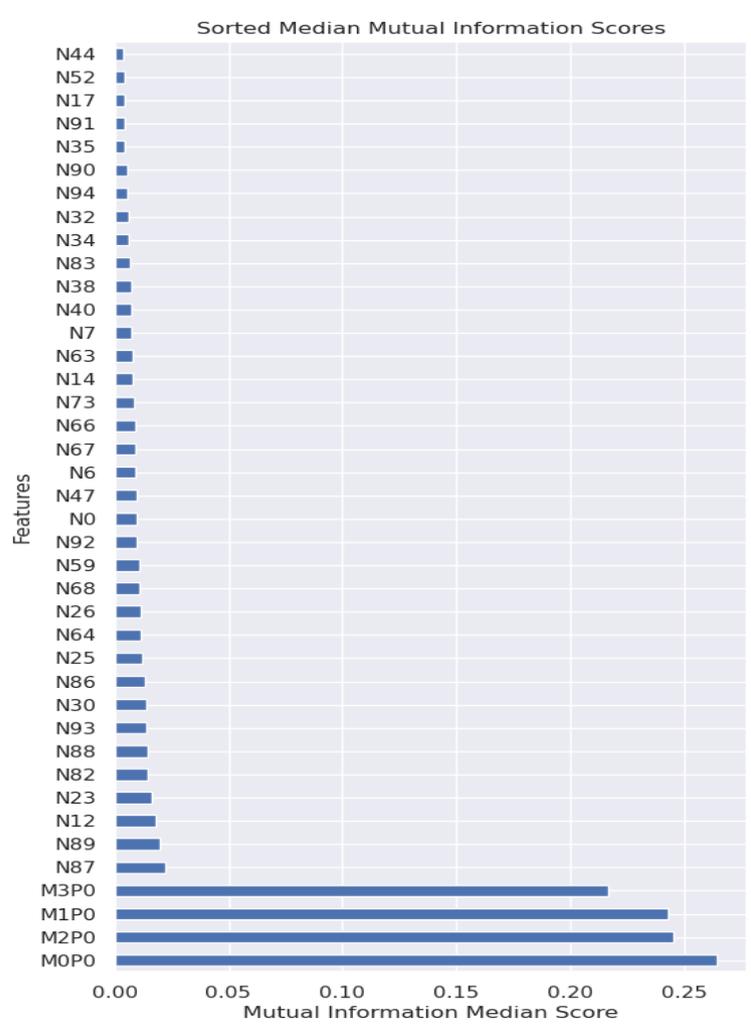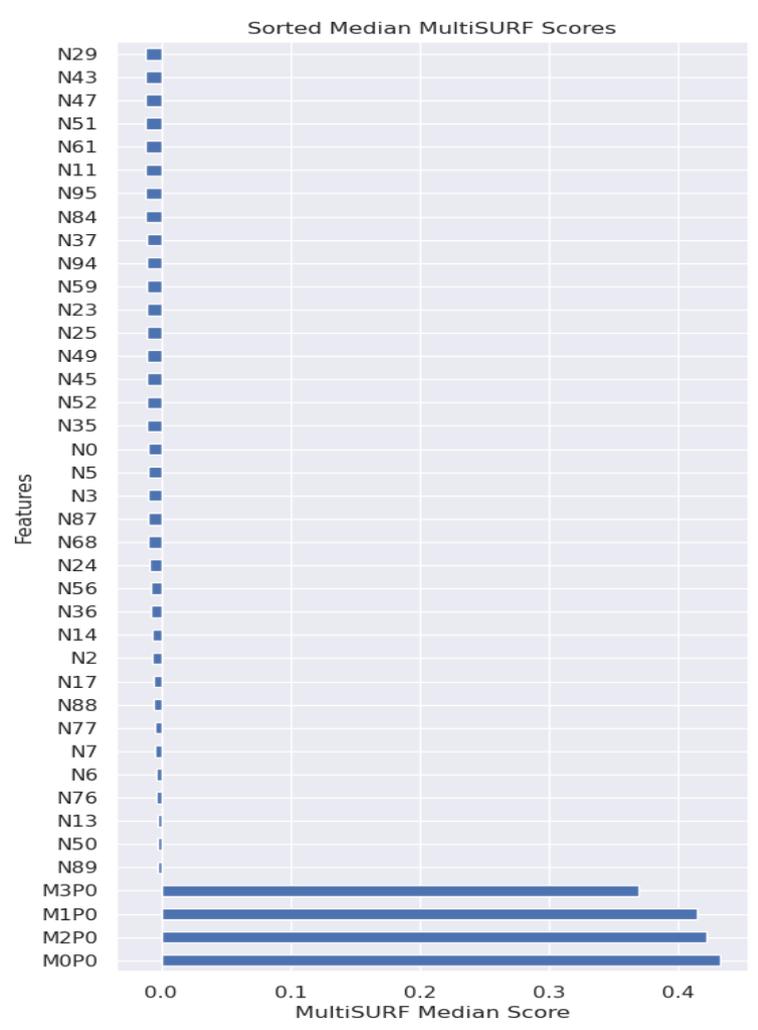

## Composite Feature Importance Plot (Normalized and Performance Weighted)

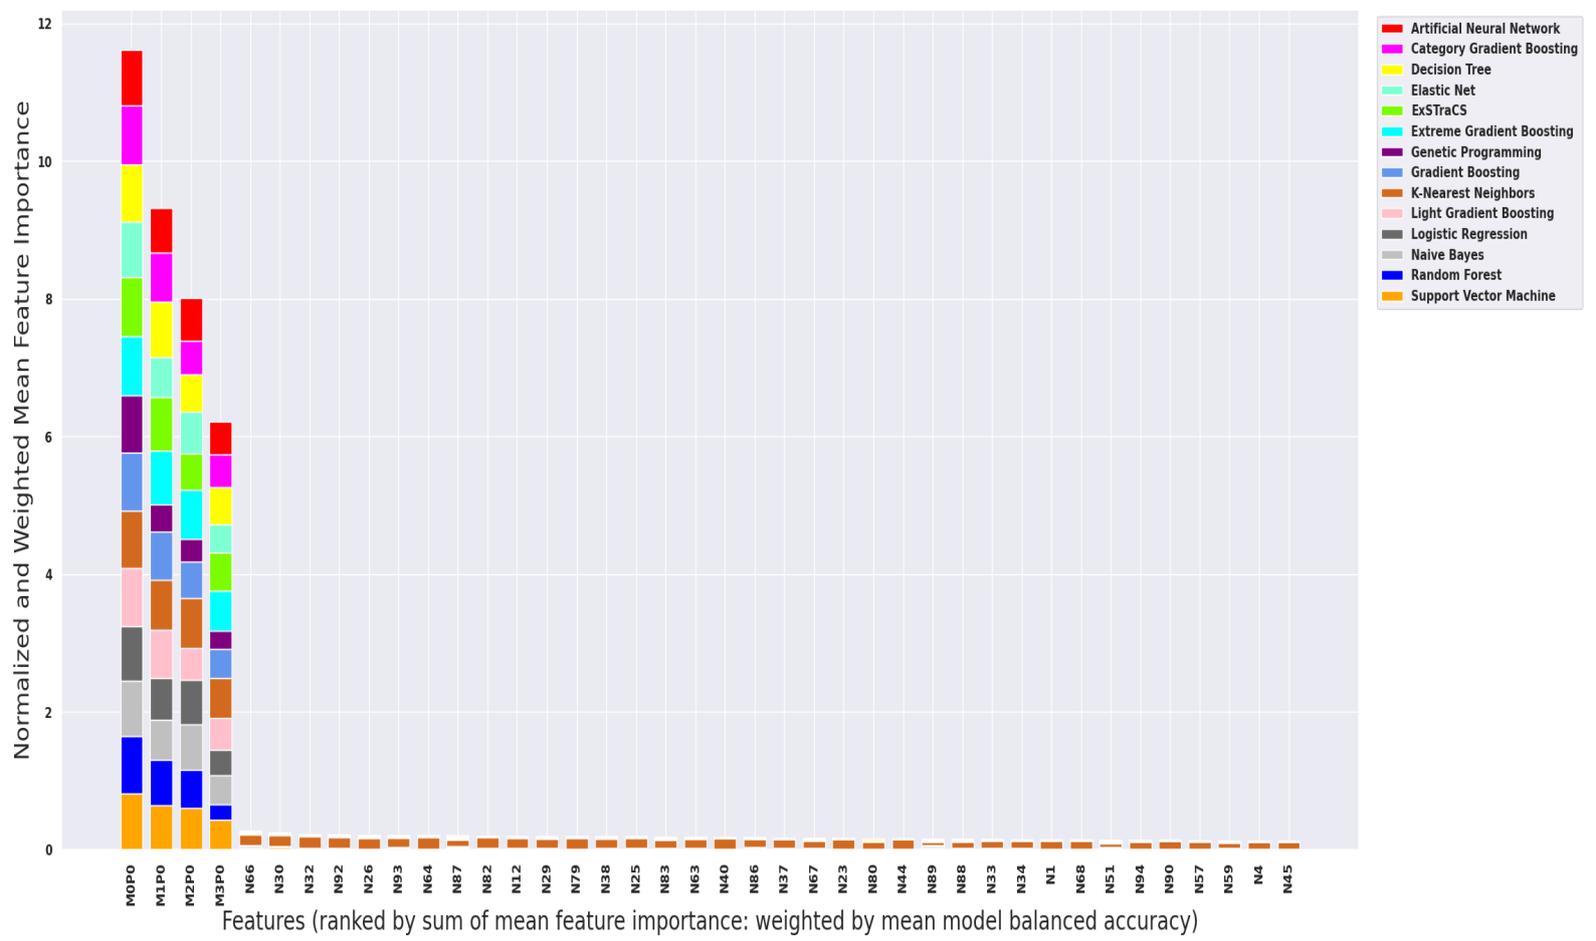

# Feature Importance Summary: D3 = C\_gametes\_uni\_4het\_L\_1\_H\_0

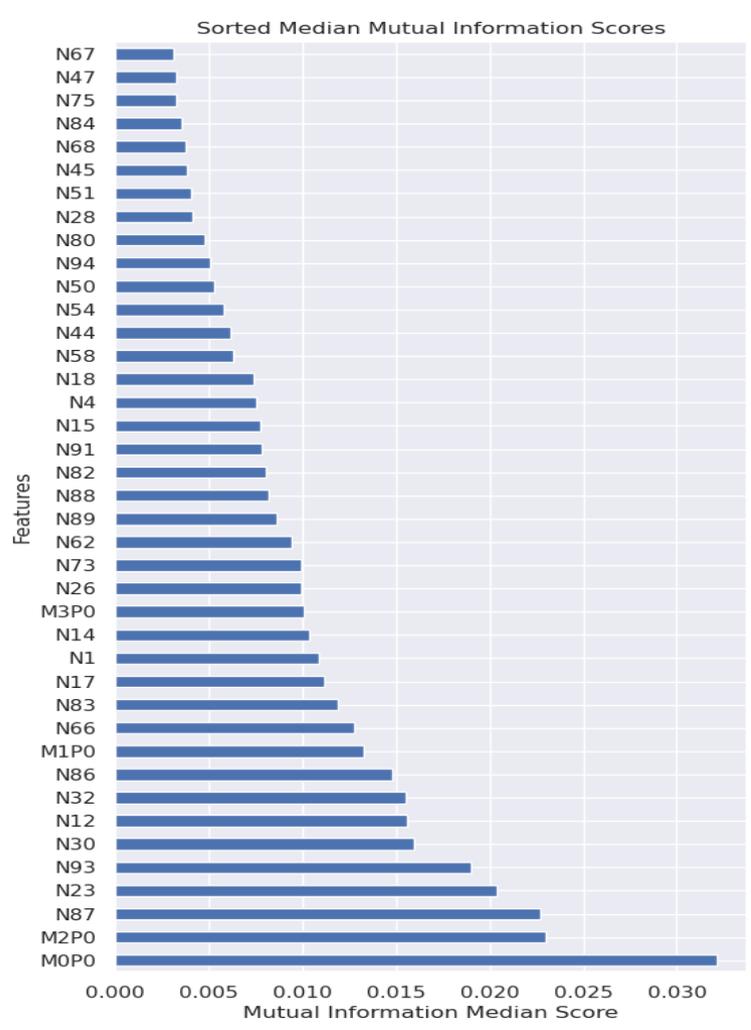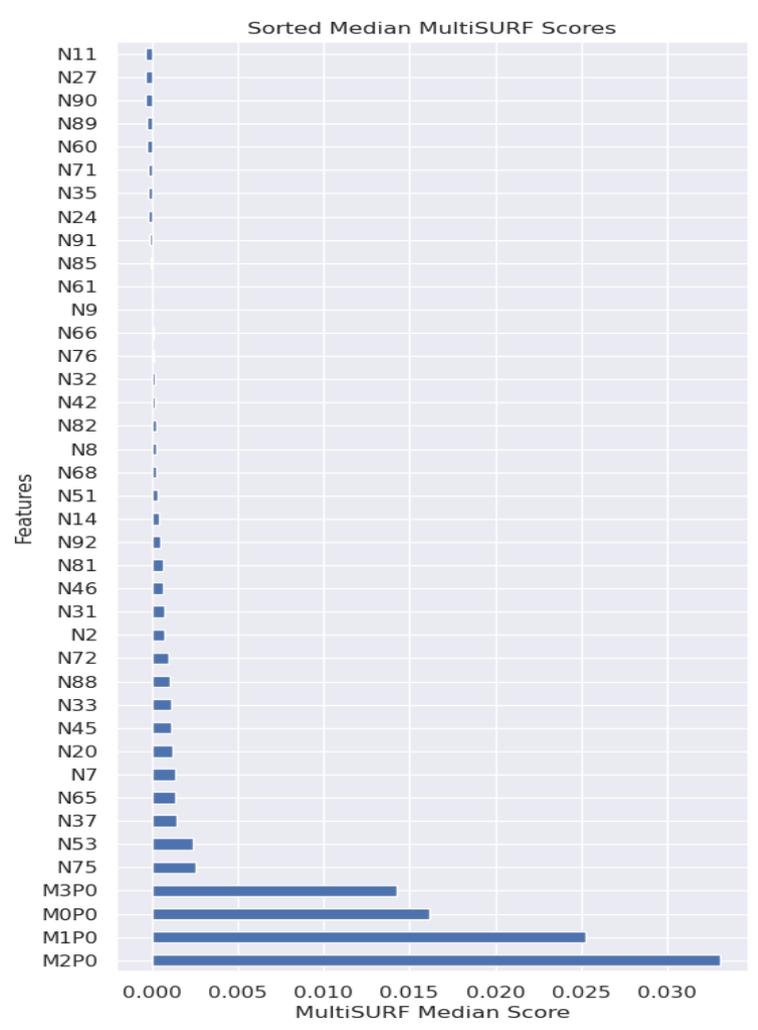

## Composite Feature Importance Plot (Normalized and Performance Weighted)

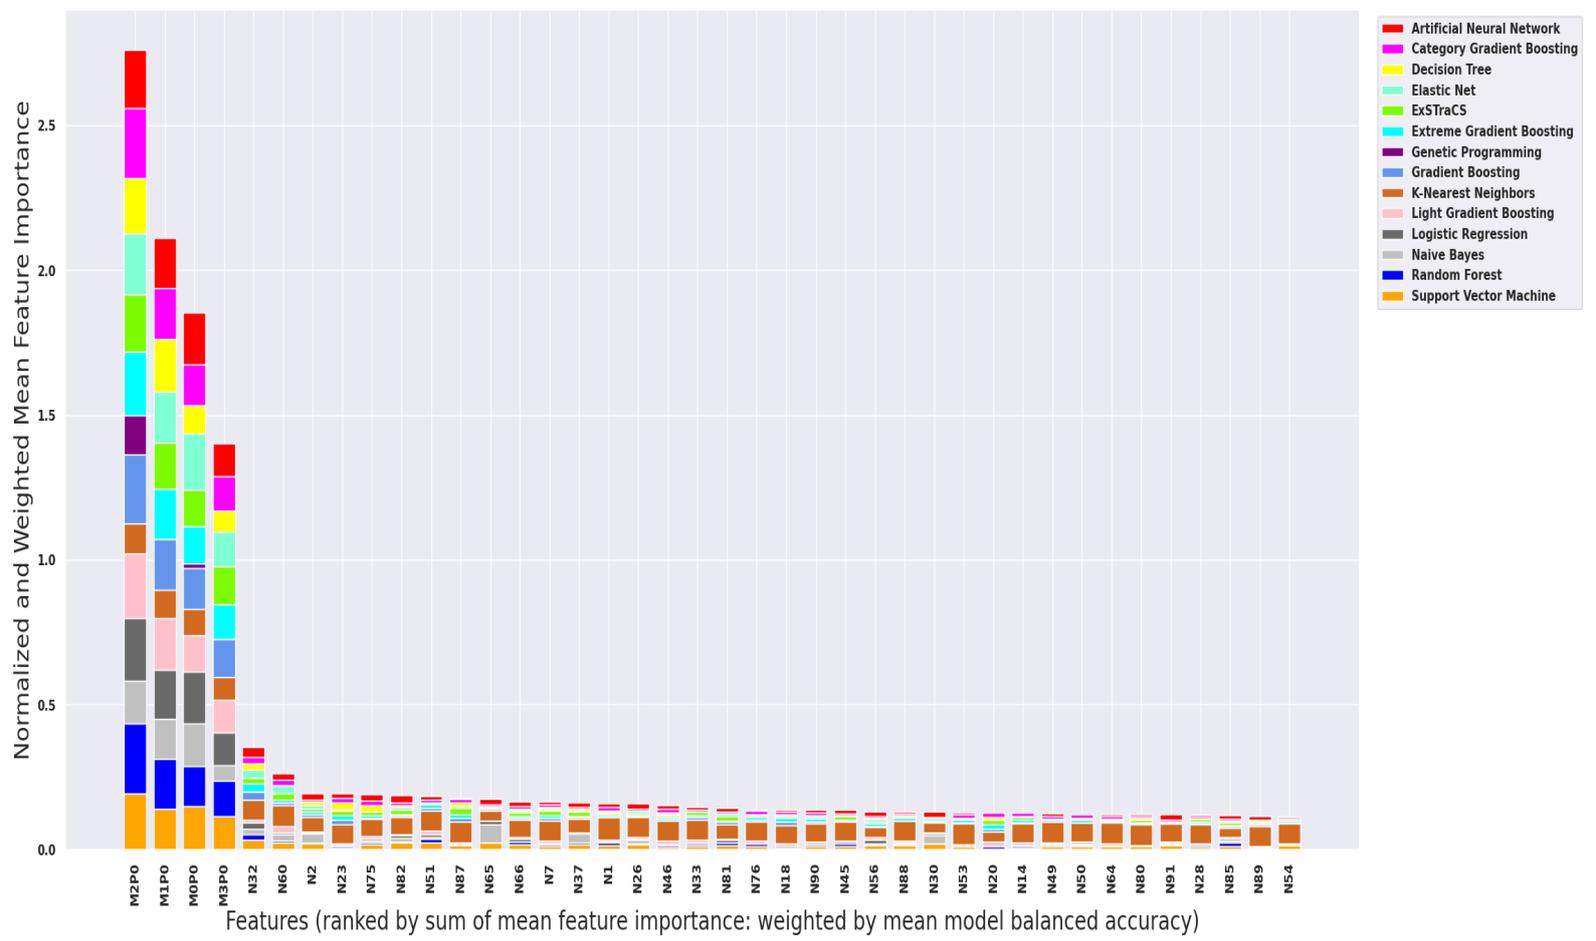

# Feature Importance Summary: D4 = D\_gametes\_2way\_epistasis\_L\_2\_H\_0

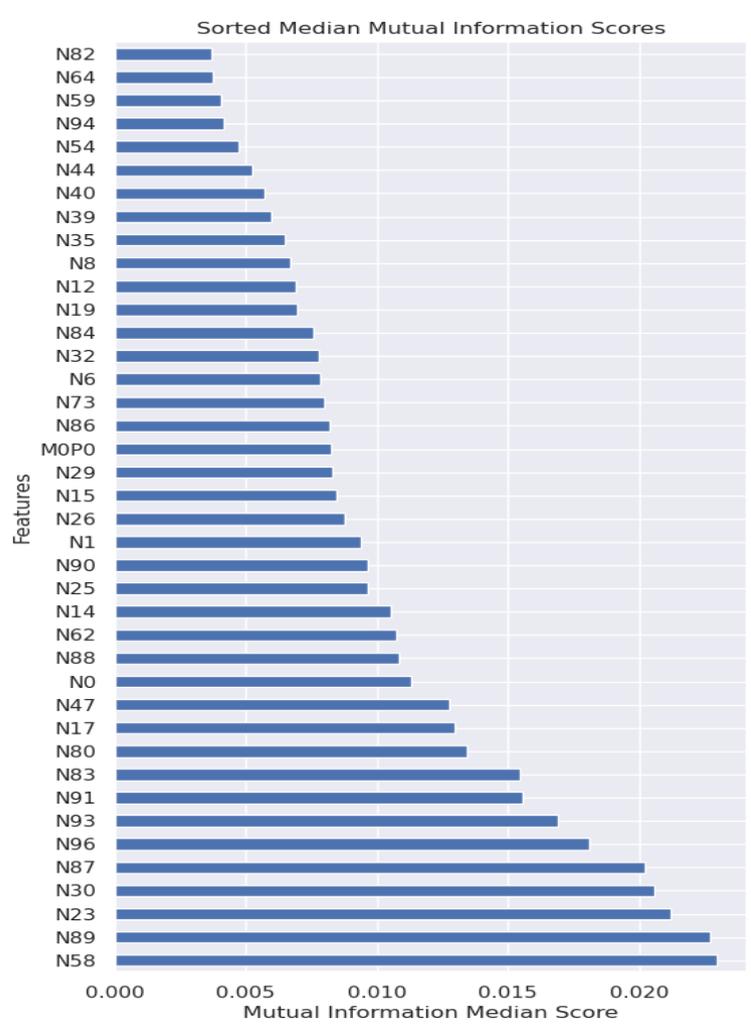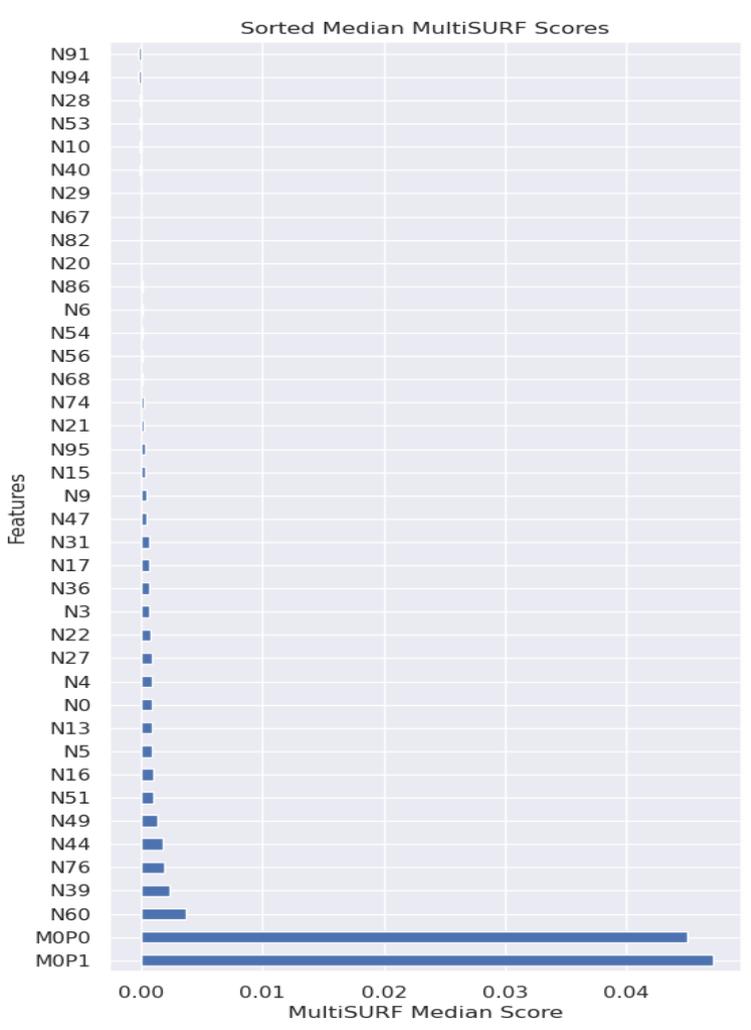

## Composite Feature Importance Plot (Normalized and Performance Weighted)

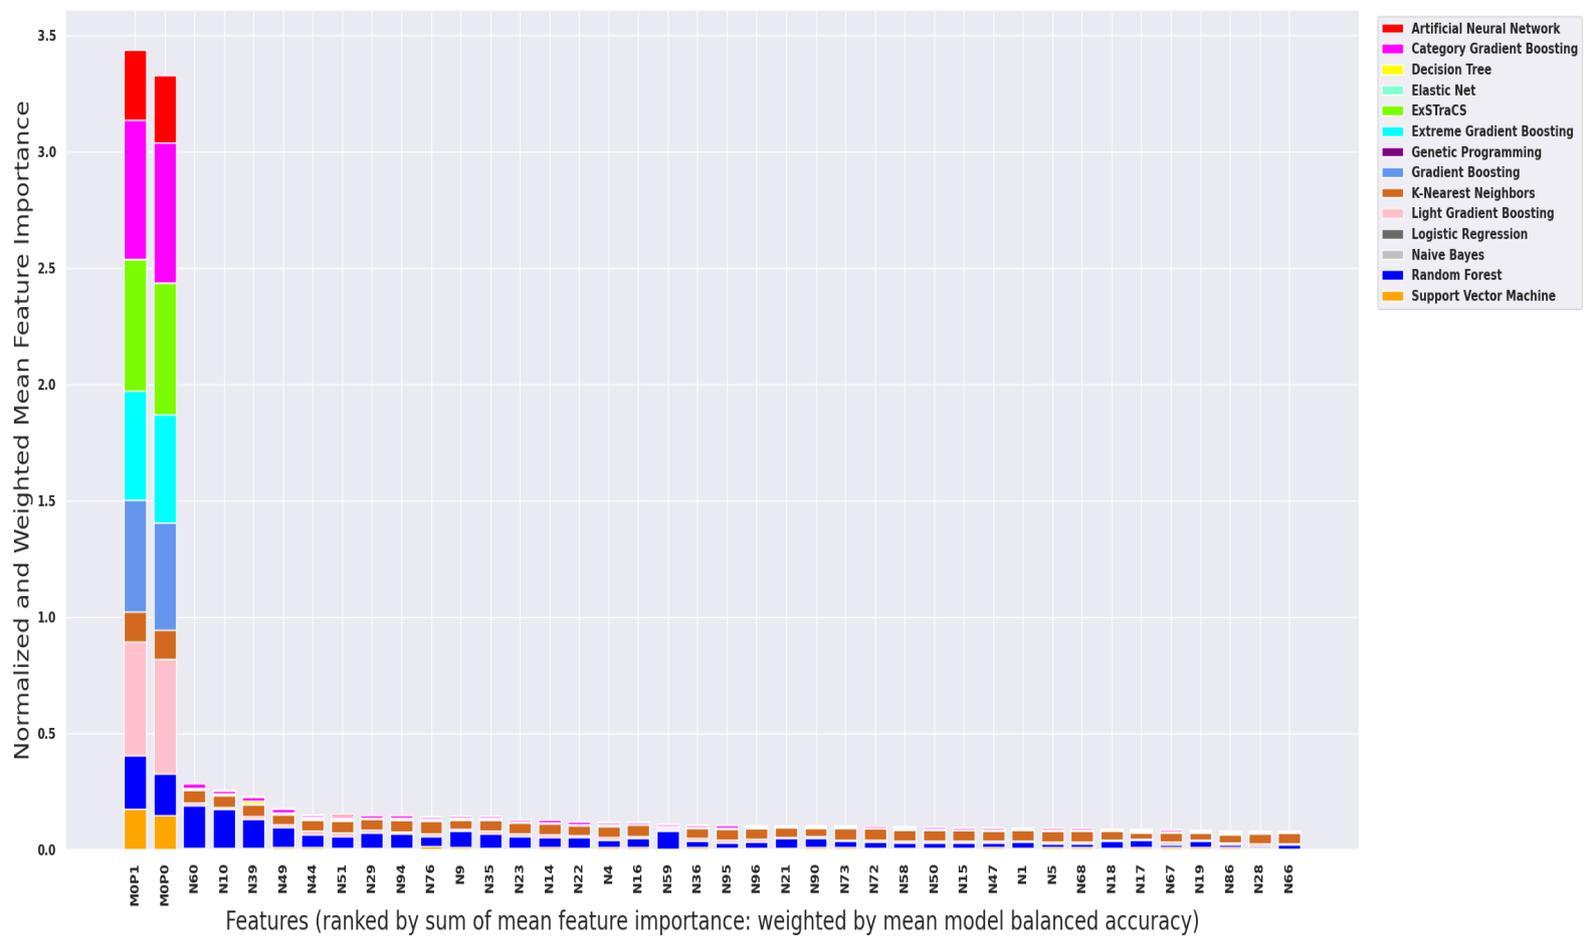

# Feature Importance Summary: D5 = E\_gametes\_2way\_epi\_2het\_L\_2\_H\_0

Sorted Median Mutual Information Scores

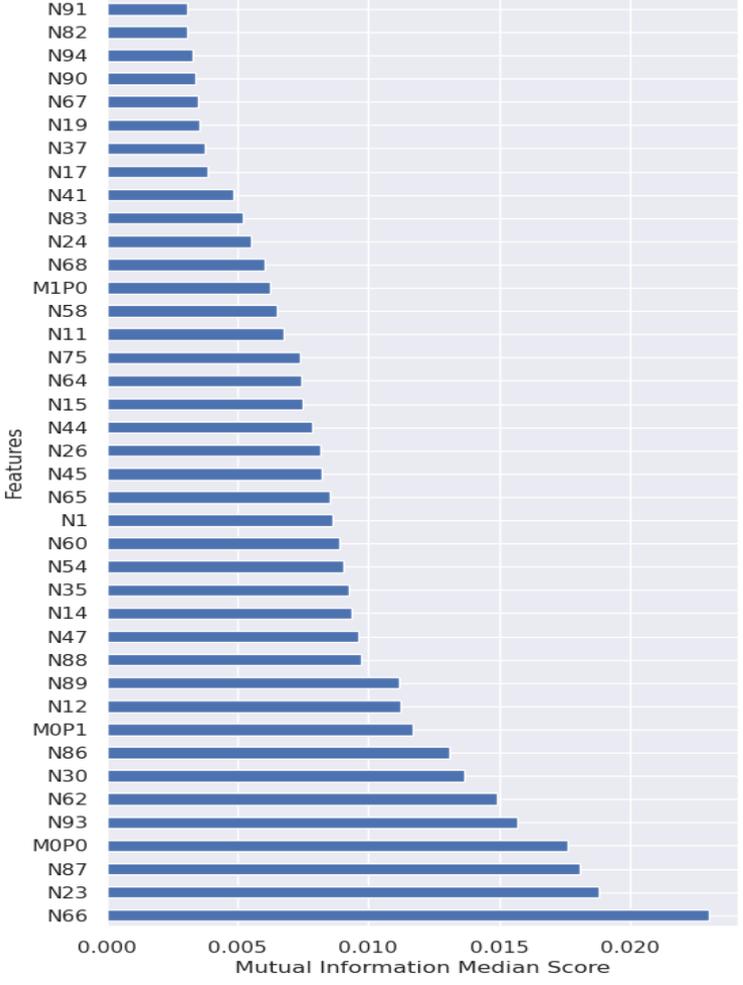

Sorted Median MultiSURF Scores

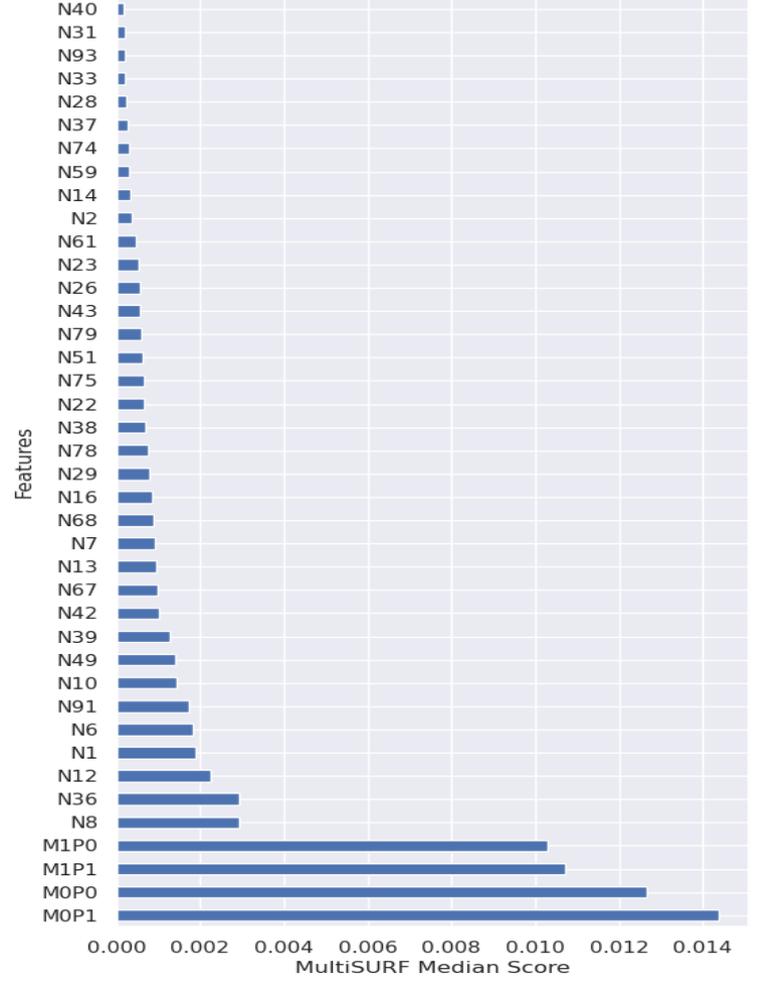

## Composite Feature Importance Plot (Normalized and Performance Weighted)

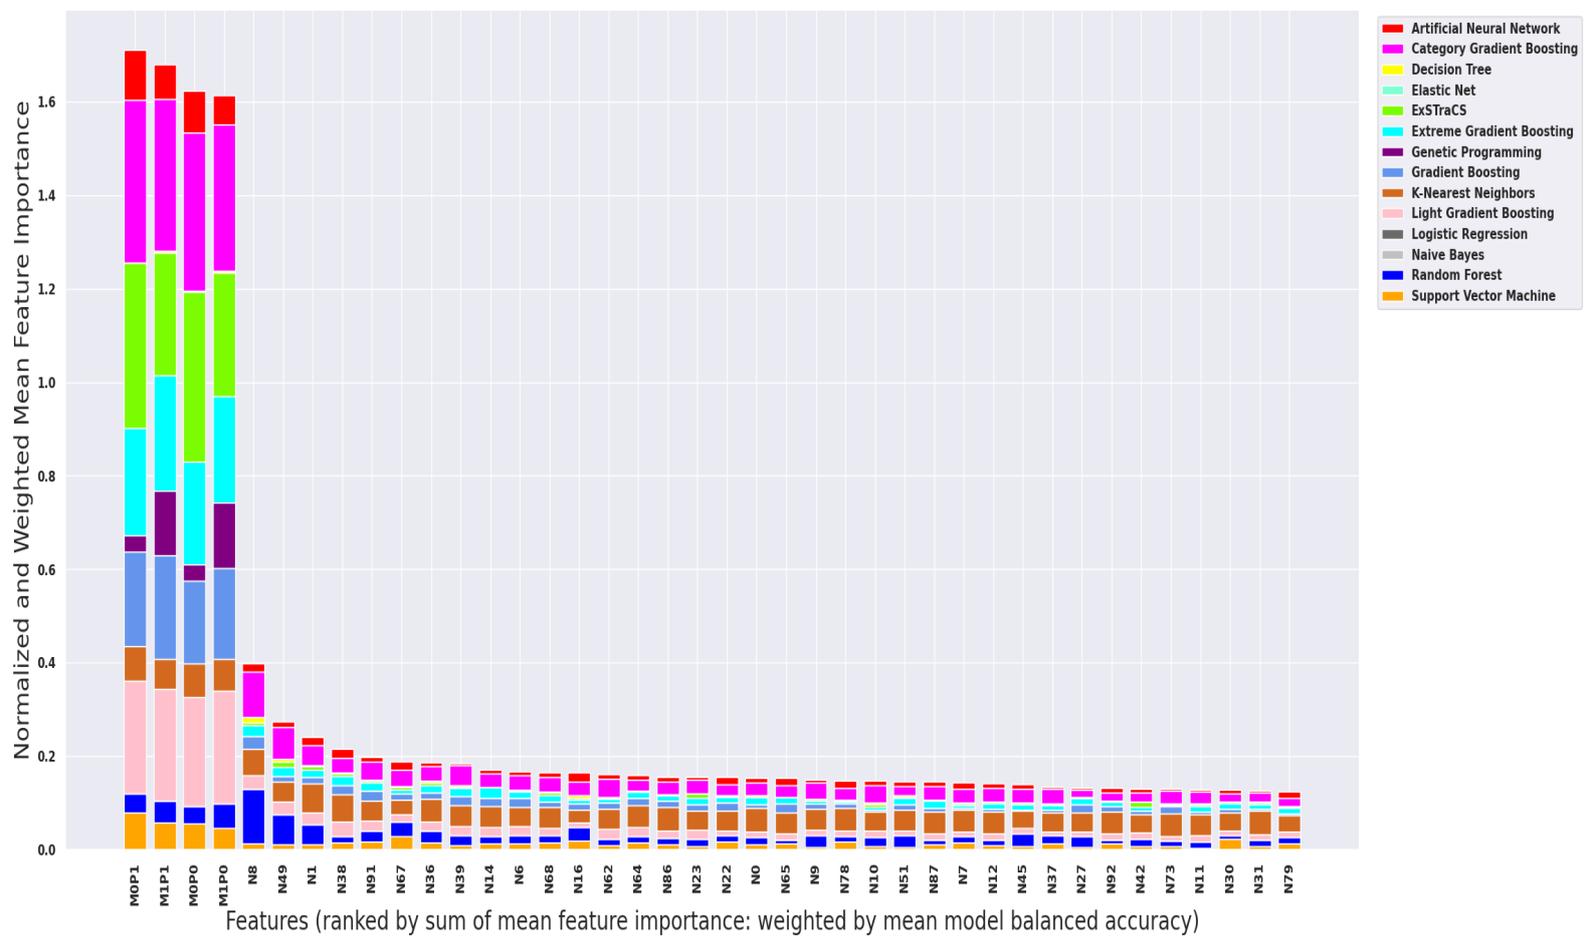

# Feature Importance Summary: D6 = F\_gametes\_3way\_epistasis\_L\_3\_H\_0

Sorted Median Mutual Information Scores

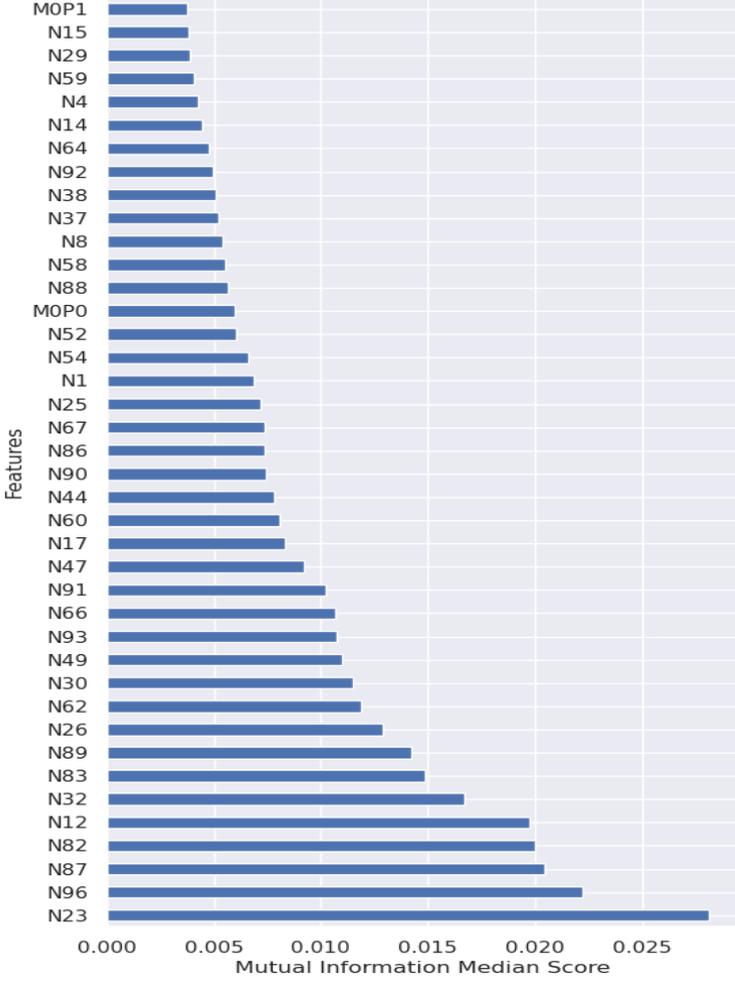

Sorted Median MultiSURF Scores

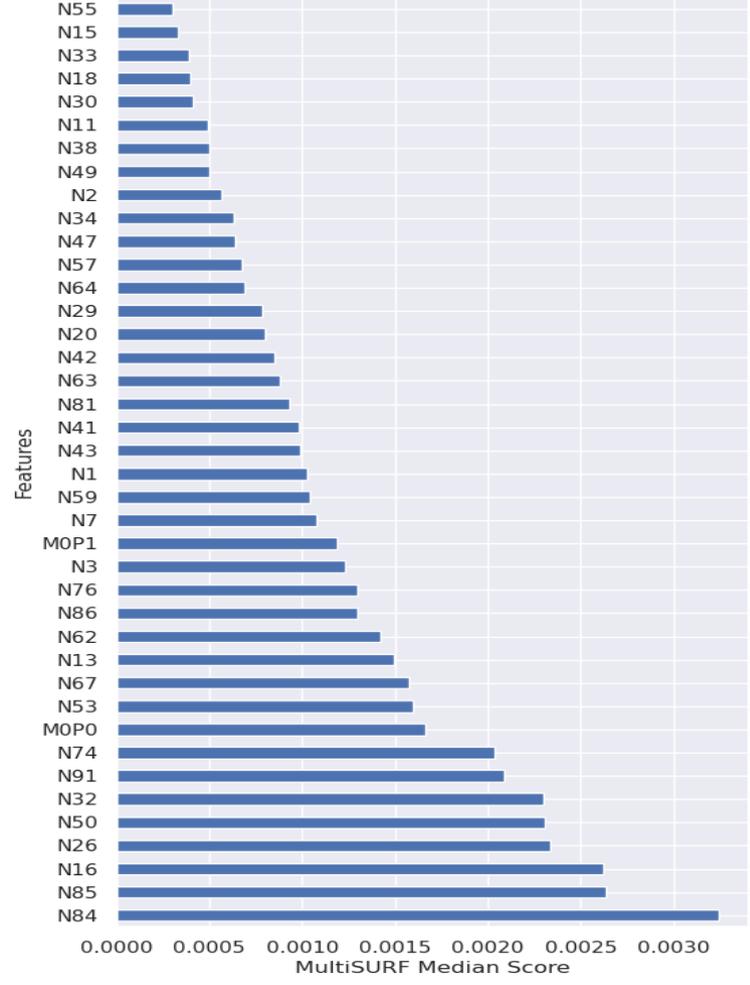

## Composite Feature Importance Plot (Normalized and Performance Weighted)

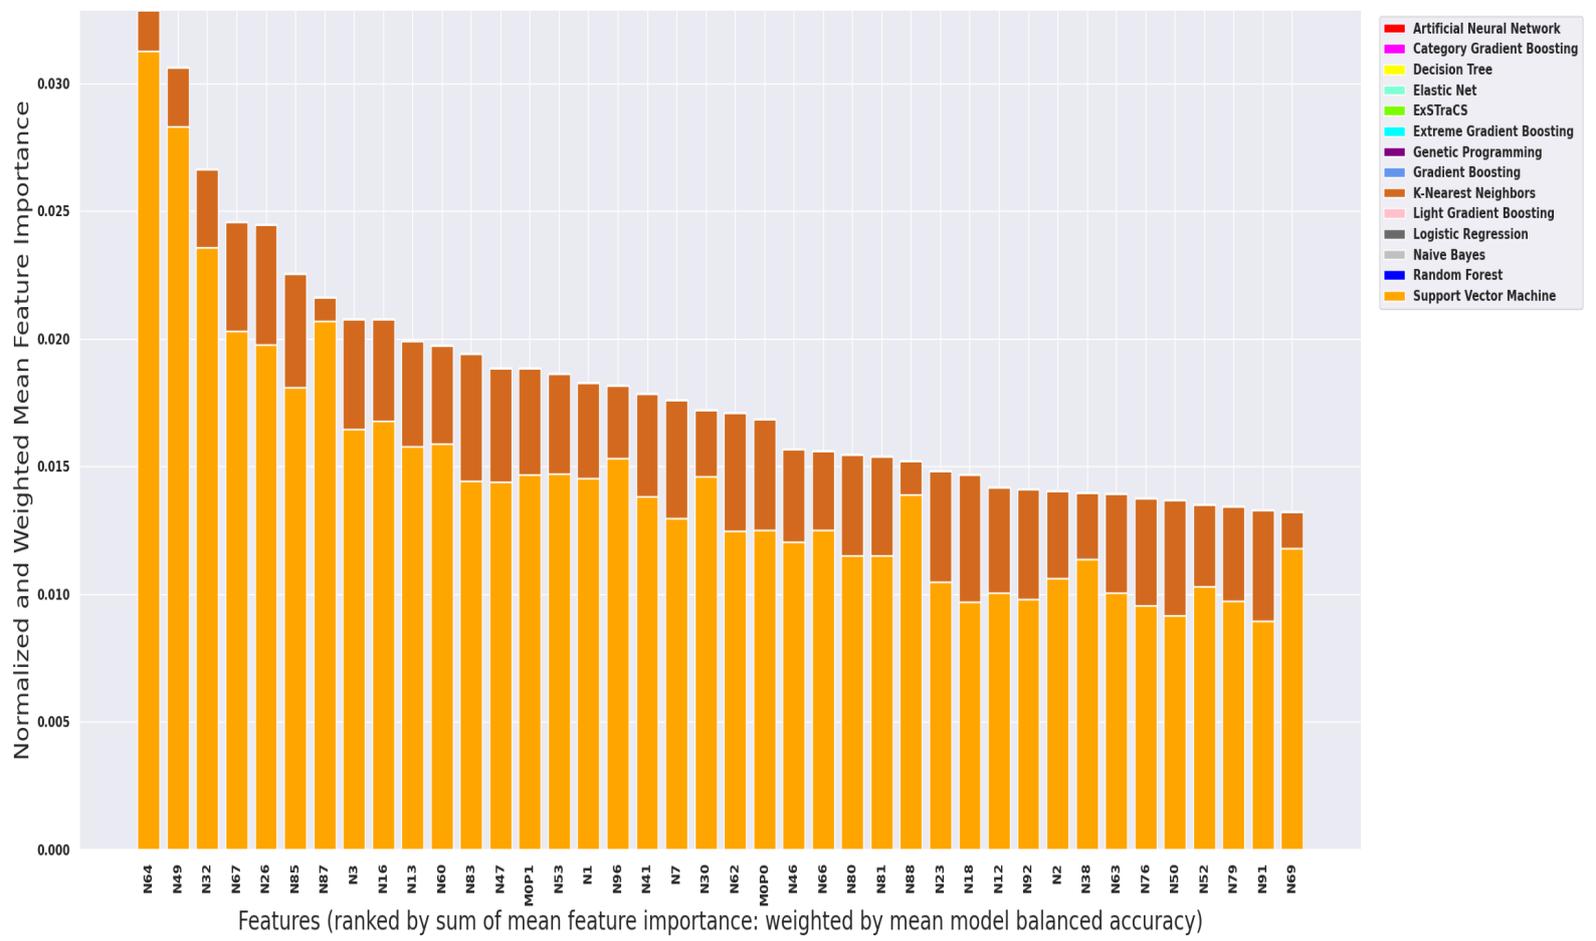

# Compare ML Performance Across Datasets

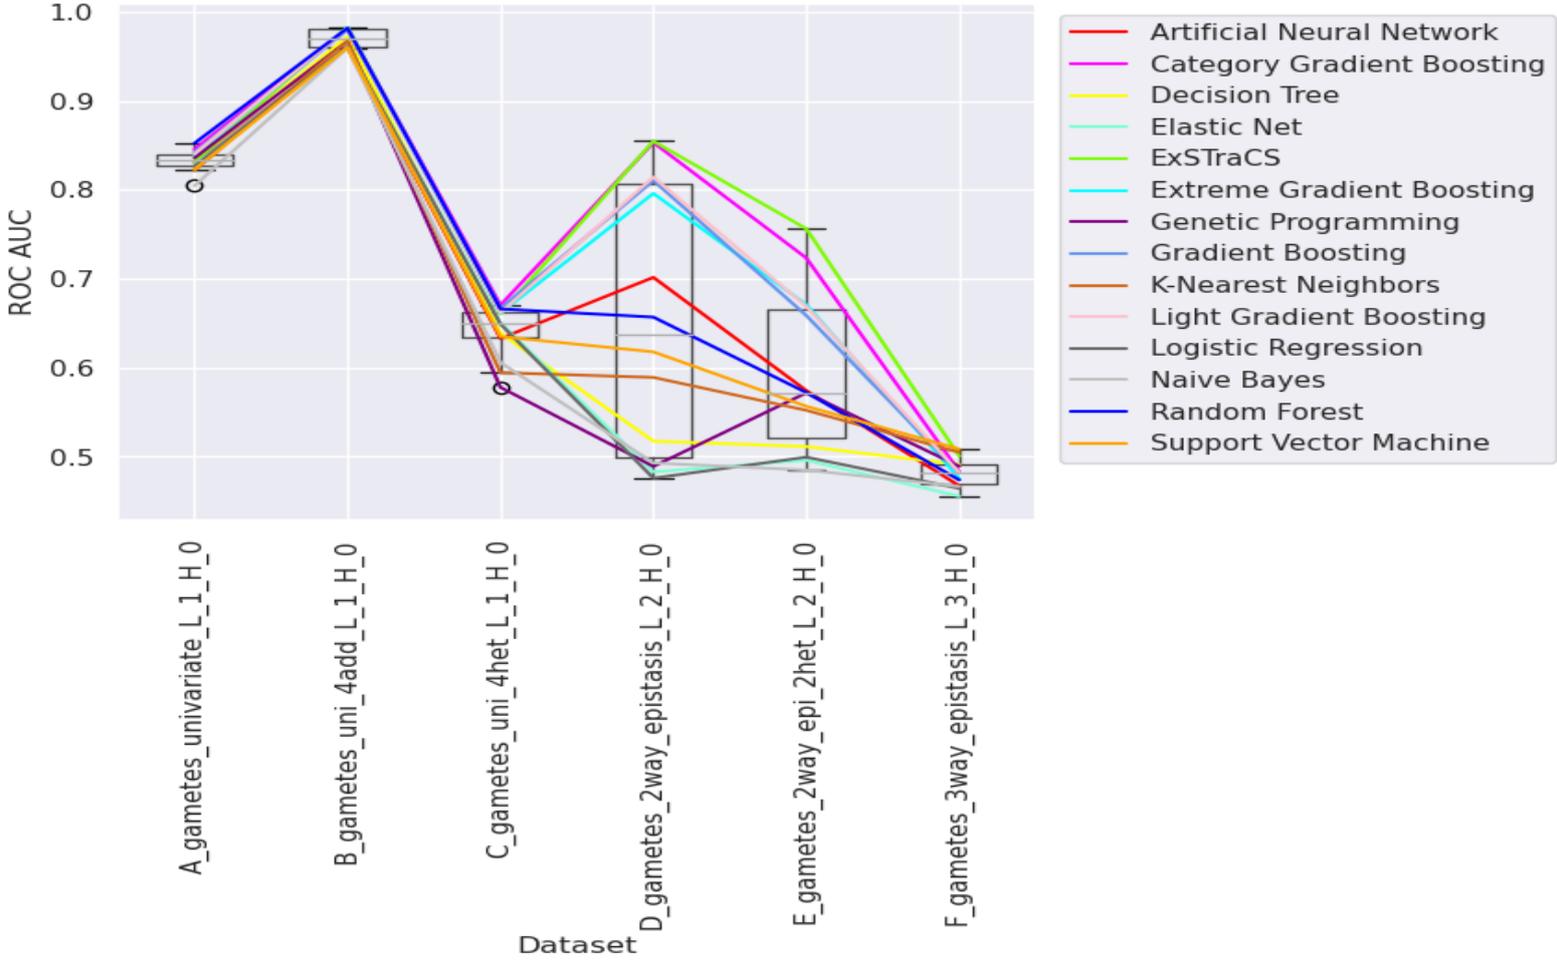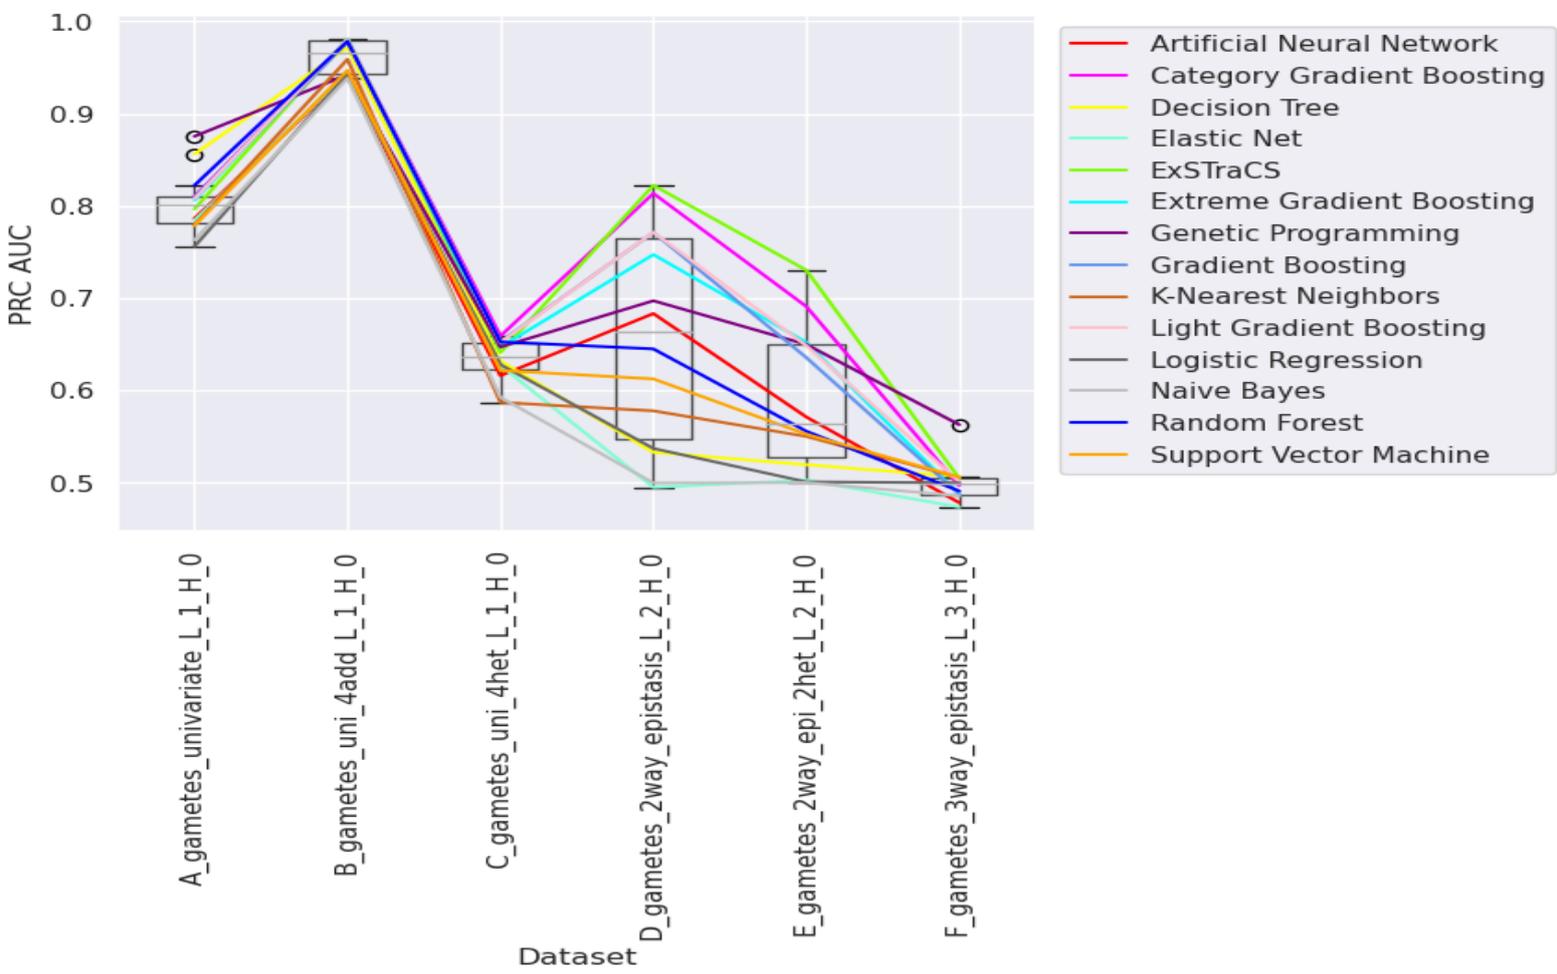

## Using Best Performing Algorithms (Kruskall Wallis Compare Datasets)

| Metrics              | P-Value | Best Alg D1                | Median D1 | Best Alg D2                | Median D2 | Best Alg D3                | Median D3 |
|----------------------|---------|----------------------------|-----------|----------------------------|-----------|----------------------------|-----------|
| Balanced Accuracy    | 0.0     | Category Gradient Boosting | 0.8312    | Extreme Gradient Boosting  | 0.9375    | Category Gradient Boosting | 0.6219    |
| Accuracy             | 0.0     | Category Gradient Boosting | 0.8312    | Extreme Gradient Boosting  | 0.9375    | Category Gradient Boosting | 0.6219    |
| F1 Score             | 0.0     | Category Gradient Boosting | 0.8258    | Extreme Gradient Boosting  | 0.9383    | Category Gradient Boosting | 0.6117    |
| Sensitivity (Recall) | 0.0     | Category Gradient Boosting | 0.8125    | ExSTraCS                   | 0.95      | Gradient Boosting          | 0.6188    |
| Specificity          | 0.0006  | Artificial Neural Network  | 0.85      | Category Gradient Boosting | 0.9312    | Genetic Programming        | 0.6938    |
| Precision (PPV)      | 0.0     | Category Gradient Boosting | 0.8477    | Category Gradient Boosting | 0.9309    | Random Forest              | 0.6338    |
| TP                   | 0.0     | Category Gradient Boosting | 65.0      | ExSTraCS                   | 76.0      | Gradient Boosting          | 49.5      |
| TN                   | 0.0006  | Artificial Neural Network  | 68.0      | Category Gradient Boosting | 74.5      | Genetic Programming        | 55.5      |
| FP                   | 0.0     | Naive Bayes                | 15.5      | Naive Bayes                | 8.0       | Artificial Neural Network  | 31.5      |
| FN                   | 0.0001  | K-Nearest Neighbors        | 19.5      | Elastic Net                | 8.0       | Genetic Programming        | 44.0      |
| NPV                  | 0.0     | Category Gradient Boosting | 0.817     | ExSTraCS                   | 0.9481    | Category Gradient Boosting | 0.6135    |
| LR+                  | 0.0     | Category Gradient Boosting | 5.5682    | Category Gradient Boosting | 13.5333   | Random Forest              | 1.7308    |
| LR-                  | 0.0     | K-Nearest Neighbors        | 0.2766    | Naive Bayes                | 0.1145    | K-Nearest Neighbors        | 0.8531    |
| ROC AUC              | 0.0     | Category Gradient Boosting | 0.8586    | Extreme Gradient Boosting  | 0.983     | Category Gradient Boosting | 0.6695    |
| PRC AUC              | 0.0     | Genetic Programming        | 0.8803    | Random Forest              | 0.982     | Category Gradient Boosting | 0.6735    |
| PRC APS              | 0.0     | Random Forest              | 0.8329    | Random Forest              | 0.9822    | Category Gradient Boosting | 0.6777    |

| Metrics              | P-Value | Best Alg D4                | Median D4 | Best Alg D5                | Median D5 | Best Alg D6                | Median D6 |
|----------------------|---------|----------------------------|-----------|----------------------------|-----------|----------------------------|-----------|
| Balanced Accuracy    | 0.0     | Category Gradient Boosting | 0.8031    | Category Gradient Boosting | 0.6812    | Decision Tree              | 0.5       |
| Accuracy             | 0.0     | Category Gradient Boosting | 0.8031    | Category Gradient Boosting | 0.6812    | Decision Tree              | 0.5       |
| F1 Score             | 0.0     | Category Gradient Boosting | 0.8195    | ExSTraCS                   | 0.6871    | Category Gradient Boosting | 0.5017    |
| Sensitivity (Recall) | 0.0     | Category Gradient Boosting | 0.9       | Genetic Programming        | 0.7312    | Support Vector Machine     | 0.525     |
| Specificity          | 0.0006  | Genetic Programming        | 1.0       | Category Gradient Boosting | 0.6625    | Genetic Programming        | 0.6       |
| Precision (PPV)      | 0.0     | Category Gradient Boosting | 0.7567    | Category Gradient Boosting | 0.6726    | Decision Tree              | 0.5       |
| TP                   | 0.0     | Category Gradient Boosting | 72.0      | Genetic Programming        | 58.5      | Support Vector Machine     | 42.0      |
| TN                   | 0.0006  | Genetic Programming        | 80.0      | Category Gradient Boosting | 53.0      | Genetic Programming        | 48.0      |
| FP                   | 0.0     | Naive Bayes                | 54.0      | Naive Bayes                | 41.0      | Category Gradient Boosting | 44.0      |
| FN                   | 0.0001  | Genetic Programming        | 80.0      | Elastic Net                | 41.5      | Genetic Programming        | 48.5      |
| NPV                  | 0.0     | Category Gradient Boosting | 0.8778    | ExSTraCS                   | 0.6883    | Support Vector Machine     | 0.5016    |
| LR+                  | 0.0     | Category Gradient Boosting | 3.1136    | Category Gradient Boosting | 2.0549    | Decision Tree              | 1.0       |
| LR-                  | 0.0     | Logistic Regression        | 1.0932    | Elastic Net                | 1.061     | Extreme Gradient Boosting  | 1.129     |
| ROC AUC              | 0.0     | ExSTraCS                   | 0.8553    | ExSTraCS                   | 0.7538    | K-Nearest Neighbors        | 0.5019    |
| PRC AUC              | 0.0     | ExSTraCS                   | 0.8151    | ExSTraCS                   | 0.736     | Genetic Programming        | 0.5424    |
| PRC APS              | 0.0     | ExSTraCS                   | 0.8194    | ExSTraCS                   | 0.7386    | Decision Tree              | 0.5129    |

# Pipeline Runtime Summary

## A gametes\_univariate\_L\_1\_H\_0

| Pipeline Component                      | Phase | Time (sec)         |
|-----------------------------------------|-------|--------------------|
| Exploratory Analysis                    | 1     | 4.73869776725769   |
| Scale and Impute                        | 2     | 1.7498915195465088 |
| Mutual Information (Feature Importance) | 3     | 5.3177361488342285 |
| MultiSURF (Feature Importance)          | 3     | 604.203547000885   |
| Feature Selection                       | 4     | 2.1695942878723145 |
| Artificial Neural Network(Modeling)     | 5     | 5320.808990716934  |
| Category Gradient Boosting(Modeling)    | 5     | 10144.0906894207   |
| Decision Tree(Modeling)                 | 5     | 38.19391870498657  |
| Elastic Net(Modeling)                   | 5     | 85.58098864555359  |
| ExSTraCS(Modeling)                      | 5     | 50726.17943096161  |
| Extreme Gradient Boosting(Modeling)     | 5     | 9209.134371519089  |
| Genetic Programming(Modeling)           | 5     | 12098.743137836456 |
| Gradient Boosting(Modeling)             | 5     | 9007.685661792755  |
| K-Nearest Neighbors(Modeling)           | 5     | 1165.746036052704  |
| Light Gradient Boosting(Modeling)       | 5     | 457.1076564788818  |
| Logistic Regression(Modeling)           | 5     | 43.08088564872742  |
| Naive Bayes(Modeling)                   | 5     | 7.421862125396728  |
| Random Forest(Modeling)                 | 5     | 5377.947291374207  |
| Support Vector Machine(Modeling)        | 5     | 174096.87625169754 |
| Stats Summary                           | 6     | 42.883432388305664 |

## B gametes\_uni\_4add\_L\_1\_H\_0

| Pipeline Component                      | Phase | Time (sec)         |
|-----------------------------------------|-------|--------------------|
| Exploratory Analysis                    | 1     | 4.566713333129883  |
| Scale and Impute                        | 2     | 1.8375630378723145 |
| Mutual Information (Feature Importance) | 3     | 6.53204083442688   |
| MultiSURF (Feature Importance)          | 3     | 610.6274473667145  |
| Feature Selection                       | 4     | 1.9258391857147217 |
| Artificial Neural Network(Modeling)     | 5     | 5225.150309085846  |
| Category Gradient Boosting(Modeling)    | 5     | 9015.743186950684  |
| Decision Tree(Modeling)                 | 5     | 38.50866222381592  |
| Elastic Net(Modeling)                   | 5     | 60.02470207214356  |
| ExSTraCS(Modeling)                      | 5     | 40043.7307229004   |
| Extreme Gradient Boosting(Modeling)     | 5     | 7936.427369832993  |
| Genetic Programming(Modeling)           | 5     | 12750.345814466476 |
| Gradient Boosting(Modeling)             | 5     | 6697.668353319168  |
| K-Nearest Neighbors(Modeling)           | 5     | 946.2350940704346  |
| Light Gradient Boosting(Modeling)       | 5     | 987.2158951759338  |
| Logistic Regression(Modeling)           | 5     | 55.01270127296448  |
| Naive Bayes(Modeling)                   | 5     | 6.482517242431641  |
| Random Forest(Modeling)                 | 5     | 6229.598489046097  |
| Support Vector Machine(Modeling)        | 5     | 5790.764683485031  |
| Stats Summary                           | 6     | 43.1333224773407   |

## C gametes\_uni\_4het\_L\_1\_H\_0

| Pipeline Component                      | Phase | Time (sec)         |
|-----------------------------------------|-------|--------------------|
| Exploratory Analysis                    | 1     | 4.433680057525635  |
| Scale and Impute                        | 2     | 1.687865972518921  |
| Mutual Information (Feature Importance) | 3     | 5.291030883789063  |
| MultiSURF (Feature Importance)          | 3     | 602.6408751010895  |
| Feature Selection                       | 4     | 2.176287889480591  |
| Artificial Neural Network(Modeling)     | 5     | 3627.900838375092  |
| Category Gradient Boosting(Modeling)    | 5     | 9944.452085971832  |
| Decision Tree(Modeling)                 | 5     | 37.09562611579895  |
| Elastic Net(Modeling)                   | 5     | 89.12952470779419  |
| ExSTraCS(Modeling)                      | 5     | 57958.41920876503  |
| Extreme Gradient Boosting(Modeling)     | 5     | 8238.559374332428  |
| Genetic Programming(Modeling)           | 5     | 12157.023282766342 |
| Gradient Boosting(Modeling)             | 5     | 7813.950355529785  |
| K-Nearest Neighbors(Modeling)           | 5     | 1281.081752061844  |
| Light Gradient Boosting(Modeling)       | 5     | 383.5631954669952  |
| Logistic Regression(Modeling)           | 5     | 64.72454810142517  |
| Naive Bayes(Modeling)                   | 5     | 8.346933603286743  |
| Random Forest(Modeling)                 | 5     | 5729.359919786453  |
| Support Vector Machine(Modeling)        | 5     | 14858.341987609863 |
| Stats Summary                           | 6     | 40.40311050415039  |

## D gametes\_2way\_epistasis\_L\_2\_H\_0

| Pipeline Component                      | Phase | Time (sec)         |
|-----------------------------------------|-------|--------------------|
| Exploratory Analysis                    | 1     | 4.650439977645874  |
| Scale and Impute                        | 2     | 1.6736793518066406 |
| Mutual Information (Feature Importance) | 3     | 5.345559120178223  |
| MultiSURF (Feature Importance)          | 3     | 608.453090429306   |
| Feature Selection                       | 4     | 2.8015153408050537 |
| Artificial Neural Network(Modeling)     | 5     | 5038.93678021431   |
| Category Gradient Boosting(Modeling)    | 5     | 10204.958746433258 |
| Decision Tree(Modeling)                 | 5     | 44.3093535900116   |
| Elastic Net(Modeling)                   | 5     | 182.16924285888672 |
| ExSTraCS(Modeling)                      | 5     | 49104.40555667877  |
| Extreme Gradient Boosting(Modeling)     | 5     | 9240.086088895798  |
| Genetic Programming(Modeling)           | 5     | 11817.11372089386  |
| Gradient Boosting(Modeling)             | 5     | 9419.505038499832  |
| K-Nearest Neighbors(Modeling)           | 5     | 1639.1401796340942 |
| Light Gradient Boosting(Modeling)       | 5     | 1490.1613273620603 |
| Logistic Regression(Modeling)           | 5     | 91.6237859725952   |
| Naive Bayes(Modeling)                   | 5     | 10.659066200256348 |
| Random Forest(Modeling)                 | 5     | 9711.13189983368   |
| Support Vector Machine(Modeling)        | 5     | 11570.261613845823 |
| Stats Summary                           | 6     | 39.379104137420654 |

## E gametes\_2way\_epi\_2het\_L\_2\_H\_0

| Pipeline Component                      | Phase | Time (sec)         |
|-----------------------------------------|-------|--------------------|
| Exploratory Analysis                    | 1     | 5.341846227645874  |
| Scale and Impute                        | 2     | 1.6624724864959717 |
| Mutual Information (Feature Importance) | 3     | 5.673290014266968  |
| MultiSURF (Feature Importance)          | 3     | 612.720006942749   |
| Feature Selection                       | 4     | 2.13039493560791   |
| Artificial Neural Network(Modeling)     | 5     | 4997.34556055069   |
| Category Gradient Boosting(Modeling)    | 5     | 10232.02905535698  |
| Decision Tree(Modeling)                 | 5     | 41.60875177383423  |
| Elastic Net(Modeling)                   | 5     | 138.28422927856445 |
| ExSTraCS(Modeling)                      | 5     | 58230.89253807068  |
| Extreme Gradient Boosting(Modeling)     | 5     | 9269.59049153328   |
| Genetic Programming(Modeling)           | 5     | 12026.985406637192 |
| Gradient Boosting(Modeling)             | 5     | 9272.694580316544  |
| K-Nearest Neighbors(Modeling)           | 5     | 4101.659785270691  |
| Light Gradient Boosting(Modeling)       | 5     | 1762.6592276096344 |
| Logistic Regression(Modeling)           | 5     | 67.74980092048645  |
| Naive Bayes(Modeling)                   | 5     | 9.383872509002686  |
| Random Forest(Modeling)                 | 5     | 7214.712219238281  |
| Support Vector Machine(Modeling)        | 5     | 13492.54438662529  |
| Stats Summary                           | 6     | 48.52452564239502  |

## F gametes\_3way\_epistasis\_L\_3\_H\_0

| Pipeline Component                      | Phase | Time (sec)         |
|-----------------------------------------|-------|--------------------|
| Exploratory Analysis                    | 1     | 3.691282272338867  |
| Scale and Impute                        | 2     | 1.7084667682647705 |
| Mutual Information (Feature Importance) | 3     | 5.339431047439575  |
| MultiSURF (Feature Importance)          | 3     | 602.4934921264648  |
| Feature Selection                       | 4     | 2.2001185417175293 |
| Artificial Neural Network(Modeling)     | 5     | 3981.604302406311  |
| Category Gradient Boosting(Modeling)    | 5     | 9912.949679851532  |
| Decision Tree(Modeling)                 | 5     | 33.5278525352478   |
| Elastic Net(Modeling)                   | 5     | 148.882572889328   |
| ExSTraCS(Modeling)                      | 5     | 69120.51602268219  |
| Extreme Gradient Boosting(Modeling)     | 5     | 9099.89913725853   |
| Genetic Programming(Modeling)           | 5     | 11580.600824594498 |
| Gradient Boosting(Modeling)             | 5     | 9491.089498758316  |
| K-Nearest Neighbors(Modeling)           | 5     | 5303.341495752335  |
| Light Gradient Boosting(Modeling)       | 5     | 2720.449346065521  |
| Logistic Regression(Modeling)           | 5     | 68.93168020248413  |
| Naive Bayes(Modeling)                   | 5     | 10.19297480583191  |
| Random Forest(Modeling)                 | 5     | 4983.866988658905  |
| Support Vector Machine(Modeling)        | 5     | 15824.628677129744 |
| Stats Summary                           | 6     | 33.97426390647888  |
