# Supplementary material for: STREAMLINE: An Automated Machine Learning Pipeline for Biomedicine Applied to Examine the Utility of Photography-Based Phenotypes for OSA Prediction Across International Sleep Centers
Source: arXiv:2312.05461 ancillary file (2023-12-09)
Supplement: Supplementary file 3 [file hcc_exp_STREAMLINE_Replication_Report.pdf]

# STREAMLINE Replication Data Evaluation Report: 2023-09-26 13:09:20.687356

## General Pipeline Settings:

CV Partitions: 10  
Partition Method: Stratified  
Categorical Cutoff: 10  
Statistical Significance Cutoff: 0.05  
Random Seed: 42  
Run From Notebook: False

## Feature Importance/Selection Settings:

Use Mutual Information: True  
Use MultiSURF: True  
Use TURF: False  
TURF Cutoff: 0.5  
MultiSURF Instance Subset: 2000  
Max Features to Keep: 2000  
Filter Poor Features: True  
Top Features to Display: 40  
Export Feature Importance Plot: True

## ML Modeling Algorithms:

Artificial Neural Network: True  
Category Gradient Boosting: True  
Decision Tree: True  
Elastic Net: True  
ExSTraCS: True  
Extreme Gradient Boosting: True  
Genetic Programming: True  
Gradient Boosting: True  
K-Nearest Neighbors: True  
Light Gradient Boosting: True  
Logistic Regression: True  
Naive Bayes: True  
Random Forest: True  
Support Vector Machine: True  
XCS: False  
eLCS: False

## Modeling Settings:

Primary Metric: balanced\_accuracy  
Training Subsample for KNN,ANN,SVM,and XGB: 0  
Uniform Feature Importance Estimation (Models): True  
Hyperparameter Sweep Number of Trials: 200  
Hyperparameter Timeout: 900  
Export Hyperparameter Sweep Plots: False

## LCS Settings (eLCS,XCS,ExSTraCS):

Do LCS Hyperparameter Sweep: False  
nu: 1  
Training Iterations: 200000  
N (Rule Population Size): 2000  
LCS Hyperparameter Sweep Timeout: 1200

## Stats and Figure Settings:

Export ROC Plot: True  
Export PRC Plot: True  
Export Metric Boxplots: True  
Export Feature Importance Boxplots: True  
Metric Weighting Composite FI Plots: balanced\_accuracy  
Top Model Features To Display: 40  
Export Feature Correlations: True

## EDA and Processing Settings:

Engineering Missingness Cutoff: 0.5  
Cleaning Missingness Cutoff: 0.5  
Correlation Removal Threshold: 1.0  
List of Exploratory Analysis Ran: ['Describe', 'Univariate Analysis', 'Feature Correlation']  
List of Exploratory Plots Saved: ['Describe', 'Univariate Analysis', 'Feature Correlation']  
Use Data Scaling: True  
Use Data Imputation: True  
Use Multivariate Imputation: True  
Overwrite CV Datasets: True

## Target Training Dataset:

hcc\_data\_custom

## Applied to Following Replication Dataset(s):

D1 = hcc\_data\_custom\_rep

## Target Data Settings:

Data Path: ./data/DemoData  
Output Path: /home/ryanurb/idata/output  
Experiment Name: hcc\_exp  
Class Label: Class  
Instance Label: InstanceID  
Match Label: None  
Ignored Features: None  
Specified Categorical Features: ./data/DemoFeatureTypes/hcc\_cat\_feat.csv  
Specified Quantitative Features: ./data/DemoFeatureTypes/hcc\_quant\_feat.csv

# Dataset and Model Prediction Summary: D1 = hcc\_data\_custom\_rep

## Data Processing/Counts Summary

|           | Instances | Total Features | Categorical Features | Quantitative Features | Missing Values | Missing Percent | Class 0 | Class 1 |
|-----------|-----------|----------------|----------------------|-----------------------|----------------|-----------------|---------|---------|
| Original  | 173       | 64             | 31                   | 33                    | 1360           | 0.1228          | 105     | 65      |
| C1        | 170       | 64             | 31                   | 33                    | 1335           | 0.1227          | 105     | 65      |
| R1        | 170       | 69             | 40                   | 29                    | 918            | 0.0783          | 105     | 65      |
| Processed | 170       | 69             | 40                   | 29                    | 918            | 0.0783          | 105     | 65      |

**Cleaning (C) and Replication (R) Elements**  
 \* C1 - Remove instances with no outcome  
 \* R1 - Add/remove same features as Phase 1

## Class Balance (Processed)

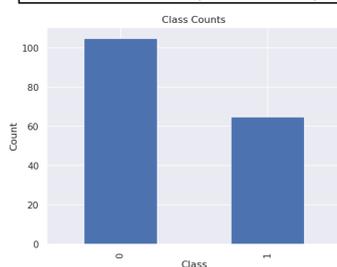

## Feature Correlations (Pearson)

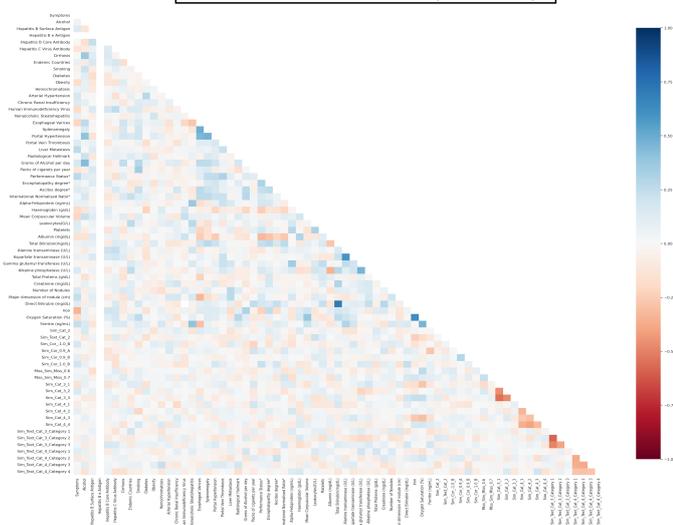

## Top ML Algorithm Results (Averaged Over CV Runs):

- Best (ROC\_AUC): Category Gradient Boosting = 0.890
- Best (Balanced Acc.): Gradient Boosting = 0.798
- Best (F1 Score): Gradient Boosting = 0.750
- Best (PRC AUC): K-Nearest Neighbors = 0.878
- Best (PRC APS): Category Gradient Boosting = 0.856

## ROC

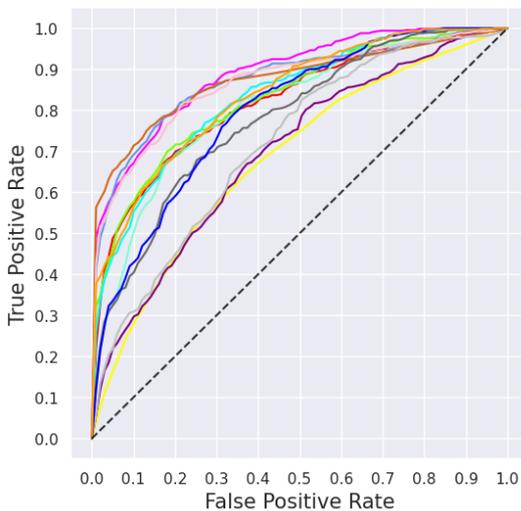

- Artificial Neural Network, AUC=0.818
- Category Gradient Boosting, AUC=0.890
- Decision Tree, AUC=0.683
- Elastic Net, AUC=0.808
- ExSTraCS, AUC=0.829
- Extreme Gradient Boosting, AUC=0.832
- Genetic Programming, AUC=0.695
- Gradient Boosting, AUC=0.873
- K-Nearest Neighbors, AUC=0.875
- Light Gradient Boosting, AUC=0.868
- Logistic Regression, AUC=0.778
- Naive Bayes, AUC=0.717
- Random Forest, AUC=0.795
- Support Vector Machine, AUC=0.838
- No-Skill

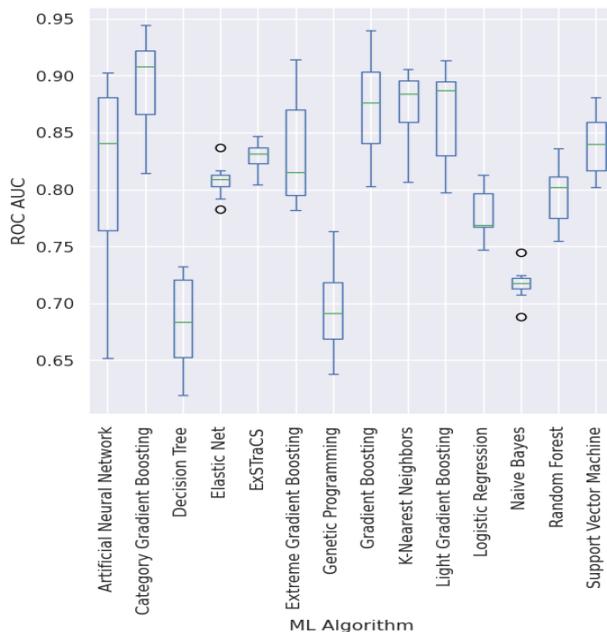

## PRC

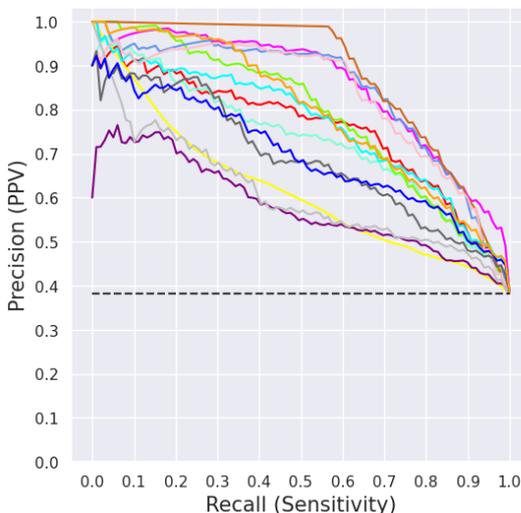

- Artificial Neural Network, AUC=0.756, APS=0.759
- Category Gradient Boosting, AUC=0.855, APS=0.856
- Decision Tree, AUC=0.618, APS=0.538
- Elastic Net, AUC=0.732, APS=0.731
- ExSTraCS, AUC=0.788, APS=0.790
- Extreme Gradient Boosting, AUC=0.766, APS=0.768
- Genetic Programming, AUC=0.580, APS=0.579
- Gradient Boosting, AUC=0.842, APS=0.844
- K-Nearest Neighbors, AUC=0.878, APS=0.851
- Light Gradient Boosting, AUC=0.830, APS=0.832
- Logistic Regression, AUC=0.690, APS=0.694
- Naive Bayes, AUC=0.609, APS=0.602
- Random Forest, AUC=0.697, APS=0.702
- Support Vector Machine, AUC=0.794, APS=0.796
- No-Skill

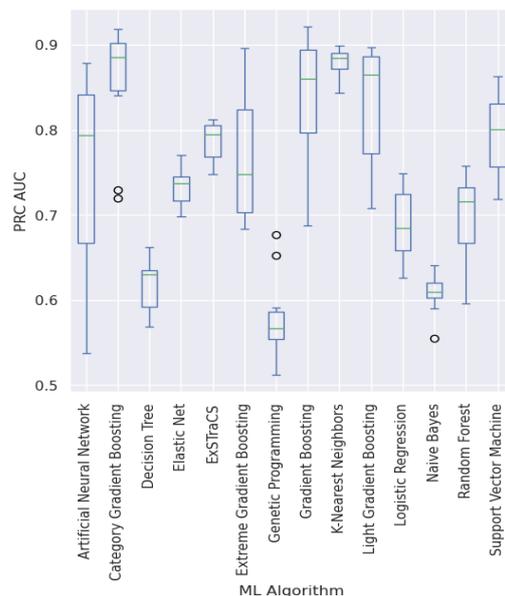

# Average Model Prediction Statistics (Rounded to 3 Decimal Points)

## D1 = hcc\_data\_custom\_rep

| ML Algorithm               | Balanced Accuracy | Accuracy | F1 Score | Sensitivity (Recall) | Specificity | Precision (PPV) | TP   | TN   | FP   | FN   | NPV   | LR+    | LR-   | ROC AUC | PRC AUC | PRC APS |
|----------------------------|-------------------|----------|----------|----------------------|-------------|-----------------|------|------|------|------|-------|--------|-------|---------|---------|---------|
| Artificial Neural Network  | 0.748             | 0.771    | 0.687    | 0.651                | 0.845       | 0.733           | 42.3 | 88.7 | 16.3 | 22.7 | 0.795 | 5.526  | 0.425 | 0.818   | 0.756   | 0.759   |
| Category Gradient Boosting | 0.776             | 0.815    | 0.714    | 0.612                | 0.94        | 0.863           | 39.8 | 98.7 | 6.3  | 25.2 | 0.798 | 16.613 | 0.413 | 0.89    | 0.855   | 0.856   |
| Decision Tree              | 0.643             | 0.661    | 0.559    | 0.566                | 0.719       | 0.564           | 36.8 | 75.5 | 29.5 | 28.2 | 0.729 | 2.146  | 0.602 | 0.683   | 0.618   | 0.538   |
| Elastic Net                | 0.734             | 0.757    | 0.662    | 0.634                | 0.833       | 0.707           | 41.2 | 87.5 | 17.5 | 23.8 | 0.789 | 4.018  | 0.436 | 0.808   | 0.732   | 0.731   |
| ExSTraCS                   | 0.748             | 0.764    | 0.687    | 0.683                | 0.813       | 0.704           | 44.4 | 85.4 | 19.6 | 20.6 | 0.808 | 4.064  | 0.386 | 0.829   | 0.788   | 0.79    |
| Extreme Gradient Boosting  | 0.742             | 0.76     | 0.682    | 0.668                | 0.817       | 0.702           | 43.4 | 85.8 | 19.2 | 21.6 | 0.799 | 4.641  | 0.408 | 0.832   | 0.766   | 0.768   |
| Genetic Programming        | 0.615             | 0.658    | 0.486    | 0.432                | 0.797       | 0.574           | 28.1 | 83.7 | 21.3 | 36.9 | 0.695 | 2.211  | 0.709 | 0.695   | 0.58    | 0.579   |
| Gradient Boosting          | 0.798             | 0.821    | 0.75     | 0.702                | 0.895       | 0.807           | 45.6 | 94.0 | 11.0 | 19.4 | 0.829 | 7.435  | 0.335 | 0.873   | 0.842   | 0.844   |
| K-Nearest Neighbors        | 0.792             | 0.829    | 0.74     | 0.634                | 0.95        | 0.893           | 41.2 | 99.8 | 5.2  | 23.8 | 0.808 | 23.522 | 0.385 | 0.875   | 0.878   | 0.851   |
| Light Gradient Boosting    | 0.788             | 0.813    | 0.738    | 0.685                | 0.892       | 0.804           | 44.5 | 93.7 | 11.3 | 20.5 | 0.82  | 8.249  | 0.354 | 0.868   | 0.83    | 0.832   |
| Logistic Regression        | 0.704             | 0.715    | 0.637    | 0.654                | 0.753       | 0.623           | 42.5 | 79.1 | 25.9 | 22.5 | 0.779 | 2.744  | 0.46  | 0.778   | 0.69    | 0.694   |
| Naive Bayes                | 0.604             | 0.669    | 0.417    | 0.331                | 0.878       | 0.66            | 21.5 | 92.2 | 12.8 | 43.5 | 0.682 | 3.585  | 0.756 | 0.717   | 0.609   | 0.602   |
| Random Forest              | 0.706             | 0.716    | 0.64     | 0.66                 | 0.751       | 0.622           | 42.9 | 78.9 | 26.1 | 22.1 | 0.781 | 2.702  | 0.454 | 0.795   | 0.697   | 0.702   |
| Support Vector Machine     | 0.744             | 0.742    | 0.692    | 0.754                | 0.734       | 0.645           | 49.0 | 77.1 | 27.9 | 16.0 | 0.829 | 3.095  | 0.335 | 0.838   | 0.794   | 0.796   |

# Median Model Prediction Statistics (Rounded to 3 Decimal Points)

## D1 = hcc\_data\_custom\_rep

| ML Algorithm               | Balanced Accuracy | Accuracy | F1 Score | Sensitivity (Recall) | Specificity | Precision (PPV) | TP   | TN    | FP   | FN   | NPV   | LR+    | LR-   | ROC AUC | PRC AUC | PRC APS |
|----------------------------|-------------------|----------|----------|----------------------|-------------|-----------------|------|-------|------|------|-------|--------|-------|---------|---------|---------|
| Artificial Neural Network  | 0.79              | 0.812    | 0.739    | 0.685                | 0.881       | 0.784           | 44.5 | 92.5  | 12.5 | 20.5 | 0.821 | 5.99   | 0.353 | 0.841   | 0.793   | 0.795   |
| Category Gradient Boosting | 0.798             | 0.826    | 0.748    | 0.646                | 0.933       | 0.861           | 42.0 | 98.0  | 7.0  | 23.0 | 0.812 | 10.038 | 0.373 | 0.908   | 0.886   | 0.886   |
| Decision Tree              | 0.632             | 0.668    | 0.554    | 0.6                  | 0.724       | 0.571           | 39.0 | 76.0  | 29.0 | 26.0 | 0.724 | 2.15   | 0.615 | 0.684   | 0.63    | 0.54    |
| Elastic Net                | 0.734             | 0.756    | 0.674    | 0.692                | 0.833       | 0.725           | 45.0 | 87.5  | 17.5 | 20.0 | 0.803 | 4.267  | 0.397 | 0.809   | 0.738   | 0.74    |
| ExSTraCS                   | 0.751             | 0.765    | 0.69     | 0.692                | 0.81        | 0.695           | 45.0 | 85.0  | 20.0 | 20.0 | 0.809 | 3.682  | 0.381 | 0.831   | 0.795   | 0.796   |
| Extreme Gradient Boosting  | 0.738             | 0.753    | 0.677    | 0.669                | 0.79        | 0.665           | 43.5 | 83.0  | 22.0 | 21.5 | 0.8   | 3.221  | 0.404 | 0.815   | 0.748   | 0.751   |
| Genetic Programming        | 0.609             | 0.656    | 0.478    | 0.423                | 0.79        | 0.563           | 27.5 | 83.0  | 22.0 | 37.5 | 0.688 | 2.084  | 0.731 | 0.691   | 0.567   | 0.575   |
| Gradient Boosting          | 0.807             | 0.829    | 0.762    | 0.723                | 0.9         | 0.816           | 47.0 | 94.5  | 10.5 | 18.0 | 0.838 | 7.174  | 0.313 | 0.876   | 0.86    | 0.861   |
| K-Nearest Neighbors        | 0.796             | 0.835    | 0.744    | 0.631                | 0.957       | 0.903           | 41.0 | 100.5 | 4.5  | 24.0 | 0.806 | 15.225 | 0.39  | 0.884   | 0.885   | 0.87    |
| Light Gradient Boosting    | 0.79              | 0.815    | 0.739    | 0.685                | 0.9         | 0.807           | 44.5 | 94.5  | 10.5 | 20.5 | 0.82  | 6.777  | 0.354 | 0.887   | 0.864   | 0.866   |
| Logistic Regression        | 0.695             | 0.706    | 0.633    | 0.677                | 0.781       | 0.616           | 44.0 | 82.0  | 23.0 | 21.0 | 0.783 | 2.608  | 0.447 | 0.769   | 0.685   | 0.689   |
| Naive Bayes                | 0.607             | 0.668    | 0.463    | 0.377                | 0.848       | 0.624           | 24.5 | 89.0  | 16.0 | 40.5 | 0.685 | 2.678  | 0.743 | 0.718   | 0.609   | 0.602   |
| Random Forest              | 0.705             | 0.718    | 0.639    | 0.654                | 0.748       | 0.624           | 42.5 | 78.5  | 26.5 | 22.5 | 0.779 | 2.681  | 0.457 | 0.802   | 0.715   | 0.72    |
| Support Vector Machine     | 0.744             | 0.735    | 0.694    | 0.769                | 0.738       | 0.633           | 50.0 | 77.5  | 27.5 | 15.0 | 0.83  | 2.789  | 0.33  | 0.84    | 0.801   | 0.802   |
