# Supplementary material for: STREAMLINE: An Automated Machine Learning Pipeline for Biomedicine Applied to Examine the Utility of Photography-Based Phenotypes for OSA Prediction Across International Sleep Centers
Source: arXiv:2312.05461 ancillary file (2023-12-09)
Supplement: Supplementary file 4 [file hcc_exp_STREAMLINE_Report.pdf]

# STREAMLINE Testing Data Evaluation Report: 2023-09-26 12:57:00.921630

## General Pipeline Settings:

CV Partitions: 10  
Partition Method: Stratified  
Categorical Cutoff: 10  
Statistical Significance Cutoff: 0.05  
Random Seed: 42  
Run From Notebook: False

## Feature Importance/Selection Settings:

Use Mutual Information: True  
Use MultiSURF: True  
Use TURF: False  
TURF Cutoff: 0.5  
MultiSURF Instance Subset: 2000  
Max Features to Keep: 2000  
Filter Poor Features: True  
Top Features to Display: 40  
Export Feature Importance Plot: True

## ML Modeling Algorithms:

Artificial Neural Network: True  
Category Gradient Boosting: True  
Decision Tree: True  
Elastic Net: True  
ExSTraCS: True  
Extreme Gradient Boosting: True  
Genetic Programming: True  
Gradient Boosting: True  
K-Nearest Neighbors: True  
Light Gradient Boosting: True  
Logistic Regression: True  
Naive Bayes: True  
Random Forest: True  
Support Vector Machine: True  
XCS: False  
eLCS: False

## Modeling Settings:

Primary Metric: balanced\_accuracy  
Training Subsample for KNN,ANN,SVM,and XGB: 0  
Uniform Feature Importance Estimation (Models): True  
Hyperparameter Sweep Number of Trials: 200  
Hyperparameter Timeout: 900  
Export Hyperparameter Sweep Plots: False

## LCS Settings (eLCS,XCS,ExSTraCS):

Do LCS Hyperparameter Sweep: False  
nu: 1  
Training Iterations: 200000  
N (Rule Population Size): 2000  
LCS Hyperparameter Sweep Timeout: 1200

## Stats and Figure Settings:

Export ROC Plot: True  
Export PRC Plot: True  
Export Metric Boxplots: True  
Export Feature Importance Boxplots: True  
Metric Weighting Composite FI Plots: balanced\_accuracy  
Top Model Features To Display: 40  
Export Feature Correlations: True

## EDA and Processing Settings:

Engineering Missingness Cutoff: 0.5  
Cleaning Missingness Cutoff: 0.5  
Correlation Removal Threshold: 1.0  
List of Exploratory Analysis Ran: ['Describe', 'Univariate Analysis', 'Feature Correlation']  
List of Exploratory Plots Saved: ['Describe', 'Univariate Analysis', 'Feature Correlation']  
Use Data Scaling: True  
Use Data Imputation: True  
Use Multivariate Imputation: True  
Overwrite CV Datasets: True

## Target Dataset(s):

D1 = hcc\_data  
D2 = hcc\_data\_custom

## Target Data Settings:

Data Path: ./data/DemoData  
Output Path: /home/ryanurb/idata/output  
Experiment Name: hcc\_exp  
Class Label: Class  
Instance Label: InstanceID  
Match Label: None  
Ignored Features: None  
Specified Categorical Features: ./data/DemoFeatureTypes/hcc\_cat\_feat.csv  
Specified Quantitative Features: ./data/DemoFeatureTypes/hcc\_quant\_feat.csv

## Univariate Analysis of Each Dataset (Top 10 Features for Each)

### D1 = hcc\_data

| Feature                      | p-value                | Test-statistic     | Test-name           |
|------------------------------|------------------------|--------------------|---------------------|
| Alkaline phosphatase (U/L)   | 8.425494437393163e-07  | 1684.5             | Mann-Whitney U Test |
| Performance Status*          | 1.8787043290235831e-06 | 1886.0             | Mann-Whitney U Test |
| Alpha-Fetoprotein (ng/mL)    | 3.763225766746508e-06  | 1629.5             | Mann-Whitney U Test |
| Haemoglobin (g/dL)           | 6.806983230077955e-05  | 4278.0             | Mann-Whitney U Test |
| Albumin (mg/dL)              | 0.000209728656698      | 4056.0             | Mann-Whitney U Test |
| Symptoms                     | 0.0006092985105592     | 11.747352356529046 | Chi Square Test     |
| Ascites degree*              | 0.0010580963945994     | 2352.0             | Mann-Whitney U Test |
| Direct Bilirubin (mg/dL)     | 0.0013544764761447     | 1148.5             | Mann-Whitney U Test |
| Aspartate transaminase (U/L) | 0.0016188344745582     | 2200.5             | Mann-Whitney U Test |
| Ferritin (ng/mL)             | 0.0019988859548087     | 548.5              | Mann-Whitney U Test |

### D2 = hcc\_data\_custom

| Feature                      | p-value                | Test-statistic     | Test-name           |
|------------------------------|------------------------|--------------------|---------------------|
| Alkaline phosphatase (U/L)   | 8.425494437393163e-07  | 1684.5             | Mann-Whitney U Test |
| Performance Status*          | 1.8787043290235831e-06 | 1886.0             | Mann-Whitney U Test |
| Alpha-Fetoprotein (ng/mL)    | 3.763225766746508e-06  | 1629.5             | Mann-Whitney U Test |
| Haemoglobin (g/dL)           | 6.806983230077955e-05  | 4278.0             | Mann-Whitney U Test |
| Albumin (mg/dL)              | 0.000209728656698      | 4056.0             | Mann-Whitney U Test |
| Symptoms                     | 0.0006092985105592     | 11.747352356529046 | Chi Square Test     |
| Ascites degree*              | 0.0010580963945994     | 2352.0             | Mann-Whitney U Test |
| Direct Bilirubin (mg/dL)     | 0.0013544764761447     | 1148.5             | Mann-Whitney U Test |
| Aspartate transaminase (U/L) | 0.0016188344745582     | 2200.5             | Mann-Whitney U Test |
| Ferritin (ng/mL)             | 0.0019988859548087     | 548.5              | Mann-Whitney U Test |

# Dataset and Model Prediction Summary: D1 = hcc\_data

## Data Processing/Counts Summary

|           | Instances | Total Features | Categorical Features | Quantitative Features | Missing Values | Missing Percent | Class 0 | Class 1 |
|-----------|-----------|----------------|----------------------|-----------------------|----------------|-----------------|---------|---------|
| Original  | 165       | 49             | 23                   | 26                    | 826            | 0.1022          | 102     | 63      |
| C1        | 165       | 49             | 23                   | 26                    | 826            | 0.1022          | 102     | 63      |
| E1        | 165       | 49             | 23                   | 26                    | 826            | 0.1022          | 102     | 63      |
| C2        | 165       | 49             | 23                   | 26                    | 826            | 0.1022          | 102     | 63      |
| C3        | 165       | 49             | 23                   | 26                    | 826            | 0.1022          | 102     | 63      |
| E2        | 165       | 49             | 23                   | 26                    | 826            | 0.1022          | 102     | 63      |
| C4        | 165       | 49             | 23                   | 26                    | 826            | 0.1022          | 102     | 63      |
| Processed | 165       | 49             | 23                   | 26                    | 826            | 0.1022          | 102     | 63      |

## Cleaning (C) and Engineering (E) Elements

- \* C1 - Remove instances with no outcome and features to ignore
- \* E1 - Add missingness features
- \* C2 - Remove features with invariance or high missingness
- \* C3 - Remove instances with high missingness
- \* E2 - Add one-hot-encoding of categorical features
- \* C4 - Remove highly correlated features

## Class Balance (Processed)

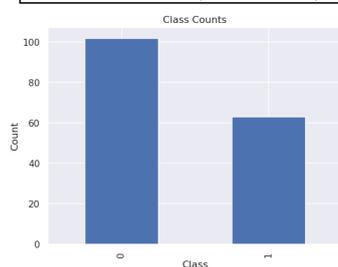

## Feature Correlations (Pearson)

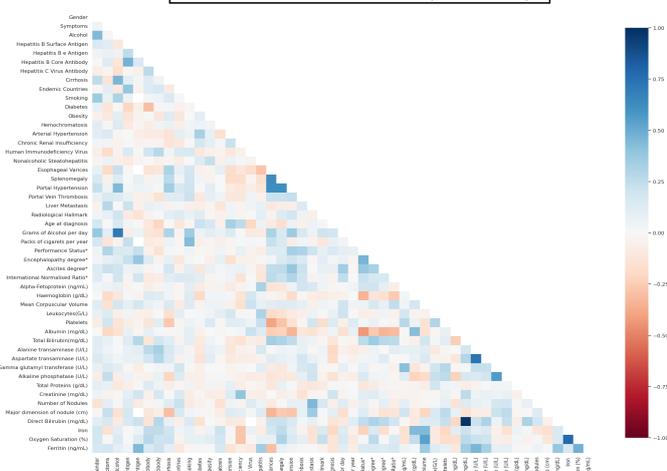

## Top ML Algorithm Results (Averaged Over CV Runs):

|                                                   |
|---------------------------------------------------|
| Best (ROC_AUC): Extreme Gradient Boosting = 0.800 |
| Best (Balanced Acc.): Elastic Net = 0.728         |
| Best (F1 Score): Elastic Net = 0.667              |
| Best (PRC AUC): Support Vector Machine = 0.718    |
| Best (PRC APS): Support Vector Machine = 0.743    |

## ROC

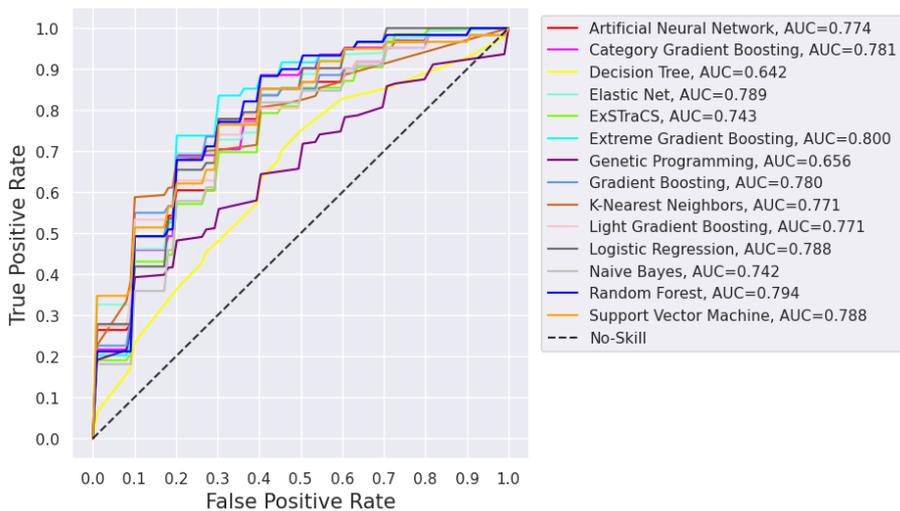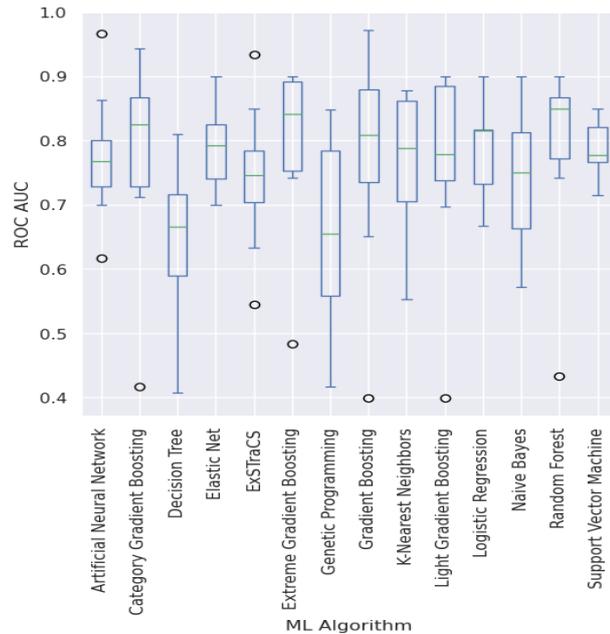

## PRC

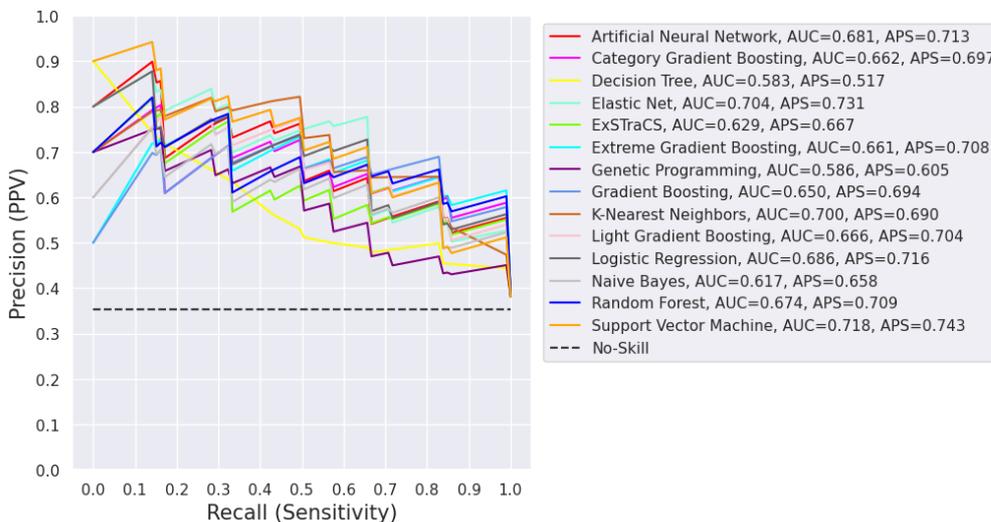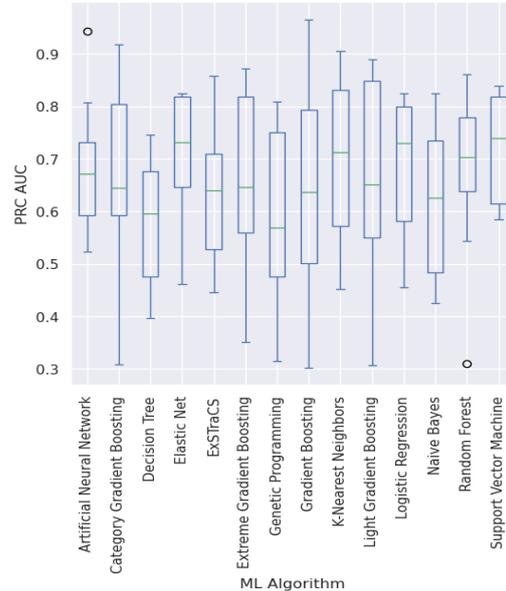

# Dataset and Model Prediction Summary: D2 = hcc\_data\_custom

## Data Processing/Counts Summary

|           | Instances | Total Features | Categorical Features | Quantitative Features | Missing Values | Missing Percent | Class 0 | Class 1 |
|-----------|-----------|----------------|----------------------|-----------------------|----------------|-----------------|---------|---------|
| Original  | 169       | 64             | 31                   | 33                    | 1323           | 0.1223          | 104     | 63      |
| C1        | 167       | 64             | 31                   | 33                    | 1308           | 0.1224          | 104     | 63      |
| E1        | 167       | 67             | 34                   | 33                    | 1308           | 0.1169          | 104     | 63      |
| C2        | 167       | 61             | 30                   | 31                    | 899            | 0.0882          | 104     | 63      |
| C3        | 165       | 61             | 30                   | 31                    | 826            | 0.0821          | 102     | 63      |
| E2        | 165       | 71             | 40                   | 31                    | 826            | 0.0705          | 102     | 63      |
| C4        | 165       | 69             | 40                   | 29                    | 826            | 0.0726          | 102     | 63      |
| Processed | 165       | 69             | 40                   | 29                    | 826            | 0.0726          | 102     | 63      |

## Cleaning (C) and Engineering (E) Elements

- \* C1 - Remove instances with no outcome and features to ignore
- \* E1 - Add missingness features
- \* C2 - Remove features with invariance or high missingness
- \* C3 - Remove instances with high missingness
- \* E2 - Add one-hot-encoding of categorical features
- \* C4 - Remove highly correlated features

## Class Balance (Processed)

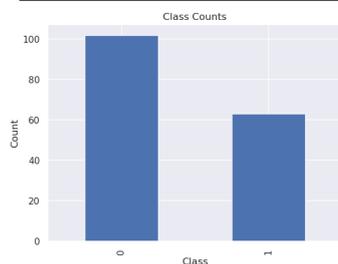

## Feature Correlations (Pearson)

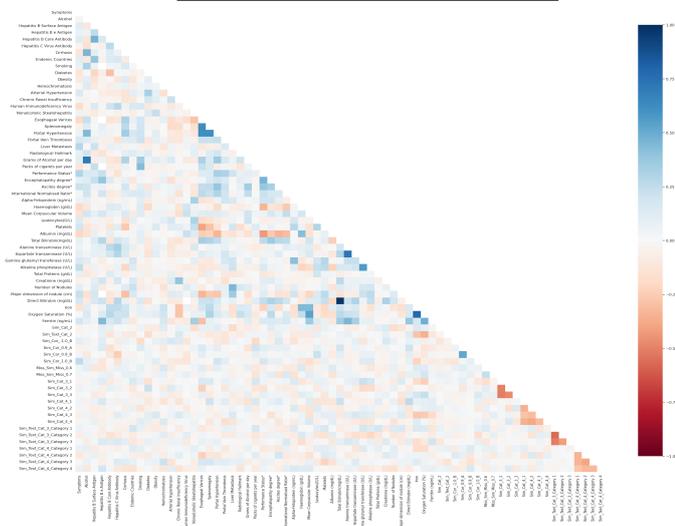

## Top ML Algorithm Results (Averaged Over CV Runs):

|                                                   |
|---------------------------------------------------|
| Best (ROC_AUC): Extreme Gradient Boosting = 0.794 |
| Best (Balanced Acc.): Random Forest = 0.697       |
| Best (F1 Score): Random Forest = 0.627            |
| Best (PRC AUC): Support Vector Machine = 0.696    |
| Best (PRC APS): Random Forest = 0.727             |

## ROC

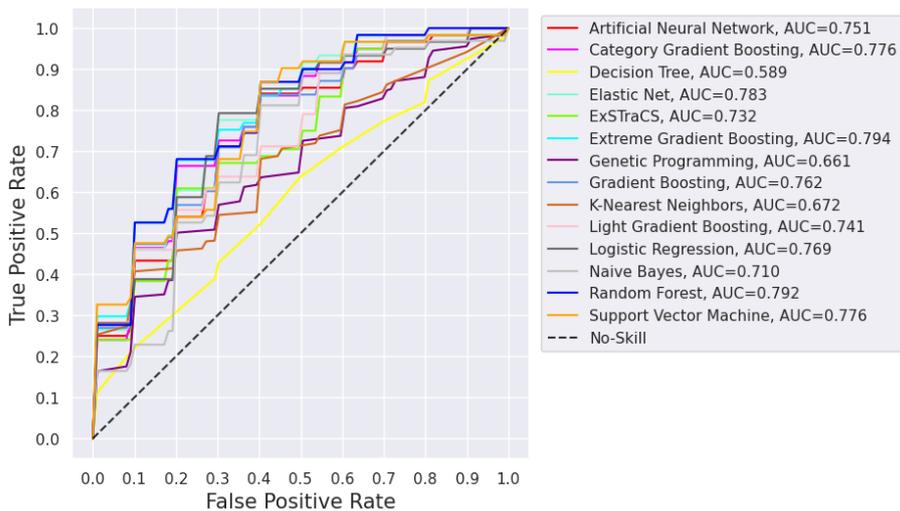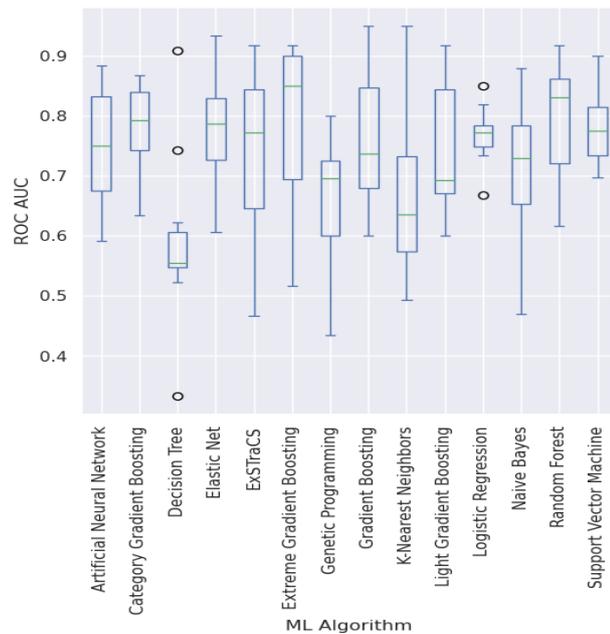

## PRC

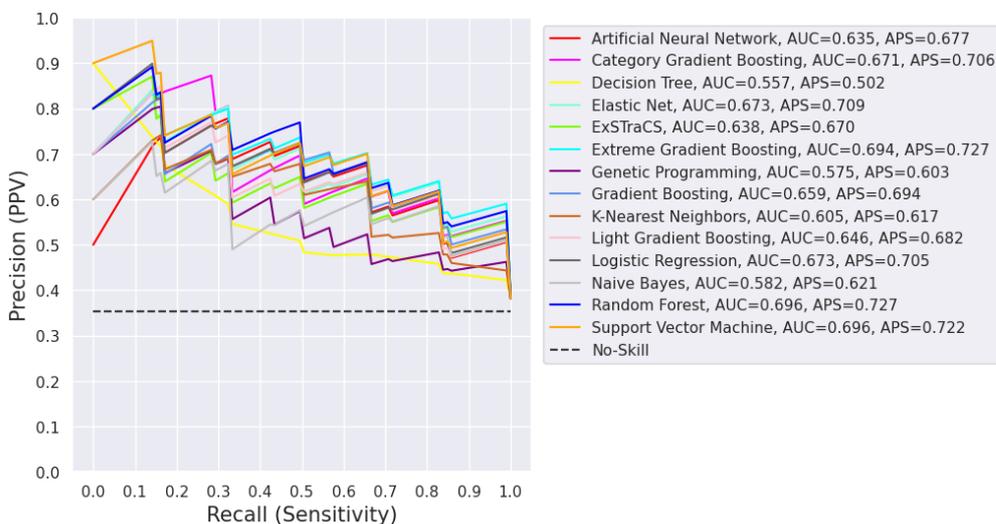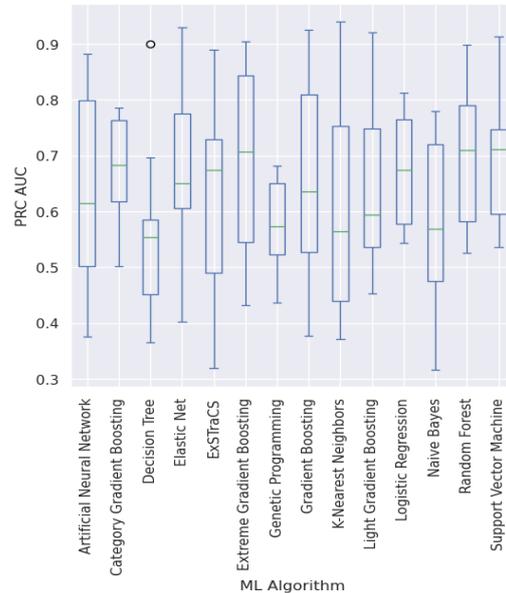

# Average Model Prediction Statistics (Rounded to 3 Decimal Points)

## D1 = hcc\_data

| ML Algorithm               | Balanced Accuracy | Accuracy | F1 Score | Sensitivity (Recall) | Specificity | Precision (PPV) | TP  | TN  | FP  | FN  | NPV   | LR+   | LR-   | ROC AUC | PRC AUC | PRC APS |
|----------------------------|-------------------|----------|----------|----------------------|-------------|-----------------|-----|-----|-----|-----|-------|-------|-------|---------|---------|---------|
| Artificial Neural Network  | 0.689             | 0.708    | 0.618    | 0.614                | 0.763       | 0.644           | 3.9 | 7.8 | 2.4 | 2.4 | 0.766 | 2.603 | 0.51  | 0.774   | 0.681   | 0.713   |
| Category Gradient Boosting | 0.684             | 0.715    | 0.569    | 0.555                | 0.814       | 0.64            | 3.5 | 8.3 | 1.9 | 2.8 | 0.764 | 2.955 | 0.551 | 0.781   | 0.662   | 0.697   |
| Decision Tree              | 0.627             | 0.619    | 0.562    | 0.667                | 0.588       | 0.506           | 4.2 | 6.0 | 4.2 | 2.1 | 0.775 | 1.831 | 0.542 | 0.642   | 0.583   | 0.517   |
| Elastic Net                | 0.728             | 0.74     | 0.667    | 0.69                 | 0.765       | 0.669           | 4.4 | 7.8 | 2.4 | 1.9 | 0.814 | 2.758 | 0.397 | 0.789   | 0.704   | 0.731   |
| ExSTraCS                   | 0.653             | 0.679    | 0.559    | 0.55                 | 0.756       | 0.6             | 3.5 | 7.7 | 2.5 | 2.8 | 0.738 | 2.876 | 0.627 | 0.743   | 0.629   | 0.667   |
| Extreme Gradient Boosting  | 0.718             | 0.733    | 0.637    | 0.662                | 0.775       | 0.631           | 4.2 | 7.9 | 2.3 | 2.1 | 0.805 | 3.5   | 0.441 | 0.8     | 0.661   | 0.708   |
| Genetic Programming        | 0.612             | 0.647    | 0.48     | 0.46                 | 0.764       | 0.541           | 2.9 | 7.8 | 2.4 | 3.4 | 0.703 | 2.481 | 0.711 | 0.656   | 0.586   | 0.605   |
| Gradient Boosting          | 0.704             | 0.733    | 0.595    | 0.583                | 0.825       | 0.65            | 3.7 | 8.4 | 1.8 | 2.6 | 0.779 | 3.539 | 0.502 | 0.78    | 0.65    | 0.694   |
| K-Nearest Neighbors        | 0.695             | 0.741    | 0.581    | 0.498                | 0.892       | 0.735           | 3.1 | 9.1 | 1.1 | 3.2 | 0.747 | 2.957 | 0.571 | 0.771   | 0.7     | 0.69    |
| Light Gradient Boosting    | 0.672             | 0.696    | 0.583    | 0.581                | 0.764       | 0.642           | 3.7 | 7.8 | 2.4 | 2.6 | 0.762 | 2.717 | 0.543 | 0.771   | 0.666   | 0.704   |
| Logistic Regression        | 0.714             | 0.715    | 0.655    | 0.724                | 0.705       | 0.61            | 4.6 | 7.2 | 3.0 | 1.7 | 0.818 | 2.637 | 0.382 | 0.788   | 0.686   | 0.716   |
| Naive Bayes                | 0.549             | 0.637    | 0.247    | 0.188                | 0.91        | 0.44            | 1.2 | 9.3 | 0.9 | 5.1 | 0.649 | 1.0   | 0.891 | 0.742   | 0.617   | 0.658   |
| Random Forest              | 0.657             | 0.667    | 0.579    | 0.617                | 0.698       | 0.567           | 3.9 | 7.1 | 3.1 | 2.4 | 0.756 | 2.823 | 0.585 | 0.794   | 0.674   | 0.709   |
| Support Vector Machine     | 0.707             | 0.71     | 0.653    | 0.71                 | 0.705       | 0.631           | 4.5 | 7.2 | 3.0 | 1.8 | 0.805 | 2.373 | 0.408 | 0.788   | 0.718   | 0.743   |

## D2 = hcc\_data\_custom

| ML Algorithm               | Balanced Accuracy | Accuracy | F1 Score | Sensitivity (Recall) | Specificity | Precision (PPV) | TP  | TN  | FP  | FN  | NPV   | LR+   | LR-   | ROC AUC | PRC AUC | PRC APS |
|----------------------------|-------------------|----------|----------|----------------------|-------------|-----------------|-----|-----|-----|-----|-------|-------|-------|---------|---------|---------|
| Artificial Neural Network  | 0.664             | 0.697    | 0.556    | 0.533                | 0.795       | 0.631           | 3.4 | 8.1 | 2.1 | 2.9 | 0.746 | 2.278 | 0.578 | 0.751   | 0.635   | 0.677   |
| Category Gradient Boosting | 0.674             | 0.715    | 0.562    | 0.495                | 0.853       | 0.694           | 3.1 | 8.7 | 1.5 | 3.2 | 0.735 | 3.428 | 0.593 | 0.776   | 0.671   | 0.706   |
| Decision Tree              | 0.562             | 0.581    | 0.464    | 0.488                | 0.636       | 0.479           | 3.1 | 6.5 | 3.7 | 3.2 | 0.683 | 1.241 | 0.844 | 0.589   | 0.557   | 0.502   |
| Elastic Net                | 0.665             | 0.691    | 0.56     | 0.564                | 0.765       | 0.617           | 3.6 | 7.8 | 2.4 | 2.7 | 0.757 | 2.428 | 0.562 | 0.783   | 0.673   | 0.709   |
| ExSTraCS                   | 0.63              | 0.643    | 0.545    | 0.581                | 0.679       | 0.527           | 3.7 | 6.9 | 3.3 | 2.6 | 0.735 | 2.849 | 0.677 | 0.732   | 0.638   | 0.67    |
| Extreme Gradient Boosting  | 0.673             | 0.685    | 0.596    | 0.619                | 0.727       | 0.599           | 3.9 | 7.4 | 2.8 | 2.4 | 0.76  | 2.893 | 0.536 | 0.794   | 0.694   | 0.727   |
| Genetic Programming        | 0.584             | 0.623    | 0.448    | 0.414                | 0.754       | 0.52            | 2.6 | 7.7 | 2.5 | 3.7 | 0.674 | 2.098 | 0.823 | 0.661   | 0.575   | 0.603   |
| Gradient Boosting          | 0.69              | 0.716    | 0.612    | 0.583                | 0.796       | 0.649           | 3.7 | 8.1 | 2.1 | 2.6 | 0.756 | 4.215 | 0.558 | 0.762   | 0.659   | 0.694   |
| K-Nearest Neighbors        | 0.569             | 0.643    | 0.34     | 0.255                | 0.883       | 0.525           | 1.6 | 9.0 | 1.2 | 4.7 | 0.658 | 1.475 | 0.866 | 0.672   | 0.605   | 0.617   |
| Light Gradient Boosting    | 0.682             | 0.704    | 0.6      | 0.588                | 0.776       | 0.671           | 3.7 | 7.9 | 2.3 | 2.6 | 0.755 | 2.44  | 0.556 | 0.741   | 0.646   | 0.682   |
| Logistic Regression        | 0.682             | 0.692    | 0.609    | 0.66                 | 0.705       | 0.583           | 4.2 | 7.2 | 3.0 | 2.1 | 0.795 | 2.405 | 0.46  | 0.769   | 0.673   | 0.705   |
| Naive Bayes                | 0.571             | 0.632    | 0.353    | 0.321                | 0.821       | 0.413           | 2.0 | 8.4 | 1.8 | 4.3 | 0.67  | 2.014 | 0.832 | 0.71    | 0.582   | 0.621   |
| Random Forest              | 0.697             | 0.704    | 0.627    | 0.667                | 0.726       | 0.61            | 4.2 | 7.4 | 2.8 | 2.1 | 0.787 | 2.779 | 0.458 | 0.792   | 0.696   | 0.727   |
| Support Vector Machine     | 0.671             | 0.667    | 0.608    | 0.707                | 0.635       | 0.546           | 4.5 | 6.5 | 3.7 | 1.8 | 0.804 | 2.014 | 0.433 | 0.776   | 0.696   | 0.722   |

# Median Model Prediction Statistics (Rounded to 3 Decimal Points)

## D1 = hcc\_data

| ML Algorithm               | Balanced Accuracy | Accuracy | F1 Score | Sensitivity (Recall) | Specificity | Precision (PPV) | TP  | TN  | FP  | FN  | NPV   | LR+   | LR-   | ROC AUC | PRC AUC | PRC APS |
|----------------------------|-------------------|----------|----------|----------------------|-------------|-----------------|-----|-----|-----|-----|-------|-------|-------|---------|---------|---------|
| Artificial Neural Network  | 0.694             | 0.697    | 0.62     | 0.619                | 0.7         | 0.586           | 4.0 | 7.0 | 3.0 | 2.5 | 0.76  | 1.964 | 0.476 | 0.768   | 0.671   | 0.699   |
| Category Gradient Boosting | 0.71              | 0.728    | 0.641    | 0.619                | 0.8         | 0.667           | 4.0 | 8.0 | 2.0 | 2.5 | 0.764 | 3.095 | 0.476 | 0.825   | 0.645   | 0.699   |
| Decision Tree              | 0.65              | 0.625    | 0.598    | 0.667                | 0.6         | 0.5             | 4.0 | 6.0 | 4.0 | 2.0 | 0.75  | 1.667 | 0.516 | 0.666   | 0.596   | 0.508   |
| Elastic Net                | 0.731             | 0.728    | 0.686    | 0.667                | 0.8         | 0.618           | 4.0 | 8.0 | 2.0 | 2.0 | 0.8   | 2.5   | 0.394 | 0.793   | 0.731   | 0.756   |
| ExSTraCS                   | 0.652             | 0.697    | 0.558    | 0.536                | 0.75        | 0.667           | 3.5 | 7.5 | 2.5 | 3.0 | 0.721 | 2.857 | 0.625 | 0.746   | 0.64    | 0.674   |
| Extreme Gradient Boosting  | 0.716             | 0.735    | 0.641    | 0.667                | 0.764       | 0.633           | 4.0 | 8.0 | 2.5 | 2.0 | 0.789 | 2.804 | 0.467 | 0.842   | 0.647   | 0.694   |
| Genetic Programming        | 0.589             | 0.618    | 0.497    | 0.5                  | 0.764       | 0.536           | 3.0 | 8.0 | 2.5 | 3.0 | 0.667 | 1.825 | 0.754 | 0.655   | 0.569   | 0.603   |
| Gradient Boosting          | 0.74              | 0.757    | 0.665    | 0.667                | 0.85        | 0.667           | 4.0 | 8.5 | 1.5 | 2.0 | 0.809 | 2.817 | 0.414 | 0.808   | 0.637   | 0.691   |
| K-Nearest Neighbors        | 0.668             | 0.697    | 0.573    | 0.5                  | 0.9         | 0.667           | 3.0 | 9.0 | 1.0 | 3.0 | 0.727 | 2.857 | 0.59  | 0.788   | 0.714   | 0.679   |
| Light Gradient Boosting    | 0.683             | 0.706    | 0.6      | 0.5                  | 0.764       | 0.633           | 3.0 | 8.0 | 2.5 | 3.0 | 0.739 | 2.321 | 0.563 | 0.779   | 0.651   | 0.698   |
| Logistic Regression        | 0.708             | 0.728    | 0.667    | 0.667                | 0.714       | 0.612           | 4.0 | 7.5 | 3.0 | 2.0 | 0.8   | 2.625 | 0.417 | 0.815   | 0.73    | 0.756   |
| Naive Bayes                | 0.552             | 0.647    | 0.254    | 0.155                | 0.9         | 0.536           | 1.0 | 9.0 | 1.0 | 5.5 | 0.657 | 0.0   | 0.893 | 0.75    | 0.625   | 0.659   |
| Random Forest              | 0.686             | 0.697    | 0.606    | 0.667                | 0.668       | 0.6             | 4.0 | 7.0 | 3.5 | 2.0 | 0.764 | 2.262 | 0.514 | 0.85    | 0.703   | 0.734   |
| Support Vector Machine     | 0.712             | 0.706    | 0.667    | 0.69                 | 0.7         | 0.6             | 4.5 | 7.0 | 3.0 | 2.0 | 0.809 | 2.113 | 0.364 | 0.778   | 0.739   | 0.756   |

## D2 = hcc\_data\_custom

| ML Algorithm               | Balanced Accuracy | Accuracy | F1 Score | Sensitivity (Recall) | Specificity | Precision (PPV) | TP  | TN  | FP  | FN  | NPV   | LR+   | LR-   | ROC AUC | PRC AUC | PRC APS |
|----------------------------|-------------------|----------|----------|----------------------|-------------|-----------------|-----|-----|-----|-----|-------|-------|-------|---------|---------|---------|
| Artificial Neural Network  | 0.662             | 0.706    | 0.558    | 0.583                | 0.809       | 0.612           | 3.5 | 8.5 | 2.0 | 2.5 | 0.75  | 2.262 | 0.583 | 0.75    | 0.615   | 0.66    |
| Category Gradient Boosting | 0.674             | 0.706    | 0.573    | 0.5                  | 0.859       | 0.708           | 3.0 | 9.0 | 1.5 | 3.0 | 0.739 | 2.804 | 0.581 | 0.792   | 0.684   | 0.728   |
| Decision Tree              | 0.55              | 0.546    | 0.453    | 0.464                | 0.6         | 0.429           | 3.0 | 6.0 | 4.0 | 3.5 | 0.667 | 1.147 | 0.833 | 0.554   | 0.555   | 0.46    |
| Elastic Net                | 0.675             | 0.697    | 0.558    | 0.583                | 0.727       | 0.586           | 3.5 | 8.0 | 3.0 | 2.5 | 0.746 | 2.143 | 0.571 | 0.786   | 0.651   | 0.692   |
| ExSTraCS                   | 0.624             | 0.636    | 0.552    | 0.667                | 0.6         | 0.55            | 4.0 | 6.0 | 4.0 | 2.0 | 0.75  | 1.905 | 0.583 | 0.772   | 0.674   | 0.702   |
| Extreme Gradient Boosting  | 0.685             | 0.688    | 0.615    | 0.619                | 0.764       | 0.619           | 4.0 | 8.0 | 2.5 | 2.5 | 0.727 | 2.54  | 0.536 | 0.85    | 0.708   | 0.744   |
| Genetic Programming        | 0.618             | 0.638    | 0.539    | 0.464                | 0.8         | 0.55            | 3.0 | 8.0 | 2.0 | 3.5 | 0.679 | 1.964 | 0.675 | 0.695   | 0.574   | 0.626   |
| Gradient Boosting          | 0.735             | 0.757    | 0.667    | 0.667                | 0.85        | 0.733           | 4.0 | 8.5 | 1.5 | 2.0 | 0.789 | 4.524 | 0.412 | 0.736   | 0.636   | 0.672   |
| K-Nearest Neighbors        | 0.568             | 0.636    | 0.382    | 0.286                | 0.9         | 0.583           | 2.0 | 9.0 | 1.0 | 5.0 | 0.643 | 0.815 | 0.843 | 0.636   | 0.564   | 0.536   |
| Light Gradient Boosting    | 0.698             | 0.728    | 0.62     | 0.667                | 0.764       | 0.646           | 4.0 | 8.0 | 2.5 | 2.0 | 0.775 | 2.115 | 0.467 | 0.693   | 0.595   | 0.642   |
| Logistic Regression        | 0.693             | 0.697    | 0.641    | 0.667                | 0.727       | 0.612           | 4.0 | 8.0 | 3.0 | 2.0 | 0.775 | 2.639 | 0.476 | 0.771   | 0.675   | 0.703   |
| Naive Bayes                | 0.582             | 0.636    | 0.444    | 0.333                | 0.85        | 0.5             | 2.0 | 8.5 | 1.5 | 4.0 | 0.67  | 1.548 | 0.779 | 0.73    | 0.569   | 0.607   |
| Random Forest              | 0.723             | 0.706    | 0.667    | 0.667                | 0.764       | 0.633           | 4.0 | 8.0 | 2.5 | 2.0 | 0.8   | 2.738 | 0.417 | 0.831   | 0.71    | 0.731   |
| Support Vector Machine     | 0.675             | 0.667    | 0.62     | 0.69                 | 0.65        | 0.556           | 4.5 | 6.5 | 3.5 | 2.0 | 0.778 | 1.935 | 0.476 | 0.775   | 0.712   | 0.733   |

# Feature Importance Summary: D1 = hcc\_data

Sorted Median Mutual Information Scores

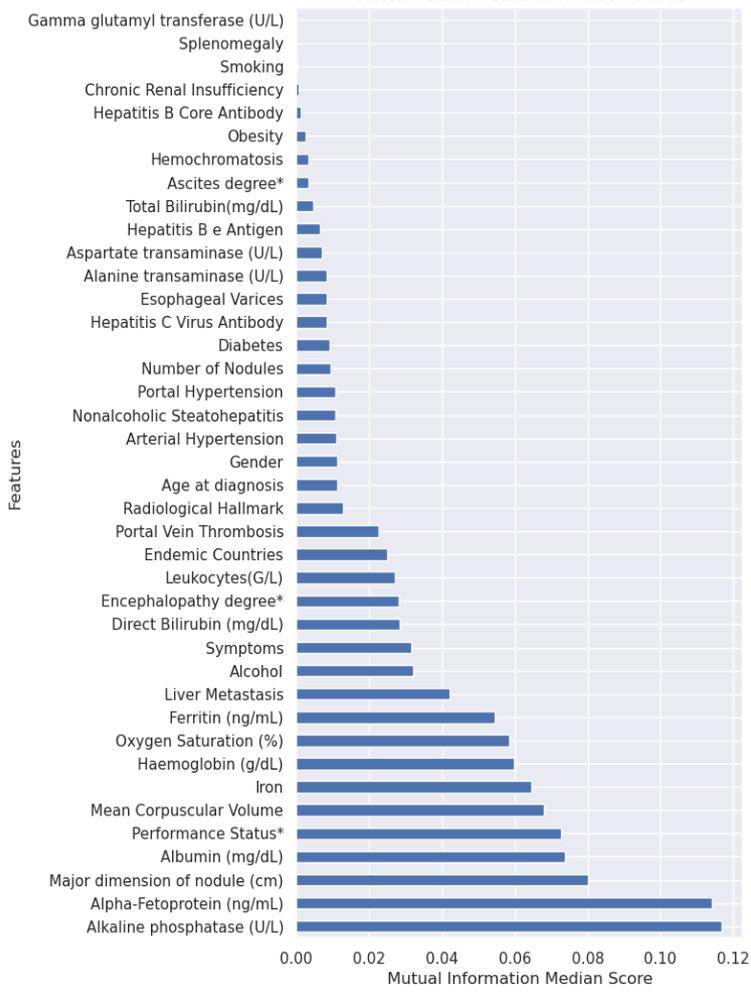

Sorted Median MultiSURF Scores

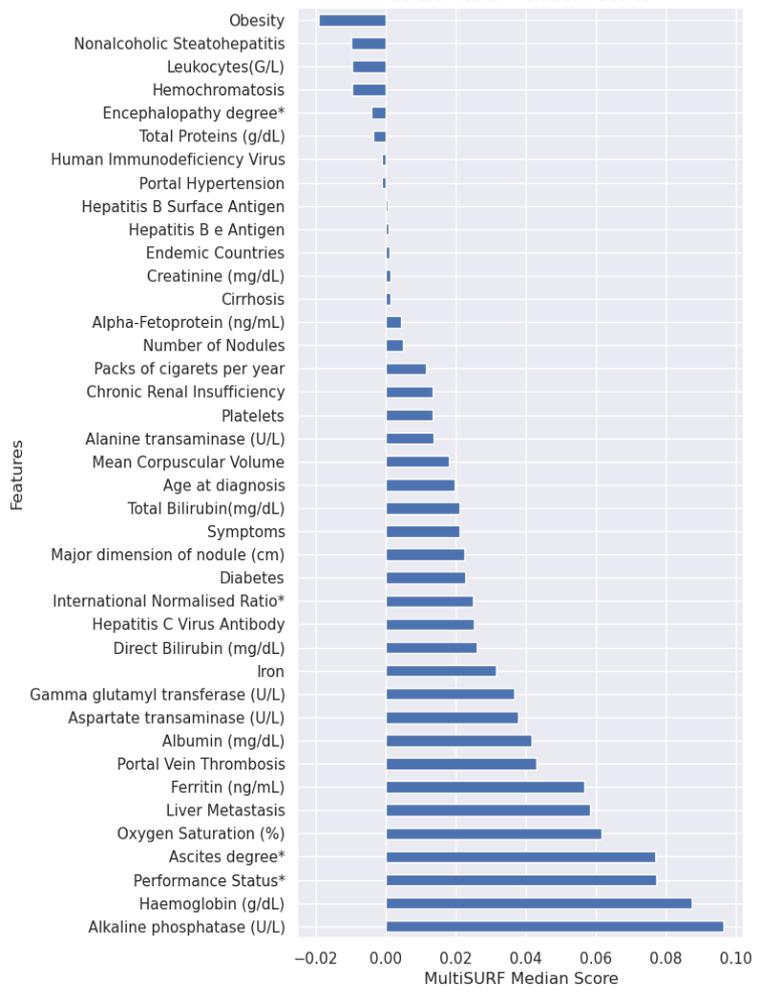

Composite Feature Importance Plot (Normalized and Performance Weighted)

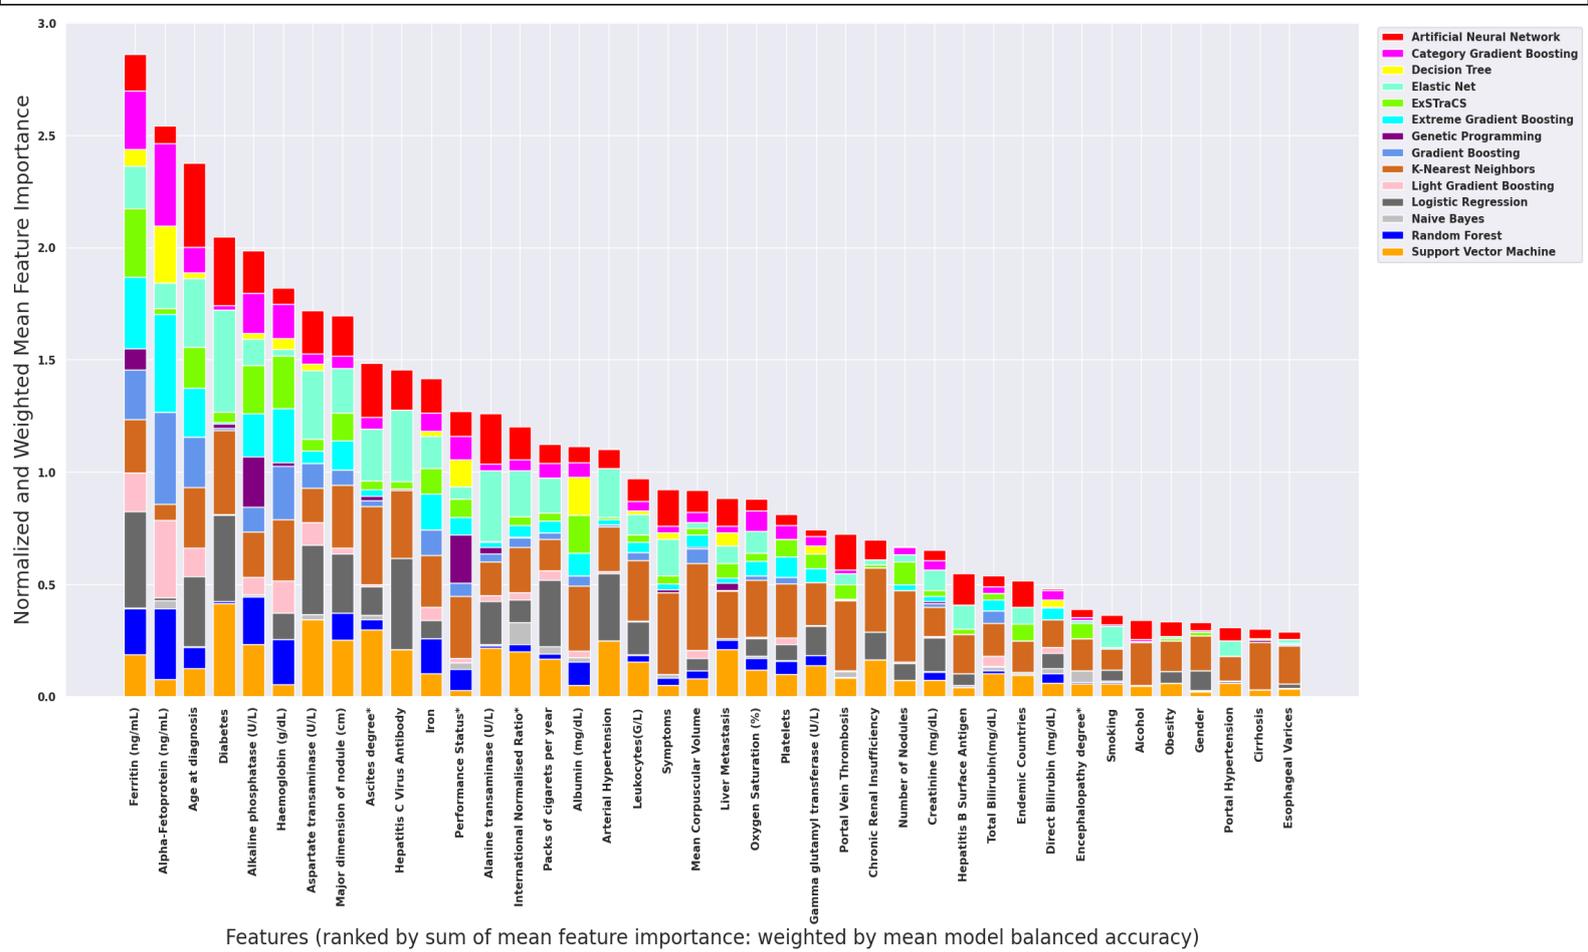

# Feature Importance Summary: D2 = hcc\_data\_custom

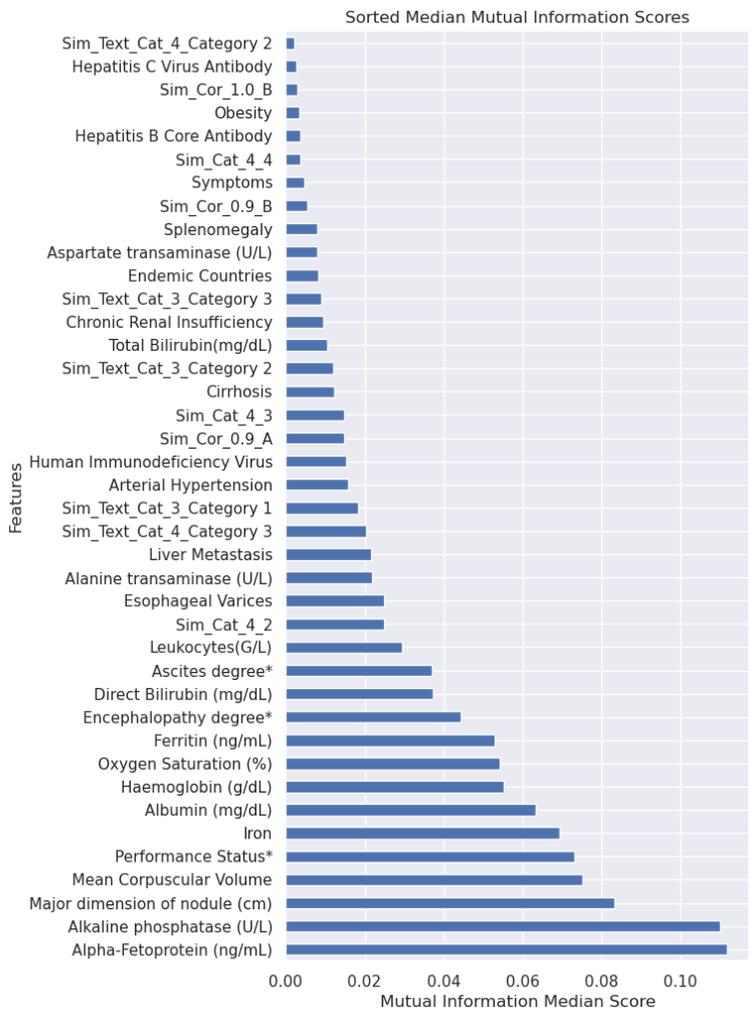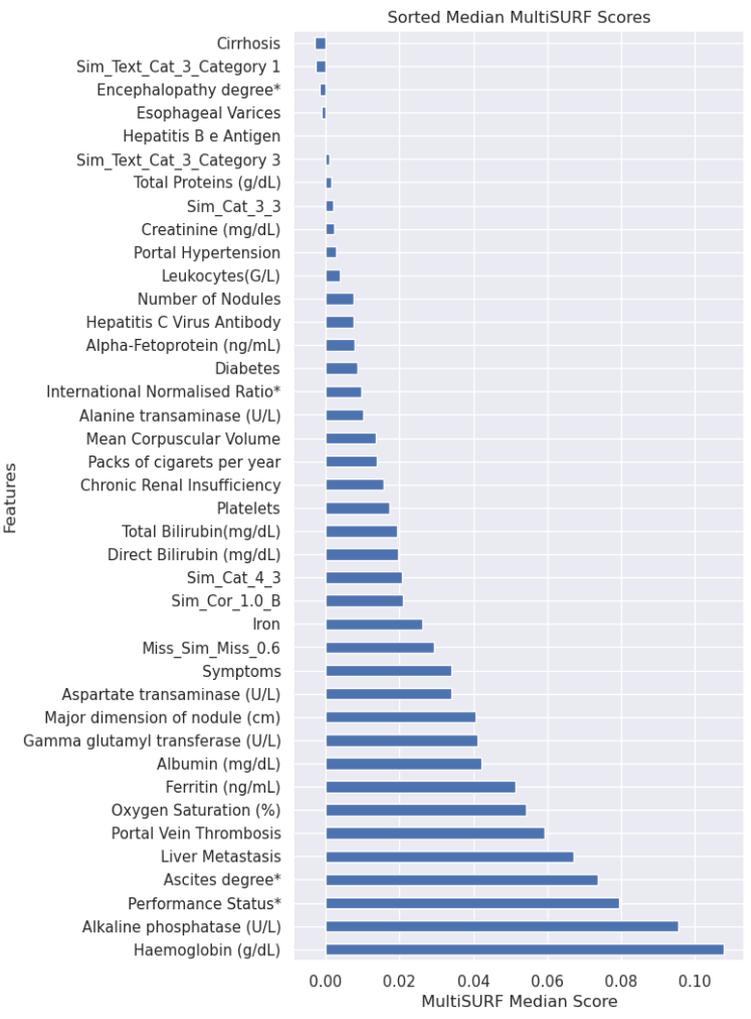

## Composite Feature Importance Plot (Normalized and Performance Weighted)

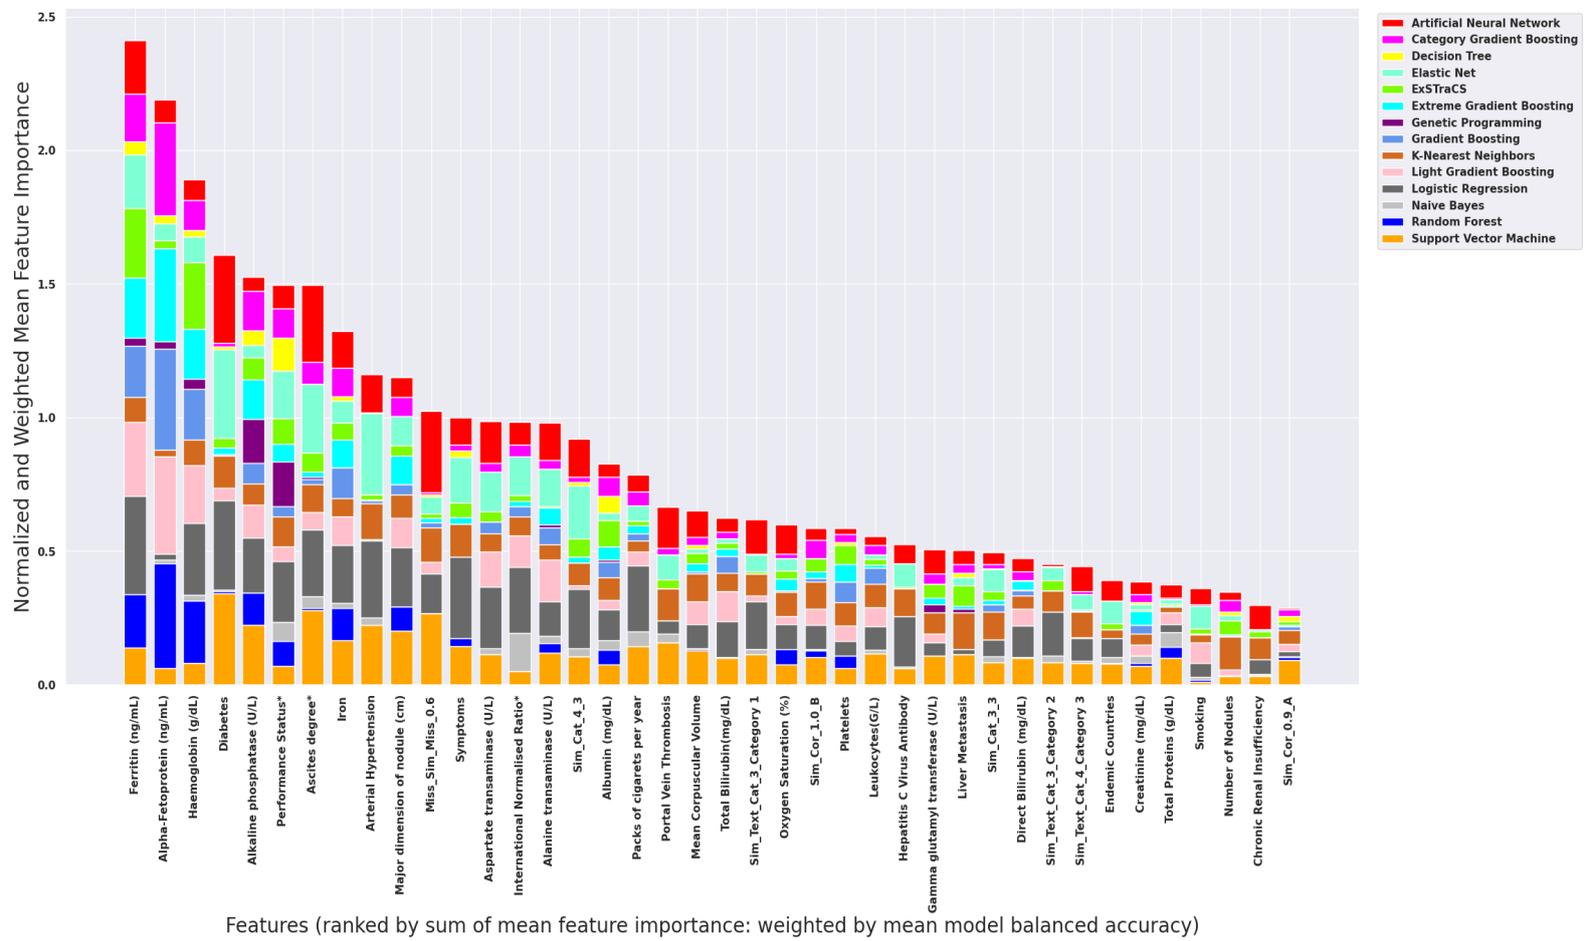

# Compare ML Performance Across Datasets

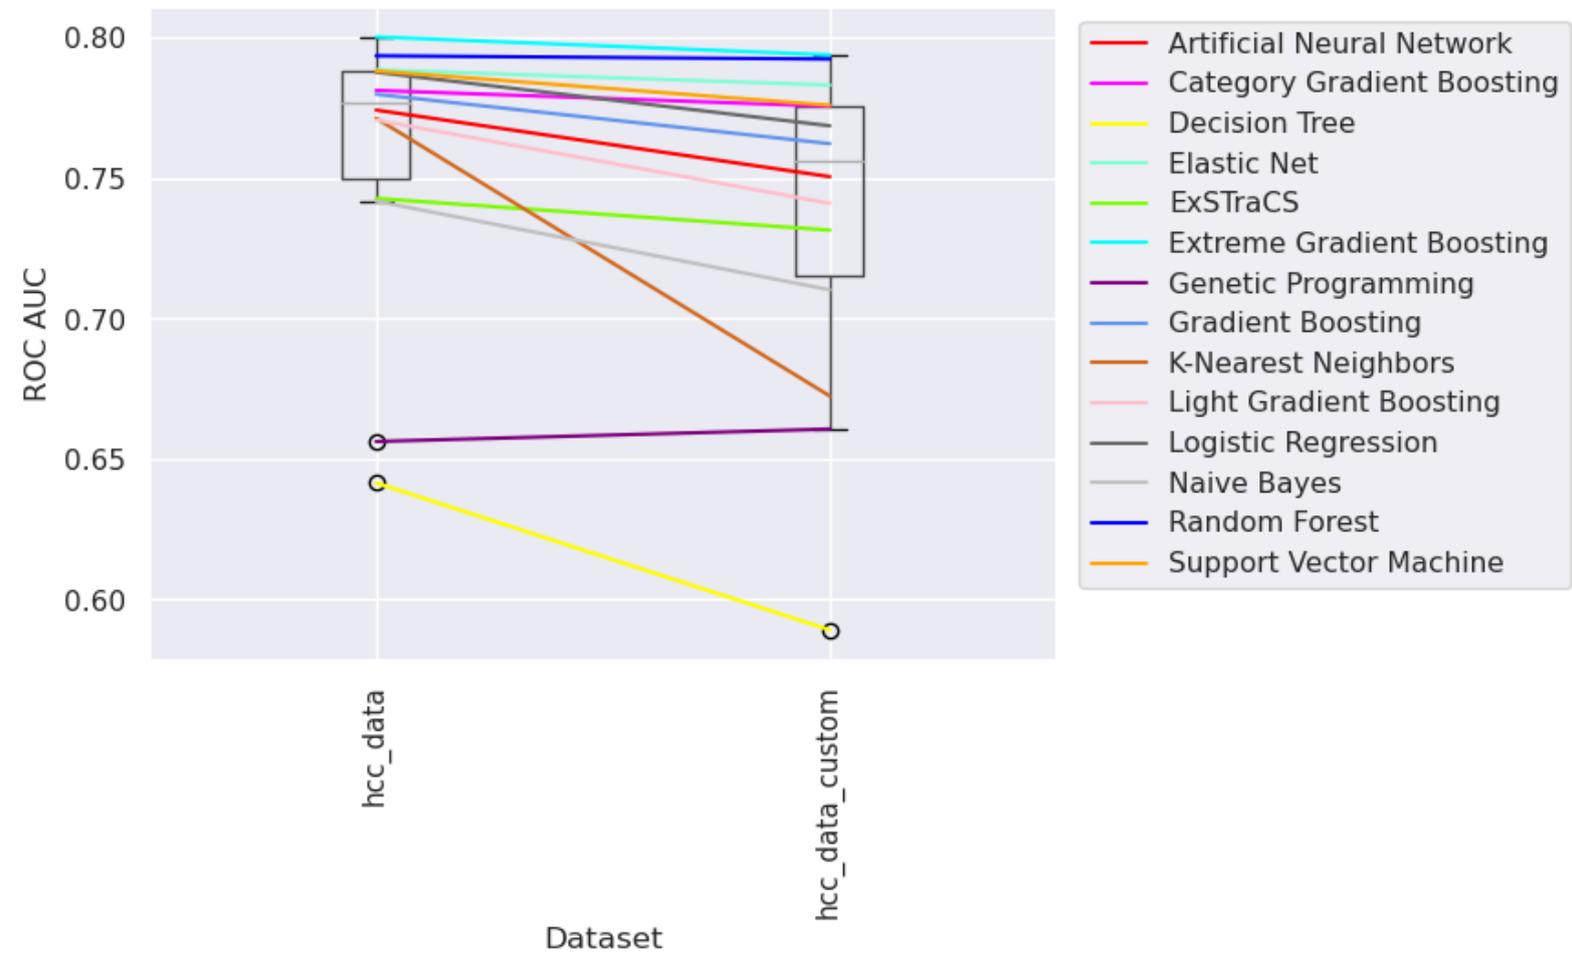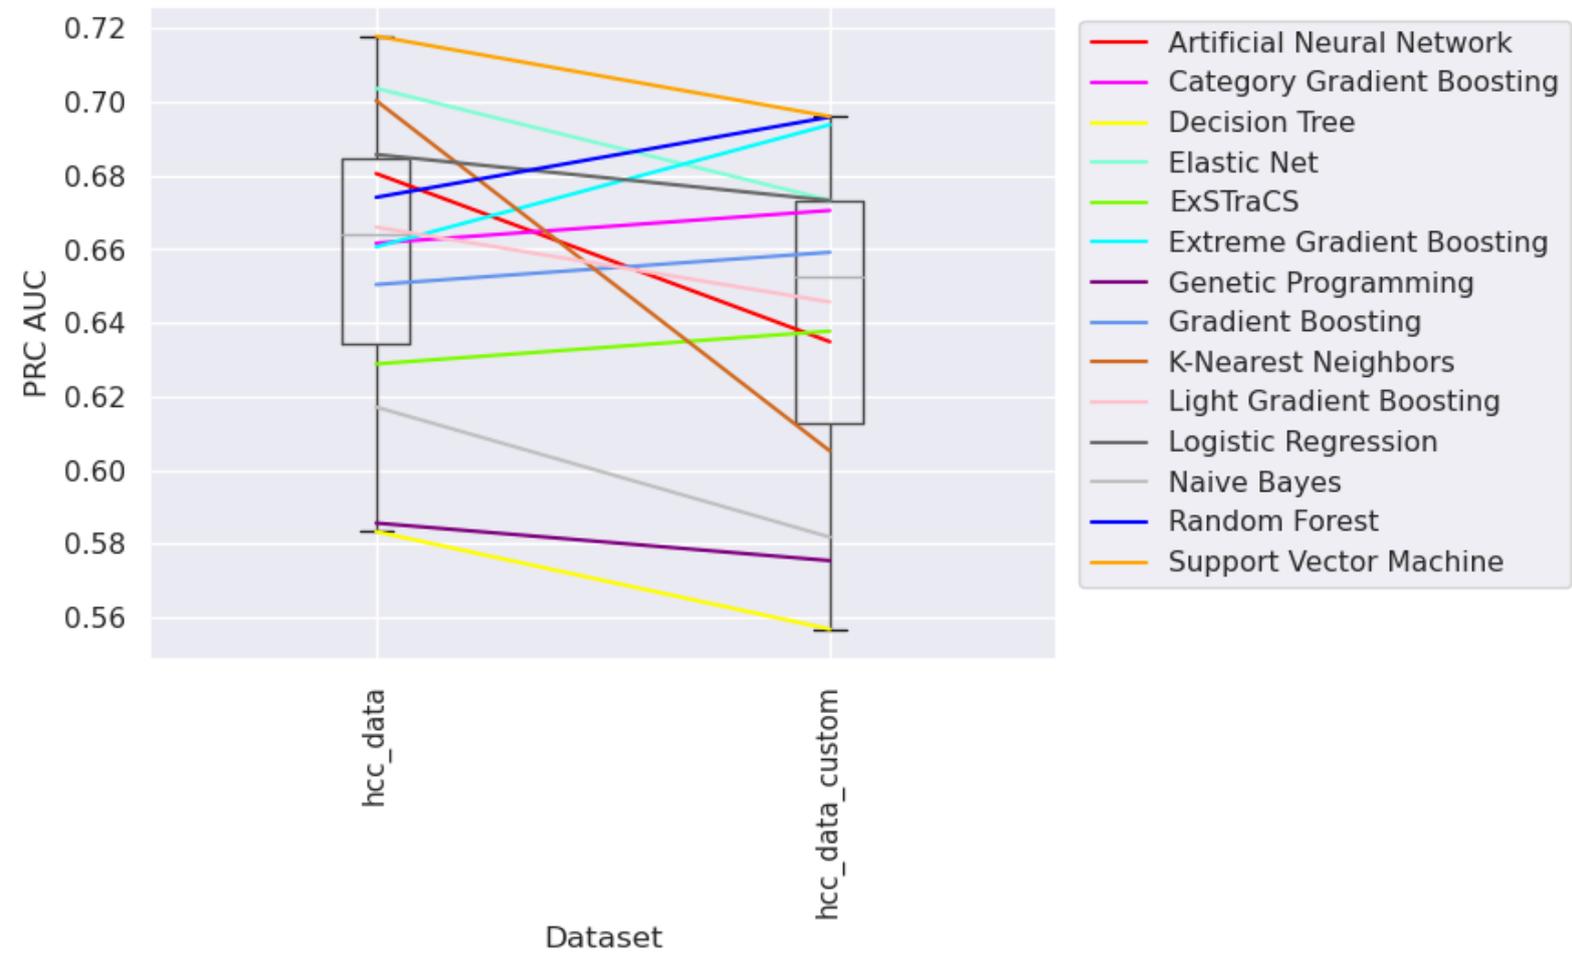

## Using Best Performing Algorithms (Kruskall Wallis Compare Datasets)

| Metrics              | P-Value | Best Alg D1                | Median D1 | Best Alg D2                | Median D2 |
|----------------------|---------|----------------------------|-----------|----------------------------|-----------|
| Balanced Accuracy    | 0.9093  | Gradient Boosting          | 0.7405    | Gradient Boosting          | 0.7345    |
| Accuracy             | 0.879   | Gradient Boosting          | 0.7574    | Gradient Boosting          | 0.7574    |
| F1 Score             | 0.6474  | Elastic Net                | 0.6863    | Gradient Boosting          | 0.6667    |
| Sensitivity (Recall) | 1.0     | Support Vector Machine     | 0.6905    | Support Vector Machine     | 0.6905    |
| Specificity          | 0.9688  | K-Nearest Neighbors        | 0.9       | K-Nearest Neighbors        | 0.9       |
| Precision (PPV)      | 0.8477  | Category Gradient Boosting | 0.6667    | Gradient Boosting          | 0.7333    |
| TP                   | 1.0     | Support Vector Machine     | 4.5       | Support Vector Machine     | 4.5       |
| TN                   | 0.4144  | K-Nearest Neighbors        | 9.0       | Category Gradient Boosting | 9.0       |
| FP                   | 0.7299  | Decision Tree              | 4.0       | Decision Tree              | 4.0       |
| FN                   | 0.457   | Naive Bayes                | 5.5       | K-Nearest Neighbors        | 5.0       |
| NPV                  | 0.8493  | Gradient Boosting          | 0.8091    | Random Forest              | 0.8       |
| LR+                  | 0.3422  | Category Gradient Boosting | 3.0952    | Gradient Boosting          | 4.5238    |
| LR-                  | 0.7906  | Naive Bayes                | 0.8929    | K-Nearest Neighbors        | 0.8433    |
| ROC AUC              | 0.7909  | Random Forest              | 0.85      | Extreme Gradient Boosting  | 0.85      |
| PRC AUC              | 0.4963  | Support Vector Machine     | 0.7394    | Support Vector Machine     | 0.7117    |
| PRC APS              | 0.7336  | Logistic Regression        | 0.7564    | Extreme Gradient Boosting  | 0.7435    |

## Pipeline Runtime Summary

| hcc_data                                |       |                    | hcc_data_custom                         |       |                    |
|-----------------------------------------|-------|--------------------|-----------------------------------------|-------|--------------------|
| Pipeline Component                      | Phase | Time (sec)         | Pipeline Component                      | Phase | Time (sec)         |
| Exploratory Analysis                    | 1     | 6.69871997833252   | Exploratory Analysis                    | 1     | 7.054031610488892  |
| Scale and Impute                        | 2     | 4.99834680557251   | Scale and Impute                        | 2     | 7.219606637954712  |
| Mutual Information (Feature Importance) | 3     | 1.0242455005645752 | Mutual Information (Feature Importance) | 3     | 1.4163403511047363 |
| MultiSURF (Feature Importance)          | 3     | 4.875789165496826  | MultiSURF (Feature Importance)          | 3     | 6.310750484466553  |
| Feature Selection                       | 4     | 2.1783766746521    | Feature Selection                       | 4     | 2.297215223312378  |
| Artificial Neural Network(Modeling)     | 5     | 720.1215507984161  | Artificial Neural Network(Modeling)     | 5     | 761.2310092449188  |
| Category Gradient Boosting(Modeling)    | 5     | 9967.622057437897  | Category Gradient Boosting(Modeling)    | 5     | 10083.57385969162  |
| Decision Tree(Modeling)                 | 5     | 26.297697067260746 | Decision Tree(Modeling)                 | 5     | 25.31545352935791  |
| Elastic Net(Modeling)                   | 5     | 28.32166838645935  | Elastic Net(Modeling)                   | 5     | 29.377707719802856 |
| ExSTraCS(Modeling)                      | 5     | 33330.48515915871  | ExSTraCS(Modeling)                      | 5     | 31350.81368899345  |
| Extreme Gradient Boosting(Modeling)     | 5     | 4925.967653751373  | Extreme Gradient Boosting(Modeling)     | 5     | 5393.255163908005  |
| Genetic Programming(Modeling)           | 5     | 10287.782114505768 | Genetic Programming(Modeling)           | 5     | 10472.36819267273  |
| Gradient Boosting(Modeling)             | 5     | 2174.4500358104706 | Gradient Boosting(Modeling)             | 5     | 1999.266121149063  |
| K-Nearest Neighbors(Modeling)           | 5     | 94.96456122398376  | K-Nearest Neighbors(Modeling)           | 5     | 173.91551637649536 |
| Light Gradient Boosting(Modeling)       | 5     | 248.33601021766663 | Light Gradient Boosting(Modeling)       | 5     | 325.8518924713135  |
| Logistic Regression(Modeling)           | 5     | 30.337548971176147 | Logistic Regression(Modeling)           | 5     | 32.568302154541016 |
| Naive Bayes(Modeling)                   | 5     | 3.310241222381592  | Naive Bayes(Modeling)                   | 5     | 3.9420104026794434 |
| Random Forest(Modeling)                 | 5     | 3903.347003221512  | Random Forest(Modeling)                 | 5     | 4630.939676761627  |
| Support Vector Machine(Modeling)        | 5     | 61.54033136367798  | Support Vector Machine(Modeling)        | 5     | 62.88093090057373  |
| Stats Summary                           | 6     | 35.92398118972778  | Stats Summary                           | 6     | 40.3692798614502   |
