# Supplementary material for: STREAMLINE: An Automated Machine Learning Pipeline for Biomedicine Applied to Examine the Utility of Photography-Based Phenotypes for OSA Prediction Across International Sleep Centers
Source: arXiv:2312.05461 ancillary file (2023-12-09)
Supplement: Supplementary file 5 [file multiplexer_exp_STREAMLINE_Report.pdf]

# STREAMLINE Testing Data Evaluation Report: 2023-09-30 17:08:33.708770

## General Pipeline Settings:

CV Partitions: 10  
Partition Method: Stratified  
Categorical Cutoff: 10  
Statistical Significance Cutoff: 0.05  
Random Seed: 42  
Run From Notebook: False

## Feature Importance/Selection Settings:

Use Mutual Information: True  
Use MultiSURF: True  
Use TURF: False  
TURF Cutoff: 0.5  
MultiSURF Instance Subset: 2000  
Max Features to Keep: 2000  
Filter Poor Features: True  
Top Features to Display: 40  
Export Feature Importance Plot: True

## ML Modeling Algorithms:

Artificial Neural Network: True  
Category Gradient Boosting: True  
Decision Tree: True  
Elastic Net: True  
ExSTraCS: True  
Extreme Gradient Boosting: True  
Genetic Programming: True  
Gradient Boosting: True  
K-Nearest Neighbors: True  
Light Gradient Boosting: True  
Logistic Regression: True  
Naive Bayes: True  
Random Forest: True  
Support Vector Machine: True  
XCS: False  
eLCS: False

## Modeling Settings:

Primary Metric: balanced\_accuracy  
Training Subsample for KNN,ANN,SVM,and XGB: 5000  
Uniform Feature Importance Estimation (Models): True  
Hyperparameter Sweep Number of Trials: 200  
Hyperparameter Timeout: 900  
Export Hyperparameter Sweep Plots: False

## LCS Settings (eLCS,XCS,ExSTraCS):

Do LCS Hyperparameter Sweep: False  
nu: 10  
Training Iterations: 500000  
N (Rule Population Size): 5000  
LCS Hyperparameter Sweep Timeout: 1200

## Stats and Figure Settings:

Export ROC Plot: True  
Export PRC Plot: True  
Export Metric Boxplots: True  
Export Feature Importance Boxplots: True  
Metric Weighting Composite FI Plots: balanced\_accuracy  
Top Model Features To Display: 40

## EDA and Processing Settings:

Engineering Missingness Cutoff: 0.5  
Cleaning Missingness Cutoff: 0.5  
Correlation Removal Threshold: 1.0  
List of Exploratory Analysis Ran: ['Describe', 'Univariate Analysis', 'Feature Correlation']  
List of Exploratory Plots Saved: ['Describe', 'Univariate Analysis', 'Feature Correlation']  
Use Data Scaling: True  
Use Data Imputation: True  
Use Multivariate Imputation: True  
Overwrite CV Datasets: True

## Target Dataset(s):

D1 = A\_6\_bit\_muxlexer\_500\_01  
D2 = B\_11\_bit\_muxlexer\_1000\_01  
D3 = C\_20\_bit\_muxlexer\_2000\_01  
D4 = D\_37\_bit\_muxlexer\_5000\_01  
D5 = E\_70\_bit\_muxlexer\_10000\_01  
D6 = F\_135\_bit\_muxlexer\_20000\_01

## Target Data Settings:

Data Path: /home/ryanurb/idata/datasets/multiplexer\_set  
Output Path: /home/ryanurb/idata/output  
Experiment Name: multiplexer\_exp  
Class Label: Class  
Instance Label: None  
Match Label: None  
Ignored Features: None  
Specified Categorical Features: None  
Specified Quantitative Features: None

# Univariate Analysis of Each Dataset (Top 10 Features for Each): Page 1

## D1 = A\_6\_bit\_muxliplexer\_500\_01

| Feature | p-value                | Test-statistic     | Test-name       |
|---------|------------------------|--------------------|-----------------|
| R_0     | 1.26939024268301e-10   | 41.35511261834883  | Chi Square Test |
| R_3     | 3.509298244030297e-07  | 25.946947904868114 | Chi Square Test |
| R_1     | 9.059261024221464e-07  | 24.118356245511887 | Chi Square Test |
| R_2     | 1.7448416343049778e-05 | 18.449308184257745 | Chi Square Test |
| A_0     | 0.5694973919380477     | 0.3235241925021814 | Chi Square Test |
| A_1     | 0.7971447941453101     | 0.0660716263614629 | Chi Square Test |

## D2 = B\_11\_bit\_muxliplexer\_1000\_01

| Feature | p-value                | Test-statistic     | Test-name       |
|---------|------------------------|--------------------|-----------------|
| R_4     | 2.2248801885218974e-05 | 17.986407101556246 | Chi Square Test |
| R_2     | 0.0001766997611545     | 14.06393430248582  | Chi Square Test |
| R_6     | 0.000193302557659      | 13.89509227496958  | Chi Square Test |
| R_0     | 0.0003044847642591     | 13.04260204068494  | Chi Square Test |
| R_1     | 0.0012360481186965     | 10.43566835329348  | Chi Square Test |
| R_7     | 0.0052238913440066     | 7.800253212299817  | Chi Square Test |
| R_3     | 0.0224712913608342     | 5.208919842115445  | Chi Square Test |
| R_5     | 0.0225536002419627     | 5.202563750638238  | Chi Square Test |
| A_2     | 0.2035317994195949     | 1.616848359505822  | Chi Square Test |
| A_0     | 0.4098568324810853     | 0.6792159709268657 | Chi Square Test |

## D3 = C\_20\_bit\_muxliplexer\_2000\_01

| Feature | p-value               | Test-statistic     | Test-name       |
|---------|-----------------------|--------------------|-----------------|
| R_2     | 8.852163558112362e-05 | 15.366983314539574 | Chi Square Test |
| R_3     | 0.0001193452640023    | 14.803003619380137 | Chi Square Test |
| R_6     | 0.000384686668138     | 12.605143690405226 | Chi Square Test |
| R_5     | 0.0008311970831204    | 11.170243702842953 | Chi Square Test |
| R_1     | 0.0008925709376199    | 11.03812492590501  | Chi Square Test |
| R_4     | 0.0016002295505668    | 9.959483349984106  | Chi Square Test |
| R_14    | 0.0023725177489401    | 9.236393524110213  | Chi Square Test |
| R_13    | 0.0033974532166476    | 8.580696865486933  | Chi Square Test |
| R_15    | 0.0048580643893158    | 7.931532124257506  | Chi Square Test |
| R_7     | 0.0050257374945953    | 7.870153924494158  | Chi Square Test |

## D4 = D\_37\_bit\_muxliplexer\_5000\_01

| Feature | p-value            | Test-statistic     | Test-name       |
|---------|--------------------|--------------------|-----------------|
| R_31    | 0.0007736754593663 | 11.303345820003502 | Chi Square Test |
| R_30    | 0.0008832966181209 | 11.057489539940754 | Chi Square Test |
| R_13    | 0.0009918366525363 | 10.842743610043753 | Chi Square Test |
| R_2     | 0.0016474655174039 | 9.905935616718336  | Chi Square Test |
| R_19    | 0.0023476917358282 | 9.255656401273008  | Chi Square Test |
| R_1     | 0.0024614843515886 | 9.169004447352131  | Chi Square Test |
| R_3     | 0.0027526782036786 | 8.964554448121605  | Chi Square Test |
| R_15    | 0.0095181037929174 | 6.722931778807654  | Chi Square Test |
| R_29    | 0.0106617018265068 | 6.5208502788115865 | Chi Square Test |
| R_5     | 0.0110527366236116 | 6.456818497651977  | Chi Square Test |

## D5 = E\_70\_bit\_muxliplexer\_10000\_01

| Feature | p-value                | Test-statistic     | Test-name       |
|---------|------------------------|--------------------|-----------------|
| R_22    | 2.225314574216959e-07  | 26.826785597019267 | Chi Square Test |
| R_34    | 3.5048304422665855e-05 | 17.12230320284783  | Chi Square Test |
| R_25    | 0.0004675117666111     | 12.240983647990896 | Chi Square Test |
| A_5     | 0.0026933624905259     | 9.004360280922796  | Chi Square Test |
| R_38    | 0.0030718690386894     | 8.764282469687348  | Chi Square Test |
| R_13    | 0.0035117346967141     | 8.520471624934709  | Chi Square Test |
| R_29    | 0.0039853662019388     | 8.290470475499852  | Chi Square Test |
| R_12    | 0.0045245747368835     | 8.060297755474451  | Chi Square Test |
| R_52    | 0.0057657049009223     | 7.622108140310798  | Chi Square Test |
| R_59    | 0.0060974802599191     | 7.521266286542581  | Chi Square Test |

## Univariate Analysis of Each Dataset (Top 10 Features for Each): Page 2

### D6 = F\_135\_bit\_mutliplexer\_20000\_01

| Feature | p-value            | Test-statistic    | Test-name       |
|---------|--------------------|-------------------|-----------------|
| R_23    | 0.0008774724917323 | 11.06975556060301 | Chi Square Test |
| R_65    | 0.0028169569692886 | 8.922389587548853 | Chi Square Test |
| R_49    | 0.0033365077024448 | 8.613662180606806 | Chi Square Test |
| R_74    | 0.0055759947488155 | 7.682465108479826 | Chi Square Test |
| R_105   | 0.0058873767124799 | 7.584454792050828 | Chi Square Test |
| R_116   | 0.0075815765786996 | 7.129738926496422 | Chi Square Test |
| R_94    | 0.0090281431801193 | 6.817251013752202 | Chi Square Test |
| R_26    | 0.0124580448268327 | 6.244487156290251 | Chi Square Test |
| R_59    | 0.0168492271574137 | 5.712010980840283 | Chi Square Test |
| R_35    | 0.0240939875657274 | 5.087854117108158 | Chi Square Test |

# Dataset and Model Prediction Summary: D1 = A\_6\_bit\_multiplexer\_500\_01

## Data Processing/Counts Summary

|           | Instances | Total Features | Categorical Features | Quantitative Features | Missing Values | Missing Percent | Class 0 | Class 1 |
|-----------|-----------|----------------|----------------------|-----------------------|----------------|-----------------|---------|---------|
| Original  | 500       | 6              | 6                    | 0                     | 0              | 0.0             | 254     | 246     |
| C1        | 500       | 6              | 6                    | 0                     | 0              | 0.0             | 254     | 246     |
| E1        | 500       | 6              | 6                    | 0                     | 0              | 0.0             | 254     | 246     |
| C2        | 500       | 6              | 6                    | 0                     | 0              | 0.0             | 254     | 246     |
| C3        | 500       | 6              | 6                    | 0                     | 0              | 0.0             | 254     | 246     |
| E2        | 500       | 6              | 6                    | 0                     | 0              | 0.0             | 254     | 246     |
| C4        | 500       | 6              | 6                    | 0                     | 0              | 0.0             | 254     | 246     |
| Processed | 500       | 6              | 6                    | 0                     | 0              | 0.0             | 254     | 246     |

## Cleaning (C) and Engineering (E) Elements

- \* C1 - Remove instances with no outcome and features to ignore
- \* E1 - Add missingness features
- \* C2 - Remove features with invariance or high missingness
- \* C3 - Remove instances with high missingness
- \* E2 - Add one-hot-encoding of categorical features
- \* C4 - Remove highly correlated features

## Class Balance (Processed)

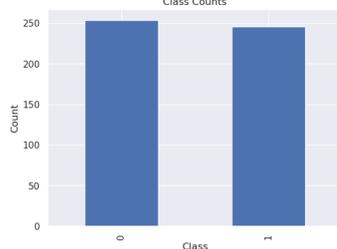

## Feature Correlations (Pearson)

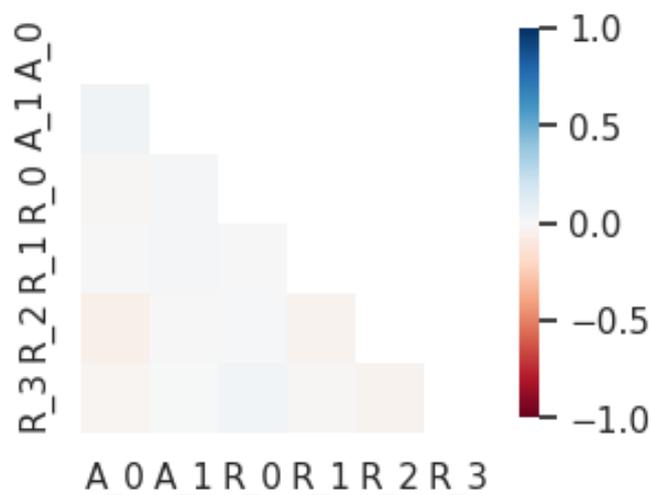

## Top ML Algorithm Results (Averaged Over CV Runs):

|                                                                |
|----------------------------------------------------------------|
| Best (ROC_AUC): Artificial Neural Network (TIE) = 1.000        |
| Best (Balanced Acc.): Category Gradient Boosting (TIE) = 1.000 |
| Best (F1 Score): Category Gradient Boosting (TIE) = 1.000      |
| Best (PRC AUC): Artificial Neural Network (TIE) = 1.000        |
| Best (PRC APS): Artificial Neural Network (TIE) = 1.000        |

## ROC

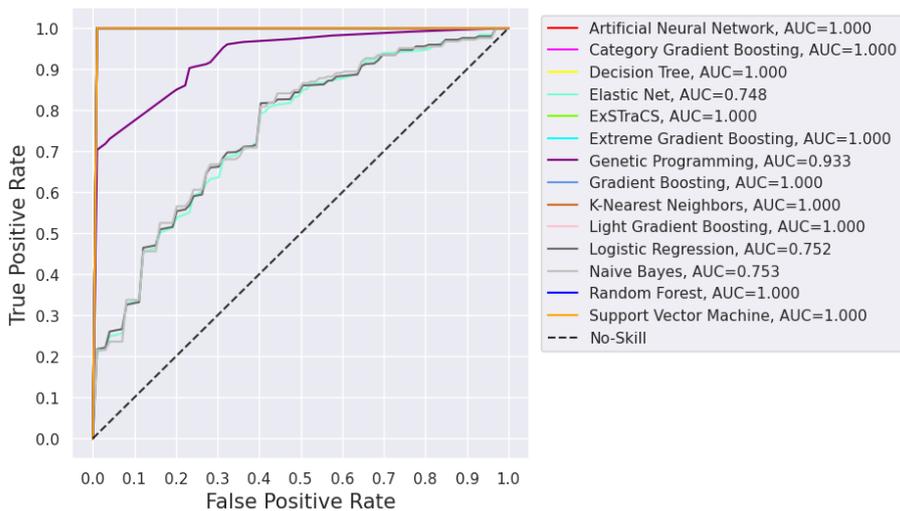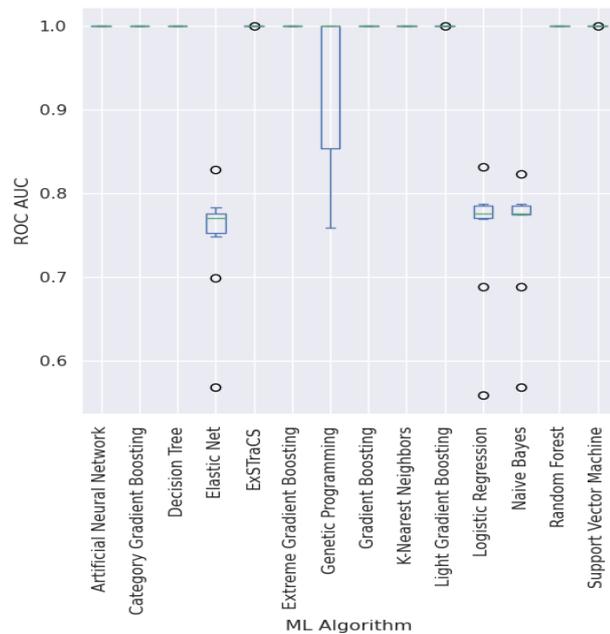

## PRC

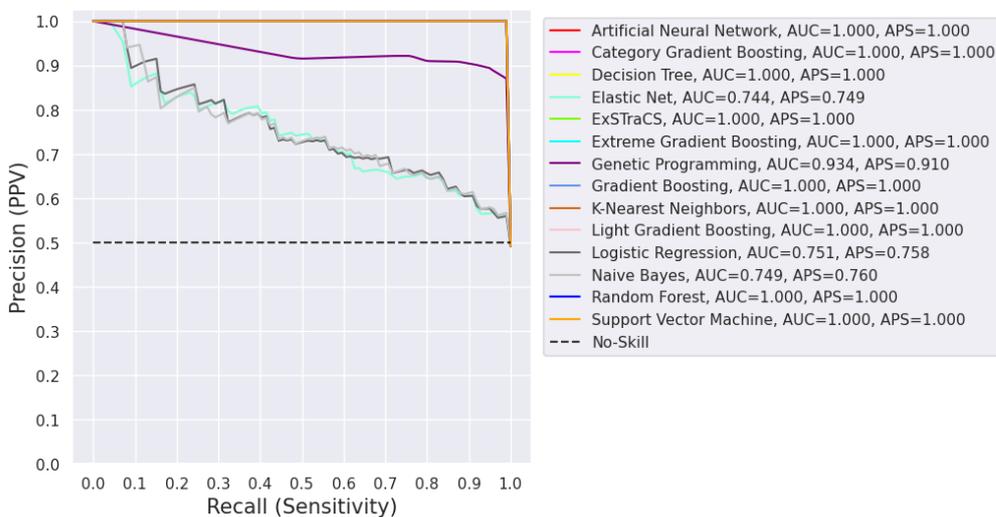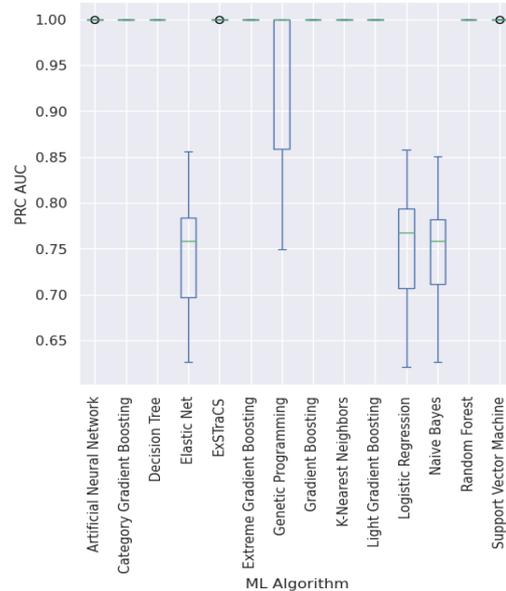

# Dataset and Model Prediction Summary: D2 = B\_11\_bit\_mutliplexer\_1000\_01

## Data Processing/Counts Summary

|           | Instances | Total Features | Categorical Features | Quantitative Features | Missing Values | Missing Percent | Class 0 | Class 1 |
|-----------|-----------|----------------|----------------------|-----------------------|----------------|-----------------|---------|---------|
| Original  | 1000      | 11             | 11                   | 0                     | 0              | 0.0             | 495     | 505     |
| C1        | 1000      | 11             | 11                   | 0                     | 0              | 0.0             | 495     | 505     |
| E1        | 1000      | 11             | 11                   | 0                     | 0              | 0.0             | 495     | 505     |
| C2        | 1000      | 11             | 11                   | 0                     | 0              | 0.0             | 495     | 505     |
| C3        | 1000      | 11             | 11                   | 0                     | 0              | 0.0             | 495     | 505     |
| E2        | 1000      | 11             | 11                   | 0                     | 0              | 0.0             | 495     | 505     |
| C4        | 1000      | 11             | 11                   | 0                     | 0              | 0.0             | 495     | 505     |
| Processed | 1000      | 11             | 11                   | 0                     | 0              | 0.0             | 495     | 505     |

## Cleaning (C) and Engineering (E) Elements

- \* C1 - Remove instances with no outcome and features to ignore
- \* E1 - Add missingness features
- \* C2 - Remove features with invariance or high missingness
- \* C3 - Remove instances with high missingness
- \* E2 - Add one-hot-encoding of categorical features
- \* C4 - Remove highly correlated features

## Class Balance (Processed)

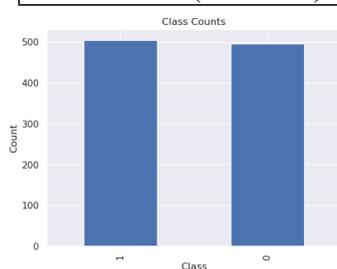

## Feature Correlations (Pearson)

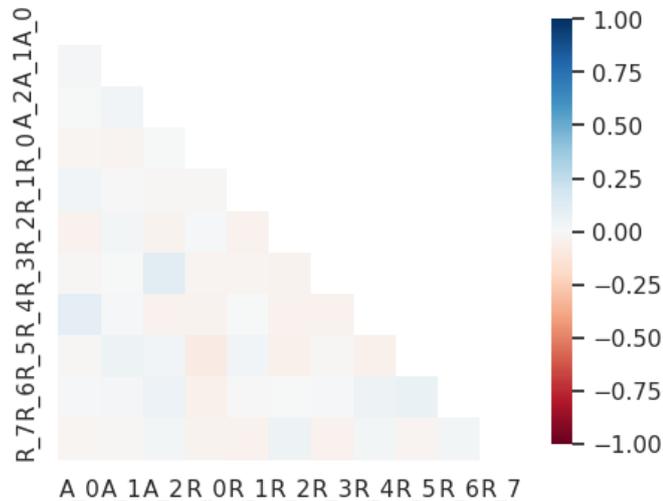

## Top ML Algorithm Results (Averaged Over CV Runs):

|                                                          |
|----------------------------------------------------------|
| Best (ROC_AUC): Random Forest = 0.982                    |
| Best (Balanced Acc.): Category Gradient Boosting = 0.920 |
| Best (F1 Score): Random Forest = 0.919                   |
| Best (PRC AUC): Random Forest = 0.983                    |
| Best (PRC APS): Random Forest = 0.983                    |

## ROC

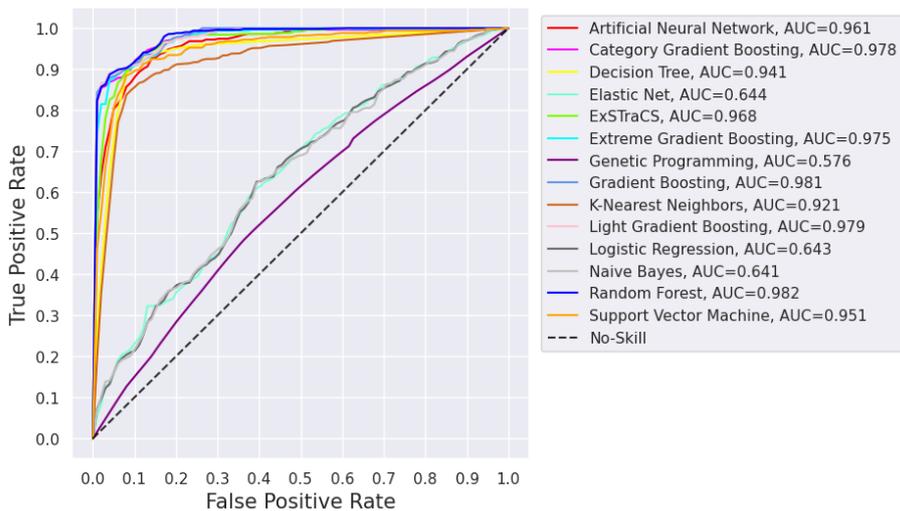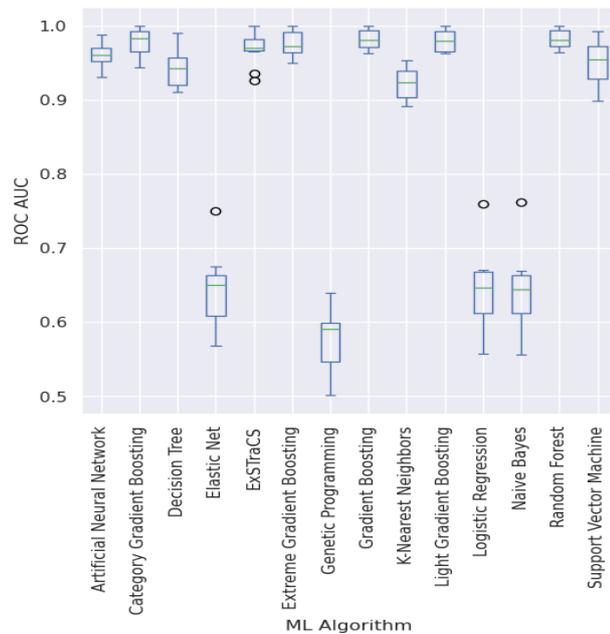

## PRC

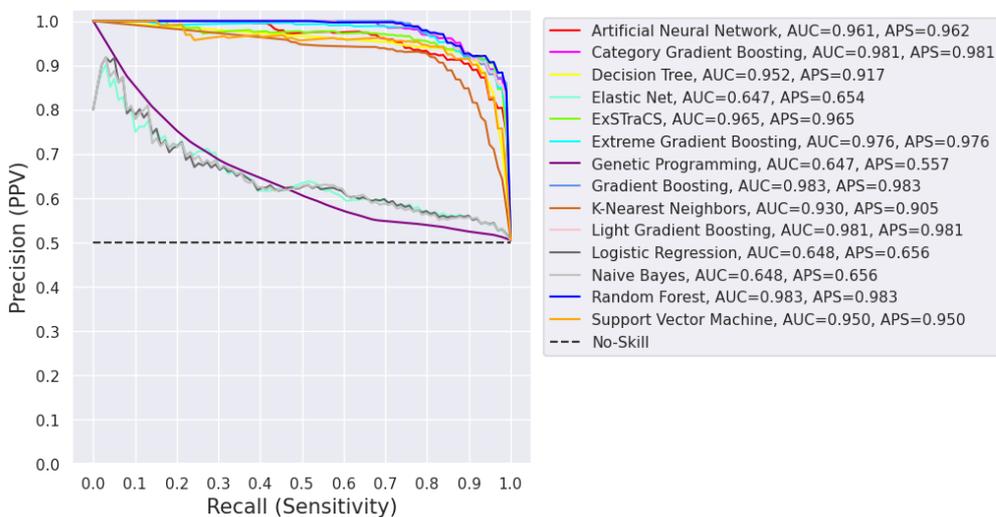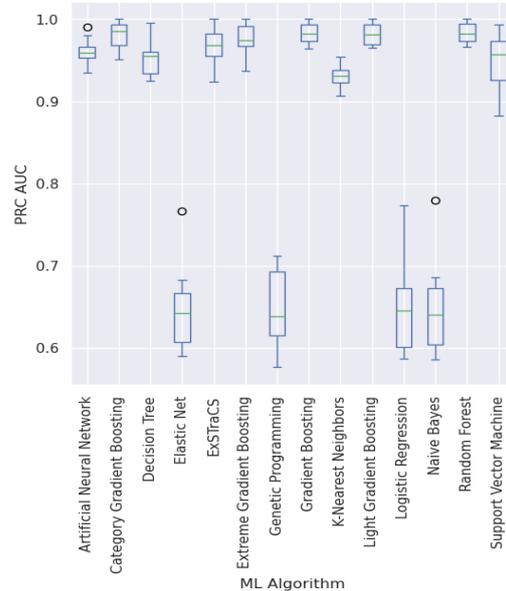

# Dataset and Model Prediction Summary: D3 = C\_20\_bit\_muxlexer\_2000\_01

## Data Processing/Counts Summary

|           | Instances | Total Features | Categorical Features | Quantitative Features | Missing Values | Missing Percent | Class 0 | Class 1 |
|-----------|-----------|----------------|----------------------|-----------------------|----------------|-----------------|---------|---------|
| Original  | 2000      | 20             | 20                   | 0                     | 0              | 0.0             | 1018    | 982     |
| C1        | 2000      | 20             | 20                   | 0                     | 0              | 0.0             | 1018    | 982     |
| E1        | 2000      | 20             | 20                   | 0                     | 0              | 0.0             | 1018    | 982     |
| C2        | 2000      | 20             | 20                   | 0                     | 0              | 0.0             | 1018    | 982     |
| C3        | 2000      | 20             | 20                   | 0                     | 0              | 0.0             | 1018    | 982     |
| E2        | 2000      | 20             | 20                   | 0                     | 0              | 0.0             | 1018    | 982     |
| C4        | 2000      | 20             | 20                   | 0                     | 0              | 0.0             | 1018    | 982     |
| Processed | 2000      | 20             | 20                   | 0                     | 0              | 0.0             | 1018    | 982     |

## Cleaning (C) and Engineering (E) Elements

- \* C1 - Remove instances with no outcome and features to ignore
- \* E1 - Add missingness features
- \* C2 - Remove features with invariance or high missingness
- \* C3 - Remove instances with high missingness
- \* E2 - Add one-hot-encoding of categorical features
- \* C4 - Remove highly correlated features

## Class Balance (Processed)

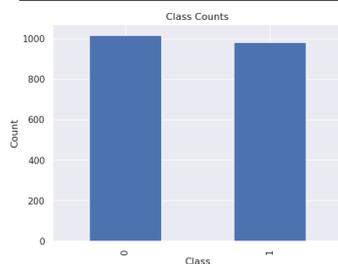

## Feature Correlations (Pearson)

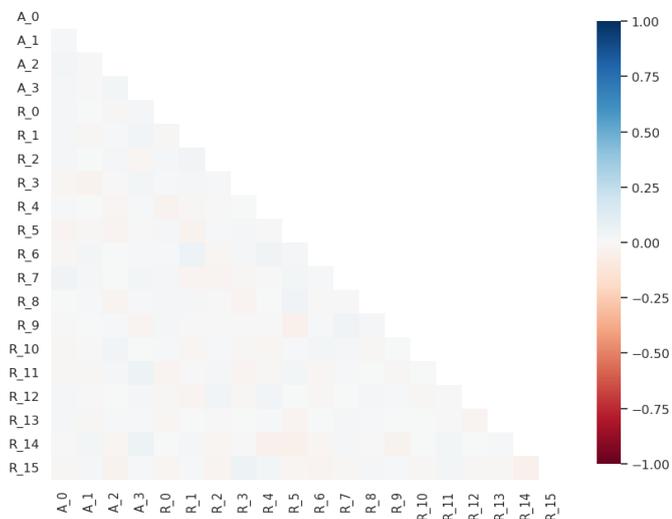

## Top ML Algorithm Results (Averaged Over CV Runs):

|                                                          |
|----------------------------------------------------------|
| Best (ROC_AUC): ExSTraCS = 0.968                         |
| Best (Balanced Acc.): Category Gradient Boosting = 0.918 |
| Best (F1 Score): Category Gradient Boosting = 0.917      |
| Best (PRC AUC): ExSTraCS = 0.970                         |
| Best (PRC APS): ExSTraCS = 0.970                         |

## ROC

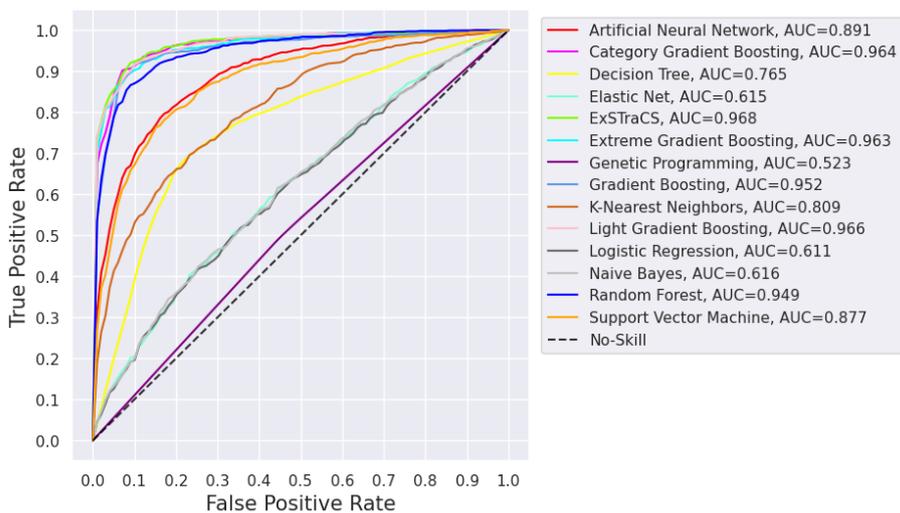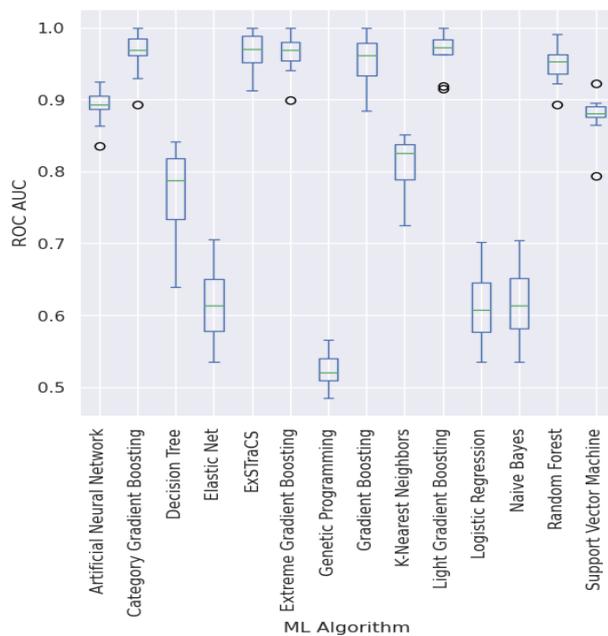

## PRC

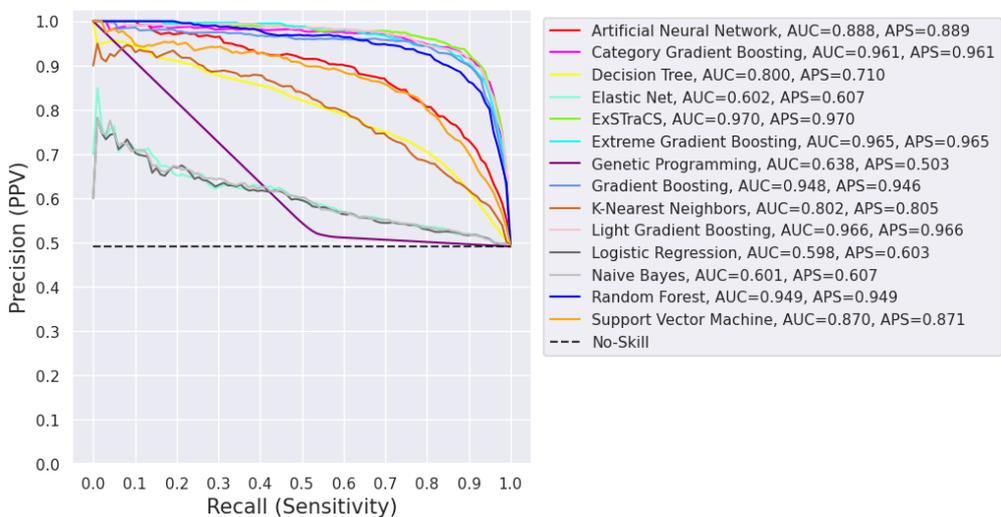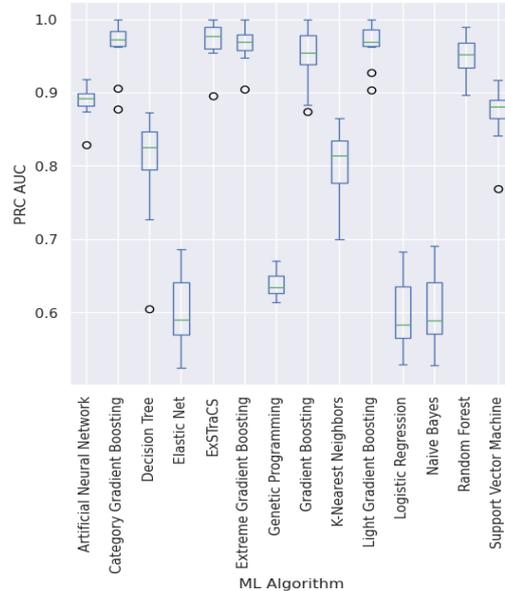

# Dataset and Model Prediction Summary: D4 = D\_37\_bit\_mutliplexer\_5000\_01

## Data Processing/Counts Summary

|           | Instances | Total Features | Categorical Features | Quantitative Features | Missing Values | Missing Percent | Class 0 | Class 1 |
|-----------|-----------|----------------|----------------------|-----------------------|----------------|-----------------|---------|---------|
| Original  | 5000      | 37             | 37                   | 0                     | 0              | 0.0             | 2522    | 2478    |
| C1        | 5000      | 37             | 37                   | 0                     | 0              | 0.0             | 2522    | 2478    |
| E1        | 5000      | 37             | 37                   | 0                     | 0              | 0.0             | 2522    | 2478    |
| C2        | 5000      | 37             | 37                   | 0                     | 0              | 0.0             | 2522    | 2478    |
| C3        | 5000      | 37             | 37                   | 0                     | 0              | 0.0             | 2522    | 2478    |
| E2        | 5000      | 37             | 37                   | 0                     | 0              | 0.0             | 2522    | 2478    |
| C4        | 5000      | 37             | 37                   | 0                     | 0              | 0.0             | 2522    | 2478    |
| Processed | 5000      | 37             | 37                   | 0                     | 0              | 0.0             | 2522    | 2478    |

**Cleaning (C) and Engineering (E) Elements**  
 \* C1 - Remove instances with no outcome and features to ignore  
 \* E1 - Add missingness features  
 \* C2 - Remove features with invariance or high missingness  
 \* C3 - Remove instances with high missingness  
 \* E2 - Add one-hot-encoding of categorical features  
 \* C4 - Remove highly correlated features

## Class Balance (Processed)

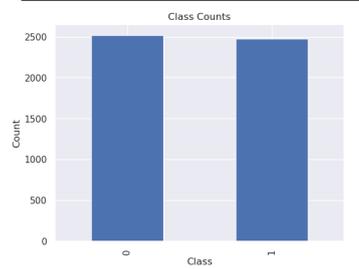

## Feature Correlations (Pearson)

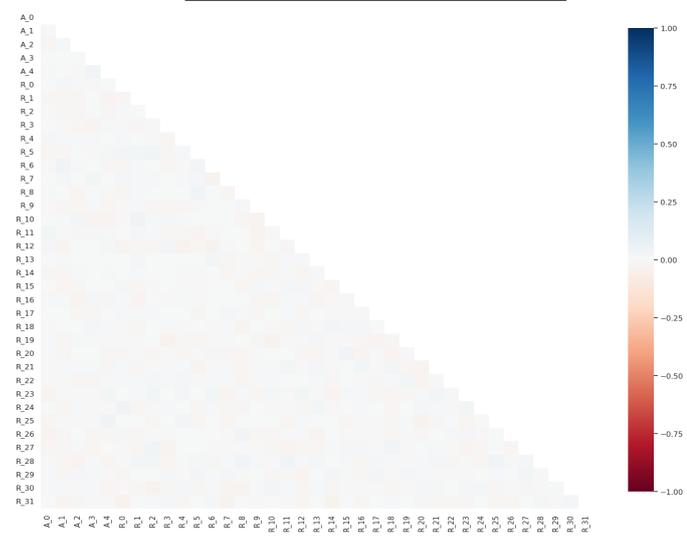

## Top ML Algorithm Results (Averaged Over CV Runs):

|                                                 |
|-------------------------------------------------|
| Best (ROC_AUC): ExSTraCS = 0.938                |
| Best (Balanced Acc.): ExSTraCS = 0.885          |
| Best (F1 Score): ExSTraCS = 0.884               |
| Best (PRC AUC): Light Gradient Boosting = 0.936 |
| Best (PRC APS): Light Gradient Boosting = 0.936 |

## ROC

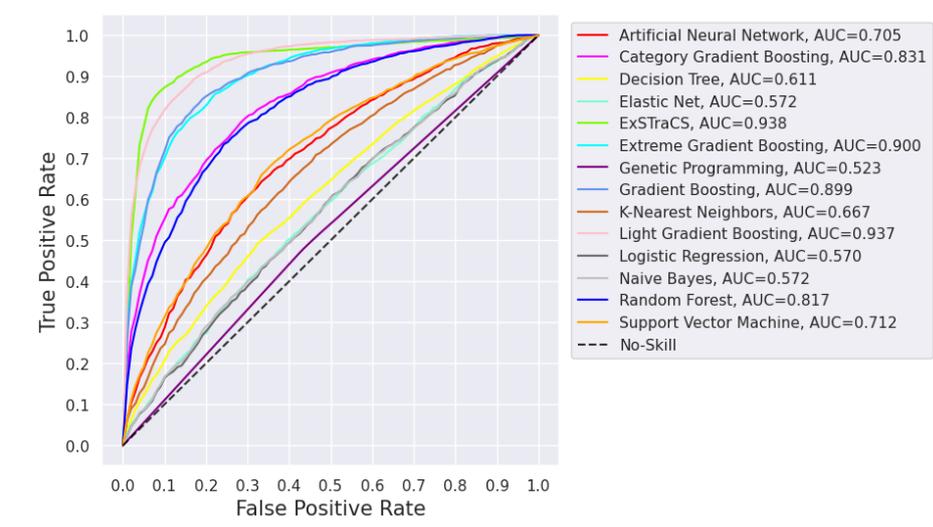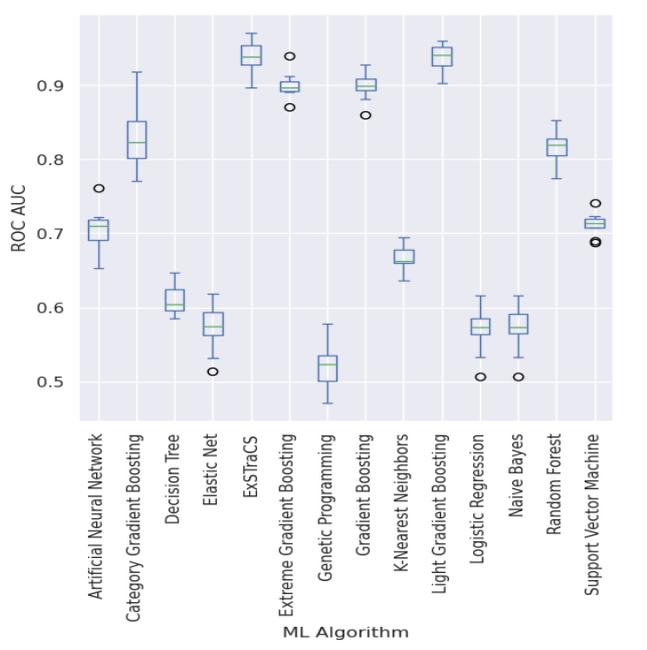

## PRC

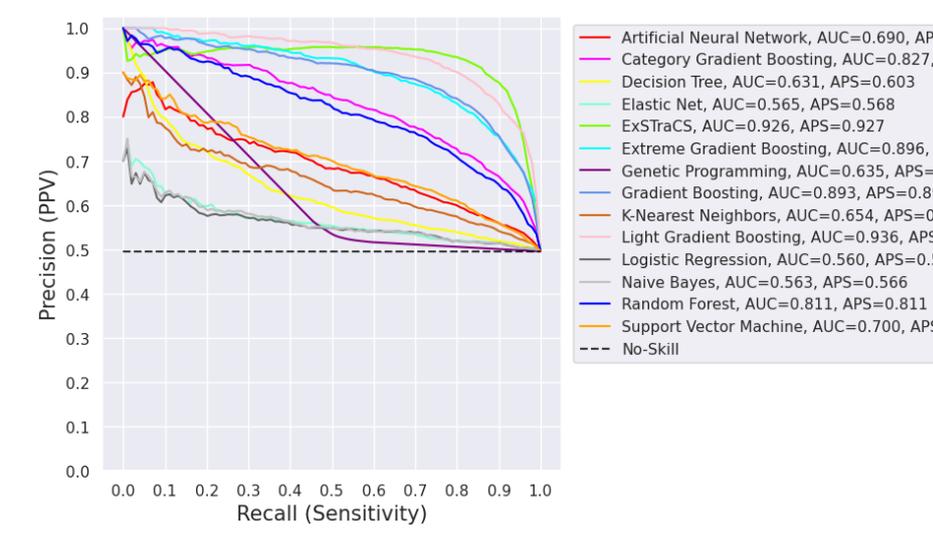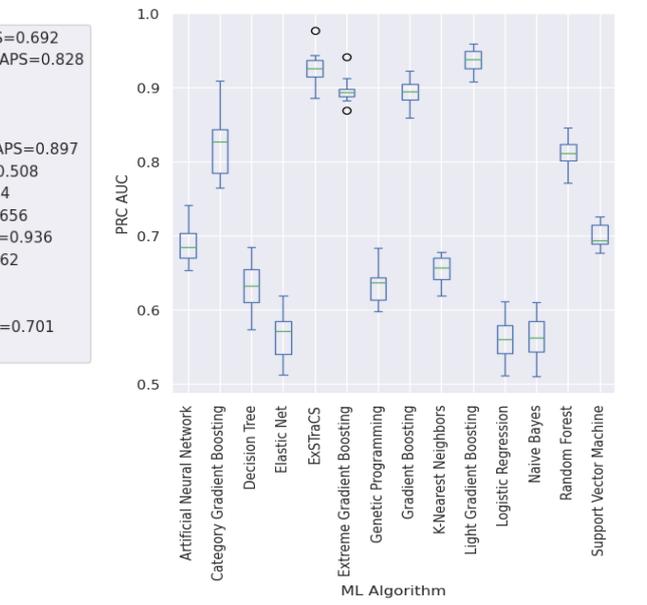

# Dataset and Model Prediction Summary: D5 = E\_70\_bit\_mutlplexer\_10000\_01

## Data Processing/Counts Summary

|           | Instances | Total Features | Categorical Features | Quantitative Features | Missing Values | Missing Percent | Class 0 | Class 1 |
|-----------|-----------|----------------|----------------------|-----------------------|----------------|-----------------|---------|---------|
| Original  | 10000     | 70             | 70                   | 0                     | 0              | 0.0             | 5011    | 4989    |
| C1        | 10000     | 70             | 70                   | 0                     | 0              | 0.0             | 5011    | 4989    |
| E1        | 10000     | 70             | 70                   | 0                     | 0              | 0.0             | 5011    | 4989    |
| C2        | 10000     | 70             | 70                   | 0                     | 0              | 0.0             | 5011    | 4989    |
| C3        | 10000     | 70             | 70                   | 0                     | 0              | 0.0             | 5011    | 4989    |
| E2        | 10000     | 70             | 70                   | 0                     | 0              | 0.0             | 5011    | 4989    |
| C4        | 10000     | 70             | 70                   | 0                     | 0              | 0.0             | 5011    | 4989    |
| Processed | 10000     | 70             | 70                   | 0                     | 0              | 0.0             | 5011    | 4989    |

## Cleaning (C) and Engineering (E) Elements

- \* C1 - Remove instances with no outcome and features to ignore
- \* E1 - Add missingness features
- \* C2 - Remove features with invariance or high missingness
- \* C3 - Remove instances with high missingness
- \* E2 - Add one-hot-encoding of categorical features
- \* C4 - Remove highly correlated features

## Class Balance (Processed)

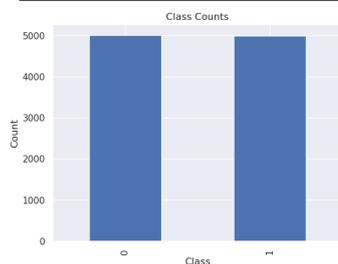

## Feature Correlations (Pearson)

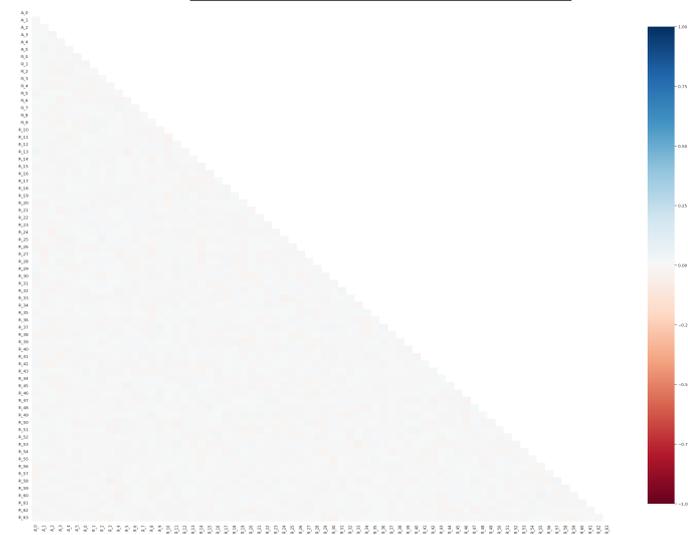

## Top ML Algorithm Results (Averaged Over CV Runs):

Best (ROC\_AUC): ExSTraCS = 0.908

Best (Balanced Acc.): ExSTraCS = 0.857

Best (F1 Score): ExSTraCS = 0.857

Best (PRC AUC): ExSTraCS = 0.888

Best (PRC APS): ExSTraCS = 0.888

## ROC

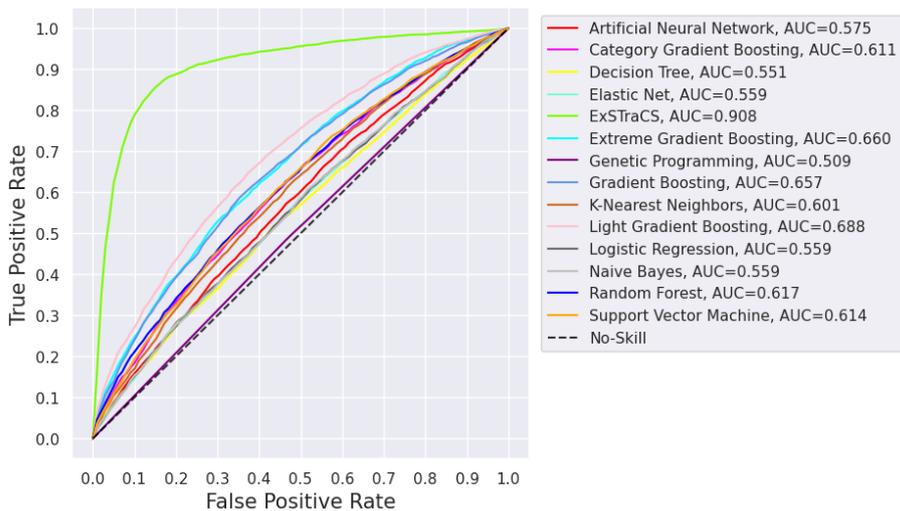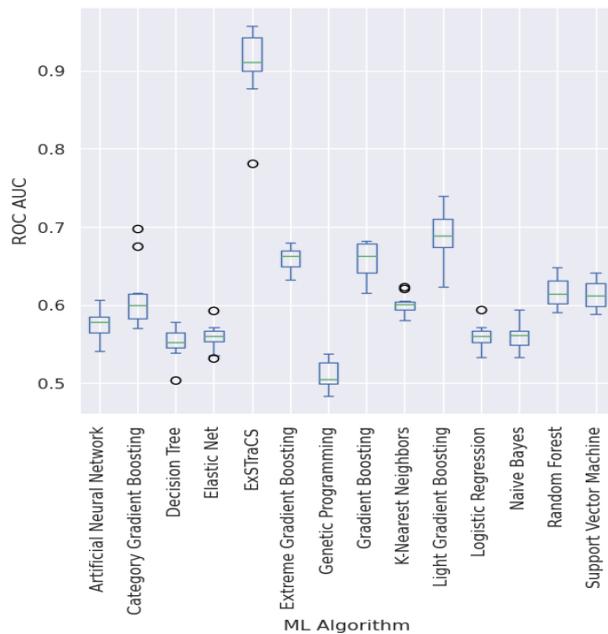

## PRC

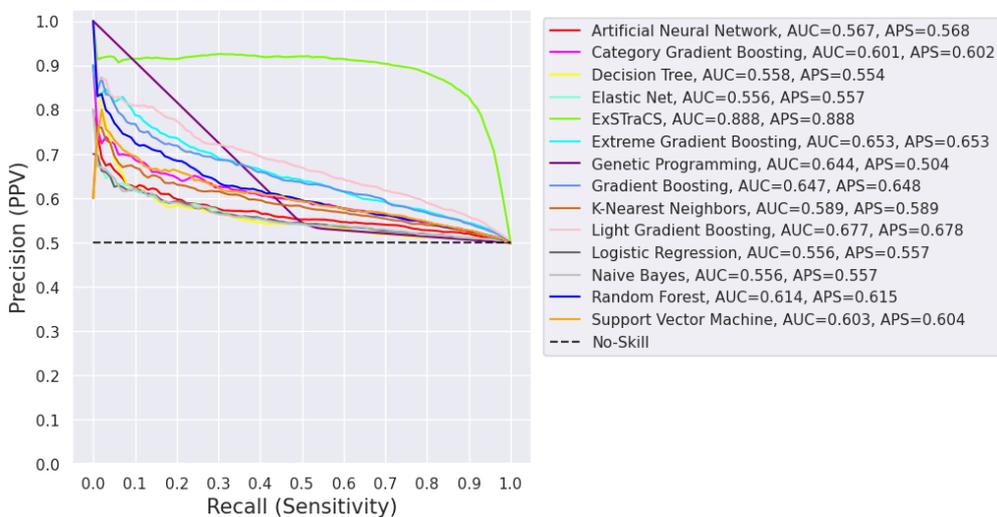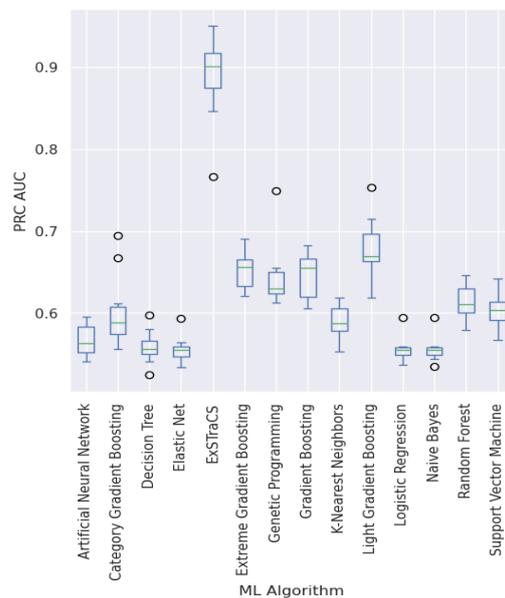

# Dataset and Model Prediction Summary: D6 = F\_135\_bit\_mutliplexer\_20000\_01

## Data Processing/Counts Summary

|           | Instances | Total Features | Categorical Features | Quantitative Features | Missing Values | Missing Percent | Class 0 | Class 1 |
|-----------|-----------|----------------|----------------------|-----------------------|----------------|-----------------|---------|---------|
| Original  | 20000     | 135            | 135                  | 0                     | 0              | 0.0             | 10073   | 9927    |
| C1        | 20000     | 135            | 135                  | 0                     | 0              | 0.0             | 10073   | 9927    |
| E1        | 20000     | 135            | 135                  | 0                     | 0              | 0.0             | 10073   | 9927    |
| C2        | 20000     | 135            | 135                  | 0                     | 0              | 0.0             | 10073   | 9927    |
| C3        | 20000     | 135            | 135                  | 0                     | 0              | 0.0             | 10073   | 9927    |
| E2        | 20000     | 135            | 135                  | 0                     | 0              | 0.0             | 10073   | 9927    |
| C4        | 20000     | 135            | 135                  | 0                     | 0              | 0.0             | 10073   | 9927    |
| Processed | 20000     | 135            | 135                  | 0                     | 0              | 0.0             | 10073   | 9927    |

## Cleaning (C) and Engineering (E) Elements

- \* C1 - Remove instances with no outcome and features to ignore
- \* E1 - Add missingness features
- \* C2 - Remove features with invariance or high missingness
- \* C3 - Remove instances with high missingness
- \* E2 - Add one-hot-encoding of categorical features
- \* C4 - Remove highly correlated features

## Class Balance (Processed)

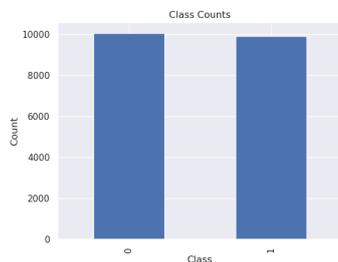

## Feature Correlations (Pearson)

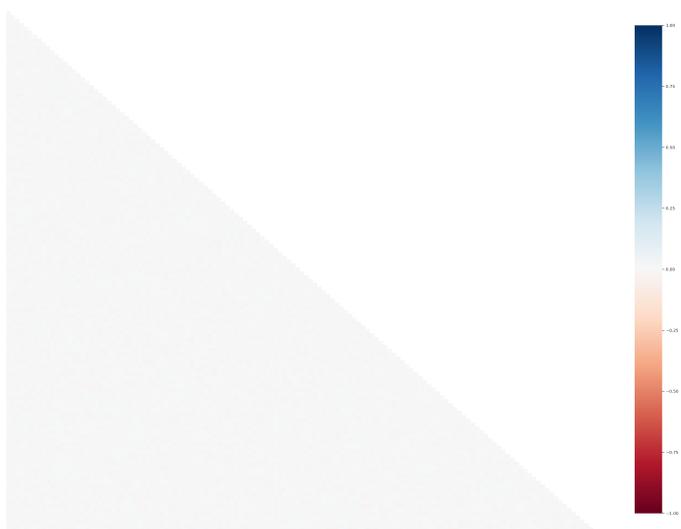

## Top ML Algorithm Results (Averaged Over CV Runs):

|                                                      |
|------------------------------------------------------|
| Best (ROC_AUC): Support Vector Machine = 0.556       |
| Best (Balanced Acc.): Support Vector Machine = 0.539 |
| Best (F1 Score): Support Vector Machine = 0.536      |
| Best (PRC AUC): Genetic Programming = 0.622          |
| Best (PRC APS): Support Vector Machine = 0.547       |

## ROC

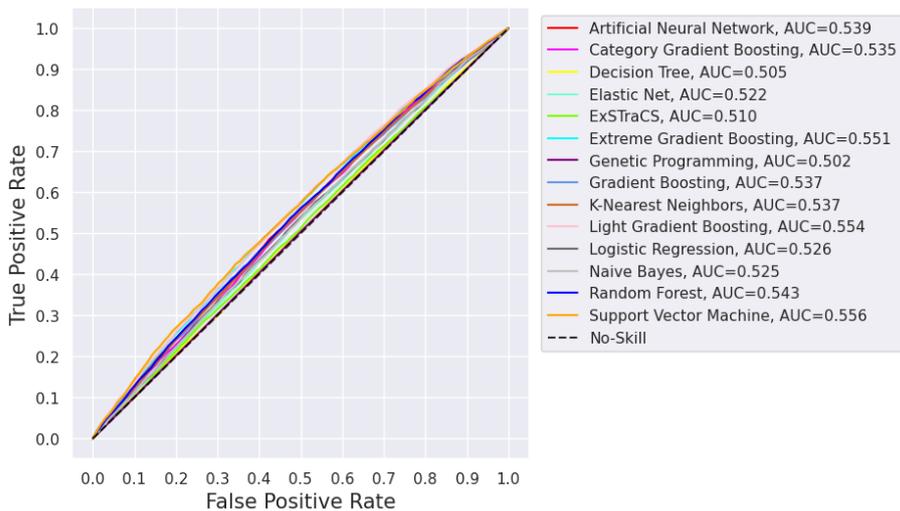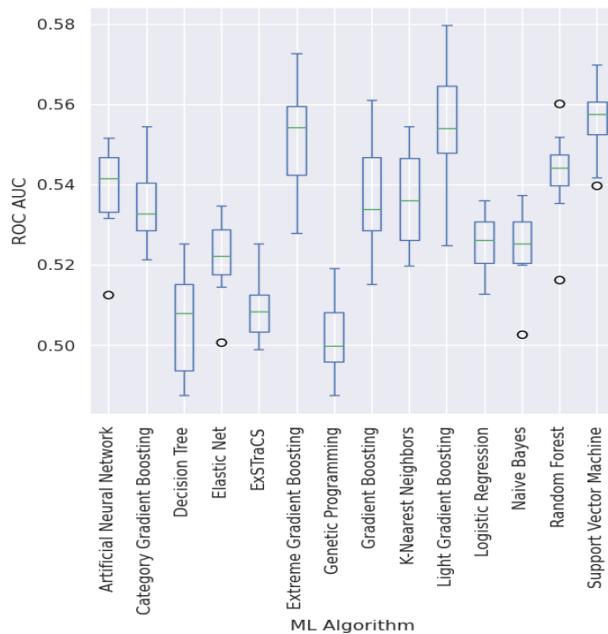

## PRC

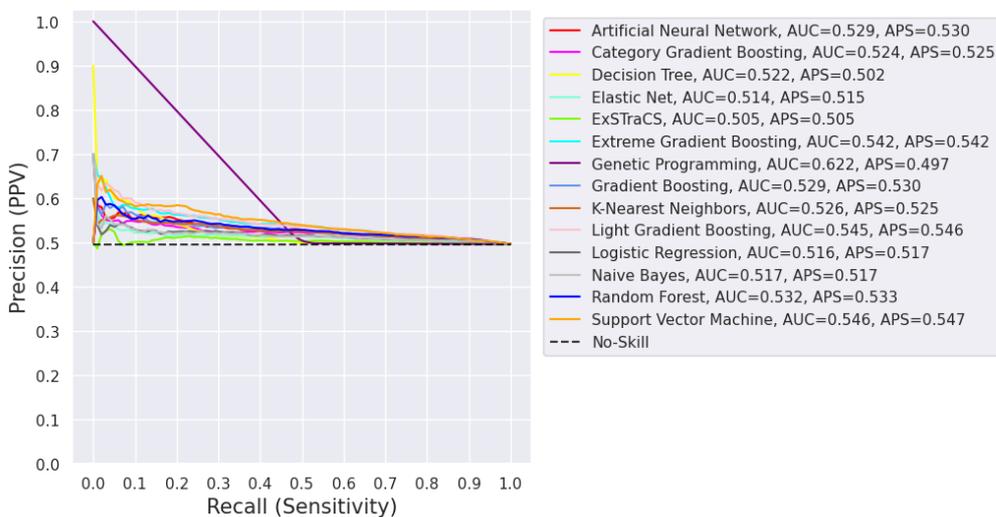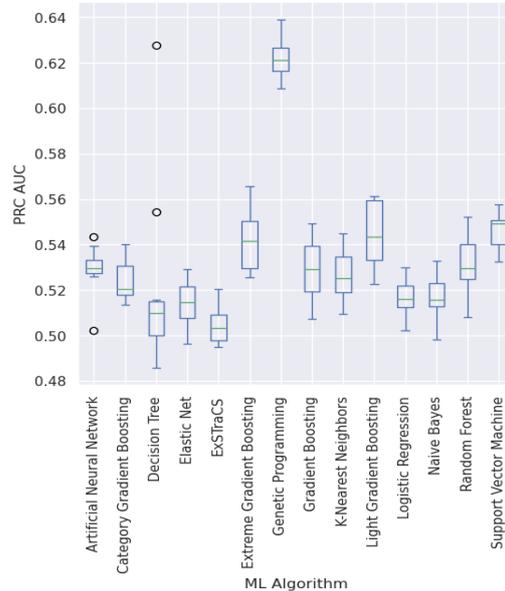

# Average Model Prediction Statistics (Rounded to 3 Decimal Points): Page 1

## D1 = A\_6\_bit\_muxliplexer\_500\_01

| ML Algorithm               | Balanced Accuracy | Accuracy | F1 Score | Sensitivity (Recall) | Specificity | Precision (PPV) | TP   | TN   | FP  | FN  | NPV   | LR+   | LR-   | ROC AUC | PRC AUC | PRC APS |
|----------------------------|-------------------|----------|----------|----------------------|-------------|-----------------|------|------|-----|-----|-------|-------|-------|---------|---------|---------|
| Artificial Neural Network  | 0.996             | 0.996    | 0.996    | 1.0                  | 0.992       | 0.992           | 24.6 | 25.2 | 0.2 | 0.0 | 1.0   | 1.3   | 0.0   | 1.0     | 1.0     | 1.0     |
| Category Gradient Boosting | 1.0               | 1.0      | 1.0      | 1.0                  | 1.0         | 1.0             | 24.6 | 25.4 | 0.0 | 0.0 | 1.0   | 0.0   | 0.0   | 1.0     | 1.0     | 1.0     |
| Decision Tree              | 1.0               | 1.0      | 1.0      | 1.0                  | 1.0         | 1.0             | 24.6 | 25.4 | 0.0 | 0.0 | 1.0   | 0.0   | 0.0   | 1.0     | 1.0     | 1.0     |
| Elastic Net                | 0.67              | 0.67     | 0.671    | 0.688                | 0.653       | 0.659           | 16.9 | 16.6 | 8.8 | 7.7 | 0.686 | 2.11  | 0.489 | 0.748   | 0.744   | 0.749   |
| ExSTraCS                   | 1.0               | 1.0      | 1.0      | 1.0                  | 1.0         | 1.0             | 24.6 | 25.4 | 0.0 | 0.0 | 1.0   | 0.0   | 0.0   | 1.0     | 1.0     | 1.0     |
| Extreme Gradient Boosting  | 1.0               | 1.0      | 1.0      | 1.0                  | 1.0         | 1.0             | 24.6 | 25.4 | 0.0 | 0.0 | 1.0   | 0.0   | 0.0   | 1.0     | 1.0     | 1.0     |
| Genetic Programming        | 0.934             | 0.934    | 0.937    | 0.955                | 0.913       | 0.922           | 23.5 | 23.2 | 2.2 | 1.1 | 0.953 | 3.454 | 0.058 | 0.933   | 0.934   | 0.91    |
| Gradient Boosting          | 1.0               | 1.0      | 1.0      | 1.0                  | 1.0         | 1.0             | 24.6 | 25.4 | 0.0 | 0.0 | 1.0   | 0.0   | 0.0   | 1.0     | 1.0     | 1.0     |
| K-Nearest Neighbors        | 1.0               | 1.0      | 1.0      | 1.0                  | 1.0         | 1.0             | 24.6 | 25.4 | 0.0 | 0.0 | 1.0   | 0.0   | 0.0   | 1.0     | 1.0     | 1.0     |
| Light Gradient Boosting    | 1.0               | 1.0      | 1.0      | 1.0                  | 1.0         | 1.0             | 24.6 | 25.4 | 0.0 | 0.0 | 1.0   | 0.0   | 0.0   | 1.0     | 1.0     | 1.0     |
| Logistic Regression        | 0.696             | 0.696    | 0.692    | 0.708                | 0.684       | 0.687           | 17.4 | 17.4 | 8.0 | 7.2 | 0.716 | 2.349 | 0.427 | 0.752   | 0.751   | 0.758   |
| Naive Bayes                | 0.7               | 0.7      | 0.694    | 0.696                | 0.704       | 0.698           | 17.1 | 17.9 | 7.5 | 7.5 | 0.707 | 2.548 | 0.441 | 0.753   | 0.749   | 0.76    |
| Random Forest              | 1.0               | 1.0      | 1.0      | 1.0                  | 1.0         | 1.0             | 24.6 | 25.4 | 0.0 | 0.0 | 1.0   | 0.0   | 0.0   | 1.0     | 1.0     | 1.0     |
| Support Vector Machine     | 1.0               | 1.0      | 1.0      | 1.0                  | 1.0         | 1.0             | 24.6 | 25.4 | 0.0 | 0.0 | 1.0   | 0.0   | 0.0   | 1.0     | 1.0     | 1.0     |

## D2 = B\_11\_bit\_muxliplexer\_1000\_01

| ML Algorithm               | Balanced Accuracy | Accuracy | F1 Score | Sensitivity (Recall) | Specificity | Precision (PPV) | TP   | TN   | FP   | FN   | NPV   | LR+    | LR-   | ROC AUC | PRC AUC | PRC APS |
|----------------------------|-------------------|----------|----------|----------------------|-------------|-----------------|------|------|------|------|-------|--------|-------|---------|---------|---------|
| Artificial Neural Network  | 0.892             | 0.892    | 0.893    | 0.899                | 0.885       | 0.889           | 45.4 | 43.8 | 5.7  | 5.1  | 0.897 | 9.027  | 0.115 | 0.961   | 0.961   | 0.962   |
| Category Gradient Boosting | 0.92              | 0.92     | 0.919    | 0.909                | 0.932       | 0.931           | 45.9 | 46.1 | 3.4  | 4.6  | 0.91  | 10.285 | 0.1   | 0.978   | 0.981   | 0.981   |
| Decision Tree              | 0.915             | 0.915    | 0.914    | 0.897                | 0.933       | 0.932           | 45.3 | 46.2 | 3.3  | 5.2  | 0.9   | 12.384 | 0.112 | 0.941   | 0.952   | 0.917   |
| Elastic Net                | 0.607             | 0.608    | 0.614    | 0.623                | 0.592       | 0.608           | 31.5 | 29.3 | 20.2 | 19.0 | 0.61  | 1.535  | 0.636 | 0.644   | 0.647   | 0.654   |
| ExSTraCS                   | 0.914             | 0.914    | 0.914    | 0.907                | 0.921       | 0.922           | 45.8 | 45.6 | 3.9  | 4.7  | 0.908 | 11.373 | 0.103 | 0.968   | 0.965   | 0.965   |
| Extreme Gradient Boosting  | 0.91              | 0.91     | 0.91     | 0.901                | 0.919       | 0.92            | 45.5 | 45.5 | 4.0  | 5.0  | 0.902 | 8.732  | 0.11  | 0.975   | 0.976   | 0.976   |
| Genetic Programming        | 0.558             | 0.559    | 0.582    | 0.616                | 0.501       | 0.56            | 31.1 | 24.8 | 24.7 | 19.4 | 0.563 | 1.264  | 0.769 | 0.576   | 0.647   | 0.557   |
| Gradient Boosting          | 0.914             | 0.914    | 0.913    | 0.901                | 0.927       | 0.927           | 45.5 | 45.9 | 3.6  | 5.0  | 0.903 | 12.466 | 0.109 | 0.981   | 0.983   | 0.983   |
| K-Nearest Neighbors        | 0.867             | 0.867    | 0.866    | 0.857                | 0.877       | 0.878           | 43.3 | 43.4 | 6.1  | 7.2  | 0.861 | 7.781  | 0.162 | 0.921   | 0.93    | 0.905   |
| Light Gradient Boosting    | 0.912             | 0.912    | 0.911    | 0.899                | 0.925       | 0.925           | 45.4 | 45.8 | 3.7  | 5.1  | 0.901 | 9.785  | 0.112 | 0.979   | 0.981   | 0.981   |
| Logistic Regression        | 0.604             | 0.605    | 0.611    | 0.621                | 0.588       | 0.606           | 31.4 | 29.1 | 20.4 | 19.1 | 0.608 | 1.512  | 0.64  | 0.643   | 0.648   | 0.656   |
| Naive Bayes                | 0.607             | 0.607    | 0.614    | 0.623                | 0.59        | 0.607           | 31.5 | 29.2 | 20.3 | 19.0 | 0.609 | 1.523  | 0.637 | 0.641   | 0.648   | 0.656   |
| Random Forest              | 0.919             | 0.919    | 0.919    | 0.915                | 0.923       | 0.925           | 46.2 | 45.7 | 3.8  | 4.3  | 0.914 | 9.824  | 0.095 | 0.982   | 0.983   | 0.983   |
| Support Vector Machine     | 0.91              | 0.91     | 0.909    | 0.899                | 0.921       | 0.923           | 45.4 | 45.6 | 3.9  | 5.1  | 0.902 | 13.364 | 0.11  | 0.951   | 0.95    | 0.95    |

## D3 = C\_20\_bit\_muxliplexer\_2000\_01

| ML Algorithm               | Balanced Accuracy | Accuracy | F1 Score | Sensitivity (Recall) | Specificity | Precision (PPV) | TP   | TN   | FP   | FN   | NPV   | LR+    | LR-   | ROC AUC | PRC AUC | PRC APS |
|----------------------------|-------------------|----------|----------|----------------------|-------------|-----------------|------|------|------|------|-------|--------|-------|---------|---------|---------|
| Artificial Neural Network  | 0.806             | 0.806    | 0.801    | 0.794                | 0.818       | 0.81            | 78.0 | 83.3 | 18.5 | 20.2 | 0.806 | 4.704  | 0.252 | 0.891   | 0.888   | 0.889   |
| Category Gradient Boosting | 0.918             | 0.918    | 0.917    | 0.912                | 0.924       | 0.922           | 89.6 | 94.1 | 7.7  | 8.6  | 0.916 | 12.076 | 0.097 | 0.964   | 0.961   | 0.961   |
| Decision Tree              | 0.737             | 0.736    | 0.731    | 0.741                | 0.732       | 0.726           | 72.8 | 74.5 | 27.3 | 25.4 | 0.752 | 2.964  | 0.358 | 0.765   | 0.8     | 0.71    |
| Elastic Net                | 0.584             | 0.584    | 0.576    | 0.575                | 0.592       | 0.58            | 56.5 | 60.3 | 41.7 | 41.7 | 0.591 | 1.477  | 0.726 | 0.615   | 0.602   | 0.607   |
| ExSTraCS                   | 0.916             | 0.916    | 0.914    | 0.902                | 0.929       | 0.926           | 88.6 | 94.6 | 7.2  | 9.6  | 0.908 | 14.759 | 0.108 | 0.968   | 0.97    | 0.97    |
| Extreme Gradient Boosting  | 0.913             | 0.914    | 0.911    | 0.906                | 0.92        | 0.917           | 89.0 | 93.7 | 8.1  | 9.2  | 0.911 | 10.857 | 0.104 | 0.963   | 0.965   | 0.965   |
| Genetic Programming        | 0.523             | 0.522    | 0.524    | 0.535                | 0.511       | 0.514           | 52.5 | 52.0 | 49.8 | 45.7 | 0.532 | 1.1    | 0.917 | 0.523   | 0.638   | 0.503   |
| Gradient Boosting          | 0.909             | 0.909    | 0.908    | 0.905                | 0.913       | 0.911           | 88.9 | 92.9 | 8.9  | 9.3  | 0.908 | 10.868 | 0.107 | 0.952   | 0.948   | 0.946   |
| K-Nearest Neighbors        | 0.728             | 0.728    | 0.717    | 0.702                | 0.753       | 0.734           | 68.9 | 76.7 | 25.1 | 29.3 | 0.724 | 2.952  | 0.399 | 0.809   | 0.802   | 0.805   |
| Light Gradient Boosting    | 0.916             | 0.916    | 0.915    | 0.912                | 0.92        | 0.918           | 89.6 | 93.7 | 8.1  | 8.6  | 0.916 | 22.826 | 0.098 | 0.966   | 0.966   | 0.966   |
| Logistic Regression        | 0.575             | 0.576    | 0.564    | 0.56                 | 0.59        | 0.572           | 55.0 | 60.1 | 41.7 | 43.2 | 0.581 | 1.431  | 0.754 | 0.611   | 0.598   | 0.603   |
| Naive Bayes                | 0.58              | 0.58     | 0.561    | 0.547                | 0.613       | 0.579           | 53.7 | 62.4 | 39.4 | 44.5 | 0.583 | 1.462  | 0.746 | 0.616   | 0.601   | 0.607   |
| Random Forest              | 0.888             | 0.888    | 0.886    | 0.883                | 0.894       | 0.89            | 86.7 | 91.0 | 10.8 | 11.5 | 0.888 | 10.348 | 0.133 | 0.949   | 0.949   | 0.949   |
| Support Vector Machine     | 0.807             | 0.808    | 0.802    | 0.794                | 0.82        | 0.81            | 78.0 | 83.5 | 18.3 | 20.2 | 0.806 | 4.589  | 0.251 | 0.877   | 0.87    | 0.871   |

## D4 = D\_37\_bit\_muxliplexer\_5000\_01

| ML Algorithm               | Balanced Accuracy | Accuracy | F1 Score | Sensitivity (Recall) | Specificity | Precision (PPV) | TP    | TN    | FP    | FN    | NPV   | LR+   | LR-   | ROC AUC | PRC AUC | PRC APS |
|----------------------------|-------------------|----------|----------|----------------------|-------------|-----------------|-------|-------|-------|-------|-------|-------|-------|---------|---------|---------|
| Artificial Neural Network  | 0.654             | 0.654    | 0.645    | 0.633                | 0.675       | 0.658           | 156.9 | 170.3 | 81.9  | 90.9  | 0.652 | 1.98  | 0.546 | 0.705   | 0.69    | 0.692   |
| Category Gradient Boosting | 0.75              | 0.751    | 0.743    | 0.73                 | 0.771       | 0.758           | 180.9 | 194.4 | 57.8  | 66.9  | 0.745 | 3.336 | 0.354 | 0.831   | 0.827   | 0.828   |
| Decision Tree              | 0.578             | 0.578    | 0.566    | 0.556                | 0.599       | 0.577           | 137.8 | 151.1 | 101.1 | 110.0 | 0.579 | 1.398 | 0.744 | 0.611   | 0.631   | 0.603   |
| Elastic Net                | 0.549             | 0.549    | 0.54     | 0.534                | 0.563       | 0.547           | 132.3 | 142.1 | 110.1 | 115.5 | 0.551 | 1.238 | 0.833 | 0.572   | 0.565   | 0.568   |
| ExSTraCS                   | 0.885             | 0.885    | 0.884    | 0.877                | 0.893       | 0.891           | 217.4 | 225.3 | 26.9  | 30.4  | 0.881 | 9.289 | 0.138 | 0.938   | 0.926   | 0.927   |
| Extreme Gradient Boosting  | 0.819             | 0.82     | 0.816    | 0.809                | 0.83        | 0.824           | 200.4 | 209.4 | 42.8  | 47.4  | 0.816 | 4.865 | 0.231 | 0.9     | 0.896   | 0.897   |
| Genetic Programming        | 0.523             | 0.523    | 0.513    | 0.507                | 0.538       | 0.518           | 125.7 | 135.7 | 116.5 | 122.1 | 0.527 | 1.104 | 0.92  | 0.523   | 0.635   | 0.508   |
| Gradient Boosting          | 0.825             | 0.825    | 0.822    | 0.816                | 0.835       | 0.829           | 202.2 | 210.5 | 41.7  | 45.6  | 0.823 | 5.07  | 0.221 | 0.899   | 0.893   | 0.894   |
| K-Nearest Neighbors        | 0.624             | 0.624    | 0.613    | 0.601                | 0.647       | 0.626           | 148.9 | 163.2 | 89.0  | 98.9  | 0.623 | 1.711 | 0.618 | 0.667   | 0.654   | 0.656   |
| Light Gradient Boosting    | 0.862             | 0.862    | 0.861    | 0.858                | 0.866       | 0.863           | 212.7 | 218.5 | 33.7  | 35.1  | 0.862 | 6.591 | 0.164 | 0.937   | 0.936   | 0.936   |
| Logistic Regression        | 0.545             | 0.546    | 0.535    | 0.528                | 0.563       | 0.543           | 130.8 | 142.0 | 110.2 | 117.0 | 0.548 | 1.22  | 0.844 | 0.57    | 0.56    | 0.562   |
| Naive Bayes                | 0.551             | 0.551    | 0.538    | 0.527                | 0.574       | 0.549           | 130.6 | 144.8 | 107.4 | 117.2 | 0.552 | 1.252 | 0.83  | 0.572   | 0.563   | 0.566   |
| Random Forest              | 0.744             | 0.744    | 0.735    | 0.717                | 0.77        | 0.754           | 177.7 | 194.2 | 58.0  | 70.1  | 0.735 | 3.152 | 0.368 | 0.817   | 0.811   | 0.811   |
| Support Vector Machine     | 0.657             | 0.657    | 0.649    | 0.64                 | 0.673       | 0.658           | 158.6 | 169.8 | 82.4  | 89.2  | 0.656 | 1.965 | 0.535 | 0.712   | 0.7     | 0.701   |

## D5 = E\_70\_bit\_muxliplexer\_10000\_01

| ML Algorithm               | Balanced Accuracy | Accuracy | F1 Score | Sensitivity (Recall) | Specificity | Precision (PPV) | TP    | TN    | FP    | FN    | NPV   | LR+   | LR-   | ROC AUC | PRC AUC | PRC APS |
|----------------------------|-------------------|----------|----------|----------------------|-------------|-----------------|-------|-------|-------|-------|-------|-------|-------|---------|---------|---------|
| Artificial Neural Network  | 0.551             | 0.552    | 0.55     | 0.55                 | 0.553       | 0.55            | 274.2 | 277.3 | 223.8 | 224.7 | 0.553 | 1.232 | 0.815 | 0.575   | 0.567   | 0.568   |
| Category Gradient Boosting | 0.579             | 0.579    | 0.575    | 0.571                | 0.587       | 0.579           | 284.8 | 294.2 | 206.9 | 214.1 | 0.579 | 1.396 | 0.735 | 0.611   | 0.601   | 0.602   |
| Decision Tree              | 0.539             | 0.539    | 0.533    | 0.527                | 0.552       | 0.54            | 263.0 | 276.4 | 224.7 | 235.9 | 0.539 | 1.182 | 0.86  | 0.551   | 0.558   | 0.554   |
| Elastic Net                | 0.539             | 0.539    | 0.536    | 0.534                | 0.545       | 0.539           | 266.3 | 273.1 | 228.0 | 232.6 | 0.54  | 1.175 | 0.856 | 0.559   | 0.556   | 0.557   |
| ExSTraCS                   | 0.857             | 0.857    | 0.857    | 0.861                | 0.852       | 0.854           | 429.6 | 427.0 | 74.1  | 69.3  | 0.86  | 7.074 | 0.169 | 0.908   | 0.888   | 0.888   |
| Extreme Gradient Boosting  | 0.612             | 0.612    | 0.612    | 0.613                | 0.612       | 0.612           | 305.6 | 306.9 | 194.2 | 193.3 | 0.614 | 1.588 | 0.634 | 0.66    | 0.653   | 0.653   |
| Genetic Programming        | 0.509             | 0.51     | 0.459    | 0.461                | 0.558       | 0.458           | 229.8 | 279.7 | 221.4 | 269.1 | 0.511 | 0.941 | 0.966 | 0.509   | 0.644   | 0.504   |
| Gradient Boosting          | 0.612             | 0.612    | 0.611    | 0.61                 | 0.614       | 0.612           | 304.5 | 307.8 | 193.3 | 194.4 | 0.613 | 1.592 | 0.636 | 0.657   | 0.647   | 0.648   |
| K-Nearest Neighbors        | 0.571             | 0.571    | 0.57     | 0.569                | 0.574       | 0.571           | 283.9 | 287.5 | 213.6 | 215.0 | 0.572 | 1.338 | 0.752 | 0.601   | 0.589   | 0.589   |
| Light Gradient Boosting    | 0.635             | 0.635    | 0.635    | 0.636                | 0.634       | 0.634           | 317.3 | 317.6 | 183.5 | 181.6 | 0.636 | 1.752 | 0.577 | 0.688   | 0.677   | 0.678   |
| Logistic Regression        | 0.541             | 0.541    | 0.531    | 0.524                | 0.558       | 0.543           | 261.3 | 279.8 | 221.3 | 227.6 | 0.541 | 1.199 | 0.854 | 0.559   | 0.556   | 0.55    |

# Average Model Prediction Statistics (Rounded to 3 Decimal Points): Page 2

## D6 = F\_135\_bit\_muxlexer\_20000\_01

| ML Algorithm               | Balanced Accuracy | Accuracy | F1 Score | Sensitivity (Recall) | Specificity | Precision (PPV) | TP    | TN    | FP    | FN    | NPV   | LR+   | LR-   | ROC AUC | PRC AUC | PRC APS |
|----------------------------|-------------------|----------|----------|----------------------|-------------|-----------------|-------|-------|-------|-------|-------|-------|-------|---------|---------|---------|
| Artificial Neural Network  | 0.529             | 0.529    | 0.528    | 0.532                | 0.526       | 0.525           | 528.3 | 529.5 | 477.8 | 464.4 | 0.533 | 1.123 | 0.89  | 0.539   | 0.529   | 0.53    |
| Category Gradient Boosting | 0.522             | 0.522    | 0.46     | 0.41                 | 0.633       | 0.524           | 406.9 | 638.1 | 369.2 | 585.8 | 0.521 | 1.121 | 0.932 | 0.535   | 0.524   | 0.525   |
| Decision Tree              | 0.503             | 0.503    | 0.492    | 0.486                | 0.519       | 0.499           | 482.4 | 523.1 | 484.2 | 510.3 | 0.506 | 1.012 | 0.991 | 0.505   | 0.522   | 0.502   |
| Elastic Net                | 0.515             | 0.515    | 0.502    | 0.493                | 0.537       | 0.512           | 489.4 | 541.3 | 466.0 | 503.3 | 0.518 | 1.065 | 0.943 | 0.522   | 0.514   | 0.515   |
| ExSTraCS                   | 0.506             | 0.507    | 0.44     | 0.416                | 0.595       | 0.506           | 413.4 | 599.8 | 407.5 | 579.3 | 0.509 | 1.038 | 0.979 | 0.51    | 0.505   | 0.505   |
| Extreme Gradient Boosting  | 0.538             | 0.538    | 0.522    | 0.508                | 0.567       | 0.536           | 504.4 | 571.5 | 435.8 | 488.3 | 0.539 | 1.176 | 0.868 | 0.551   | 0.542   | 0.542   |
| Genetic Programming        | 0.502             | 0.502    | 0.497    | 0.497                | 0.507       | 0.498           | 493.1 | 510.7 | 496.6 | 499.6 | 0.506 | 1.008 | 0.993 | 0.502   | 0.622   | 0.497   |
| Gradient Boosting          | 0.527             | 0.527    | 0.518    | 0.513                | 0.541       | 0.524           | 508.8 | 545.0 | 462.3 | 483.9 | 0.53  | 1.118 | 0.901 | 0.537   | 0.529   | 0.53    |
| K-Nearest Neighbors        | 0.528             | 0.528    | 0.512    | 0.499                | 0.556       | 0.526           | 495.8 | 560.1 | 447.2 | 496.9 | 0.53  | 1.126 | 0.901 | 0.537   | 0.526   | 0.525   |
| Light Gradient Boosting    | 0.537             | 0.537    | 0.529    | 0.525                | 0.548       | 0.534           | 521.2 | 552.1 | 455.2 | 471.5 | 0.54  | 1.162 | 0.867 | 0.554   | 0.545   | 0.546   |
| Logistic Regression        | 0.52              | 0.52     | 0.492    | 0.475                | 0.564       | 0.519           | 471.8 | 568.3 | 439.0 | 520.9 | 0.522 | 1.095 | 0.929 | 0.526   | 0.516   | 0.517   |
| Naive Bayes                | 0.517             | 0.517    | 0.5      | 0.487                | 0.546       | 0.514           | 483.9 | 549.6 | 457.7 | 508.8 | 0.519 | 1.073 | 0.94  | 0.525   | 0.517   | 0.517   |
| Random Forest              | 0.528             | 0.528    | 0.513    | 0.503                | 0.553       | 0.525           | 499.3 | 556.9 | 450.4 | 493.4 | 0.531 | 1.124 | 0.898 | 0.543   | 0.532   | 0.533   |
| Support Vector Machine     | 0.539             | 0.539    | 0.536    | 0.536                | 0.543       | 0.536           | 531.7 | 546.5 | 460.8 | 461.0 | 0.543 | 1.171 | 0.856 | 0.556   | 0.546   | 0.547   |

# Median Model Prediction Statistics (Rounded to 3 Decimal Points): Page 1

## D1 = A\_6\_bit\_muxliplexer\_500\_01

| ML Algorithm               | Balanced Accuracy | Accuracy | F1 Score | Sensitivity (Recall) | Specificity | Precision (PPV) | TP   | TN   | FP  | FN  | NPV   | LR+   | LR-   | ROC AUC | PRC AUC | PRC APS |
|----------------------------|-------------------|----------|----------|----------------------|-------------|-----------------|------|------|-----|-----|-------|-------|-------|---------|---------|---------|
| Artificial Neural Network  | 1.0               | 1.0      | 1.0      | 1.0                  | 1.0         | 1.0             | 25.0 | 25.0 | 0.0 | 0.0 | 1.0   | 0.0   | 0.0   | 1.0     | 1.0     | 1.0     |
| Category Gradient Boosting | 1.0               | 1.0      | 1.0      | 1.0                  | 1.0         | 1.0             | 25.0 | 25.0 | 0.0 | 0.0 | 1.0   | 0.0   | 0.0   | 1.0     | 1.0     | 1.0     |
| Decision Tree              | 1.0               | 1.0      | 1.0      | 1.0                  | 1.0         | 1.0             | 25.0 | 25.0 | 0.0 | 0.0 | 1.0   | 0.0   | 0.0   | 1.0     | 1.0     | 1.0     |
| Elastic Net                | 0.68              | 0.68     | 0.681    | 0.694                | 0.647       | 0.673           | 17.0 | 16.5 | 9.0 | 7.5 | 0.688 | 2.062 | 0.467 | 0.77    | 0.758   | 0.753   |
| ExSTraCS                   | 1.0               | 1.0      | 1.0      | 1.0                  | 1.0         | 1.0             | 25.0 | 25.0 | 0.0 | 0.0 | 1.0   | 0.0   | 0.0   | 1.0     | 1.0     | 1.0     |
| Extreme Gradient Boosting  | 1.0               | 1.0      | 1.0      | 1.0                  | 1.0         | 1.0             | 25.0 | 25.0 | 0.0 | 0.0 | 1.0   | 0.0   | 0.0   | 1.0     | 1.0     | 1.0     |
| Genetic Programming        | 1.0               | 1.0      | 1.0      | 1.0                  | 1.0         | 1.0             | 24.0 | 25.0 | 0.0 | 0.0 | 1.0   | 0.0   | 0.0   | 1.0     | 1.0     | 1.0     |
| Gradient Boosting          | 1.0               | 1.0      | 1.0      | 1.0                  | 1.0         | 1.0             | 25.0 | 25.0 | 0.0 | 0.0 | 1.0   | 0.0   | 0.0   | 1.0     | 1.0     | 1.0     |
| K-Nearest Neighbors        | 1.0               | 1.0      | 1.0      | 1.0                  | 1.0         | 1.0             | 25.0 | 25.0 | 0.0 | 0.0 | 1.0   | 0.0   | 0.0   | 1.0     | 1.0     | 1.0     |
| Light Gradient Boosting    | 1.0               | 1.0      | 1.0      | 1.0                  | 1.0         | 1.0             | 25.0 | 25.0 | 0.0 | 0.0 | 1.0   | 0.0   | 0.0   | 1.0     | 1.0     | 1.0     |
| Logistic Regression        | 0.718             | 0.72     | 0.712    | 0.734                | 0.686       | 0.688           | 18.0 | 17.5 | 8.0 | 6.5 | 0.735 | 2.255 | 0.377 | 0.775   | 0.768   | 0.761   |
| Naive Bayes                | 0.721             | 0.72     | 0.72     | 0.729                | 0.725       | 0.7             | 17.5 | 18.5 | 7.0 | 6.5 | 0.732 | 2.501 | 0.381 | 0.776   | 0.758   | 0.769   |
| Random Forest              | 1.0               | 1.0      | 1.0      | 1.0                  | 1.0         | 1.0             | 25.0 | 25.0 | 0.0 | 0.0 | 1.0   | 0.0   | 0.0   | 1.0     | 1.0     | 1.0     |
| Support Vector Machine     | 1.0               | 1.0      | 1.0      | 1.0                  | 1.0         | 1.0             | 25.0 | 25.0 | 0.0 | 0.0 | 1.0   | 0.0   | 0.0   | 1.0     | 1.0     | 1.0     |

## D2 = B\_11\_bit\_muxliplexer\_1000\_01

| ML Algorithm               | Balanced Accuracy | Accuracy | F1 Score | Sensitivity (Recall) | Specificity | Precision (PPV) | TP   | TN   | FP   | FN   | NPV   | LR+    | LR-   | ROC AUC | PRC AUC | PRC APS |
|----------------------------|-------------------|----------|----------|----------------------|-------------|-----------------|------|------|------|------|-------|--------|-------|---------|---------|---------|
| Artificial Neural Network  | 0.895             | 0.895    | 0.896    | 0.91                 | 0.889       | 0.888           | 45.5 | 44.0 | 5.5  | 4.5  | 0.906 | 7.95   | 0.104 | 0.96    | 0.959   | 0.96    |
| Category Gradient Boosting | 0.915             | 0.915    | 0.914    | 0.911                | 0.929       | 0.929           | 46.0 | 46.0 | 3.5  | 4.5  | 0.909 | 8.439  | 0.098 | 0.983   | 0.985   | 0.985   |
| Decision Tree              | 0.915             | 0.915    | 0.915    | 0.91                 | 0.929       | 0.927           | 45.5 | 46.0 | 3.5  | 4.5  | 0.911 | 11.375 | 0.098 | 0.942   | 0.955   | 0.919   |
| Elastic Net                | 0.599             | 0.6      | 0.612    | 0.614                | 0.62        | 0.6             | 31.0 | 31.0 | 19.0 | 19.5 | 0.59  | 1.469  | 0.667 | 0.65    | 0.643   | 0.65    |
| ExSTraCS                   | 0.905             | 0.905    | 0.904    | 0.901                | 0.919       | 0.922           | 45.5 | 45.5 | 4.0  | 5.0  | 0.899 | 8.92   | 0.11  | 0.97    | 0.968   | 0.968   |
| Extreme Gradient Boosting  | 0.89              | 0.89     | 0.891    | 0.891                | 0.919       | 0.916           | 45.0 | 45.5 | 4.0  | 5.5  | 0.889 | 7.638  | 0.123 | 0.972   | 0.974   | 0.974   |
| Genetic Programming        | 0.57              | 0.57     | 0.59     | 0.594                | 0.51        | 0.559           | 30.0 | 25.0 | 24.0 | 20.5 | 0.568 | 1.265  | 0.746 | 0.59    | 0.638   | 0.56    |
| Gradient Boosting          | 0.915             | 0.915    | 0.914    | 0.9                  | 0.929       | 0.925           | 45.0 | 45.5 | 3.5  | 5.0  | 0.903 | 9.304  | 0.108 | 0.981   | 0.983   | 0.983   |
| K-Nearest Neighbors        | 0.871             | 0.87     | 0.867    | 0.861                | 0.869       | 0.875           | 43.5 | 43.0 | 6.5  | 7.0  | 0.858 | 6.725  | 0.162 | 0.923   | 0.931   | 0.906   |
| Light Gradient Boosting    | 0.91              | 0.91     | 0.907    | 0.891                | 0.929       | 0.93            | 45.0 | 46.0 | 3.5  | 5.5  | 0.89  | 7.542  | 0.121 | 0.979   | 0.982   | 0.982   |
| Logistic Regression        | 0.591             | 0.59     | 0.606    | 0.624                | 0.61        | 0.602           | 31.5 | 30.5 | 19.5 | 19.0 | 0.59  | 1.492  | 0.679 | 0.646   | 0.645   | 0.651   |
| Naive Bayes                | 0.601             | 0.6      | 0.611    | 0.624                | 0.6         | 0.606           | 31.5 | 30.0 | 20.0 | 19.0 | 0.598 | 1.539  | 0.659 | 0.644   | 0.641   | 0.647   |
| Random Forest              | 0.915             | 0.915    | 0.914    | 0.9                  | 0.919       | 0.921           | 45.0 | 45.5 | 4.0  | 5.0  | 0.903 | 7.99   | 0.108 | 0.981   | 0.982   | 0.983   |
| Support Vector Machine     | 0.9               | 0.9      | 0.9      | 0.9                  | 0.918       | 0.921           | 45.0 | 45.0 | 4.0  | 5.0  | 0.896 | 10.328 | 0.117 | 0.954   | 0.957   | 0.958   |

## D3 = C\_20\_bit\_muxliplexer\_2000\_01

| ML Algorithm               | Balanced Accuracy | Accuracy | F1 Score | Sensitivity (Recall) | Specificity | Precision (PPV) | TP   | TN   | FP   | FN   | NPV   | LR+    | LR-   | ROC AUC | PRC AUC | PRC APS |
|----------------------------|-------------------|----------|----------|----------------------|-------------|-----------------|------|------|------|------|-------|--------|-------|---------|---------|---------|
| Artificial Neural Network  | 0.813             | 0.812    | 0.81     | 0.803                | 0.823       | 0.809           | 79.5 | 83.5 | 18.0 | 19.5 | 0.815 | 4.423  | 0.234 | 0.893   | 0.892   | 0.893   |
| Category Gradient Boosting | 0.925             | 0.925    | 0.923    | 0.909                | 0.931       | 0.929           | 89.5 | 94.5 | 7.0  | 9.0  | 0.914 | 12.042 | 0.097 | 0.969   | 0.972   | 0.972   |
| Decision Tree              | 0.76              | 0.76     | 0.759    | 0.776                | 0.725       | 0.725           | 76.0 | 74.0 | 28.0 | 22.0 | 0.768 | 2.715  | 0.313 | 0.787   | 0.825   | 0.736   |
| Elastic Net                | 0.585             | 0.585    | 0.579    | 0.589                | 0.576       | 0.572           | 58.0 | 58.5 | 43.0 | 40.5 | 0.593 | 1.393  | 0.715 | 0.614   | 0.59    | 0.597   |
| ExSTraCS                   | 0.917             | 0.918    | 0.913    | 0.898                | 0.936       | 0.933           | 88.0 | 95.5 | 6.5  | 10.0 | 0.904 | 11.928 | 0.11  | 0.97    | 0.976   | 0.976   |
| Extreme Gradient Boosting  | 0.92              | 0.92     | 0.918    | 0.908                | 0.926       | 0.924           | 89.0 | 94.5 | 7.5  | 9.0  | 0.912 | 10.95  | 0.101 | 0.969   | 0.969   | 0.969   |
| Genetic Programming        | 0.52              | 0.52     | 0.519    | 0.533                | 0.515       | 0.51            | 52.5 | 52.5 | 49.5 | 46.0 | 0.53  | 1.085  | 0.922 | 0.52    | 0.634   | 0.5     |
| Gradient Boosting          | 0.915             | 0.915    | 0.914    | 0.913                | 0.926       | 0.922           | 89.5 | 94.0 | 7.5  | 8.5  | 0.918 | 10.307 | 0.094 | 0.961   | 0.955   | 0.953   |
| K-Nearest Neighbors        | 0.73              | 0.73     | 0.724    | 0.704                | 0.754       | 0.733           | 69.0 | 76.5 | 25.0 | 29.0 | 0.735 | 2.829  | 0.375 | 0.825   | 0.814   | 0.818   |
| Light Gradient Boosting    | 0.92              | 0.92     | 0.917    | 0.913                | 0.931       | 0.927           | 89.5 | 94.5 | 7.0  | 8.5  | 0.916 | 13.178 | 0.095 | 0.972   | 0.969   | 0.97    |
| Logistic Regression        | 0.576             | 0.577    | 0.571    | 0.574                | 0.564       | 0.564           | 56.5 | 57.5 | 44.5 | 42.0 | 0.58  | 1.35   | 0.753 | 0.608   | 0.583   | 0.59    |
| Naive Bayes                | 0.583             | 0.582    | 0.567    | 0.548                | 0.588       | 0.571           | 54.0 | 60.0 | 42.0 | 44.5 | 0.59  | 1.383  | 0.715 | 0.613   | 0.588   | 0.595   |
| Random Forest              | 0.885             | 0.885    | 0.884    | 0.883                | 0.897       | 0.891           | 87.0 | 91.5 | 10.5 | 11.5 | 0.89  | 8.487  | 0.127 | 0.952   | 0.952   | 0.953   |
| Support Vector Machine     | 0.818             | 0.817    | 0.81     | 0.806                | 0.814       | 0.806           | 79.0 | 83.0 | 19.0 | 19.0 | 0.814 | 4.331  | 0.238 | 0.881   | 0.881   | 0.882   |

## D4 = D\_37\_bit\_muxliplexer\_5000\_01

| ML Algorithm               | Balanced Accuracy | Accuracy | F1 Score | Sensitivity (Recall) | Specificity | Precision (PPV) | TP    | TN    | FP    | FN    | NPV   | LR+   | LR-   | ROC AUC | PRC AUC | PRC APS |
|----------------------------|-------------------|----------|----------|----------------------|-------------|-----------------|-------|-------|-------|-------|-------|-------|-------|---------|---------|---------|
| Artificial Neural Network  | 0.66              | 0.66     | 0.646    | 0.635                | 0.689       | 0.663           | 157.5 | 174.0 | 78.5  | 90.5  | 0.653 | 2.001 | 0.54  | 0.71    | 0.685   | 0.686   |
| Category Gradient Boosting | 0.751             | 0.751    | 0.741    | 0.722                | 0.76        | 0.754           | 179.0 | 191.5 | 60.5  | 69.0  | 0.74  | 3.107 | 0.359 | 0.823   | 0.827   | 0.828   |
| Decision Tree              | 0.578             | 0.578    | 0.568    | 0.562                | 0.601       | 0.576           | 139.5 | 151.5 | 100.5 | 108.5 | 0.58  | 1.386 | 0.739 | 0.605   | 0.632   | 0.603   |
| Elastic Net                | 0.544             | 0.544    | 0.542    | 0.54                 | 0.554       | 0.54            | 134.0 | 139.5 | 112.5 | 114.0 | 0.548 | 1.196 | 0.839 | 0.575   | 0.571   | 0.574   |
| ExSTraCS                   | 0.89              | 0.89     | 0.889    | 0.883                | 0.885       | 0.883           | 218.5 | 223.5 | 29.0  | 29.0  | 0.889 | 7.68  | 0.128 | 0.939   | 0.926   | 0.926   |
| Extreme Gradient Boosting  | 0.818             | 0.818    | 0.813    | 0.815                | 0.837       | 0.827           | 202.0 | 211.0 | 41.0  | 46.0  | 0.819 | 4.874 | 0.225 | 0.897   | 0.893   | 0.894   |
| Genetic Programming        | 0.524             | 0.524    | 0.515    | 0.505                | 0.538       | 0.519           | 125.0 | 135.5 | 116.5 | 122.5 | 0.528 | 1.101 | 0.911 | 0.524   | 0.636   | 0.508   |
| Gradient Boosting          | 0.825             | 0.825    | 0.825    | 0.827                | 0.827       | 0.819           | 205.0 | 208.5 | 43.5  | 43.0  | 0.829 | 4.606 | 0.21  | 0.899   | 0.895   | 0.895   |
| K-Nearest Neighbors        | 0.623             | 0.623    | 0.613    | 0.6                  | 0.649       | 0.625           | 148.5 | 164.0 | 88.5  | 99.0  | 0.621 | 1.696 | 0.62  | 0.663   | 0.656   | 0.658   |
| Light Gradient Boosting    | 0.858             | 0.858    | 0.857    | 0.859                | 0.867       | 0.859           | 213.0 | 219.0 | 33.5  | 35.0  | 0.862 | 6.241 | 0.163 | 0.94    | 0.938   | 0.938   |
| Logistic Regression        | 0.544             | 0.544    | 0.532    | 0.522                | 0.565       | 0.542           | 129.5 | 142.5 | 109.5 | 118.5 | 0.546 | 1.202 | 0.845 | 0.574   | 0.561   | 0.563   |
| Naive Bayes                | 0.548             | 0.548    | 0.543    | 0.538                | 0.572       | 0.545           | 133.5 | 144.5 | 108.0 | 114.5 | 0.551 | 1.216 | 0.827 | 0.574   | 0.562   | 0.565   |
| Random Forest              | 0.743             | 0.743    | 0.734    | 0.706                | 0.768       | 0.753           | 175.0 | 193.5 | 58.5  | 73.0  | 0.734 | 3.122 | 0.37  | 0.819   | 0.811   | 0.811   |
| Support Vector Machine     | 0.658             | 0.658    | 0.644    | 0.633                | 0.665       | 0.66            | 157.0 | 168.0 | 84.5  | 91.0  | 0.652 | 1.971 | 0.543 | 0.713   | 0.694   | 0.695   |

## D5 = E\_70\_bit\_muxliplexer\_10000\_01

| ML Algorithm               | Balanced Accuracy | Accuracy | F1 Score | Sensitivity (Recall) | Specificity | Precision (PPV) | TP      | TN    | FP    | FN    | NPV   | LR+   | LR-   | ROC AUC | PRC AUC | PRC APS |
|----------------------------|-------------------|----------|----------|----------------------|-------------|-----------------|---------|-------|-------|-------|-------|-------|-------|---------|---------|---------|
| Artificial Neural Network  | 0.551             | 0.551    | 0.551    | 0.552                | 0.556       | 0.549           | 275.5   | 278.5 | 222.5 | 223.5 | 0.552 | 1.225 | 0.814 | 0.579   | 0.563   | 0.564   |
| Category Gradient Boosting | 0.571             | 0.571    | 0.564    | 0.56                 | 0.584       | 0.572           | 279.5   | 292.5 | 208.5 | 219.5 | 0.569 | 1.346 | 0.76  | 0.6     | 0.588   | 0.589   |
| Decision Tree              | 0.541             | 0.542    | 0.532    | 0.53                 | 0.551       | 0.542           | 264.5   | 276.5 | 225.0 | 234.5 | 0.541 | 1.189 | 0.852 | 0.552   | 0.556   | 0.551   |
| Elastic Net                | 0.54              | 0.54     | 0.539    | 0.538                | 0.539       | 0.54            | 268.0   | 270.0 | 231.0 | 230.5 | 0.541 | 1.177 | 0.851 | 0.56    | 0.555   | 0.556   |
| ExSTraCS                   | 0.86              | 0.86     | 0.859    | 0.87                 | 0.864       | 0.865           | 434.0   | 433.0 | 68.0  | 65.0  | 0.867 | 6.468 | 0.154 | 0.911   | 0.9     | 0.901   |
| Extreme Gradient Boosting  | 0.609             | 0.609    | 0.608    | 0.609                | 0.61        | 0.61            | 304.0   | 305.5 | 195.5 | 195.0 | 0.61  | 1.572 | 0.642 | 0.663   | 0.656   | 0.657   |
| Genetic Programming        | 0.504             | 0.504    | 0.502    | 0.504                | 0.518       | 0.503           | 251.0   | 259.5 | 241.5 | 247.5 | 0.506 | 1.018 | 0.983 | 0.504   | 0.63    | 0.501   |
| Gradient Boosting          | 0.624             | 0.624    | 0.622    | 0.612                | 0.617       | 0.619           | 305.0   | 309.0 | 192.0 | 193.5 | 0.624 | 1.629 | 0.604 | 0.662   | 0.655   | 0.656   |
| K-Nearest Neighbors        | 0.57              | 0.569    | 0.568    | 0.567                | 0.574       | 0.568           | 283.0   | 287.5 | 213.5 | 216.0 | 0.571 | 1.325 | 0.757 | 0.601   | 0.587   | 0.589   |
| Light Gradient Boosting    | 0.635             | 0.635    | 0.632    | 0.633                | 0.645       | 0.637           | 316.0   | 323.0 | 178.0 | 183.0 | 0.633 | 1.76  | 0.581 | 0.689   | 0.669   | 0.67    |
| Logistic Regression        | 0.541             | 0.54     | 0.539    | 0.54                 | 0.544       | 0.54            | 269.0   | 272.5 | 228.5 | 229.5 | 0.542 | 1.18  | 0.849 | 0.56    | 0.555   | 0.557   |
| Naive Bayes                | 0.539             | 0.539    | 0.541    | 0.545                | 0.537       | 0.537           | 272.0</ |       |       |       |       |       |       |         |         |         |

# Median Model Prediction Statistics (Rounded to 3 Decimal Points): Page 2

## D6 = F\_135\_bit\_muxlexer\_20000\_01

| ML Algorithm               | Balanced Accuracy | Accuracy | F1 Score | Sensitivity (Recall) | Specificity | Precision (PPV) | TP    | TN    | FP    | FN    | NPV   | LR+   | LR-   | ROC AUC | PRC AUC | PRC APS |
|----------------------------|-------------------|----------|----------|----------------------|-------------|-----------------|-------|-------|-------|-------|-------|-------|-------|---------|---------|---------|
| Artificial Neural Network  | 0.53              | 0.53     | 0.531    | 0.539                | 0.521       | 0.526           | 534.5 | 524.5 | 482.5 | 458.0 | 0.534 | 1.124 | 0.885 | 0.541   | 0.53    | 0.53    |
| Category Gradient Boosting | 0.52              | 0.521    | 0.457    | 0.401                | 0.634       | 0.521           | 398.5 | 638.5 | 369.0 | 594.5 | 0.52  | 1.102 | 0.937 | 0.533   | 0.52    | 0.521   |
| Decision Tree              | 0.506             | 0.506    | 0.497    | 0.489                | 0.524       | 0.503           | 485.0 | 527.5 | 480.0 | 507.5 | 0.51  | 1.027 | 0.975 | 0.508   | 0.51    | 0.501   |
| Elastic Net                | 0.514             | 0.514    | 0.498    | 0.487                | 0.536       | 0.511           | 483.5 | 540.5 | 467.0 | 509.5 | 0.517 | 1.06  | 0.947 | 0.522   | 0.515   | 0.515   |
| ExSTraCS                   | 0.505             | 0.506    | 0.476    | 0.446                | 0.578       | 0.504           | 443.0 | 582.0 | 425.0 | 550.0 | 0.509 | 1.03  | 0.978 | 0.508   | 0.503   | 0.504   |
| Extreme Gradient Boosting  | 0.537             | 0.537    | 0.521    | 0.509                | 0.568       | 0.536           | 505.0 | 572.0 | 435.5 | 487.5 | 0.538 | 1.172 | 0.872 | 0.554   | 0.541   | 0.542   |
| Genetic Programming        | 0.5               | 0.5      | 0.497    | 0.498                | 0.509       | 0.496           | 494.5 | 512.5 | 495.0 | 498.5 | 0.504 | 0.999 | 1.001 | 0.5     | 0.621   | 0.496   |
| Gradient Boosting          | 0.523             | 0.523    | 0.51     | 0.506                | 0.54        | 0.52            | 502.5 | 544.0 | 463.0 | 490.5 | 0.525 | 1.099 | 0.917 | 0.534   | 0.529   | 0.53    |
| K-Nearest Neighbors        | 0.529             | 0.53     | 0.518    | 0.512                | 0.553       | 0.528           | 508.5 | 557.5 | 450.0 | 484.5 | 0.532 | 1.136 | 0.893 | 0.536   | 0.525   | 0.524   |
| Light Gradient Boosting    | 0.536             | 0.536    | 0.531    | 0.527                | 0.552       | 0.534           | 523.0 | 556.0 | 451.0 | 470.0 | 0.539 | 1.161 | 0.867 | 0.554   | 0.543   | 0.544   |
| Logistic Regression        | 0.521             | 0.522    | 0.504    | 0.499                | 0.531       | 0.52            | 495.0 | 535.5 | 472.5 | 497.5 | 0.523 | 1.099 | 0.927 | 0.526   | 0.516   | 0.517   |
| Naive Bayes                | 0.518             | 0.518    | 0.502    | 0.49                 | 0.543       | 0.515           | 486.5 | 547.0 | 460.0 | 506.5 | 0.52  | 1.078 | 0.937 | 0.525   | 0.516   | 0.517   |
| Random Forest              | 0.53              | 0.53     | 0.521    | 0.511                | 0.555       | 0.529           | 507.5 | 559.5 | 448.0 | 485.5 | 0.532 | 1.137 | 0.893 | 0.544   | 0.53    | 0.531   |
| Support Vector Machine     | 0.539             | 0.539    | 0.536    | 0.538                | 0.543       | 0.535           | 533.5 | 546.5 | 460.5 | 459.0 | 0.543 | 1.17  | 0.856 | 0.558   | 0.549   | 0.549   |

# Feature Importance Summary: D1 = A\_6\_bit\_mutlplexer\_500\_01

Sorted Median Mutual Information Scores

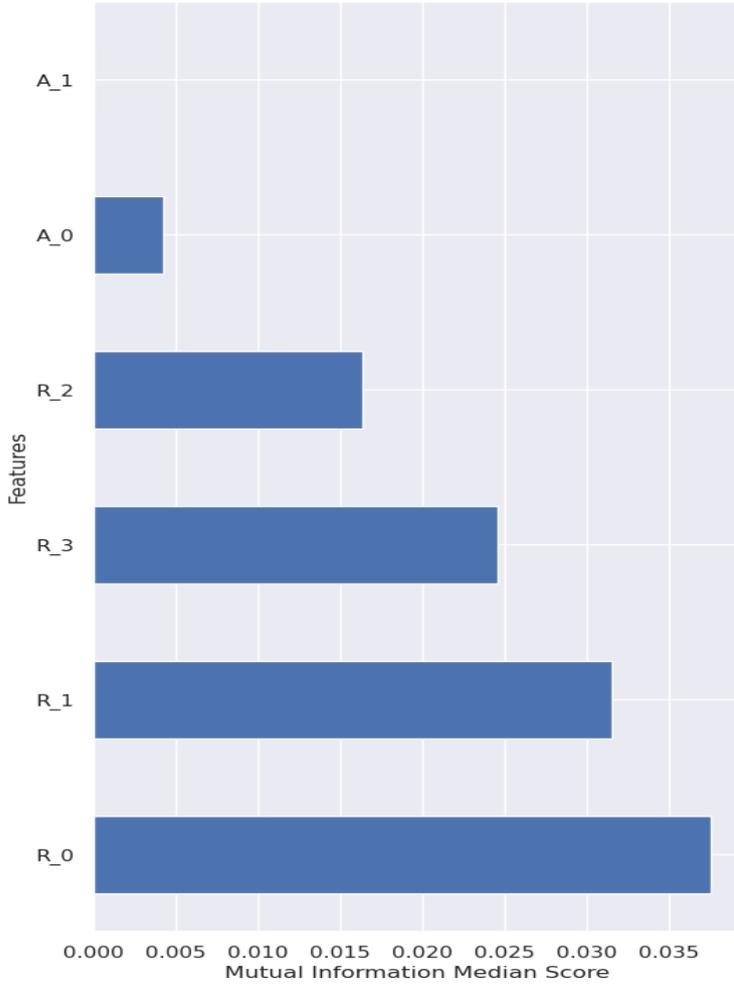

Sorted Median MultiSURF Scores

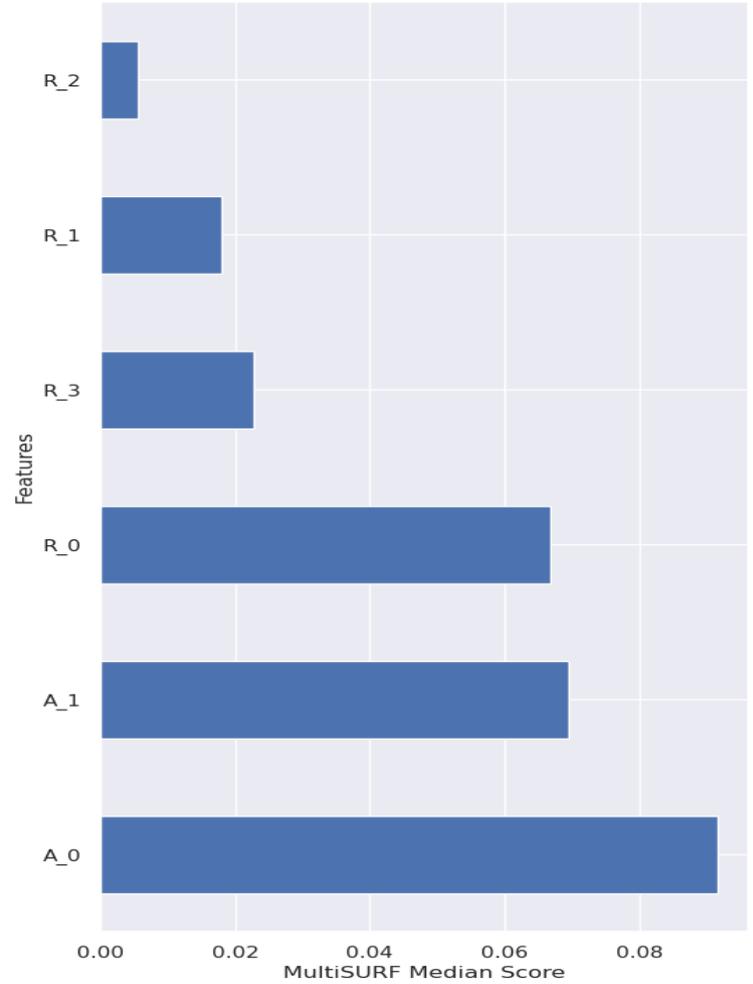

## Composite Feature Importance Plot (Normalized and Performance Weighted)

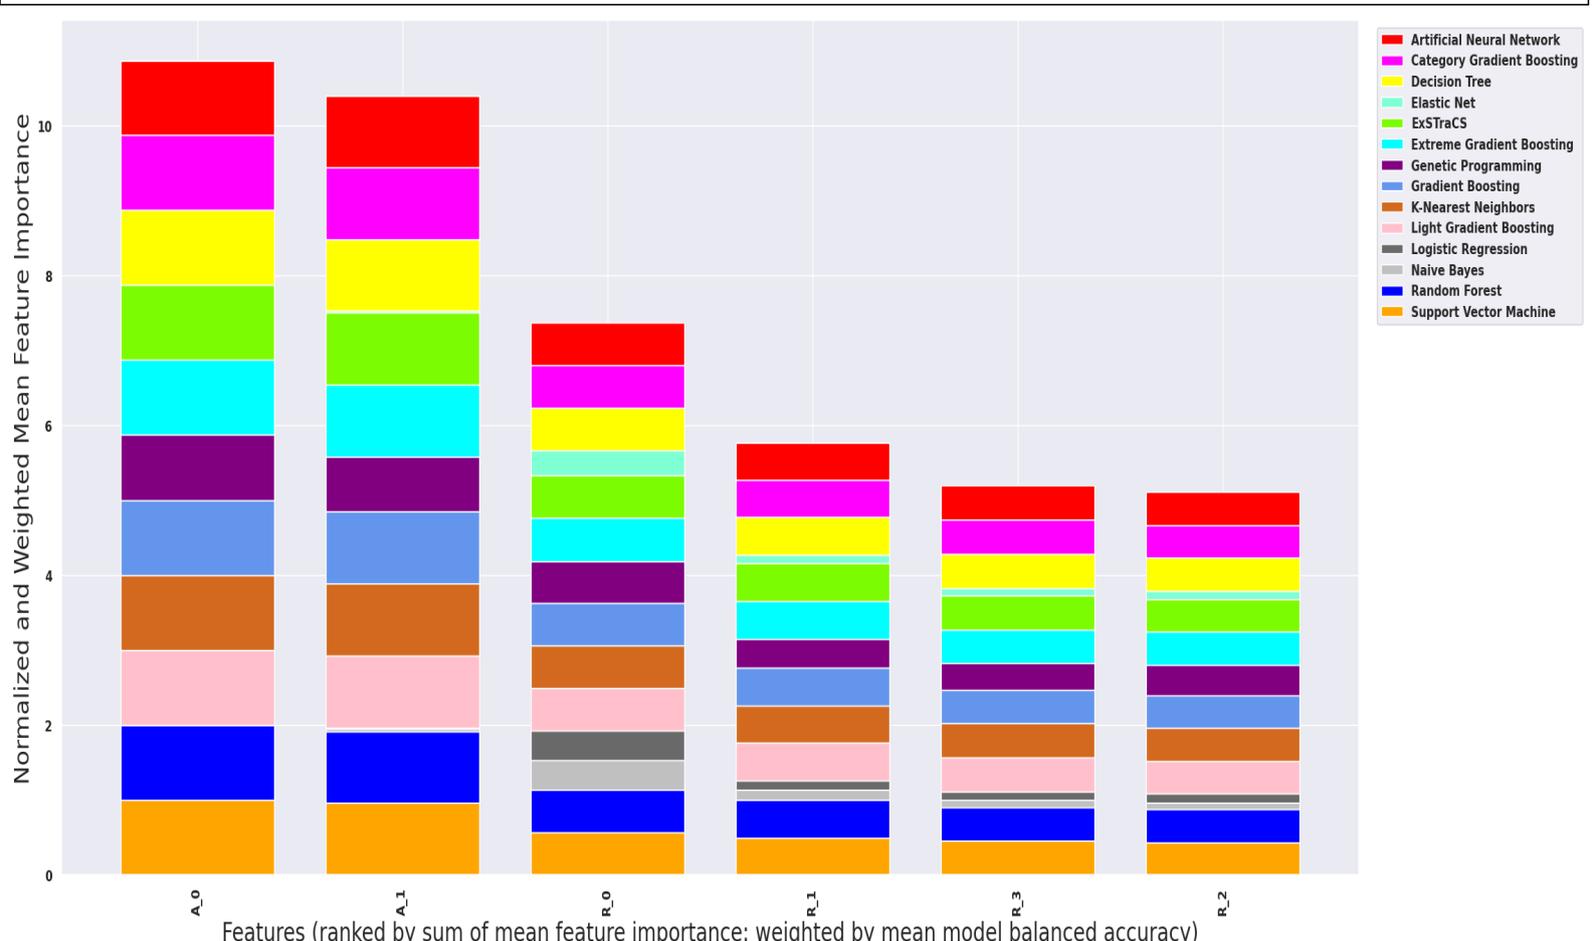

# Feature Importance Summary: D2 = B\_11\_bit\_mutliplexer\_1000\_01

Sorted Median Mutual Information Scores

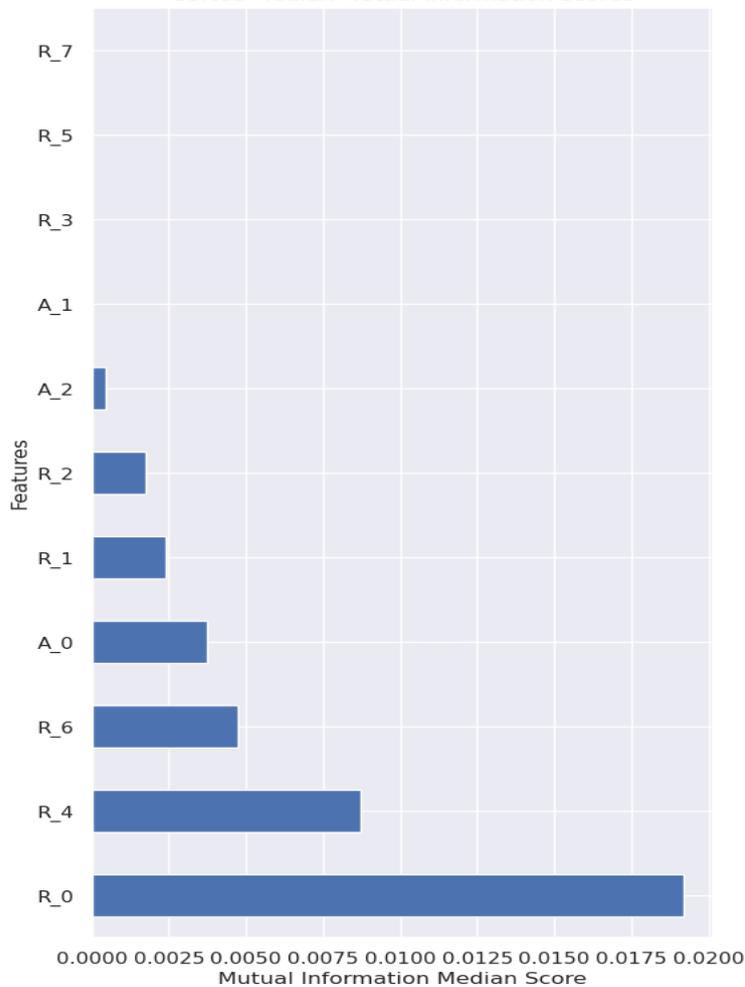

Sorted Median MultiSURF Scores

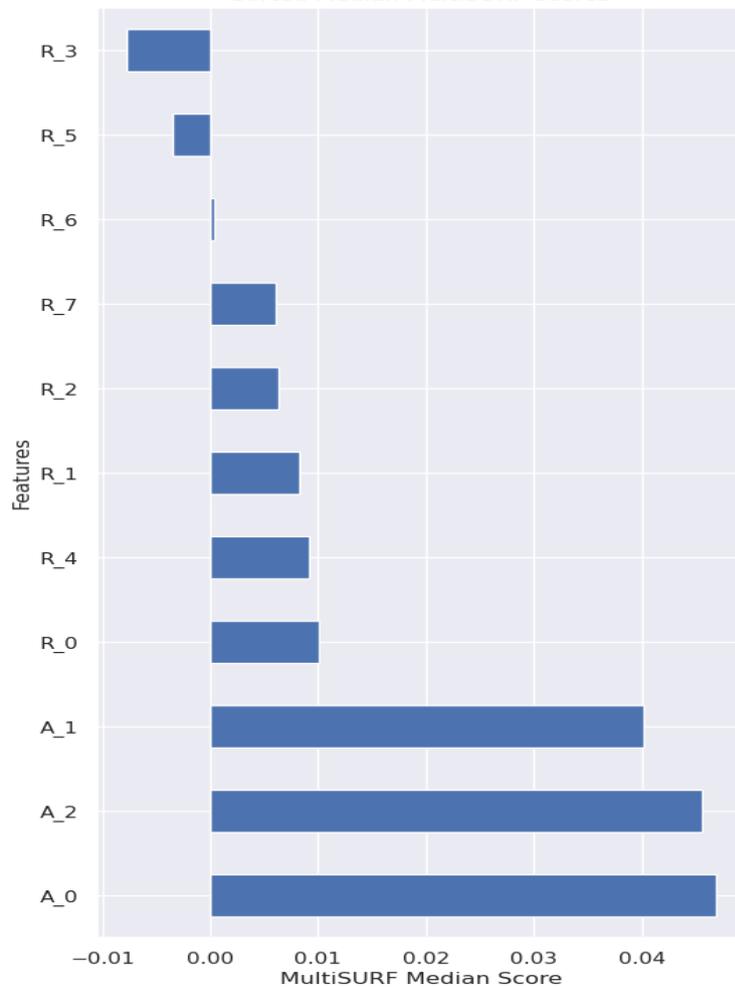

## Composite Feature Importance Plot (Normalized and Performance Weighted)

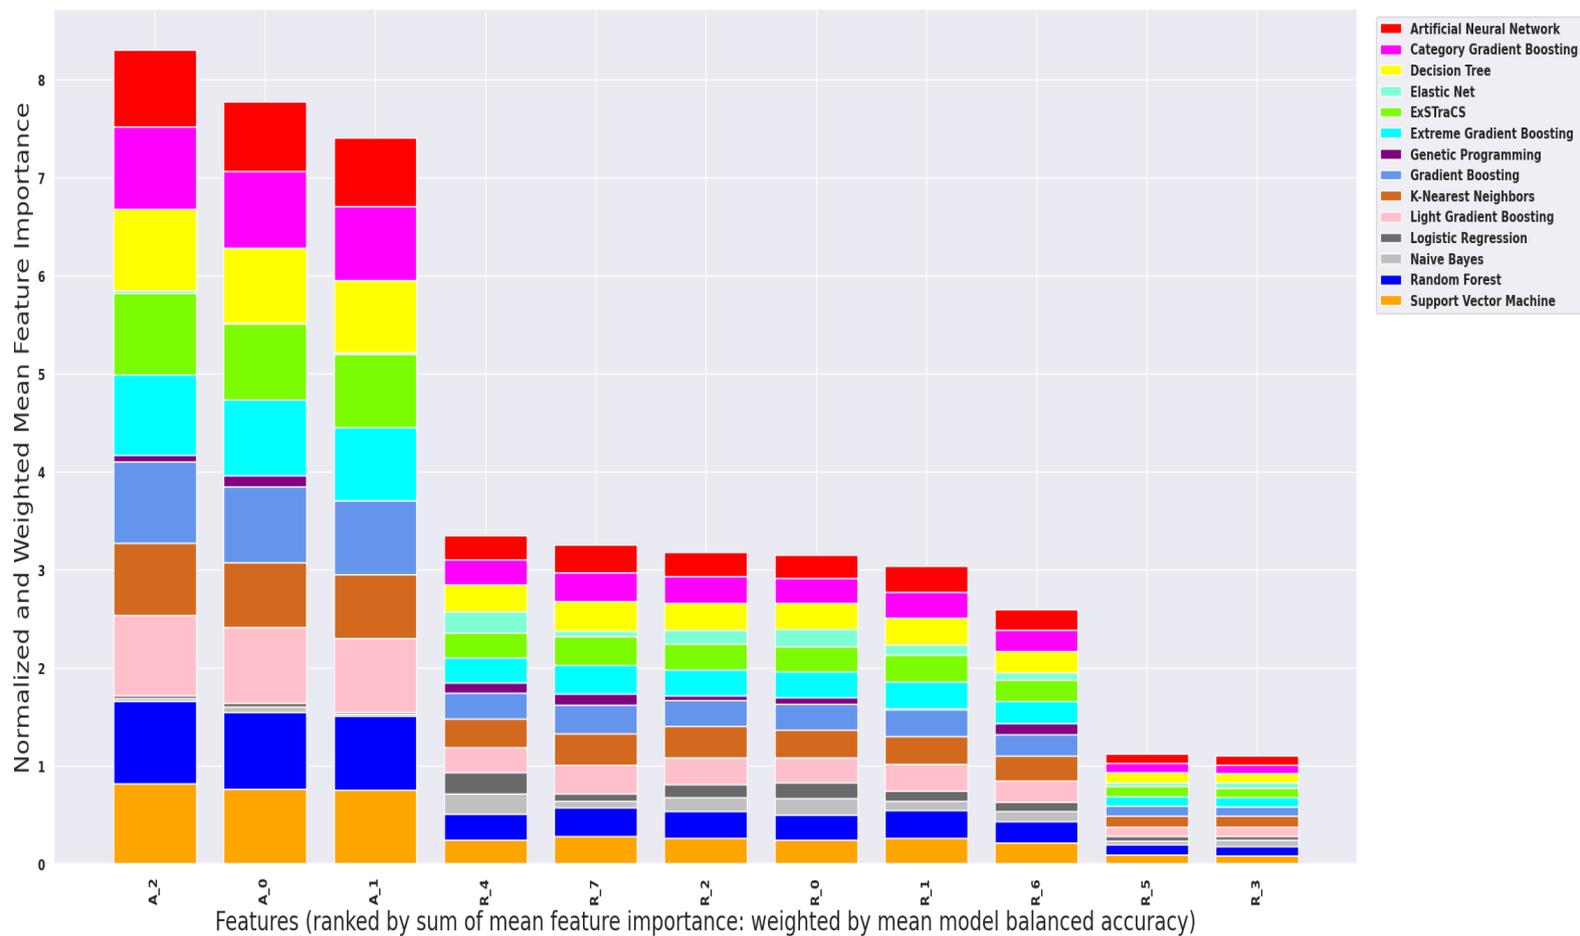

# Feature Importance Summary: D3 = C\_20\_bit\_mutliplexer\_2000\_01

Sorted Median Mutual Information Scores

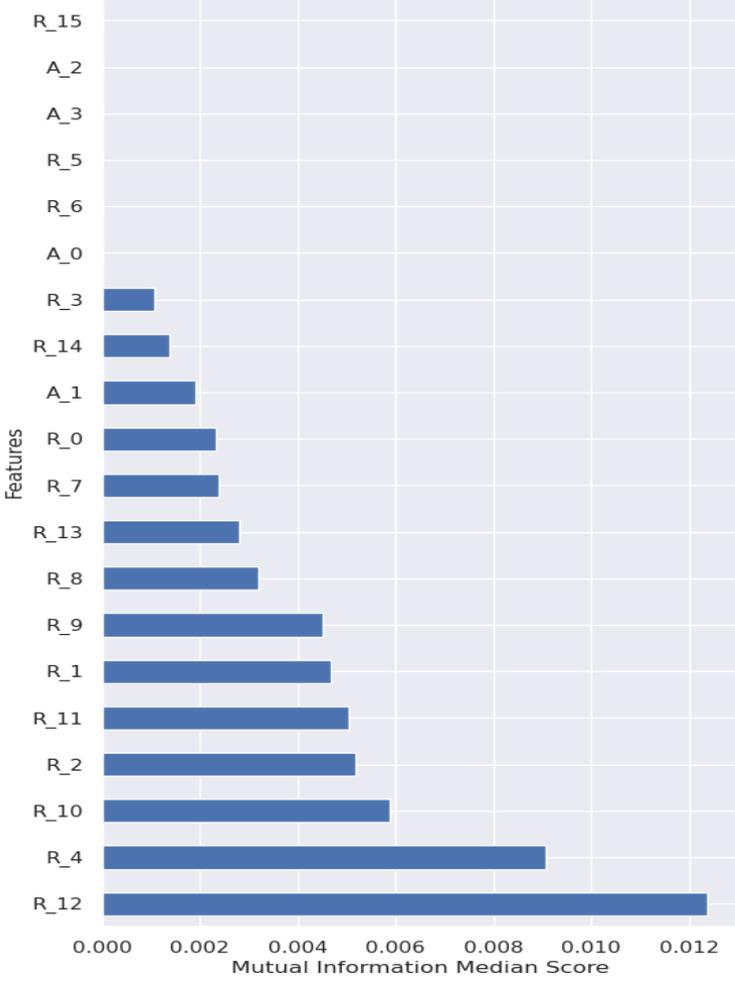

Sorted Median MultiSURF Scores

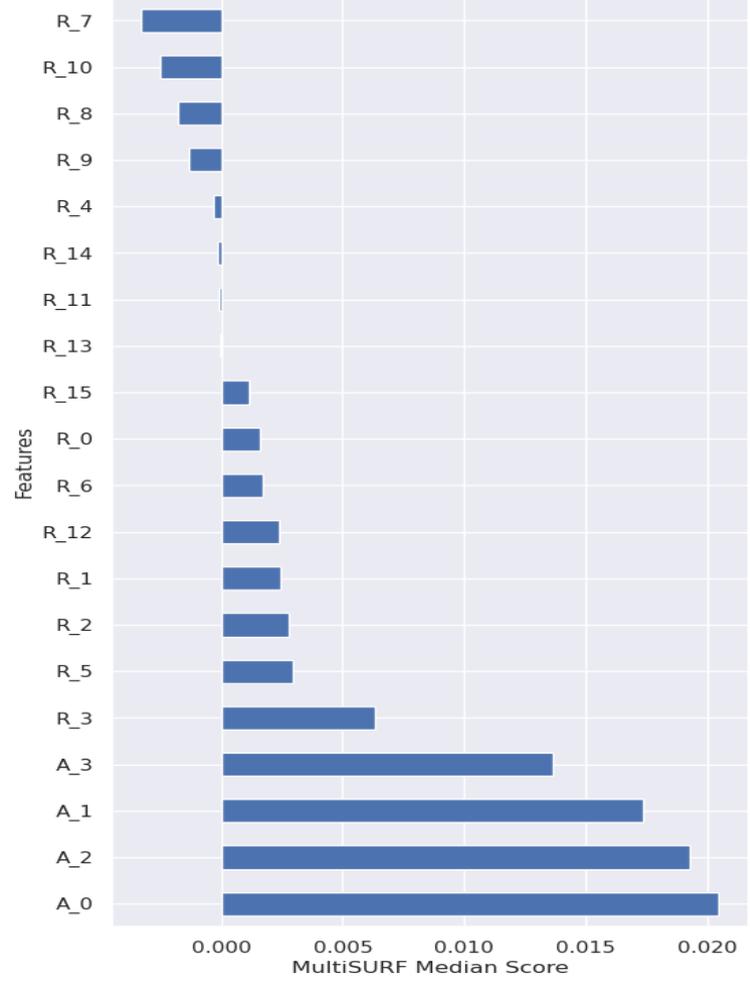

## Composite Feature Importance Plot (Normalized and Performance Weighted)

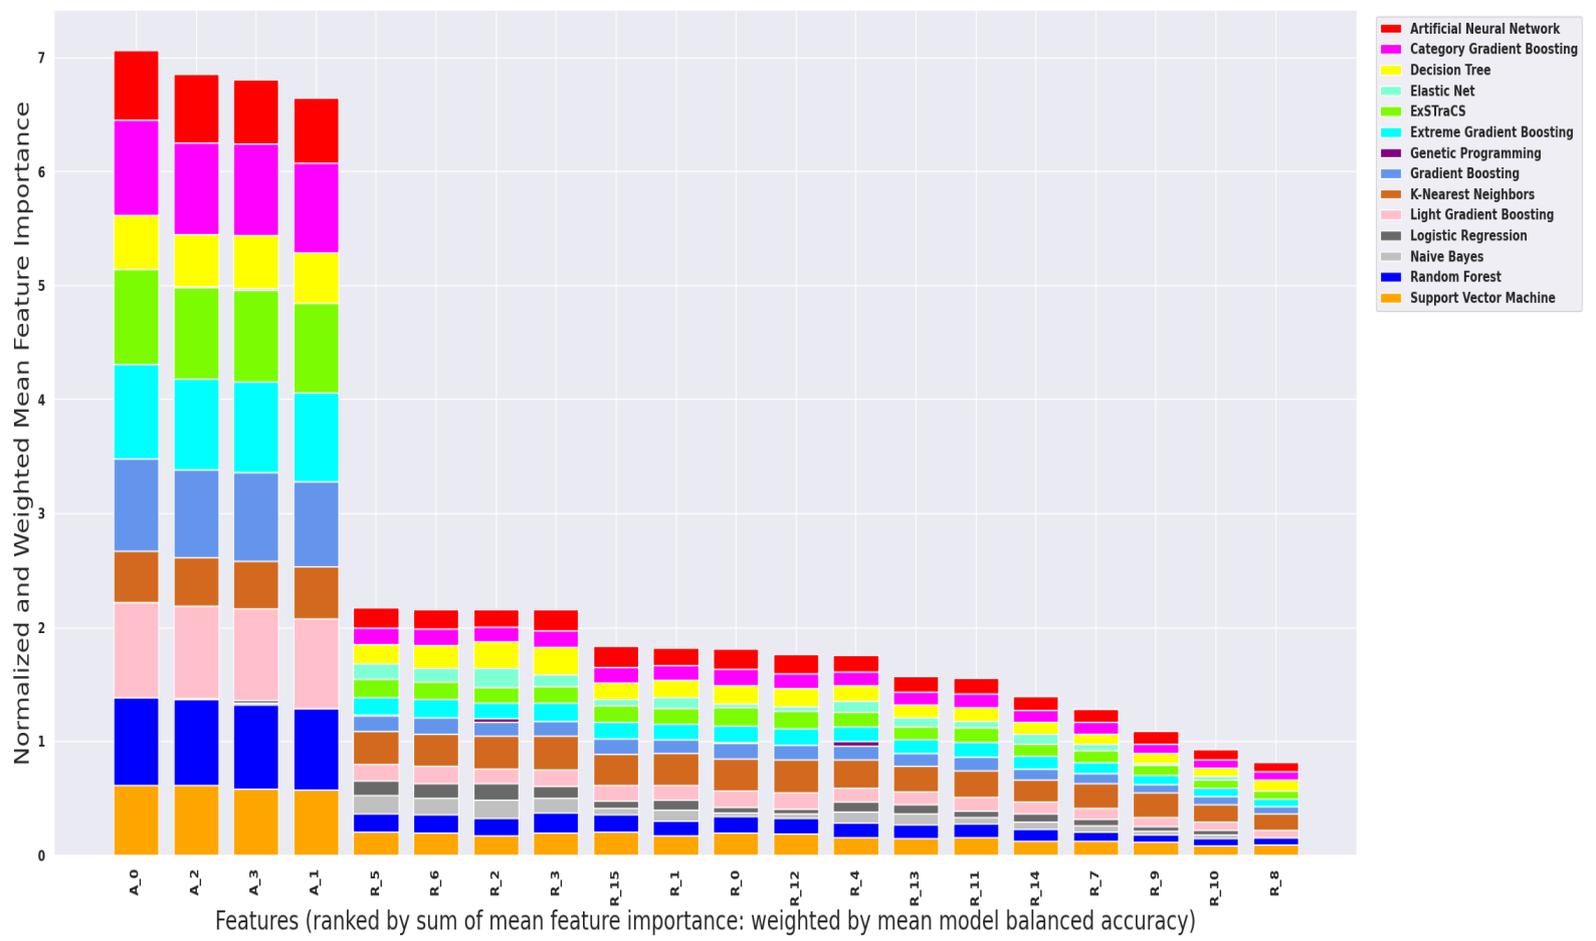

# Feature Importance Summary: D4 = D\_37\_bit\_mutlplexer\_5000\_01

Sorted Median Mutual Information Scores

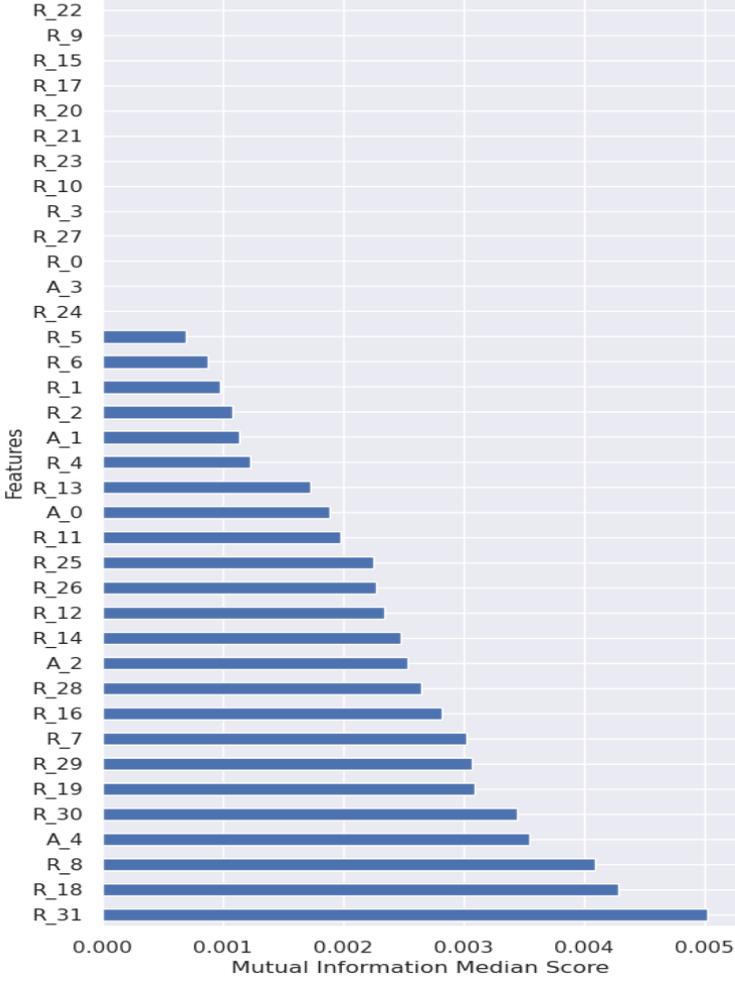

Sorted Median MultiSURF Scores

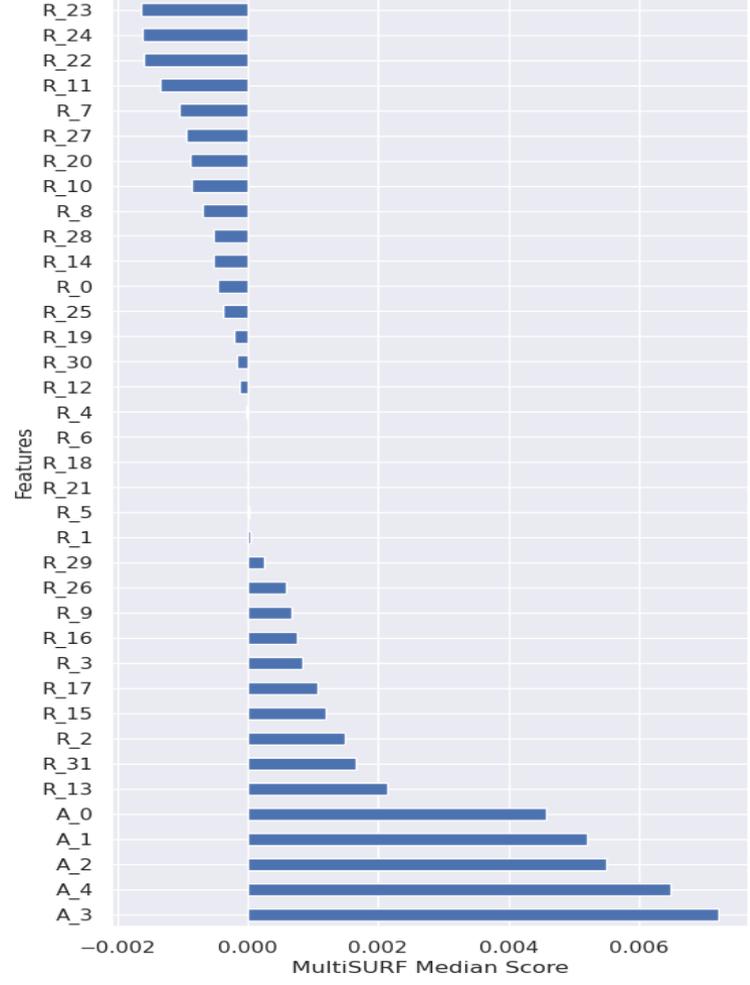

## Composite Feature Importance Plot (Normalized and Performance Weighted)

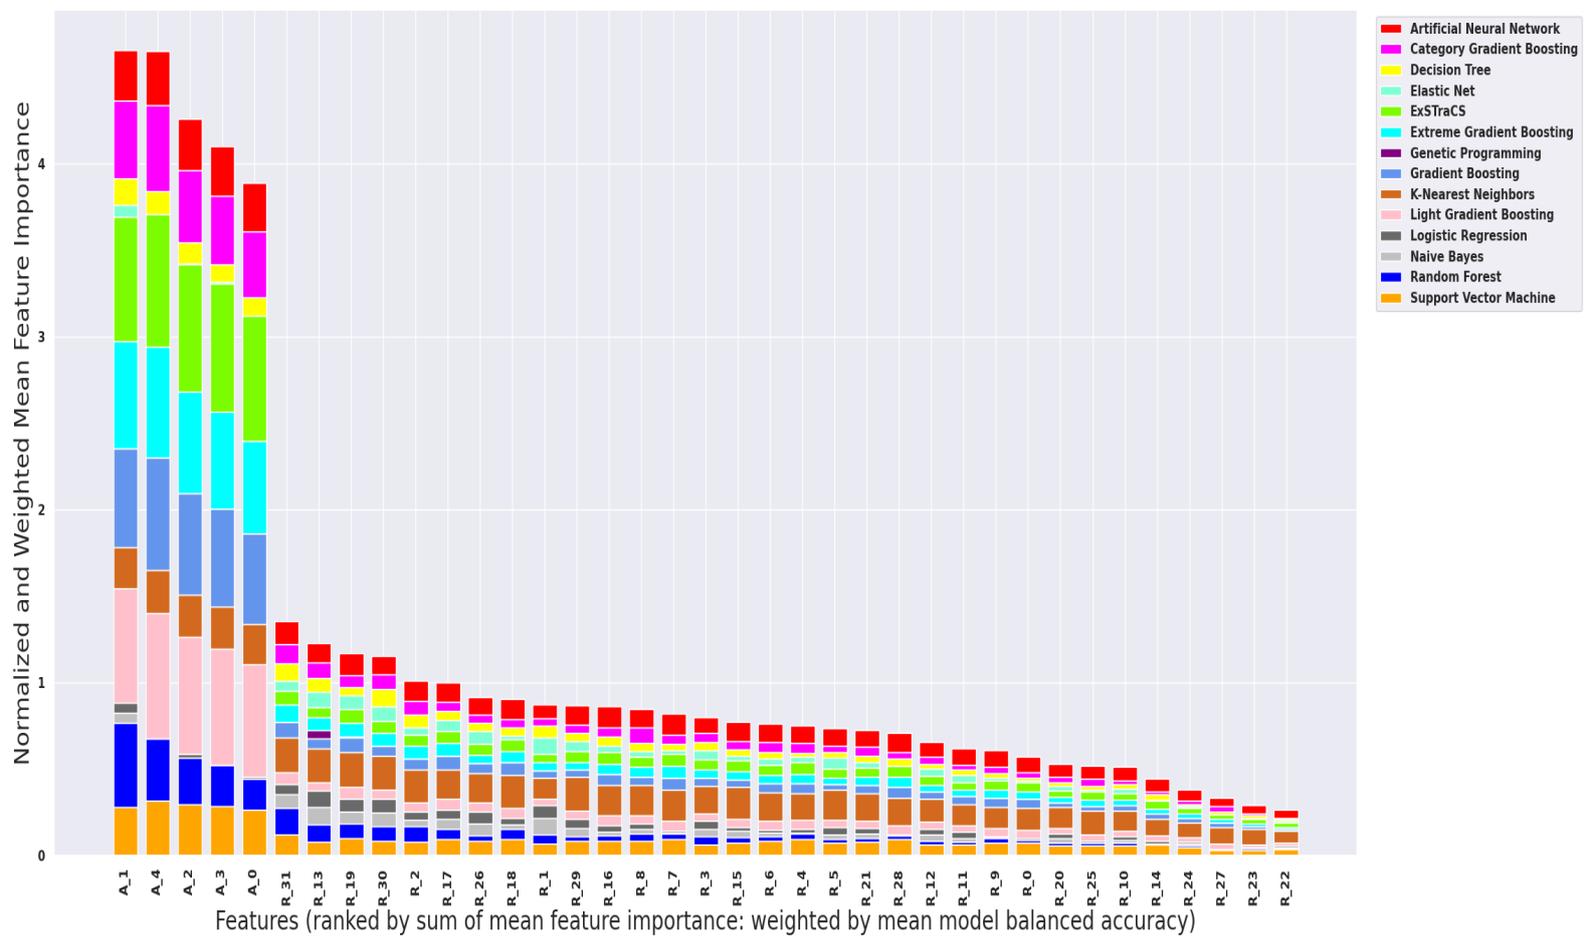

# Feature Importance Summary: D5 = E\_70\_bit\_mutliplexer\_10000\_01

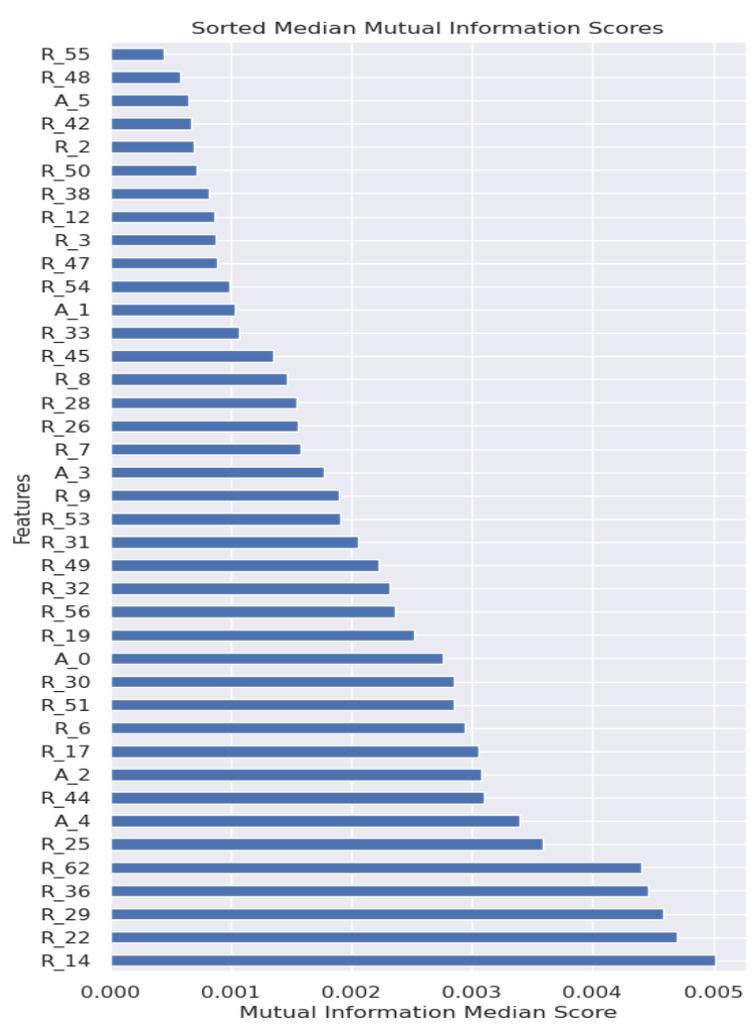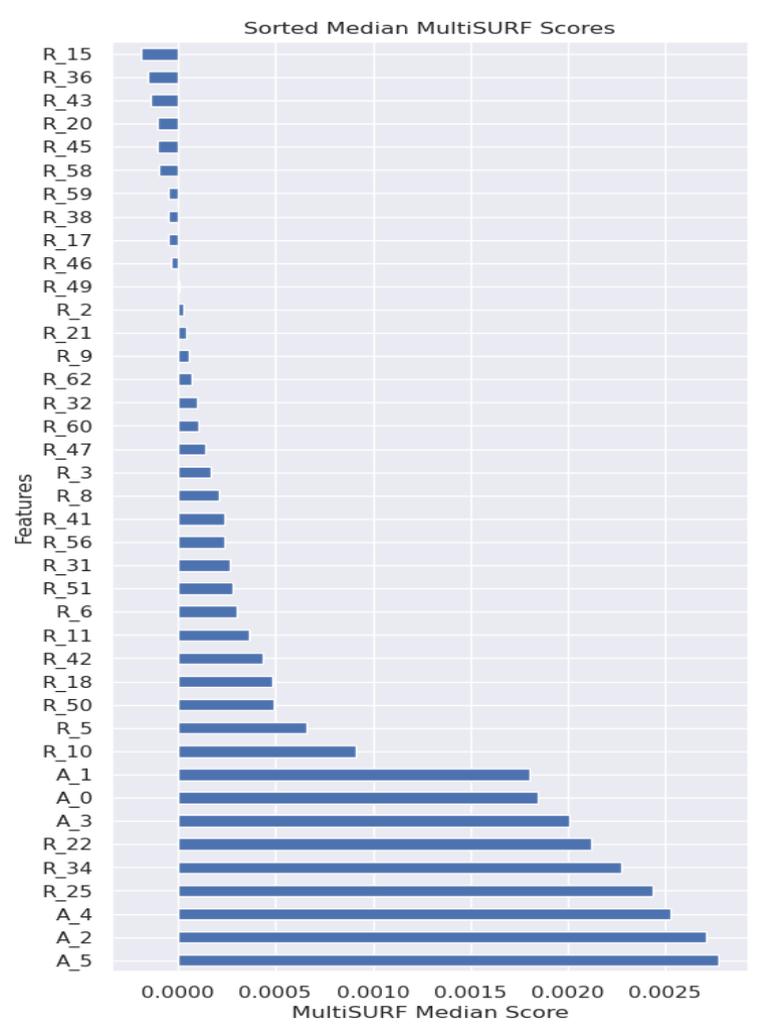

## Composite Feature Importance Plot (Normalized and Performance Weighted)

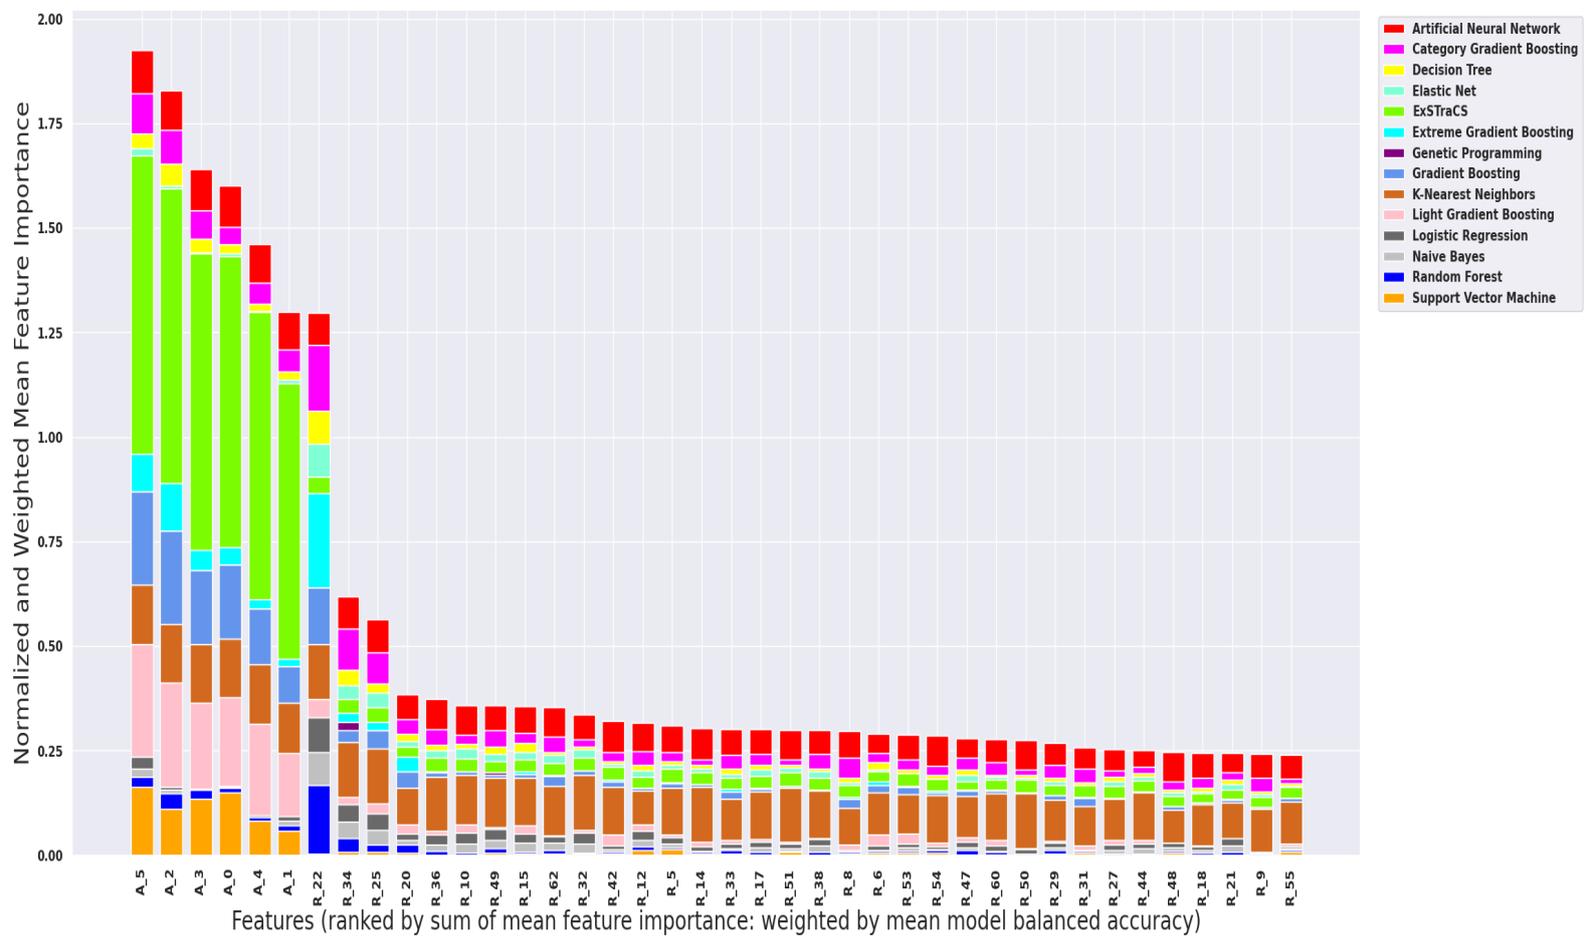

# Feature Importance Summary: D6 = F\_135\_bit\_multiplexer\_20000\_01

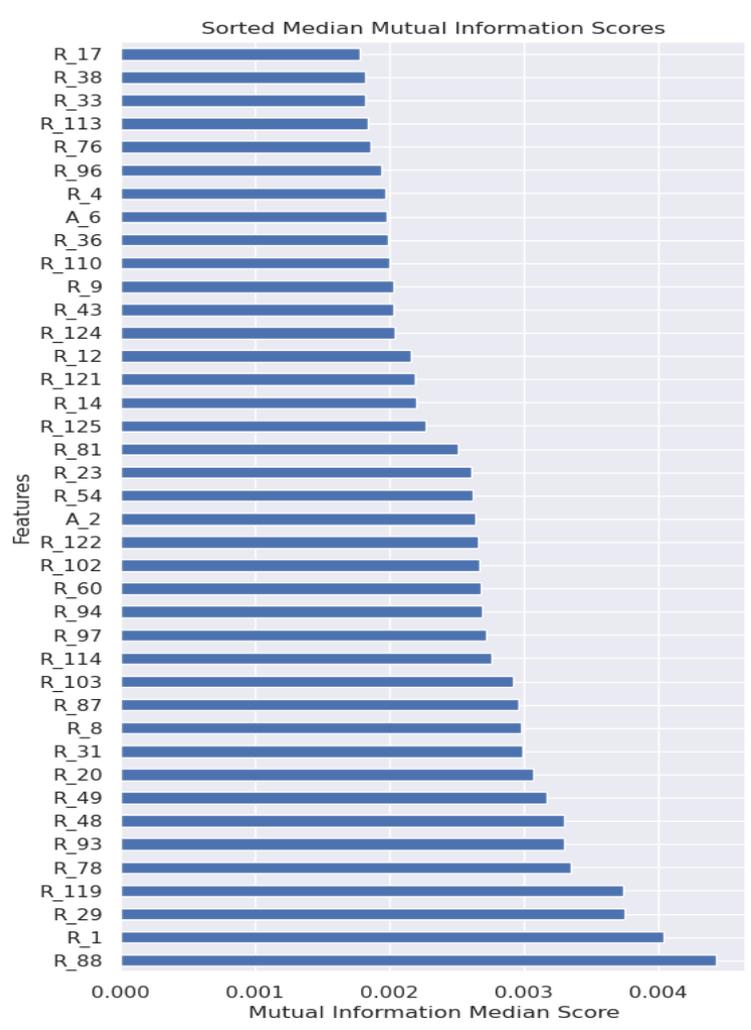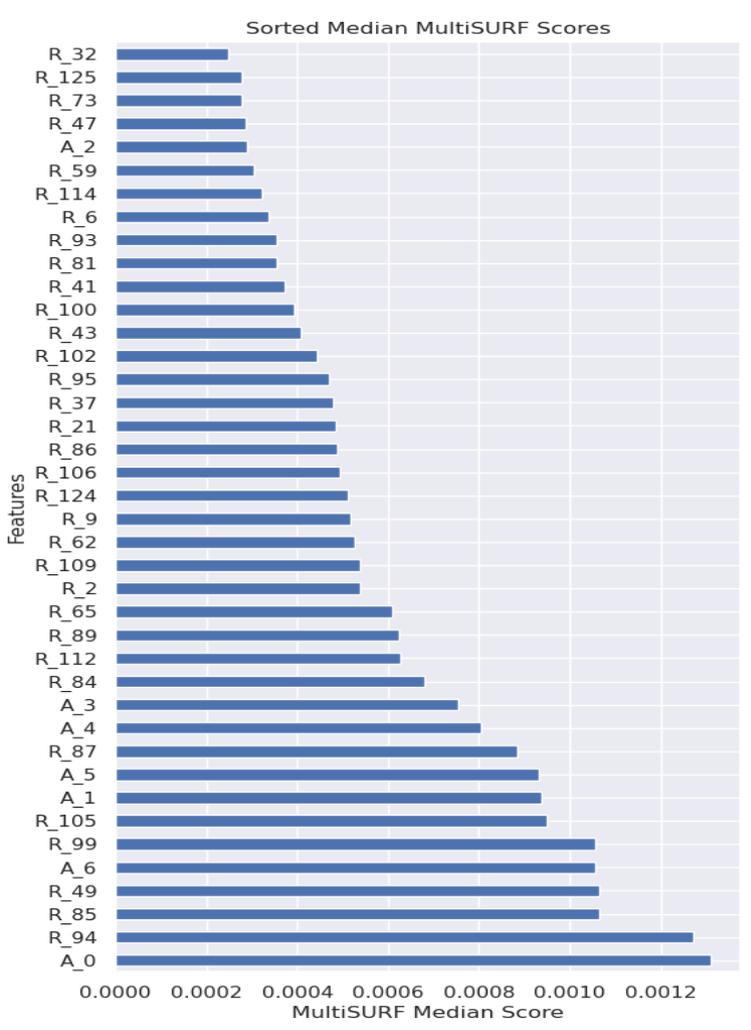

## Composite Feature Importance Plot (Normalized and Performance Weighted)

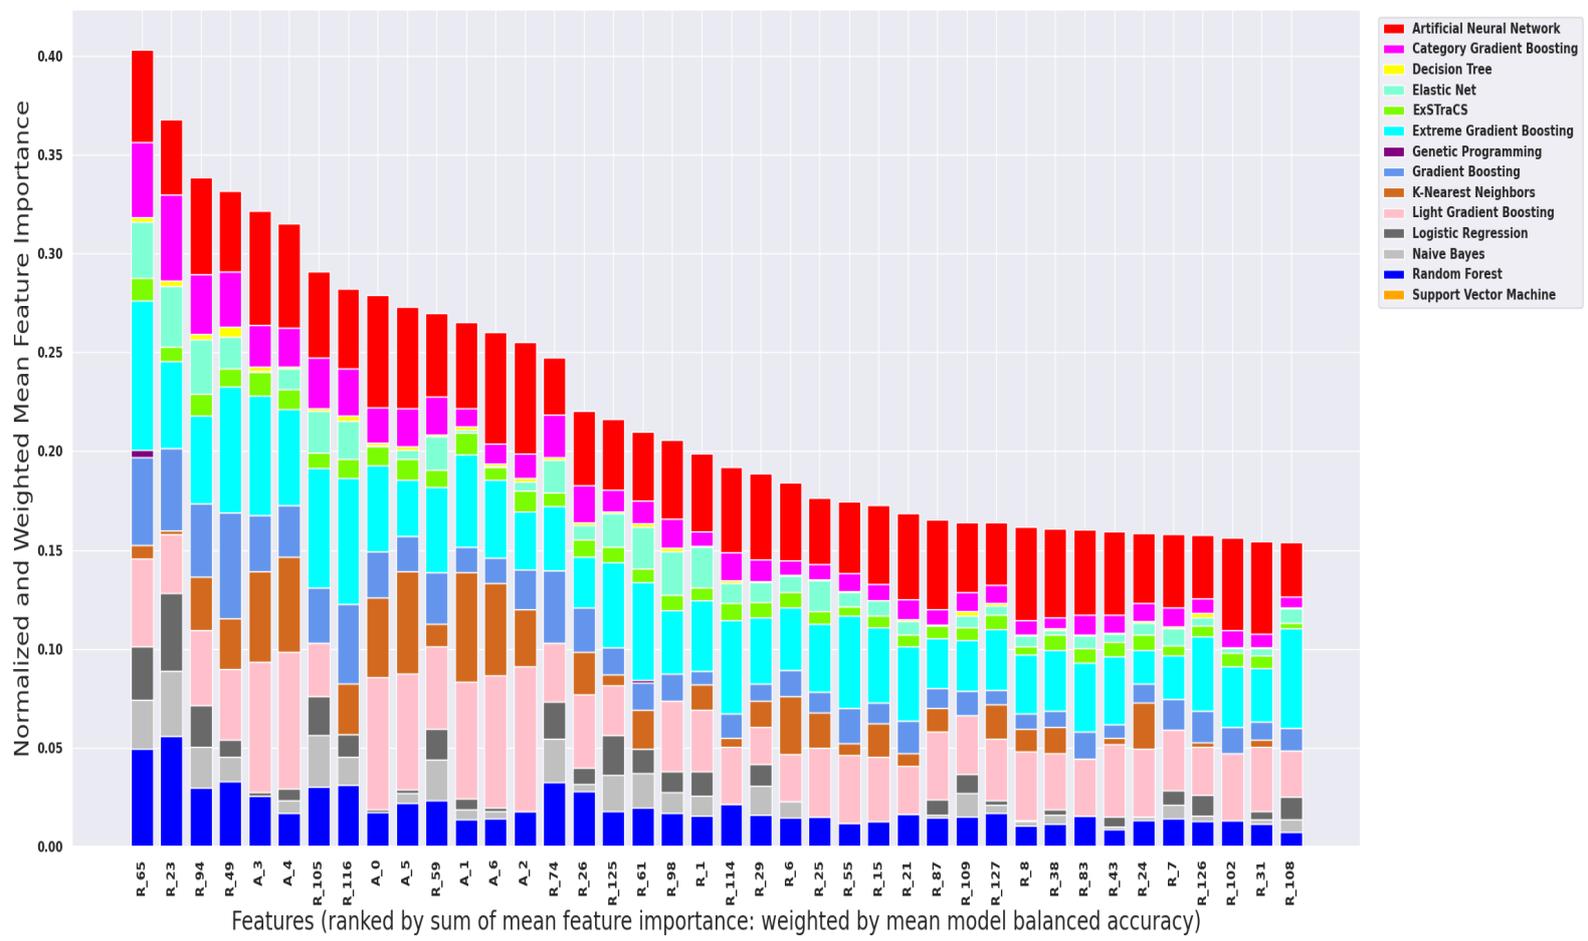

# Compare ML Performance Across Datasets

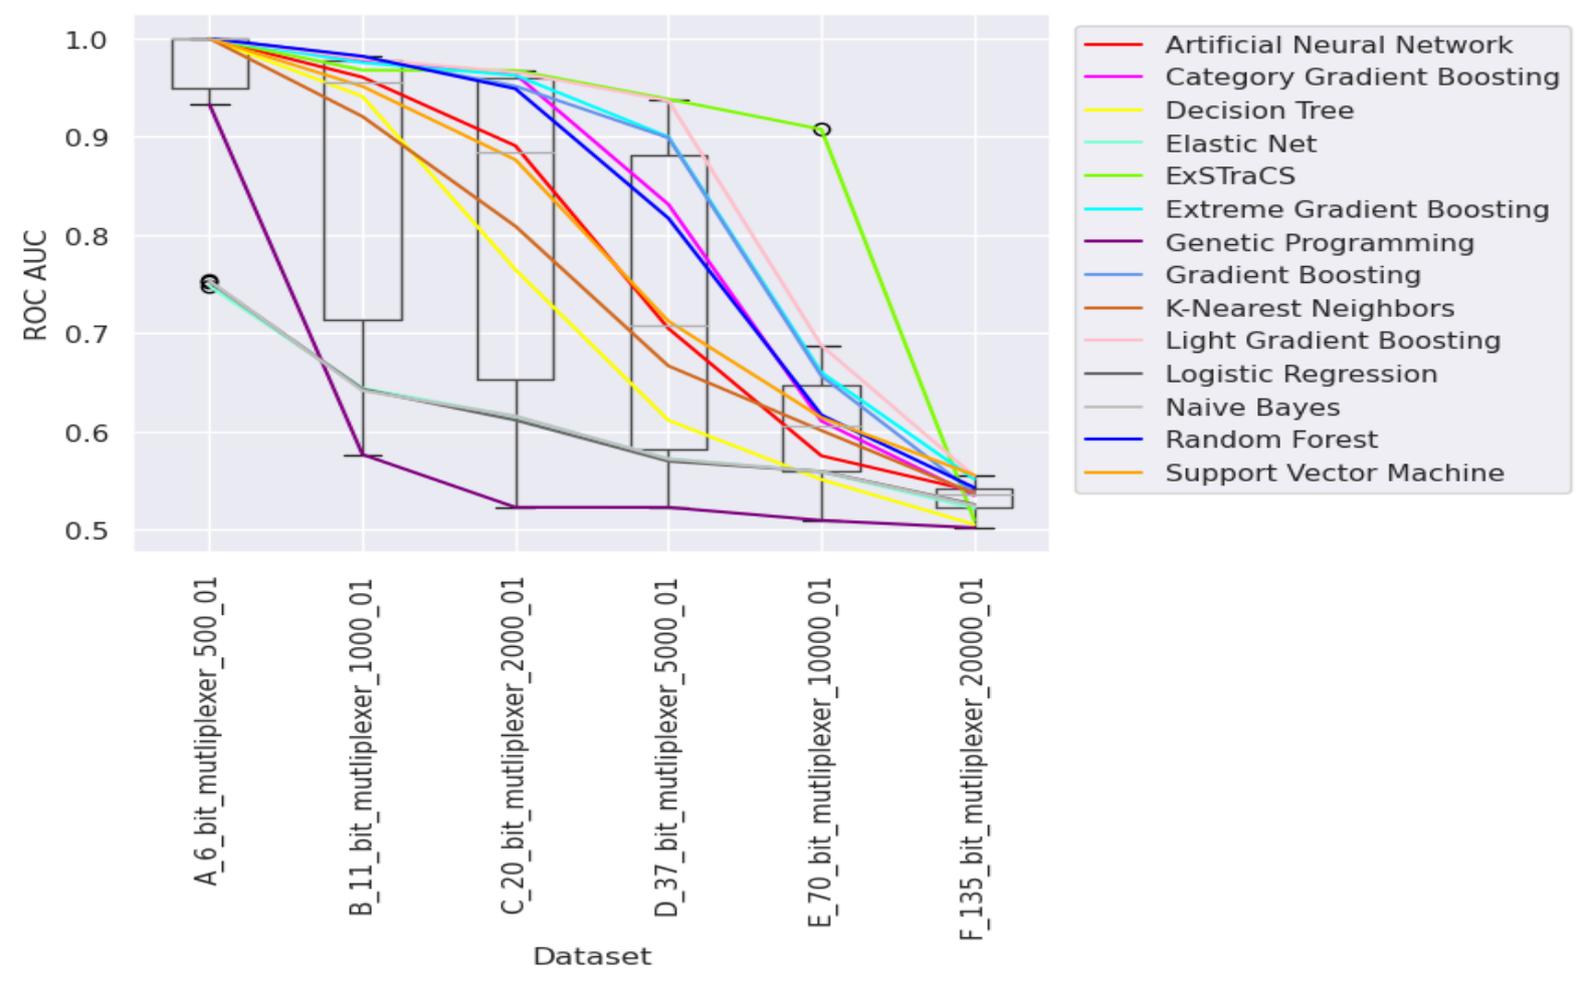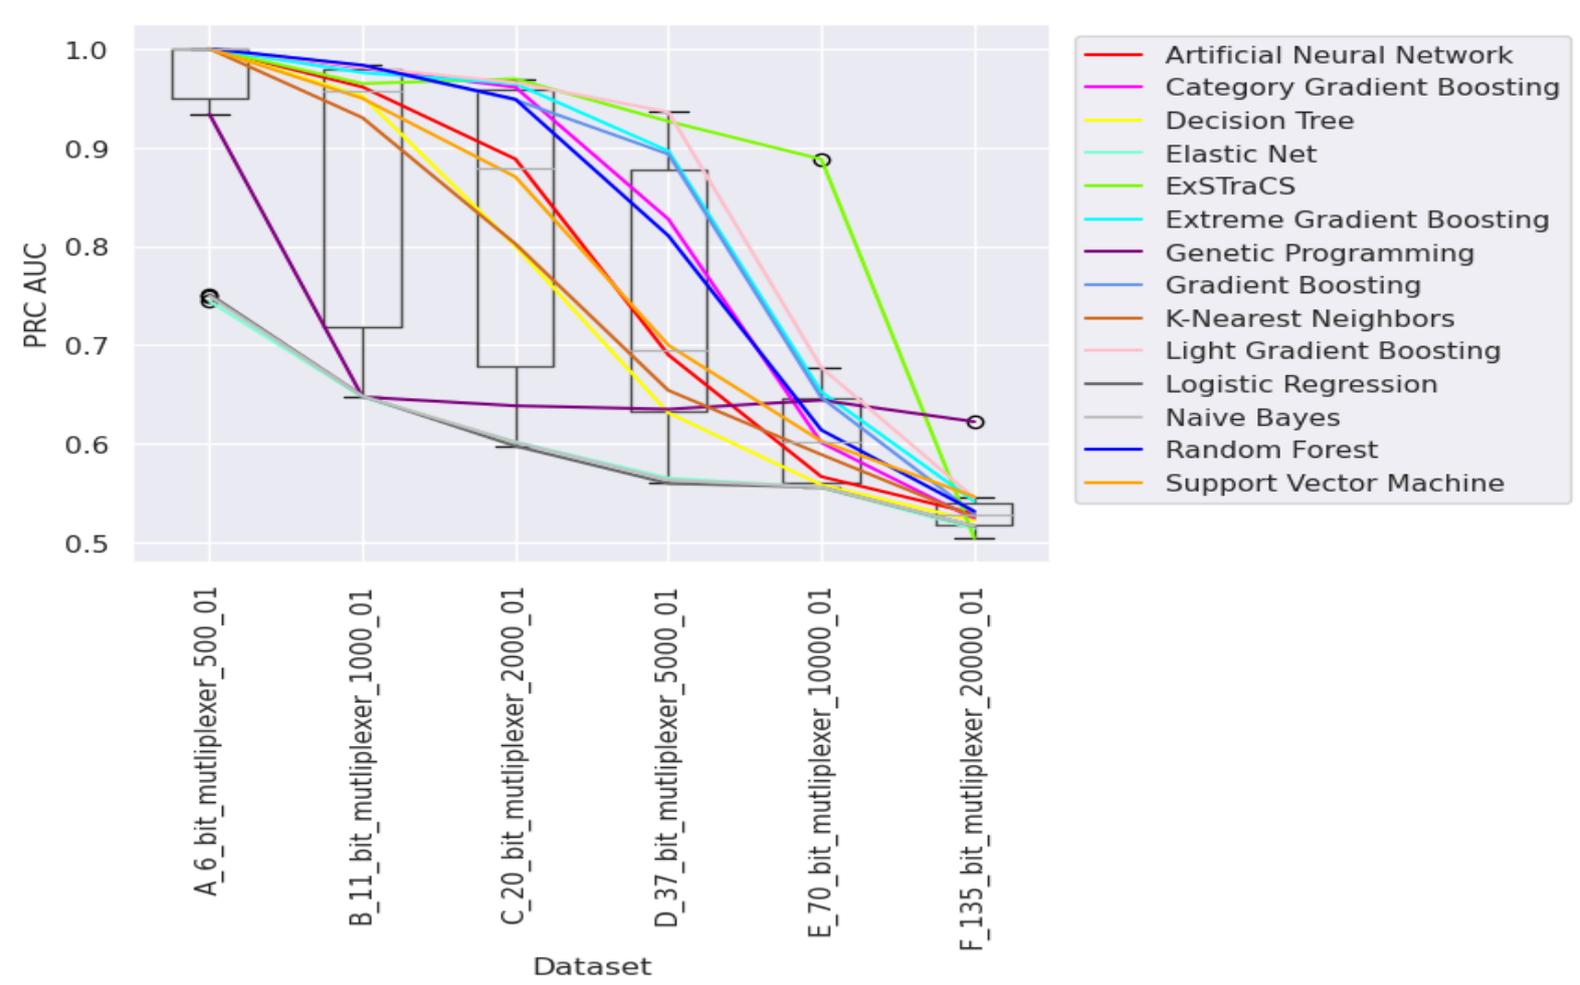

## Using Best Performing Algorithms (Kruskall Wallis Compare Datasets)

| Metrics              | P-Value | Best Alg D1               | Median D1 | Best Alg D2                | Median D2 | Best Alg D3                | Median D3 |
|----------------------|---------|---------------------------|-----------|----------------------------|-----------|----------------------------|-----------|
| Balanced Accuracy    | 0.0     | Artificial Neural Network | 1.0       | Decision Tree              | 0.915     | Category Gradient Boosting | 0.9247    |
| Accuracy             | 0.0     | Artificial Neural Network | 1.0       | Category Gradient Boosting | 0.915     | Category Gradient Boosting | 0.925     |
| F1 Score             | 0.0     | Artificial Neural Network | 1.0       | Decision Tree              | 0.9145    | Category Gradient Boosting | 0.9227    |
| Sensitivity (Recall) | 0.0     | Artificial Neural Network | 1.0       | Category Gradient Boosting | 0.9108    | Gradient Boosting          | 0.9133    |
| Specificity          | 0.0     | Artificial Neural Network | 1.0       | Decision Tree              | 0.9294    | ExSTraCS                   | 0.9363    |
| Precision (PPV)      | 0.0     | Artificial Neural Network | 1.0       | Light Gradient Boosting    | 0.9298    | ExSTraCS                   | 0.9327    |
| TP                   | 0.0     | Artificial Neural Network | 25.0      | Category Gradient Boosting | 46.0      | Category Gradient Boosting | 89.5      |
| TN                   | 0.0     | Artificial Neural Network | 25.0      | Category Gradient Boosting | 46.0      | ExSTraCS                   | 95.5      |
| FP                   | 0.0     | Elastic Net               | 9.0       | Genetic Programming        | 24.0      | Genetic Programming        | 49.5      |
| FN                   | 0.0     | Elastic Net               | 7.5       | Genetic Programming        | 20.5      | Genetic Programming        | 46.0      |
| NPV                  | 0.0     | Artificial Neural Network | 1.0       | Decision Tree              | 0.911     | Gradient Boosting          | 0.9175    |
| LR+                  | 0.0     | Naive Bayes               | 2.5007    | Decision Tree              | 11.375    | Light Gradient Boosting    | 13.178    |
| LR-                  | 0.0     | Elastic Net               | 0.4674    | Genetic Programming        | 0.746     | Genetic Programming        | 0.9219    |
| ROC AUC              | 0.0     | Artificial Neural Network | 1.0       | Category Gradient Boosting | 0.9833    | Light Gradient Boosting    | 0.9718    |
| PRC AUC              | 0.0     | Artificial Neural Network | 1.0       | Category Gradient Boosting | 0.9849    | ExSTraCS                   | 0.9763    |
| PRC APS              | 0.0     | Artificial Neural Network | 1.0       | Category Gradient Boosting | 0.985     | ExSTraCS                   | 0.9764    |

| Metrics              | P-Value | Best Alg D4             | Median D4 | Best Alg D5         | Median D5 | Best Alg D6                | Median D6 |
|----------------------|---------|-------------------------|-----------|---------------------|-----------|----------------------------|-----------|
| Balanced Accuracy    | 0.0     | ExSTraCS                | 0.8901    | ExSTraCS            | 0.8605    | Support Vector Machine     | 0.539     |
| Accuracy             | 0.0     | ExSTraCS                | 0.89      | ExSTraCS            | 0.8605    | Support Vector Machine     | 0.539     |
| F1 Score             | 0.0     | ExSTraCS                | 0.8887    | ExSTraCS            | 0.8593    | Support Vector Machine     | 0.5362    |
| Sensitivity (Recall) | 0.0     | ExSTraCS                | 0.8829    | ExSTraCS            | 0.8697    | Artificial Neural Network  | 0.5385    |
| Specificity          | 0.0     | ExSTraCS                | 0.8851    | ExSTraCS            | 0.8643    | Category Gradient Boosting | 0.6337    |
| Precision (PPV)      | 0.0     | ExSTraCS                | 0.8827    | ExSTraCS            | 0.8652    | Extreme Gradient Boosting  | 0.5355    |
| TP                   | 0.0     | ExSTraCS                | 218.5     | ExSTraCS            | 434.0     | Artificial Neural Network  | 534.5     |
| TN                   | 0.0     | ExSTraCS                | 223.5     | ExSTraCS            | 433.0     | Category Gradient Boosting | 638.5     |
| FP                   | 0.0     | Genetic Programming     | 116.5     | Genetic Programming | 241.5     | Genetic Programming        | 495.0     |
| FN                   | 0.0     | Genetic Programming     | 122.5     | Genetic Programming | 247.5     | Category Gradient Boosting | 594.5     |
| NPV                  | 0.0     | ExSTraCS                | 0.8885    | ExSTraCS            | 0.8667    | Support Vector Machine     | 0.5426    |
| LR+                  | 0.0     | ExSTraCS                | 7.6795    | ExSTraCS            | 6.4684    | Extreme Gradient Boosting  | 1.1717    |
| LR-                  | 0.0     | Genetic Programming     | 0.9112    | Genetic Programming | 0.9826    | Genetic Programming        | 1.0006    |
| ROC AUC              | 0.0     | Light Gradient Boosting | 0.94      | ExSTraCS            | 0.9112    | Support Vector Machine     | 0.5576    |
| PRC AUC              | 0.0     | Light Gradient Boosting | 0.9377    | ExSTraCS            | 0.9004    | Genetic Programming        | 0.6211    |
| PRC APS              | 0.0     | Light Gradient Boosting | 0.9378    | ExSTraCS            | 0.9007    | Support Vector Machine     | 0.5494    |

## Pipeline Runtime Summary

### A 6\_bit\_mutlplexer\_500\_01

| Pipeline Component                      | Phase | Time (sec)         |
|-----------------------------------------|-------|--------------------|
| Exploratory Analysis                    | 1     | 2.67712664604187   |
| Scale and Impute                        | 2     | 0.2740089893341064 |
| Mutual Information (Feature Importance) | 3     | 0.2864735126495361 |
| MultiSURF (Feature Importance)          | 3     | 6.460580587387085  |
| Feature Selection                       | 4     | 0.6904375553131104 |
| Artificial Neural Network(Modeling)     | 5     | 1072.8720622062683 |
| Category Gradient Boosting(Modeling)    | 5     | 7494.828892230988  |
| Decision Tree(Modeling)                 | 5     | 19.377732753753666 |
| Elastic Net(Modeling)                   | 5     | 21.71495056152344  |
| ExSTraCS(Modeling)                      | 5     | 21138.58070540428  |
| Extreme Gradient Boosting(Modeling)     | 5     | 5866.088219642639  |
| Genetic Programming(Modeling)           | 5     | 13048.591044187546 |
| Gradient Boosting(Modeling)             | 5     | 1876.241208314896  |
| K-Nearest Neighbors(Modeling)           | 5     | 72.01324462890625  |
| Light Gradient Boosting(Modeling)       | 5     | 385.7054343223572  |
| Logistic Regression(Modeling)           | 5     | 24.653773546218872 |
| Naive Bayes(Modeling)                   | 5     | 0.5989038944244385 |
| Random Forest(Modeling)                 | 5     | 3404.157678127289  |
| Support Vector Machine(Modeling)        | 5     | 2251.232235431671  |
| Stats Summary                           | 6     | 27.36684823036194  |

### B 11\_bit\_mutlplexer\_1000\_01

| Pipeline Component                      | Phase | Time (sec)          |
|-----------------------------------------|-------|---------------------|
| Exploratory Analysis                    | 1     | 3.510809898376465   |
| Scale and Impute                        | 2     | 0.3256189823150635  |
| Mutual Information (Feature Importance) | 3     | 0.5946216583251953  |
| MultiSURF (Feature Importance)          | 3     | 32.66403889656067   |
| Feature Selection                       | 4     | 0.7494640350341797  |
| Artificial Neural Network(Modeling)     | 5     | 2341.3973276615143  |
| Category Gradient Boosting(Modeling)    | 5     | 10236.114404678345  |
| Decision Tree(Modeling)                 | 5     | 23.9583592414856    |
| Elastic Net(Modeling)                   | 5     | 27.12389159202576   |
| ExSTraCS(Modeling)                      | 5     | 111231.33455729485  |
| Extreme Gradient Boosting(Modeling)     | 5     | 5770.540885686874   |
| Genetic Programming(Modeling)           | 5     | 11472.030278205872  |
| Gradient Boosting(Modeling)             | 5     | 5021.442324638367   |
| K-Nearest Neighbors(Modeling)           | 5     | 101.39071726799013  |
| Light Gradient Boosting(Modeling)       | 5     | 856.4688177108765   |
| Logistic Regression(Modeling)           | 5     | 30.968572854995728  |
| Naive Bayes(Modeling)                   | 5     | 1.0038552284240725  |
| Random Forest(Modeling)                 | 5     | 4492.77170920372    |
| Support Vector Machine(Modeling)        | 5     | 1736.18875112207031 |
| Stats Summary                           | 6     | 33.16046404838562   |

### C 20\_bit\_mutlplexer\_2000\_01

| Pipeline Component                      | Phase | Time (sec)         |
|-----------------------------------------|-------|--------------------|
| Exploratory Analysis                    | 1     | 4.43428111076355   |
| Scale and Impute                        | 2     | 0.5926880836486816 |
| Mutual Information (Feature Importance) | 3     | 1.613957405090332  |
| MultiSURF (Feature Importance)          | 3     | 197.78458094596863 |
| Feature Selection                       | 4     | 1.174454689025879  |
| Artificial Neural Network(Modeling)     | 5     | 6057.136718273163  |
| Category Gradient Boosting(Modeling)    | 5     | 9952.95704960823   |
| Decision Tree(Modeling)                 | 5     | 33.52086925506592  |
| Elastic Net(Modeling)                   | 5     | 48.7155704498291   |
| ExSTraCS(Modeling)                      | 5     | 229077.84328961367 |
| Extreme Gradient Boosting(Modeling)     | 5     | 8649.876857995987  |
| Genetic Programming(Modeling)           | 5     | 11099.113930940628 |
| Gradient Boosting(Modeling)             | 5     | 9006.2832634449    |
| K-Nearest Neighbors(Modeling)           | 5     | 1352.0665411949158 |
| Light Gradient Boosting(Modeling)       | 5     | 2388.5692188739777 |
| Logistic Regression(Modeling)           | 5     | 61.44512200335553  |
| Naive Bayes(Modeling)                   | 5     | 2.328498601913452  |
| Random Forest(Modeling)                 | 5     | 7468.761832475662  |
| Support Vector Machine(Modeling)        | 5     | 5280.826467752457  |
| Stats Summary                           | 6     | 39.98420333862305  |

### D 37\_bit\_mutlplexer\_5000\_01

| Pipeline Component                      | Phase | Time (sec)         |
|-----------------------------------------|-------|--------------------|
| Exploratory Analysis                    | 1     | 7.409142017364502  |
| Scale and Impute                        | 2     | 1.783540964126587  |
| Mutual Information (Feature Importance) | 3     | 6.538389205932617  |
| MultiSURF (Feature Importance)          | 3     | 483.53567814826965 |
| Feature Selection                       | 4     | 2.2569901943206787 |
| Artificial Neural Network(Modeling)     | 5     | 8741.390830755234  |
| Category Gradient Boosting(Modeling)    | 5     | 10444.06927871704  |
| Decision Tree(Modeling)                 | 5     | 74.10389852523804  |
| Elastic Net(Modeling)                   | 5     | 110.8091447353363  |
| ExSTraCS(Modeling)                      | 5     | 263212.5577878952  |
| Extreme Gradient Boosting(Modeling)     | 5     | 9457.452483654022  |
| Genetic Programming(Modeling)           | 5     | 11609.894495010376 |
| Gradient Boosting(Modeling)             | 5     | 9580.27242398262   |
| K-Nearest Neighbors(Modeling)           | 5     | 22205.503813505173 |
| Light Gradient Boosting(Modeling)       | 5     | 5302.768069267273  |
| Logistic Regression(Modeling)           | 5     | 106.97014045715332 |
| Naive Bayes(Modeling)                   | 5     | 7.06707763671875   |
| Random Forest(Modeling)                 | 5     | 10470.864454507828 |
| Support Vector Machine(Modeling)        | 5     | 16616.57949781418  |
| Stats Summary                           | 6     | 45.88159823417664  |

### E 70\_bit\_mutlplexer\_10000\_01

| Pipeline Component                      | Phase | Time (sec)         |
|-----------------------------------------|-------|--------------------|
| Exploratory Analysis                    | 1     | 10.389281034469604 |
| Scale and Impute                        | 2     | 5.9340245723724365 |
| Mutual Information (Feature Importance) | 3     | 26.03225040435791  |
| MultiSURF (Feature Importance)          | 3     | 888.8911199569702  |
| Feature Selection                       | 4     | 6.917673349380493  |
| Artificial Neural Network(Modeling)     | 5     | 9186.195650100708  |
| Category Gradient Boosting(Modeling)    | 5     | 12019.572035551071 |
| Decision Tree(Modeling)                 | 5     | 158.33335375785828 |
| Elastic Net(Modeling)                   | 5     | 324.11168456077576 |
| ExSTraCS(Modeling)                      | 5     | 454642.4105942249  |
| Extreme Gradient Boosting(Modeling)     | 5     | 11321.671221017838 |
| Genetic Programming(Modeling)           | 5     | 13118.048599243164 |
| Gradient Boosting(Modeling)             | 5     | 10956.142976999285 |
| K-Nearest Neighbors(Modeling)           | 5     | 203914.9919500351  |
| Light Gradient Boosting(Modeling)       | 5     | 11464.409035921097 |
| Logistic Regression(Modeling)           | 5     | 622.9291326999664  |
| Naive Bayes(Modeling)                   | 5     | 47.17171025276184  |
| Random Forest(Modeling)                 | 5     | 12332.294057369232 |
| Support Vector Machine(Modeling)        | 5     | 33183.3055369854   |
| Stats Summary                           | 6     | 41.75016260147095  |

### F 135\_bit\_mutlplexer\_20000\_01

| Pipeline Component                      | Phase | Time (sec)         |
|-----------------------------------------|-------|--------------------|
| Exploratory Analysis                    | 1     | 12.506709814071655 |
| Scale and Impute                        | 2     | 21.760517835617065 |
| Mutual Information (Feature Importance) | 3     | 106.97442984580994 |
| MultiSURF (Feature Importance)          | 3     | 1647.38024020195   |
| Feature Selection                       | 4     | 19.285180807113647 |
| Artificial Neural Network(Modeling)     | 5     | 9486.72973060608   |
| Category Gradient Boosting(Modeling)    | 5     | 16686.76847934723  |
| Decision Tree(Modeling)                 | 5     | 546.2360656261444  |
| Elastic Net(Modeling)                   | 5     | 1253.041860818863  |
| ExSTraCS(Modeling)                      | 5     | 1321166.3120145798 |
| Extreme Gradient Boosting(Modeling)     | 5     | 15829.22190451622  |
| Genetic Programming(Modeling)           | 5     | 15846.014689683914 |
| Gradient Boosting(Modeling)             | 5     | 20822.73474264145  |
| K-Nearest Neighbors(Modeling)           | 5     | 1604220.13211298   |
| Light Gradient Boosting(Modeling)       | 5     | 18967.921857357025 |
| Logistic Regression(Modeling)           | 5     | 2569.354686021805  |
| Naive Bayes(Modeling)                   | 5     | 280.4918615818024  |
| Random Forest(Modeling)                 | 5     | 23444.557268619537 |
| Support Vector Machine(Modeling)        | 5     | 161188.32617139816 |
| Stats Summary                           | 6     | 46.8548789024353   |
