# Supplementary material for: STREAMLINE: An Automated Machine Learning Pipeline for Biomedicine Applied to Examine the Utility of Photography-Based Phenotypes for OSA Prediction Across International Sleep Centers
Source: arXiv:2312.05461 ancillary file (2023-12-09)
Supplement: Supplementary file 6 [file sagic_exp_STREAMLINE_Report.pdf]

# STREAMLINE Testing Data Evaluation Report: 2023-10-14 14:27:18.674361

## General Pipeline Settings:

CV Partitions: 10  
Partition Method: Stratified  
Categorical Cutoff: 10  
Statistical Significance Cutoff: 0.05  
Random Seed: 42  
Run From Notebook: False

## Feature Importance/Selection Settings:

Use Mutual Information: True  
Use MultiSURF: True  
Use TURF: False  
TURF Cutoff: 0.5  
MultiSURF Instance Subset: 3000  
Max Features to Keep: 2000  
Filter Poor Features: True  
Top Features to Display: 40  
Export Feature Importance Plot: True

## ML Modeling Algorithms:

Artificial Neural Network: True  
Category Gradient Boosting: True  
Decision Tree: True  
Elastic Net: True  
ExSTraCS: True  
Extreme Gradient Boosting: True  
Genetic Programming: True  
Gradient Boosting: True  
K-Nearest Neighbors: True  
Light Gradient Boosting: True  
Logistic Regression: True  
Naive Bayes: True  
Random Forest: True  
Support Vector Machine: True  
XCS: False  
eLCS: False

## Modeling Settings:

Primary Metric: balanced\_accuracy  
Training Subsample for KNN,ANN,SVM,and XGB: 0  
Uniform Feature Importance Estimation (Models): True  
Hyperparameter Sweep Number of Trials: 200  
Hyperparameter Timeout: 900  
Export Hyperparameter Sweep Plots: False

## LCS Settings (eLCS,XCS,ExSTraCS):

Do LCS Hyperparameter Sweep: False  
nu: 1  
Training Iterations: 400000  
N (Rule Population Size): 2000  
LCS Hyperparameter Sweep Timeout: 1200

## Stats and Figure Settings:

Export ROC Plot: True  
Export PRC Plot: True  
Export Metric Boxplots: True  
Export Feature Importance Boxplots: True  
Metric Weighting Composite FI Plots: balanced\_accuracy  
Top Model Features To Display: 40

## EDA and Processing Settings:

Engineering Missingness Cutoff: 0.5  
Cleaning Missingness Cutoff: 0.5  
Correlation Removal Threshold: 1.0  
List of Exploratory Analysis Ran: ['Describe', 'Univariate Analysis', 'Feature Correlation']  
List of Exploratory Plots Saved: ['Describe', 'Univariate Analysis', 'Feature Correlation']  
Use Data Scaling: True  
Use Data Imputation: True  
Use Multivariate Imputation: True  
Overwrite CV Datasets: True

## Target Dataset(s):

D1 = A\_GE15\_DEM  
D2 = B\_GE15\_DX  
D3 = C\_GE15\_SYM  
D4 = D\_GE15\_CF  
D5 = E\_GE15\_IO  
D6 = F\_GE15\_DEMDX  
D7 = G\_GE15\_DEMDXSYM  
D8 = H\_GE15\_DEMDXSYMCF  
D9 = I\_GE15\_DEMDXSYMIO  
D10 = J\_GE15\_DEMDXSYMCFIO  
D11 = K\_GE5\_DEM  
D12 = L\_GE5\_DX  
D13 = M\_GE5\_SYM  
D14 = N\_GE5\_CF  
D15 = O\_GE5\_IO  
D16 = P\_GE5\_DEMDX  
D17 = Q\_GE5\_DEMDXSYM  
D18 = R\_GE5\_DEMDXSYMCF  
D19 = S\_GE5\_DEMDXSYMIO  
D20 = T\_GE5\_DEMDXSYMCFIO

## Target Data Settings:

Data Path: /home/ryanurb/idata/datasets/OSA\_9\_25\_23  
Output Path: /home/ryanurb/idata/output  
Experiment Name: sagic\_exp  
Class Label: class  
Instance Label: subnum  
Match Label: None  
Ignored Features: None  
Specified Categorical Features:  
/home/ryanurb/idata/datasets/OSA\_9\_25\_23\_Rep/FeatureTypes/SAGIC\_Cat\_Features.csv  
Specified Quantitative Features: None

# Univariate Analysis of Each Dataset (Top 10 Features for Each): Page 1

## D1 = A\_GE15\_DEM

| Feature   | p-value                | Test-statistic     | Test-name           |
|-----------|------------------------|--------------------|---------------------|
| bmi       | 1.3279641470736552e-38 | 400589.5           | Mann-Whitney U Test |
| male      | 4.063766784119089e-24  | 102.6182292551845  | Chi Square Test     |
| csamer    | 6.122341940895255e-14  | 56.3316035421966   | Chi Square Test     |
| asian     | 2.723022010333082e-07  | 26.436805154571545 | Chi Square Test     |
| age       | 0.0003928813591798     | 538872.5           | Mann-Whitney U Test |
| aframer   | 0.0188088690561117     | 5.5191990106447655 | Chi Square Test     |
| other     | 0.3552586983732356     | 0.8545842635793259 | Chi Square Test     |
| caucasian | 0.5714063223516979     | 0.3203351155752309 | Chi Square Test     |

## D2 = B\_GE15\_DX

| Feature          | p-value               | Test-statistic     | Test-name       |
|------------------|-----------------------|--------------------|-----------------|
| medhx_hbp        | 5.436404585485976e-06 | 20.677037913403264 | Chi Square Test |
| medhx_ldl        | 0.0156053557685671    | 5.846805305518504  | Chi Square Test |
| medhx_cad        | 0.0221031111289531    | 5.237650038798381  | Chi Square Test |
| medhx_stroke     | 0.053245659900618     | 3.7361920818776966 | Chi Square Test |
| medhx_heart_fail | 0.2735592031749072    | 1.1988122367733356 | Chi Square Test |
| medhx_dm         | 0.2802812113271561    | 1.165725828523342  | Chi Square Test |
| medhx_afib       | 0.7071614752558567    | 0.1411287251795834 | Chi Square Test |

## D3 = C\_GE15\_SYM

| Feature    | p-value                | Test-statistic | Test-name           |
|------------|------------------------|----------------|---------------------|
| loud_snore | 1.3390949170859947e-24 | 299477.5       | Mann-Whitney U Test |
| map_index  | 2.95727320453731e-23   | 299237.0       | Mann-Whitney U Test |
| choke      | 5.71259367300313e-16   | 325136.5       | Mann-Whitney U Test |
| gaspings   | 5.053318765476038e-10  | 342768.5       | Mann-Whitney U Test |

## D4 = D\_GE15\_CF

| Feature               | p-value                | Test-statistic | Test-name           |
|-----------------------|------------------------|----------------|---------------------|
| face_width            | 1.0456019441332584e-51 | 371046.5       | Mann-Whitney U Test |
| mand_width            | 1.4138297267890205e-50 | 373520.5       | Mann-Whitney U Test |
| max_mand_vol          | 9.670980103736678e-36  | 407717.0       | Mann-Whitney U Test |
| max_tri_area          | 2.541450087867167e-34  | 412405.0       | Mann-Whitney U Test |
| cer_ang               | 8.806560696102838e-31  | 342422.0       | Mann-Whitney U Test |
| cranial_base_tri_area | 1.529649920196137e-28  | 429862.5       | Mann-Whitney U Test |
| mand_vol              | 3.193897432853109e-28  | 431267.5       | Mann-Whitney U Test |
| mand_tri_area         | 6.9060105404607e-27    | 435382.0       | Mann-Whitney U Test |
| max_mand_box_area     | 1.249565144133052e-26  | 434456.5       | Mann-Whitney U Test |
| lat_fac_ht            | 2.386581976985256e-26  | 435398.0       | Mann-Whitney U Test |

## D5 = E\_GE15\_IO

| Feature                 | p-value                | Test-statistic     | Test-name           |
|-------------------------|------------------------|--------------------|---------------------|
| tongue_width_f_te_m     | 2.9412683339317208e-08 | 478698.0           | Mann-Whitney U Test |
| tongue_thickness_p_te_m | 1.176660747491191e-07  | 483558.5           | Mann-Whitney U Test |
| tongue_curvature_p_te_m | 2.190800737870203e-05  | 620727.5           | Mann-Whitney U Test |
| mal_score_ftem_c2       | 0.0001939169943048     | 13.889127633950542 | Chi Square Test     |
| tongue_width_tim_nph    | 0.0008556357128635     | 406956.5           | Mann-Whitney U Test |
| mal_score_ftem_c4       | 0.0011588349812228     | 10.554851888071893 | Chi Square Test     |
| open_wid_f_te_m         | 0.0161205985985049     | 512054.0           | Mann-Whitney U Test |
| tongue_length_f         | 0.0380529957228        | 562047.0           | Mann-Whitney U Test |
| tongue_length_p_te_m    | 0.0407263438803211     | 590342.5           | Mann-Whitney U Test |
| open_wid_tim_nph        | 0.0659470910577001     | 537129.5           | Mann-Whitney U Test |

## Univariate Analysis of Each Dataset (Top 10 Features for Each): Page 2

### D6 = F\_GE15\_DEMDX

| Feature      | p-value                | Test-statistic     | Test-name           |
|--------------|------------------------|--------------------|---------------------|
| bmi          | 1.3509487479288172e-27 | 287292.5           | Mann-Whitney U Test |
| male         | 1.0711955315634748e-19 | 82.47307251944947  | Chi Square Test     |
| asian        | 1.2112176647400883e-06 | 23.5593128435826   | Chi Square Test     |
| medhx_hbp    | 1.1965811309096403e-05 | 19.16872140582105  | Chi Square Test     |
| csamer       | 4.5337438301078574e-05 | 16.633733967283316 | Chi Square Test     |
| medhx_ldl    | 0.0143765463631614     | 5.991306999906243  | Chi Square Test     |
| age          | 0.0261830241509545     | 383435.5           | Mann-Whitney U Test |
| medhx_cad    | 0.0328738640882567     | 4.5523361473384245 | Chi Square Test     |
| caucasian    | 0.055191637017405      | 3.6762867442781815 | Chi Square Test     |
| medhx_stroke | 0.0574187129523506     | 3.6104172216344153 | Chi Square Test     |

### D7 = G\_GE15\_DEMDXSYM

| Feature    | p-value                | Test-statistic     | Test-name           |
|------------|------------------------|--------------------|---------------------|
| bmi        | 7.240125083249458e-28  | 295298.5           | Mann-Whitney U Test |
| loud_snore | 5.1510060637006595e-24 | 304207.0           | Mann-Whitney U Test |
| map_index  | 9.093977834331397e-22  | 309380.5           | Mann-Whitney U Test |
| male       | 2.1910609515206543e-20 | 85.61052527333156  | Chi Square Test     |
| choke      | 9.372957385296172e-16  | 327983.0           | Mann-Whitney U Test |
| gasping    | 6.638321702334852e-10  | 344036.0           | Mann-Whitney U Test |
| asian      | 3.742082708726812e-06  | 21.392622806929    | Chi Square Test     |
| medhx_hbp  | 1.1965811309096403e-05 | 19.16872140582105  | Chi Square Test     |
| csamer     | 4.776502299174941e-05  | 16.534812259483008 | Chi Square Test     |
| medhx_ldl  | 0.0143765463631614     | 5.991306999906243  | Chi Square Test     |

### D8 = H\_GE15\_DEMDXSYMCF

| Feature               | p-value                | Test-statistic | Test-name           |
|-----------------------|------------------------|----------------|---------------------|
| face_width            | 1.0456019441332584e-51 | 371046.5       | Mann-Whitney U Test |
| mand_width            | 1.4138297267890205e-50 | 373520.5       | Mann-Whitney U Test |
| bmi                   | 1.0818438086456103e-38 | 402018.5       | Mann-Whitney U Test |
| max_mand_vol          | 9.670980103736678e-36  | 407717.0       | Mann-Whitney U Test |
| max_tri_area          | 2.541450087867167e-34  | 412405.0       | Mann-Whitney U Test |
| cer_ang               | 8.806560696102838e-31  | 342422.0       | Mann-Whitney U Test |
| cranial_base_tri_area | 1.529649920196137e-28  | 429862.5       | Mann-Whitney U Test |
| mand_vol              | 3.193897432853109e-28  | 431267.5       | Mann-Whitney U Test |
| mand_tri_area         | 6.9060105404607e-27    | 435382.0       | Mann-Whitney U Test |
| max_mand_box_area     | 1.249565144133052e-26  | 434456.5       | Mann-Whitney U Test |

### D9 = I\_GE15\_DEMDXSYMIO

| Feature                 | p-value                | Test-statistic     | Test-name           |
|-------------------------|------------------------|--------------------|---------------------|
| bmi                     | 5.547109003672217e-38  | 398904.5           | Mann-Whitney U Test |
| loud_snore              | 3.9958061444914374e-24 | 304329.5           | Mann-Whitney U Test |
| male                    | 9.147462276938349e-24  | 101.0109873113873  | Chi Square Test     |
| map_index               | 1.0236239731714e-21    | 310646.0           | Mann-Whitney U Test |
| choke                   | 9.372957385296172e-16  | 327983.0           | Mann-Whitney U Test |
| csamer                  | 4.550759920307722e-14  | 56.91493771208839  | Chi Square Test     |
| gasping                 | 7.64987826488691e-10   | 345050.0           | Mann-Whitney U Test |
| tongue_width_f_te_m     | 1.2155027739330397e-07 | 480890.5           | Mann-Whitney U Test |
| asian                   | 1.485453007400471e-07  | 27.608231086037208 | Chi Square Test     |
| tongue_thickness_p_te_m | 2.111475179835431e-07  | 484665.0           | Mann-Whitney U Test |

### D10 = J\_GE15\_DEMDXSYMCFIO

| Feature               | p-value                | Test-statistic | Test-name           |
|-----------------------|------------------------|----------------|---------------------|
| face_width            | 1.0456019441332584e-51 | 371046.5       | Mann-Whitney U Test |
| mand_width            | 1.4138297267890205e-50 | 373520.5       | Mann-Whitney U Test |
| bmi                   | 1.0818438086456103e-38 | 402018.5       | Mann-Whitney U Test |
| max_mand_vol          | 9.670980103736678e-36  | 407717.0       | Mann-Whitney U Test |
| max_tri_area          | 2.541450087867167e-34  | 412405.0       | Mann-Whitney U Test |
| cer_ang               | 8.806560696102838e-31  | 342422.0       | Mann-Whitney U Test |
| cranial_base_tri_area | 1.529649920196137e-28  | 429862.5       | Mann-Whitney U Test |
| mand_vol              | 3.193897432853109e-28  | 431267.5       | Mann-Whitney U Test |
| mand_tri_area         | 6.9060105404607e-27    | 435382.0       | Mann-Whitney U Test |
| max_mand_box_area     | 1.249565144133052e-26  | 434456.5       | Mann-Whitney U Test |

## Univariate Analysis of Each Dataset (Top 10 Features for Each): Page 3

### D11 = K\_GE5\_DEM

| Feature   | p-value                | Test-statistic     | Test-name           |
|-----------|------------------------|--------------------|---------------------|
| bmi       | 8.174211225062187e-43  | 294715.5           | Mann-Whitney U Test |
| male      | 1.7536240458986958e-16 | 67.86183983520638  | Chi Square Test     |
| age       | 3.0297735055184925e-13 | 378982.5           | Mann-Whitney U Test |
| csamer    | 2.3995020523019037e-10 | 40.11086887325932  | Chi Square Test     |
| asian     | 7.584227701175714e-05  | 15.659211361477006 | Chi Square Test     |
| aframer   | 0.0050007757272225     | 7.879158026395546  | Chi Square Test     |
| other     | 0.3344824686692011     | 0.9314652551850056 | Chi Square Test     |
| caucasian | 0.6219577202789        | 0.2431255717360346 | Chi Square Test     |

### D12 = L\_GE5\_DX

| Feature          | p-value                | Test-statistic     | Test-name       |
|------------------|------------------------|--------------------|-----------------|
| medhx_hbp        | 1.9001513332403911e-06 | 22.693443333051277 | Chi Square Test |
| medhx_dm         | 0.0004250504516488     | 12.418724486621256 | Chi Square Test |
| medhx_ldl        | 0.0038811086030071     | 8.338619100187122  | Chi Square Test |
| medhx_cad        | 0.0336632260136647     | 4.511727460751411  | Chi Square Test |
| medhx_stroke     | 0.4490145880663584     | 0.5731381472424522 | Chi Square Test |
| medhx_afib       | 0.5728854962096509     | 0.3178783185915509 | Chi Square Test |
| medhx_heart_fail | 0.6235836030881907     | 0.2408628630548689 | Chi Square Test |

### D13 = M\_GE5\_SYM

| Feature    | p-value                | Test-statistic | Test-name           |
|------------|------------------------|----------------|---------------------|
| loud_snore | 2.9470901078367264e-26 | 210278.5       | Mann-Whitney U Test |
| map_index  | 5.108187821901815e-25  | 209085.0       | Mann-Whitney U Test |
| choke      | 7.692701180983842e-16  | 235826.0       | Mann-Whitney U Test |
| gaspings   | 4.6037830784688426e-10 | 250504.0       | Mann-Whitney U Test |

### D14 = N\_GE5\_CF

| Feature               | p-value                | Test-statistic | Test-name           |
|-----------------------|------------------------|----------------|---------------------|
| mand_width            | 1.3393701011729151e-40 | 301119.0       | Mann-Whitney U Test |
| face_width            | 5.267142235112682e-38  | 307115.0       | Mann-Whitney U Test |
| cer_ang               | 6.350365104348193e-33  | 258706.5       | Mann-Whitney U Test |
| max_mand_vol          | 1.4636689241435042e-30 | 323896.5       | Mann-Whitney U Test |
| mand_vol              | 1.623254199885122e-27  | 333591.0       | Mann-Whitney U Test |
| max_tri_area          | 1.8651129514064285e-26 | 336101.0       | Mann-Whitney U Test |
| mand_tri_area         | 4.20290678553797e-24   | 343357.0       | Mann-Whitney U Test |
| lat_fac_ht            | 4.6352654751415204e-24 | 342626.0       | Mann-Whitney U Test |
| cranial_base_tri_area | 3.0334437247273095e-23 | 345693.5       | Mann-Whitney U Test |
| max_mand_box_area     | 8.271108273066063e-23  | 346783.0       | Mann-Whitney U Test |

### D15 = O\_GE5\_IO

| Feature                 | p-value               | Test-statistic     | Test-name           |
|-------------------------|-----------------------|--------------------|---------------------|
| tongue_thickness_p_te_m | 5.995536263941659e-13 | 361769.5           | Mann-Whitney U Test |
| tongue_width_f_te_m     | 6.868829440250053e-07 | 388283.5           | Mann-Whitney U Test |
| tongue_width_tim_nph    | 6.589098297641054e-06 | 320494.0           | Mann-Whitney U Test |
| mal_score_ftem_c4       | 0.0008462948680038    | 11.136849928250667 | Chi Square Test     |
| mal_score_ftem_c2       | 0.0098983591298759    | 6.653097658472456  | Chi Square Test     |
| tongue_area_p_te_m      | 0.011647351812285     | 422843.5           | Mann-Whitney U Test |
| tongue_curvature_p_te_m | 0.0342119818329418    | 481625.0           | Mann-Whitney U Test |
| open_wid_tim_nph        | 0.0454824932563639    | 429708.5           | Mann-Whitney U Test |
| open_area_tim_nph       | 0.0482015205412715    | 429450.5           | Mann-Whitney U Test |
| mal_score_ftem_c3       | 0.0606163903246592    | 3.5204389844228148 | Chi Square Test     |

## Univariate Analysis of Each Dataset (Top 10 Features for Each): Page 4

### D16 = P\_GE5\_DEMDX

| Feature   | p-value                | Test-statistic     | Test-name           |
|-----------|------------------------|--------------------|---------------------|
| bmi       | 8.222363047682099e-31  | 195395.0           | Mann-Whitney U Test |
| male      | 4.940864212277696e-14  | 56.75319915006119  | Chi Square Test     |
| age       | 4.057311159061167e-09  | 249863.0           | Mann-Whitney U Test |
| medhx_hbp | 1.8139793244436493e-06 | 22.782629005241255 | Chi Square Test     |
| asian     | 0.0003223753495614     | 12.935696029321257 | Chi Square Test     |
| medhx_dm  | 0.0004481372301081     | 12.319972804490098 | Chi Square Test     |
| csamer    | 0.0022522296235311     | 9.33170286312965   | Chi Square Test     |
| medhx_ldl | 0.0031388257879919     | 8.724962192762037  | Chi Square Test     |
| other     | 0.0233267600825835     | 5.144006089823659  | Chi Square Test     |
| aframer   | 0.024385105233409      | 5.067031717329436  | Chi Square Test     |

### D17 = Q\_GE5\_DEMDXSYM

| Feature    | p-value                | Test-statistic     | Test-name           |
|------------|------------------------|--------------------|---------------------|
| bmi        | 3.379652374764037e-31  | 201622.5           | Mann-Whitney U Test |
| loud_snore | 1.8667013832208623e-25 | 213808.0           | Mann-Whitney U Test |
| map_index  | 1.0143364282727228e-23 | 215547.5           | Mann-Whitney U Test |
| choke      | 1.521767249141592e-15  | 237437.0           | Mann-Whitney U Test |
| male       | 1.0288074897552176e-14 | 59.84019245637027  | Chi Square Test     |
| gasping    | 5.643276533262147e-10  | 250176.0           | Mann-Whitney U Test |
| age        | 5.874496693712653e-09  | 258716.0           | Mann-Whitney U Test |
| medhx_hbp  | 1.8139793244436493e-06 | 22.782629005241255 | Chi Square Test     |
| asian      | 0.0003544367676502     | 12.758279483045012 | Chi Square Test     |
| medhx_dm   | 0.0004481372301081     | 12.319972804490098 | Chi Square Test     |

### D18 = R\_GE5\_DEMDXSYCMCF

| Feature       | p-value                | Test-statistic | Test-name           |
|---------------|------------------------|----------------|---------------------|
| bmi           | 1.0604459797522213e-42 | 296375.5       | Mann-Whitney U Test |
| mand_width    | 1.3393701011729151e-40 | 301119.0       | Mann-Whitney U Test |
| face_width    | 5.267142235112682e-38  | 307115.0       | Mann-Whitney U Test |
| cer_ang       | 6.350365104348193e-33  | 258706.5       | Mann-Whitney U Test |
| max_mand_vol  | 1.4636689241435042e-30 | 323896.5       | Mann-Whitney U Test |
| mand_vol      | 1.623254199885122e-27  | 333591.0       | Mann-Whitney U Test |
| max_tri_area  | 1.8651129514064285e-26 | 336101.0       | Mann-Whitney U Test |
| loud_snore    | 1.7214821169803898e-25 | 214783.5       | Mann-Whitney U Test |
| mand_tri_area | 4.20290678553797e-24   | 343357.0       | Mann-Whitney U Test |
| lat_fac_ht    | 4.6352654751415204e-24 | 342626.0       | Mann-Whitney U Test |

### D19 = S\_GE5\_DEMDXSYMIO

| Feature                 | p-value                | Test-statistic    | Test-name           |
|-------------------------|------------------------|-------------------|---------------------|
| bmi                     | 5.811619782519763e-42  | 293407.0          | Mann-Whitney U Test |
| loud_snore              | 1.7214821169803898e-25 | 214783.5          | Mann-Whitney U Test |
| map_index               | 1.6435813725692653e-23 | 217793.5          | Mann-Whitney U Test |
| male                    | 2.288366194636403e-16  | 67.33708115720516 | Chi Square Test     |
| choke                   | 1.331628057579479e-15  | 238082.0          | Mann-Whitney U Test |
| age                     | 5.161276452115644e-13  | 376257.5          | Mann-Whitney U Test |
| tongue thickness p te m | 5.998664232296849e-13  | 360361.0          | Mann-Whitney U Test |
| csamer                  | 1.2797205050439662e-10 | 41.33926910426314 | Chi Square Test     |
| gasping                 | 5.521829753902209e-10  | 251721.0          | Mann-Whitney U Test |
| tongue width f te m     | 1.4431742102266163e-06 | 388827.5          | Mann-Whitney U Test |

### D20 = T\_GE5\_DEMDXSYCMCFIO

| Feature       | p-value                | Test-statistic | Test-name           |
|---------------|------------------------|----------------|---------------------|
| bmi           | 1.0604459797522213e-42 | 296375.5       | Mann-Whitney U Test |
| mand_width    | 1.3393701011729151e-40 | 301119.0       | Mann-Whitney U Test |
| face_width    | 5.267142235112682e-38  | 307115.0       | Mann-Whitney U Test |
| cer_ang       | 6.350365104348193e-33  | 258706.5       | Mann-Whitney U Test |
| max_mand_vol  | 1.4636689241435042e-30 | 323896.5       | Mann-Whitney U Test |
| mand_vol      | 1.623254199885122e-27  | 333591.0       | Mann-Whitney U Test |
| max_tri_area  | 1.8651129514064285e-26 | 336101.0       | Mann-Whitney U Test |
| loud_snore    | 1.7214821169803898e-25 | 214783.5       | Mann-Whitney U Test |
| mand_tri_area | 4.20290678553797e-24   | 343357.0       | Mann-Whitney U Test |
| lat_fac_ht    | 4.6352654751415204e-24 | 342626.0       | Mann-Whitney U Test |

# Dataset and Model Prediction Summary: D1 = A\_GE15\_DEM

## Data Processing/Counts Summary

|           | Instances | Total Features | Categorical Features | Quantitative Features | Missing Values | Missing Percent | Class 0 | Class 1 |
|-----------|-----------|----------------|----------------------|-----------------------|----------------|-----------------|---------|---------|
| Original  | 2178      | 8              | 6                    | 2                     | 20             | 0.0011          | 1098    | 1080    |
| C1        | 2178      | 8              | 6                    | 2                     | 20             | 0.0011          | 1098    | 1080    |
| E1        | 2178      | 8              | 6                    | 2                     | 20             | 0.0011          | 1098    | 1080    |
| C2        | 2178      | 8              | 6                    | 2                     | 20             | 0.0011          | 1098    | 1080    |
| C3        | 2174      | 8              | 6                    | 2                     | 0              | 0.0             | 1097    | 1077    |
| E2        | 2174      | 8              | 6                    | 2                     | 0              | 0.0             | 1097    | 1077    |
| C4        | 2174      | 8              | 6                    | 2                     | 0              | 0.0             | 1097    | 1077    |
| Processed | 2174      | 8              | 6                    | 2                     | 0              | 0.0             | 1097    | 1077    |

## Cleaning (C) and Engineering (E) Elements

- \* C1 - Remove instances with no outcome and features to ignore
- \* E1 - Add missingness features
- \* C2 - Remove features with invariance or high missingness
- \* C3 - Remove instances with high missingness
- \* E2 - Add one-hot-encoding of categorical features
- \* C4 - Remove highly correlated features

## Class Balance (Processed)

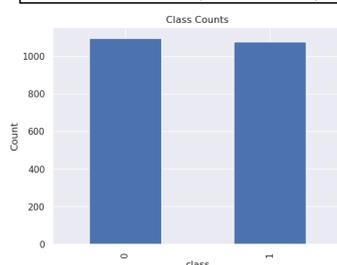

## Feature Correlations (Pearson)

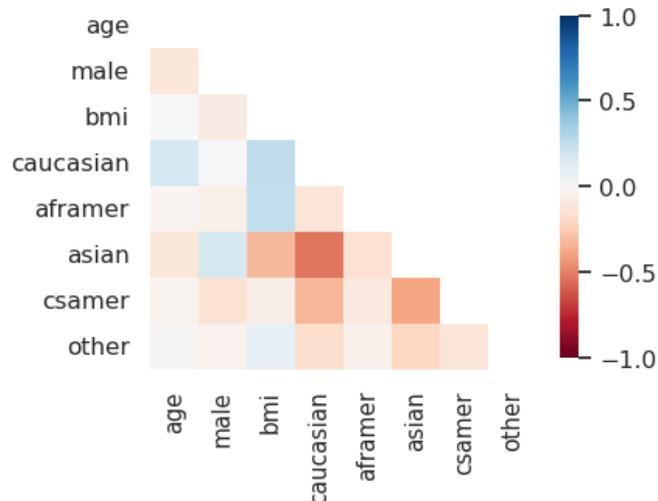

## Top ML Algorithm Results (Averaged Over CV Runs):

|                                                          |
|----------------------------------------------------------|
| Best (ROC_AUC): Category Gradient Boosting = 0.736       |
| Best (Balanced Acc.): Category Gradient Boosting = 0.670 |
| Best (F1 Score): ExSTraCS = 0.681                        |
| Best (PRC AUC): Category Gradient Boosting = 0.725       |
| Best (PRC APS): Category Gradient Boosting = 0.727       |

## ROC

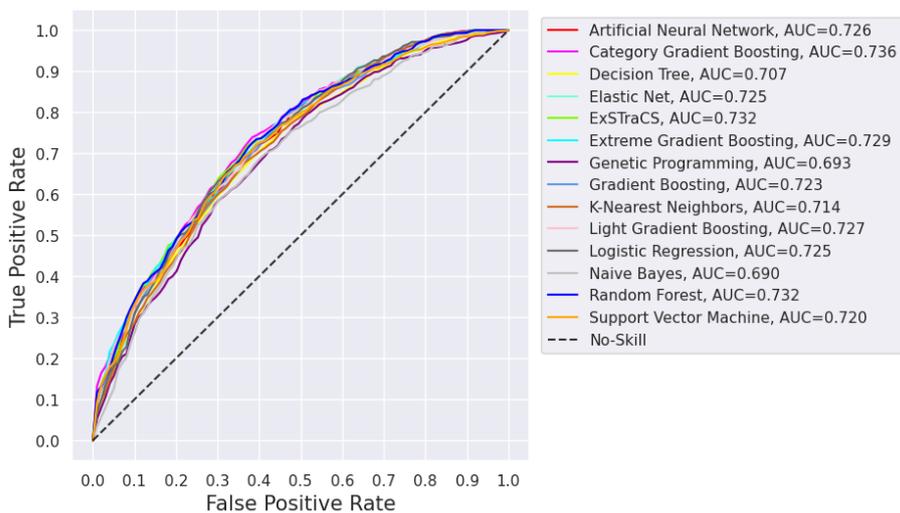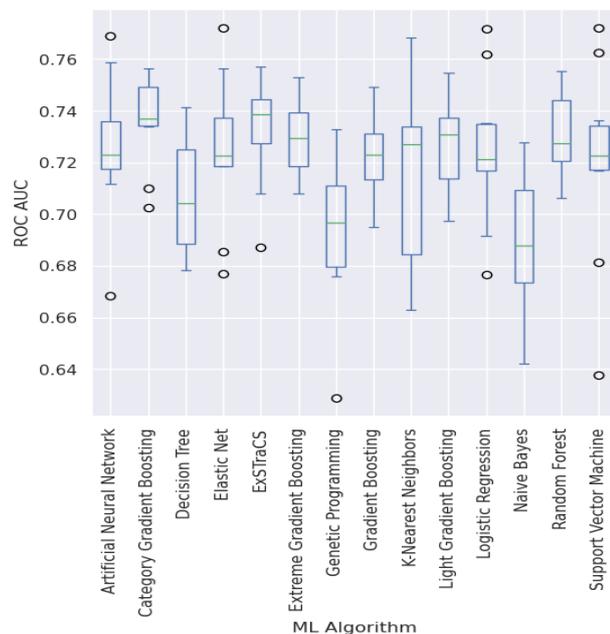

## PRC

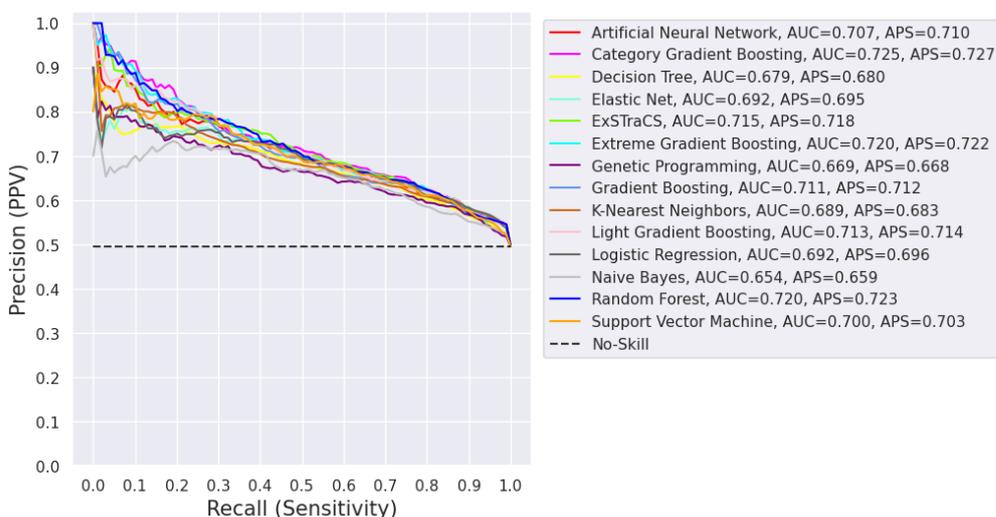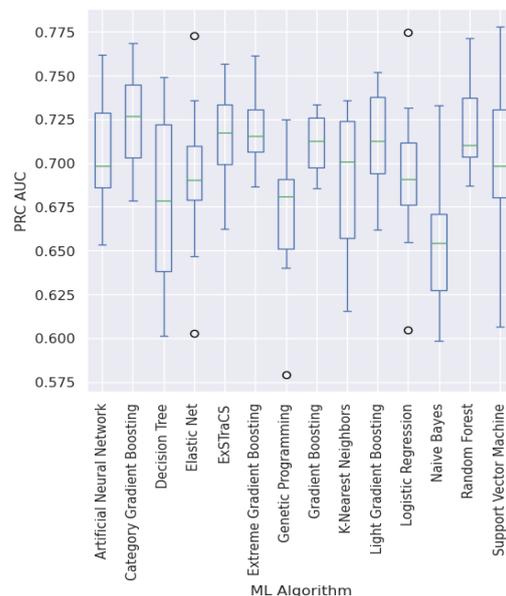

# Dataset and Model Prediction Summary: D2 = B\_GE15\_DX

## Data Processing/Counts Summary

|           | Instances | Total Features | Categorical Features | Quantitative Features | Missing Values | Missing Percent | Class 0 | Class 1 |
|-----------|-----------|----------------|----------------------|-----------------------|----------------|-----------------|---------|---------|
| Original  | 2178      | 7              | 7                    | 0                     | 2877           | 0.1887          | 1098    | 1080    |
| C1        | 2178      | 7              | 7                    | 0                     | 2877           | 0.1887          | 1098    | 1080    |
| E1        | 2178      | 7              | 7                    | 0                     | 2877           | 0.1887          | 1098    | 1080    |
| C2        | 2178      | 7              | 7                    | 0                     | 2877           | 0.1887          | 1098    | 1080    |
| C3        | 1794      | 7              | 7                    | 0                     | 229            | 0.0182          | 840     | 954     |
| E2        | 1794      | 7              | 7                    | 0                     | 229            | 0.0182          | 840     | 954     |
| C4        | 1794      | 7              | 7                    | 0                     | 229            | 0.0182          | 840     | 954     |
| Processed | 1794      | 7              | 7                    | 0                     | 229            | 0.0182          | 840     | 954     |

## Cleaning (C) and Engineering (E) Elements

- \* C1 - Remove instances with no outcome and features to ignore
- \* E1 - Add missingness features
- \* C2 - Remove features with invariance or high missingness
- \* C3 - Remove instances with high missingness
- \* E2 - Add one-hot-encoding of categorical features
- \* C4 - Remove highly correlated features

## Class Balance (Processed)

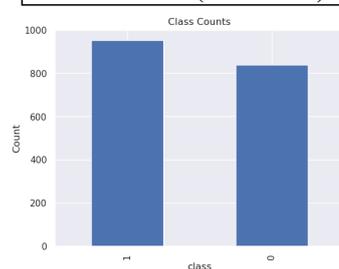

## Feature Correlations (Pearson)

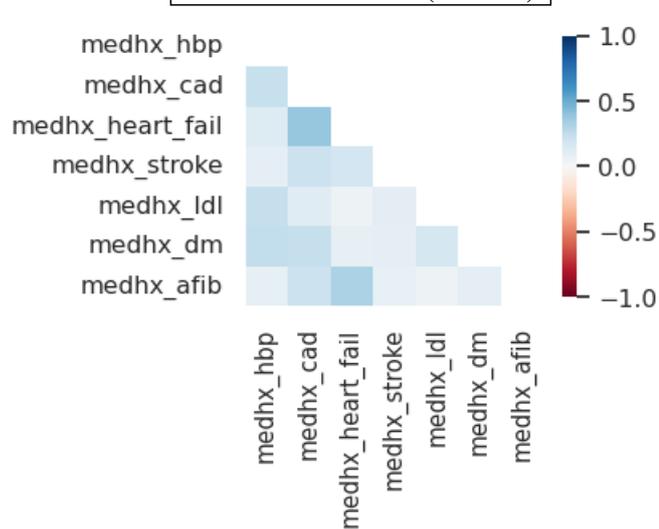

## Top ML Algorithm Results (Averaged Over CV Runs):

|                                                         |
|---------------------------------------------------------|
| Best (ROC_AUC): Naive Bayes = 0.571                     |
| Best (Balanced Acc.): Extreme Gradient Boosting = 0.560 |
| Best (F1 Score): Naive Bayes = 0.585                    |
| Best (PRC AUC): Genetic Programming = 0.679             |
| Best (PRC APS): Naive Bayes = 0.582                     |

## ROC

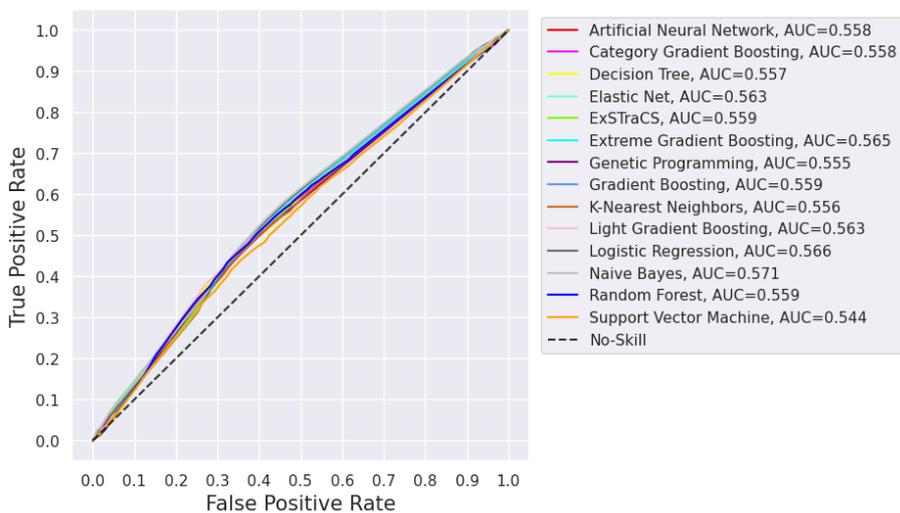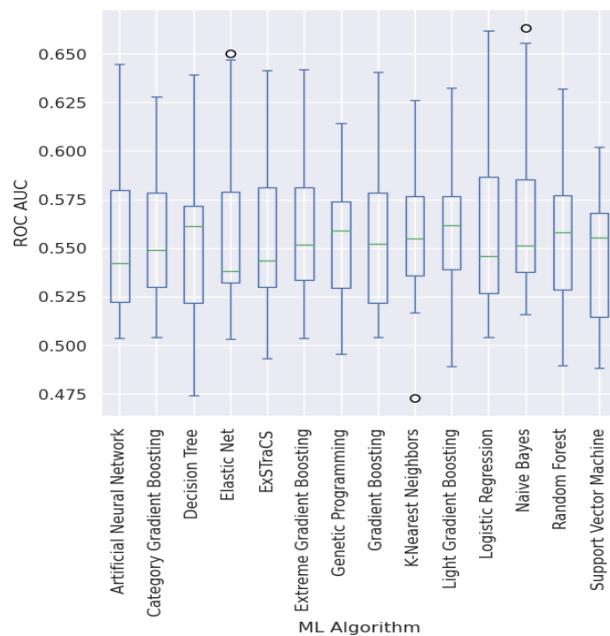

## PRC

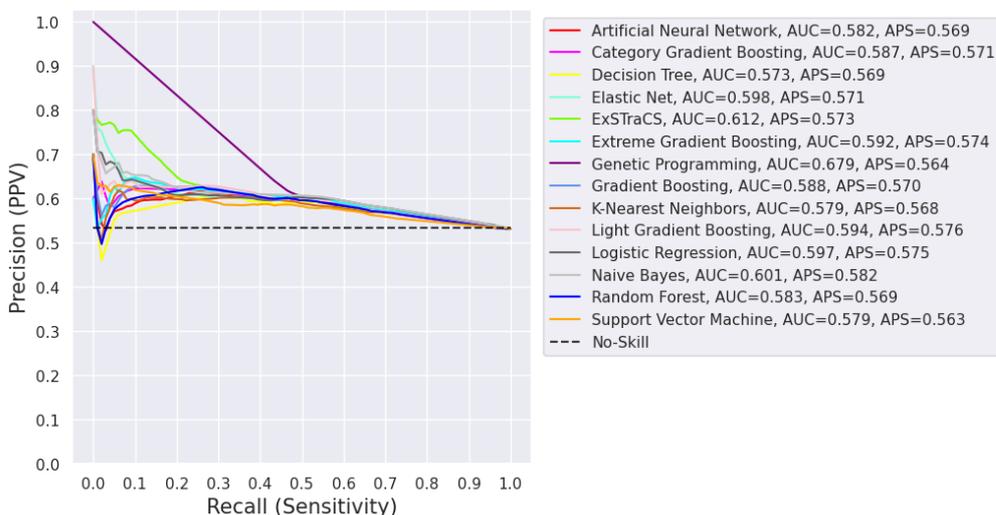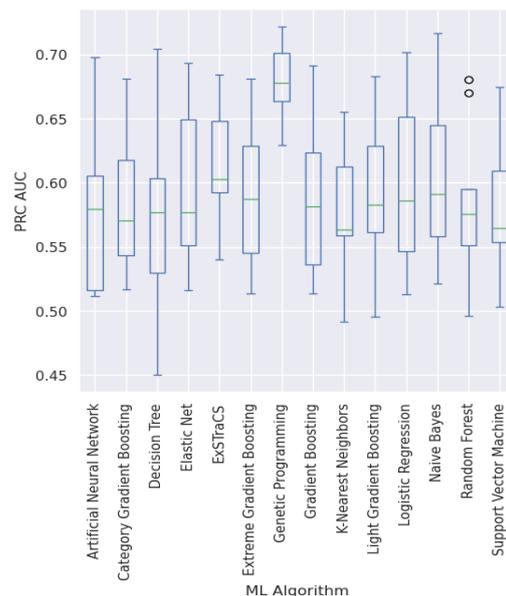

# Dataset and Model Prediction Summary: D3 = C\_GE15\_SYM

## Data Processing/Counts Summary

|           | Instances | Total Features | Categorical Features | Quantitative Features | Missing Values | Missing Percent | Class 0 | Class 1 |
|-----------|-----------|----------------|----------------------|-----------------------|----------------|-----------------|---------|---------|
| Original  | 2178      | 4              | 0                    | 4                     | 1442           | 0.1655          | 1098    | 1080    |
| C1        | 2178      | 4              | 0                    | 4                     | 1442           | 0.1655          | 1098    | 1080    |
| E1        | 2178      | 4              | 0                    | 4                     | 1442           | 0.1655          | 1098    | 1080    |
| C2        | 2178      | 4              | 0                    | 4                     | 1442           | 0.1655          | 1098    | 1080    |
| C3        | 1810      | 4              | 0                    | 4                     | 10             | 0.0014          | 855     | 955     |
| E2        | 1810      | 4              | 0                    | 4                     | 10             | 0.0014          | 855     | 955     |
| C4        | 1810      | 4              | 0                    | 4                     | 10             | 0.0014          | 855     | 955     |
| Processed | 1810      | 4              | 0                    | 4                     | 10             | 0.0014          | 855     | 955     |

## Cleaning (C) and Engineering (E) Elements

- \* C1 - Remove instances with no outcome and features to ignore
- \* E1 - Add missingness features
- \* C2 - Remove features with invariance or high missingness
- \* C3 - Remove instances with high missingness
- \* E2 - Add one-hot-encoding of categorical features
- \* C4 - Remove highly correlated features

## Class Balance (Processed)

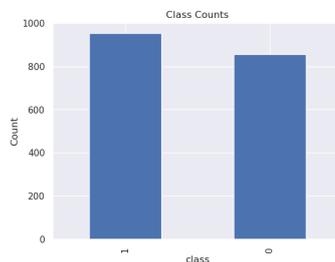

## Feature Correlations (Pearson)

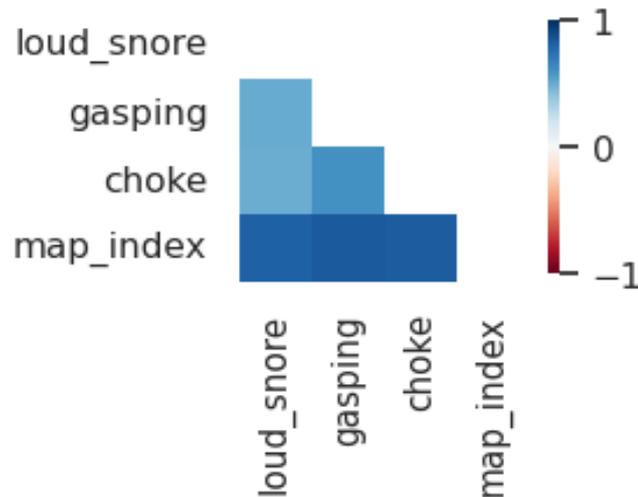

## Top ML Algorithm Results (Averaged Over CV Runs):

- Best (ROC\_AUC): Category Gradient Boosting = 0.649
- Best (Balanced Acc.): Light Gradient Boosting = 0.623
- Best (F1 Score): Gradient Boosting = 0.629
- Best (PRC AUC): Genetic Programming = 0.704
- Best (PRC APS): Elastic Net = 0.669

## ROC

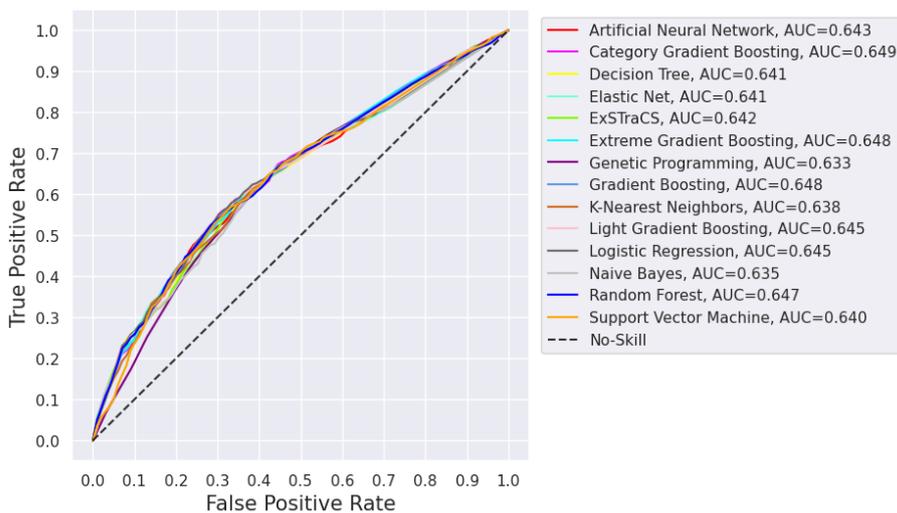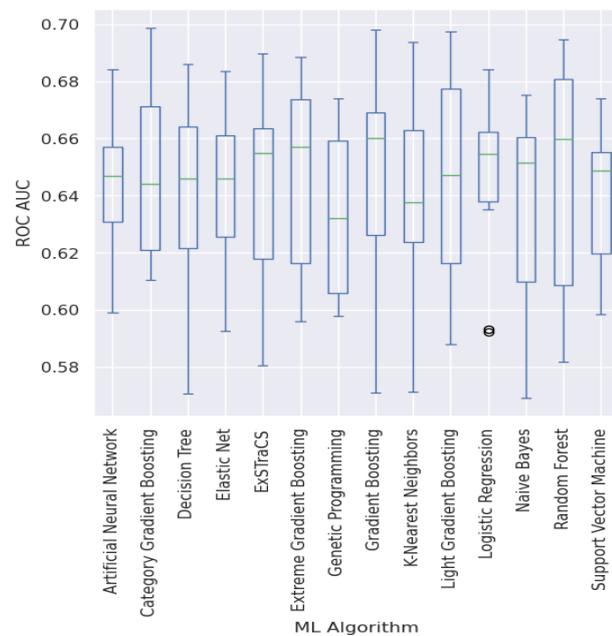

## PRC

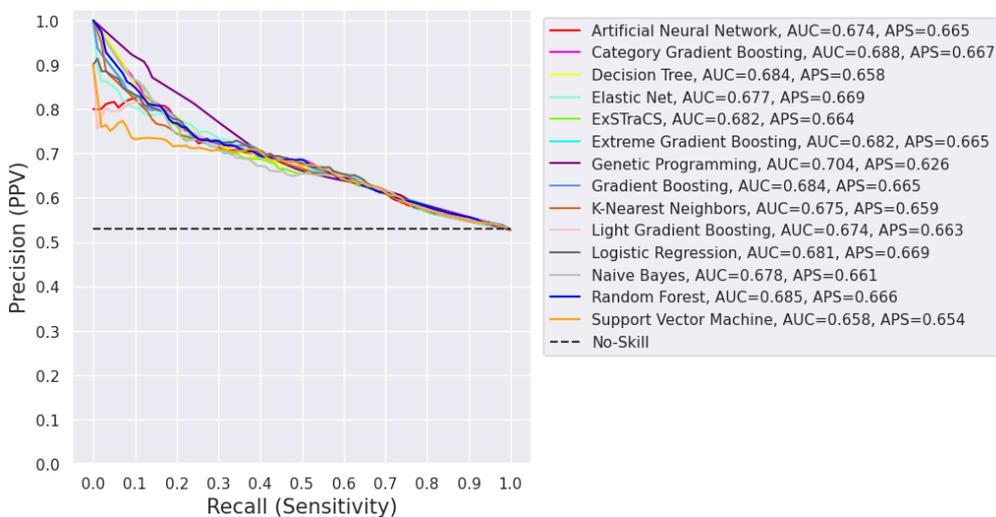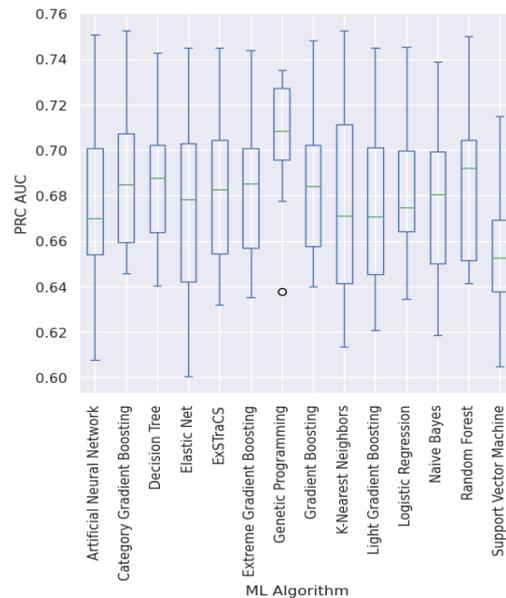

# Dataset and Model Prediction Summary: D4 = D\_GE15\_CF

## Data Processing/Counts Summary

|           | Instances | Total Features | Categorical Features | Quantitative Features | Missing Values | Missing Percent | Class 0 | Class 1 |
|-----------|-----------|----------------|----------------------|-----------------------|----------------|-----------------|---------|---------|
| Original  | 2178      | 46             | 0                    | 46                    | 360            | 0.0036          | 1098    | 1080    |
| C1        | 2178      | 46             | 0                    | 46                    | 360            | 0.0036          | 1098    | 1080    |
| E1        | 2178      | 46             | 0                    | 46                    | 360            | 0.0036          | 1098    | 1080    |
| C2        | 2178      | 46             | 0                    | 46                    | 360            | 0.0036          | 1098    | 1080    |
| C3        | 2178      | 46             | 0                    | 46                    | 360            | 0.0036          | 1098    | 1080    |
| E2        | 2178      | 46             | 0                    | 46                    | 360            | 0.0036          | 1098    | 1080    |
| C4        | 2178      | 46             | 0                    | 46                    | 360            | 0.0036          | 1098    | 1080    |
| Processed | 2178      | 46             | 0                    | 46                    | 360            | 0.0036          | 1098    | 1080    |

## Cleaning (C) and Engineering (E) Elements

- \* C1 - Remove instances with no outcome and features to ignore
- \* E1 - Add missingness features
- \* C2 - Remove features with invariance or high missingness
- \* C3 - Remove instances with high missingness
- \* E2 - Add one-hot-encoding of categorical features
- \* C4 - Remove highly correlated features

## Class Balance (Processed)

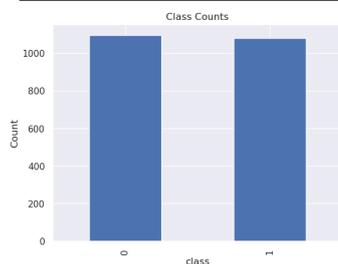

## Feature Correlations (Pearson)

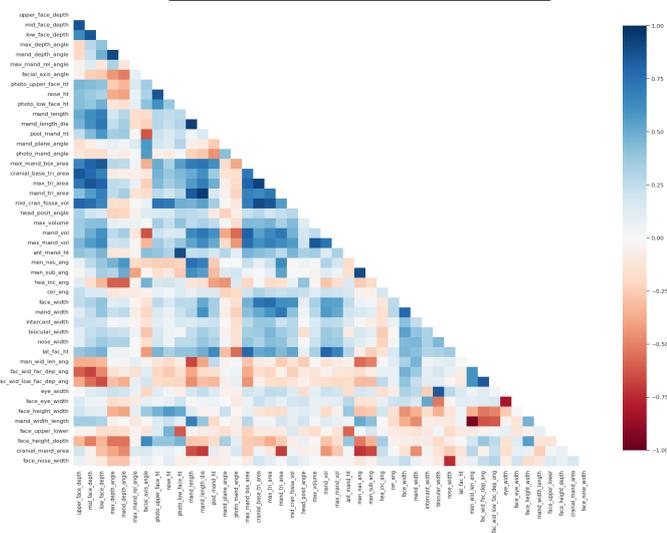

## Top ML Algorithm Results (Averaged Over CV Runs):

|                                                    |
|----------------------------------------------------|
| Best (ROC_AUC): Elastic Net = 0.729                |
| Best (Balanced Acc.): Elastic Net = 0.670          |
| Best (F1 Score): Artificial Neural Network = 0.670 |
| Best (PRC AUC): Category Gradient Boosting = 0.714 |
| Best (PRC APS): Category Gradient Boosting = 0.717 |

## ROC

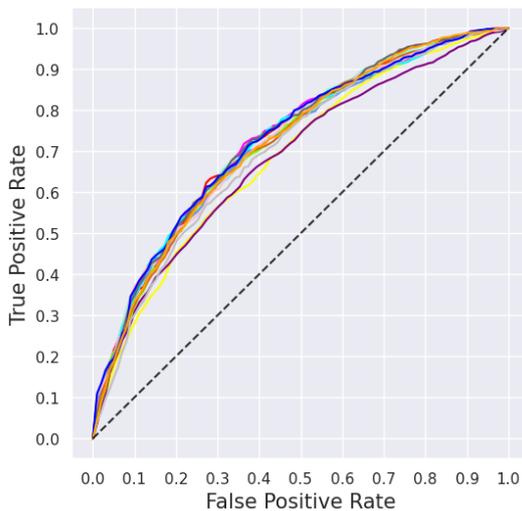

- Artificial Neural Network, AUC=0.726
- Category Gradient Boosting, AUC=0.727
- Decision Tree, AUC=0.684
- Elastic Net, AUC=0.729
- ExStrACS, AUC=0.716
- Extreme Gradient Boosting, AUC=0.723
- Genetic Programming, AUC=0.681
- Gradient Boosting, AUC=0.717
- K-Nearest Neighbors, AUC=0.718
- Light Gradient Boosting, AUC=0.722
- Logistic Regression, AUC=0.728
- Naive Bayes, AUC=0.701
- Random Forest, AUC=0.727
- Support Vector Machine, AUC=0.719
- No-Skill

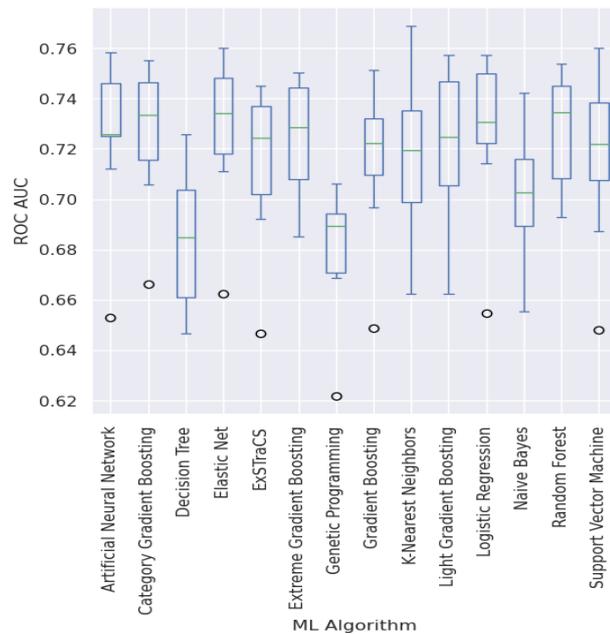

## PRC

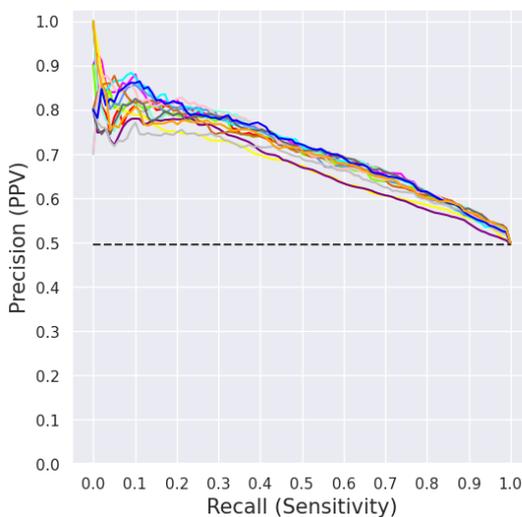

- Artificial Neural Network, AUC=0.705, APS=0.708
- Category Gradient Boosting, AUC=0.714, APS=0.717
- Decision Tree, AUC=0.672, APS=0.663
- Elastic Net, AUC=0.706, APS=0.708
- ExStrACS, AUC=0.698, APS=0.702
- Extreme Gradient Boosting, AUC=0.711, APS=0.714
- Genetic Programming, AUC=0.667, APS=0.665
- Gradient Boosting, AUC=0.704, APS=0.708
- K-Nearest Neighbors, AUC=0.701, APS=0.701
- Light Gradient Boosting, AUC=0.709, APS=0.712
- Logistic Regression, AUC=0.703, APS=0.707
- Naive Bayes, AUC=0.673, APS=0.677
- Random Forest, AUC=0.712, APS=0.716
- Support Vector Machine, AUC=0.696, APS=0.700
- No-Skill

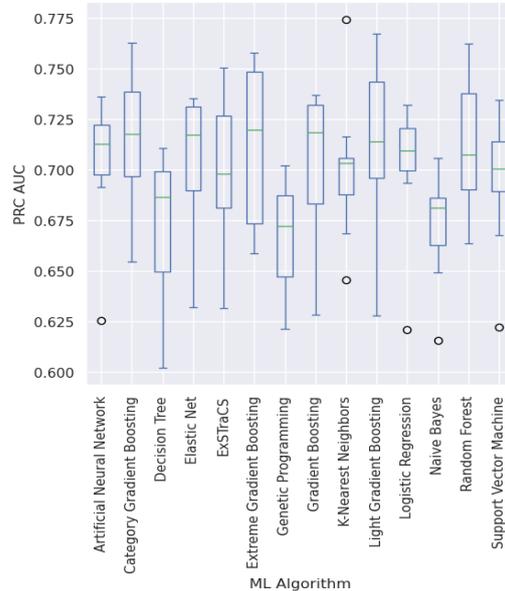

# Dataset and Model Prediction Summary: D5 = E\_GE15\_IO

## Data Processing/Counts Summary

|           | Instances | Total Features | Categorical Features | Quantitative Features | Missing Values | Missing Percent | Class 0 | Class 1 |
|-----------|-----------|----------------|----------------------|-----------------------|----------------|-----------------|---------|---------|
| Original  | 2178      | 20             | 8                    | 12                    | 2183           | 0.0501          | 1098    | 1080    |
| C1        | 2178      | 20             | 8                    | 12                    | 2183           | 0.0501          | 1098    | 1080    |
| E1        | 2178      | 20             | 8                    | 12                    | 2183           | 0.0501          | 1098    | 1080    |
| C2        | 2178      | 20             | 8                    | 12                    | 2183           | 0.0501          | 1098    | 1080    |
| C3        | 2139      | 20             | 8                    | 12                    | 1719           | 0.0402          | 1090    | 1049    |
| E2        | 2139      | 20             | 8                    | 12                    | 1719           | 0.0402          | 1090    | 1049    |
| C4        | 2139      | 20             | 8                    | 12                    | 1719           | 0.0402          | 1090    | 1049    |
| Processed | 2139      | 20             | 8                    | 12                    | 1719           | 0.0402          | 1090    | 1049    |

## Cleaning (C) and Engineering (E) Elements

- \* C1 - Remove instances with no outcome and features to ignore
- \* E1 - Add missingness features
- \* C2 - Remove features with invariance or high missingness
- \* C3 - Remove instances with high missingness
- \* E2 - Add one-hot-encoding of categorical features
- \* C4 - Remove highly correlated features

## Class Balance (Processed)

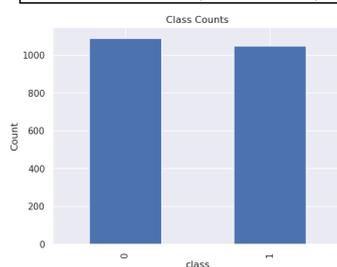

## Feature Correlations (Pearson)

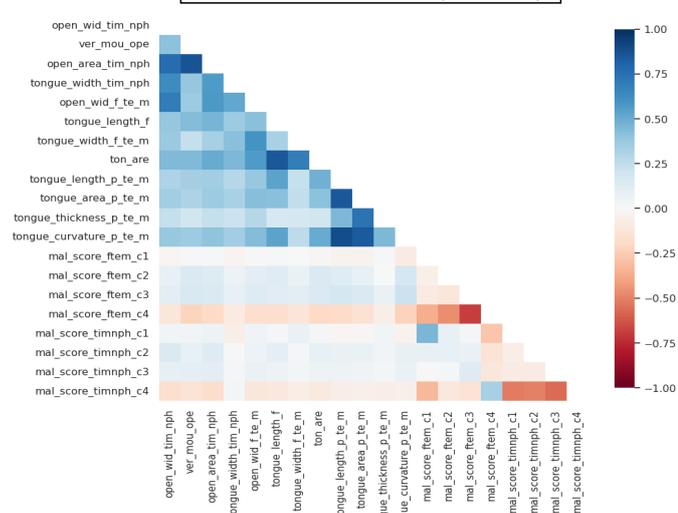

## Top ML Algorithm Results (Averaged Over CV Runs):

Best (ROC\_AUC): Logistic Regression = 0.640

Best (Balanced Acc.): Logistic Regression = 0.602

Best (F1 Score): Logistic Regression = 0.596

Best (PRC AUC): Support Vector Machine = 0.624

Best (PRC APS): Artificial Neural Network = 0.628

## ROC

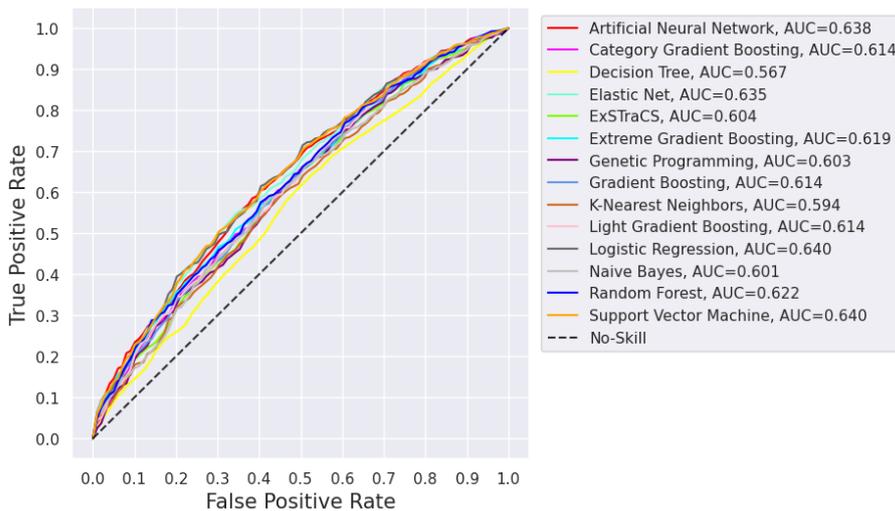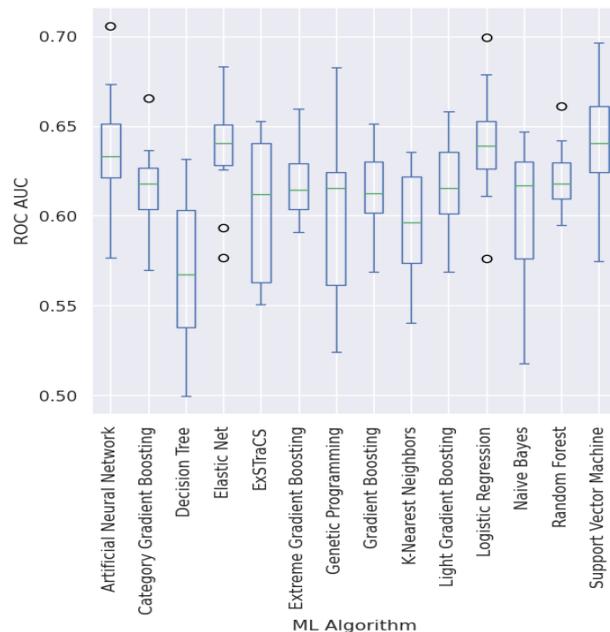

## PRC

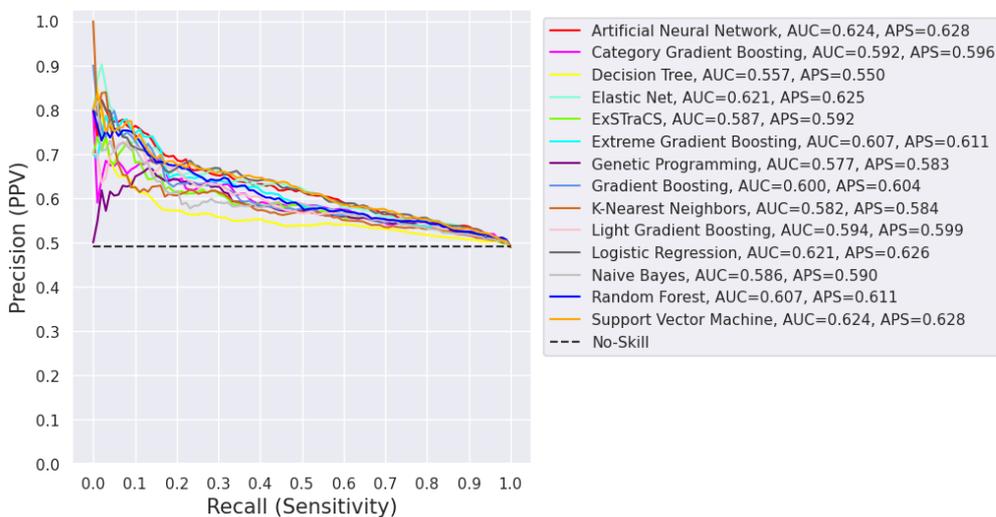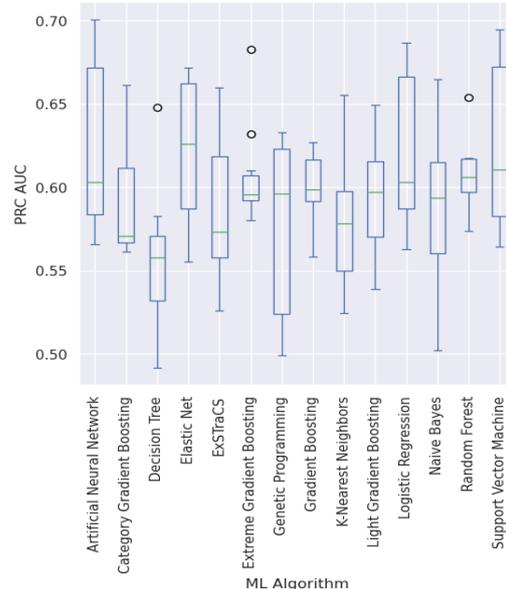

# Dataset and Model Prediction Summary: D6 = F\_GE15\_DEMDX

## Data Processing/Counts Summary

|           | Instances | Total Features | Categorical Features | Quantitative Features | Missing Values | Missing Percent | Class 0 | Class 1 |
|-----------|-----------|----------------|----------------------|-----------------------|----------------|-----------------|---------|---------|
| Original  | 2178      | 15             | 13                   | 2                     | 2897           | 0.0887          | 1098    | 1080    |
| C1        | 2178      | 15             | 13                   | 2                     | 2897           | 0.0887          | 1098    | 1080    |
| E1        | 2178      | 15             | 13                   | 2                     | 2897           | 0.0887          | 1098    | 1080    |
| C2        | 2178      | 15             | 13                   | 2                     | 2897           | 0.0887          | 1098    | 1080    |
| C3        | 1810      | 15             | 13                   | 2                     | 306            | 0.0113          | 852     | 958     |
| E2        | 1810      | 15             | 13                   | 2                     | 306            | 0.0113          | 852     | 958     |
| C4        | 1810      | 15             | 13                   | 2                     | 306            | 0.0113          | 852     | 958     |
| Processed | 1810      | 15             | 13                   | 2                     | 306            | 0.0113          | 852     | 958     |

## Cleaning (C) and Engineering (E) Elements

- \* C1 - Remove instances with no outcome and features to ignore
- \* E1 - Add missingness features
- \* C2 - Remove features with invariance or high missingness
- \* C3 - Remove instances with high missingness
- \* E2 - Add one-hot-encoding of categorical features
- \* C4 - Remove highly correlated features

## Class Balance (Processed)

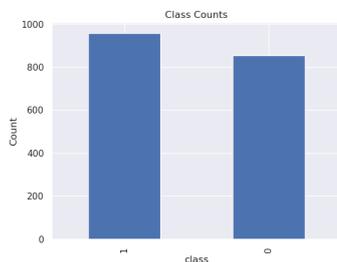

## Feature Correlations (Pearson)

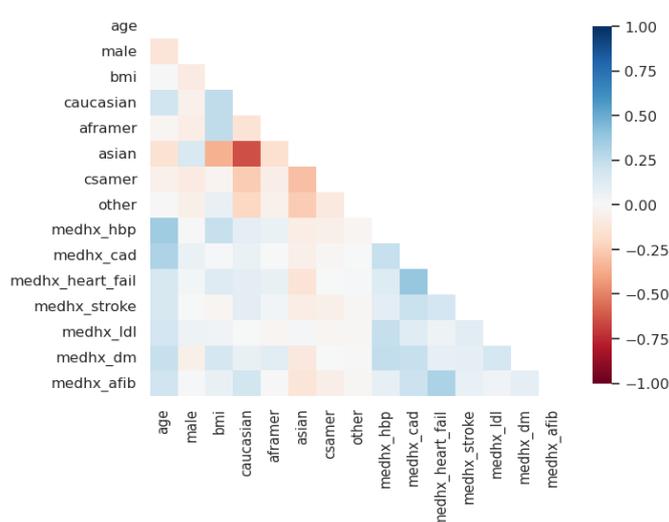

## Top ML Algorithm Results (Averaged Over CV Runs):

|                                                         |
|---------------------------------------------------------|
| Best (ROC_AUC): Category Gradient Boosting = 0.719      |
| Best (Balanced Acc.): Extreme Gradient Boosting = 0.661 |
| Best (F1 Score): Category Gradient Boosting = 0.695     |
| Best (PRC AUC): Category Gradient Boosting = 0.736      |
| Best (PRC APS): Category Gradient Boosting = 0.738      |

## ROC

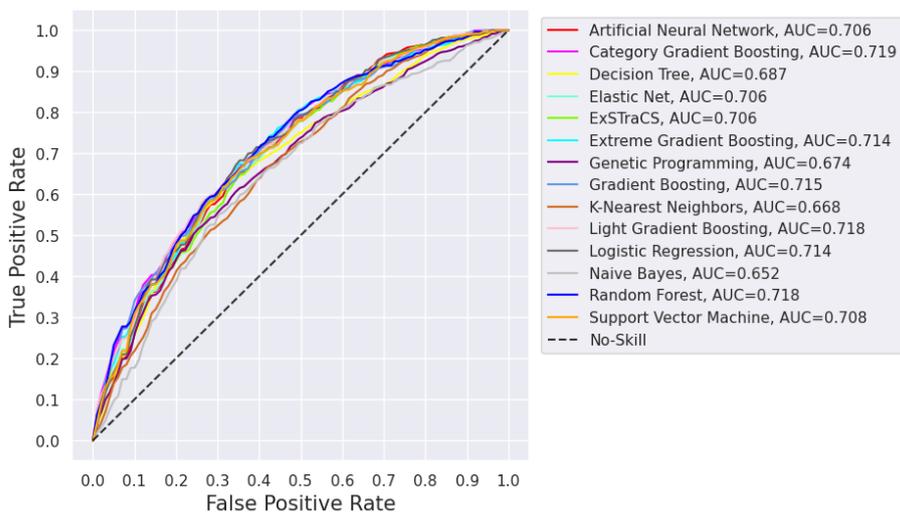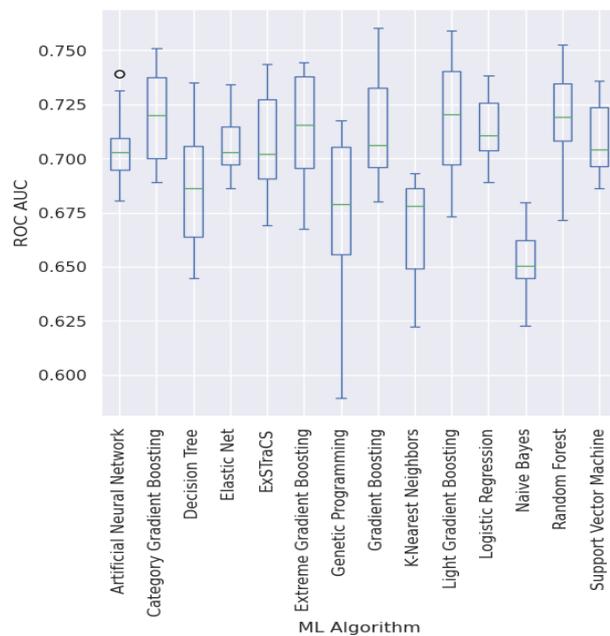

## PRC

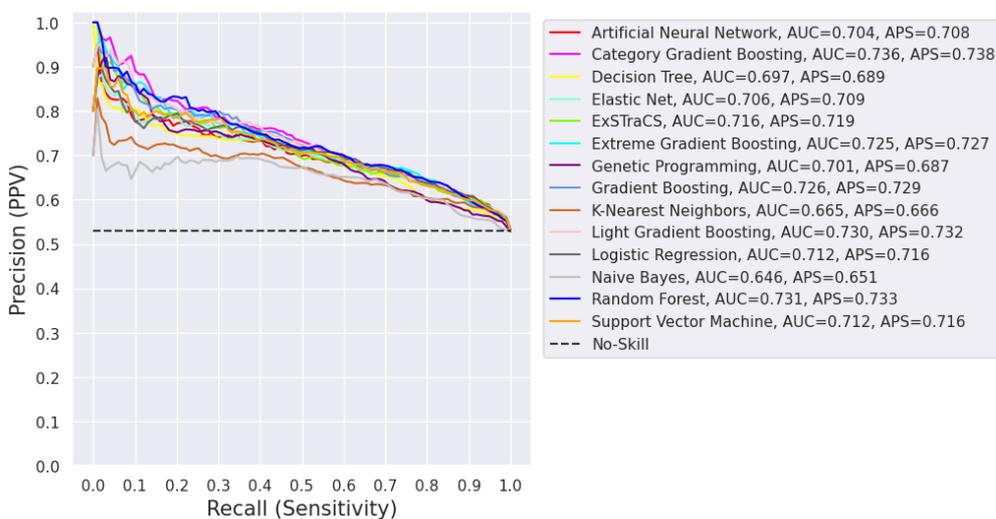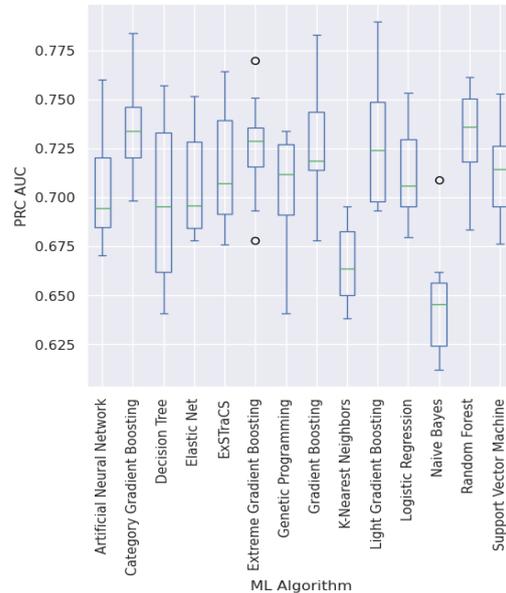

# Dataset and Model Prediction Summary: D7 = G\_GE15\_DEMDXSYM

## Data Processing/Counts Summary

|           | Instances | Total Features | Categorical Features | Quantitative Features | Missing Values | Missing Percent | Class 0 | Class 1 |
|-----------|-----------|----------------|----------------------|-----------------------|----------------|-----------------|---------|---------|
| Original  | 2178      | 19             | 13                   | 6                     | 4339           | 0.1048          | 1098    | 1080    |
| C1        | 2178      | 19             | 13                   | 6                     | 4339           | 0.1048          | 1098    | 1080    |
| E1        | 2178      | 19             | 13                   | 6                     | 4339           | 0.1048          | 1098    | 1080    |
| C2        | 2178      | 19             | 13                   | 6                     | 4339           | 0.1048          | 1098    | 1080    |
| C3        | 1834      | 19             | 13                   | 6                     | 546            | 0.0157          | 867     | 967     |
| E2        | 1834      | 19             | 13                   | 6                     | 546            | 0.0157          | 867     | 967     |
| C4        | 1834      | 19             | 13                   | 6                     | 546            | 0.0157          | 867     | 967     |
| Processed | 1834      | 19             | 13                   | 6                     | 546            | 0.0157          | 867     | 967     |

## Cleaning (C) and Engineering (E) Elements

- \* C1 - Remove instances with no outcome and features to ignore
- \* E1 - Add missingness features
- \* C2 - Remove features with invariance or high missingness
- \* C3 - Remove instances with high missingness
- \* E2 - Add one-hot-encoding of categorical features
- \* C4 - Remove highly correlated features

## Class Balance (Processed)

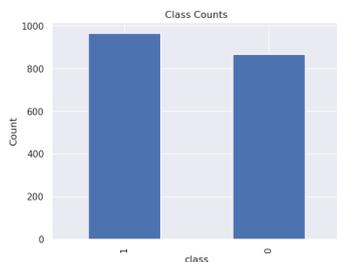

## Feature Correlations (Pearson)

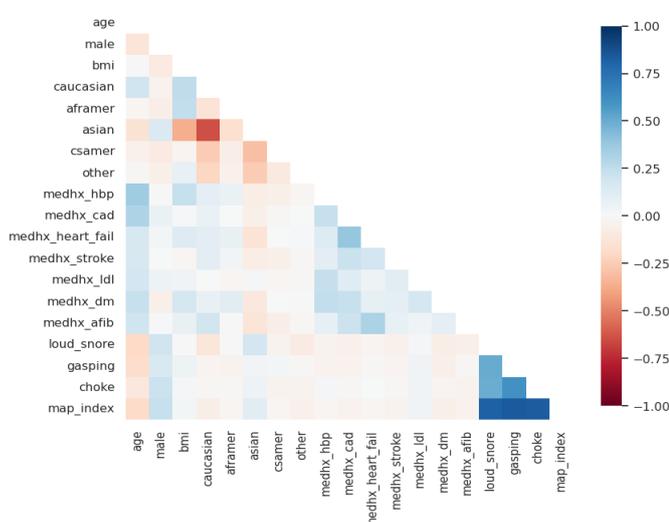

## Top ML Algorithm Results (Averaged Over CV Runs):

- Best (ROC\_AUC): Extreme Gradient Boosting = 0.739
- Best (Balanced Acc.): ExSTraCS = 0.677
- Best (F1 Score): Gradient Boosting = 0.710
- Best (PRC AUC): Extreme Gradient Boosting = 0.748
- Best (PRC APS): Extreme Gradient Boosting = 0.751

## ROC

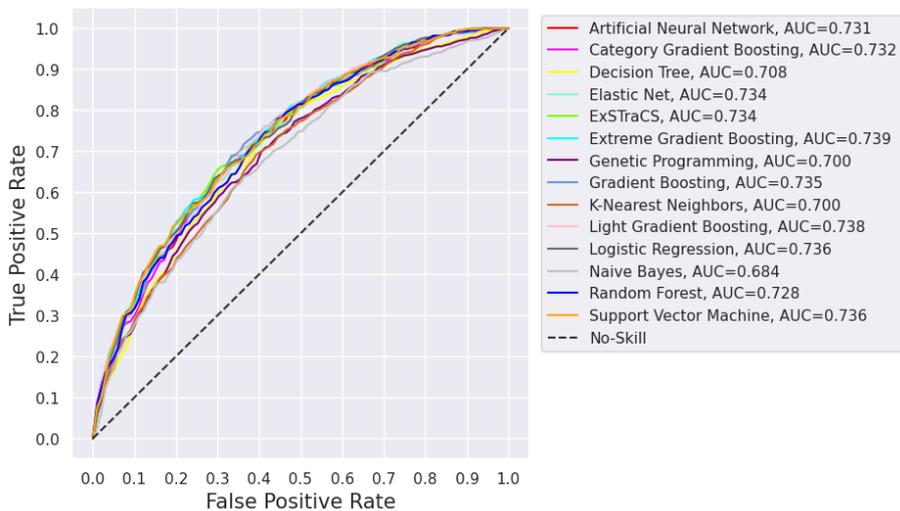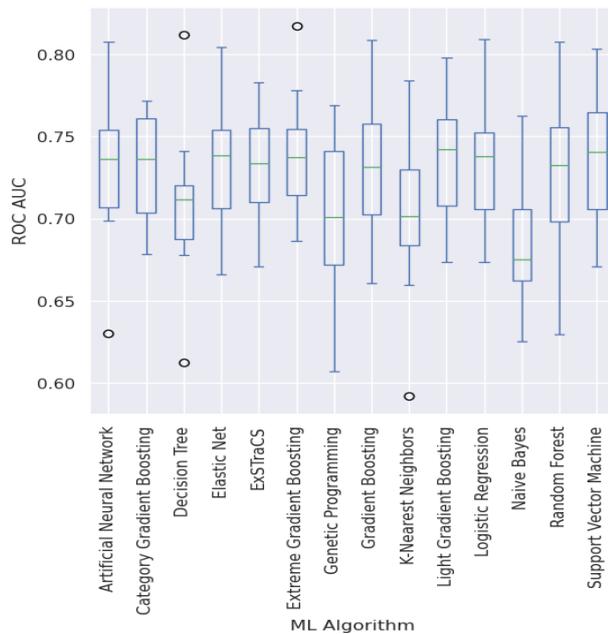

## PRC

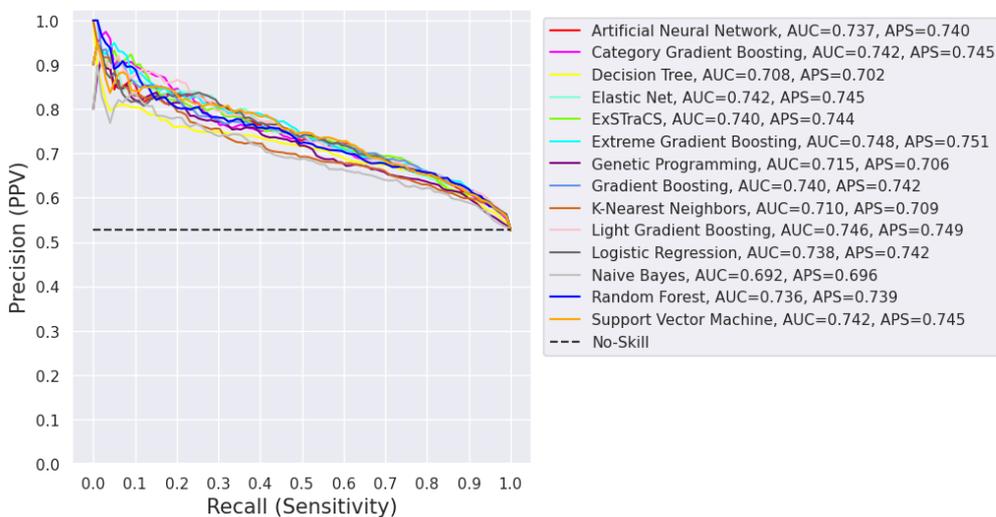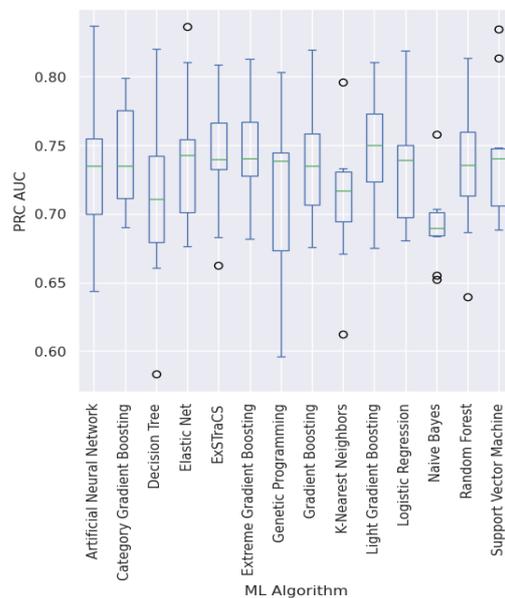

# Dataset and Model Prediction Summary: D8 = H\_GE15\_DEMDXSYMCF

## Data Processing/Counts Summary

|           | Instances | Total Features | Categorical Features | Quantitative Features | Missing Values | Missing Percent | Class 0 | Class 1 |
|-----------|-----------|----------------|----------------------|-----------------------|----------------|-----------------|---------|---------|
| Original  | 2178      | 65             | 13                   | 52                    | 4699           | 0.0332          | 1098    | 1080    |
| C1        | 2178      | 65             | 13                   | 52                    | 4699           | 0.0332          | 1098    | 1080    |
| E1        | 2178      | 65             | 13                   | 52                    | 4699           | 0.0332          | 1098    | 1080    |
| C2        | 2178      | 65             | 13                   | 52                    | 4699           | 0.0332          | 1098    | 1080    |
| C3        | 2178      | 65             | 13                   | 52                    | 4699           | 0.0332          | 1098    | 1080    |
| E2        | 2178      | 65             | 13                   | 52                    | 4699           | 0.0332          | 1098    | 1080    |
| C4        | 2178      | 65             | 13                   | 52                    | 4699           | 0.0332          | 1098    | 1080    |
| Processed | 2178      | 65             | 13                   | 52                    | 4699           | 0.0332          | 1098    | 1080    |

## Cleaning (C) and Engineering (E) Elements

- \* C1 - Remove instances with no outcome and features to ignore
- \* E1 - Add missingness features
- \* C2 - Remove features with invariance or high missingness
- \* C3 - Remove instances with high missingness
- \* E2 - Add one-hot-encoding of categorical features
- \* C4 - Remove highly correlated features

## Class Balance (Processed)

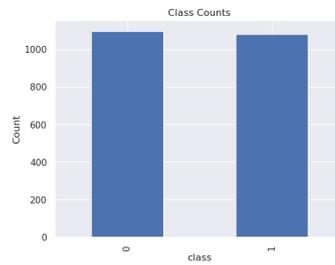

## Feature Correlations (Pearson)

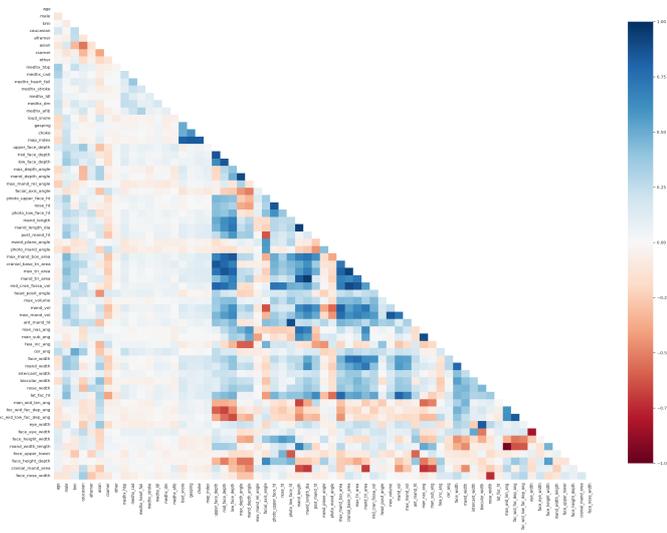

## Top ML Algorithm Results (Averaged Over CV Runs):

Best (ROC\_AUC): Logistic Regression = 0.765

Best (Balanced Acc.): ExSTraCS = 0.691

Best (F1 Score): ExSTraCS = 0.704

Best (PRC AUC): Random Forest = 0.750

Best (PRC APS): Random Forest = 0.752

## ROC

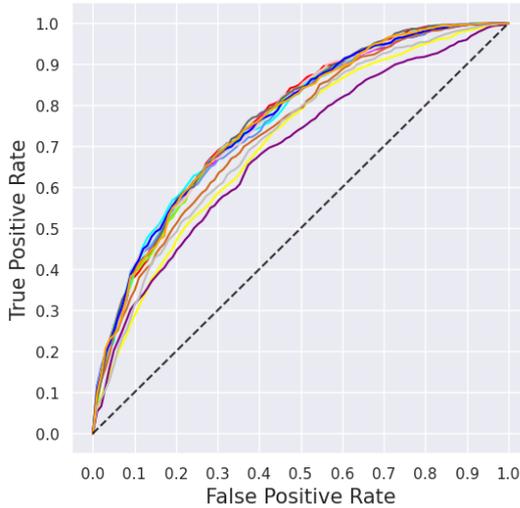

- Artificial Neural Network, AUC=0.764
- Category Gradient Boosting, AUC=0.761
- Decision Tree, AUC=0.707
- Elastic Net, AUC=0.762
- ExSTraCS, AUC=0.759
- Extreme Gradient Boosting, AUC=0.763
- Genetic Programming, AUC=0.685
- Gradient Boosting, AUC=0.757
- K-Nearest Neighbors, AUC=0.737
- Light Gradient Boosting, AUC=0.763
- Logistic Regression, AUC=0.765
- Naive Bayes, AUC=0.718
- Random Forest, AUC=0.763
- Support Vector Machine, AUC=0.760
- No-Skill

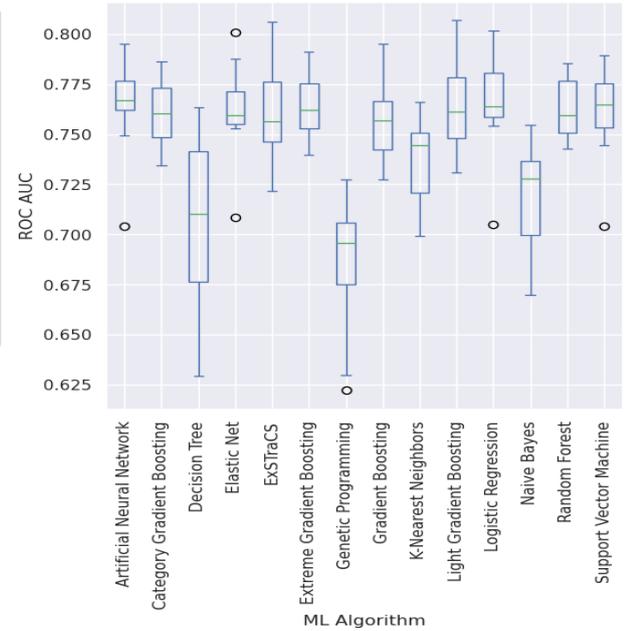

## PRC

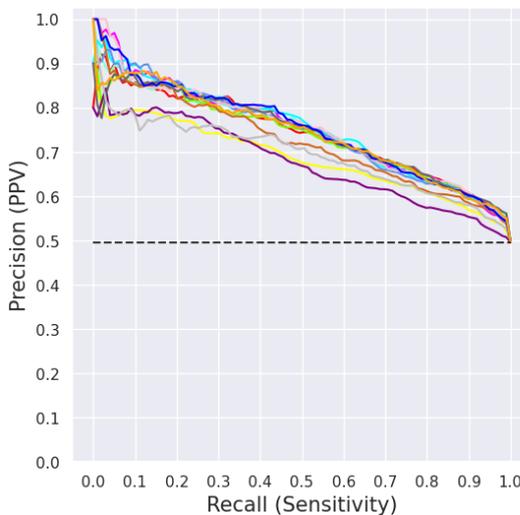

- Artificial Neural Network, AUC=0.741, APS=0.744
- Category Gradient Boosting, AUC=0.749, APS=0.751
- Decision Tree, AUC=0.684, APS=0.676
- Elastic Net, AUC=0.745, APS=0.746
- ExSTraCS, AUC=0.738, APS=0.741
- Extreme Gradient Boosting, AUC=0.750, APS=0.752
- Genetic Programming, AUC=0.674, APS=0.675
- Gradient Boosting, AUC=0.745, APS=0.748
- K-Nearest Neighbors, AUC=0.724, APS=0.724
- Light Gradient Boosting, AUC=0.750, APS=0.752
- Logistic Regression, AUC=0.743, APS=0.746
- Naive Bayes, AUC=0.693, APS=0.695
- Random Forest, AUC=0.750, APS=0.752
- Support Vector Machine, AUC=0.742, APS=0.745
- No-Skill

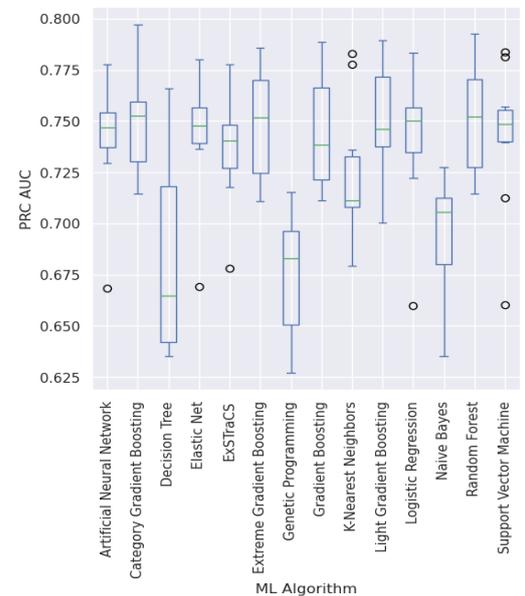

# Dataset and Model Prediction Summary: D9 = I\_GE15\_DEMDXSYMIO

## Data Processing/Counts Summary

|           | Instances | Total Features | Categorical Features | Quantitative Features | Missing Values | Missing Percent | Class 0 | Class 1 |
|-----------|-----------|----------------|----------------------|-----------------------|----------------|-----------------|---------|---------|
| Original  | 2178      | 39             | 21                   | 18                    | 6522           | 0.0768          | 1098    | 1080    |
| C1        | 2178      | 39             | 21                   | 18                    | 6522           | 0.0768          | 1098    | 1080    |
| E1        | 2178      | 39             | 21                   | 18                    | 6522           | 0.0768          | 1098    | 1080    |
| C2        | 2178      | 39             | 21                   | 18                    | 6522           | 0.0768          | 1098    | 1080    |
| C3        | 2166      | 39             | 21                   | 18                    | 6281           | 0.0743          | 1092    | 1074    |
| E2        | 2166      | 39             | 21                   | 18                    | 6281           | 0.0743          | 1092    | 1074    |
| C4        | 2166      | 39             | 21                   | 18                    | 6281           | 0.0743          | 1092    | 1074    |
| Processed | 2166      | 39             | 21                   | 18                    | 6281           | 0.0743          | 1092    | 1074    |

## Cleaning (C) and Engineering (E) Elements

- \* C1 - Remove instances with no outcome and features to ignore
- \* E1 - Add missingness features
- \* C2 - Remove features with invariance or high missingness
- \* C3 - Remove instances with high missingness
- \* E2 - Add one-hot-encoding of categorical features
- \* C4 - Remove highly correlated features

## Class Balance (Processed)

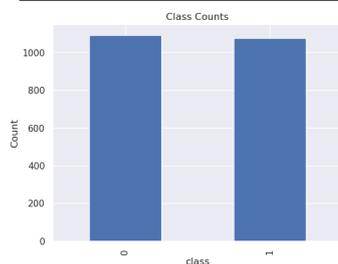

## Feature Correlations (Pearson)

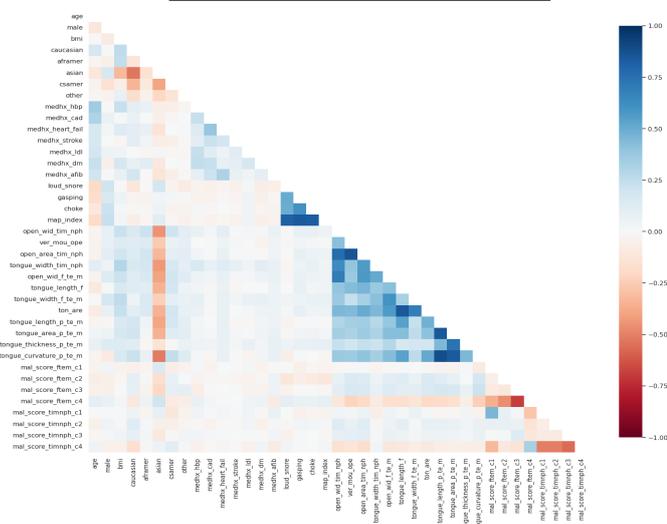

## Top ML Algorithm Results (Averaged Over CV Runs):

Best (ROC\_AUC): ExSTraCS = 0.752

Best (Balanced Acc.): Random Forest = 0.678

Best (F1 Score): Random Forest = 0.689

Best (PRC AUC): ExSTraCS = 0.739

Best (PRC APS): ExSTraCS = 0.741

## ROC

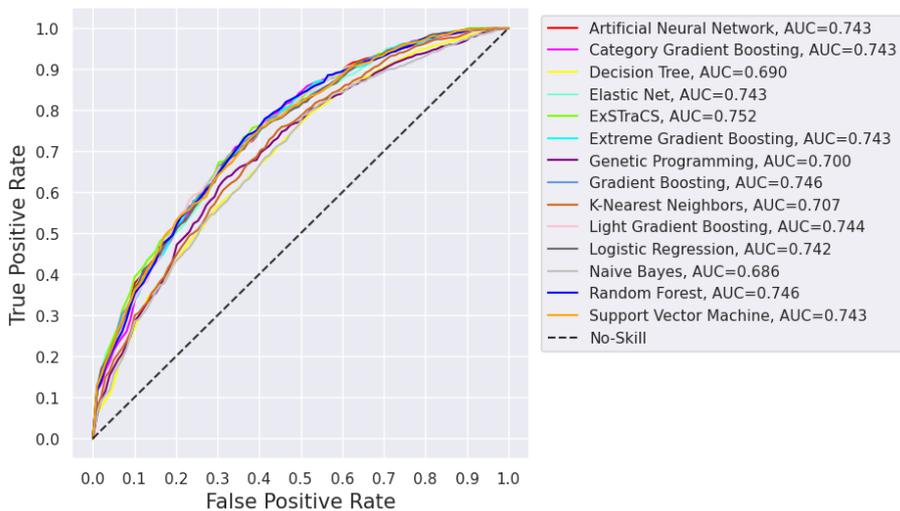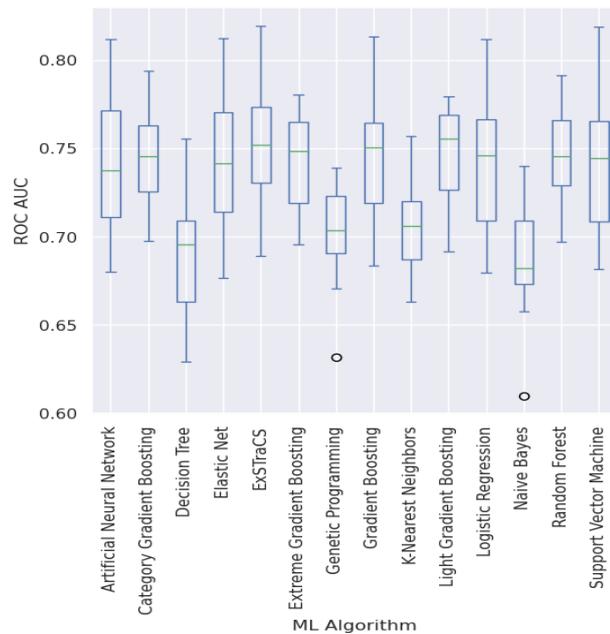

## PRC

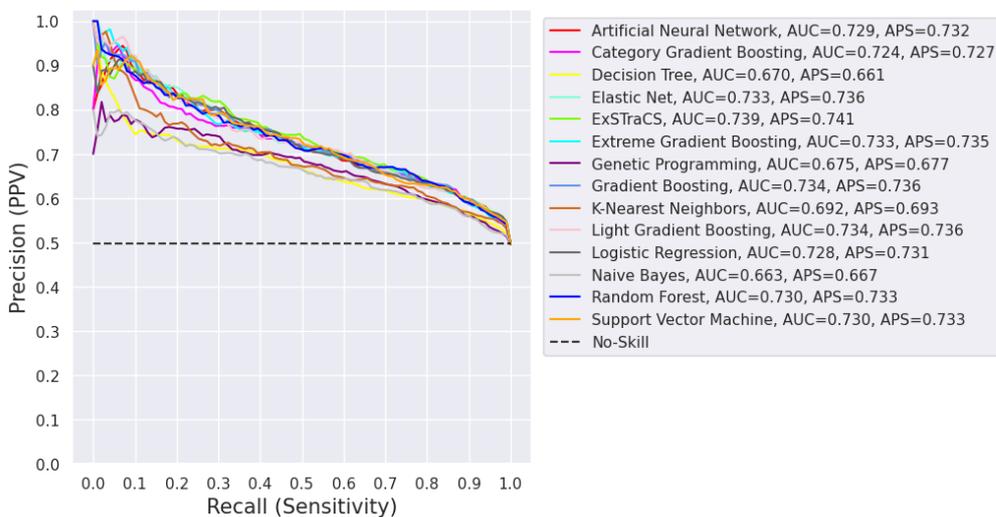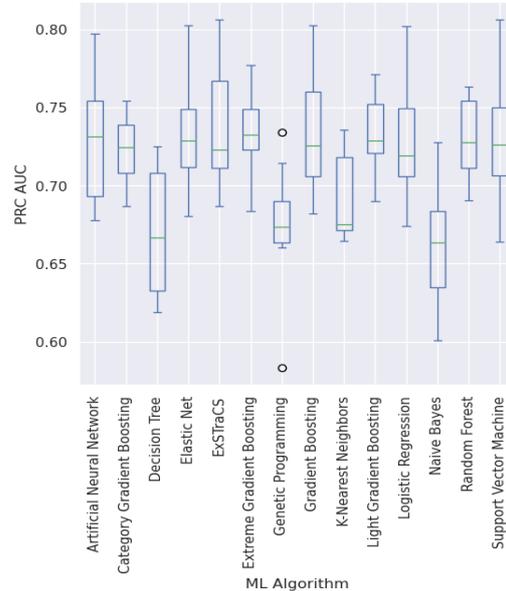

# Dataset and Model Prediction Summary: D10 = J\_GE15\_DEMDXSYMCFIO

## Data Processing/Counts Summary

|           | Instances | Total Features | Categorical Features | Quantitative Features | Missing Values | Missing Percent | Class 0 | Class 1 |
|-----------|-----------|----------------|----------------------|-----------------------|----------------|-----------------|---------|---------|
| Original  | 2178      | 85             | 21                   | 64                    | 6882           | 0.0372          | 1098    | 1080    |
| C1        | 2178      | 85             | 21                   | 64                    | 6882           | 0.0372          | 1098    | 1080    |
| E1        | 2178      | 85             | 21                   | 64                    | 6882           | 0.0372          | 1098    | 1080    |
| C2        | 2178      | 85             | 21                   | 64                    | 6882           | 0.0372          | 1098    | 1080    |
| C3        | 2178      | 85             | 21                   | 64                    | 6882           | 0.0372          | 1098    | 1080    |
| E2        | 2178      | 85             | 21                   | 64                    | 6882           | 0.0372          | 1098    | 1080    |
| C4        | 2178      | 85             | 21                   | 64                    | 6882           | 0.0372          | 1098    | 1080    |
| Processed | 2178      | 85             | 21                   | 64                    | 6882           | 0.0372          | 1098    | 1080    |

## Cleaning (C) and Engineering (E) Elements

- \* C1 - Remove instances with no outcome and features to ignore
- \* E1 - Add missingness features
- \* C2 - Remove features with invariance or high missingness
- \* C3 - Remove instances with high missingness
- \* E2 - Add one-hot-encoding of categorical features
- \* C4 - Remove highly correlated features

## Class Balance (Processed)

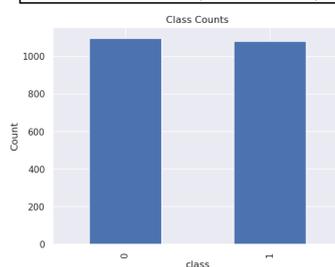

## Feature Correlations (Pearson)

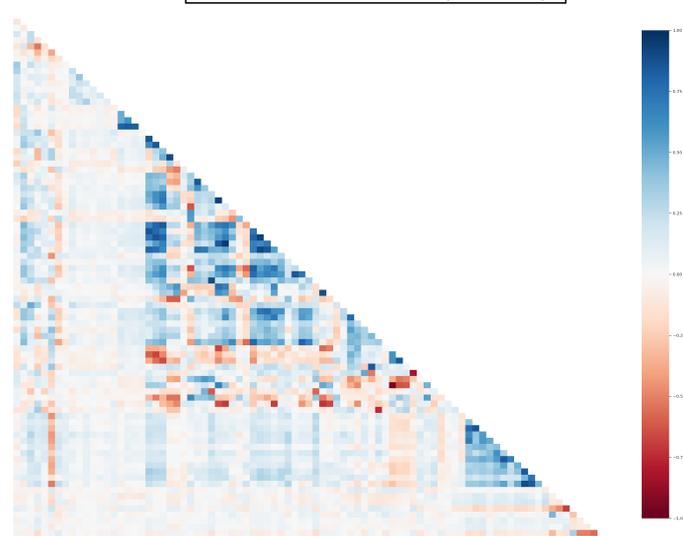

## Top ML Algorithm Results (Averaged Over CV Runs):

|                                                          |
|----------------------------------------------------------|
| Best (ROC_AUC): Random Forest = 0.763                    |
| Best (Balanced Acc.): Category Gradient Boosting = 0.696 |
| Best (F1 Score): Category Gradient Boosting = 0.693      |
| Best (PRC AUC): Random Forest = 0.750                    |
| Best (PRC APS): Random Forest = 0.753                    |

## ROC

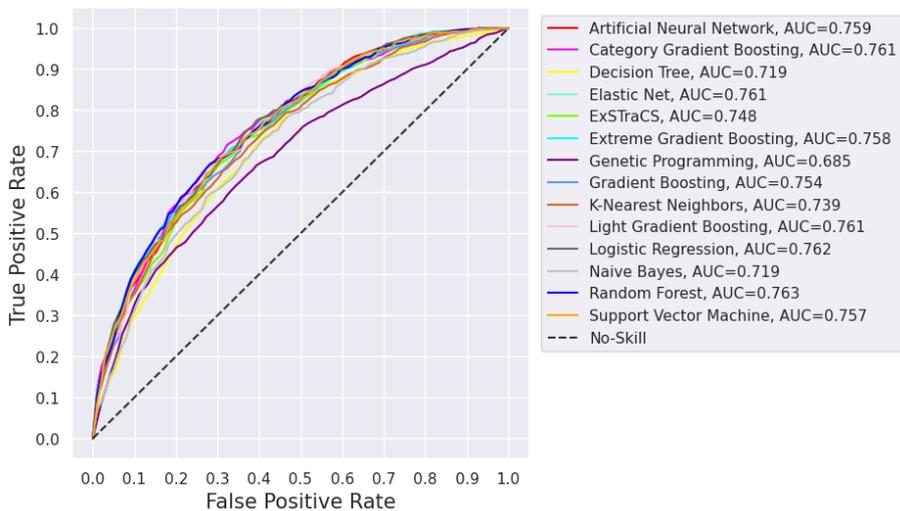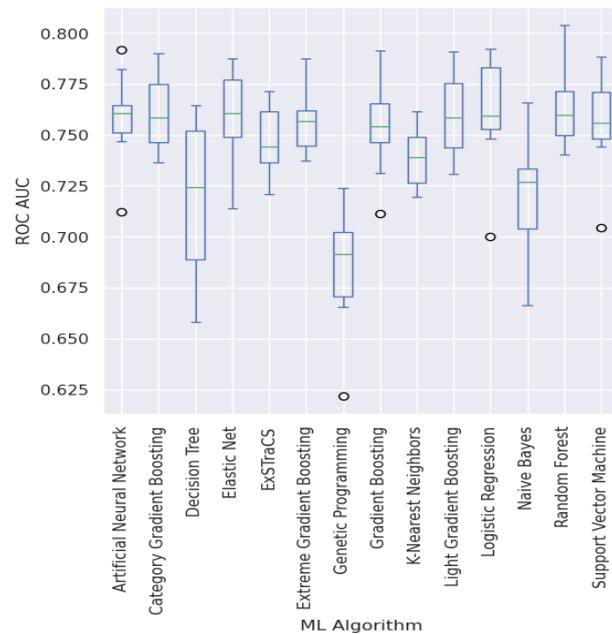

## PRC

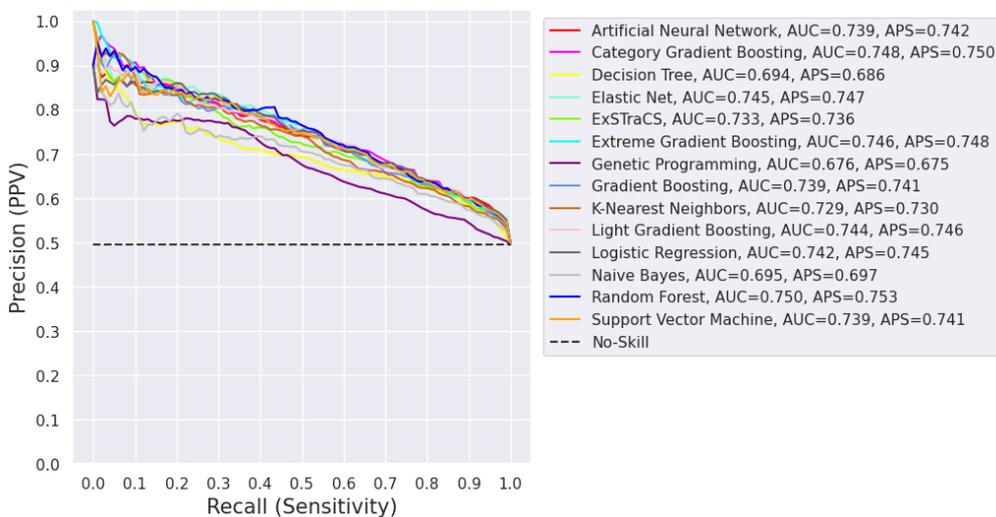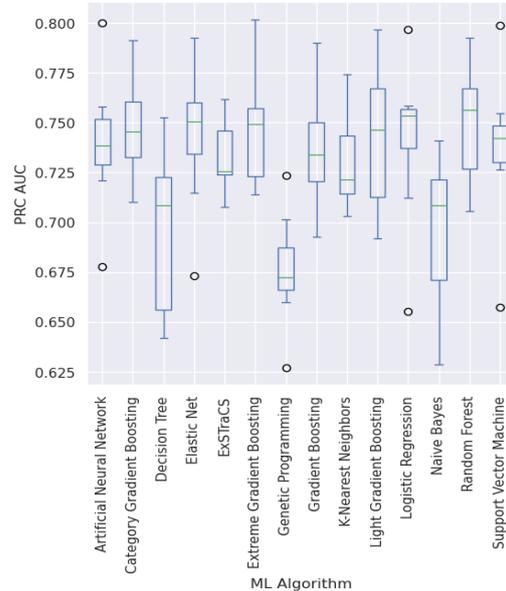

# Dataset and Model Prediction Summary: D11 = K\_GE5\_DEM

## Data Processing/Counts Summary

|           | Instances | Total Features | Categorical Features | Quantitative Features | Missing Values | Missing Percent | Class 0 | Class 1 |
|-----------|-----------|----------------|----------------------|-----------------------|----------------|-----------------|---------|---------|
| Original  | 2179      | 8              | 6                    | 2                     | 25             | 0.0014          | 606     | 1573    |
| C1        | 2179      | 8              | 6                    | 2                     | 25             | 0.0014          | 606     | 1573    |
| E1        | 2179      | 8              | 6                    | 2                     | 25             | 0.0014          | 606     | 1573    |
| C2        | 2179      | 8              | 6                    | 2                     | 25             | 0.0014          | 606     | 1573    |
| C3        | 2174      | 8              | 6                    | 2                     | 0              | 0.0             | 605     | 1569    |
| E2        | 2174      | 8              | 6                    | 2                     | 0              | 0.0             | 605     | 1569    |
| C4        | 2174      | 8              | 6                    | 2                     | 0              | 0.0             | 605     | 1569    |
| Processed | 2174      | 8              | 6                    | 2                     | 0              | 0.0             | 605     | 1569    |

## Cleaning (C) and Engineering (E) Elements

- \* C1 - Remove instances with no outcome and features to ignore
- \* E1 - Add missingness features
- \* C2 - Remove features with invariance or high missingness
- \* C3 - Remove instances with high missingness
- \* E2 - Add one-hot-encoding of categorical features
- \* C4 - Remove highly correlated features

## Class Balance (Processed)

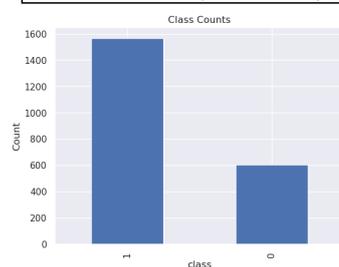

## Feature Correlations (Pearson)

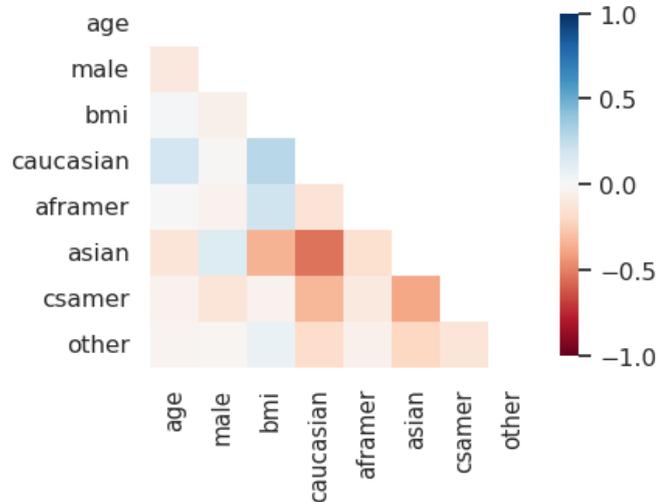

## Top ML Algorithm Results (Averaged Over CV Runs):

|                                                       |
|-------------------------------------------------------|
| Best (ROC_AUC): Artificial Neural Network = 0.763     |
| Best (Balanced Acc.): Light Gradient Boosting = 0.692 |
| Best (F1 Score): Artificial Neural Network = 0.866    |
| Best (PRC AUC): Artificial Neural Network = 0.873     |
| Best (PRC APS): Artificial Neural Network = 0.874     |

## ROC

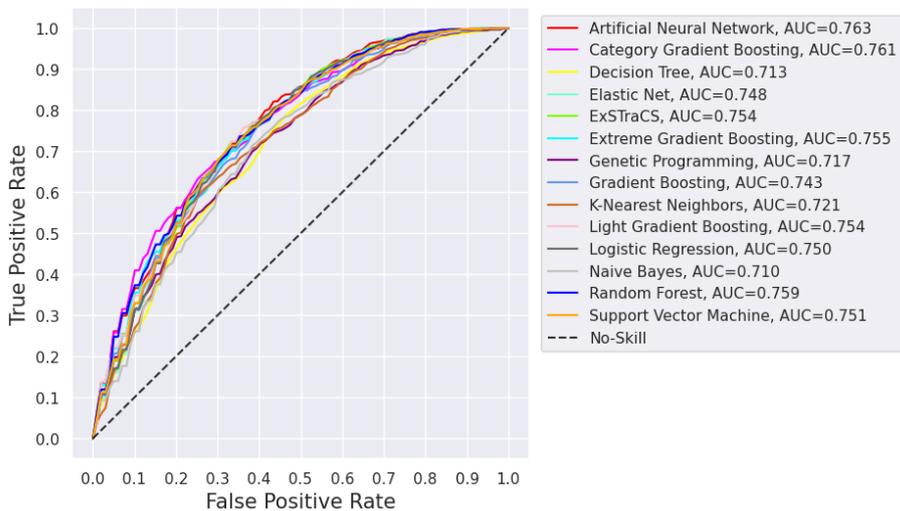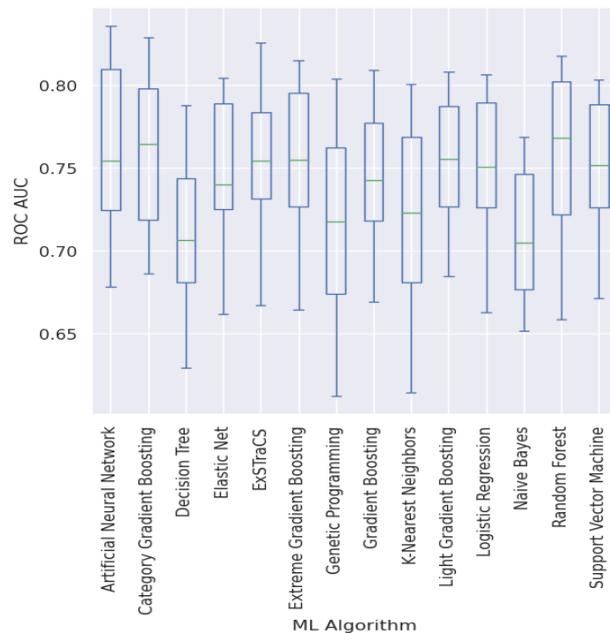

## PRC

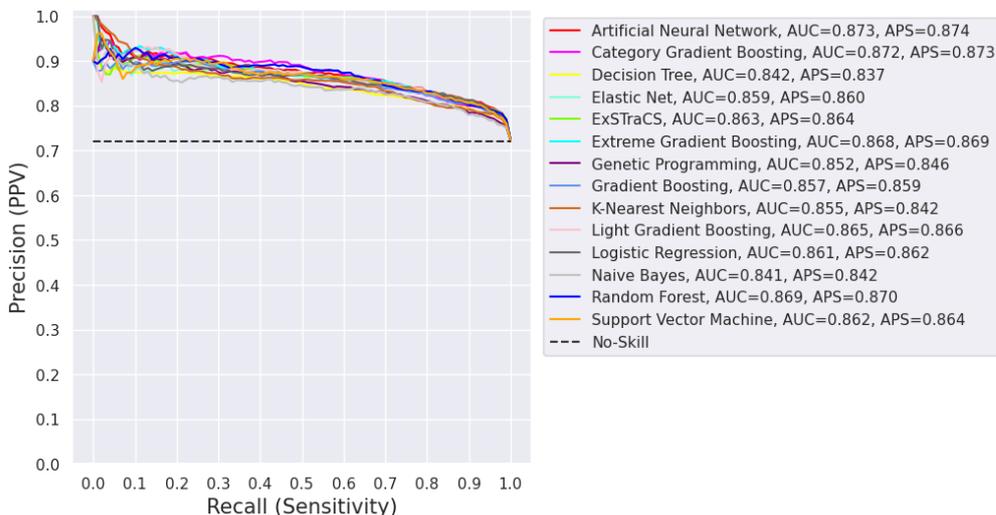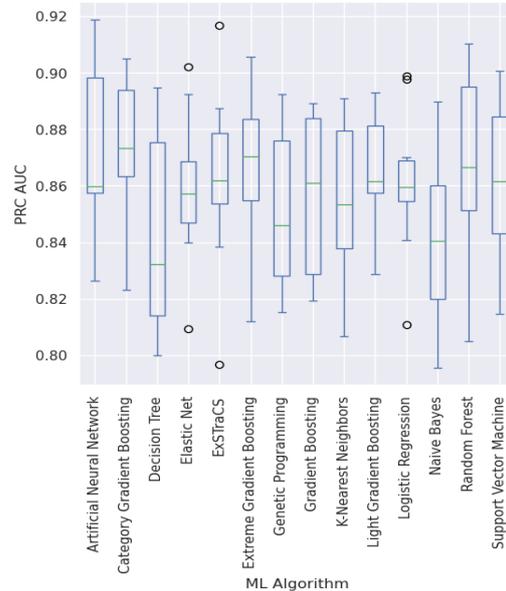

# Dataset and Model Prediction Summary: D12 = L\_GE5\_DX

## Data Processing/Counts Summary

|           | Instances | Total Features | Categorical Features | Quantitative Features | Missing Values | Missing Percent | Class 0 | Class 1 |
|-----------|-----------|----------------|----------------------|-----------------------|----------------|-----------------|---------|---------|
| Original  | 2179      | 7              | 7                    | 0                     | 2866           | 0.1879          | 606     | 1573    |
| C1        | 2179      | 7              | 7                    | 0                     | 2866           | 0.1879          | 606     | 1573    |
| E1        | 2179      | 7              | 7                    | 0                     | 2866           | 0.1879          | 606     | 1573    |
| C2        | 2179      | 7              | 7                    | 0                     | 2866           | 0.1879          | 606     | 1573    |
| C3        | 1798      | 7              | 7                    | 0                     | 233            | 0.0185          | 447     | 1351    |
| E2        | 1798      | 7              | 7                    | 0                     | 233            | 0.0185          | 447     | 1351    |
| C4        | 1798      | 7              | 7                    | 0                     | 233            | 0.0185          | 447     | 1351    |
| Processed | 1798      | 7              | 7                    | 0                     | 233            | 0.0185          | 447     | 1351    |

## Cleaning (C) and Engineering (E) Elements

- \* C1 - Remove instances with no outcome and features to ignore
- \* E1 - Add missingness features
- \* C2 - Remove features with invariance or high missingness
- \* C3 - Remove instances with high missingness
- \* E2 - Add one-hot-encoding of categorical features
- \* C4 - Remove highly correlated features

## Class Balance (Processed)

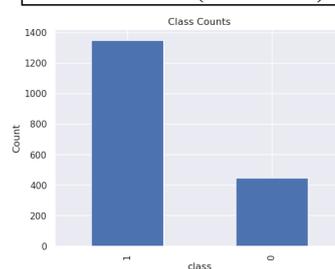

## Feature Correlations (Pearson)

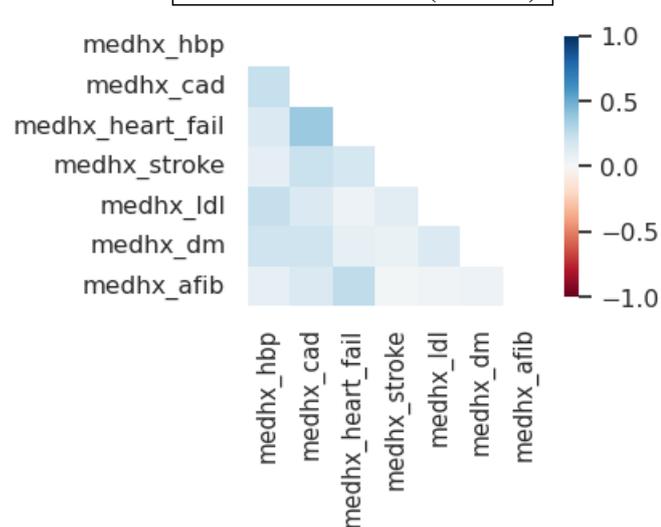

## Top ML Algorithm Results (Averaged Over CV Runs):

|                                                       |
|-------------------------------------------------------|
| Best (ROC_AUC): Elastic Net = 0.591                   |
| Best (Balanced Acc.): Light Gradient Boosting = 0.579 |
| Best (F1 Score): Genetic Programming = 0.858          |
| Best (PRC AUC): Genetic Programming = 0.845           |
| Best (PRC APS): Extreme Gradient Boosting = 0.797     |

## ROC

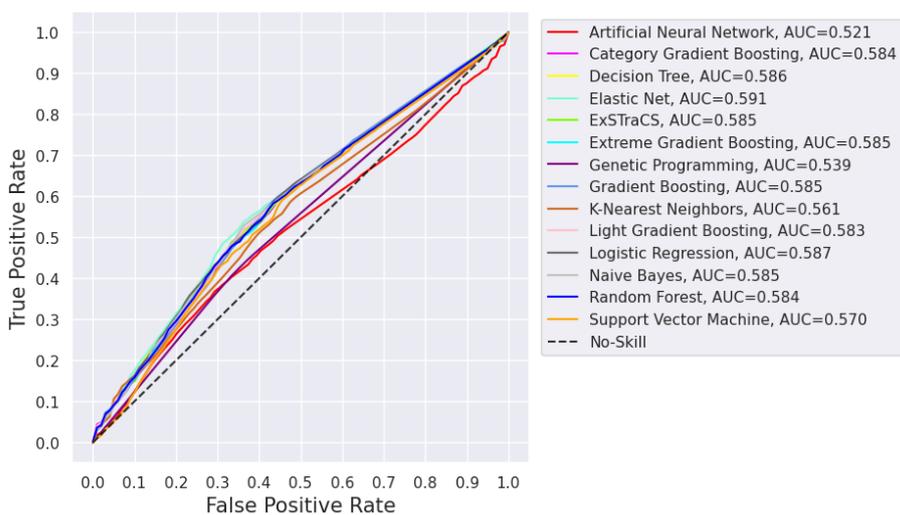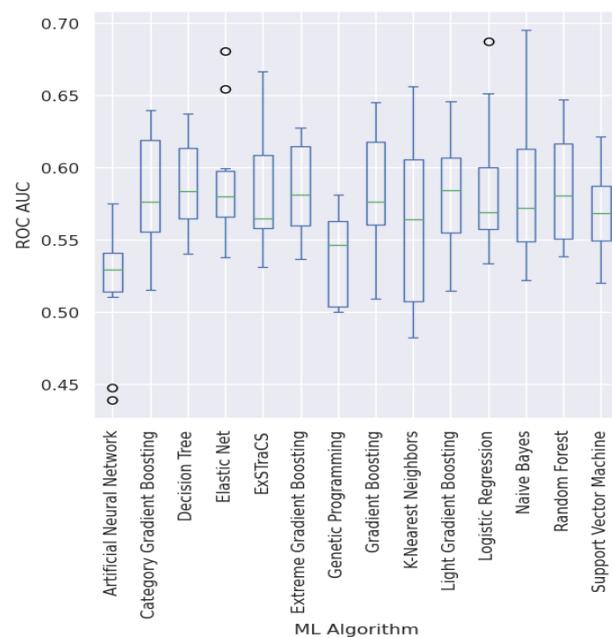

## PRC

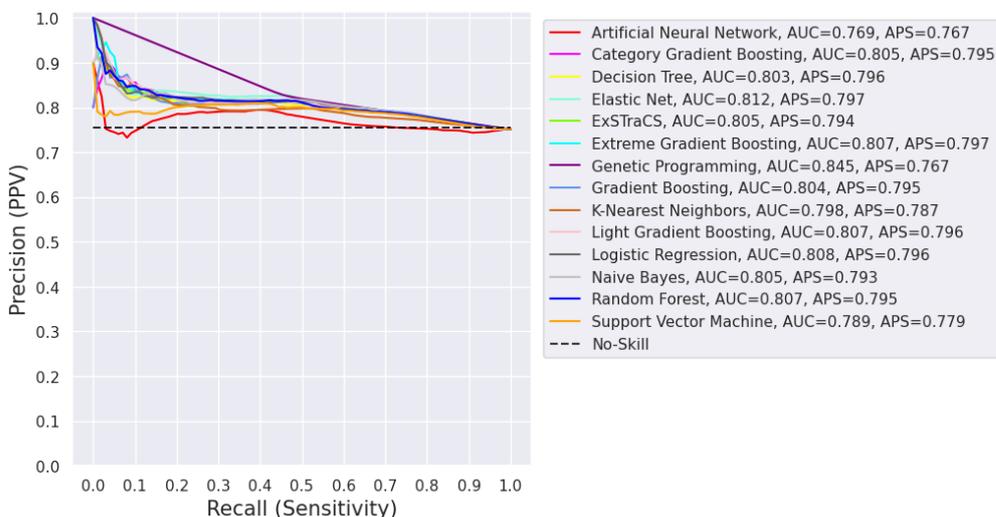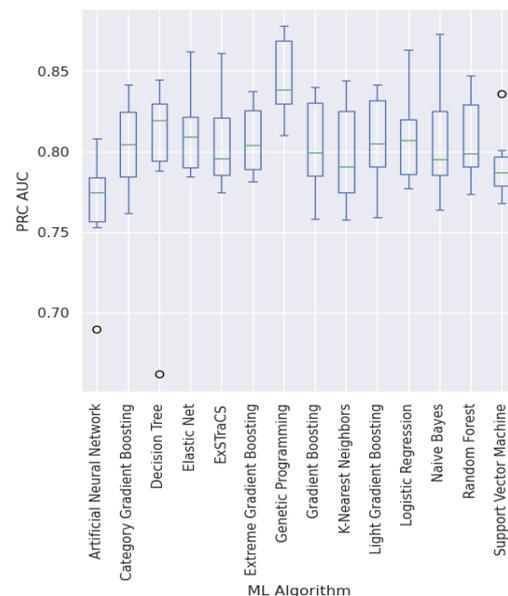

# Dataset and Model Prediction Summary: D13 = M\_GE5\_SYM

## Data Processing/Counts Summary

|           | Instances | Total Features | Categorical Features | Quantitative Features | Missing Values | Missing Percent | Class 0 | Class 1 |
|-----------|-----------|----------------|----------------------|-----------------------|----------------|-----------------|---------|---------|
| Original  | 2179      | 4              | 0                    | 4                     | 1408           | 0.1615          | 606     | 1573    |
| C1        | 2179      | 4              | 0                    | 4                     | 1408           | 0.1615          | 606     | 1573    |
| E1        | 2179      | 4              | 0                    | 4                     | 1408           | 0.1615          | 606     | 1573    |
| C2        | 2179      | 4              | 0                    | 4                     | 1408           | 0.1615          | 606     | 1573    |
| C3        | 1820      | 4              | 0                    | 4                     | 10             | 0.0014          | 449     | 1371    |
| E2        | 1820      | 4              | 0                    | 4                     | 10             | 0.0014          | 449     | 1371    |
| C4        | 1820      | 4              | 0                    | 4                     | 10             | 0.0014          | 449     | 1371    |
| Processed | 1820      | 4              | 0                    | 4                     | 10             | 0.0014          | 449     | 1371    |

## Cleaning (C) and Engineering (E) Elements

- \* C1 - Remove instances with no outcome and features to ignore
- \* E1 - Add missingness features
- \* C2 - Remove features with invariance or high missingness
- \* C3 - Remove instances with high missingness
- \* E2 - Add one-hot-encoding of categorical features
- \* C4 - Remove highly correlated features

## Class Balance (Processed)

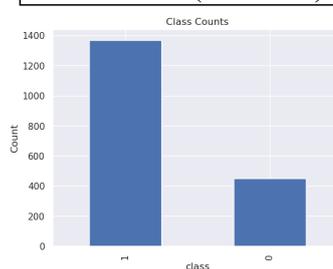

## Feature Correlations (Pearson)

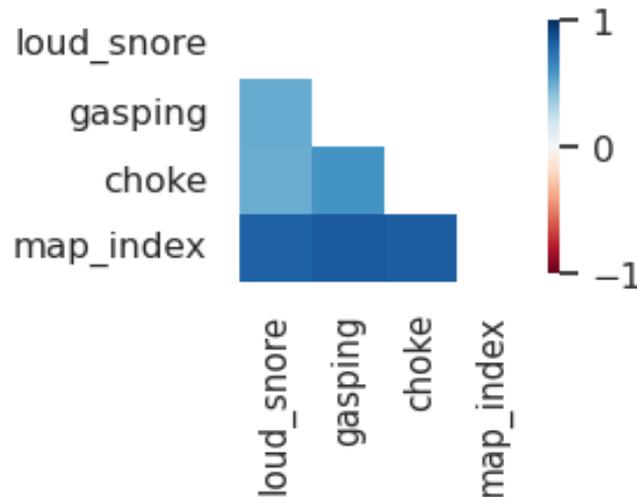

## Top ML Algorithm Results (Averaged Over CV Runs):

|                                                         |
|---------------------------------------------------------|
| Best (ROC_AUC): Elastic Net = 0.667                     |
| Best (Balanced Acc.): Extreme Gradient Boosting = 0.650 |
| Best (F1 Score): Artificial Neural Network = 0.859      |
| Best (PRC AUC): Genetic Programming = 0.867             |
| Best (PRC APS): Elastic Net = 0.850                     |

## ROC

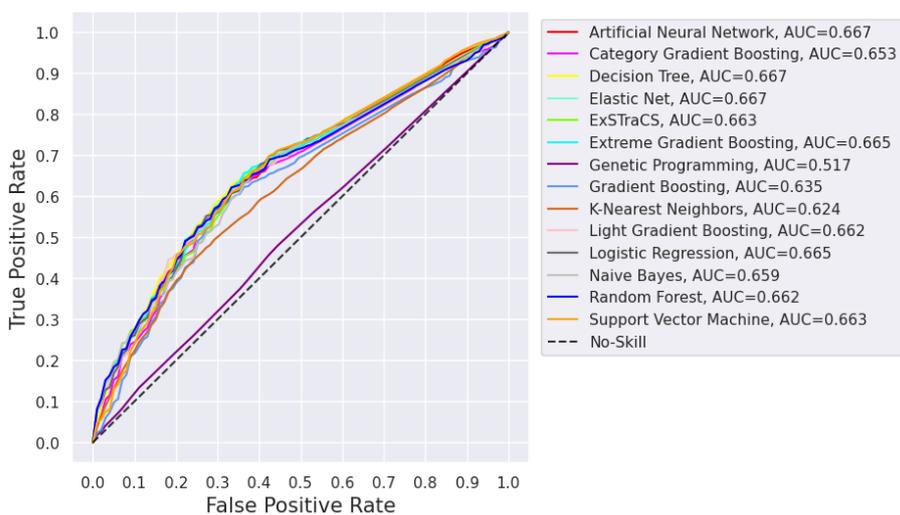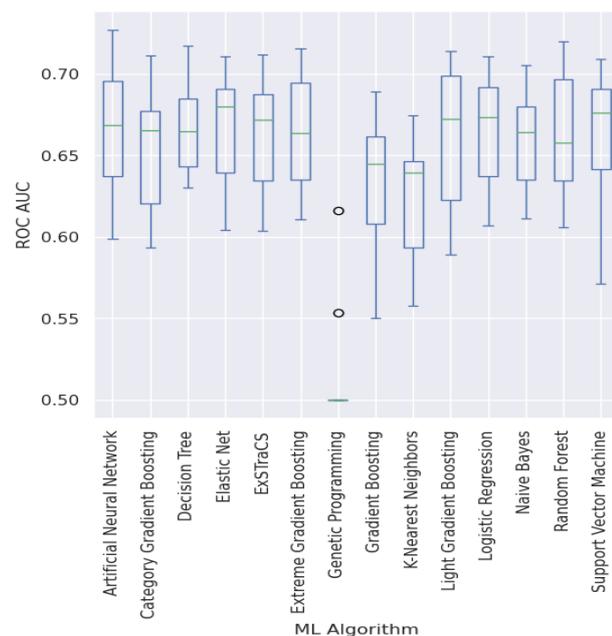

## PRC

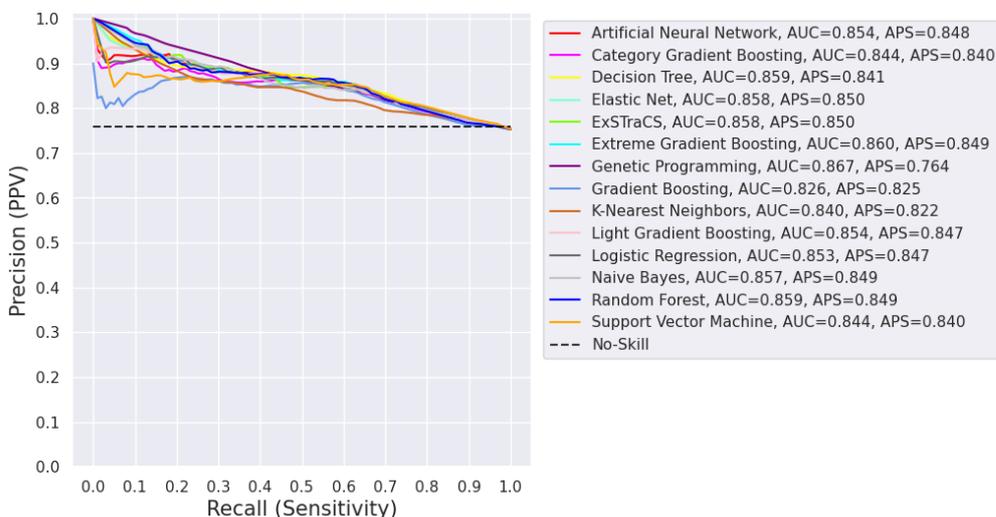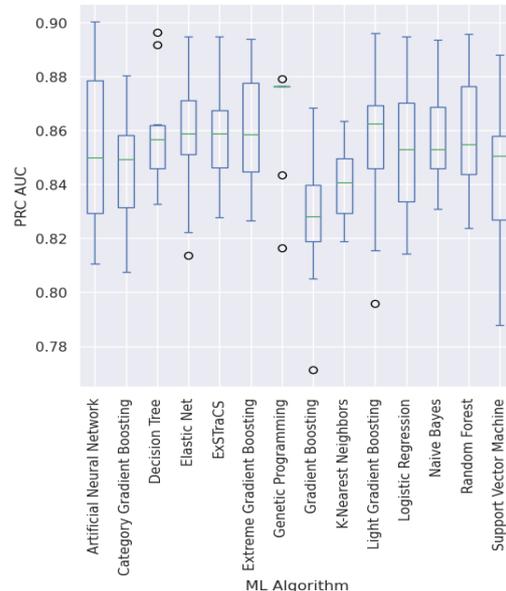

# Dataset and Model Prediction Summary: D14 = N\_GE5\_CF

## Data Processing/Counts Summary

|           | Instances | Total Features | Categorical Features | Quantitative Features | Missing Values | Missing Percent | Class 0 | Class 1 |
|-----------|-----------|----------------|----------------------|-----------------------|----------------|-----------------|---------|---------|
| Original  | 2179      | 46             | 0                    | 46                    | 336            | 0.0034          | 606     | 1573    |
| C1        | 2179      | 46             | 0                    | 46                    | 336            | 0.0034          | 606     | 1573    |
| E1        | 2179      | 46             | 0                    | 46                    | 336            | 0.0034          | 606     | 1573    |
| C2        | 2179      | 46             | 0                    | 46                    | 336            | 0.0034          | 606     | 1573    |
| C3        | 2179      | 46             | 0                    | 46                    | 336            | 0.0034          | 606     | 1573    |
| E2        | 2179      | 46             | 0                    | 46                    | 336            | 0.0034          | 606     | 1573    |
| C4        | 2179      | 46             | 0                    | 46                    | 336            | 0.0034          | 606     | 1573    |
| Processed | 2179      | 46             | 0                    | 46                    | 336            | 0.0034          | 606     | 1573    |

## Cleaning (C) and Engineering (E) Elements

- \* C1 - Remove instances with no outcome and features to ignore
- \* E1 - Add missingness features
- \* C2 - Remove features with invariance or high missingness
- \* C3 - Remove instances with high missingness
- \* E2 - Add one-hot-encoding of categorical features
- \* C4 - Remove highly correlated features

## Class Balance (Processed)

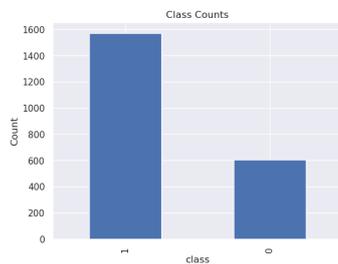

## Feature Correlations (Pearson)

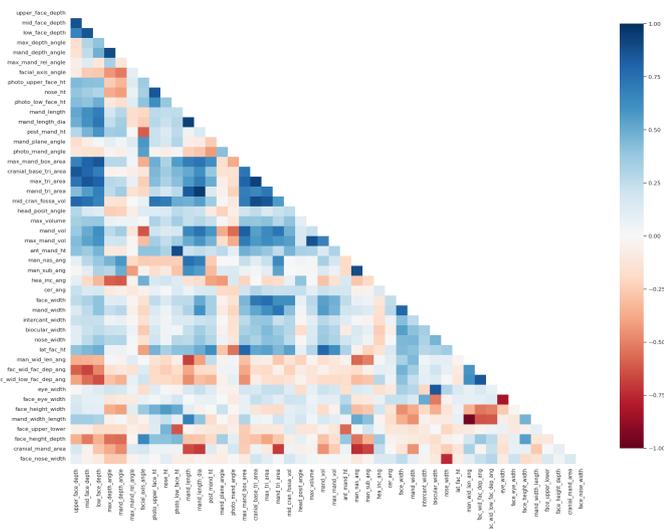

## Top ML Algorithm Results (Averaged Over CV Runs):

|                                                      |
|------------------------------------------------------|
| Best (ROC_AUC): Random Forest = 0.746                |
| Best (Balanced Acc.): Support Vector Machine = 0.684 |
| Best (F1 Score): Category Gradient Boosting = 0.851  |
| Best (PRC AUC): Support Vector Machine = 0.867       |
| Best (PRC APS): Support Vector Machine = 0.868       |

## ROC

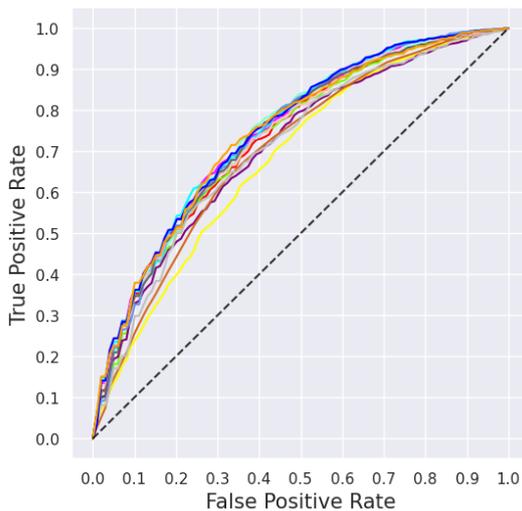

- Artificial Neural Network, AUC=0.731
- Category Gradient Boosting, AUC=0.742
- Decision Tree, AUC=0.679
- Elastic Net, AUC=0.742
- ExStrACS, AUC=0.727
- Extreme Gradient Boosting, AUC=0.745
- Genetic Programming, AUC=0.707
- Gradient Boosting, AUC=0.739
- K-Nearest Neighbors, AUC=0.700
- Light Gradient Boosting, AUC=0.734
- Logistic Regression, AUC=0.737
- Naive Bayes, AUC=0.706
- Random Forest, AUC=0.746
- Support Vector Machine, AUC=0.743
- No-Skill

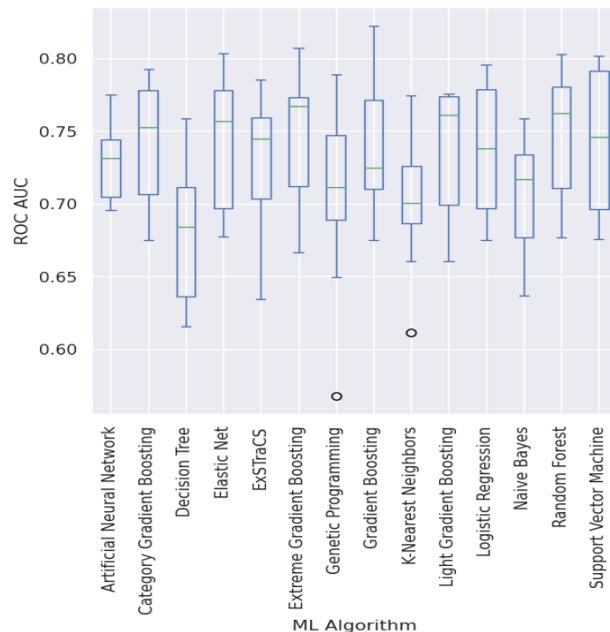

## PRC

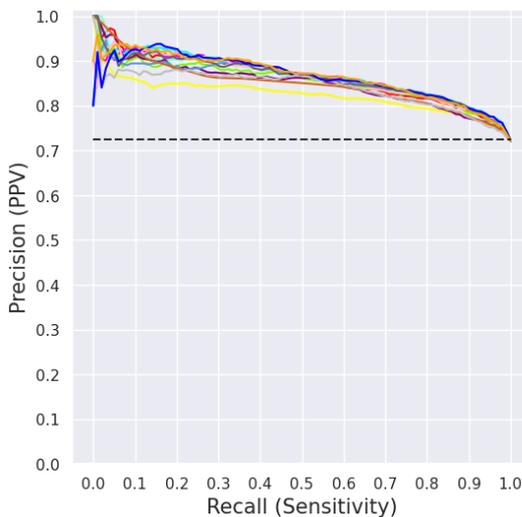

- Artificial Neural Network, AUC=0.863, APS=0.864
- Category Gradient Boosting, AUC=0.864, APS=0.865
- Decision Tree, AUC=0.824, APS=0.824
- Elastic Net, AUC=0.865, APS=0.866
- ExStrACS, AUC=0.855, APS=0.857
- Extreme Gradient Boosting, AUC=0.866, APS=0.867
- Genetic Programming, AUC=0.850, APS=0.850
- Gradient Boosting, AUC=0.857, APS=0.857
- K-Nearest Neighbors, AUC=0.849, APS=0.827
- Light Gradient Boosting, AUC=0.861, APS=0.863
- Logistic Regression, AUC=0.862, APS=0.863
- Naive Bayes, AUC=0.841, APS=0.842
- Random Forest, AUC=0.865, APS=0.867
- Support Vector Machine, AUC=0.867, APS=0.868
- No-Skill

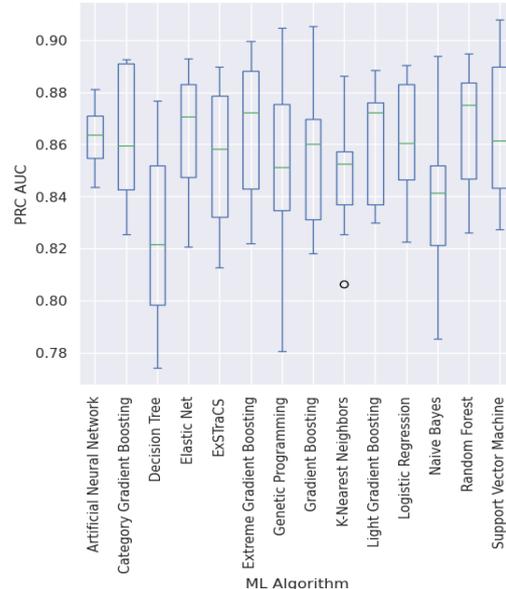

# Dataset and Model Prediction Summary: D15 = O\_GE5\_IO

## Data Processing/Counts Summary

|           | Instances | Total Features | Categorical Features | Quantitative Features | Missing Values | Missing Percent | Class 0 | Class 1 |
|-----------|-----------|----------------|----------------------|-----------------------|----------------|-----------------|---------|---------|
| Original  | 2179      | 20             | 8                    | 12                    | 2170           | 0.0498          | 606     | 1573    |
| C1        | 2179      | 20             | 8                    | 12                    | 2170           | 0.0498          | 606     | 1573    |
| E1        | 2179      | 20             | 8                    | 12                    | 2170           | 0.0498          | 606     | 1573    |
| C2        | 2179      | 20             | 8                    | 12                    | 2170           | 0.0498          | 606     | 1573    |
| C3        | 2137      | 20             | 8                    | 12                    | 1673           | 0.0391          | 603     | 1534    |
| E2        | 2137      | 20             | 8                    | 12                    | 1673           | 0.0391          | 603     | 1534    |
| C4        | 2137      | 20             | 8                    | 12                    | 1673           | 0.0391          | 603     | 1534    |
| Processed | 2137      | 20             | 8                    | 12                    | 1673           | 0.0391          | 603     | 1534    |

### Cleaning (C) and Engineering (E) Elements

- \* C1 - Remove instances with no outcome and features to ignore
- \* E1 - Add missingness features
- \* C2 - Remove features with invariance or high missingness
- \* C3 - Remove instances with high missingness
- \* E2 - Add one-hot-encoding of categorical features
- \* C4 - Remove highly correlated features

### Class Balance (Processed)

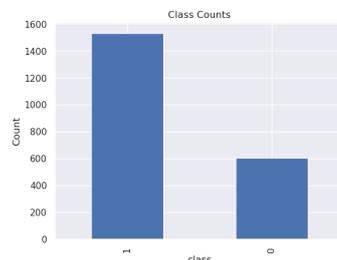

### Feature Correlations (Pearson)

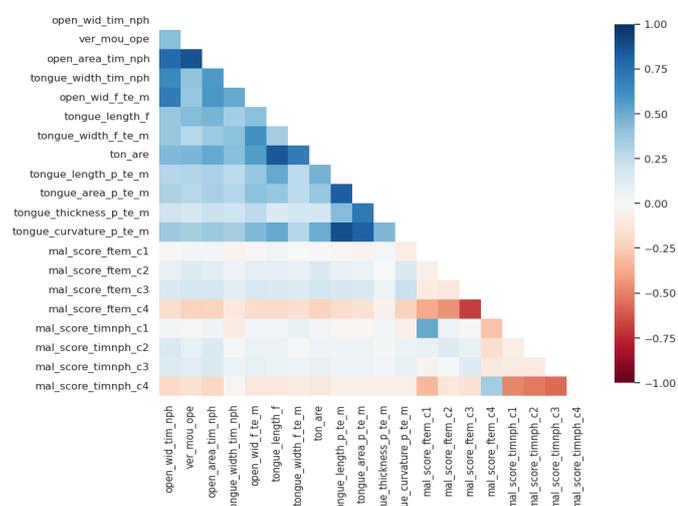

### Top ML Algorithm Results (Averaged Over CV Runs):

|                                                     |
|-----------------------------------------------------|
| Best (ROC_AUC): Elastic Net = 0.650                 |
| Best (Balanced Acc.): Elastic Net = 0.618           |
| Best (F1 Score): Category Gradient Boosting = 0.837 |
| Best (PRC AUC): Genetic Programming = 0.842         |
| Best (PRC APS): Random Forest = 0.818               |

### ROC

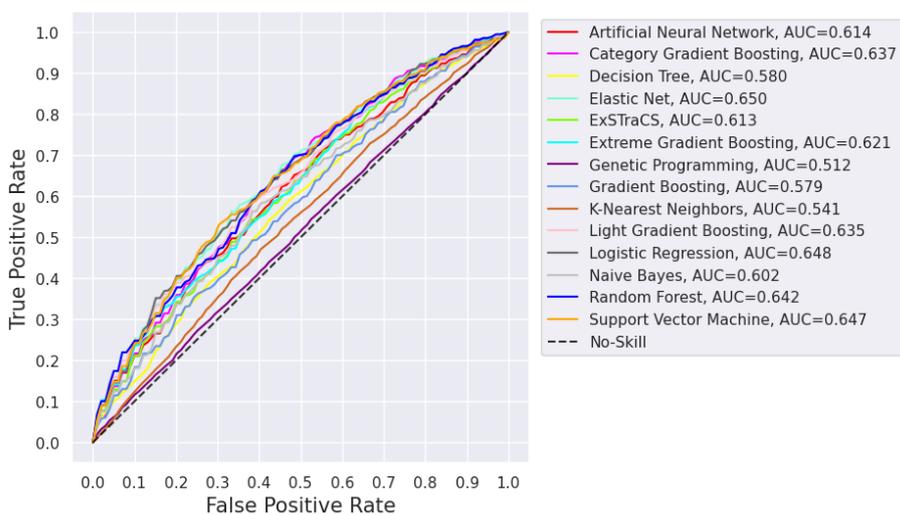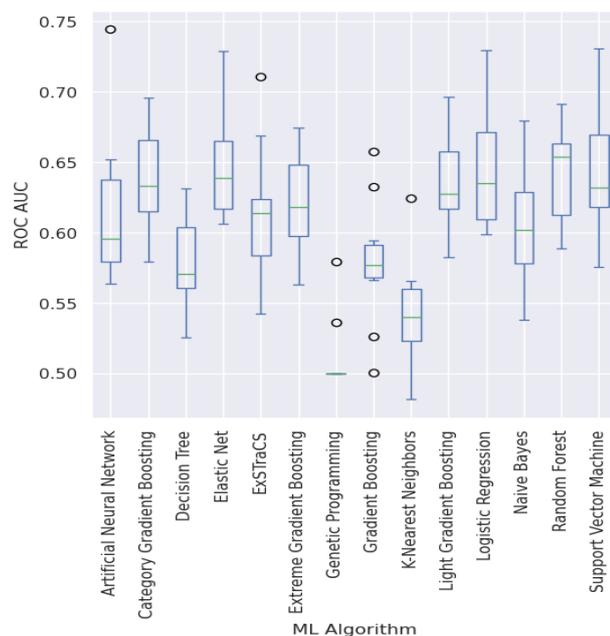

### PRC

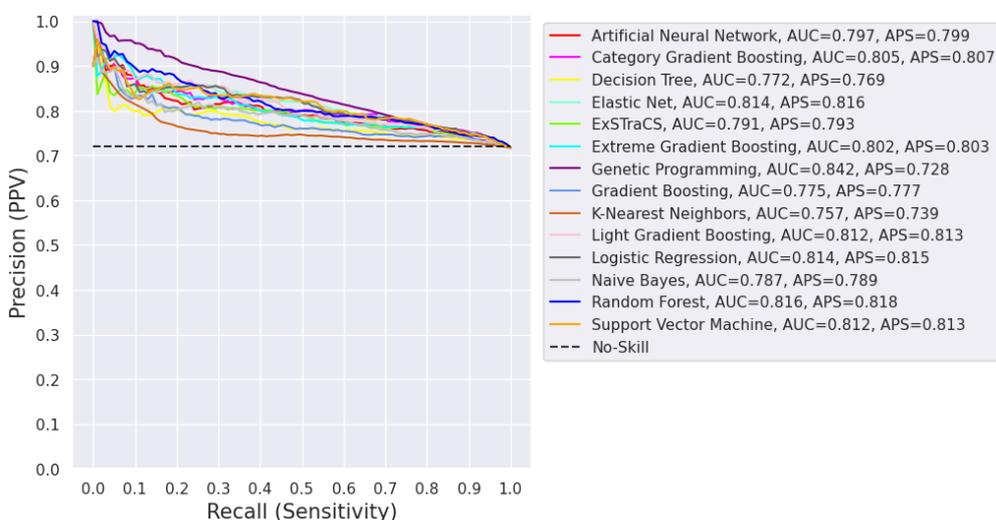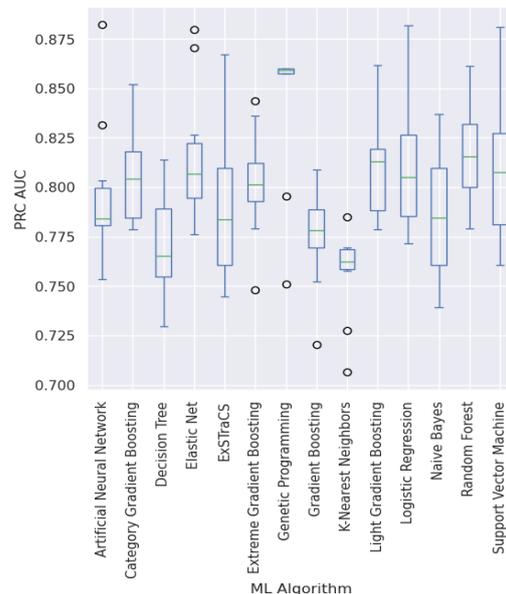

# Dataset and Model Prediction Summary: D16 = P\_GE5\_DEMDX

## Data Processing/Counts Summary

|           | Instances | Total Features | Categorical Features | Quantitative Features | Missing Values | Missing Percent | Class 0 | Class 1 |
|-----------|-----------|----------------|----------------------|-----------------------|----------------|-----------------|---------|---------|
| Original  | 2179      | 15             | 13                   | 2                     | 2891           | 0.0885          | 606     | 1573    |
| C1        | 2179      | 15             | 13                   | 2                     | 2891           | 0.0885          | 606     | 1573    |
| E1        | 2179      | 15             | 13                   | 2                     | 2891           | 0.0885          | 606     | 1573    |
| C2        | 2179      | 15             | 13                   | 2                     | 2891           | 0.0885          | 606     | 1573    |
| C3        | 1812      | 15             | 13                   | 2                     | 302            | 0.0111          | 450     | 1362    |
| E2        | 1812      | 15             | 13                   | 2                     | 302            | 0.0111          | 450     | 1362    |
| C4        | 1812      | 15             | 13                   | 2                     | 302            | 0.0111          | 450     | 1362    |
| Processed | 1812      | 15             | 13                   | 2                     | 302            | 0.0111          | 450     | 1362    |

**Cleaning (C) and Engineering (E) Elements**

- \* C1 - Remove instances with no outcome and features to ignore
- \* E1 - Add missingness features
- \* C2 - Remove features with invariance or high missingness
- \* C3 - Remove instances with high missingness
- \* E2 - Add one-hot-encoding of categorical features
- \* C4 - Remove highly correlated features

## Class Balance (Processed)

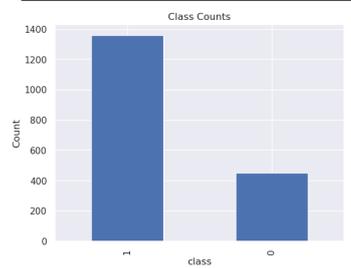

## Feature Correlations (Pearson)

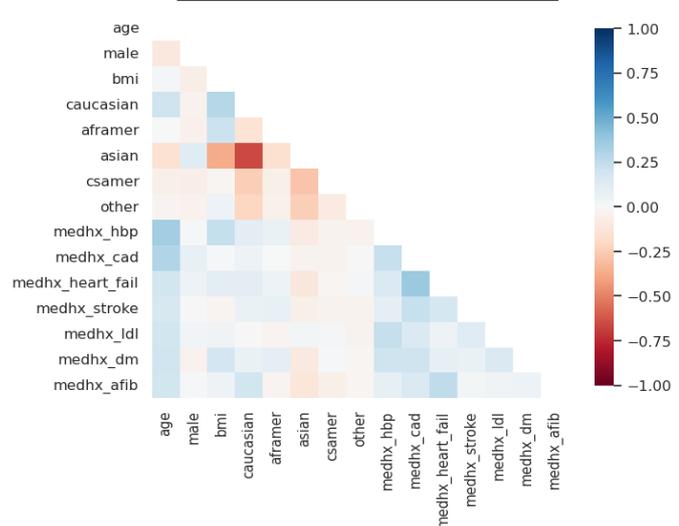

## Top ML Algorithm Results (Averaged Over CV Runs):

|                                                    |
|----------------------------------------------------|
| Best (ROC_AUC): Artificial Neural Network = 0.754  |
| Best (Balanced Acc.): ExSTraCS = 0.687             |
| Best (F1 Score): Artificial Neural Network = 0.872 |
| Best (PRC AUC): Category Gradient Boosting = 0.883 |
| Best (PRC APS): Category Gradient Boosting = 0.884 |

## ROC

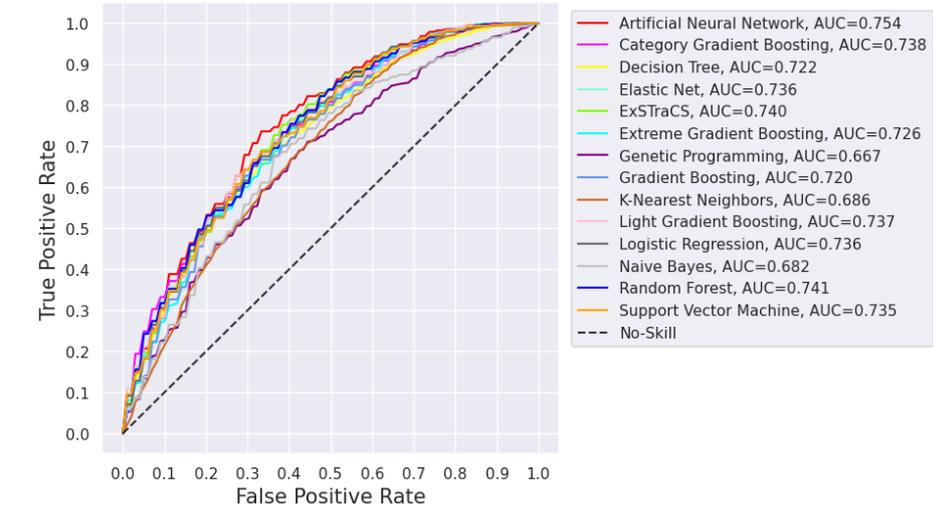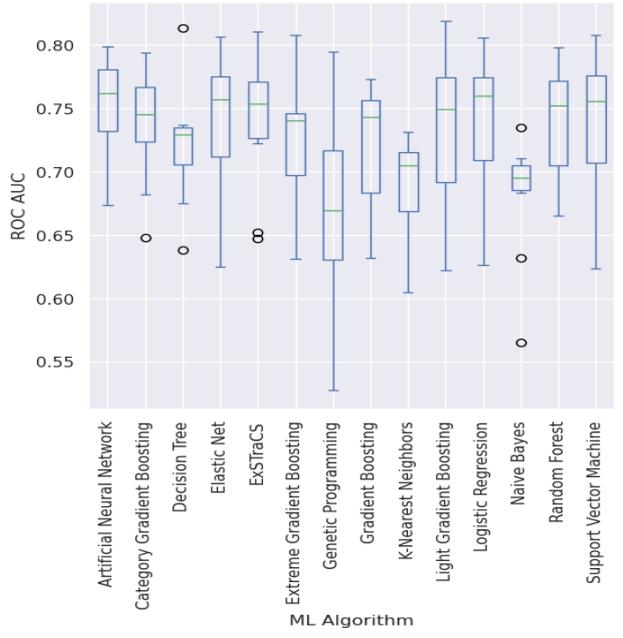

## PRC

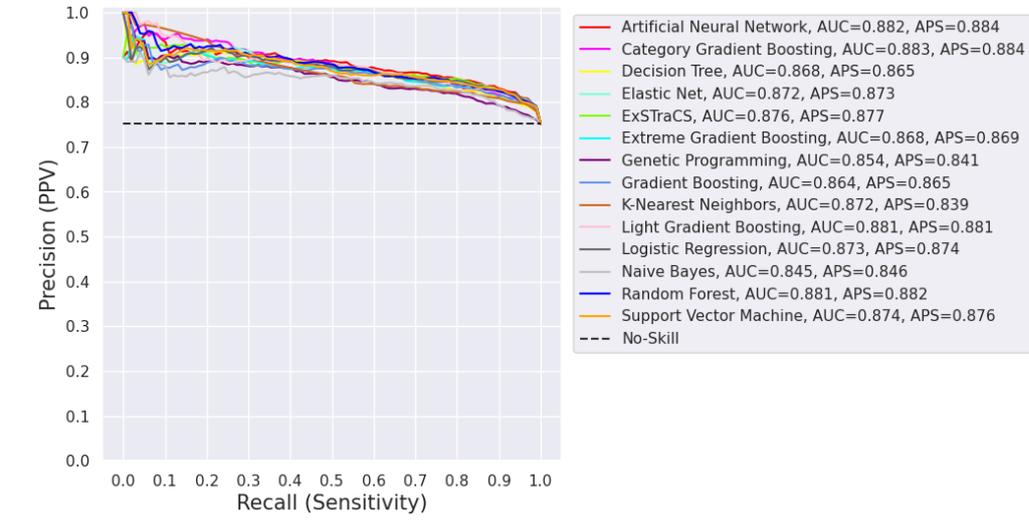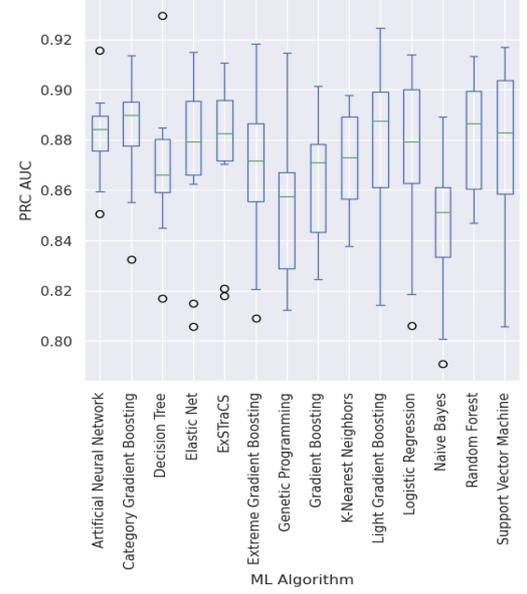

# Dataset and Model Prediction Summary: D17 = Q\_GE5\_DEMDXSYM

## Data Processing/Counts Summary

|           | Instances | Total Features | Categorical Features | Quantitative Features | Missing Values | Missing Percent | Class 0 | Class 1 |
|-----------|-----------|----------------|----------------------|-----------------------|----------------|-----------------|---------|---------|
| Original  | 2179      | 19             | 13                   | 6                     | 4299           | 0.1038          | 606     | 1573    |
| C1        | 2179      | 19             | 13                   | 6                     | 4299           | 0.1038          | 606     | 1573    |
| E1        | 2179      | 19             | 13                   | 6                     | 4299           | 0.1038          | 606     | 1573    |
| C2        | 2179      | 19             | 13                   | 6                     | 4299           | 0.1038          | 606     | 1573    |
| C3        | 1840      | 19             | 13                   | 6                     | 566            | 0.0162          | 457     | 1383    |
| E2        | 1840      | 19             | 13                   | 6                     | 566            | 0.0162          | 457     | 1383    |
| C4        | 1840      | 19             | 13                   | 6                     | 566            | 0.0162          | 457     | 1383    |
| Processed | 1840      | 19             | 13                   | 6                     | 566            | 0.0162          | 457     | 1383    |

## Cleaning (C) and Engineering (E) Elements

- \* C1 - Remove instances with no outcome and features to ignore
- \* E1 - Add missingness features
- \* C2 - Remove features with invariance or high missingness
- \* C3 - Remove instances with high missingness
- \* E2 - Add one-hot-encoding of categorical features
- \* C4 - Remove highly correlated features

## Class Balance (Processed)

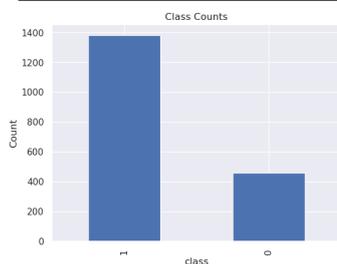

## Feature Correlations (Pearson)

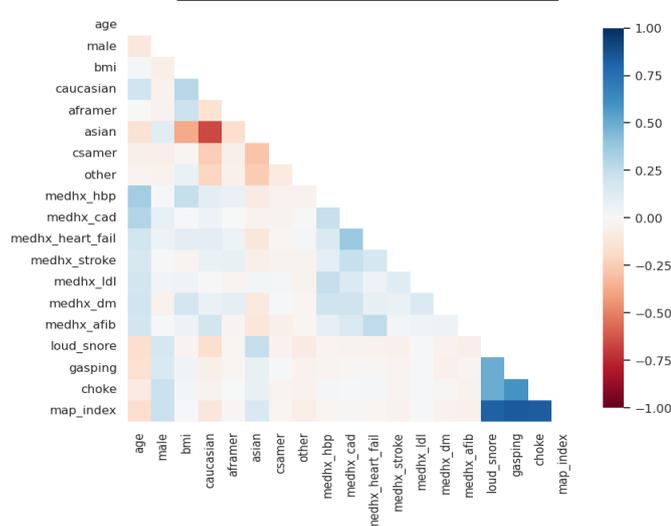

## Top ML Algorithm Results (Averaged Over CV Runs):

|                                                      |
|------------------------------------------------------|
| Best (ROC_AUC): Logistic Regression = 0.769          |
| Best (Balanced Acc.): Support Vector Machine = 0.702 |
| Best (F1 Score): Artificial Neural Network = 0.874   |
| Best (PRC AUC): Logistic Regression = 0.897          |
| Best (PRC APS): Logistic Regression = 0.898          |

## ROC

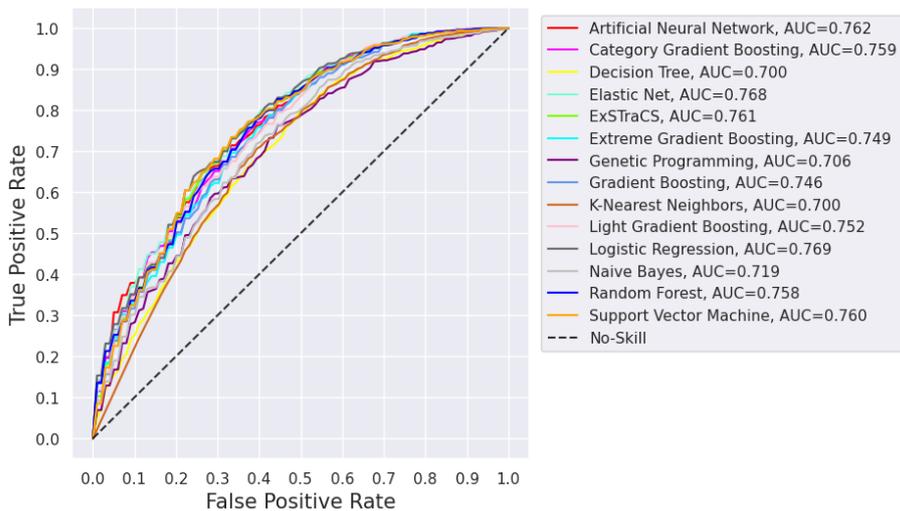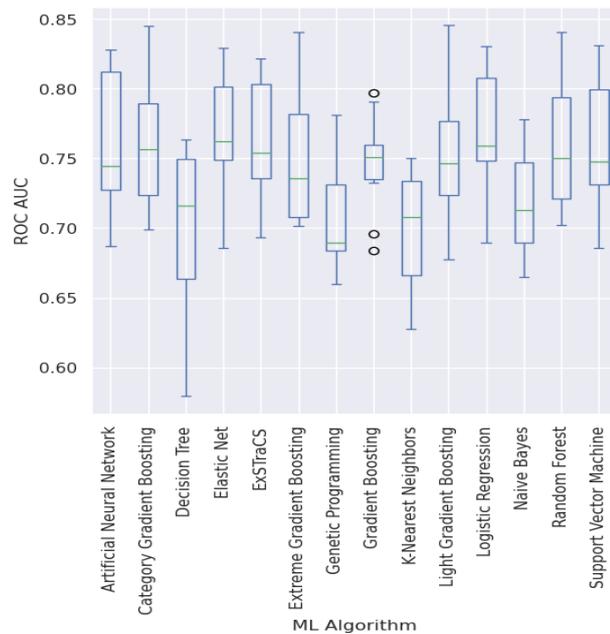

## PRC

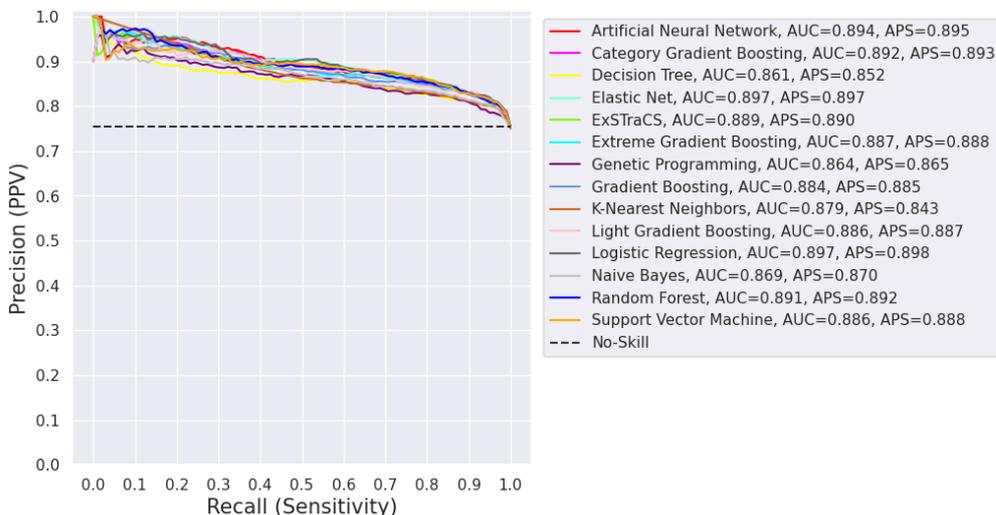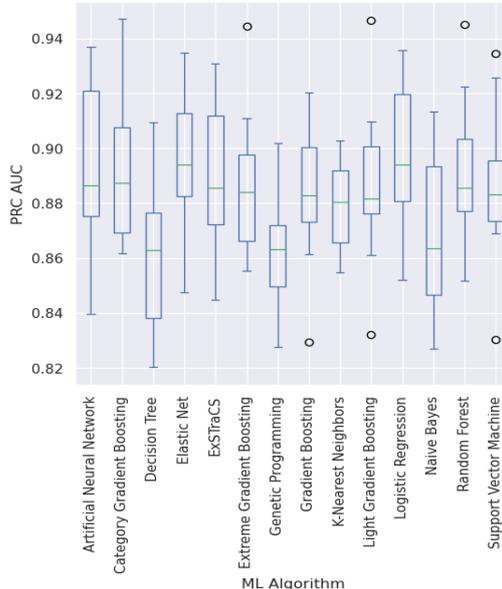

# Dataset and Model Prediction Summary: D18 = R\_GE5\_DEMDXSYMCF

## Data Processing/Counts Summary

|           | Instances | Total Features | Categorical Features | Quantitative Features | Missing Values | Missing Percent | Class 0 | Class 1 |
|-----------|-----------|----------------|----------------------|-----------------------|----------------|-----------------|---------|---------|
| Original  | 2179      | 65             | 13                   | 52                    | 4635           | 0.0327          | 606     | 1573    |
| C1        | 2179      | 65             | 13                   | 52                    | 4635           | 0.0327          | 606     | 1573    |
| E1        | 2179      | 65             | 13                   | 52                    | 4635           | 0.0327          | 606     | 1573    |
| C2        | 2179      | 65             | 13                   | 52                    | 4635           | 0.0327          | 606     | 1573    |
| C3        | 2179      | 65             | 13                   | 52                    | 4635           | 0.0327          | 606     | 1573    |
| E2        | 2179      | 65             | 13                   | 52                    | 4635           | 0.0327          | 606     | 1573    |
| C4        | 2179      | 65             | 13                   | 52                    | 4635           | 0.0327          | 606     | 1573    |
| Processed | 2179      | 65             | 13                   | 52                    | 4635           | 0.0327          | 606     | 1573    |

## Cleaning (C) and Engineering (E) Elements

- \* C1 - Remove instances with no outcome and features to ignore
- \* E1 - Add missingness features
- \* C2 - Remove features with invariance or high missingness
- \* C3 - Remove instances with high missingness
- \* E2 - Add one-hot-encoding of categorical features
- \* C4 - Remove highly correlated features

## Class Balance (Processed)

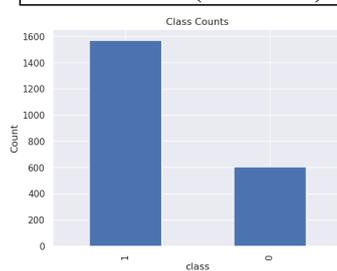

## Feature Correlations (Pearson)

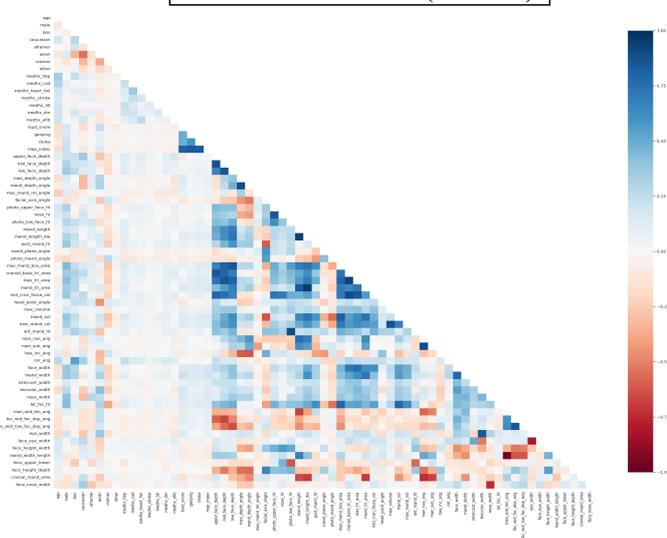

## Top ML Algorithm Results (Averaged Over CV Runs):

Best (ROC\_AUC): Extreme Gradient Boosting = 0.793

Best (Balanced Acc.): ExSTraCS = 0.719

Best (F1 Score): Category Gradient Boosting = 0.867

Best (PRC AUC): Extreme Gradient Boosting = 0.895

Best (PRC APS): Extreme Gradient Boosting = 0.895

## ROC

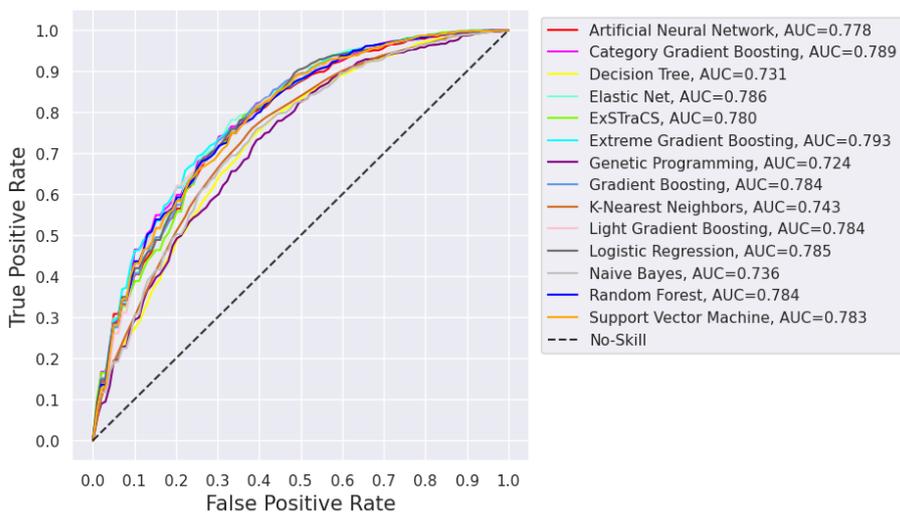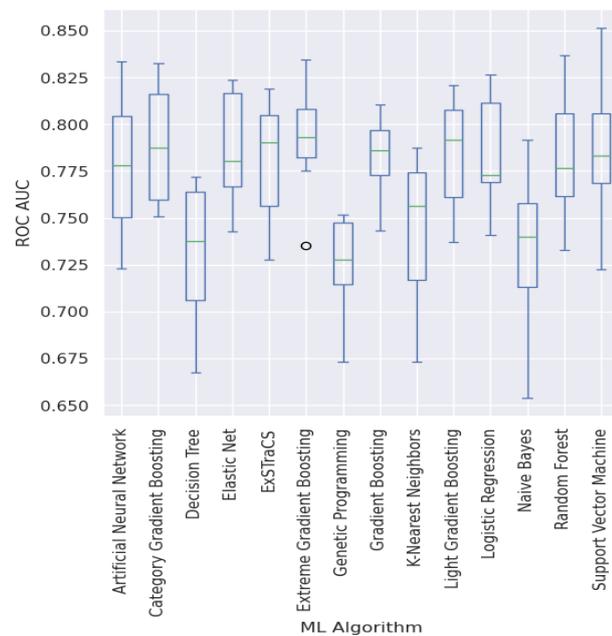

## PRC

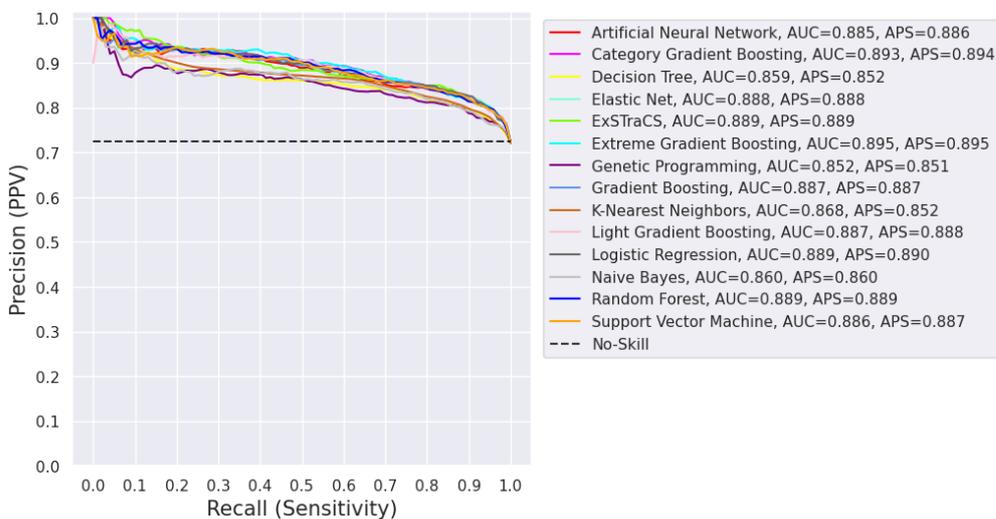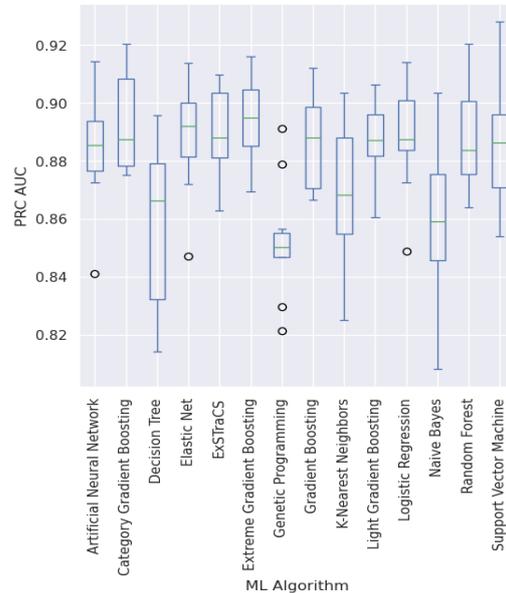

# Dataset and Model Prediction Summary: D19 = S\_GE5\_DEMDXSYMIO

## Data Processing/Counts Summary

|           | Instances | Total Features | Categorical Features | Quantitative Features | Missing Values | Missing Percent | Class 0 | Class 1 |
|-----------|-----------|----------------|----------------------|-----------------------|----------------|-----------------|---------|---------|
| Original  | 2179      | 39             | 21                   | 18                    | 6469           | 0.0761          | 606     | 1573    |
| C1        | 2179      | 39             | 21                   | 18                    | 6469           | 0.0761          | 606     | 1573    |
| E1        | 2179      | 39             | 21                   | 18                    | 6469           | 0.0761          | 606     | 1573    |
| C2        | 2179      | 39             | 21                   | 18                    | 6469           | 0.0761          | 606     | 1573    |
| C3        | 2168      | 39             | 21                   | 18                    | 6244           | 0.0738          | 600     | 1568    |
| E2        | 2168      | 39             | 21                   | 18                    | 6244           | 0.0738          | 600     | 1568    |
| C4        | 2168      | 39             | 21                   | 18                    | 6244           | 0.0738          | 600     | 1568    |
| Processed | 2168      | 39             | 21                   | 18                    | 6244           | 0.0738          | 600     | 1568    |

## Cleaning (C) and Engineering (E) Elements

- \* C1 - Remove instances with no outcome and features to ignore
- \* E1 - Add missingness features
- \* C2 - Remove features with invariance or high missingness
- \* C3 - Remove instances with high missingness
- \* E2 - Add one-hot-encoding of categorical features
- \* C4 - Remove highly correlated features

## Class Balance (Processed)

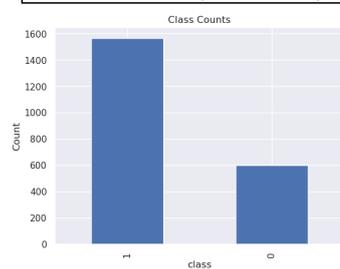

## Feature Correlations (Pearson)

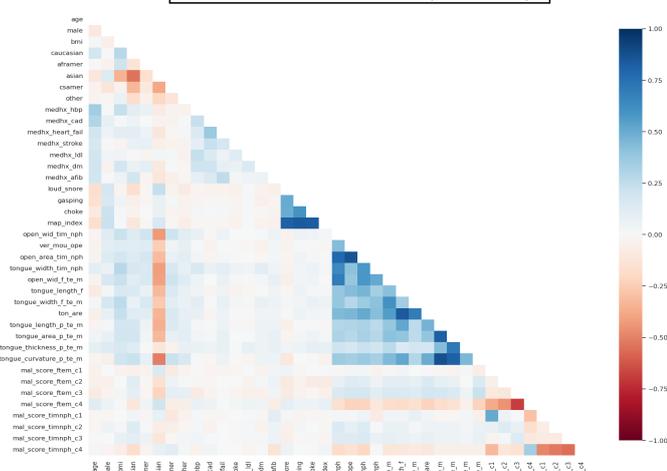

## Top ML Algorithm Results (Averaged Over CV Runs):

- Best (ROC\_AUC): Category Gradient Boosting = 0.774
- Best (Balanced Acc.): ExSTraCS = 0.705
- Best (F1 Score): Category Gradient Boosting = 0.863
- Best (PRC AUC): Logistic Regression = 0.885
- Best (PRC APS): Logistic Regression = 0.886

## ROC

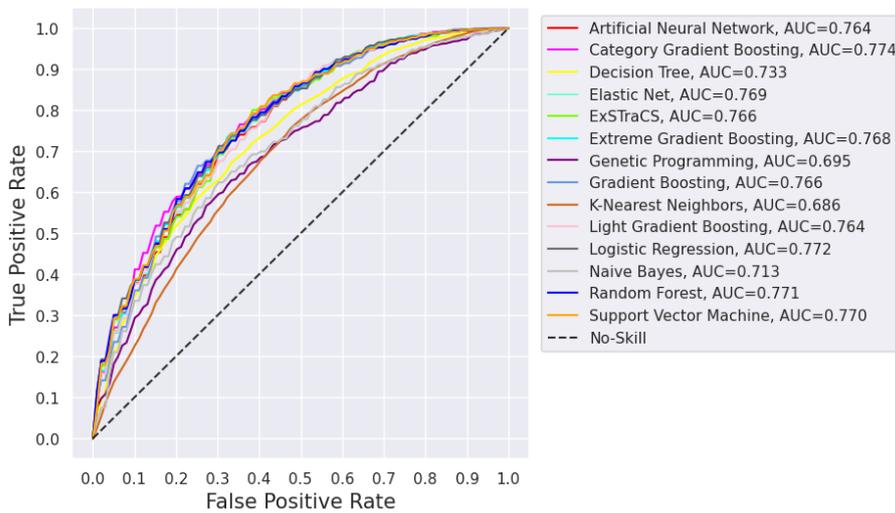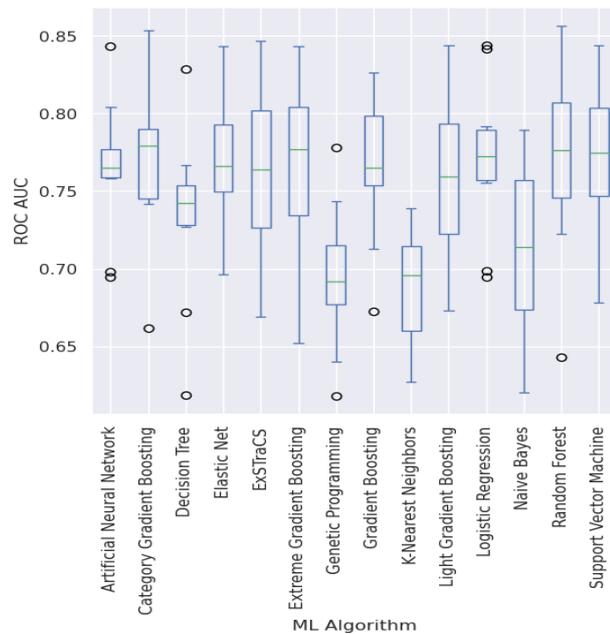

## PRC

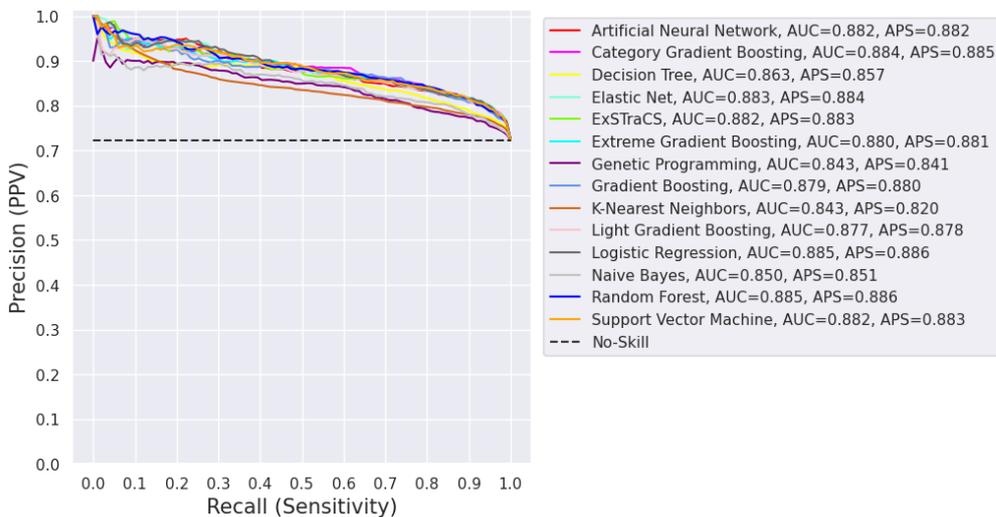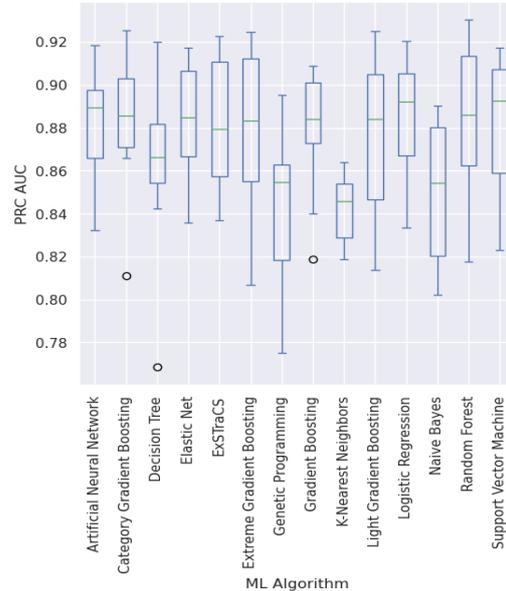

# Dataset and Model Prediction Summary: D20 = T\_GE5\_DEMDXSYMCFIO

## Data Processing/Counts Summary

|           | Instances | Total Features | Categorical Features | Quantitative Features | Missing Values | Missing Percent | Class 0 | Class 1 |
|-----------|-----------|----------------|----------------------|-----------------------|----------------|-----------------|---------|---------|
| Original  | 2179      | 85             | 21                   | 64                    | 6805           | 0.0367          | 606     | 1573    |
| C1        | 2179      | 85             | 21                   | 64                    | 6805           | 0.0367          | 606     | 1573    |
| E1        | 2179      | 85             | 21                   | 64                    | 6805           | 0.0367          | 606     | 1573    |
| C2        | 2179      | 85             | 21                   | 64                    | 6805           | 0.0367          | 606     | 1573    |
| C3        | 2179      | 85             | 21                   | 64                    | 6805           | 0.0367          | 606     | 1573    |
| E2        | 2179      | 85             | 21                   | 64                    | 6805           | 0.0367          | 606     | 1573    |
| C4        | 2179      | 85             | 21                   | 64                    | 6805           | 0.0367          | 606     | 1573    |
| Processed | 2179      | 85             | 21                   | 64                    | 6805           | 0.0367          | 606     | 1573    |

## Cleaning (C) and Engineering (E) Elements

- \* C1 - Remove instances with no outcome and features to ignore
- \* E1 - Add missingness features
- \* C2 - Remove features with invariance or high missingness
- \* C3 - Remove instances with high missingness
- \* E2 - Add one-hot-encoding of categorical features
- \* C4 - Remove highly correlated features

## Class Balance (Processed)

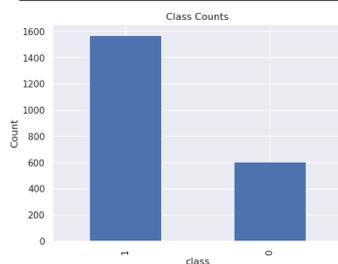

## Feature Correlations (Pearson)

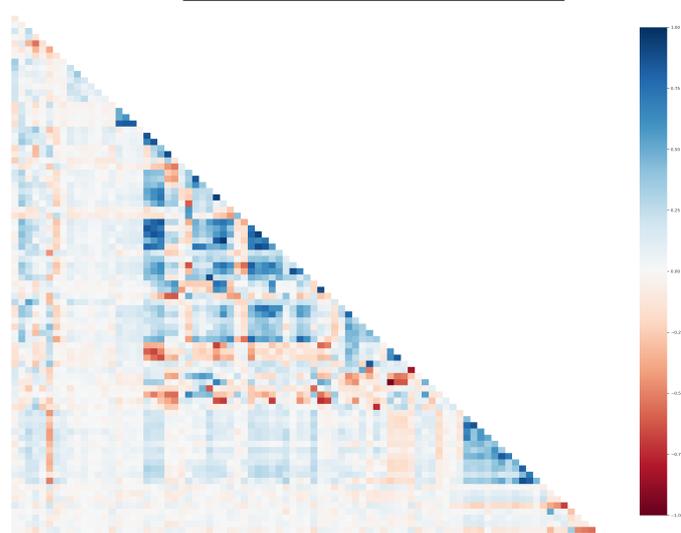

## Top ML Algorithm Results (Averaged Over CV Runs):

|                                                     |
|-----------------------------------------------------|
| Best (ROC_AUC): Extreme Gradient Boosting = 0.790   |
| Best (Balanced Acc.): ExSTraCS = 0.716              |
| Best (F1 Score): Category Gradient Boosting = 0.869 |
| Best (PRC AUC): Extreme Gradient Boosting = 0.895   |
| Best (PRC APS): Extreme Gradient Boosting = 0.896   |

## ROC

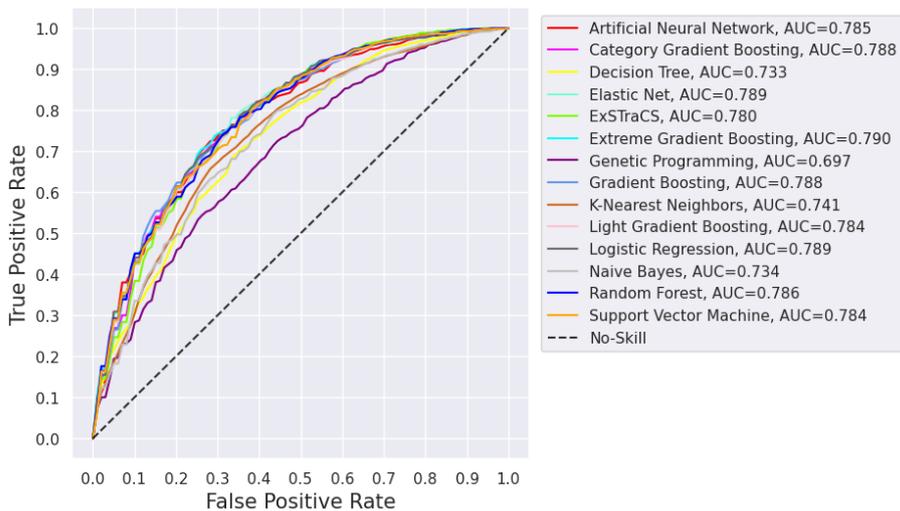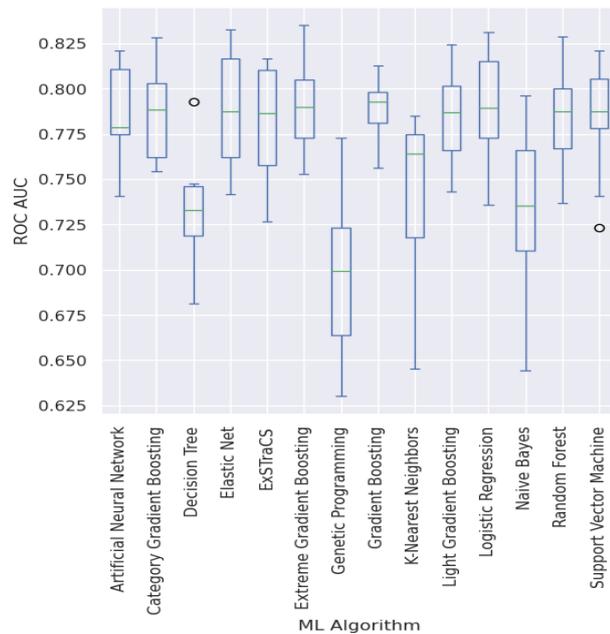

## PRC

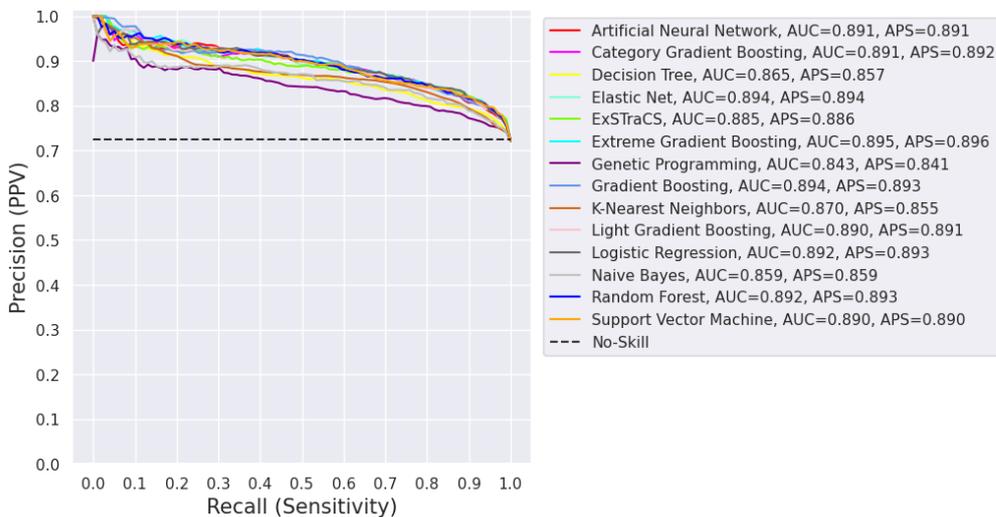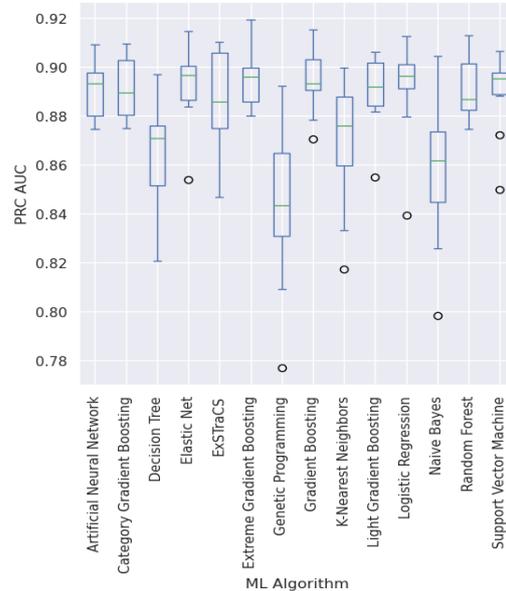

# Average Model Prediction Statistics (Rounded to 3 Decimal Points): Page 1

## D1 = A\_GE15\_DEM

| ML Algorithm               | Balanced Accuracy | Accuracy | F1 Score | Sensitivity (Recall) | Specificity | Precision (PPV) | TP   | TN   | FP   | FN   | NPV   | LR+   | LR-   | ROC AUC | PRC AUC | PRC APS |
|----------------------------|-------------------|----------|----------|----------------------|-------------|-----------------|------|------|------|------|-------|-------|-------|---------|---------|---------|
| Artificial Neural Network  | 0.659             | 0.659    | 0.661    | 0.672                | 0.645       | 0.651           | 72.4 | 70.8 | 38.9 | 35.3 | 0.668 | 1.913 | 0.508 | 0.726   | 0.707   | 0.71    |
| Category Gradient Boosting | 0.67              | 0.67     | 0.669    | 0.676                | 0.664       | 0.664           | 72.8 | 72.8 | 36.9 | 34.9 | 0.678 | 2.024 | 0.486 | 0.736   | 0.725   | 0.727   |
| Decision Tree              | 0.653             | 0.652    | 0.655    | 0.671                | 0.635       | 0.644           | 72.2 | 69.6 | 40.1 | 35.5 | 0.665 | 1.855 | 0.517 | 0.707   | 0.679   | 0.68    |
| Elastic Net                | 0.664             | 0.663    | 0.672    | 0.696                | 0.631       | 0.649           | 75.0 | 69.2 | 40.5 | 32.7 | 0.68  | 1.901 | 0.483 | 0.725   | 0.692   | 0.695   |
| ExSTraCS                   | 0.663             | 0.663    | 0.681    | 0.727                | 0.6         | 0.642           | 78.3 | 65.8 | 43.9 | 29.4 | 0.692 | 1.848 | 0.457 | 0.732   | 0.715   | 0.718   |
| Extreme Gradient Boosting  | 0.662             | 0.661    | 0.667    | 0.685                | 0.638       | 0.652           | 73.8 | 70.0 | 39.7 | 33.9 | 0.676 | 1.919 | 0.491 | 0.729   | 0.72    | 0.722   |
| Genetic Programming        | 0.636             | 0.636    | 0.633    | 0.635                | 0.637       | 0.634           | 68.4 | 69.9 | 39.8 | 39.3 | 0.642 | 1.78  | 0.571 | 0.693   | 0.669   | 0.668   |
| Gradient Boosting          | 0.656             | 0.656    | 0.663    | 0.685                | 0.627       | 0.645           | 73.8 | 68.8 | 40.9 | 33.9 | 0.672 | 1.866 | 0.501 | 0.723   | 0.711   | 0.712   |
| K-Nearest Neighbors        | 0.653             | 0.653    | 0.654    | 0.663                | 0.644       | 0.647           | 71.4 | 70.6 | 39.1 | 36.3 | 0.661 | 1.894 | 0.527 | 0.714   | 0.689   | 0.683   |
| Light Gradient Boosting    | 0.659             | 0.659    | 0.667    | 0.693                | 0.625       | 0.647           | 74.6 | 68.6 | 41.1 | 33.1 | 0.676 | 1.874 | 0.489 | 0.727   | 0.713   | 0.714   |
| Logistic Regression        | 0.664             | 0.664    | 0.67     | 0.69                 | 0.638       | 0.652           | 74.3 | 70.0 | 39.7 | 33.4 | 0.678 | 1.924 | 0.488 | 0.725   | 0.692   | 0.696   |
| Naive Bayes                | 0.64              | 0.64     | 0.64     | 0.65                 | 0.63        | 0.634           | 70.0 | 69.1 | 40.6 | 37.7 | 0.649 | 1.776 | 0.553 | 0.69    | 0.654   | 0.659   |
| Random Forest              | 0.662             | 0.662    | 0.665    | 0.678                | 0.646       | 0.654           | 73.0 | 70.9 | 38.8 | 34.7 | 0.672 | 1.941 | 0.498 | 0.732   | 0.72    | 0.723   |
| Support Vector Machine     | 0.659             | 0.658    | 0.673    | 0.71                 | 0.607       | 0.64            | 76.5 | 66.6 | 43.1 | 31.2 | 0.682 | 1.832 | 0.478 | 0.72    | 0.7     | 0.703   |

## D2 = B\_GE15\_DX

| ML Algorithm               | Balanced Accuracy | Accuracy | F1 Score | Sensitivity (Recall) | Specificity | Precision (PPV) | TP   | TN   | FP   | FN   | NPV   | LR+   | LR-   | ROC AUC | PRC AUC | PRC APS |
|----------------------------|-------------------|----------|----------|----------------------|-------------|-----------------|------|------|------|------|-------|-------|-------|---------|---------|---------|
| Artificial Neural Network  | 0.555             | 0.555    | 0.569    | 0.56                 | 0.55        | 0.587           | 53.4 | 46.2 | 37.8 | 42.0 | 0.525 | 1.276 | 0.807 | 0.558   | 0.582   | 0.569   |
| Category Gradient Boosting | 0.551             | 0.552    | 0.571    | 0.567                | 0.536       | 0.583           | 54.1 | 45.0 | 39.0 | 41.3 | 0.522 | 1.259 | 0.817 | 0.558   | 0.587   | 0.571   |
| Decision Tree              | 0.548             | 0.548    | 0.561    | 0.551                | 0.544       | 0.581           | 52.6 | 45.7 | 38.3 | 42.8 | 0.517 | 1.264 | 0.837 | 0.557   | 0.573   | 0.569   |
| Elastic Net                | 0.557             | 0.553    | 0.545    | 0.506                | 0.607       | 0.598           | 48.3 | 51.0 | 33.0 | 47.1 | 0.519 | 1.349 | 0.824 | 0.563   | 0.598   | 0.571   |
| ExSTraCS                   | 0.554             | 0.555    | 0.573    | 0.569                | 0.539       | 0.587           | 54.3 | 45.3 | 38.7 | 41.1 | 0.525 | 1.288 | 0.81  | 0.559   | 0.612   | 0.573   |
| Extreme Gradient Boosting  | 0.56              | 0.561    | 0.575    | 0.568                | 0.552       | 0.593           | 54.2 | 46.4 | 37.6 | 41.2 | 0.531 | 1.324 | 0.791 | 0.565   | 0.592   | 0.574   |
| Genetic Programming        | 0.555             | 0.551    | 0.539    | 0.495                | 0.614       | 0.594           | 47.2 | 51.6 | 32.4 | 48.2 | 0.517 | 1.314 | 0.829 | 0.555   | 0.679   | 0.564   |
| Gradient Boosting          | 0.555             | 0.555    | 0.57     | 0.563                | 0.546       | 0.587           | 53.7 | 45.9 | 38.1 | 41.7 | 0.525 | 1.281 | 0.808 | 0.559   | 0.588   | 0.57    |
| K-Nearest Neighbors        | 0.53              | 0.517    | 0.39     | 0.327                | 0.732       | 0.594           | 31.2 | 61.5 | 22.5 | 64.2 | 0.492 | 1.429 | 0.915 | 0.556   | 0.579   | 0.568   |
| Light Gradient Boosting    | 0.553             | 0.553    | 0.57     | 0.564                | 0.542       | 0.584           | 53.8 | 45.5 | 38.5 | 41.6 | 0.524 | 1.263 | 0.812 | 0.563   | 0.594   | 0.576   |
| Logistic Regression        | 0.554             | 0.552    | 0.549    | 0.519                | 0.589       | 0.594           | 49.5 | 49.5 | 34.5 | 45.9 | 0.517 | 1.339 | 0.829 | 0.566   | 0.597   | 0.575   |
| Naive Bayes                | 0.546             | 0.551    | 0.585    | 0.624                | 0.469       | 0.579           | 59.5 | 39.4 | 44.6 | 35.9 | 0.553 | 1.234 | 0.736 | 0.571   | 0.601   | 0.582   |
| Random Forest              | 0.555             | 0.555    | 0.57     | 0.563                | 0.546       | 0.587           | 53.7 | 45.9 | 38.1 | 41.7 | 0.526 | 1.279 | 0.807 | 0.559   | 0.583   | 0.569   |
| Support Vector Machine     | 0.551             | 0.55     | 0.559    | 0.543                | 0.558       | 0.587           | 51.8 | 46.9 | 37.1 | 43.6 | 0.517 | 1.28  | 0.827 | 0.544   | 0.579   | 0.563   |

## D3 = C\_GE15\_SYM

| ML Algorithm               | Balanced Accuracy | Accuracy | F1 Score | Sensitivity (Recall) | Specificity | Precision (PPV) | TP   | TN   | FP   | FN   | NPV   | LR+   | LR-   | ROC AUC | PRC AUC | PRC APS |
|----------------------------|-------------------|----------|----------|----------------------|-------------|-----------------|------|------|------|------|-------|-------|-------|---------|---------|---------|
| Artificial Neural Network  | 0.617             | 0.617    | 0.624    | 0.605                | 0.629       | 0.645           | 57.8 | 53.8 | 31.7 | 37.7 | 0.59  | 1.636 | 0.627 | 0.643   | 0.674   | 0.665   |
| Category Gradient Boosting | 0.608             | 0.608    | 0.62     | 0.607                | 0.61        | 0.635           | 58.0 | 52.1 | 33.4 | 37.5 | 0.583 | 1.585 | 0.647 | 0.649   | 0.688   | 0.667   |
| Decision Tree              | 0.616             | 0.614    | 0.611    | 0.579                | 0.653       | 0.653           | 55.3 | 55.8 | 29.7 | 40.2 | 0.583 | 1.729 | 0.645 | 0.641   | 0.684   | 0.658   |
| Elastic Net                | 0.612             | 0.613    | 0.629    | 0.624                | 0.6         | 0.638           | 59.6 | 51.3 | 34.2 | 35.9 | 0.589 | 1.595 | 0.626 | 0.641   | 0.677   | 0.669   |
| ExSTraCS                   | 0.594             | 0.584    | 0.512    | 0.419                | 0.768       | 0.668           | 40.0 | 65.7 | 19.8 | 55.5 | 0.543 | 1.83  | 0.756 | 0.642   | 0.682   | 0.664   |
| Extreme Gradient Boosting  | 0.615             | 0.613    | 0.61     | 0.576                | 0.655       | 0.652           | 55.0 | 56.0 | 29.5 | 40.5 | 0.581 | 1.712 | 0.651 | 0.648   | 0.682   | 0.665   |
| Genetic Programming        | 0.605             | 0.604    | 0.606    | 0.581                | 0.629       | 0.636           | 55.5 | 53.8 | 31.7 | 40.0 | 0.576 | 1.583 | 0.664 | 0.633   | 0.704   | 0.626   |
| Gradient Boosting          | 0.614             | 0.614    | 0.629    | 0.622                | 0.606       | 0.64            | 59.4 | 51.8 | 33.7 | 36.1 | 0.59  | 1.608 | 0.625 | 0.648   | 0.684   | 0.665   |
| K-Nearest Neighbors        | 0.607             | 0.606    | 0.608    | 0.583                | 0.63        | 0.639           | 55.7 | 53.9 | 31.6 | 39.8 | 0.577 | 1.609 | 0.663 | 0.638   | 0.675   | 0.659   |
| Light Gradient Boosting    | 0.623             | 0.619    | 0.609    | 0.562                | 0.683       | 0.667           | 53.7 | 58.4 | 27.1 | 41.8 | 0.583 | 1.843 | 0.643 | 0.645   | 0.674   | 0.663   |
| Logistic Regression        | 0.614             | 0.614    | 0.627    | 0.619                | 0.608       | 0.64            | 59.1 | 52.0 | 33.5 | 36.4 | 0.59  | 1.612 | 0.627 | 0.645   | 0.681   | 0.669   |
| Naive Bayes                | 0.602             | 0.596    | 0.561    | 0.494                | 0.709       | 0.653           | 47.2 | 60.6 | 24.9 | 48.3 | 0.558 | 1.734 | 0.717 | 0.635   | 0.678   | 0.661   |
| Random Forest              | 0.611             | 0.609    | 0.604    | 0.567                | 0.656       | 0.651           | 54.1 | 56.1 | 29.4 | 41.4 | 0.576 | 1.73  | 0.665 | 0.647   | 0.685   | 0.666   |
| Support Vector Machine     | 0.613             | 0.611    | 0.61     | 0.578                | 0.648       | 0.649           | 55.2 | 55.4 | 30.1 | 40.3 | 0.58  | 1.677 | 0.651 | 0.64    | 0.658   | 0.654   |

## D4 = D\_GE15\_CF

| ML Algorithm               | Balanced Accuracy | Accuracy | F1 Score | Sensitivity (Recall) | Specificity | Precision (PPV) | TP   | TN   | FP   | FN   | NPV   | LR+   | LR-   | ROC AUC | PRC AUC | PRC APS |
|----------------------------|-------------------|----------|----------|----------------------|-------------|-----------------|------|------|------|------|-------|-------|-------|---------|---------|---------|
| Artificial Neural Network  | 0.67              | 0.67     | 0.678    | 0.662                | 0.662       | 0.664           | 73.2 | 72.7 | 37.1 | 34.8 | 0.677 | 2.03  | 0.489 | 0.726   | 0.705   | 0.708   |
| Category Gradient Boosting | 0.665             | 0.666    | 0.648    | 0.623                | 0.708       | 0.677           | 67.3 | 77.7 | 32.1 | 40.7 | 0.657 | 2.141 | 0.532 | 0.727   | 0.714   | 0.717   |
| Decision Tree              | 0.626             | 0.626    | 0.622    | 0.625                | 0.626       | 0.624           | 67.5 | 68.8 | 41.0 | 40.5 | 0.631 | 1.707 | 0.598 | 0.684   | 0.672   | 0.663   |
| Elastic Net                | 0.67              | 0.67     | 0.668    | 0.669                | 0.672       | 0.668           | 72.2 | 73.8 | 36.0 | 35.8 | 0.674 | 2.082 | 0.496 | 0.729   | 0.706   | 0.708   |
| ExSTraCS                   | 0.661             | 0.66     | 0.667    | 0.689                | 0.632       | 0.65            | 74.4 | 69.4 | 40.4 | 33.6 | 0.675 | 1.922 | 0.494 | 0.716   | 0.698   | 0.702   |
| Extreme Gradient Boosting  | 0.661             | 0.662    | 0.654    | 0.645                | 0.678       | 0.663           | 69.7 | 74.4 | 35.4 | 38.3 | 0.661 | 2.012 | 0.523 | 0.723   | 0.711   | 0.714   |
| Genetic Programming        | 0.631             | 0.632    | 0.618    | 0.601                | 0.662       | 0.636           | 64.9 | 72.7 | 37.1 | 43.1 | 0.628 | 1.784 | 0.603 | 0.681   | 0.667   | 0.665   |
| Gradient Boosting          | 0.657             | 0.658    | 0.651    | 0.644                | 0.67        | 0.658           | 69.6 | 73.6 | 36.2 | 38.4 | 0.658 | 1.987 | 0.532 | 0.717   | 0.704   | 0.708   |
| K-Nearest Neighbors        | 0.661             | 0.661    | 0.649    | 0.633                | 0.689       | 0.669           | 68.4 | 75.6 | 34.2 | 39.6 | 0.656 | 2.099 | 0.535 | 0.718   | 0.701   | 0.701   |
| Light Gradient Boosting    | 0.656             | 0.657    | 0.65     | 0.645                | 0.668       | 0.657           | 69.7 | 73.0 | 36.5 | 38.3 | 0.659 | 1.959 | 0.531 | 0.722   | 0.709   | 0.712   |
| Logistic Regression        | 0.669             | 0.669    | 0.669    | 0.674                | 0.665       | 0.664           | 72.8 | 73.3 | 36.8 | 35.2 | 0.676 | 2.031 | 0.492 | 0.728   | 0.703   | 0.707   |
| Naive Bayes                | 0.642             | 0.642    | 0.632    | 0.621                | 0.663       | 0.645           | 67.1 | 72.8 | 37.0 | 40.9 | 0.641 | 1.868 | 0.572 | 0.701   | 0.673   | 0.677   |
| Random Forest              | 0.663             | 0.663    | 0.658    | 0.656                | 0.67        | 0.662           | 70.8 | 73.6 | 36.2 | 37.2 | 0.665 | 2.002 | 0.514 | 0.727   | 0.712   | 0.716   |
| Support Vector Machine     | 0.657             | 0.657    | 0.658    | 0.667                | 0.647       | 0.65            | 72.0 | 71.1 | 38.7 | 36.0 | 0.665 | 1.912 | 0.518 | 0.719   | 0.696   | 0.7     |

## D5 = E\_GE15\_IO

| ML Algorithm               | Balanced Accuracy | Accuracy | F1 Score | Sensitivity (Recall) | Specificity | Precision (PPV) | TP   | TN   | FP   | FN   | NPV   | LR+   | LR-   | ROC AUC | PRC AUC | PRC APS |
|----------------------------|-------------------|----------|----------|----------------------|-------------|-----------------|------|------|------|------|-------|-------|-------|---------|---------|---------|
| Artificial Neural Network  | 0.597             | 0.597    | 0.586    | 0.582                | 0.611       | 0.59            | 61.1 | 66.6 | 42.4 | 43.8 | 0.604 | 1.509 | 0.685 | 0.638   | 0.624   | 0.628   |
| Category Gradient Boosting | 0.576             | 0.577    | 0.548    | 0.525                | 0.627       | 0.574           | 55.1 | 68.3 | 40.7 | 49.8 | 0.58  | 1.419 | 0.759 | 0.614   | 0.592   | 0.596   |
| Decision Tree              | 0.548             | 0.548    | 0.551    | 0.568                | 0.528       | 0.537           | 59.6 | 57.6 | 51.4 | 45.3 | 0.561 | 1.213 | 0.821 | 0.567   | 0.557   | 0.55    |
| Elastic Net                | 0.591             | 0.591    | 0.58     | 0.577                | 0.606       | 0.584           | 60.5 | 66.0 | 43.0 | 44.4 | 0.598 | 1.471 | 0.701 | 0.635   | 0.621   | 0.625   |
| ExSTraCS                   | 0.577             | 0.576    | 0.571    | 0.58                 | 0.573       | 0.566           | 60.8 | 62.5 | 46.5 | 44.1 | 0.589 | 1.364 | 0.731 | 0.604   | 0.587   | 0.592   |
| Extreme Gradient Boosting  | 0.582             | 0.582    | 0.566    | 0.557                | 0.606       | 0.578           | 58.4 | 66.1 | 42.9 | 46.5 | 0.587 | 1.43  | 0.733 | 0.619   | 0.607   | 0.611   |
| Genetic Programming        | 0.573             | 0.573    | 0.559    | 0.553                | 0.593       | 0.566           | 58.0 | 64.6 | 44.4 | 46.9 | 0.58  | 1.366 | 0.757 | 0.603   | 0.577   | 0.583   |
| Gradient Boosting          | 0.573             | 0.573    | 0.553    | 0.539                | 0.606       | 0.57            | 56.5 | 66.1 | 42.9 | 48.4 | 0.577 | 1.393 | 0.765 | 0.614   | 0.6     | 0.604   |
| K-Nearest Neighbors        | 0.562             | 0.564    | 0.52     | 0.484                | 0.64        | 0.563           | 50.8 | 69.8 | 39.2 | 54.1 | 0.565 | 1.355 | 0.806 | 0.594   | 0.582   | 0.584   |
| Light Gradient Boosting    | 0.569             | 0.569    | 0.557    | 0.555                | 0.583       | 0.561           | 58.2 | 63.5 | 45.5 | 46.7 | 0.577 | 1.338 | 0.765 | 0.614   | 0.594   | 0.599   |
| Logistic Regression        | 0.602             |          |          |                      |             |                 |      |      |      |      |       |       |       |         |         |         |

# Average Model Prediction Statistics (Rounded to 3 Decimal Points): Page 2

## D6 = F\_GE15\_DEMDX

| ML Algorithm               | Balanced Accuracy | Accuracy | F1 Score | Sensitivity (Recall) | Specificity | Precision (PPV) | TP   | TN   | FP   | FN   | NPV   | LR+   | LR-   | ROC AUC | PRC AUC | PRC APS |
|----------------------------|-------------------|----------|----------|----------------------|-------------|-----------------|------|------|------|------|-------|-------|-------|---------|---------|---------|
| Artificial Neural Network  | 0.645             | 0.65     | 0.684    | 0.718                | 0.573       | 0.654           | 68.8 | 48.8 | 36.4 | 27.0 | 0.646 | 1.693 | 0.494 | 0.706   | 0.704   | 0.708   |
| Category Gradient Boosting | 0.646             | 0.652    | 0.695    | 0.749                | 0.543       | 0.649           | 71.8 | 46.3 | 38.9 | 24.0 | 0.659 | 1.664 | 0.464 | 0.719   | 0.736   | 0.738   |
| Decision Tree              | 0.643             | 0.645    | 0.667    | 0.676                | 0.61        | 0.661           | 64.8 | 52.0 | 33.2 | 31.0 | 0.629 | 1.74  | 0.528 | 0.687   | 0.697   | 0.689   |
| Elastic Net                | 0.646             | 0.65     | 0.681    | 0.708                | 0.585       | 0.658           | 67.8 | 49.8 | 35.4 | 28.0 | 0.642 | 1.728 | 0.501 | 0.706   | 0.706   | 0.709   |
| ExSTraCS                   | 0.64              | 0.642    | 0.664    | 0.669                | 0.611       | 0.66            | 64.1 | 52.1 | 33.1 | 31.7 | 0.622 | 1.734 | 0.543 | 0.706   | 0.716   | 0.719   |
| Extreme Gradient Boosting  | 0.661             | 0.664    | 0.692    | 0.713                | 0.609       | 0.673           | 68.3 | 51.9 | 33.3 | 27.5 | 0.655 | 1.862 | 0.474 | 0.714   | 0.725   | 0.727   |
| Genetic Programming        | 0.626             | 0.629    | 0.657    | 0.674                | 0.577       | 0.643           | 64.6 | 49.2 | 36.0 | 31.2 | 0.613 | 1.608 | 0.565 | 0.674   | 0.701   | 0.687   |
| Gradient Boosting          | 0.65              | 0.656    | 0.695    | 0.741                | 0.56        | 0.655           | 71.0 | 47.7 | 37.5 | 24.8 | 0.658 | 1.7   | 0.465 | 0.715   | 0.726   | 0.729   |
| K-Nearest Neighbors        | 0.611             | 0.617    | 0.658    | 0.699                | 0.523       | 0.623           | 67.0 | 44.6 | 40.6 | 28.8 | 0.609 | 1.476 | 0.575 | 0.668   | 0.665   | 0.666   |
| Light Gradient Boosting    | 0.649             | 0.652    | 0.682    | 0.705                | 0.594       | 0.662           | 67.5 | 50.6 | 34.6 | 28.3 | 0.642 | 1.775 | 0.501 | 0.718   | 0.73    | 0.732   |
| Logistic Regression        | 0.655             | 0.657    | 0.682    | 0.695                | 0.615       | 0.67            | 66.6 | 52.4 | 32.8 | 29.2 | 0.644 | 1.827 | 0.497 | 0.714   | 0.712   | 0.716   |
| Naive Bayes                | 0.61              | 0.615    | 0.657    | 0.697                | 0.523       | 0.623           | 66.8 | 44.6 | 40.6 | 29.0 | 0.607 | 1.479 | 0.579 | 0.652   | 0.646   | 0.651   |
| Random Forest              | 0.656             | 0.659    | 0.689    | 0.716                | 0.595       | 0.667           | 68.6 | 50.7 | 34.5 | 27.2 | 0.653 | 1.805 | 0.477 | 0.718   | 0.731   | 0.733   |
| Support Vector Machine     | 0.648             | 0.653    | 0.691    | 0.734                | 0.562       | 0.654           | 70.3 | 47.9 | 37.3 | 25.5 | 0.655 | 1.692 | 0.474 | 0.708   | 0.712   | 0.716   |

## D7 = G\_GE15\_DEMDXSYM

| ML Algorithm               | Balanced Accuracy | Accuracy | F1 Score | Sensitivity (Recall) | Specificity | Precision (PPV) | TP   | TN   | FP   | FN   | NPV   | LR+   | LR-   | ROC AUC | PRC AUC | PRC APS |
|----------------------------|-------------------|----------|----------|----------------------|-------------|-----------------|------|------|------|------|-------|-------|-------|---------|---------|---------|
| Artificial Neural Network  | 0.661             | 0.665    | 0.697    | 0.732                | 0.59        | 0.666           | 70.8 | 51.2 | 35.5 | 25.9 | 0.666 | 1.806 | 0.456 | 0.731   | 0.737   | 0.74    |
| Category Gradient Boosting | 0.662             | 0.666    | 0.7      | 0.737                | 0.587       | 0.667           | 71.3 | 50.9 | 35.8 | 25.4 | 0.667 | 1.825 | 0.452 | 0.732   | 0.742   | 0.745   |
| Decision Tree              | 0.654             | 0.657    | 0.683    | 0.702                | 0.607       | 0.667           | 67.9 | 52.6 | 34.1 | 28.8 | 0.648 | 1.837 | 0.494 | 0.708   | 0.708   | 0.702   |
| Elastic Net                | 0.664             | 0.666    | 0.69     | 0.706                | 0.622       | 0.677           | 68.3 | 53.9 | 32.8 | 28.4 | 0.656 | 1.899 | 0.475 | 0.734   | 0.742   | 0.745   |
| ExSTraCS                   | 0.677             | 0.68     | 0.707    | 0.734                | 0.619       | 0.686           | 71.0 | 53.7 | 33.0 | 25.7 | 0.678 | 1.992 | 0.428 | 0.734   | 0.74    | 0.744   |
| Extreme Gradient Boosting  | 0.666             | 0.669    | 0.696    | 0.719                | 0.613       | 0.676           | 69.5 | 53.2 | 33.5 | 27.2 | 0.662 | 1.904 | 0.462 | 0.739   | 0.748   | 0.751   |
| Genetic Programming        | 0.64              | 0.643    | 0.675    | 0.711                | 0.569       | 0.648           | 68.7 | 49.3 | 37.4 | 28.0 | 0.645 | 1.665 | 0.506 | 0.7     | 0.715   | 0.706   |
| Gradient Boosting          | 0.675             | 0.679    | 0.7      | 0.747                | 0.604       | 0.679           | 72.2 | 52.4 | 34.3 | 24.5 | 0.683 | 1.935 | 0.424 | 0.735   | 0.74    | 0.742   |
| K-Nearest Neighbors        | 0.641             | 0.646    | 0.686    | 0.735                | 0.547       | 0.644           | 71.1 | 47.4 | 39.3 | 25.6 | 0.652 | 1.638 | 0.487 | 0.7     | 0.71    | 0.709   |
| Light Gradient Boosting    | 0.668             | 0.67     | 0.694    | 0.713                | 0.623       | 0.679           | 68.9 | 54.0 | 32.7 | 27.8 | 0.662 | 1.928 | 0.463 | 0.738   | 0.746   | 0.749   |
| Logistic Regression        | 0.662             | 0.665    | 0.691    | 0.71                 | 0.613       | 0.673           | 68.7 | 53.2 | 33.5 | 28.0 | 0.655 | 1.876 | 0.478 | 0.736   | 0.738   | 0.742   |
| Naive Bayes                | 0.63              | 0.629    | 0.635    | 0.614                | 0.646       | 0.66            | 59.4 | 56.0 | 30.7 | 37.3 | 0.601 | 1.764 | 0.6   | 0.684   | 0.692   | 0.696   |
| Random Forest              | 0.664             | 0.668    | 0.704    | 0.749                | 0.579       | 0.666           | 72.4 | 50.2 | 36.5 | 24.3 | 0.673 | 1.822 | 0.441 | 0.728   | 0.736   | 0.739   |
| Support Vector Machine     | 0.659             | 0.665    | 0.705    | 0.761                | 0.557       | 0.659           | 73.6 | 48.3 | 38.4 | 23.1 | 0.678 | 1.744 | 0.429 | 0.736   | 0.742   | 0.745   |

## D8 = H\_GE15\_DEMDXSYMCF

| ML Algorithm               | Balanced Accuracy | Accuracy | F1 Score | Sensitivity (Recall) | Specificity | Precision (PPV) | TP   | TN   | FP   | FN   | NPV   | LR+   | LR-   | ROC AUC | PRC AUC | PRC APS |
|----------------------------|-------------------|----------|----------|----------------------|-------------|-----------------|------|------|------|------|-------|-------|-------|---------|---------|---------|
| Artificial Neural Network  | 0.688             | 0.688    | 0.686    | 0.687                | 0.689       | 0.685           | 74.2 | 75.7 | 34.1 | 33.8 | 0.692 | 2.232 | 0.455 | 0.764   | 0.741   | 0.744   |
| Category Gradient Boosting | 0.681             | 0.681    | 0.678    | 0.676                | 0.687       | 0.681           | 73.0 | 75.4 | 34.4 | 35.0 | 0.684 | 2.195 | 0.473 | 0.761   | 0.749   | 0.751   |
| Decision Tree              | 0.651             | 0.651    | 0.653    | 0.662                | 0.639       | 0.646           | 71.5 | 70.2 | 39.6 | 36.5 | 0.657 | 1.893 | 0.534 | 0.707   | 0.684   | 0.676   |
| Elastic Net                | 0.684             | 0.684    | 0.684    | 0.692                | 0.676       | 0.677           | 74.7 | 74.2 | 35.6 | 33.3 | 0.691 | 2.153 | 0.458 | 0.762   | 0.745   | 0.746   |
| ExSTraCS                   | 0.691             | 0.691    | 0.704    | 0.741                | 0.642       | 0.672           | 80.0 | 70.5 | 39.3 | 28.0 | 0.717 | 2.115 | 0.404 | 0.759   | 0.738   | 0.741   |
| Extreme Gradient Boosting  | 0.682             | 0.682    | 0.682    | 0.689                | 0.675       | 0.676           | 74.4 | 74.1 | 35.7 | 33.6 | 0.689 | 2.138 | 0.462 | 0.763   | 0.75    | 0.752   |
| Genetic Programming        | 0.637             | 0.637    | 0.634    | 0.638                | 0.637       | 0.632           | 68.9 | 69.9 | 39.9 | 39.1 | 0.644 | 1.754 | 0.566 | 0.685   | 0.674   | 0.675   |
| Gradient Boosting          | 0.681             | 0.681    | 0.677    | 0.676                | 0.686       | 0.68            | 73.0 | 75.3 | 34.5 | 35.0 | 0.683 | 2.172 | 0.472 | 0.757   | 0.745   | 0.748   |
| K-Nearest Neighbors        | 0.669             | 0.669    | 0.651    | 0.624                | 0.713       | 0.682           | 67.4 | 78.3 | 31.5 | 40.6 | 0.659 | 2.2   | 0.527 | 0.737   | 0.724   | 0.724   |
| Light Gradient Boosting    | 0.687             | 0.687    | 0.69     | 0.702                | 0.673       | 0.68            | 75.8 | 73.9 | 35.9 | 32.2 | 0.697 | 2.184 | 0.443 | 0.763   | 0.75    | 0.752   |
| Logistic Regression        | 0.69              | 0.69     | 0.69     | 0.698                | 0.681       | 0.683           | 75.4 | 74.8 | 35.0 | 32.6 | 0.697 | 2.211 | 0.444 | 0.765   | 0.743   | 0.746   |
| Naive Bayes                | 0.658             | 0.658    | 0.654    | 0.654                | 0.662       | 0.657           | 70.6 | 72.7 | 37.1 | 37.4 | 0.661 | 1.965 | 0.524 | 0.718   | 0.693   | 0.695   |
| Random Forest              | 0.686             | 0.685    | 0.687    | 0.697                | 0.674       | 0.678           | 75.3 | 74.0 | 35.8 | 32.7 | 0.694 | 2.15  | 0.449 | 0.763   | 0.75    | 0.752   |
| Support Vector Machine     | 0.689             | 0.689    | 0.693    | 0.706                | 0.672       | 0.68            | 76.3 | 73.8 | 36.0 | 31.7 | 0.7   | 2.174 | 0.438 | 0.76    | 0.742   | 0.745   |

## D9 = I\_GE15\_DEMDXSYMIO

| ML Algorithm               | Balanced Accuracy | Accuracy | F1 Score | Sensitivity (Recall) | Specificity | Precision (PPV) | TP   | TN   | FP   | FN   | NPV   | LR+   | LR-   | ROC AUC | PRC AUC | PRC APS |
|----------------------------|-------------------|----------|----------|----------------------|-------------|-----------------|------|------|------|------|-------|-------|-------|---------|---------|---------|
| Artificial Neural Network  | 0.668             | 0.668    | 0.669    | 0.679                | 0.657       | 0.662           | 72.9 | 71.7 | 37.5 | 34.5 | 0.676 | 2.03  | 0.493 | 0.743   | 0.729   | 0.732   |
| Category Gradient Boosting | 0.675             | 0.675    | 0.685    | 0.713                | 0.637       | 0.66            | 76.6 | 69.6 | 39.6 | 30.8 | 0.693 | 2.0   | 0.453 | 0.743   | 0.724   | 0.727   |
| Decision Tree              | 0.633             | 0.633    | 0.635    | 0.648                | 0.617       | 0.627           | 69.6 | 67.4 | 41.8 | 37.8 | 0.642 | 1.725 | 0.57  | 0.69    | 0.67    | 0.661   |
| Elastic Net                | 0.671             | 0.671    | 0.675    | 0.688                | 0.655       | 0.664           | 73.9 | 71.5 | 37.7 | 33.5 | 0.681 | 2.053 | 0.481 | 0.743   | 0.733   | 0.736   |
| ExSTraCS                   | 0.674             | 0.674    | 0.686    | 0.717                | 0.631       | 0.66            | 77.0 | 68.9 | 40.3 | 30.4 | 0.693 | 2.034 | 0.454 | 0.752   | 0.739   | 0.741   |
| Extreme Gradient Boosting  | 0.678             | 0.678    | 0.684    | 0.705                | 0.651       | 0.666           | 75.7 | 71.1 | 38.1 | 31.7 | 0.692 | 2.049 | 0.455 | 0.743   | 0.733   | 0.735   |
| Genetic Programming        | 0.647             | 0.647    | 0.652    | 0.669                | 0.625       | 0.639           | 71.9 | 68.2 | 41.0 | 35.5 | 0.659 | 1.829 | 0.529 | 0.7     | 0.675   | 0.677   |
| Gradient Boosting          | 0.673             | 0.673    | 0.679    | 0.696                | 0.651       | 0.664           | 74.7 | 71.1 | 38.1 | 32.7 | 0.685 | 2.053 | 0.471 | 0.746   | 0.734   | 0.736   |
| K-Nearest Neighbors        | 0.635             | 0.635    | 0.624    | 0.613                | 0.657       | 0.638           | 65.8 | 71.8 | 37.4 | 41.6 | 0.634 | 1.812 | 0.591 | 0.707   | 0.692   | 0.693   |
| Light Gradient Boosting    | 0.675             | 0.675    | 0.68     | 0.696                | 0.655       | 0.666           | 74.7 | 71.5 | 37.7 | 32.7 | 0.686 | 2.052 | 0.467 | 0.744   | 0.734   | 0.736   |
| Logistic Regression        | 0.663             | 0.663    | 0.667    | 0.681                | 0.646       | 0.655           | 73.1 | 70.5 | 38.7 | 34.3 | 0.673 | 1.978 | 0.5   | 0.742   | 0.728   | 0.731   |
| Naive Bayes                | 0.625             | 0.625    | 0.593    | 0.554                | 0.695       | 0.641           | 59.5 | 75.9 | 33.3 | 47.9 | 0.614 | 1.858 | 0.645 | 0.686   | 0.663   | 0.667   |
| Random Forest              | 0.678             | 0.678    | 0.689    | 0.721                | 0.635       | 0.661           | 77.4 | 69.4 | 39.8 | 30.0 | 0.698 | 2.004 | 0.441 | 0.746   | 0.73    | 0.733   |
| Support Vector Machine     | 0.666             | 0.666    | 0.673    | 0.694                | 0.638       | 0.655           | 74.5 | 69.7 | 39.5 | 32.9 | 0.68  | 1.973 | 0.484 | 0.743   | 0.73    | 0.733   |

## D10 = J\_GE15\_DEMDXSYMCFIO

| ML Algorithm               | Balanced Accuracy | Accuracy | F1 Score | Sensitivity (Recall) | Specificity | Precision (PPV) | TP   | TN   | FP   | FN   | NPV   | LR+   | LR-   | ROC AUC | PRC AUC | PRC APS |
|----------------------------|-------------------|----------|----------|----------------------|-------------|-----------------|------|------|------|------|-------|-------|-------|---------|---------|---------|
| Artificial Neural Network  | 0.685             | 0.685    | 0.685    | 0.691                | 0.678       | 0.68            | 74.6 | 74.5 | 35.3 | 33.4 | 0.691 | 2.169 | 0.456 | 0.759   | 0.739   | 0.742   |
| Category Gradient Boosting | 0.696             | 0.696    | 0.693    | 0.694                | 0.697       | 0.693           | 75.0 | 76.5 | 33.3 | 33.0 | 0.7   | 2.31  | 0.438 | 0.761   | 0.748   | 0.75    |
| Decision Tree              | 0.661             | 0.661    | 0.666    | 0.685                | 0.637       | 0.651           | 74.0 | 70.0 | 39.8 | 34.0 | 0.676 | 1.911 | 0.493 | 0.719   | 0.694   | 0.686   |
| Elastic Net                | 0.678             | 0.678    | 0.678    | 0.684                | 0.672       | 0.672           | 73.9 | 73.8 | 36.0 | 34.1 | 0.684 | 2.105 | 0.472 | 0.761   | 0.745   | 0.747   |
| ExSTraCS                   | 0.679             | 0.679    | 0.688    | 0.716                | 0.642       | 0.664           | 77.3 | 70.5 | 39.3 | 30.7 | 0.697 | 2.03  | 0.444 | 0.748   | 0.733   | 0.736   |
| Extreme Gradient Boosting  | 0.685             | 0.685    | 0.683    | 0.684                | 0.685       | 0.681           | 73.9 | 75.2 | 34.6 | 34.1 | 0.688 | 2.184 | 0.461 | 0.758   | 0.746   | 0.748   |
| Genetic Programming        | 0.633             | 0.633    | 0.623    | 0.614                | 0.651       | 0.634           | 66.3 | 71.5 | 38.3 | 41.7 | 0.633 | 1.763 | 0.591 | 0.685   | 0.676   | 0.675   |
| Gradient Boosting          | 0.68              | 0.68     | 0.677    | 0.676                | 0.684       | 0.679           | 73.0 | 75.1 | 34.7 | 35.0 | 0.683 | 2.177 | 0.474 | 0.754   | 0.739   | 0.741   |
| K-Nearest Neighbors        | 0.668             | 0.669    | 0.646    | 0.609                | 0.728       | 0.688           | 65.8 | 79.9 | 29.9 | 42.2 | 0.655 | 2.248 | 0.537 | 0.739   | 0.729   | 0.73    |
| Light Gradient Boosting    | 0.684             | 0.684    | 0.681    | 0.681                | 0.687       | 0.682           | 73.5 | 75.4 | 34.4 | 34.5 | 0.687 | 2.194 | 0.466 | 0.761   | 0.744   | 0.746   |

# Average Model Prediction Statistics (Rounded to 3 Decimal Points): Page 3

## D11 = K\_GE5\_DEM

| ML Algorithm               | Balanced Accuracy | Accuracy | F1 Score | Sensitivity (Recall) | Specificity | Precision (PPV) | TP    | TN   | FP   | FN   | NPV   | LR+   | LR-   | ROC AUC | PRC AUC | PRC APS |
|----------------------------|-------------------|----------|----------|----------------------|-------------|-----------------|-------|------|------|------|-------|-------|-------|---------|---------|---------|
| Artificial Neural Network  | 0.66              | 0.788    | 0.866    | 0.949                | 0.372       | 0.797           | 148.9 | 22.5 | 38.0 | 8.0  | 0.736 | 1.527 | 0.144 | 0.763   | 0.873   | 0.874   |
| Category Gradient Boosting | 0.645             | 0.779    | 0.861    | 0.946                | 0.344       | 0.789           | 148.5 | 20.8 | 39.7 | 8.4  | 0.719 | 1.457 | 0.166 | 0.761   | 0.872   | 0.873   |
| Decision Tree              | 0.657             | 0.672    | 0.75     | 0.69                 | 0.623       | 0.828           | 108.3 | 37.7 | 22.8 | 48.6 | 0.441 | 1.934 | 0.496 | 0.713   | 0.842   | 0.837   |
| Elastic Net                | 0.678             | 0.68     | 0.754    | 0.683                | 0.673       | 0.844           | 107.1 | 40.7 | 19.8 | 49.8 | 0.451 | 2.144 | 0.477 | 0.748   | 0.859   | 0.86    |
| ExSTraCS                   | 0.687             | 0.731    | 0.808    | 0.786                | 0.587       | 0.832           | 123.4 | 35.5 | 25.0 | 33.5 | 0.516 | 1.952 | 0.371 | 0.754   | 0.863   | 0.864   |
| Extreme Gradient Boosting  | 0.689             | 0.718    | 0.794    | 0.753                | 0.625       | 0.839           | 118.2 | 37.8 | 22.7 | 38.7 | 0.495 | 2.056 | 0.401 | 0.755   | 0.868   | 0.869   |
| Genetic Programming        | 0.63              | 0.757    | 0.844    | 0.915                | 0.345       | 0.785           | 143.6 | 20.9 | 39.6 | 13.3 | 0.616 | 1.433 | 0.25  | 0.717   | 0.852   | 0.846   |
| Gradient Boosting          | 0.649             | 0.773    | 0.855    | 0.929                | 0.368       | 0.792           | 145.7 | 22.3 | 38.2 | 11.2 | 0.679 | 1.49  | 0.2   | 0.743   | 0.857   | 0.859   |
| K-Nearest Neighbors        | 0.632             | 0.749    | 0.837    | 0.897                | 0.367       | 0.786           | 140.7 | 22.2 | 38.3 | 16.2 | 0.605 | 1.423 | 0.285 | 0.721   | 0.855   | 0.842   |
| Light Gradient Boosting    | 0.692             | 0.712    | 0.786    | 0.737                | 0.646       | 0.844           | 115.6 | 39.1 | 21.4 | 41.3 | 0.488 | 2.129 | 0.412 | 0.754   | 0.865   | 0.866   |
| Logistic Regression        | 0.68              | 0.682    | 0.756    | 0.685                | 0.674       | 0.845           | 107.5 | 40.8 | 19.7 | 49.4 | 0.455 | 2.177 | 0.474 | 0.75    | 0.861   | 0.862   |
| Naive Bayes                | 0.652             | 0.729    | 0.815    | 0.826                | 0.478       | 0.804           | 129.6 | 28.9 | 31.6 | 27.3 | 0.517 | 1.609 | 0.373 | 0.71    | 0.841   | 0.842   |
| Random Forest              | 0.683             | 0.713    | 0.791    | 0.752                | 0.613       | 0.834           | 118.0 | 37.1 | 23.4 | 38.9 | 0.491 | 1.98  | 0.409 | 0.759   | 0.869   | 0.87    |
| Support Vector Machine     | 0.689             | 0.71     | 0.785    | 0.735                | 0.643       | 0.843           | 115.4 | 38.9 | 21.6 | 41.5 | 0.485 | 2.146 | 0.416 | 0.751   | 0.862   | 0.864   |

## D12 = L\_GE5\_DX

| ML Algorithm               | Balanced Accuracy | Accuracy | F1 Score | Sensitivity (Recall) | Specificity | Precision (PPV) | TP    | TN   | FP   | FN   | NPV   | LR+   | LR-   | ROC AUC | PRC AUC | PRC APS |
|----------------------------|-------------------|----------|----------|----------------------|-------------|-----------------|-------|------|------|------|-------|-------|-------|---------|---------|---------|
| Artificial Neural Network  | 0.518             | 0.594    | 0.674    | 0.672                | 0.365       | 0.772           | 90.7  | 16.2 | 28.5 | 44.4 | 0.253 | 1.2   | 0.598 | 0.521   | 0.769   | 0.767   |
| Category Gradient Boosting | 0.501             | 0.75     | 0.857    | 0.997                | 0.004       | 0.752           | 134.7 | 0.2  | 44.5 | 0.4  | 0.2   | 1.002 | 0.0   | 0.584   | 0.805   | 0.795   |
| Decision Tree              | 0.57              | 0.566    | 0.659    | 0.563                | 0.577       | 0.802           | 76.0  | 25.8 | 18.9 | 59.1 | 0.304 | 1.353 | 0.762 | 0.586   | 0.803   | 0.796   |
| Elastic Net                | 0.578             | 0.536    | 0.615    | 0.494                | 0.662       | 0.816           | 66.8  | 29.6 | 15.1 | 68.3 | 0.302 | 1.508 | 0.768 | 0.591   | 0.812   | 0.797   |
| ExSTraCS                   | 0.546             | 0.673    | 0.779    | 0.799                | 0.292       | 0.779           | 108.0 | 13.0 | 31.7 | 27.1 | 0.316 | 1.201 | 0.554 | 0.585   | 0.805   | 0.794   |
| Extreme Gradient Boosting  | 0.57              | 0.568    | 0.661    | 0.565                | 0.575       | 0.802           | 76.4  | 25.7 | 19.0 | 58.7 | 0.304 | 1.355 | 0.762 | 0.585   | 0.807   | 0.797   |
| Genetic Programming        | 0.5               | 0.751    | 0.858    | 1.0                  | 0.0         | 0.751           | 135.1 | 0.0  | 44.7 | 0.0  | 0.0   | 1.0   | 0.0   | 0.539   | 0.845   | 0.767   |
| Gradient Boosting          | 0.498             | 0.747    | 0.855    | 0.994                | 0.002       | 0.751           | 134.3 | 0.1  | 44.6 | 0.8  | 0.1   | 0.996 | 0.0   | 0.585   | 0.804   | 0.795   |
| K-Nearest Neighbors        | 0.52              | 0.662    | 0.772    | 0.802                | 0.238       | 0.764           | 108.4 | 10.6 | 34.1 | 26.7 | 0.203 | 1.101 | 0.638 | 0.561   | 0.798   | 0.787   |
| Light Gradient Boosting    | 0.579             | 0.578    | 0.669    | 0.577                | 0.581       | 0.808           | 78.0  | 26.0 | 18.7 | 57.1 | 0.315 | 1.421 | 0.736 | 0.583   | 0.807   | 0.796   |
| Logistic Regression        | 0.578             | 0.544    | 0.627    | 0.511                | 0.644       | 0.813           | 69.0  | 28.8 | 15.9 | 66.1 | 0.303 | 1.486 | 0.766 | 0.587   | 0.808   | 0.796   |
| Naive Bayes                | 0.503             | 0.729    | 0.84     | 0.952                | 0.054       | 0.753           | 128.6 | 2.4  | 42.3 | 6.5  | 0.263 | 1.007 | 1.001 | 0.585   | 0.805   | 0.793   |
| Random Forest              | 0.563             | 0.566    | 0.66     | 0.568                | 0.559       | 0.798           | 76.7  | 25.0 | 19.7 | 58.4 | 0.299 | 1.319 | 0.783 | 0.584   | 0.807   | 0.795   |
| Support Vector Machine     | 0.564             | 0.554    | 0.644    | 0.544                | 0.584       | 0.801           | 73.5  | 26.1 | 18.6 | 61.6 | 0.295 | 1.361 | 0.798 | 0.57    | 0.789   | 0.779   |

## D13 = M\_GE5\_SYM

| ML Algorithm               | Balanced Accuracy | Accuracy | F1 Score | Sensitivity (Recall) | Specificity | Precision (PPV) | TP    | TN   | FP   | FN   | NPV   | LR+   | LR-   | ROC AUC | PRC AUC | PRC APS |
|----------------------------|-------------------|----------|----------|----------------------|-------------|-----------------|-------|------|------|------|-------|-------|-------|---------|---------|---------|
| Artificial Neural Network  | 0.499             | 0.752    | 0.859    | 0.999                | 0.0         | 0.753           | 136.9 | 0.0  | 44.9 | 0.2  | 0.0   | 0.999 | 0.0   | 0.667   | 0.854   | 0.848   |
| Category Gradient Boosting | 0.497             | 0.741    | 0.85     | 0.978                | 0.016       | 0.752           | 134.1 | 0.7  | 44.2 | 3.0  | 0.159 | 0.994 | 0.898 | 0.653   | 0.844   | 0.84    |
| Decision Tree              | 0.646             | 0.627    | 0.71     | 0.608                | 0.684       | 0.855           | 83.4  | 30.7 | 14.2 | 53.7 | 0.364 | 1.982 | 0.575 | 0.667   | 0.859   | 0.841   |
| Elastic Net                | 0.649             | 0.64     | 0.725    | 0.632                | 0.666       | 0.853           | 86.6  | 29.9 | 15.0 | 50.5 | 0.372 | 1.946 | 0.556 | 0.667   | 0.858   | 0.85    |
| ExSTraCS                   | 0.626             | 0.607    | 0.688    | 0.587                | 0.666       | 0.843           | 80.5  | 29.9 | 15.0 | 56.6 | 0.351 | 1.8   | 0.617 | 0.663   | 0.858   | 0.85    |
| Extreme Gradient Boosting  | 0.65              | 0.64     | 0.725    | 0.63                 | 0.67        | 0.855           | 86.4  | 30.1 | 14.8 | 50.7 | 0.373 | 1.971 | 0.553 | 0.665   | 0.86    | 0.849   |
| Genetic Programming        | 0.502             | 0.742    | 0.849    | 0.975                | 0.029       | 0.754           | 133.7 | 1.3  | 43.6 | 3.4  | 0.028 | 1.006 | 0.086 | 0.517   | 0.867   | 0.764   |
| Gradient Boosting          | 0.501             | 0.737    | 0.847    | 0.968                | 0.033       | 0.754           | 132.7 | 1.5  | 43.4 | 4.4  | 0.213 | 1.003 | 0.865 | 0.635   | 0.826   | 0.825   |
| K-Nearest Neighbors        | 0.567             | 0.647    | 0.752    | 0.724                | 0.41        | 0.792           | 99.3  | 18.4 | 26.5 | 37.8 | 0.32  | 1.268 | 0.731 | 0.624   | 0.84    | 0.822   |
| Light Gradient Boosting    | 0.639             | 0.627    | 0.712    | 0.615                | 0.664       | 0.848           | 84.3  | 29.8 | 15.1 | 52.8 | 0.362 | 1.887 | 0.586 | 0.662   | 0.854   | 0.847   |
| Logistic Regression        | 0.649             | 0.642    | 0.728    | 0.635                | 0.664       | 0.853           | 87.1  | 29.8 | 15.1 | 50.0 | 0.373 | 1.929 | 0.552 | 0.665   | 0.853   | 0.847   |
| Naive Bayes                | 0.631             | 0.658    | 0.75     | 0.683                | 0.579       | 0.832           | 93.7  | 26.0 | 18.9 | 43.4 | 0.375 | 1.654 | 0.552 | 0.659   | 0.857   | 0.849   |
| Random Forest              | 0.646             | 0.641    | 0.727    | 0.636                | 0.657       | 0.851           | 87.2  | 29.5 | 15.4 | 49.9 | 0.372 | 1.912 | 0.557 | 0.662   | 0.859   | 0.849   |
| Support Vector Machine     | 0.646             | 0.635    | 0.72     | 0.624                | 0.668       | 0.853           | 85.6  | 30.0 | 14.9 | 51.5 | 0.368 | 1.931 | 0.564 | 0.663   | 0.844   | 0.84    |

## D14 = N\_GE5\_CF

| ML Algorithm               | Balanced Accuracy | Accuracy | F1 Score | Sensitivity (Recall) | Specificity | Precision (PPV) | TP    | TN   | FP   | FN   | NPV   | LR+   | LR-   | ROC AUC | PRC AUC | PRC APS |
|----------------------------|-------------------|----------|----------|----------------------|-------------|-----------------|-------|------|------|------|-------|-------|-------|---------|---------|---------|
| Artificial Neural Network  | 0.645             | 0.751    | 0.836    | 0.883                | 0.408       | 0.795           | 138.9 | 24.7 | 35.9 | 18.4 | 0.574 | 1.505 | 0.289 | 0.731   | 0.863   | 0.864   |
| Category Gradient Boosting | 0.608             | 0.76     | 0.851    | 0.95                 | 0.266       | 0.771           | 149.5 | 16.1 | 44.5 | 7.8  | 0.682 | 1.3   | 0.189 | 0.742   | 0.864   | 0.865   |
| Decision Tree              | 0.633             | 0.642    | 0.724    | 0.652                | 0.614       | 0.814           | 102.6 | 37.2 | 23.4 | 54.7 | 0.407 | 1.733 | 0.574 | 0.679   | 0.824   | 0.824   |
| Elastic Net                | 0.684             | 0.68     | 0.752    | 0.675                | 0.693       | 0.851           | 106.1 | 42.0 | 18.6 | 51.2 | 0.451 | 2.301 | 0.475 | 0.742   | 0.865   | 0.866   |
| ExSTraCS                   | 0.664             | 0.72     | 0.802    | 0.789                | 0.54        | 0.817           | 124.1 | 32.7 | 27.9 | 33.2 | 0.497 | 1.76  | 0.401 | 0.727   | 0.855   | 0.857   |
| Extreme Gradient Boosting  | 0.676             | 0.706    | 0.784    | 0.743                | 0.609       | 0.831           | 116.9 | 36.9 | 23.7 | 40.4 | 0.483 | 1.953 | 0.428 | 0.745   | 0.866   | 0.867   |
| Genetic Programming        | 0.584             | 0.729    | 0.828    | 0.912                | 0.256       | 0.765           | 143.4 | 15.5 | 45.1 | 13.9 | 0.452 | 1.299 | 0.272 | 0.707   | 0.85    | 0.85    |
| Gradient Boosting          | 0.643             | 0.767    | 0.851    | 0.922                | 0.365       | 0.79            | 145.0 | 22.1 | 38.5 | 12.3 | 0.647 | 1.458 | 0.217 | 0.739   | 0.857   | 0.857   |
| K-Nearest Neighbors        | 0.637             | 0.732    | 0.821    | 0.852                | 0.422       | 0.793           | 134.0 | 25.6 | 35.0 | 23.3 | 0.536 | 1.494 | 0.348 | 0.7     | 0.849   | 0.827   |
| Light Gradient Boosting    | 0.666             | 0.685    | 0.764    | 0.708                | 0.625       | 0.831           | 111.3 | 37.9 | 22.7 | 46.0 | 0.452 | 1.952 | 0.475 | 0.734   | 0.861   | 0.863   |
| Logistic Regression        | 0.672             | 0.671    | 0.745    | 0.669                | 0.675       | 0.842           | 105.2 | 40.9 | 19.7 | 52.1 | 0.441 | 2.13  | 0.496 | 0.737   | 0.862   | 0.863   |
| Naive Bayes                | 0.658             | 0.649    | 0.724    | 0.637                | 0.68        | 0.838           | 100.2 | 41.2 | 19.4 | 57.1 | 0.419 | 2.073 | 0.539 | 0.706   | 0.841   | 0.842   |
| Random Forest              | 0.674             | 0.721    | 0.801    | 0.779                | 0.569       | 0.825           | 122.6 | 34.5 | 26.1 | 34.7 | 0.501 | 1.839 | 0.392 | 0.746   | 0.865   | 0.867   |
| Support Vector Machine     | 0.684             | 0.696    | 0.77     | 0.71                 | 0.658       | 0.844           | 111.7 | 39.9 | 20.7 | 45.6 | 0.469 | 2.15  | 0.444 | 0.743   | 0.867   | 0.868   |

## D15 = O\_GE5\_IO

| ML Algorithm               | Balanced Accuracy | Accuracy | F1 Score | Sensitivity (Recall) | Specificity | Precision (PPV) | TP    | TN   | FP   | FN   | NPV   | LR+   | LR-   | ROC AUC | PRC AUC | PRC APS |
|----------------------------|-------------------|----------|----------|----------------------|-------------|-----------------|-------|------|------|------|-------|-------|-------|---------|---------|---------|
| Artificial Neural Network  | 0.551             | 0.694    | 0.8      | 0.879                | 0.222       | 0.745           | 134.9 | 13.4 | 46.9 | 18.5 | 0.452 | 1.155 | 0.493 | 0.614   | 0.797   | 0.799   |
| Category Gradient Boosting | 0.513             | 0.722    | 0.837    | 0.993                | 0.033       | 0.724           | 152.3 | 2.0  | 58.3 | 1.1  | 0.312 | 1.032 | 0.063 | 0.637   | 0.805   | 0.807   |
| Decision Tree              | 0.563             | 0.567    | 0.65     | 0.571                | 0.555       | 0.767           | 87.6  | 33.5 | 26.8 | 65.8 | 0.342 | 1.31  | 0.772 | 0.58    | 0.772   | 0.769   |
| Elastic Net                | 0.618             | 0.616    | 0.695    | 0.613                | 0.622       | 0.806           | 94.1  | 37.5 | 22.8 | 59.3 | 0.388 | 1.672 | 0.626 | 0.65    | 0.814   | 0.816   |
| ExSTraCS                   | 0.568             | 0.635    | 0.737    | 0.722                | 0.415       | 0.758           | 110.7 | 25.0 | 35.3 | 42.7 | 0.375 | 1.245 | 0.679 | 0.613   | 0.791   | 0.793   |
| Extreme Gradient Boosting  | 0.572             | 0.589    | 0.679    | 0.611                | 0.532       | 0.768           | 93.7  | 32.1 | 28.2 | 59.7 | 0.352 | 1.323 | 0.734 | 0.621   | 0.802   | 0.803   |
| Genetic Programming        | 0.502             | 0.716    | 0.834    | 0.993                | 0.01        | 0.719           | 152.4 | 0.6  | 59.7 | 1.0  | 0.038 | 1.004 | 0.066 | 0.512   | 0.842   | 0.728   |
| Gradient Boosting          | 0.55              | 0.688    | 0.799    | 0.867                | 0.232       | 0.742           | 133.0 | 14.0 | 46.3 | 20.4 | 0.431 | 1.131 | 0.568 | 0.579   | 0.775   | 0.777   |
| K-Nearest Neighbors        | 0.524             | 0.664    | 0.783    | 0.847                | 0.201       | 0.73            | 129.9 | 12.1 | 48.2 | 23.5 | 0.352 | 1.066 | 0.794 | 0.541   | 0.757   | 0.739   |
| Light Gradient Boosting    | 0.592             | 0.597    | 0.681    | 0.602                | 0.582       | 0.785           | 92.4  | 35.1 | 25.2 | 61.0 | 0.366 | 1.454 | 0.688 | 0.635   | 0.812   | 0.813   |
| Logistic Regression        | 0.6               |          |          |                      |             |                 |       |      |      |      |       |       |       |         |         |         |

# Average Model Prediction Statistics (Rounded to 3 Decimal Points): Page 4

## D16 = P\_GE5\_DEMDX

| ML Algorithm               | Balanced Accuracy | Accuracy | F1 Score | Sensitivity (Recall) | Specificity | Precision (PPV) | TP    | TN   | FP   | FN   | NPV   | LR+   | LR-   | ROC AUC | PRC AUC | PRC APS |
|----------------------------|-------------------|----------|----------|----------------------|-------------|-----------------|-------|------|------|------|-------|-------|-------|---------|---------|---------|
| Artificial Neural Network  | 0.645             | 0.793    | 0.872    | 0.939                | 0.351       | 0.814           | 127.9 | 15.8 | 29.2 | 8.3  | 0.665 | 1.463 | 0.175 | 0.754   | 0.882   | 0.884   |
| Category Gradient Boosting | 0.633             | 0.786    | 0.868    | 0.938                | 0.329       | 0.809           | 127.7 | 14.8 | 30.2 | 8.5  | 0.641 | 1.41  | 0.196 | 0.738   | 0.883   | 0.884   |
| Decision Tree              | 0.657             | 0.662    | 0.747    | 0.667                | 0.647       | 0.852           | 90.9  | 29.1 | 15.9 | 45.3 | 0.392 | 1.983 | 0.518 | 0.722   | 0.868   | 0.865   |
| Elastic Net                | 0.664             | 0.677    | 0.762    | 0.689                | 0.638       | 0.853           | 93.9  | 28.7 | 16.3 | 42.3 | 0.404 | 2.022 | 0.499 | 0.736   | 0.872   | 0.873   |
| ExSTraCS                   | 0.687             | 0.753    | 0.832    | 0.818                | 0.556       | 0.849           | 111.4 | 25.0 | 20.0 | 24.8 | 0.502 | 1.909 | 0.334 | 0.74    | 0.876   | 0.877   |
| Extreme Gradient Boosting  | 0.654             | 0.693    | 0.781    | 0.73                 | 0.578       | 0.841           | 99.5  | 26.0 | 19.0 | 36.7 | 0.414 | 1.866 | 0.481 | 0.726   | 0.868   | 0.869   |
| Genetic Programming        | 0.563             | 0.76     | 0.857    | 0.955                | 0.171       | 0.778           | 130.1 | 7.7  | 37.3 | 6.1  | 0.449 | 1.171 | 0.219 | 0.667   | 0.854   | 0.841   |
| Gradient Boosting          | 0.634             | 0.78     | 0.863    | 0.924                | 0.344       | 0.81            | 125.8 | 15.5 | 29.5 | 10.4 | 0.6   | 1.42  | 0.228 | 0.72    | 0.864   | 0.865   |
| K-Nearest Neighbors        | 0.634             | 0.746    | 0.835    | 0.856                | 0.411       | 0.816           | 116.6 | 18.5 | 26.5 | 19.6 | 0.489 | 1.482 | 0.349 | 0.686   | 0.872   | 0.839   |
| Light Gradient Boosting    | 0.666             | 0.702    | 0.788    | 0.737                | 0.596       | 0.847           | 100.4 | 26.8 | 18.2 | 35.8 | 0.428 | 1.932 | 0.459 | 0.737   | 0.881   | 0.881   |
| Logistic Regression        | 0.664             | 0.673    | 0.758    | 0.681                | 0.647       | 0.854           | 92.8  | 29.1 | 15.9 | 43.4 | 0.402 | 2.009 | 0.502 | 0.736   | 0.873   | 0.874   |
| Naive Bayes                | 0.623             | 0.737    | 0.828    | 0.85                 | 0.396       | 0.811           | 115.7 | 17.8 | 27.2 | 20.5 | 0.481 | 1.444 | 0.378 | 0.682   | 0.845   | 0.846   |
| Random Forest              | 0.671             | 0.724    | 0.809    | 0.777                | 0.564       | 0.845           | 105.8 | 25.4 | 19.6 | 30.4 | 0.454 | 1.863 | 0.405 | 0.741   | 0.881   | 0.882   |
| Support Vector Machine     | 0.671             | 0.701    | 0.786    | 0.731                | 0.611       | 0.851           | 99.6  | 27.5 | 17.5 | 36.6 | 0.429 | 1.969 | 0.451 | 0.735   | 0.874   | 0.876   |

## D17 = Q\_GE5\_DEMDXSYM

| ML Algorithm               | Balanced Accuracy | Accuracy | F1 Score | Sensitivity (Recall) | Specificity | Precision (PPV) | TP    | TN   | FP   | FN   | NPV   | LR+   | LR-   | ROC AUC | PRC AUC | PRC APS |
|----------------------------|-------------------|----------|----------|----------------------|-------------|-----------------|-------|------|------|------|-------|-------|-------|---------|---------|---------|
| Artificial Neural Network  | 0.661             | 0.798    | 0.874    | 0.933                | 0.389       | 0.822           | 129.1 | 17.8 | 27.9 | 9.2  | 0.665 | 1.541 | 0.174 | 0.762   | 0.894   | 0.895   |
| Category Gradient Boosting | 0.65              | 0.795    | 0.873    | 0.938                | 0.363       | 0.817           | 129.7 | 16.6 | 29.1 | 8.6  | 0.665 | 1.488 | 0.174 | 0.759   | 0.892   | 0.893   |
| Decision Tree              | 0.645             | 0.646    | 0.731    | 0.646                | 0.643       | 0.848           | 89.4  | 29.4 | 16.3 | 48.9 | 0.377 | 1.908 | 0.554 | 0.7     | 0.861   | 0.852   |
| Elastic Net                | 0.689             | 0.703    | 0.784    | 0.717                | 0.661       | 0.865           | 99.1  | 30.2 | 15.5 | 39.2 | 0.435 | 2.216 | 0.435 | 0.768   | 0.897   | 0.897   |
| ExSTraCS                   | 0.699             | 0.755    | 0.833    | 0.81                 | 0.588       | 0.858           | 112.0 | 26.9 | 18.8 | 26.3 | 0.503 | 2.115 | 0.33  | 0.761   | 0.889   | 0.89    |
| Extreme Gradient Boosting  | 0.68              | 0.728    | 0.81     | 0.774                | 0.586       | 0.851           | 107.1 | 26.8 | 18.9 | 31.2 | 0.462 | 1.965 | 0.391 | 0.749   | 0.887   | 0.888   |
| Genetic Programming        | 0.595             | 0.767    | 0.858    | 0.936                | 0.254       | 0.792           | 129.5 | 11.6 | 34.1 | 8.8  | 0.514 | 1.276 | 0.242 | 0.706   | 0.864   | 0.865   |
| Gradient Boosting          | 0.65              | 0.788    | 0.867    | 0.923                | 0.376       | 0.818           | 127.7 | 17.2 | 28.5 | 10.6 | 0.626 | 1.489 | 0.206 | 0.746   | 0.884   | 0.885   |
| K-Nearest Neighbors        | 0.644             | 0.746    | 0.833    | 0.847                | 0.442       | 0.822           | 117.1 | 20.2 | 25.5 | 21.2 | 0.492 | 1.533 | 0.35  | 0.7     | 0.879   | 0.843   |
| Light Gradient Boosting    | 0.679             | 0.716    | 0.799    | 0.752                | 0.606       | 0.854           | 104.0 | 27.7 | 18.0 | 34.3 | 0.447 | 2.002 | 0.411 | 0.752   | 0.886   | 0.887   |
| Logistic Regression        | 0.697             | 0.709    | 0.788    | 0.72                 | 0.674       | 0.871           | 99.6  | 30.8 | 14.9 | 38.7 | 0.442 | 2.359 | 0.421 | 0.769   | 0.897   | 0.898   |
| Naive Bayes                | 0.651             | 0.682    | 0.769    | 0.711                | 0.59        | 0.841           | 98.4  | 27.0 | 18.7 | 39.9 | 0.407 | 1.783 | 0.488 | 0.719   | 0.869   | 0.87    |
| Random Forest              | 0.686             | 0.746    | 0.827    | 0.806                | 0.567       | 0.85            | 111.4 | 25.9 | 19.8 | 26.9 | 0.491 | 1.938 | 0.346 | 0.758   | 0.891   | 0.892   |
| Support Vector Machine     | 0.702             | 0.725    | 0.803    | 0.748                | 0.656       | 0.869           | 103.4 | 30.0 | 15.7 | 34.9 | 0.464 | 2.332 | 0.39  | 0.76    | 0.886   | 0.888   |

## D18 = R\_GE5\_DEMDXSYMCF

| ML Algorithm               | Balanced Accuracy | Accuracy | F1 Score | Sensitivity (Recall) | Specificity | Precision (PPV) | TP    | TN   | FP   | FN   | NPV   | LR+   | LR-   | ROC AUC | PRC AUC | PRC APS |
|----------------------------|-------------------|----------|----------|----------------------|-------------|-----------------|-------|------|------|------|-------|-------|-------|---------|---------|---------|
| Artificial Neural Network  | 0.682             | 0.785    | 0.86     | 0.914                | 0.451       | 0.812           | 143.7 | 27.3 | 33.3 | 13.6 | 0.668 | 1.704 | 0.203 | 0.778   | 0.885   | 0.886   |
| Category Gradient Boosting | 0.651             | 0.788    | 0.867    | 0.959                | 0.343       | 0.792           | 150.8 | 20.8 | 39.8 | 6.5  | 0.762 | 1.476 | 0.127 | 0.789   | 0.893   | 0.894   |
| Decision Tree              | 0.678             | 0.695    | 0.771    | 0.715                | 0.642       | 0.839           | 112.5 | 38.9 | 21.7 | 44.8 | 0.466 | 2.084 | 0.446 | 0.731   | 0.859   | 0.852   |
| Elastic Net                | 0.714             | 0.718    | 0.787    | 0.723                | 0.705       | 0.864           | 113.8 | 42.7 | 17.9 | 43.5 | 0.498 | 2.503 | 0.395 | 0.786   | 0.888   | 0.888   |
| ExSTraCS                   | 0.719             | 0.76     | 0.83     | 0.811                | 0.627       | 0.85            | 127.6 | 38.0 | 22.6 | 29.7 | 0.565 | 2.245 | 0.301 | 0.78    | 0.889   | 0.889   |
| Extreme Gradient Boosting  | 0.705             | 0.746    | 0.819    | 0.797                | 0.612       | 0.842           | 125.4 | 37.1 | 23.5 | 31.9 | 0.54  | 2.086 | 0.334 | 0.793   | 0.895   | 0.895   |
| Genetic Programming        | 0.625             | 0.755    | 0.844    | 0.917                | 0.333       | 0.782           | 144.3 | 20.2 | 40.4 | 13.0 | 0.608 | 1.407 | 0.258 | 0.724   | 0.852   | 0.851   |
| Gradient Boosting          | 0.674             | 0.786    | 0.862    | 0.926                | 0.423       | 0.806           | 145.7 | 25.6 | 35.0 | 11.6 | 0.689 | 1.619 | 0.179 | 0.784   | 0.887   | 0.887   |
| K-Nearest Neighbors        | 0.666             | 0.746    | 0.828    | 0.847                | 0.485       | 0.81            | 133.2 | 29.4 | 31.2 | 24.1 | 0.554 | 1.678 | 0.321 | 0.743   | 0.868   | 0.852   |
| Light Gradient Boosting    | 0.702             | 0.73     | 0.803    | 0.766                | 0.637       | 0.845           | 120.5 | 38.6 | 22.0 | 36.8 | 0.514 | 2.137 | 0.369 | 0.784   | 0.887   | 0.888   |
| Logistic Regression        | 0.704             | 0.71     | 0.781    | 0.718                | 0.69        | 0.857           | 112.9 | 41.8 | 18.8 | 44.4 | 0.487 | 2.378 | 0.412 | 0.785   | 0.889   | 0.89    |
| Naive Bayes                | 0.679             | 0.672    | 0.745    | 0.664                | 0.693       | 0.849           | 104.5 | 42.0 | 18.6 | 52.8 | 0.444 | 2.247 | 0.487 | 0.736   | 0.86    | 0.86    |
| Random Forest              | 0.704             | 0.748    | 0.82     | 0.802                | 0.605       | 0.841           | 126.2 | 36.7 | 23.9 | 31.1 | 0.549 | 2.06  | 0.327 | 0.784   | 0.889   | 0.889   |
| Support Vector Machine     | 0.705             | 0.736    | 0.809    | 0.774                | 0.635       | 0.847           | 121.8 | 38.5 | 22.1 | 35.5 | 0.521 | 2.188 | 0.359 | 0.783   | 0.886   | 0.887   |

## D19 = S\_GE5\_DEMDXSYMIO

| ML Algorithm               | Balanced Accuracy | Accuracy | F1 Score | Sensitivity (Recall) | Specificity | Precision (PPV) | TP    | TN   | FP   | FN   | NPV   | LR+   | LR-   | ROC AUC | PRC AUC | PRC APS |
|----------------------------|-------------------|----------|----------|----------------------|-------------|-----------------|-------|------|------|------|-------|-------|-------|---------|---------|---------|
| Artificial Neural Network  | 0.667             | 0.78     | 0.858    | 0.92                 | 0.413       | 0.804           | 144.3 | 24.8 | 35.2 | 12.5 | 0.669 | 1.591 | 0.198 | 0.764   | 0.882   | 0.882   |
| Category Gradient Boosting | 0.63              | 0.779    | 0.863    | 0.963                | 0.297       | 0.782           | 151.0 | 17.8 | 42.2 | 5.8  | 0.754 | 1.378 | 0.134 | 0.774   | 0.884   | 0.885   |
| Decision Tree              | 0.673             | 0.692    | 0.77     | 0.716                | 0.63        | 0.837           | 112.3 | 37.8 | 22.2 | 44.5 | 0.461 | 2.056 | 0.454 | 0.733   | 0.863   | 0.857   |
| Elastic Net                | 0.689             | 0.699    | 0.773    | 0.711                | 0.668       | 0.848           | 111.4 | 40.1 | 19.9 | 45.4 | 0.471 | 2.255 | 0.441 | 0.769   | 0.883   | 0.884   |
| ExSTraCS                   | 0.705             | 0.74     | 0.813    | 0.784                | 0.627       | 0.845           | 122.9 | 37.6 | 22.4 | 33.9 | 0.534 | 2.197 | 0.355 | 0.766   | 0.882   | 0.883   |
| Extreme Gradient Boosting  | 0.694             | 0.74     | 0.816    | 0.797                | 0.59        | 0.836           | 125.0 | 35.4 | 24.6 | 31.8 | 0.527 | 2.043 | 0.354 | 0.768   | 0.88    | 0.881   |
| Genetic Programming        | 0.585             | 0.715    | 0.815    | 0.877                | 0.293       | 0.767           | 137.5 | 17.6 | 42.4 | 19.3 | 0.447 | 1.275 | 0.365 | 0.695   | 0.843   | 0.841   |
| Gradient Boosting          | 0.665             | 0.779    | 0.857    | 0.92                 | 0.41        | 0.803           | 144.2 | 24.6 | 35.4 | 12.6 | 0.665 | 1.576 | 0.201 | 0.766   | 0.879   | 0.88    |
| K-Nearest Neighbors        | 0.629             | 0.731    | 0.82     | 0.857                | 0.4         | 0.789           | 134.4 | 24.0 | 36.0 | 22.4 | 0.536 | 1.445 | 0.356 | 0.686   | 0.843   | 0.82    |
| Light Gradient Boosting    | 0.691             | 0.726    | 0.802    | 0.769                | 0.613       | 0.839           | 120.5 | 36.8 | 23.2 | 36.3 | 0.506 | 2.058 | 0.383 | 0.764   | 0.877   | 0.878   |
| Logistic Regression        | 0.694             | 0.703    | 0.777    | 0.715                | 0.673       | 0.851           | 112.1 | 40.4 | 19.6 | 44.7 | 0.477 | 2.268 | 0.429 | 0.772   | 0.885   | 0.886   |
| Naive Bayes                | 0.647             | 0.659    | 0.74     | 0.673                | 0.622       | 0.823           | 105.5 | 37.3 | 22.7 | 51.3 | 0.423 | 1.885 | 0.541 | 0.713   | 0.85    | 0.851   |
| Random Forest              | 0.694             | 0.747    | 0.822    | 0.812                | 0.577       | 0.834           | 127.3 | 34.6 | 25.4 | 29.5 | 0.546 | 1.971 | 0.334 | 0.771   | 0.885   | 0.886   |
| Support Vector Machine     | 0.698             | 0.715    | 0.788    | 0.736                | 0.66        | 0.85            | 115.4 | 39.6 | 20.4 | 41.4 | 0.49  | 2.253 | 0.407 | 0.77    | 0.882   | 0.883   |

## D20 = T\_GE5\_DEMDXSYMCFIO

| ML Algorithm               | Balanced Accuracy | Accuracy | F1 Score | Sensitivity (Recall) | Specificity | Precision (PPV) | TP    | TN   | FP   | FN   | NPV   | LR+   | LR-   | ROC AUC | PRC AUC | PRC APS |
|----------------------------|-------------------|----------|----------|----------------------|-------------|-----------------|-------|------|------|------|-------|-------|-------|---------|---------|---------|
| Artificial Neural Network  | 0.673             | 0.772    | 0.85     | 0.896                | 0.449       | 0.809           | 141.0 | 27.2 | 33.4 | 16.3 | 0.627 | 1.65  | 0.234 | 0.785   | 0.891   | 0.891   |
| Category Gradient Boosting | 0.65              | 0.79     | 0.869    | 0.966                | 0.333       | 0.79            | 152.0 | 20.2 | 40.4 | 5.3  | 0.793 | 1.46  | 0.105 | 0.788   | 0.891   | 0.892   |
| Decision Tree              | 0.666             | 0.685    | 0.763    | 0.708                | 0.625       | 0.832           | 111.3 | 37.9 | 22.7 | 46.0 | 0.455 | 1.941 | 0.467 | 0.733   | 0.865   | 0.857   |
| Elastic Net                | 0.716             | 0.724    | 0.793    | 0.734                | 0.698       | 0.863           | 115.4 | 42.3 | 18.3 | 41.9 | 0.504 | 2.504 | 0.384 | 0.789   | 0.894   | 0.894   |
| ExSTraCS                   | 0.716             | 0.753    | 0.823    | 0.799                | 0.634       | 0.85            | 125.7 | 38.4 | 22.2 | 31.6 | 0.551 | 2.247 | 0.319 | 0.78    | 0.885   | 0.886   |
| Extreme Gradient Boosting  | 0.713             | 0.747    | 0.818    | 0.79                 | 0.635       | 0.849           | 124.3 | 38.5 | 22.1 | 33.0 | 0.544 | 2.182 | 0.331 | 0.79    | 0.895   | 0.896   |
| Genetic Programming        | 0.598             | 0.742    | 0.838    | 0.923                | 0.272       | 0.768           | 145.2 | 16.5 | 44.1 | 12.1 | 0.588 | 1.279 | 0.28  | 0.697   | 0.843   | 0.841   |
| Gradient Boosting          | 0.672             | 0.78     | 0.857    | 0.916                | 0.427       | 0.806           | 144.1 | 25.9 | 34.7 | 13.2 | 0.666 | 1.613 | 0.199 | 0.788   | 0.894   | 0.893   |
| K-Nearest Neighbors        | 0.672             | 0.752    | 0.832    | 0.852                | 0.492       | 0.813           | 134.0 | 29.8 | 30.8 | 23.3 | 0.567 | 1.705 | 0.304 | 0.741   | 0.87    | 0.855   |
| Light Gradient Boosting    | 0.705             | 0.736    | 0.809    | 0.776                | 0.634       | 0.846           | 122.0 | 38.4 | 22.2 | 35.3 | 0.523 | 2.144 |       |         |         |         |

# Median Model Prediction Statistics (Rounded to 3 Decimal Points): Page 1

## D1 = A\_GE15\_DEM

| ML Algorithm               | Balanced Accuracy | Accuracy | F1 Score | Sensitivity (Recall) | Specificity | Precision (PPV) | TP   | TN   | FP   | FN   | NPV   | LR+   | LR-   | ROC AUC | PRC AUC | PRC APS |
|----------------------------|-------------------|----------|----------|----------------------|-------------|-----------------|------|------|------|------|-------|-------|-------|---------|---------|---------|
| Artificial Neural Network  | 0.658             | 0.658    | 0.658    | 0.665                | 0.65        | 0.652           | 71.5 | 71.5 | 38.5 | 36.0 | 0.664 | 1.918 | 0.517 | 0.723   | 0.698   | 0.702   |
| Category Gradient Boosting | 0.675             | 0.675    | 0.679    | 0.681                | 0.662       | 0.665           | 73.5 | 72.5 | 37.0 | 34.5 | 0.684 | 2.005 | 0.469 | 0.737   | 0.727   | 0.729   |
| Decision Tree              | 0.66              | 0.66     | 0.662    | 0.679                | 0.63        | 0.646           | 73.0 | 69.0 | 40.5 | 34.5 | 0.672 | 1.875 | 0.503 | 0.704   | 0.679   | 0.672   |
| Elastic Net                | 0.656             | 0.656    | 0.664    | 0.685                | 0.63        | 0.646           | 74.0 | 69.0 | 40.5 | 34.0 | 0.668 | 1.859 | 0.503 | 0.723   | 0.691   | 0.692   |
| ExSTraCS                   | 0.667             | 0.667    | 0.677    | 0.731                | 0.618       | 0.649           | 79.0 | 68.0 | 42.0 | 29.0 | 0.685 | 1.888 | 0.469 | 0.739   | 0.718   | 0.721   |
| Extreme Gradient Boosting  | 0.664             | 0.664    | 0.67     | 0.685                | 0.673       | 0.655           | 74.0 | 74.0 | 36.0 | 34.0 | 0.677 | 1.936 | 0.488 | 0.729   | 0.716   | 0.717   |
| Genetic Programming        | 0.637             | 0.637    | 0.636    | 0.648                | 0.639       | 0.63            | 70.0 | 70.0 | 39.5 | 38.0 | 0.644 | 1.731 | 0.566 | 0.697   | 0.681   | 0.669   |
| Gradient Boosting          | 0.656             | 0.656    | 0.668    | 0.694                | 0.635       | 0.64            | 75.0 | 69.5 | 40.0 | 33.0 | 0.675 | 1.81  | 0.49  | 0.723   | 0.713   | 0.715   |
| K-Nearest Neighbors        | 0.658             | 0.658    | 0.656    | 0.657                | 0.644       | 0.648           | 71.0 | 70.5 | 39.0 | 37.0 | 0.664 | 1.882 | 0.519 | 0.727   | 0.701   | 0.689   |
| Light Gradient Boosting    | 0.659             | 0.658    | 0.673    | 0.694                | 0.648       | 0.651           | 75.0 | 71.0 | 38.5 | 33.0 | 0.682 | 1.902 | 0.477 | 0.731   | 0.713   | 0.709   |
| Logistic Regression        | 0.653             | 0.653    | 0.661    | 0.679                | 0.626       | 0.643           | 73.0 | 68.5 | 41.0 | 34.5 | 0.667 | 1.833 | 0.511 | 0.721   | 0.691   | 0.694   |
| Naive Bayes                | 0.641             | 0.641    | 0.65     | 0.674                | 0.618       | 0.631           | 72.5 | 68.0 | 42.0 | 35.0 | 0.657 | 1.743 | 0.535 | 0.688   | 0.654   | 0.66    |
| Random Forest              | 0.657             | 0.657    | 0.664    | 0.698                | 0.667       | 0.663           | 75.0 | 73.0 | 36.5 | 32.5 | 0.671 | 1.988 | 0.5   | 0.727   | 0.71    | 0.713   |
| Support Vector Machine     | 0.664             | 0.664    | 0.68     | 0.704                | 0.595       | 0.639           | 76.0 | 65.5 | 44.5 | 32.0 | 0.69  | 1.813 | 0.456 | 0.723   | 0.699   | 0.701   |

## D2 = B\_GE15\_DX

| ML Algorithm               | Balanced Accuracy | Accuracy | F1 Score | Sensitivity (Recall) | Specificity | Precision (PPV) | TP   | TN   | FP   | FN   | NPV   | LR+   | LR-   | ROC AUC | PRC AUC | PRC APS |
|----------------------------|-------------------|----------|----------|----------------------|-------------|-----------------|------|------|------|------|-------|-------|-------|---------|---------|---------|
| Artificial Neural Network  | 0.547             | 0.549    | 0.576    | 0.563                | 0.56        | 0.573           | 53.5 | 47.0 | 37.0 | 41.5 | 0.514 | 1.188 | 0.832 | 0.542   | 0.58    | 0.566   |
| Category Gradient Boosting | 0.534             | 0.539    | 0.58     | 0.563                | 0.53        | 0.562           | 53.5 | 44.5 | 39.5 | 41.5 | 0.51  | 1.132 | 0.851 | 0.549   | 0.57    | 0.565   |
| Decision Tree              | 0.531             | 0.535    | 0.568    | 0.547                | 0.536       | 0.56            | 52.0 | 45.0 | 39.0 | 43.0 | 0.503 | 1.122 | 0.87  | 0.561   | 0.577   | 0.575   |
| Elastic Net                | 0.556             | 0.554    | 0.549    | 0.492                | 0.607       | 0.591           | 47.0 | 51.0 | 33.0 | 48.5 | 0.52  | 1.271 | 0.812 | 0.538   | 0.577   | 0.554   |
| ExSTraCS                   | 0.544             | 0.547    | 0.578    | 0.558                | 0.524       | 0.569           | 53.0 | 44.0 | 40.0 | 42.0 | 0.517 | 1.167 | 0.823 | 0.543   | 0.603   | 0.562   |
| Extreme Gradient Boosting  | 0.552             | 0.556    | 0.589    | 0.574                | 0.542       | 0.578           | 54.5 | 45.5 | 38.5 | 40.5 | 0.529 | 1.21  | 0.789 | 0.552   | 0.587   | 0.572   |
| Genetic Programming        | 0.559             | 0.553    | 0.528    | 0.474                | 0.613       | 0.601           | 45.5 | 51.5 | 32.5 | 50.5 | 0.517 | 1.326 | 0.819 | 0.559   | 0.678   | 0.566   |
| Gradient Boosting          | 0.544             | 0.547    | 0.576    | 0.558                | 0.536       | 0.57            | 53.0 | 45.0 | 39.0 | 42.0 | 0.517 | 1.171 | 0.823 | 0.552   | 0.582   | 0.564   |
| K-Nearest Neighbors        | 0.525             | 0.508    | 0.442    | 0.367                | 0.738       | 0.604           | 35.0 | 62.0 | 22.0 | 60.5 | 0.484 | 1.342 | 0.943 | 0.555   | 0.564   | 0.563   |
| Light Gradient Boosting    | 0.547             | 0.55     | 0.58     | 0.563                | 0.542       | 0.572           | 53.5 | 45.5 | 38.5 | 41.5 | 0.518 | 1.182 | 0.82  | 0.562   | 0.583   | 0.571   |
| Logistic Regression        | 0.539             | 0.543    | 0.553    | 0.487                | 0.583       | 0.568           | 46.5 | 49.0 | 35.0 | 49.0 | 0.512 | 1.162 | 0.838 | 0.546   | 0.586   | 0.564   |
| Naive Bayes                | 0.539             | 0.55     | 0.571    | 0.558                | 0.536       | 0.569           | 53.0 | 45.0 | 39.0 | 42.0 | 0.533 | 1.167 | 0.771 | 0.551   | 0.591   | 0.569   |
| Random Forest              | 0.548             | 0.55     | 0.574    | 0.553                | 0.536       | 0.574           | 52.5 | 45.0 | 39.0 | 42.5 | 0.517 | 1.191 | 0.822 | 0.558   | 0.576   | 0.575   |
| Support Vector Machine     | 0.544             | 0.547    | 0.556    | 0.532                | 0.56        | 0.569           | 50.5 | 47.0 | 37.0 | 44.5 | 0.517 | 1.169 | 0.82  | 0.555   | 0.564   | 0.571   |

## D3 = C\_GE15\_SYM

| ML Algorithm               | Balanced Accuracy | Accuracy | F1 Score | Sensitivity (Recall) | Specificity | Precision (PPV) | TP   | TN   | FP   | FN   | NPV   | LR+   | LR-   | ROC AUC | PRC AUC | PRC APS |
|----------------------------|-------------------|----------|----------|----------------------|-------------|-----------------|------|------|------|------|-------|-------|-------|---------|---------|---------|
| Artificial Neural Network  | 0.623             | 0.622    | 0.631    | 0.616                | 0.628       | 0.648           | 58.5 | 54.0 | 32.0 | 36.5 | 0.597 | 1.664 | 0.612 | 0.647   | 0.67    | 0.66    |
| Category Gradient Boosting | 0.614             | 0.616    | 0.624    | 0.615                | 0.585       | 0.627           | 59.0 | 50.0 | 35.5 | 37.0 | 0.589 | 1.521 | 0.624 | 0.644   | 0.685   | 0.667   |
| Decision Tree              | 0.617             | 0.616    | 0.607    | 0.576                | 0.647       | 0.644           | 55.0 | 55.0 | 30.0 | 40.5 | 0.579 | 1.622 | 0.652 | 0.646   | 0.688   | 0.668   |
| Elastic Net                | 0.619             | 0.622    | 0.626    | 0.613                | 0.579       | 0.629           | 58.5 | 49.5 | 36.0 | 37.0 | 0.585 | 1.536 | 0.628 | 0.646   | 0.678   | 0.661   |
| ExSTraCS                   | 0.592             | 0.583    | 0.519    | 0.419                | 0.76        | 0.674           | 40.0 | 65.0 | 20.5 | 55.5 | 0.543 | 1.855 | 0.754 | 0.655   | 0.683   | 0.663   |
| Extreme Gradient Boosting  | 0.615             | 0.613    | 0.61     | 0.578                | 0.651       | 0.65            | 55.5 | 56.0 | 30.0 | 40.5 | 0.579 | 1.659 | 0.646 | 0.657   | 0.685   | 0.675   |
| Genetic Programming        | 0.607             | 0.608    | 0.622    | 0.597                | 0.616       | 0.63            | 57.0 | 53.0 | 33.0 | 38.5 | 0.585 | 1.527 | 0.636 | 0.632   | 0.709   | 0.624   |
| Gradient Boosting          | 0.608             | 0.608    | 0.635    | 0.615                | 0.597       | 0.634           | 59.0 | 51.0 | 34.5 | 37.0 | 0.591 | 1.57  | 0.625 | 0.66    | 0.684   | 0.673   |
| K-Nearest Neighbors        | 0.618             | 0.619    | 0.63     | 0.618                | 0.616       | 0.642           | 59.0 | 53.0 | 33.0 | 36.5 | 0.594 | 1.604 | 0.611 | 0.638   | 0.671   | 0.65    |
| Light Gradient Boosting    | 0.624             | 0.622    | 0.602    | 0.56                 | 0.678       | 0.659           | 53.5 | 58.0 | 27.5 | 42.0 | 0.579 | 1.748 | 0.651 | 0.647   | 0.671   | 0.666   |
| Logistic Regression        | 0.622             | 0.622    | 0.628    | 0.615                | 0.593       | 0.641           | 59.0 | 51.0 | 35.0 | 37.0 | 0.592 | 1.616 | 0.618 | 0.655   | 0.675   | 0.671   |
| Naive Bayes                | 0.613             | 0.608    | 0.582    | 0.516                | 0.708       | 0.671           | 49.5 | 60.5 | 25.0 | 46.5 | 0.568 | 1.813 | 0.681 | 0.652   | 0.68    | 0.662   |
| Random Forest              | 0.612             | 0.61     | 0.592    | 0.552                | 0.637       | 0.647           | 53.0 | 54.5 | 31.0 | 43.0 | 0.571 | 1.628 | 0.673 | 0.66    | 0.692   | 0.673   |
| Support Vector Machine     | 0.61              | 0.608    | 0.611    | 0.578                | 0.64        | 0.638           | 55.5 | 55.0 | 31.0 | 40.5 | 0.576 | 1.597 | 0.664 | 0.649   | 0.652   | 0.649   |

## D4 = D\_GE15\_CF

| ML Algorithm               | Balanced Accuracy | Accuracy | F1 Score | Sensitivity (Recall) | Specificity | Precision (PPV) | TP   | TN   | FP   | FN   | NPV   | LR+   | LR-   | ROC AUC | PRC AUC | PRC APS |
|----------------------------|-------------------|----------|----------|----------------------|-------------|-----------------|------|------|------|------|-------|-------|-------|---------|---------|---------|
| Artificial Neural Network  | 0.677             | 0.677    | 0.679    | 0.699                | 0.662       | 0.668           | 75.5 | 72.5 | 37.0 | 32.5 | 0.686 | 2.051 | 0.466 | 0.726   | 0.713   | 0.716   |
| Category Gradient Boosting | 0.664             | 0.664    | 0.651    | 0.62                 | 0.708       | 0.676           | 67.0 | 77.5 | 32.0 | 41.0 | 0.657 | 2.107 | 0.53  | 0.733   | 0.718   | 0.72    |
| Decision Tree              | 0.628             | 0.628    | 0.627    | 0.634                | 0.614       | 0.62            | 68.5 | 67.5 | 42.5 | 39.5 | 0.63  | 1.665 | 0.596 | 0.685   | 0.687   | 0.674   |
| Elastic Net                | 0.674             | 0.674    | 0.679    | 0.681                | 0.659       | 0.661           | 73.5 | 72.5 | 37.5 | 34.5 | 0.686 | 1.981 | 0.466 | 0.734   | 0.717   | 0.72    |
| ExSTraCS                   | 0.657             | 0.656    | 0.667    | 0.69                 | 0.644       | 0.639           | 74.5 | 70.5 | 39.0 | 33.5 | 0.677 | 1.994 | 0.486 | 0.724   | 0.698   | 0.702   |
| Extreme Gradient Boosting  | 0.671             | 0.671    | 0.66     | 0.644                | 0.677       | 0.664           | 69.5 | 74.5 | 35.5 | 38.5 | 0.667 | 2.009 | 0.509 | 0.728   | 0.72    | 0.722   |
| Genetic Programming        | 0.627             | 0.628    | 0.618    | 0.606                | 0.655       | 0.631           | 65.5 | 72.0 | 38.0 | 42.5 | 0.625 | 1.734 | 0.608 | 0.689   | 0.672   | 0.669   |
| Gradient Boosting          | 0.663             | 0.663    | 0.651    | 0.653                | 0.65        | 0.661           | 70.5 | 71.5 | 38.5 | 37.5 | 0.658 | 1.975 | 0.53  | 0.722   | 0.719   | 0.721   |
| K-Nearest Neighbors        | 0.663             | 0.663    | 0.66     | 0.639                | 0.677       | 0.66            | 69.0 | 74.5 | 35.5 | 39.0 | 0.667 | 1.981 | 0.509 | 0.719   | 0.703   | 0.707   |
| Light Gradient Boosting    | 0.661             | 0.661    | 0.664    | 0.653                | 0.664       | 0.663           | 70.5 | 73.0 | 37.0 | 37.5 | 0.668 | 1.991 | 0.503 | 0.725   | 0.714   | 0.717   |
| Logistic Regression        | 0.678             | 0.678    | 0.679    | 0.681                | 0.671       | 0.673           | 73.5 | 73.5 | 36.0 | 34.5 | 0.683 | 2.085 | 0.47  | 0.731   | 0.709   | 0.714   |
| Naive Bayes                | 0.642             | 0.642    | 0.639    | 0.602                | 0.659       | 0.639           | 65.0 | 72.5 | 37.5 | 43.0 | 0.644 | 1.792 | 0.56  | 0.702   | 0.681   | 0.686   |
| Random Forest              | 0.669             | 0.669    | 0.667    | 0.653                | 0.68        | 0.67            | 70.5 | 74.5 | 35.0 | 37.5 | 0.673 | 2.057 | 0.496 | 0.734   | 0.708   | 0.711   |
| Support Vector Machine     | 0.661             | 0.661    | 0.662    | 0.667                | 0.645       | 0.658           | 72.0 | 71.0 | 39.0 | 36.0 | 0.668 | 1.959 | 0.506 | 0.722   | 0.7     | 0.703   |

## D5 = E\_GE15\_IO

| ML Algorithm               | Balanced Accuracy | Accuracy | F1 Score | Sensitivity (Recall) | Specificity | Precision (PPV) | TP   | TN   | FP   | FN   | NPV   | LR+   | LR-   | ROC AUC | PRC AUC | PRC APS |
|----------------------------|-------------------|----------|----------|----------------------|-------------|-----------------|------|------|------|------|-------|-------|-------|---------|---------|---------|
| Artificial Neural Network  | 0.597             | 0.597    | 0.592    | 0.589                | 0.615       | 0.587           | 61.5 | 67.0 | 42.0 | 43.0 | 0.607 | 1.483 | 0.674 | 0.633   | 0.603   | 0.607   |
| Category Gradient Boosting | 0.573             | 0.574    | 0.536    | 0.505                | 0.624       | 0.572           | 53.0 | 68.0 | 41.0 | 52.0 | 0.573 | 1.392 | 0.774 | 0.618   | 0.571   | 0.578   |
| Decision Tree              | 0.55              | 0.549    | 0.55     | 0.548                | 0.541       | 0.537           | 57.5 | 59.0 | 50.0 | 47.5 | 0.564 | 1.204 | 0.804 | 0.567   | 0.558   | 0.549   |
| Elastic Net                | 0.591             | 0.591    | 0.586    | 0.576                | 0.619       | 0.588           | 60.5 | 67.5 | 41.5 | 44.5 | 0.6   | 1.481 | 0.691 | 0.64    | 0.626   | 0.629   |
| ExSTraCS                   | 0.582             | 0.582    | 0.582    | 0.595                | 0.592       | 0.567           | 62.5 | 64.5 | 44.5 | 42.5 | 0.59  | 1.364 | 0.721 | 0.612   | 0.573   | 0.58    |
| Extreme Gradient Boosting  | 0.574             | 0.575    | 0.569    | 0.562                | 0.615       | 0.574           | 59.0 | 67.0 | 42.0 | 46.0 | 0.582 | 1.399 | 0.746 | 0.614   | 0.596   | 0.6     |
| Genetic Programming        | 0.579             | 0.579    | 0.554    | 0.543                | 0.596       | 0.574           | 57.0 | 65.0 | 44.0 | 48.0 | 0.582 | 1.397 | 0.747 | 0.615   | 0.596   | 0.601   |
| Gradient Boosting          | 0.568             | 0.568    | 0.552    | 0.529                | 0.596       | 0.56            | 55.5 | 65.0 | 44.0 | 49.5 | 0.576 | 1.323 | 0.766 | 0.612   | 0.599   | 0.603   |
| K-Nearest Neighbors        | 0.562             | 0.563    | 0.526    | 0.481                | 0.647       | 0.561           | 50.5 | 70.5 | 38.5 | 54.5 | 0.567 | 1.329 | 0.798 | 0.596   | 0.578   | 0.582   |
| Light Gradient Boosting    | 0.58              | 0.579    | 0.575    | 0.557                | 0.587       | 0.567           | 58.5 | 64.0 | 45.0 | 46.5 | 0.594 | 1.36  | 0.71  | 0.615   | 0.597   | 0.603   |
| Logistic Regression        | 0.602             | 0.60     |          |                      |             |                 |      |      |      |      |       |       |       |         |         |         |

## Median Model Prediction Statistics (Rounded to 3 Decimal Points): Page 2

### D6 = F\_GE15\_DEMDX

| ML Algorithm               | Balanced Accuracy | Accuracy | F1 Score | Sensitivity (Recall) | Specificity | Precision (PPV) | TP   | TN   | FP   | FN   | NPV   | LR+   | LR-   | ROC AUC | PRC AUC | PRC APS |
|----------------------------|-------------------|----------|----------|----------------------|-------------|-----------------|------|------|------|------|-------|-------|-------|---------|---------|---------|
| Artificial Neural Network  | 0.637             | 0.641    | 0.673    | 0.698                | 0.571       | 0.646           | 67.0 | 48.5 | 36.5 | 29.0 | 0.632 | 1.613 | 0.521 | 0.703   | 0.694   | 0.699   |
| Category Gradient Boosting | 0.642             | 0.649    | 0.692    | 0.738                | 0.52        | 0.642           | 70.5 | 44.5 | 41.0 | 25.0 | 0.657 | 1.587 | 0.467 | 0.72    | 0.734   | 0.736   |
| Decision Tree              | 0.646             | 0.649    | 0.675    | 0.677                | 0.608       | 0.662           | 65.0 | 52.0 | 33.5 | 31.0 | 0.633 | 1.732 | 0.514 | 0.686   | 0.695   | 0.678   |
| Elastic Net                | 0.642             | 0.646    | 0.681    | 0.696                | 0.561       | 0.646           | 66.5 | 48.0 | 37.5 | 29.0 | 0.641 | 1.614 | 0.501 | 0.703   | 0.696   | 0.698   |
| ExSTraCS                   | 0.638             | 0.638    | 0.663    | 0.663                | 0.624       | 0.66            | 63.0 | 53.0 | 32.0 | 32.0 | 0.621 | 1.735 | 0.546 | 0.702   | 0.707   | 0.711   |
| Extreme Gradient Boosting  | 0.662             | 0.666    | 0.703    | 0.724                | 0.6         | 0.671           | 69.5 | 51.0 | 34.0 | 26.5 | 0.667 | 1.81  | 0.443 | 0.715   | 0.729   | 0.731   |
| Genetic Programming        | 0.623             | 0.624    | 0.657    | 0.677                | 0.588       | 0.645           | 65.0 | 50.0 | 35.0 | 31.0 | 0.608 | 1.607 | 0.577 | 0.679   | 0.712   | 0.699   |
| Gradient Boosting          | 0.641             | 0.649    | 0.7      | 0.745                | 0.556       | 0.645           | 71.5 | 47.5 | 38.0 | 24.5 | 0.664 | 1.625 | 0.447 | 0.706   | 0.718   | 0.723   |
| K-Nearest Neighbors        | 0.616             | 0.622    | 0.663    | 0.703                | 0.529       | 0.63            | 67.5 | 45.0 | 40.0 | 28.5 | 0.611 | 1.523 | 0.563 | 0.678   | 0.664   | 0.667   |
| Light Gradient Boosting    | 0.642             | 0.646    | 0.688    | 0.703                | 0.582       | 0.653           | 67.5 | 49.5 | 35.5 | 28.5 | 0.647 | 1.663 | 0.483 | 0.721   | 0.724   | 0.726   |
| Logistic Regression        | 0.647             | 0.649    | 0.674    | 0.688                | 0.612       | 0.662           | 66.0 | 52.0 | 33.0 | 30.0 | 0.634 | 1.751 | 0.517 | 0.711   | 0.706   | 0.71    |
| Naive Bayes                | 0.609             | 0.613    | 0.66     | 0.698                | 0.532       | 0.621           | 67.0 | 45.5 | 40.0 | 29.0 | 0.603 | 1.465 | 0.588 | 0.65    | 0.646   | 0.653   |
| Random Forest              | 0.657             | 0.663    | 0.693    | 0.729                | 0.576       | 0.664           | 70.0 | 49.0 | 36.0 | 26.0 | 0.652 | 1.764 | 0.472 | 0.719   | 0.736   | 0.739   |
| Support Vector Machine     | 0.64              | 0.644    | 0.686    | 0.728                | 0.556       | 0.647           | 69.5 | 47.5 | 38.0 | 26.0 | 0.647 | 1.642 | 0.488 | 0.704   | 0.714   | 0.719   |

### D7 = G\_GE15\_DEMDXSYM

| ML Algorithm               | Balanced Accuracy | Accuracy | F1 Score | Sensitivity (Recall) | Specificity | Precision (PPV) | TP   | TN   | FP   | FN   | NPV   | LR+   | LR-   | ROC AUC | PRC AUC | PRC APS |
|----------------------------|-------------------|----------|----------|----------------------|-------------|-----------------|------|------|------|------|-------|-------|-------|---------|---------|---------|
| Artificial Neural Network  | 0.662             | 0.665    | 0.7      | 0.751                | 0.603       | 0.67            | 72.5 | 52.5 | 34.5 | 24.0 | 0.674 | 1.833 | 0.439 | 0.737   | 0.735   | 0.74    |
| Category Gradient Boosting | 0.67              | 0.673    | 0.704    | 0.747                | 0.615       | 0.674           | 72.5 | 53.5 | 33.5 | 24.5 | 0.67  | 1.867 | 0.441 | 0.737   | 0.735   | 0.74    |
| Decision Tree              | 0.658             | 0.658    | 0.68     | 0.706                | 0.603       | 0.665           | 68.5 | 52.5 | 34.5 | 28.5 | 0.638 | 1.801 | 0.507 | 0.712   | 0.711   | 0.7     |
| Elastic Net                | 0.675             | 0.676    | 0.701    | 0.716                | 0.626       | 0.679           | 69.5 | 54.5 | 32.5 | 27.5 | 0.67  | 1.921 | 0.442 | 0.738   | 0.743   | 0.746   |
| ExSTraCS                   | 0.691             | 0.691    | 0.706    | 0.732                | 0.621       | 0.683           | 71.0 | 54.0 | 33.0 | 26.0 | 0.677 | 1.931 | 0.432 | 0.734   | 0.74    | 0.743   |
| Extreme Gradient Boosting  | 0.667             | 0.67     | 0.697    | 0.711                | 0.626       | 0.67            | 69.0 | 54.5 | 32.5 | 28.0 | 0.663 | 1.83  | 0.457 | 0.737   | 0.74    | 0.743   |
| Genetic Programming        | 0.634             | 0.635    | 0.671    | 0.686                | 0.598       | 0.645           | 66.5 | 52.0 | 35.0 | 30.5 | 0.626 | 1.626 | 0.536 | 0.701   | 0.738   | 0.707   |
| Gradient Boosting          | 0.689             | 0.692    | 0.719    | 0.741                | 0.626       | 0.684           | 71.5 | 54.5 | 32.5 | 25.0 | 0.691 | 1.954 | 0.403 | 0.732   | 0.735   | 0.738   |
| K-Nearest Neighbors        | 0.643             | 0.648    | 0.689    | 0.762                | 0.561       | 0.654           | 73.5 | 48.5 | 38.0 | 23.0 | 0.654 | 1.683 | 0.477 | 0.702   | 0.717   | 0.716   |
| Light Gradient Boosting    | 0.658             | 0.658    | 0.691    | 0.74                 | 0.632       | 0.685           | 71.0 | 55.0 | 32.0 | 25.0 | 0.655 | 1.948 | 0.472 | 0.742   | 0.75    | 0.752   |
| Logistic Regression        | 0.666             | 0.668    | 0.696    | 0.706                | 0.638       | 0.68            | 68.5 | 55.5 | 31.5 | 28.5 | 0.665 | 1.918 | 0.455 | 0.738   | 0.739   | 0.745   |
| Naive Bayes                | 0.624             | 0.624    | 0.628    | 0.613                | 0.644       | 0.658           | 59.5 | 56.0 | 31.0 | 37.5 | 0.597 | 1.733 | 0.609 | 0.675   | 0.69    | 0.694   |
| Random Forest              | 0.669             | 0.673    | 0.705    | 0.751                | 0.592       | 0.667           | 72.5 | 51.5 | 35.5 | 24.0 | 0.675 | 1.804 | 0.434 | 0.733   | 0.736   | 0.738   |
| Support Vector Machine     | 0.67              | 0.673    | 0.715    | 0.768                | 0.566       | 0.665           | 74.5 | 49.0 | 37.5 | 22.5 | 0.69  | 1.791 | 0.404 | 0.741   | 0.74    | 0.744   |

### D8 = H\_GE15\_DEMDXSYMCF

| ML Algorithm               | Balanced Accuracy | Accuracy | F1 Score | Sensitivity (Recall) | Specificity | Precision (PPV) | TP   | TN   | FP   | FN   | NPV   | LR+   | LR-   | ROC AUC | PRC AUC | PRC APS |
|----------------------------|-------------------|----------|----------|----------------------|-------------|-----------------|------|------|------|------|-------|-------|-------|---------|---------|---------|
| Artificial Neural Network  | 0.69              | 0.69     | 0.687    | 0.694                | 0.695       | 0.687           | 75.0 | 76.5 | 33.5 | 33.0 | 0.691 | 2.236 | 0.453 | 0.767   | 0.747   | 0.751   |
| Category Gradient Boosting | 0.674             | 0.674    | 0.671    | 0.685                | 0.689       | 0.682           | 74.0 | 75.5 | 34.0 | 34.0 | 0.678 | 2.187 | 0.484 | 0.76    | 0.753   | 0.754   |
| Decision Tree              | 0.663             | 0.663    | 0.663    | 0.676                | 0.636       | 0.652           | 73.0 | 70.0 | 40.0 | 35.0 | 0.67  | 1.91  | 0.502 | 0.71    | 0.665   | 0.662   |
| Elastic Net                | 0.677             | 0.677    | 0.674    | 0.685                | 0.682       | 0.675           | 74.0 | 75.0 | 35.0 | 34.0 | 0.679 | 2.111 | 0.479 | 0.76    | 0.748   | 0.75    |
| ExSTraCS                   | 0.694             | 0.694    | 0.703    | 0.741                | 0.644       | 0.67            | 80.0 | 70.5 | 39.0 | 28.0 | 0.717 | 2.055 | 0.4   | 0.757   | 0.741   | 0.743   |
| Extreme Gradient Boosting  | 0.687             | 0.687    | 0.687    | 0.685                | 0.68        | 0.68            | 74.0 | 74.5 | 35.0 | 34.0 | 0.691 | 2.158 | 0.454 | 0.762   | 0.752   | 0.754   |
| Genetic Programming        | 0.642             | 0.642    | 0.64     | 0.639                | 0.641       | 0.634           | 69.0 | 70.5 | 39.5 | 39.0 | 0.647 | 1.765 | 0.556 | 0.696   | 0.683   | 0.681   |
| Gradient Boosting          | 0.683             | 0.683    | 0.676    | 0.671                | 0.682       | 0.676           | 72.5 | 75.0 | 35.0 | 35.5 | 0.68  | 2.123 | 0.477 | 0.757   | 0.739   | 0.741   |
| K-Nearest Neighbors        | 0.672             | 0.672    | 0.651    | 0.63                 | 0.718       | 0.68            | 68.0 | 79.0 | 31.0 | 40.0 | 0.657 | 2.169 | 0.53  | 0.744   | 0.711   | 0.715   |
| Light Gradient Boosting    | 0.681             | 0.68     | 0.696    | 0.708                | 0.673       | 0.667           | 76.5 | 74.0 | 36.0 | 31.5 | 0.703 | 2.029 | 0.431 | 0.761   | 0.746   | 0.748   |
| Logistic Regression        | 0.679             | 0.679    | 0.687    | 0.704                | 0.691       | 0.675           | 76.0 | 76.0 | 34.0 | 32.0 | 0.695 | 2.105 | 0.445 | 0.764   | 0.75    | 0.753   |
| Naive Bayes                | 0.665             | 0.665    | 0.659    | 0.648                | 0.655       | 0.657           | 70.0 | 72.0 | 38.0 | 38.0 | 0.665 | 1.947 | 0.513 | 0.728   | 0.705   | 0.709   |
| Random Forest              | 0.685             | 0.685    | 0.687    | 0.694                | 0.668       | 0.674           | 75.0 | 73.5 | 36.5 | 33.0 | 0.692 | 2.096 | 0.452 | 0.76    | 0.752   | 0.754   |
| Support Vector Machine     | 0.685             | 0.685    | 0.687    | 0.704                | 0.658       | 0.671           | 76.0 | 72.0 | 37.5 | 32.0 | 0.693 | 2.068 | 0.451 | 0.765   | 0.749   | 0.751   |

### D9 = I\_GE15\_DEMDXSYMIO

| ML Algorithm               | Balanced Accuracy | Accuracy | F1 Score | Sensitivity (Recall) | Specificity | Precision (PPV) | TP   | TN   | FP   | FN   | NPV   | LR+   | LR-   | ROC AUC | PRC AUC | PRC APS |
|----------------------------|-------------------|----------|----------|----------------------|-------------|-----------------|------|------|------|------|-------|-------|-------|---------|---------|---------|
| Artificial Neural Network  | 0.661             | 0.661    | 0.668    | 0.682                | 0.642       | 0.657           | 73.0 | 70.0 | 39.0 | 34.0 | 0.673 | 1.956 | 0.492 | 0.737   | 0.731   | 0.734   |
| Category Gradient Boosting | 0.672             | 0.672    | 0.68     | 0.721                | 0.656       | 0.668           | 77.5 | 71.5 | 37.5 | 30.0 | 0.689 | 2.043 | 0.46  | 0.745   | 0.724   | 0.727   |
| Decision Tree              | 0.632             | 0.633    | 0.635    | 0.657                | 0.626       | 0.636           | 71.0 | 68.5 | 41.0 | 37.0 | 0.638 | 1.772 | 0.578 | 0.696   | 0.667   | 0.66    |
| Elastic Net                | 0.685             | 0.685    | 0.685    | 0.693                | 0.665       | 0.675           | 74.5 | 72.5 | 36.5 | 33.0 | 0.691 | 2.104 | 0.455 | 0.741   | 0.729   | 0.731   |
| ExSTraCS                   | 0.685             | 0.685    | 0.692    | 0.729                | 0.647       | 0.67            | 78.0 | 70.5 | 38.5 | 29.0 | 0.699 | 2.057 | 0.437 | 0.752   | 0.723   | 0.725   |
| Extreme Gradient Boosting  | 0.682             | 0.682    | 0.689    | 0.712                | 0.656       | 0.674           | 76.5 | 71.5 | 37.5 | 31.0 | 0.693 | 2.108 | 0.447 | 0.749   | 0.733   | 0.734   |
| Genetic Programming        | 0.647             | 0.647    | 0.652    | 0.673                | 0.628       | 0.634           | 72.0 | 68.5 | 40.5 | 35.0 | 0.654 | 1.757 | 0.537 | 0.704   | 0.673   | 0.679   |
| Gradient Boosting          | 0.676             | 0.676    | 0.676    | 0.679                | 0.647       | 0.66            | 73.0 | 70.5 | 38.5 | 34.5 | 0.681 | 1.98  | 0.476 | 0.75    | 0.725   | 0.728   |
| K-Nearest Neighbors        | 0.626             | 0.626    | 0.617    | 0.611                | 0.661       | 0.631           | 66.0 | 72.0 | 37.0 | 42.0 | 0.624 | 1.735 | 0.611 | 0.706   | 0.675   | 0.677   |
| Light Gradient Boosting    | 0.682             | 0.681    | 0.686    | 0.698                | 0.661       | 0.665           | 75.0 | 72.0 | 37.0 | 32.5 | 0.691 | 2.024 | 0.452 | 0.755   | 0.729   | 0.732   |
| Logistic Regression        | 0.658             | 0.658    | 0.657    | 0.684                | 0.647       | 0.657           | 73.5 | 70.5 | 38.5 | 34.0 | 0.664 | 1.946 | 0.517 | 0.746   | 0.719   | 0.722   |
| Naive Bayes                | 0.611             | 0.612    | 0.585    | 0.549                | 0.697       | 0.633           | 59.0 | 76.0 | 33.0 | 48.5 | 0.601 | 1.761 | 0.674 | 0.682   | 0.663   | 0.667   |
| Random Forest              | 0.683             | 0.683    | 0.69     | 0.721                | 0.648       | 0.668           | 77.5 | 71.0 | 38.5 | 30.0 | 0.697 | 2.041 | 0.438 | 0.745   | 0.727   | 0.73    |
| Support Vector Machine     | 0.665             | 0.665    | 0.671    | 0.702                | 0.628       | 0.657           | 75.5 | 68.5 | 40.5 | 32.0 | 0.68  | 1.96  | 0.483 | 0.745   | 0.726   | 0.728   |

### D10 = J\_GE15\_DEMDXSYMCFIO

| ML Algorithm               | Balanced Accuracy | Accuracy | F1 Score | Sensitivity (Recall) | Specificity | Precision (PPV) | TP   | TN   | FP   | FN   | NPV   | LR+   | LR-   | ROC AUC | PRC AUC | PRC APS |
|----------------------------|-------------------|----------|----------|----------------------|-------------|-----------------|------|------|------|------|-------|-------|-------|---------|---------|---------|
| Artificial Neural Network  | 0.681             | 0.68     | 0.686    | 0.685                | 0.686       | 0.675           | 74.0 | 75.5 | 34.5 | 34.0 | 0.693 | 2.111 | 0.45  | 0.761   | 0.739   | 0.742   |
| Category Gradient Boosting | 0.693             | 0.693    | 0.699    | 0.704                | 0.694       | 0.692           | 76.0 | 76.0 | 33.5 | 32.0 | 0.705 | 2.285 | 0.425 | 0.758   | 0.746   | 0.748   |
| Decision Tree              | 0.656             | 0.656    | 0.667    | 0.69                 | 0.627       | 0.641           | 74.5 | 69.0 | 41.0 | 33.5 | 0.674 | 1.819 | 0.494 | 0.724   | 0.708   | 0.696   |
| Elastic Net                | 0.68              | 0.68     | 0.68     | 0.681                | 0.677       | 0.676           | 73.5 | 74.5 | 35.5 | 34.5 | 0.685 | 2.115 | 0.466 | 0.761   | 0.751   | 0.752   |
| ExSTraCS                   | 0.68              | 0.679    | 0.693    | 0.722                | 0.641       | 0.655           | 78.0 | 70.5 | 39.5 | 30.0 | 0.701 | 1.937 | 0.431 | 0.744   | 0.726   | 0.729   |
| Extreme Gradient Boosting  | 0.677             | 0.677    | 0.679    | 0.681                | 0.679       | 0.676           | 73.5 | 74.0 | 35.0 | 34.5 | 0.684 | 2.128 | 0.47  | 0.757   | 0.749   | 0.751   |
| Genetic Programming        | 0.631             | 0.631    | 0.619    | 0.602                | 0.655       | 0.631           | 65.0 | 72.0 | 38.0 | 43.0 | 0.628 | 1.734 | 0.601 | 0.691   | 0.672   | 0.671   |
| Gradient Boosting          | 0.682             | 0.682    | 0.682    | 0.69                 | 0.677       | 0.674           | 74.5 | 74.5 | 35.5 | 33.5 | 0.687 | 2.097 | 0.463 | 0.754   | 0.734   | 0.736   |
| K-Nearest Neighbors        | 0.665             | 0.665    | 0.646    | 0.62                 | 0.723       | 0.691           | 67.0 | 79.5 | 30.5 | 41.0 | 0.652 | 2.267 | 0.54  | 0.739   | 0.721   | 0.723   |
| Light Gradient Boosting    | 0.677             | 0.677    | 0.673    | 0.681                | 0.691       | 0.68            | 73.5 | 76.0 | 34.0 | 34.5 | 0.679 | 2.16  | 0.482 | 0.758   | 0.746   | 0.748   |
| Logistic                   |                   |          |          |                      |             |                 |      |      |      |      |       |       |       |         |         |         |

# Median Model Prediction Statistics (Rounded to 3 Decimal Points): Page 3

## D11 = K\_GE5\_DEM

| ML Algorithm               | Balanced Accuracy | Accuracy | F1 Score | Sensitivity (Recall) | Specificity | Precision (PPV) | TP    | TN   | FP   | FN   | NPV   | LR+   | LR-   | ROC AUC | PRC AUC | PRC APS |
|----------------------------|-------------------|----------|----------|----------------------|-------------|-----------------|-------|------|------|------|-------|-------|-------|---------|---------|---------|
| Artificial Neural Network  | 0.654             | 0.783    | 0.864    | 0.949                | 0.372       | 0.795           | 149.0 | 22.5 | 38.0 | 8.0  | 0.723 | 1.491 | 0.148 | 0.754   | 0.86    | 0.861   |
| Category Gradient Boosting | 0.646             | 0.775    | 0.857    | 0.946                | 0.339       | 0.789           | 148.5 | 20.5 | 40.0 | 8.5  | 0.691 | 1.44  | 0.172 | 0.764   | 0.873   | 0.874   |
| Decision Tree              | 0.649             | 0.683    | 0.758    | 0.704                | 0.628       | 0.822           | 110.5 | 38.0 | 22.5 | 46.5 | 0.45  | 1.77  | 0.472 | 0.707   | 0.832   | 0.833   |
| Elastic Net                | 0.678             | 0.678    | 0.753    | 0.682                | 0.694       | 0.851           | 107.0 | 42.0 | 18.5 | 50.0 | 0.447 | 2.187 | 0.474 | 0.74    | 0.857   | 0.858   |
| ExSTraCS                   | 0.693             | 0.729    | 0.803    | 0.777                | 0.6         | 0.837           | 122.0 | 36.0 | 24.0 | 35.0 | 0.51  | 1.976 | 0.371 | 0.754   | 0.862   | 0.863   |
| Extreme Gradient Boosting  | 0.703             | 0.729    | 0.803    | 0.768                | 0.633       | 0.847           | 120.5 | 38.0 | 22.0 | 36.5 | 0.509 | 2.126 | 0.372 | 0.755   | 0.87    | 0.87    |
| Genetic Programming        | 0.63              | 0.761    | 0.84     | 0.92                 | 0.339       | 0.783           | 144.5 | 20.5 | 40.0 | 12.5 | 0.601 | 1.392 | 0.257 | 0.718   | 0.846   | 0.845   |
| Gradient Boosting          | 0.63              | 0.77     | 0.856    | 0.939                | 0.342       | 0.785           | 147.5 | 20.5 | 39.5 | 9.5  | 0.667 | 1.408 | 0.193 | 0.743   | 0.861   | 0.862   |
| K-Nearest Neighbors        | 0.632             | 0.752    | 0.84     | 0.908                | 0.385       | 0.786           | 142.5 | 23.5 | 37.5 | 14.5 | 0.587 | 1.404 | 0.271 | 0.723   | 0.853   | 0.84    |
| Light Gradient Boosting    | 0.703             | 0.719    | 0.792    | 0.744                | 0.658       | 0.85            | 116.5 | 39.5 | 20.5 | 40.0 | 0.494 | 2.186 | 0.391 | 0.755   | 0.861   | 0.863   |
| Logistic Regression        | 0.677             | 0.677    | 0.754    | 0.682                | 0.678       | 0.848           | 107.0 | 41.0 | 19.5 | 50.0 | 0.444 | 2.142 | 0.479 | 0.751   | 0.86    | 0.861   |
| Naive Bayes                | 0.64              | 0.722    | 0.811    | 0.825                | 0.471       | 0.799           | 129.5 | 28.5 | 32.0 | 27.5 | 0.5   | 1.529 | 0.386 | 0.705   | 0.841   | 0.842   |
| Random Forest              | 0.686             | 0.729    | 0.802    | 0.76                 | 0.612       | 0.837           | 119.0 | 37.0 | 23.5 | 37.5 | 0.51  | 1.978 | 0.37  | 0.768   | 0.867   | 0.868   |
| Support Vector Machine     | 0.695             | 0.72     | 0.791    | 0.742                | 0.656       | 0.845           | 116.5 | 40.0 | 21.0 | 40.5 | 0.497 | 2.143 | 0.39  | 0.752   | 0.862   | 0.862   |

## D12 = L\_GE5\_DX

| ML Algorithm               | Balanced Accuracy | Accuracy | F1 Score | Sensitivity (Recall) | Specificity | Precision (PPV) | TP    | TN   | FP   | FN   | NPV   | LR+   | LR-   | ROC AUC | PRC AUC | PRC APS |
|----------------------------|-------------------|----------|----------|----------------------|-------------|-----------------|-------|------|------|------|-------|-------|-------|---------|---------|---------|
| Artificial Neural Network  | 0.506             | 0.597    | 0.678    | 0.652                | 0.329       | 0.752           | 88.0  | 14.5 | 30.0 | 47.0 | 0.241 | 1.011 | 0.798 | 0.53    | 0.775   | 0.768   |
| Category Gradient Boosting | 0.5               | 0.75     | 0.857    | 1.0                  | 0.0         | 0.751           | 135.0 | 0.0  | 44.5 | 0.0  | 0.0   | 1.0   | 0.0   | 0.576   | 0.804   | 0.792   |
| Decision Tree              | 0.574             | 0.565    | 0.662    | 0.557                | 0.614       | 0.804           | 75.5  | 27.0 | 17.0 | 60.0 | 0.303 | 1.363 | 0.76  | 0.584   | 0.819   | 0.794   |
| Elastic Net                | 0.576             | 0.531    | 0.614    | 0.5                  | 0.663       | 0.812           | 67.5  | 29.0 | 15.0 | 67.5 | 0.301 | 1.44  | 0.774 | 0.58    | 0.809   | 0.791   |
| ExSTraCS                   | 0.522             | 0.668    | 0.767    | 0.734                | 0.348       | 0.764           | 99.5  | 15.5 | 29.0 | 36.0 | 0.306 | 1.069 | 0.656 | 0.565   | 0.796   | 0.787   |
| Extreme Gradient Boosting  | 0.58              | 0.569    | 0.664    | 0.57                 | 0.602       | 0.808           | 77.0  | 26.5 | 17.5 | 58.0 | 0.309 | 1.402 | 0.747 | 0.581   | 0.804   | 0.791   |
| Genetic Programming        | 0.5               | 0.75     | 0.857    | 1.0                  | 0.0         | 0.75            | 135.0 | 0.0  | 45.0 | 0.0  | 0.0   | 1.0   | 0.0   | 0.546   | 0.839   | 0.768   |
| Gradient Boosting          | 0.5               | 0.75     | 0.857    | 1.0                  | 0.0         | 0.75            | 135.0 | 0.0  | 45.0 | 0.0  | 0.0   | 1.0   | 0.0   | 0.576   | 0.799   | 0.791   |
| K-Nearest Neighbors        | 0.5               | 0.689    | 0.797    | 0.812                | 0.167       | 0.752           | 110.0 | 7.5  | 37.5 | 25.5 | 0.223 | 1.0   | 0.658 | 0.564   | 0.79    | 0.779   |
| Light Gradient Boosting    | 0.576             | 0.578    | 0.683    | 0.593                | 0.618       | 0.806           | 80.0  | 27.5 | 17.0 | 55.0 | 0.309 | 1.381 | 0.747 | 0.585   | 0.805   | 0.793   |
| Logistic Regression        | 0.578             | 0.532    | 0.625    | 0.504                | 0.641       | 0.815           | 68.0  | 28.5 | 16.0 | 67.0 | 0.302 | 1.467 | 0.771 | 0.569   | 0.807   | 0.793   |
| Naive Bayes                | 0.502             | 0.731    | 0.841    | 0.956                | 0.044       | 0.752           | 129.0 | 2.0  | 43.0 | 6.0  | 0.268 | 1.004 | 0.783 | 0.572   | 0.795   | 0.787   |
| Random Forest              | 0.57              | 0.564    | 0.66     | 0.557                | 0.607       | 0.803           | 75.5  | 27.0 | 17.5 | 60.0 | 0.3   | 1.351 | 0.778 | 0.581   | 0.799   | 0.79    |
| Support Vector Machine     | 0.568             | 0.549    | 0.632    | 0.515                | 0.641       | 0.805           | 69.5  | 28.5 | 16.0 | 65.5 | 0.297 | 1.358 | 0.779 | 0.568   | 0.787   | 0.782   |

## D13 = M\_GE5\_SYM

| ML Algorithm               | Balanced Accuracy | Accuracy | F1 Score | Sensitivity (Recall) | Specificity | Precision (PPV) | TP    | TN   | FP   | FN   | NPV   | LR+   | LR-   | ROC AUC | PRC AUC | PRC APS |
|----------------------------|-------------------|----------|----------|----------------------|-------------|-----------------|-------|------|------|------|-------|-------|-------|---------|---------|---------|
| Artificial Neural Network  | 0.5               | 0.753    | 0.859    | 1.0                  | 0.0         | 0.753           | 137.0 | 0.0  | 45.0 | 0.0  | 0.0   | 1.0   | 0.0   | 0.668   | 0.85    | 0.841   |
| Category Gradient Boosting | 0.5               | 0.747    | 0.855    | 0.989                | 0.022       | 0.753           | 135.5 | 1.0  | 44.0 | 1.5  | 0.108 | 1.0   | 0.411 | 0.665   | 0.849   | 0.847   |
| Decision Tree              | 0.651             | 0.621    | 0.701    | 0.595                | 0.689       | 0.858           | 81.5  | 31.0 | 14.0 | 55.5 | 0.364 | 1.988 | 0.575 | 0.665   | 0.857   | 0.874   |
| Elastic Net                | 0.649             | 0.646    | 0.728    | 0.631                | 0.667       | 0.851           | 86.5  | 30.0 | 15.0 | 50.5 | 0.373 | 1.875 | 0.546 | 0.68    | 0.859   | 0.849   |
| ExSTraCS                   | 0.631             | 0.626    | 0.72     | 0.628                | 0.667       | 0.844           | 86.0  | 30.0 | 15.0 | 51.0 | 0.35  | 1.747 | 0.611 | 0.672   | 0.859   | 0.849   |
| Extreme Gradient Boosting  | 0.655             | 0.637    | 0.723    | 0.628                | 0.652       | 0.853           | 86.0  | 29.0 | 15.5 | 51.0 | 0.375 | 1.903 | 0.547 | 0.664   | 0.859   | 0.847   |
| Genetic Programming        | 0.5               | 0.753    | 0.859    | 1.0                  | 0.0         | 0.753           | 137.0 | 0.0  | 45.0 | 0.0  | 0.0   | 1.0   | 0.0   | 0.5     | 0.876   | 0.753   |
| Gradient Boosting          | 0.496             | 0.736    | 0.846    | 0.971                | 0.022       | 0.753           | 133.0 | 1.0  | 44.0 | 4.0  | 0.155 | 0.993 | 0.411 | 0.645   | 0.828   | 0.83    |
| K-Nearest Neighbors        | 0.577             | 0.657    | 0.762    | 0.73                 | 0.456       | 0.798           | 100.0 | 20.5 | 24.5 | 37.0 | 0.323 | 1.299 | 0.69  | 0.639   | 0.841   | 0.827   |
| Light Gradient Boosting    | 0.649             | 0.637    | 0.717    | 0.617                | 0.674       | 0.853           | 84.5  | 30.0 | 14.5 | 52.5 | 0.375 | 1.912 | 0.548 | 0.672   | 0.863   | 0.849   |
| Logistic Regression        | 0.651             | 0.646    | 0.728    | 0.631                | 0.667       | 0.852           | 86.5  | 30.0 | 15.0 | 50.5 | 0.377 | 1.886 | 0.535 | 0.673   | 0.853   | 0.845   |
| Naive Bayes                | 0.639             | 0.659    | 0.751    | 0.686                | 0.589       | 0.839           | 94.0  | 26.5 | 18.5 | 43.0 | 0.377 | 1.713 | 0.543 | 0.664   | 0.853   | 0.845   |
| Random Forest              | 0.649             | 0.646    | 0.731    | 0.639                | 0.656       | 0.854           | 87.5  | 29.5 | 15.5 | 49.5 | 0.376 | 1.928 | 0.538 | 0.657   | 0.855   | 0.845   |
| Support Vector Machine     | 0.653             | 0.637    | 0.721    | 0.617                | 0.667       | 0.852           | 84.5  | 30.0 | 15.0 | 52.5 | 0.373 | 1.886 | 0.553 | 0.676   | 0.851   | 0.848   |

## D14 = N\_GE5\_CF

| ML Algorithm               | Balanced Accuracy | Accuracy | F1 Score | Sensitivity (Recall) | Specificity | Precision (PPV) | TP    | TN   | FP   | FN   | NPV   | LR+   | LR-   | ROC AUC | PRC AUC | PRC APS |
|----------------------------|-------------------|----------|----------|----------------------|-------------|-----------------|-------|------|------|------|-------|-------|-------|---------|---------|---------|
| Artificial Neural Network  | 0.653             | 0.748    | 0.836    | 0.886                | 0.438       | 0.802           | 139.5 | 26.5 | 34.0 | 18.0 | 0.566 | 1.547 | 0.295 | 0.731   | 0.864   | 0.865   |
| Category Gradient Boosting | 0.603             | 0.757    | 0.849    | 0.946                | 0.264       | 0.767           | 149.0 | 16.0 | 44.5 | 8.5  | 0.663 | 1.279 | 0.198 | 0.753   | 0.86    | 0.862   |
| Decision Tree              | 0.627             | 0.638    | 0.722    | 0.651                | 0.607       | 0.81            | 102.5 | 37.0 | 24.0 | 55.0 | 0.399 | 1.641 | 0.579 | 0.684   | 0.822   | 0.829   |
| Elastic Net                | 0.683             | 0.686    | 0.755    | 0.67                 | 0.713       | 0.852           | 105.5 | 43.5 | 17.5 | 52.0 | 0.455 | 2.24  | 0.46  | 0.757   | 0.871   | 0.872   |
| ExSTraCS                   | 0.671             | 0.725    | 0.804    | 0.797                | 0.554       | 0.821           | 125.5 | 33.5 | 27.0 | 32.0 | 0.503 | 1.768 | 0.379 | 0.745   | 0.858   | 0.86    |
| Extreme Gradient Boosting  | 0.693             | 0.706    | 0.781    | 0.745                | 0.639       | 0.841           | 117.0 | 39.0 | 22.0 | 40.0 | 0.482 | 1.029 | 0.417 | 0.767   | 0.872   | 0.874   |
| Genetic Programming        | 0.577             | 0.732    | 0.836    | 0.93                 | 0.231       | 0.755           | 146.0 | 14.0 | 46.5 | 11.0 | 0.542 | 1.194 | 0.262 | 0.711   | 0.851   | 0.851   |
| Gradient Boosting          | 0.644             | 0.761    | 0.845    | 0.917                | 0.372       | 0.792           | 144.5 | 22.5 | 38.0 | 13.0 | 0.61  | 1.465 | 0.248 | 0.725   | 0.86    | 0.854   |
| K-Nearest Neighbors        | 0.633             | 0.743    | 0.829    | 0.87                 | 0.402       | 0.793           | 137.0 | 24.5 | 36.5 | 20.5 | 0.544 | 1.487 | 0.32  | 0.7     | 0.852   | 0.826   |
| Light Gradient Boosting    | 0.683             | 0.692    | 0.768    | 0.711                | 0.645       | 0.845           | 112.0 | 39.0 | 21.5 | 45.5 | 0.463 | 2.077 | 0.445 | 0.761   | 0.872   | 0.875   |
| Logistic Regression        | 0.664             | 0.654    | 0.734    | 0.667                | 0.689       | 0.839           | 105.0 | 42.0 | 19.0 | 52.5 | 0.426 | 2.007 | 0.523 | 0.738   | 0.861   | 0.861   |
| Naive Bayes                | 0.666             | 0.648    | 0.719    | 0.64                 | 0.694       | 0.845           | 100.5 | 42.0 | 18.5 | 56.5 | 0.421 | 2.117 | 0.533 | 0.717   | 0.842   | 0.842   |
| Random Forest              | 0.686             | 0.72     | 0.801    | 0.78                 | 0.587       | 0.829           | 122.5 | 35.5 | 25.0 | 34.5 | 0.497 | 1.868 | 0.393 | 0.762   | 0.875   | 0.877   |
| Support Vector Machine     | 0.678             | 0.688    | 0.773    | 0.721                | 0.672       | 0.847           | 113.5 | 41.0 | 20.0 | 44.0 | 0.452 | 2.153 | 0.463 | 0.746   | 0.861   | 0.863   |

## D15 = O\_GE5\_IO

| ML Algorithm               | Balanced Accuracy | Accuracy | F1 Score | Sensitivity (Recall) | Specificity | Precision (PPV) | TP    | TN   | FP   | FN     | NPV   | LR+   | LR-   | ROC AUC | PRC AUC | PRC APS |
|----------------------------|-------------------|----------|----------|----------------------|-------------|-----------------|-------|------|------|--------|-------|-------|-------|---------|---------|---------|
| Artificial Neural Network  | 0.555             | 0.71     | 0.819    | 0.915                | 0.173       | 0.743           | 140.5 | 10.5 | 50.0 | 13.0   | 0.45  | 1.137 | 0.479 | 0.596   | 0.784   | 0.786   |
| Category Gradient Boosting | 0.5               | 0.719    | 0.837    | 1.0                  | 0.0         | 0.72            | 153.0 | 0.0  | 60.0 | 0.0    | 0.0   | 1.0   | 0.0   | 0.633   | 0.804   | 0.807   |
| Decision Tree              | 0.568             | 0.567    | 0.657    | 0.567                | 0.542       | 0.769           | 87.0  | 32.5 | 27.5 | 66.5   | 0.335 | 1.329 | 0.785 | 0.571   | 0.765   | 0.764   |
| Elastic Net                | 0.612             | 0.607    | 0.69     | 0.606                | 0.625       | 0.799           | 93.0  | 37.5 | 22.5 | 60.5   | 0.381 | 1.56  | 0.643 | 0.639   | 0.807   | 0.808   |
| ExSTraCS                   | 0.563             | 0.628    | 0.729    | 0.704                | 0.425       | 0.76            | 108.0 | 25.5 | 34.5 | 45.5   | 0.371 | 1.257 | 0.67  | 0.614   | 0.784   | 0.787   |
| Extreme Gradient Boosting  | 0.57              | 0.591    | 0.681    | 0.621                | 0.525       | 0.766           | 95.0  | 31.5 | 28.5 | 58.0   | 0.353 | 1.273 | 0.719 | 0.619   | 0.801   | 0.801   |
| Genetic Programming        | 0.5               | 0.718    | 0.836    | 1.0                  | 0.0         | 0.719           | 153.0 | 0.0  | 60.0 | 0.0    | 0.0   | 1.0   | 0.0   | 0.5     | 0.859   | 0.72    |
| Gradient Boosting          | 0.544             | 0.687    | 0.796    | 0.854                | 0.217       | 0.738           | 131.5 | 13.0 | 47.0 | 22.5   | 0.396 | 1.11  | 0.602 | 0.577   | 0.778   | 0.777   |
| K-Nearest Neighbors        | 0.521             | 0.656    | 0.78     | 0.85                 | 0.217       | 0.726           | 130.5 | 13.0 | 47.0 | 23.0   | 0.342 | 1.053 | 0.759 | 0.54    | 0.762   | 0.739   |
| Light Gradient Boosting    | 0.609             | 0.61     | 0.691    | 0.607                | 0.578       | 0.794           | 93.5  | 35.0 | 25.5 | 60.5   | 0.379 | 1.52  | 0.637 | 0.627   | 0.813   | 0.815   |
| Logistic Regression        | 0.587             | 0.588    | 0.673    | 0.588                | 0.575       | 0.783           | 90.0  | 34.5 | 25.5 | 63.0</ |       |       |       |         |         |         |

# Median Model Prediction Statistics (Rounded to 3 Decimal Points): Page 4

## D16 = P\_GE5\_DEMDX

| ML Algorithm               | Balanced Accuracy | Accuracy | F1 Score | Sensitivity (Recall) | Specificity | Precision (PPV) | TP    | TN   | FP   | FN   | NPV   | LR+   | LR-   | ROC AUC | PRC AUC | PRC APS |
|----------------------------|-------------------|----------|----------|----------------------|-------------|-----------------|-------|------|------|------|-------|-------|-------|---------|---------|---------|
| Artificial Neural Network  | 0.652             | 0.796    | 0.875    | 0.934                | 0.389       | 0.82            | 127.5 | 17.5 | 27.5 | 9.0  | 0.673 | 1.499 | 0.16  | 0.762   | 0.884   | 0.885   |
| Category Gradient Boosting | 0.637             | 0.785    | 0.87     | 0.941                | 0.333       | 0.811           | 128.0 | 15.0 | 30.0 | 8.0  | 0.667 | 1.419 | 0.165 | 0.745   | 0.89    | 0.891   |
| Decision Tree              | 0.664             | 0.666    | 0.752    | 0.658                | 0.644       | 0.853           | 89.5  | 29.0 | 16.0 | 46.5 | 0.394 | 1.926 | 0.509 | 0.73    | 0.866   | 0.86    |
| Elastic Net                | 0.674             | 0.677    | 0.764    | 0.696                | 0.667       | 0.864           | 95.0  | 30.0 | 15.0 | 41.5 | 0.404 | 2.095 | 0.486 | 0.757   | 0.879   | 0.879   |
| ExSTraCS                   | 0.684             | 0.754    | 0.831    | 0.82                 | 0.556       | 0.846           | 111.5 | 25.0 | 20.0 | 24.5 | 0.504 | 1.814 | 0.325 | 0.754   | 0.883   | 0.883   |
| Extreme Gradient Boosting  | 0.666             | 0.696    | 0.78     | 0.739                | 0.6         | 0.847           | 100.5 | 27.0 | 18.0 | 35.5 | 0.418 | 1.832 | 0.459 | 0.741   | 0.872   | 0.874   |
| Genetic Programming        | 0.58              | 0.76     | 0.859    | 0.949                | 0.2         | 0.784           | 129.0 | 9.0  | 36.0 | 7.0  | 0.567 | 1.2   | 0.226 | 0.67    | 0.858   | 0.841   |
| Gradient Boosting          | 0.632             | 0.779    | 0.862    | 0.919                | 0.344       | 0.81            | 125.0 | 15.5 | 29.5 | 11.0 | 0.588 | 1.415 | 0.233 | 0.743   | 0.871   | 0.872   |
| K-Nearest Neighbors        | 0.623             | 0.746    | 0.837    | 0.857                | 0.4         | 0.81            | 116.5 | 18.0 | 27.0 | 19.5 | 0.488 | 1.41  | 0.348 | 0.705   | 0.873   | 0.842   |
| Light Gradient Boosting    | 0.686             | 0.713    | 0.794    | 0.74                 | 0.633       | 0.861           | 101.0 | 28.5 | 16.5 | 35.5 | 0.446 | 2.047 | 0.41  | 0.75    | 0.888   | 0.888   |
| Logistic Regression        | 0.667             | 0.676    | 0.761    | 0.684                | 0.667       | 0.859           | 93.0  | 30.0 | 15.0 | 43.0 | 0.4   | 2.006 | 0.492 | 0.76    | 0.879   | 0.88    |
| Naive Bayes                | 0.629             | 0.74     | 0.83     | 0.846                | 0.4         | 0.814           | 115.0 | 18.0 | 27.0 | 21.0 | 0.481 | 1.446 | 0.358 | 0.695   | 0.851   | 0.853   |
| Random Forest              | 0.671             | 0.728    | 0.811    | 0.779                | 0.6         | 0.849           | 106.0 | 27.0 | 18.0 | 30.0 | 0.462 | 1.859 | 0.384 | 0.753   | 0.887   | 0.888   |
| Support Vector Machine     | 0.688             | 0.71     | 0.79     | 0.733                | 0.633       | 0.862           | 100.0 | 28.5 | 16.5 | 36.5 | 0.443 | 2.06  | 0.415 | 0.756   | 0.883   | 0.884   |

## D17 = Q\_GE5\_DEMDXSYM

| ML Algorithm               | Balanced Accuracy | Accuracy | F1 Score | Sensitivity (Recall) | Specificity | Precision (PPV) | TP    | TN   | FP   | FN   | NPV   | LR+   | LR-   | ROC AUC | PRC AUC | PRC APS |
|----------------------------|-------------------|----------|----------|----------------------|-------------|-----------------|-------|------|------|------|-------|-------|-------|---------|---------|---------|
| Artificial Neural Network  | 0.649             | 0.802    | 0.878    | 0.942                | 0.374       | 0.817           | 130.0 | 17.0 | 28.5 | 8.0  | 0.681 | 1.468 | 0.152 | 0.744   | 0.886   | 0.887   |
| Category Gradient Boosting | 0.652             | 0.793    | 0.872    | 0.935                | 0.351       | 0.817           | 129.0 | 16.0 | 29.5 | 9.0  | 0.642 | 1.47  | 0.183 | 0.756   | 0.887   | 0.888   |
| Decision Tree              | 0.645             | 0.66     | 0.744    | 0.663                | 0.641       | 0.846           | 91.5  | 29.5 | 16.5 | 46.5 | 0.382 | 1.833 | 0.532 | 0.716   | 0.863   | 0.858   |
| Elastic Net                | 0.68              | 0.701    | 0.781    | 0.717                | 0.656       | 0.863           | 99.0  | 29.5 | 15.5 | 39.0 | 0.435 | 2.035 | 0.432 | 0.762   | 0.894   | 0.895   |
| ExSTraCS                   | 0.696             | 0.755    | 0.833    | 0.805                | 0.554       | 0.849           | 111.5 | 25.5 | 20.5 | 27.0 | 0.504 | 1.891 | 0.325 | 0.754   | 0.886   | 0.886   |
| Extreme Gradient Boosting  | 0.674             | 0.728    | 0.81     | 0.765                | 0.589       | 0.851           | 106.0 | 26.5 | 18.5 | 32.5 | 0.462 | 1.846 | 0.382 | 0.736   | 0.884   | 0.885   |
| Genetic Programming        | 0.605             | 0.766    | 0.859    | 0.931                | 0.264       | 0.794           | 128.5 | 12.0 | 33.5 | 9.5  | 0.559 | 1.284 | 0.213 | 0.69    | 0.863   | 0.864   |
| Gradient Boosting          | 0.647             | 0.791    | 0.869    | 0.92                 | 0.363       | 0.816           | 127.0 | 16.5 | 29.0 | 11.0 | 0.618 | 1.453 | 0.203 | 0.751   | 0.883   | 0.884   |
| K-Nearest Neighbors        | 0.655             | 0.755    | 0.843    | 0.862                | 0.45        | 0.828           | 119.0 | 20.5 | 25.0 | 19.0 | 0.506 | 1.584 | 0.32  | 0.708   | 0.881   | 0.844   |
| Light Gradient Boosting    | 0.671             | 0.717    | 0.8      | 0.747                | 0.616       | 0.852           | 103.5 | 28.0 | 17.5 | 35.0 | 0.446 | 1.894 | 0.414 | 0.747   | 0.882   | 0.883   |
| Logistic Regression        | 0.68              | 0.707    | 0.783    | 0.718                | 0.656       | 0.863           | 99.5  | 29.5 | 15.5 | 39.0 | 0.435 | 2.037 | 0.426 | 0.759   | 0.894   | 0.895   |
| Naive Bayes                | 0.647             | 0.682    | 0.772    | 0.729                | 0.583       | 0.835           | 101.0 | 26.5 | 19.0 | 37.5 | 0.412 | 1.684 | 0.469 | 0.713   | 0.864   | 0.865   |
| Random Forest              | 0.676             | 0.747    | 0.826    | 0.798                | 0.578       | 0.85            | 110.5 | 26.0 | 19.0 | 28.0 | 0.489 | 1.838 | 0.343 | 0.75    | 0.886   | 0.887   |
| Support Vector Machine     | 0.695             | 0.717    | 0.794    | 0.736                | 0.667       | 0.87            | 102.0 | 30.0 | 15.0 | 36.5 | 0.457 | 2.177 | 0.396 | 0.747   | 0.883   | 0.885   |

## D18 = R\_GE5\_DEMDXSYMCF

| ML Algorithm               | Balanced Accuracy | Accuracy | F1 Score | Sensitivity (Recall) | Specificity | Precision (PPV) | TP    | TN   | FP   | FN   | NPV   | LR+   | LR-   | ROC AUC | PRC AUC | PRC APS |
|----------------------------|-------------------|----------|----------|----------------------|-------------|-----------------|-------|------|------|------|-------|-------|-------|---------|---------|---------|
| Artificial Neural Network  | 0.681             | 0.782    | 0.858    | 0.911                | 0.454       | 0.813           | 144.0 | 27.5 | 33.0 | 14.0 | 0.656 | 1.666 | 0.201 | 0.778   | 0.885   | 0.886   |
| Category Gradient Boosting | 0.649             | 0.789    | 0.869    | 0.962                | 0.344       | 0.791           | 152.0 | 21.0 | 40.0 | 6.0  | 0.76  | 1.45  | 0.122 | 0.787   | 0.888   | 0.888   |
| Decision Tree              | 0.678             | 0.686    | 0.766    | 0.726                | 0.645       | 0.843           | 114.0 | 39.0 | 21.5 | 43.0 | 0.454 | 2.077 | 0.467 | 0.738   | 0.866   | 0.86    |
| Elastic Net                | 0.719             | 0.72     | 0.788    | 0.721                | 0.705       | 0.863           | 113.5 | 43.0 | 18.0 | 44.0 | 0.494 | 2.439 | 0.391 | 0.781   | 0.892   | 0.89    |
| ExSTraCS                   | 0.719             | 0.754    | 0.829    | 0.806                | 0.648       | 0.853           | 126.5 | 39.5 | 21.5 | 30.5 | 0.553 | 2.26  | 0.308 | 0.79    | 0.888   | 0.889   |
| Extreme Gradient Boosting  | 0.702             | 0.748    | 0.819    | 0.796                | 0.603       | 0.838           | 125.0 | 36.5 | 24.0 | 32.0 | 0.541 | 2.017 | 0.328 | 0.793   | 0.895   | 0.896   |
| Genetic Programming        | 0.621             | 0.755    | 0.843    | 0.911                | 0.306       | 0.778           | 143.5 | 18.5 | 42.0 | 14.0 | 0.607 | 1.349 | 0.252 | 0.727   | 0.85    | 0.85    |
| Gradient Boosting          | 0.667             | 0.782    | 0.86     | 0.927                | 0.422       | 0.803           | 146.0 | 25.5 | 35.0 | 11.5 | 0.685 | 1.582 | 0.177 | 0.786   | 0.888   | 0.887   |
| K-Nearest Neighbors        | 0.659             | 0.743    | 0.824    | 0.844                | 0.475       | 0.805           | 133.0 | 29.0 | 32.0 | 24.5 | 0.544 | 1.585 | 0.326 | 0.756   | 0.868   | 0.86    |
| Light Gradient Boosting    | 0.694             | 0.725    | 0.799    | 0.753                | 0.623       | 0.839           | 119.0 | 38.0 | 23.0 | 39.0 | 0.5   | 2.028 | 0.381 | 0.792   | 0.887   | 0.889   |
| Logistic Regression        | 0.704             | 0.704    | 0.773    | 0.699                | 0.686       | 0.855           | 110.5 | 41.5 | 19.0 | 47.5 | 0.478 | 2.265 | 0.421 | 0.773   | 0.887   | 0.888   |
| Naive Bayes                | 0.679             | 0.67     | 0.743    | 0.666                | 0.689       | 0.848           | 104.5 | 42.0 | 19.0 | 52.5 | 0.443 | 2.153 | 0.488 | 0.74    | 0.859   | 0.86    |
| Random Forest              | 0.71              | 0.743    | 0.82     | 0.803                | 0.612       | 0.844           | 126.5 | 37.0 | 23.5 | 31.0 | 0.533 | 2.101 | 0.332 | 0.776   | 0.884   | 0.885   |
| Support Vector Machine     | 0.699             | 0.734    | 0.806    | 0.771                | 0.639       | 0.844           | 121.0 | 39.0 | 22.0 | 36.0 | 0.517 | 2.102 | 0.358 | 0.783   | 0.886   | 0.887   |

## D19 = S\_GE5\_DEMDXSYMIO

| ML Algorithm               | Balanced Accuracy | Accuracy | F1 Score | Sensitivity (Recall) | Specificity | Precision (PPV) | TP    | TN   | FP   | FN   | NPV   | LR+   | LR-   | ROC AUC | PRC AUC | PRC APS |
|----------------------------|-------------------|----------|----------|----------------------|-------------|-----------------|-------|------|------|------|-------|-------|-------|---------|---------|---------|
| Artificial Neural Network  | 0.668             | 0.776    | 0.856    | 0.911                | 0.425       | 0.804           | 143.0 | 25.5 | 34.5 | 14.0 | 0.648 | 1.568 | 0.208 | 0.765   | 0.89    | 0.89    |
| Category Gradient Boosting | 0.628             | 0.776    | 0.861    | 0.962                | 0.292       | 0.781           | 151.0 | 17.5 | 42.5 | 6.0  | 0.735 | 1.363 | 0.138 | 0.779   | 0.885   | 0.886   |
| Decision Tree              | 0.685             | 0.702    | 0.778    | 0.71                 | 0.658       | 0.839           | 111.5 | 39.5 | 20.5 | 45.5 | 0.466 | 1.995 | 0.439 | 0.742   | 0.866   | 0.858   |
| Elastic Net                | 0.694             | 0.694    | 0.762    | 0.688                | 0.667       | 0.847           | 108.0 | 40.0 | 20.0 | 49.0 | 0.465 | 2.122 | 0.439 | 0.766   | 0.885   | 0.885   |
| ExSTraCS                   | 0.709             | 0.74     | 0.812    | 0.786                | 0.625       | 0.847           | 123.0 | 37.5 | 22.5 | 33.5 | 0.524 | 2.123 | 0.347 | 0.764   | 0.879   | 0.88    |
| Extreme Gradient Boosting  | 0.687             | 0.735    | 0.812    | 0.792                | 0.6         | 0.835           | 124.0 | 36.0 | 24.0 | 32.5 | 0.52  | 1.935 | 0.353 | 0.777   | 0.883   | 0.884   |
| Genetic Programming        | 0.593             | 0.711    | 0.819    | 0.889                | 0.317       | 0.772           | 139.5 | 19.0 | 41.0 | 17.5 | 0.459 | 1.297 | 0.434 | 0.692   | 0.855   | 0.842   |
| Gradient Boosting          | 0.662             | 0.776    | 0.855    | 0.92                 | 0.425       | 0.803           | 144.5 | 25.5 | 34.5 | 12.5 | 0.662 | 1.562 | 0.195 | 0.765   | 0.884   | 0.885   |
| K-Nearest Neighbors        | 0.623             | 0.749    | 0.832    | 0.872                | 0.392       | 0.782           | 136.5 | 23.5 | 36.5 | 20.0 | 0.558 | 1.375 | 0.303 | 0.696   | 0.846   | 0.82    |
| Light Gradient Boosting    | 0.678             | 0.721    | 0.799    | 0.764                | 0.592       | 0.83            | 119.5 | 35.5 | 24.5 | 37.0 | 0.496 | 1.87  | 0.389 | 0.76    | 0.884   | 0.885   |
| Logistic Regression        | 0.701             | 0.694    | 0.765    | 0.697                | 0.683       | 0.857           | 109.5 | 41.0 | 19.0 | 47.5 | 0.465 | 2.299 | 0.441 | 0.773   | 0.892   | 0.893   |
| Naive Bayes                | 0.665             | 0.666    | 0.746    | 0.669                | 0.633       | 0.833           | 105.0 | 38.0 | 22.0 | 52.0 | 0.432 | 1.903 | 0.502 | 0.714   | 0.854   | 0.855   |
| Random Forest              | 0.695             | 0.739    | 0.819    | 0.825                | 0.592       | 0.838           | 129.5 | 35.5 | 24.5 | 27.5 | 0.53  | 1.987 | 0.34  | 0.777   | 0.886   | 0.887   |
| Support Vector Machine     | 0.702             | 0.718    | 0.787    | 0.719                | 0.683       | 0.852           | 112.5 | 41.0 | 19.0 | 44.0 | 0.494 | 2.202 | 0.393 | 0.775   | 0.892   | 0.893   |

## D20 = T\_GE5\_DEMDXSYMCFIO

| ML Algorithm               | Balanced Accuracy | Accuracy | F1 Score | Sensitivity (Recall) | Specificity | Precision (PPV) | TP    | TN   | FP   | FN   | NPV   | LR+   | LR-   | ROC AUC | PRC AUC | PRC APS |
|----------------------------|-------------------|----------|----------|----------------------|-------------|-----------------|-------|------|------|------|-------|-------|-------|---------|---------|---------|
| Artificial Neural Network  | 0.666             | 0.768    | 0.849    | 0.902                | 0.438       | 0.805           | 142.0 | 26.5 | 34.0 | 15.5 | 0.624 | 1.588 | 0.234 | 0.779   | 0.893   | 0.894   |
| Category Gradient Boosting | 0.654             | 0.794    | 0.871    | 0.965                | 0.352       | 0.791           | 152.0 | 21.5 | 39.5 | 5.5  | 0.789 | 1.468 | 0.103 | 0.789   | 0.89    | 0.89    |
| Decision Tree              | 0.679             | 0.687    | 0.761    | 0.691                | 0.645       | 0.836           | 108.5 | 39.0 | 21.5 | 48.5 | 0.458 | 1.958 | 0.456 | 0.733   | 0.871   | 0.862   |
| Elastic Net                | 0.719             | 0.725    | 0.795    | 0.733                | 0.697       | 0.864           | 115.5 | 42.5 | 18.5 | 42.0 | 0.502 | 2.464 | 0.383 | 0.787   | 0.897   | 0.897   |
| ExSTraCS                   | 0.707             | 0.748    | 0.818    | 0.803                | 0.631       | 0.848           | 126.5 | 38.5 | 22.5 | 31.0 | 0.539 | 2.168 | 0.332 | 0.787   | 0.886   | 0.887   |
| Extreme Gradient Boosting  | 0.717             | 0.75     | 0.819    | 0.79                 | 0.636       | 0.851           | 124.0 | 38.5 | 22.0 | 33.0 | 0.541 | 2.193 | 0.328 | 0.79    | 0.896   | 0.896   |
| Genetic Programming        | 0.605             | 0.745    | 0.841    | 0.93                 | 0.283       | 0.771           | 146.5 | 17.0 | 43.0 | 11.0 | 0.59  | 1.293 | 0.267 | 0.699   | 0.844   | 0.843   |
| Gradient Boosting          | 0.675             | 0.782    | 0.858    | 0.917                | 0.421       | 0.808           | 144.5 | 25.5 | 35.0 | 13.0 | 0.667 | 1.602 | 0.193 | 0.793   | 0.893   | 0.894   |
| K-Nearest Neighbors        | 0.669             | 0.764    | 0.846    | 0.867                | 0.508       | 0.812           | 136.5 | 31.0 | 30.0 | 21.0 | 0.606 | 1.682 | 0.25  | 0.764   | 0.876   | 0.868   |
| Light Gradient Boosting    | 0.707             | 0.733    | 0.807    | 0.775                | 0.628       | 0.845           | 122.0 | 38.0 | 22.5 | 35.5 | 0.517 | 2.097 | 0.36  | 0       |         |         |

# Feature Importance Summary: D1 = A\_GE15\_DEM

Sorted Median Mutual Information Scores

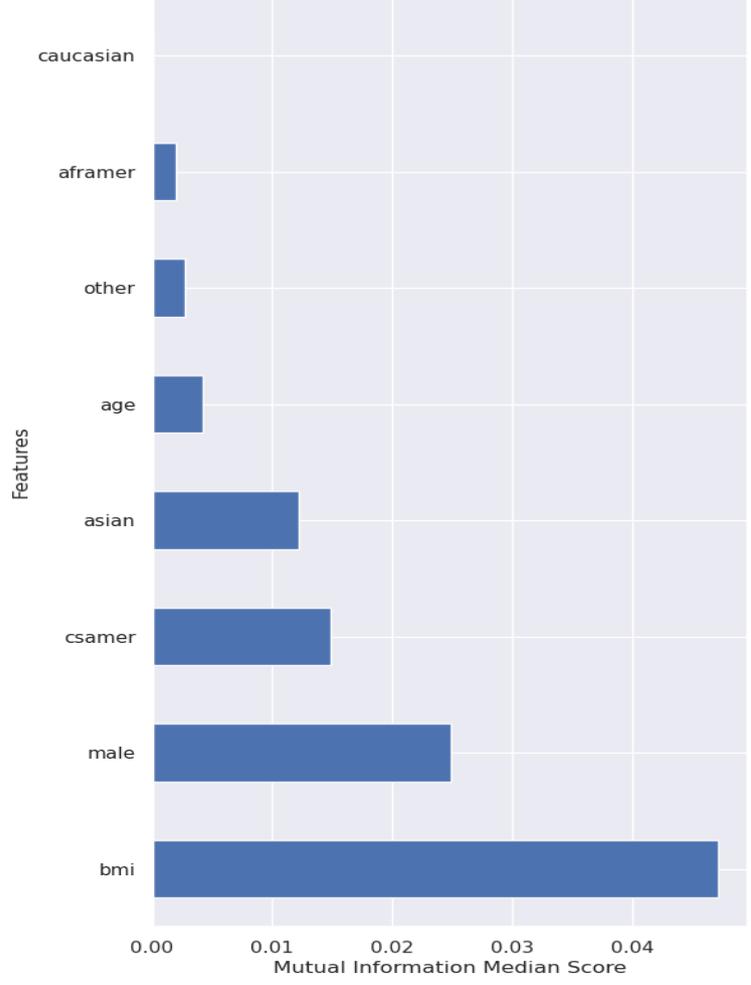

Sorted Median MultiSURF Scores

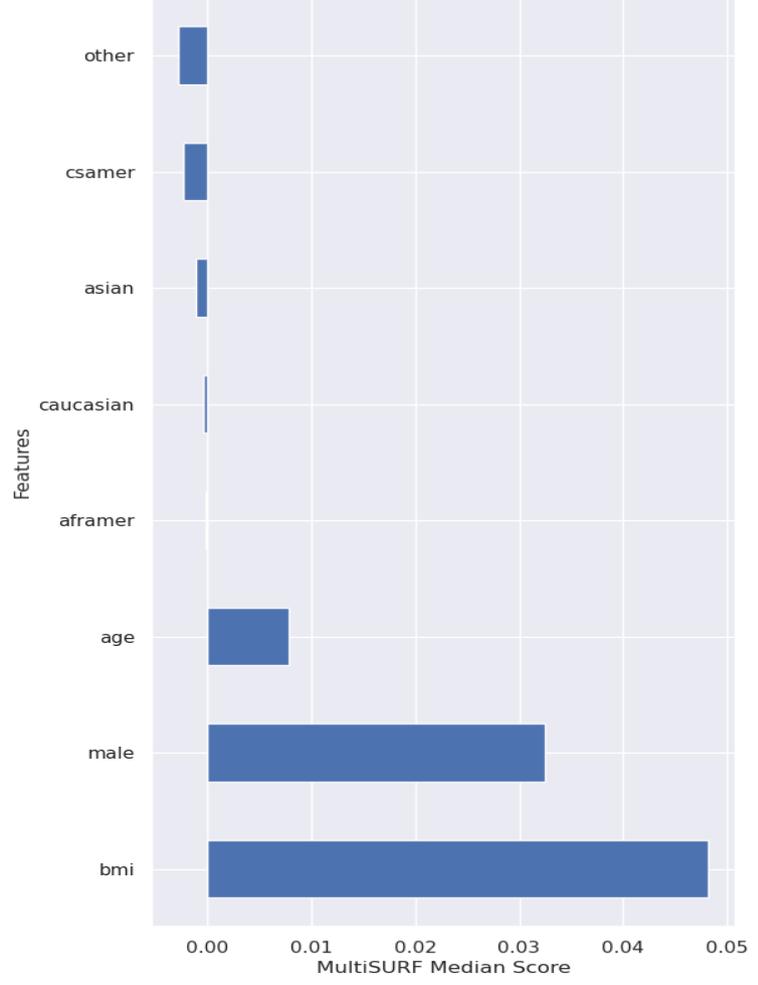

## Composite Feature Importance Plot (Normalized and Performance Weighted)

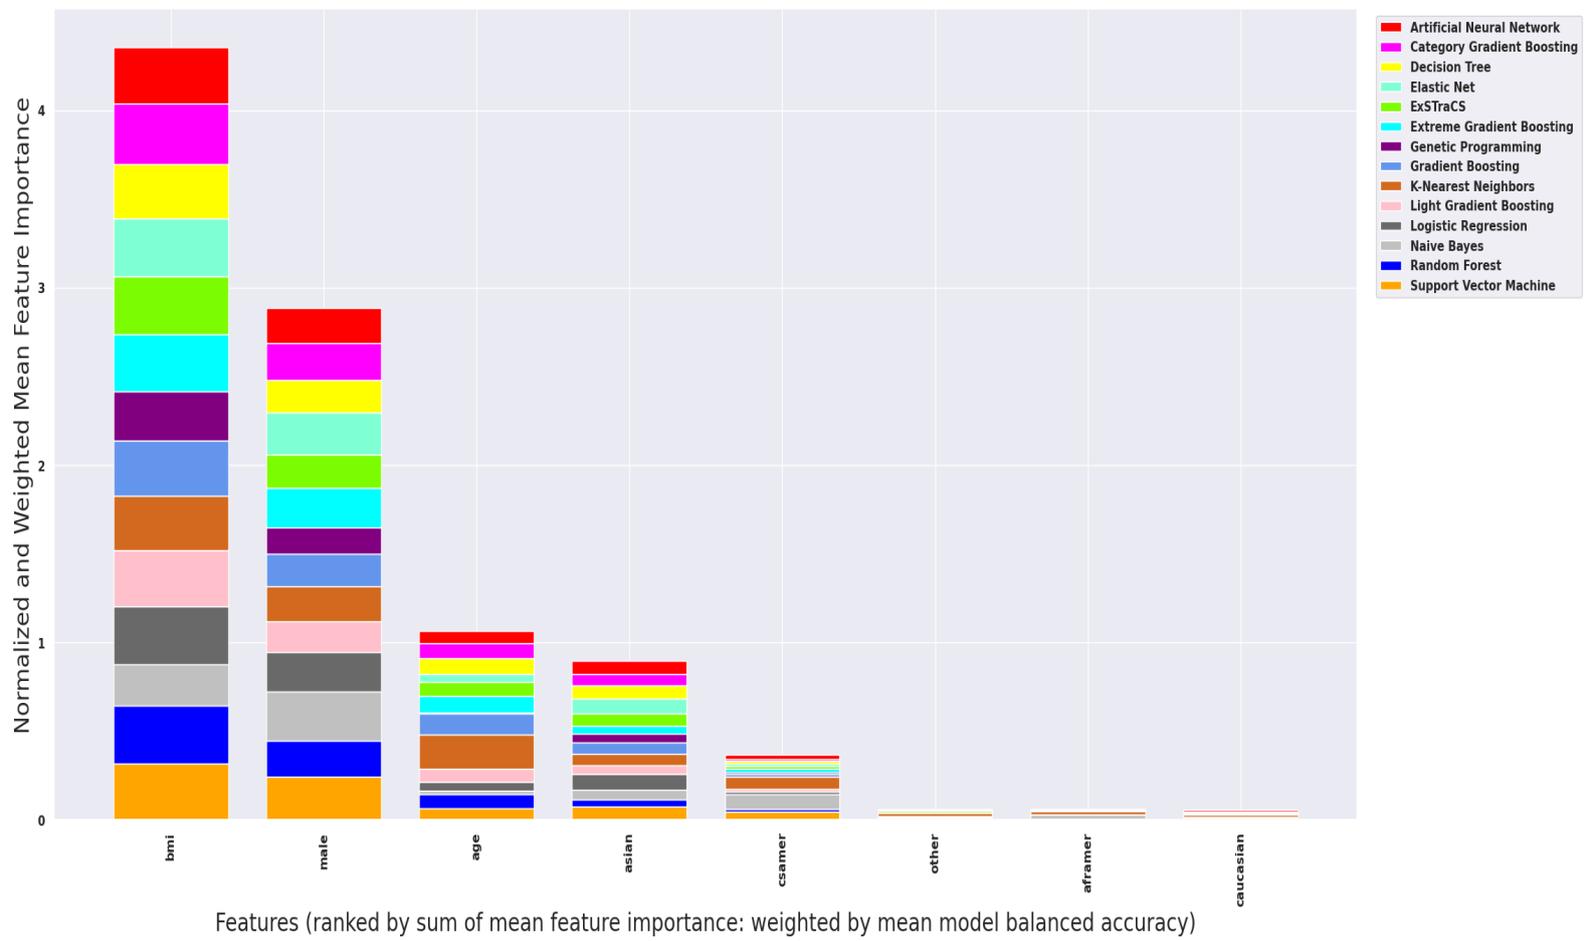

# Feature Importance Summary: D2 = B\_GE15\_DX

Sorted Median Mutual Information Scores

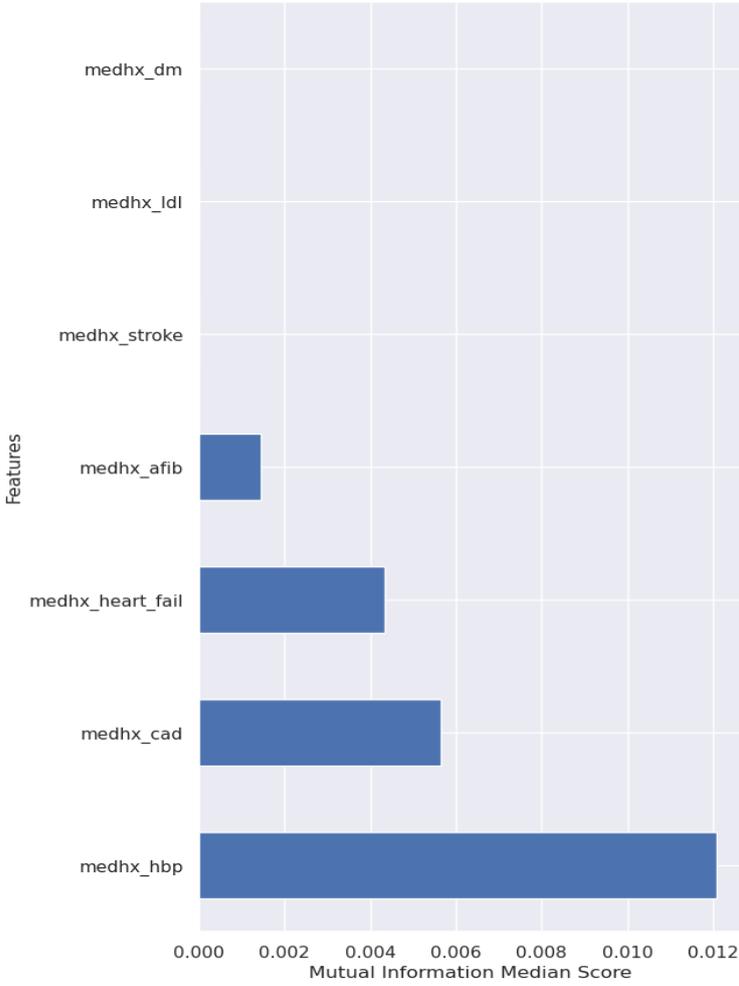

Sorted Median MultiSURF Scores

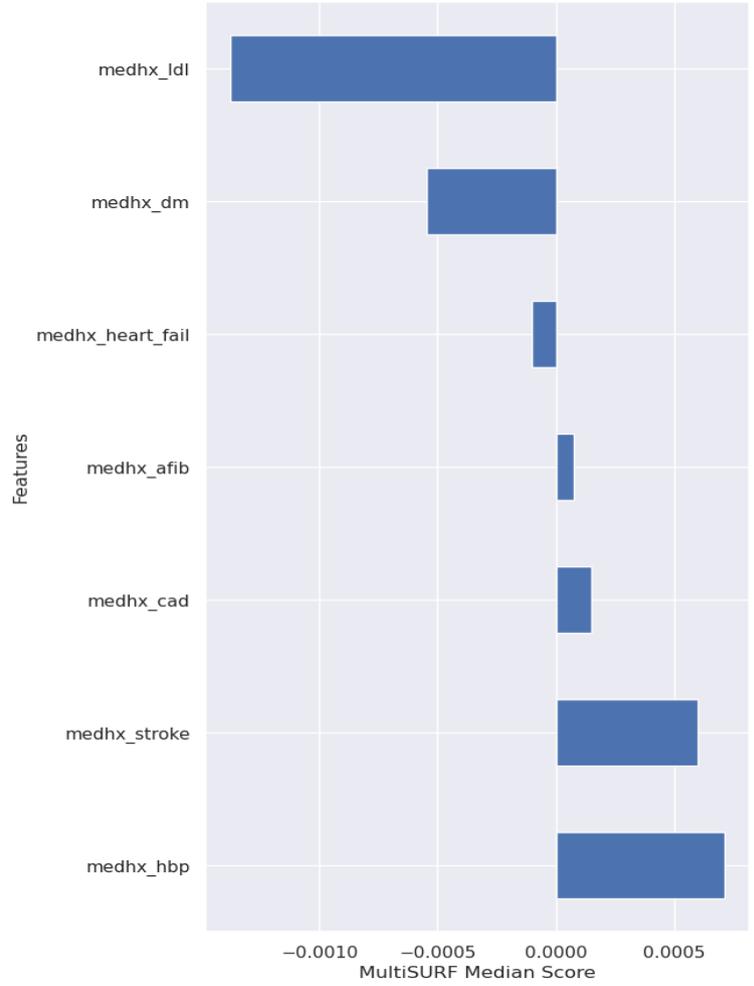

## Composite Feature Importance Plot (Normalized and Performance Weighted)

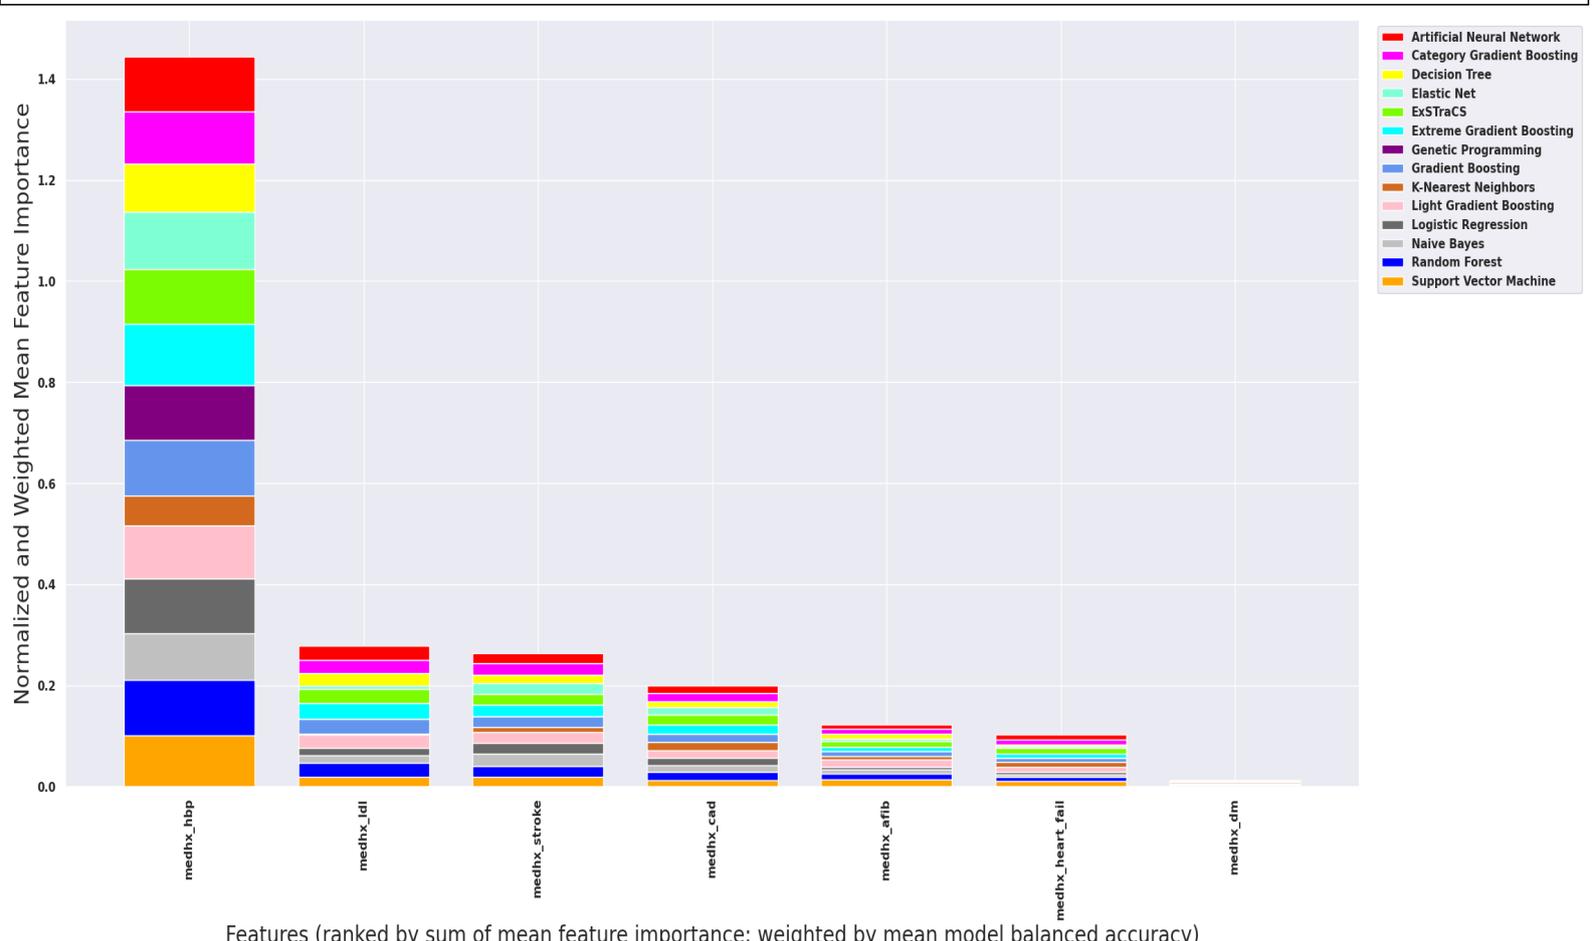

# Feature Importance Summary: D3 = C\_GE15\_SYM

Sorted Median Mutual Information Scores

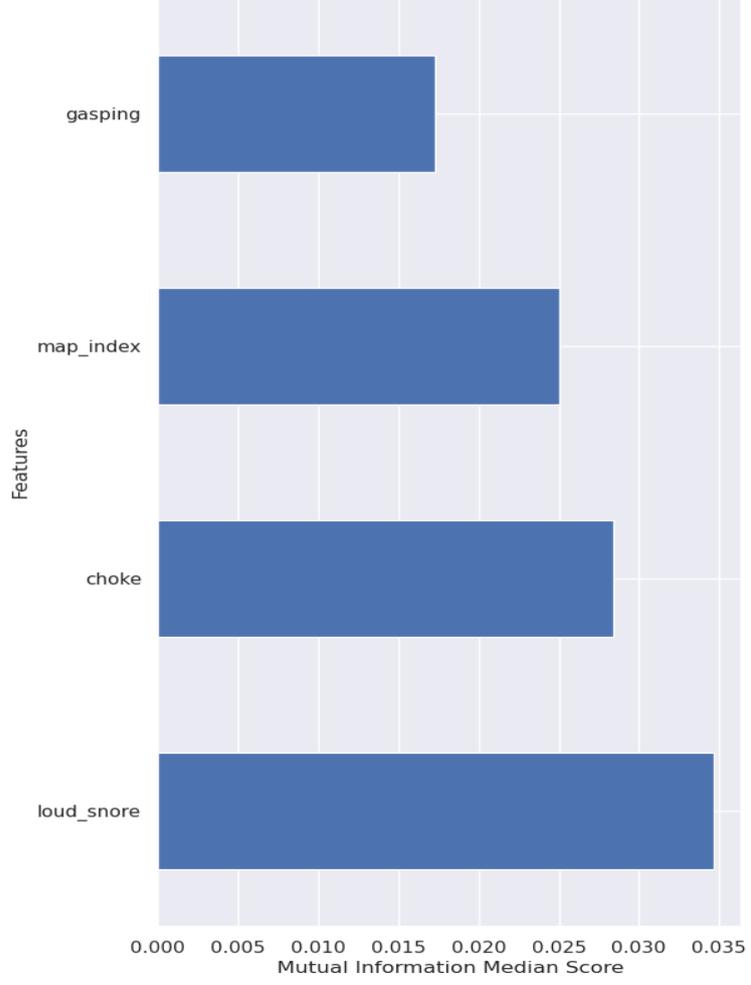

Sorted Median MultiSURF Scores

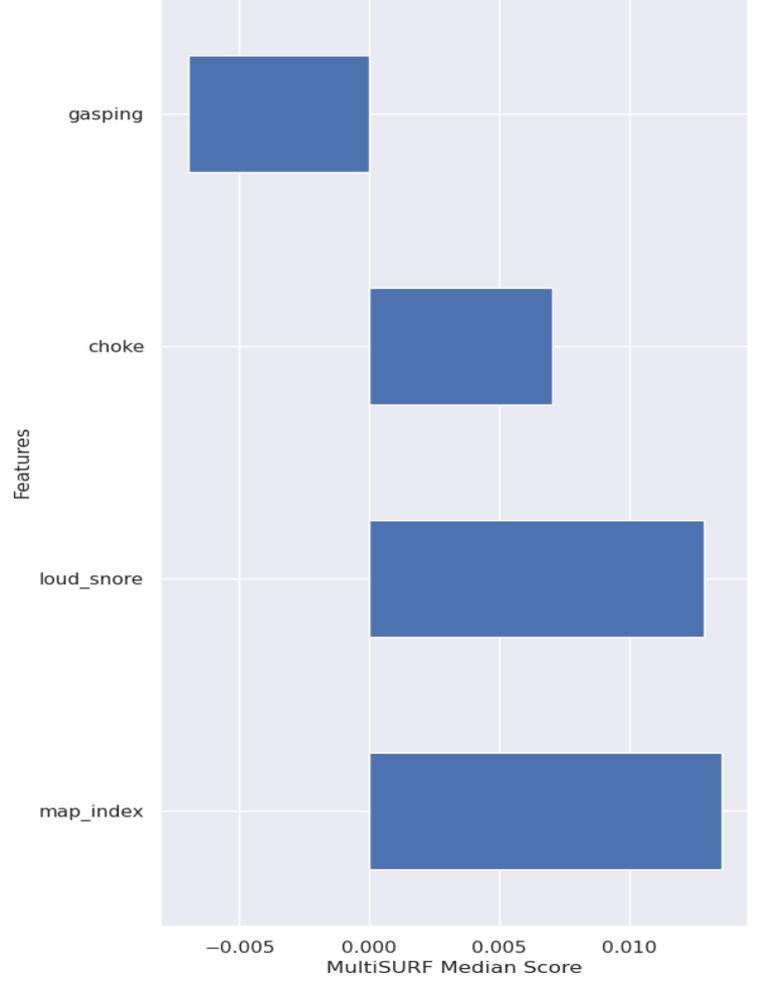

## Composite Feature Importance Plot (Normalized and Performance Weighted)

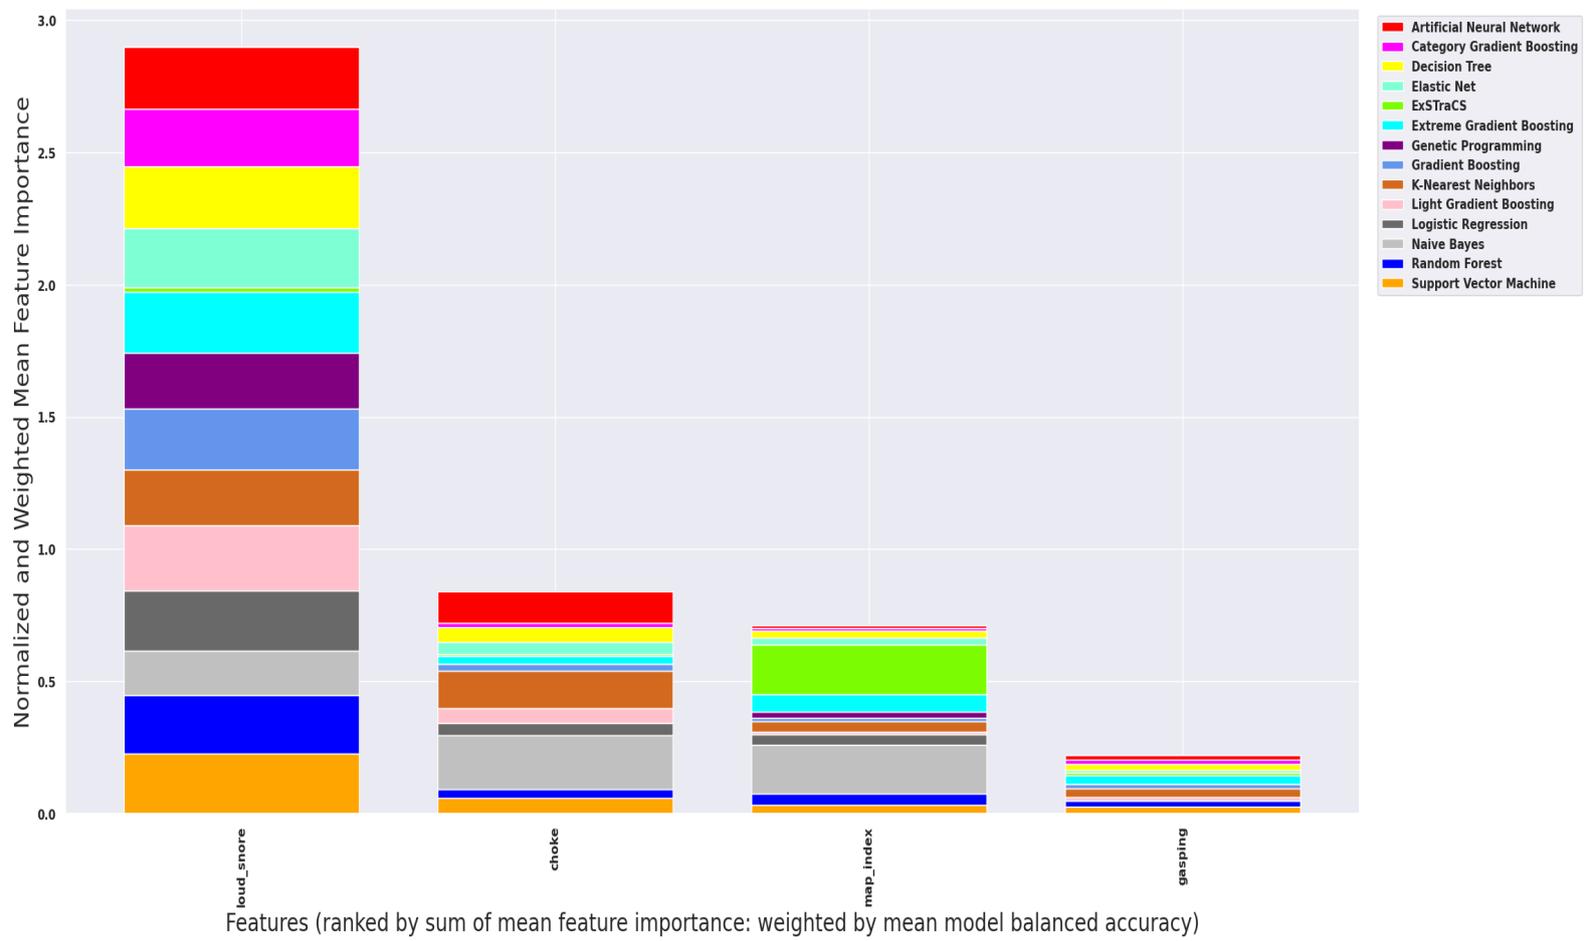

Features (ranked by sum of mean feature importance: weighted by mean model balanced accuracy)

# Feature Importance Summary: D4 = D\_GE15\_CF

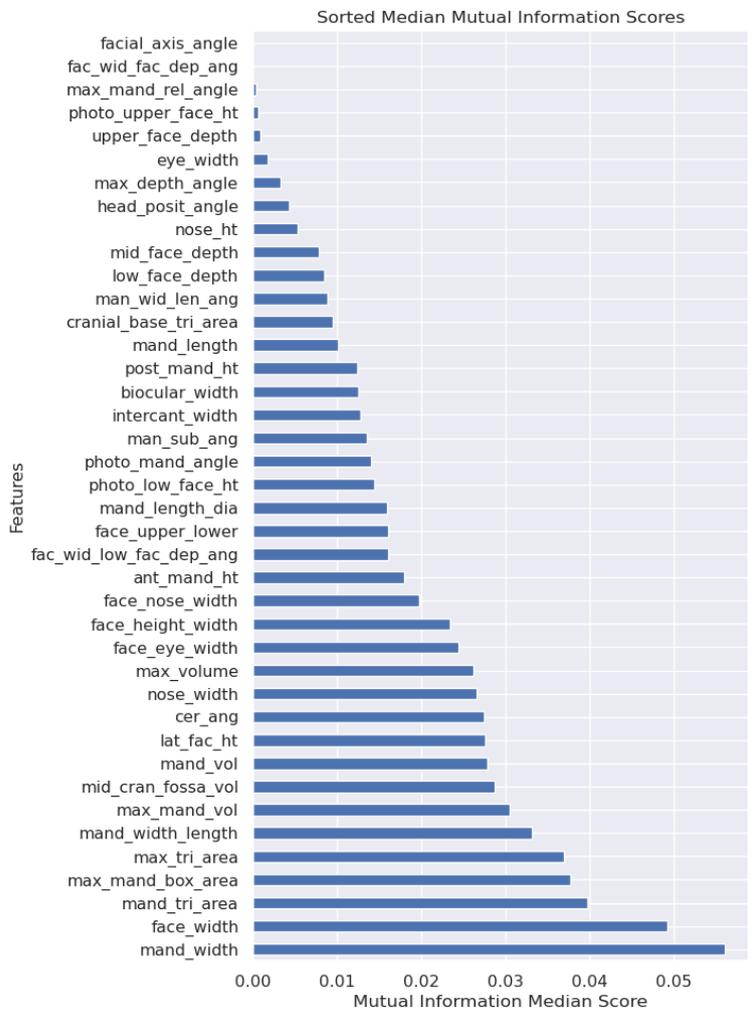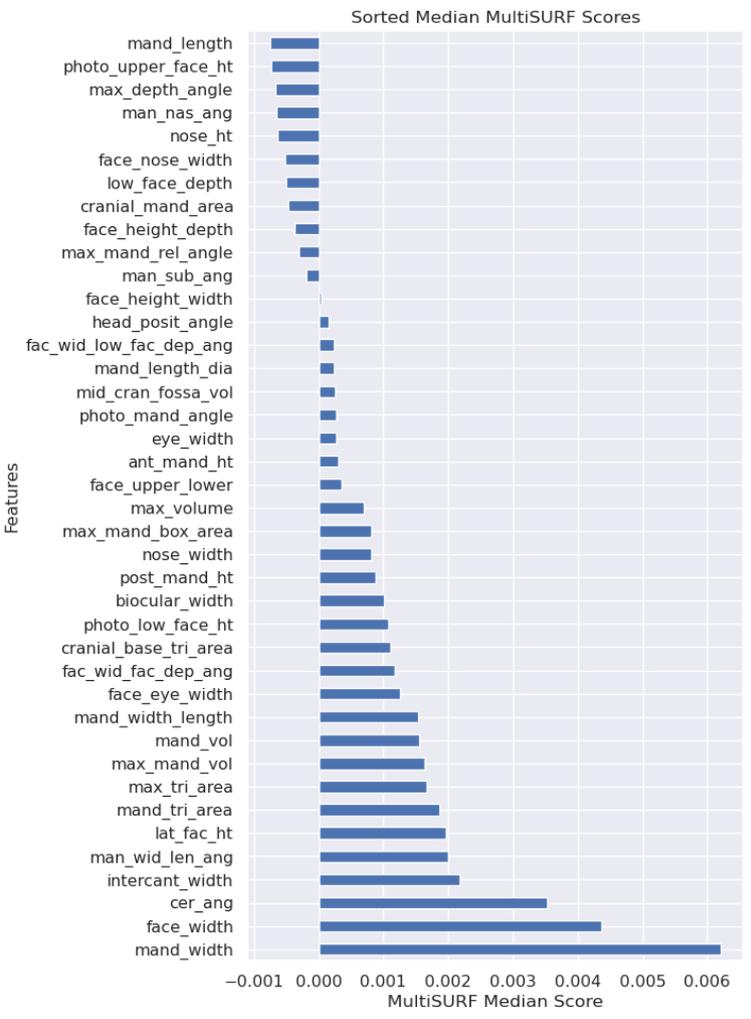

## Composite Feature Importance Plot (Normalized and Performance Weighted)

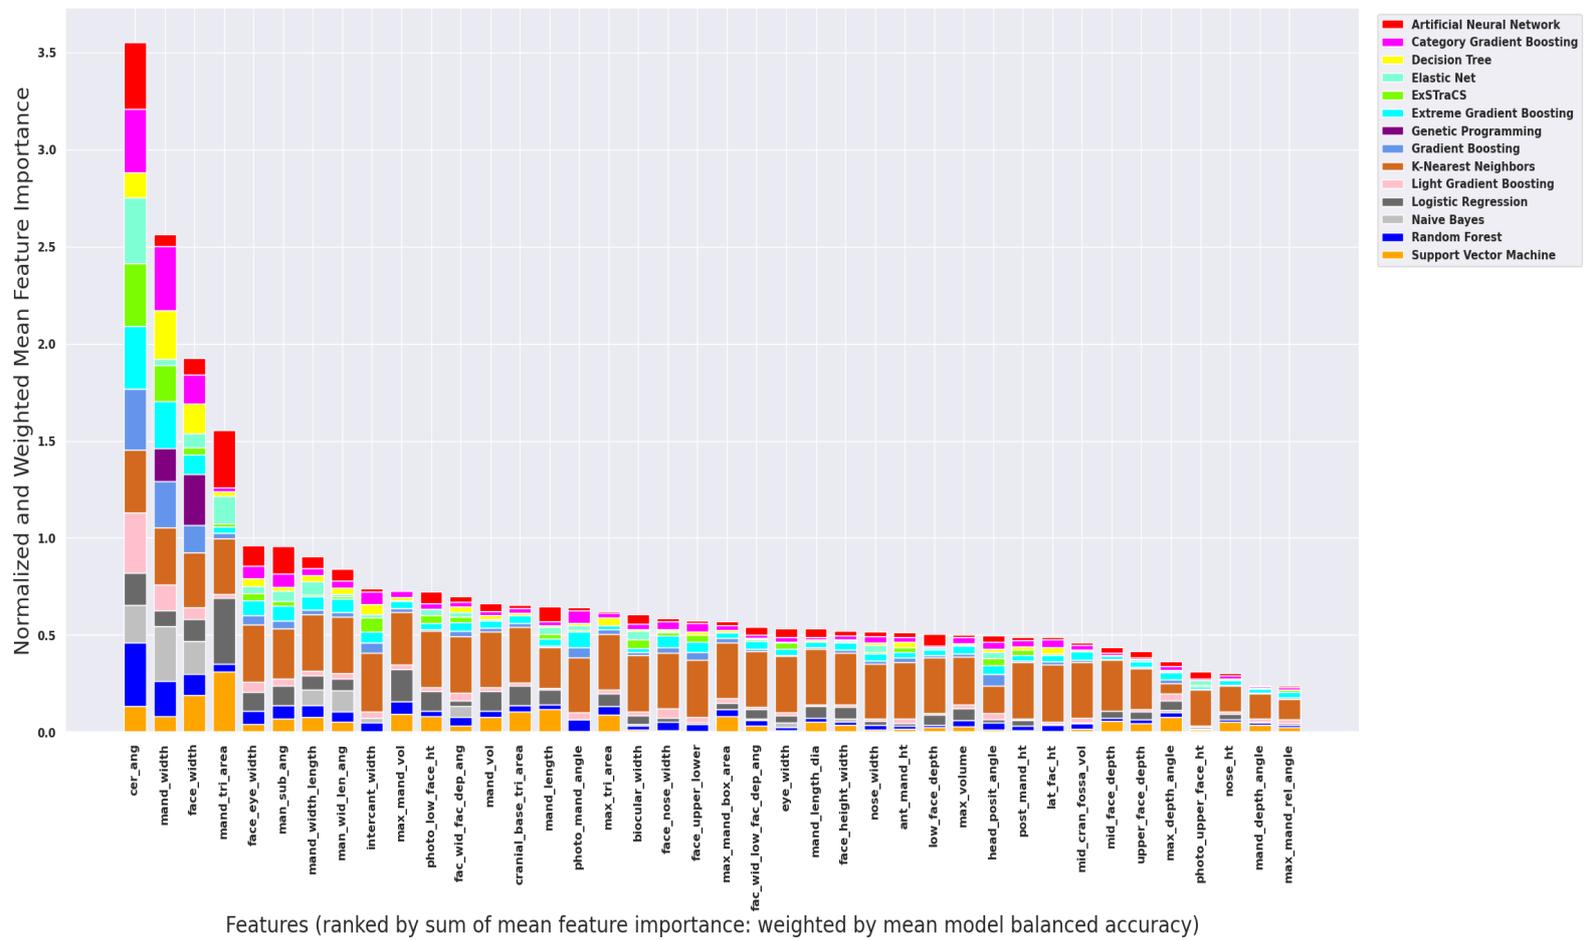

Features (ranked by sum of mean feature importance: weighted by mean model balanced accuracy)

# Feature Importance Summary: D5 = E\_GE15\_IO

Sorted Median Mutual Information Scores

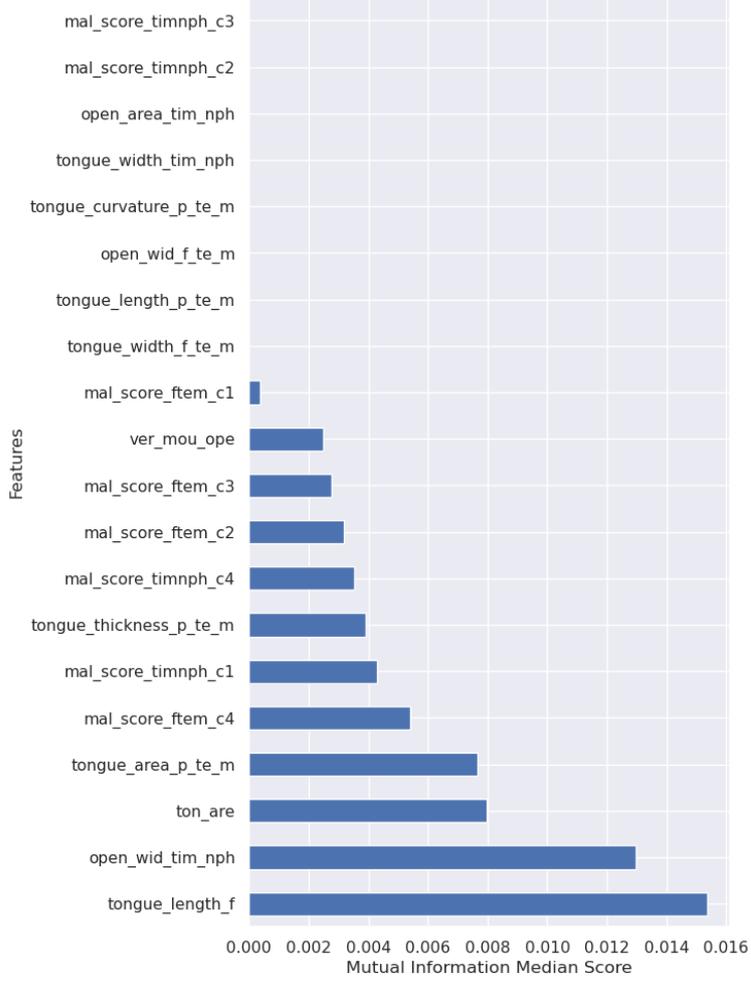

Sorted Median MultiSURF Scores

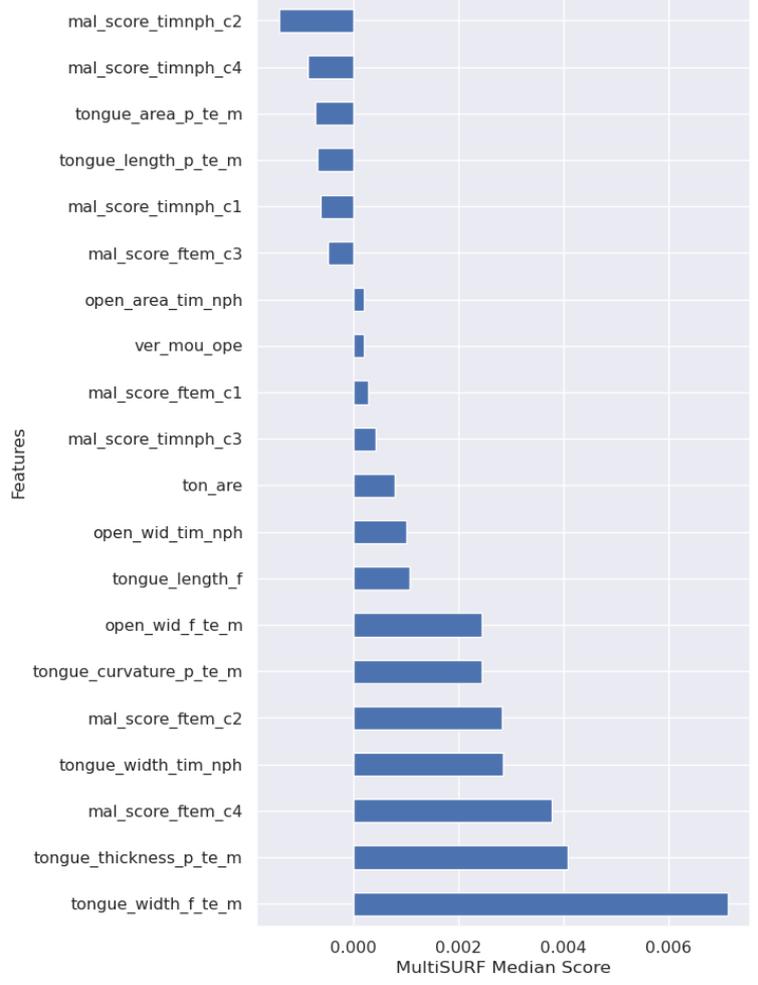

Composite Feature Importance Plot (Normalized and Performance Weighted)

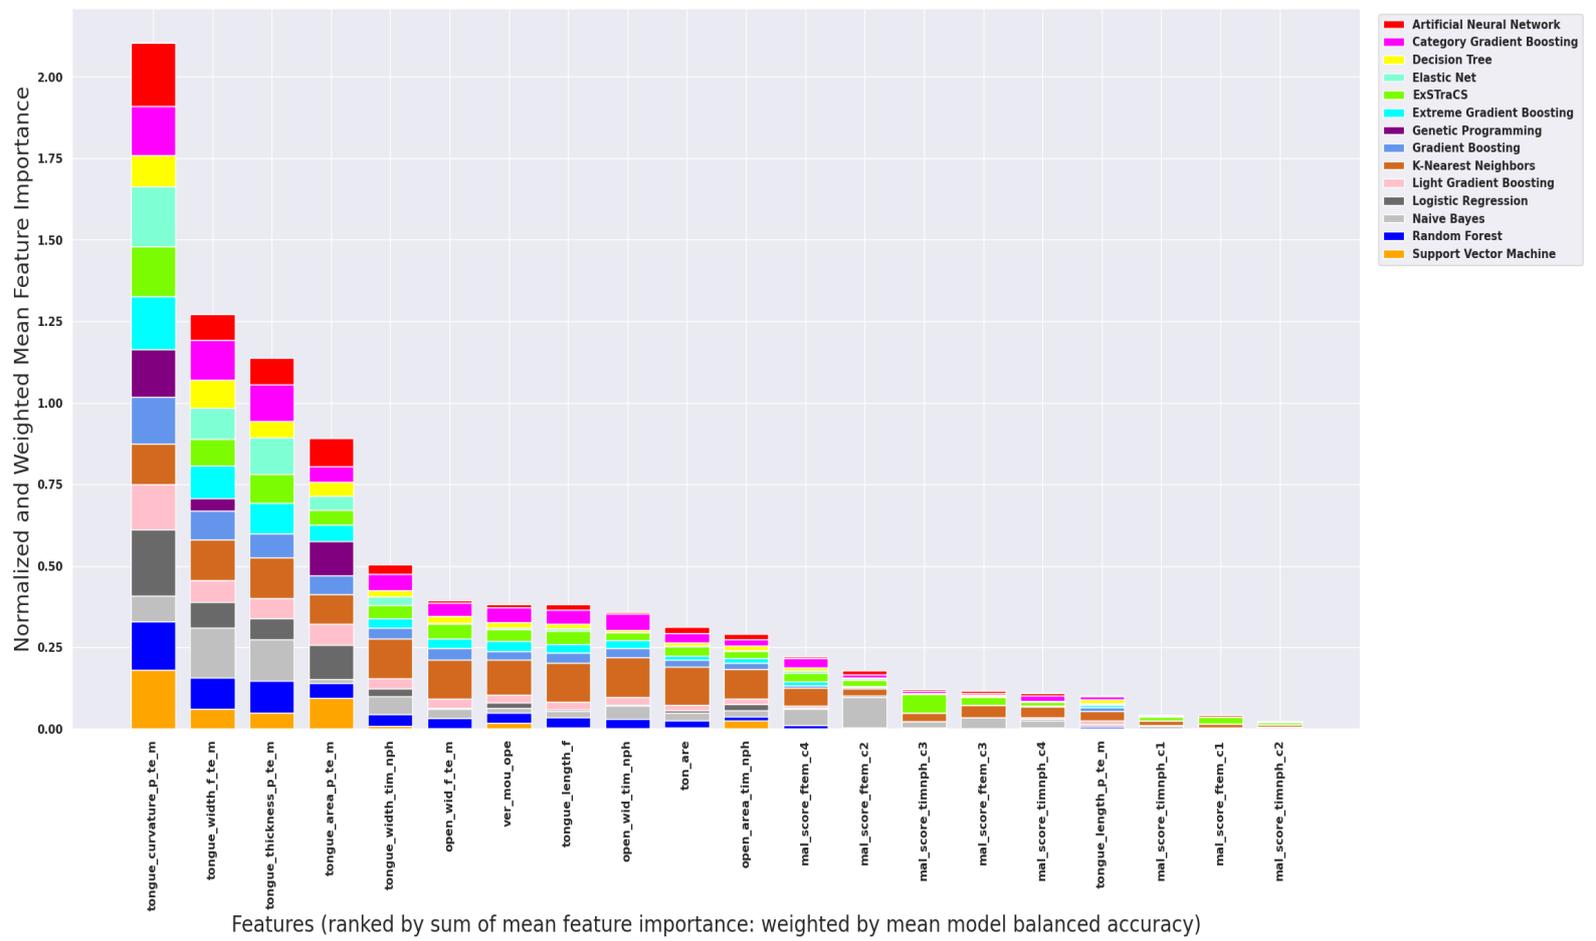

Features (ranked by sum of mean feature importance: weighted by mean model balanced accuracy)

# Feature Importance Summary: D6 = F\_GE15\_DEMDX

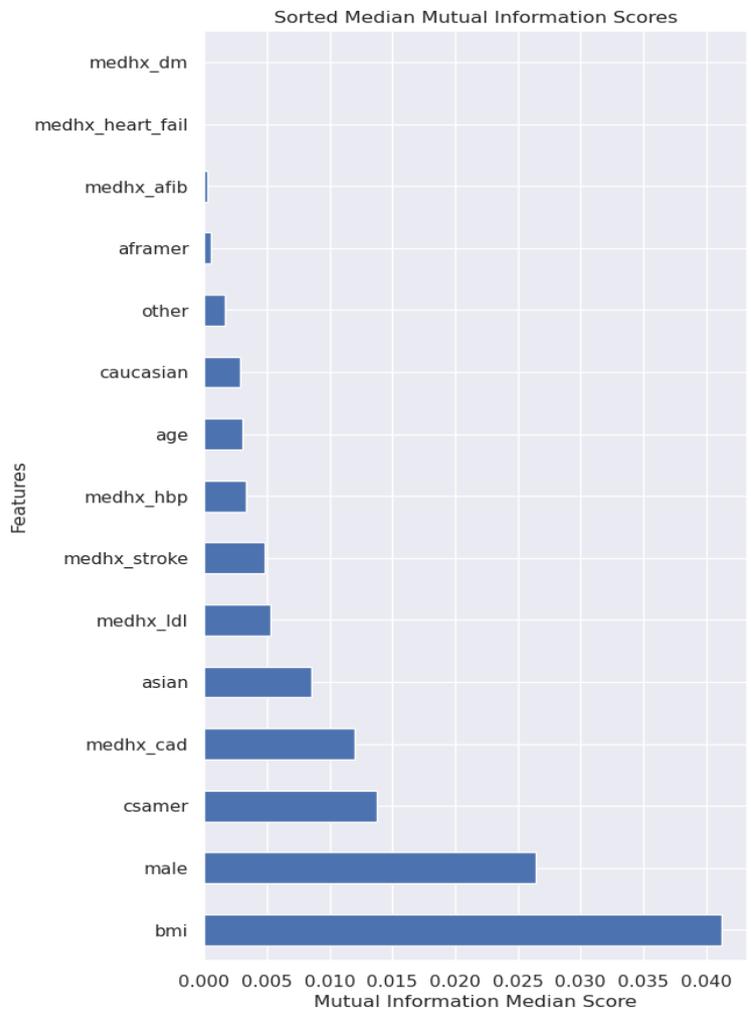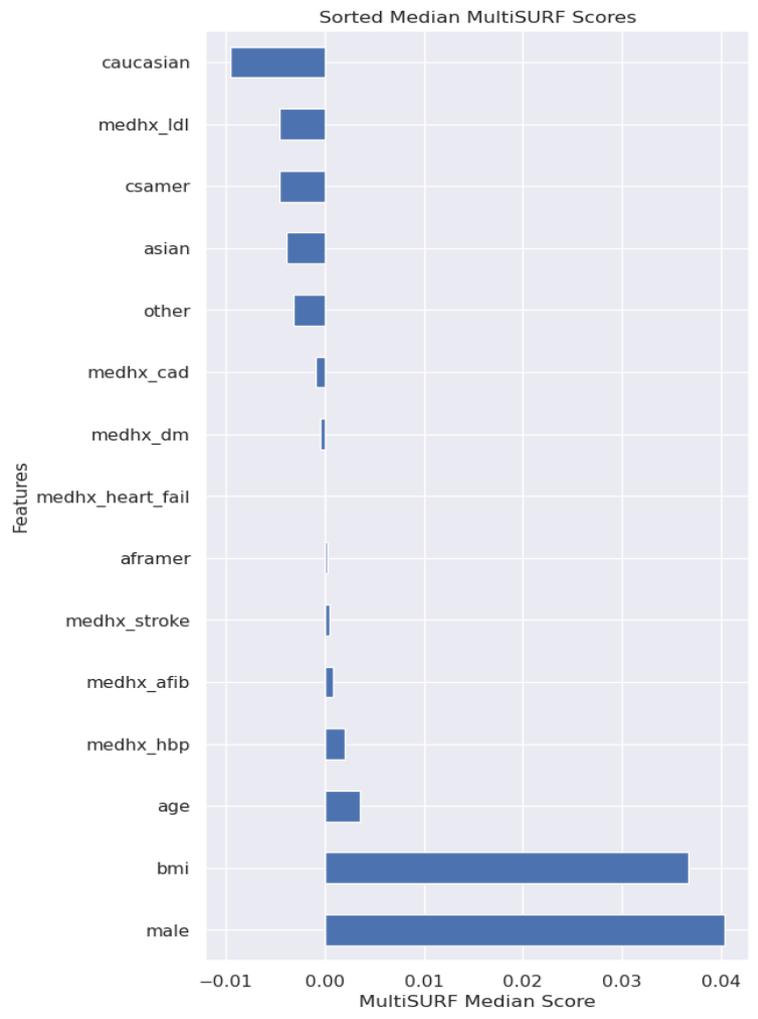

## Composite Feature Importance Plot (Normalized and Performance Weighted)

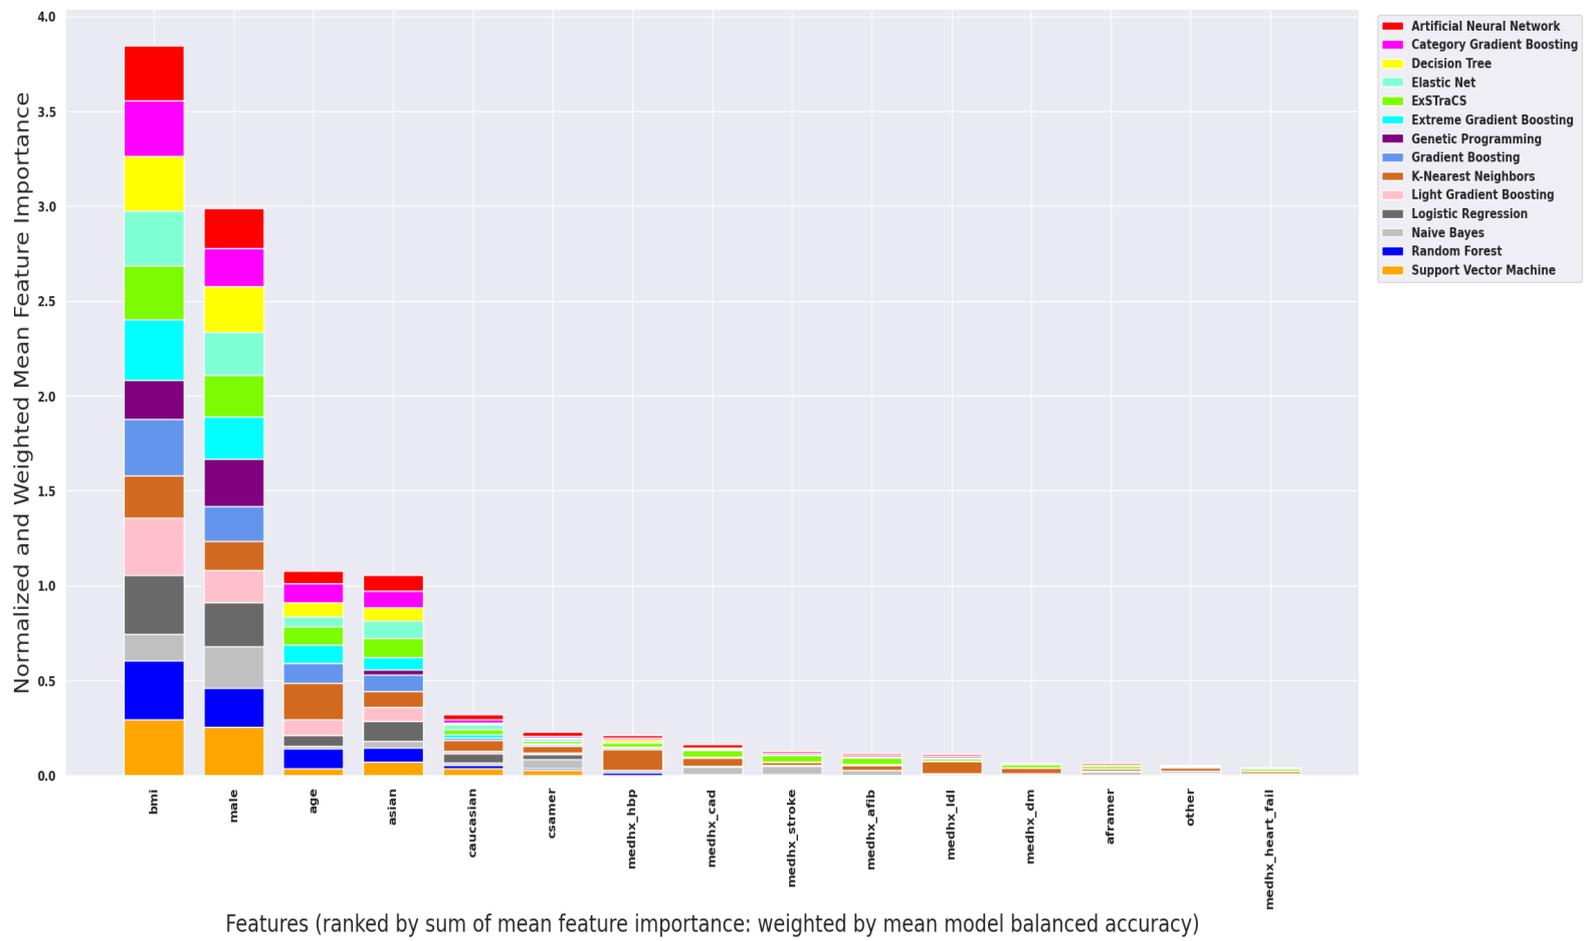

# Feature Importance Summary: D7 = G\_GE15\_DEMDXSYM

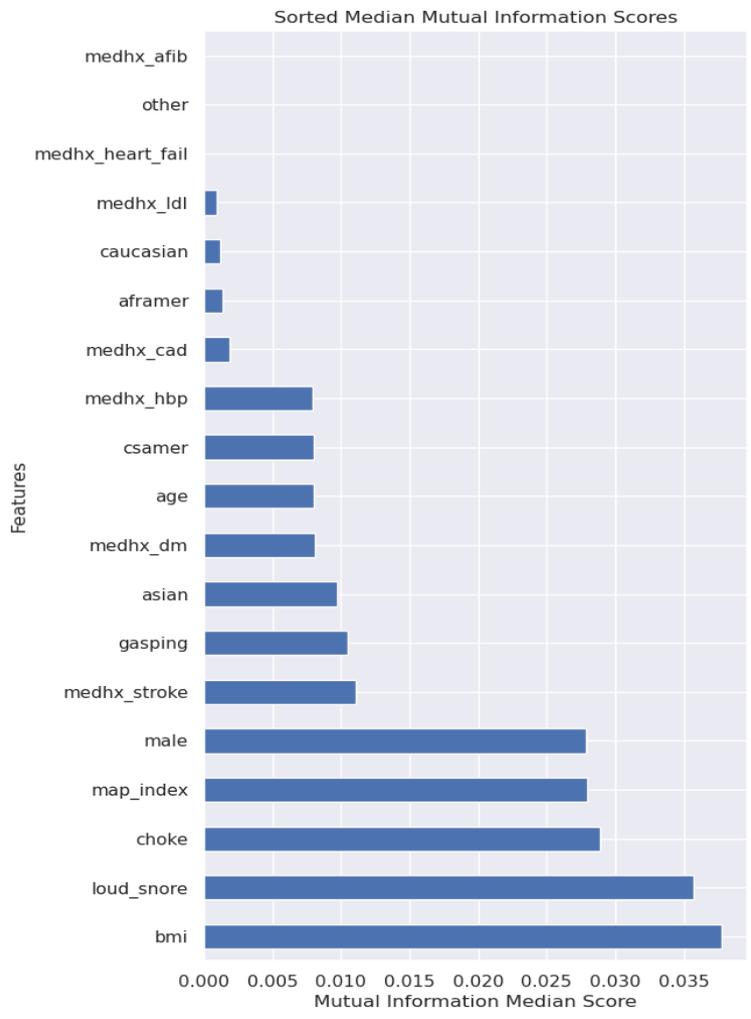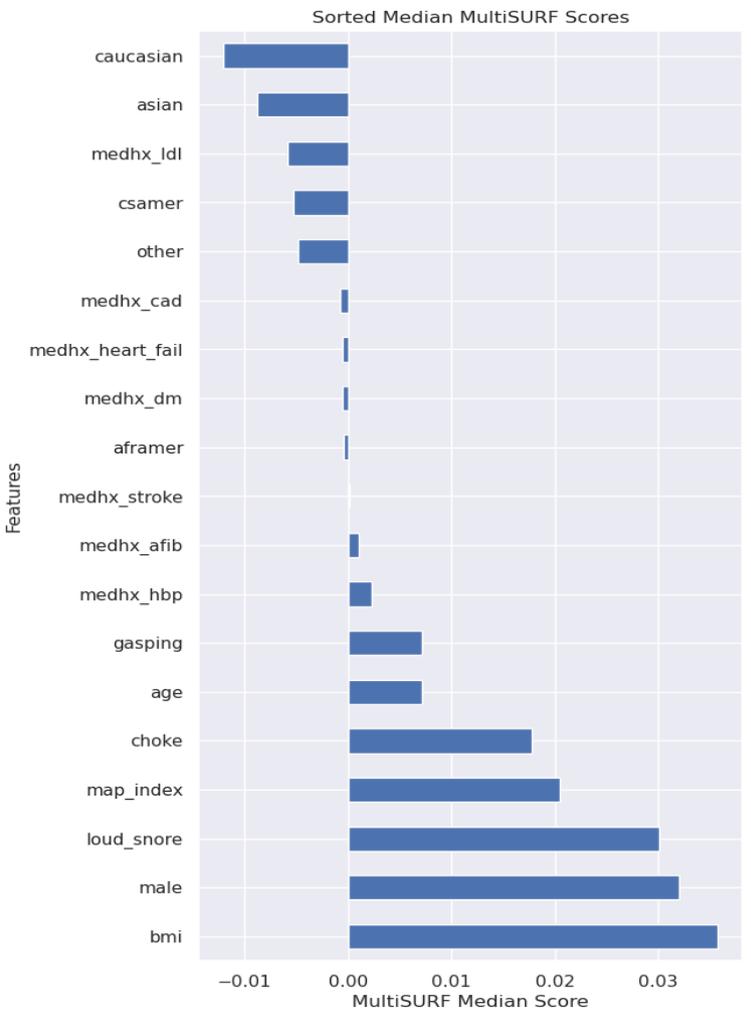

## Composite Feature Importance Plot (Normalized and Performance Weighted)

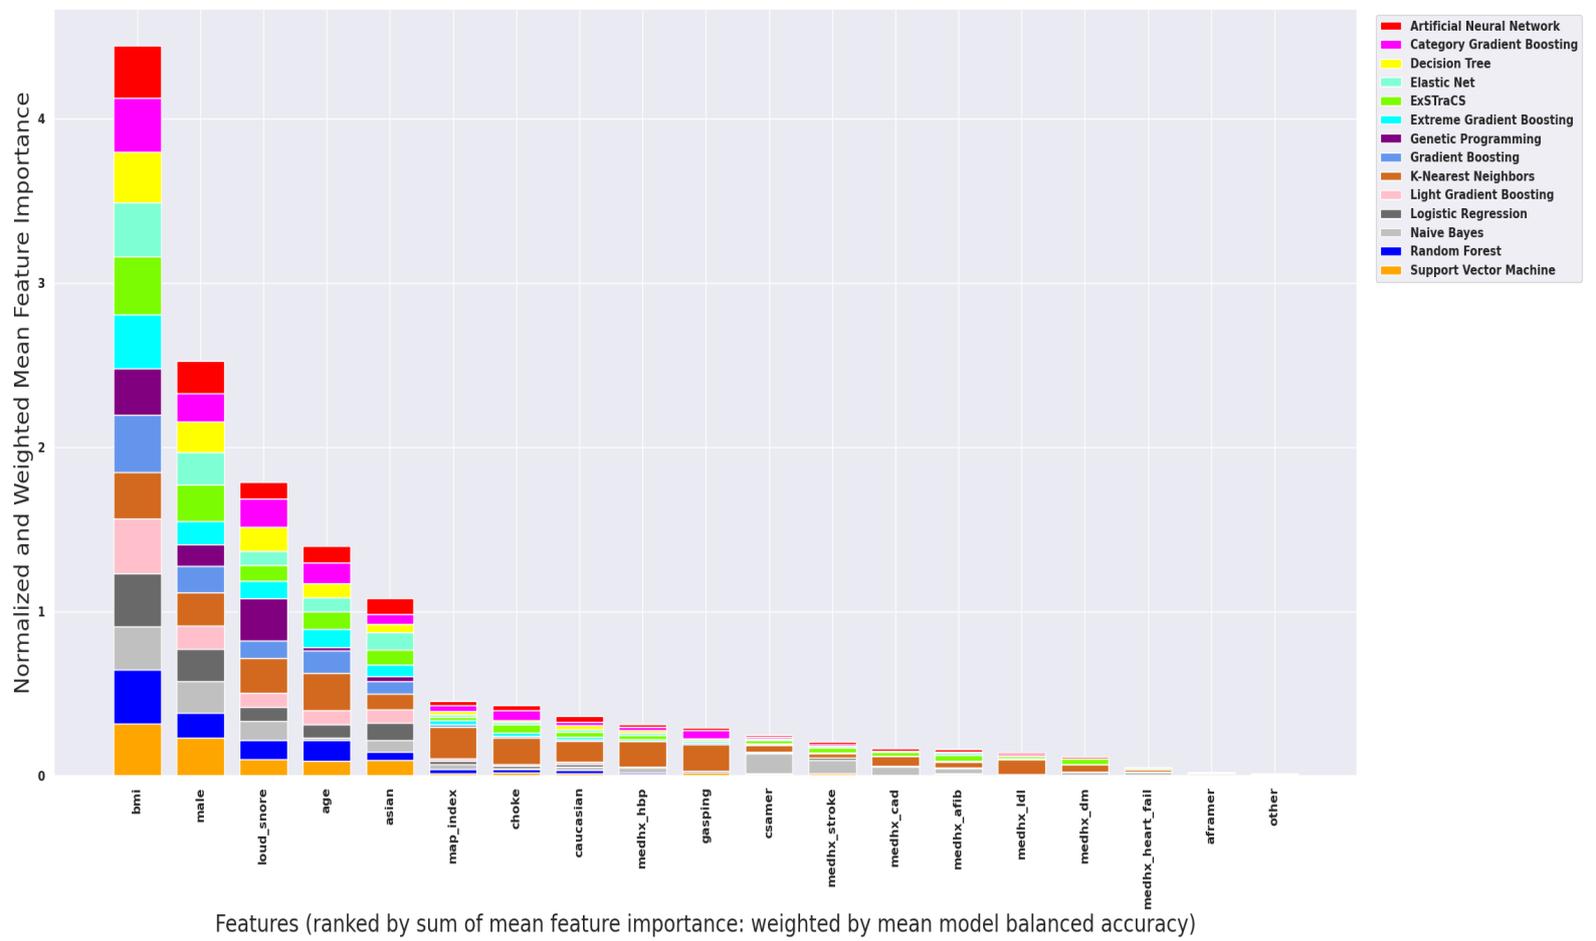

# Feature Importance Summary: D8 = H\_GE15\_DEMDXSYMCF

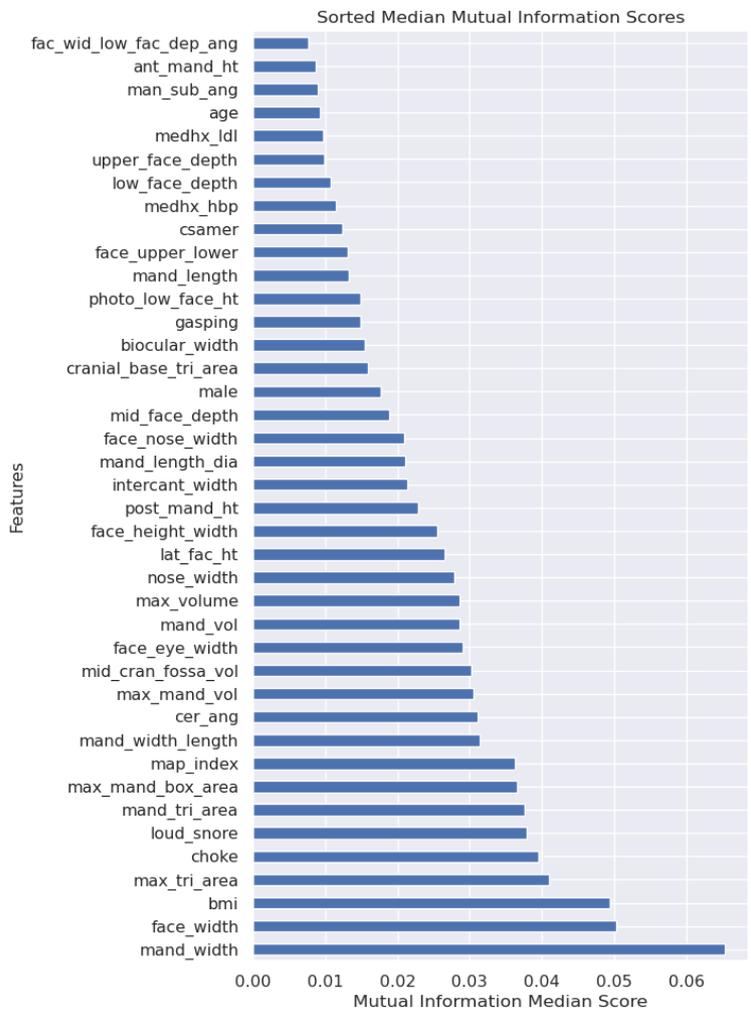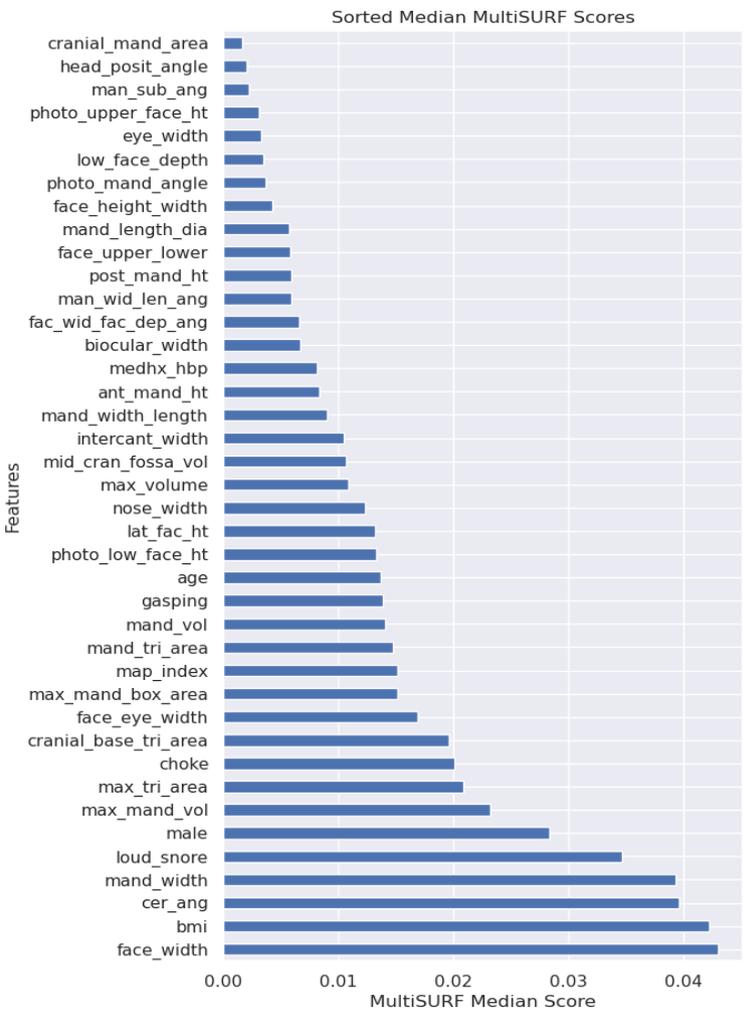

## Composite Feature Importance Plot (Normalized and Performance Weighted)

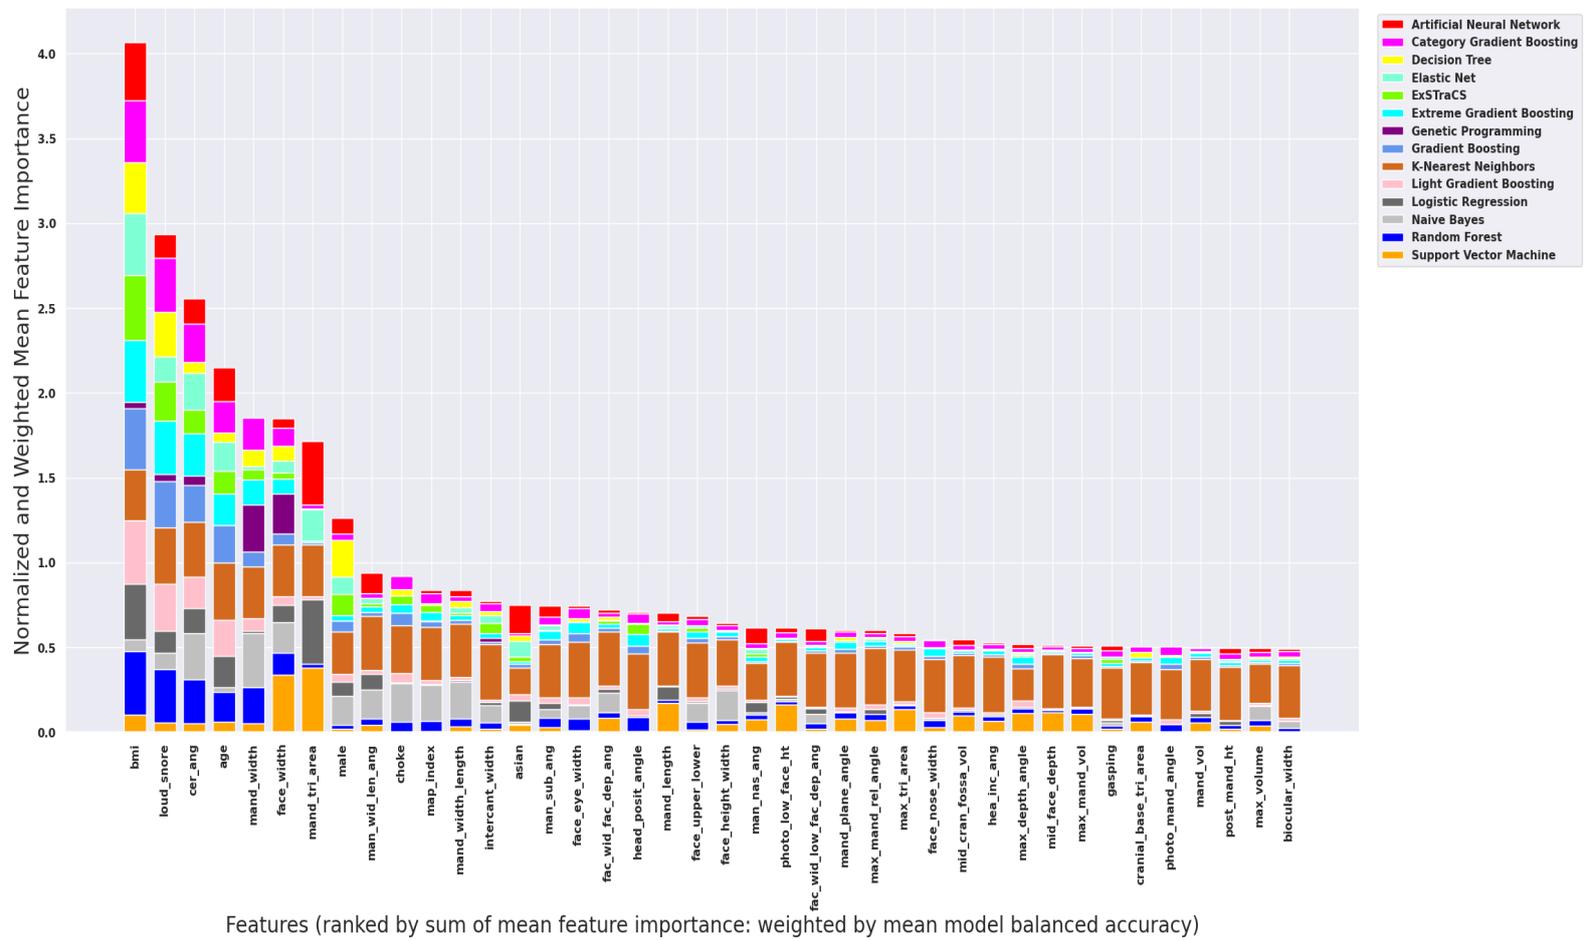

Features (ranked by sum of mean feature importance: weighted by mean model balanced accuracy)

# Feature Importance Summary: D9 = I\_GE15\_DEMDXSVMIO

Sorted Median Mutual Information Scores

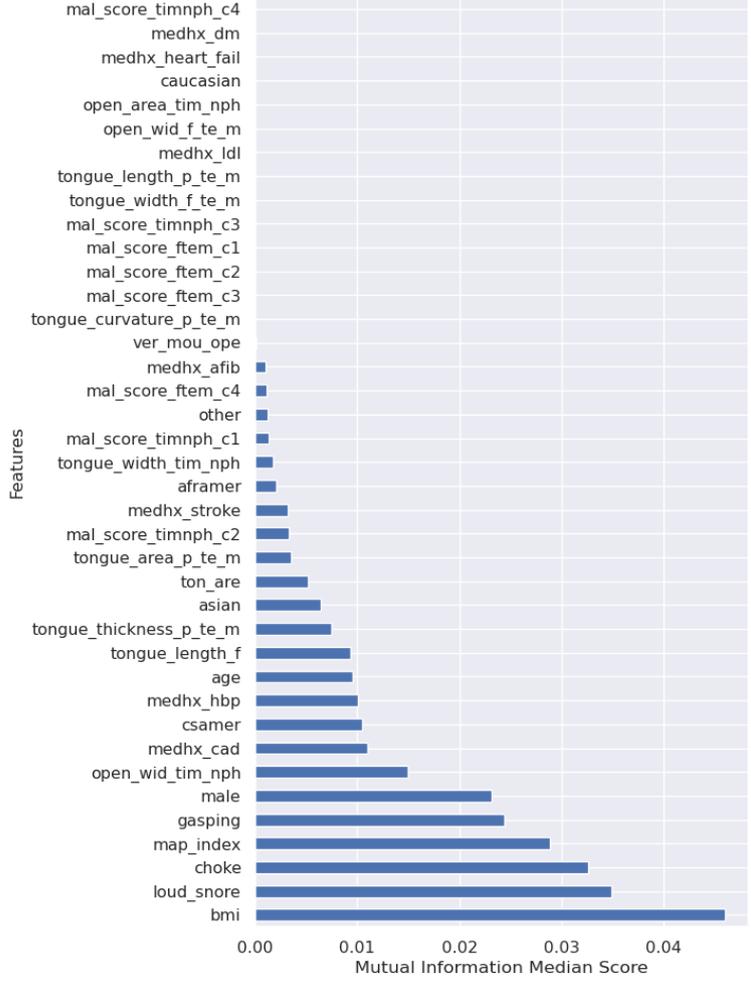

Sorted Median MultiSURF Scores

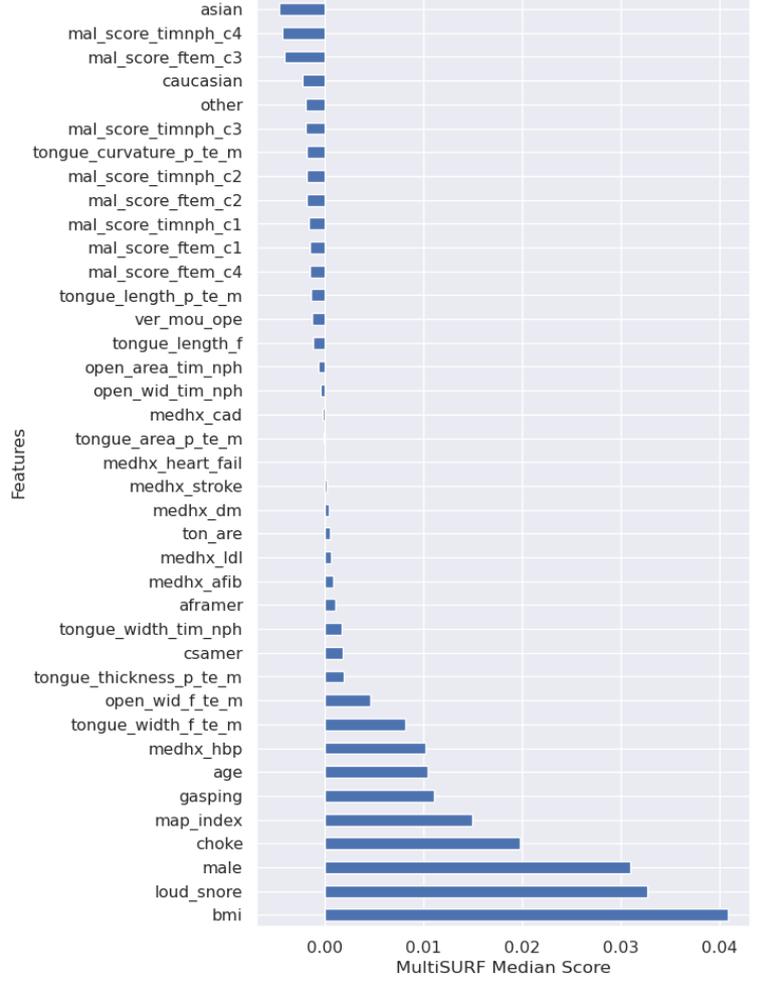

Composite Feature Importance Plot (Normalized and Performance Weighted)

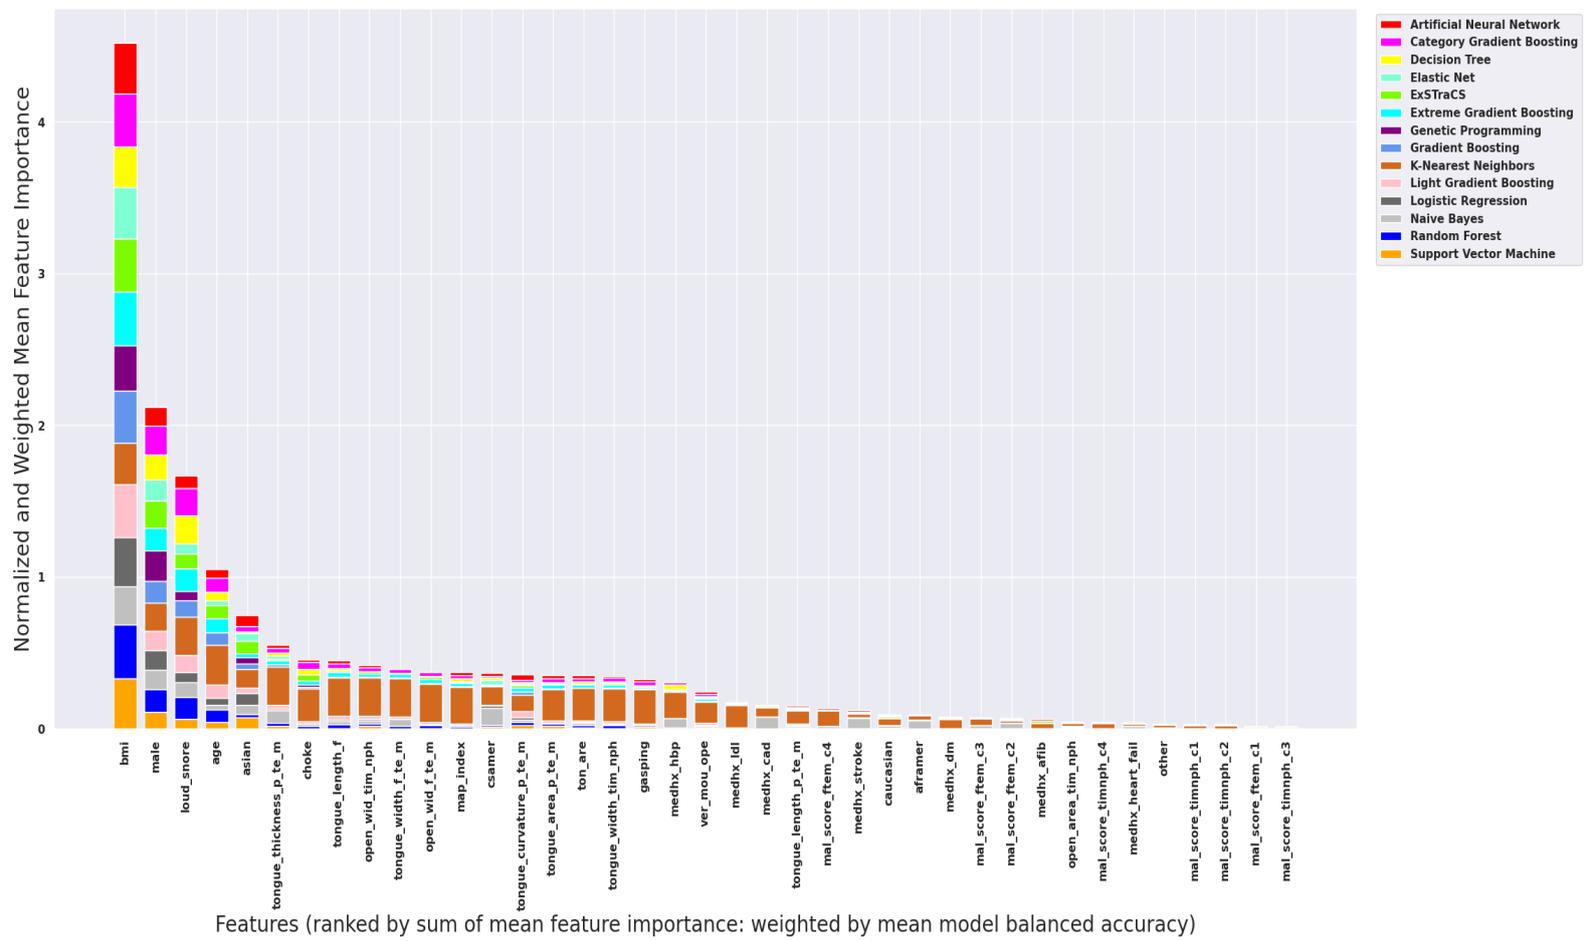

Features (ranked by sum of mean feature importance: weighted by mean model balanced accuracy)

# Feature Importance Summary: D10 = J\_GE15\_DEMDXSYMCFFIO

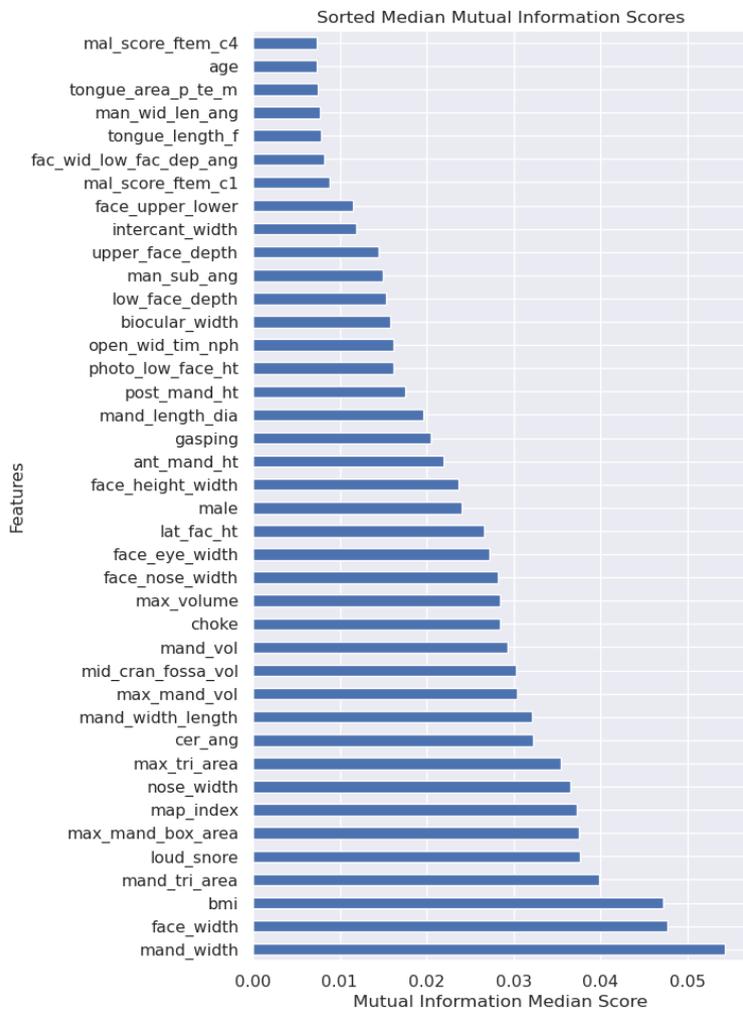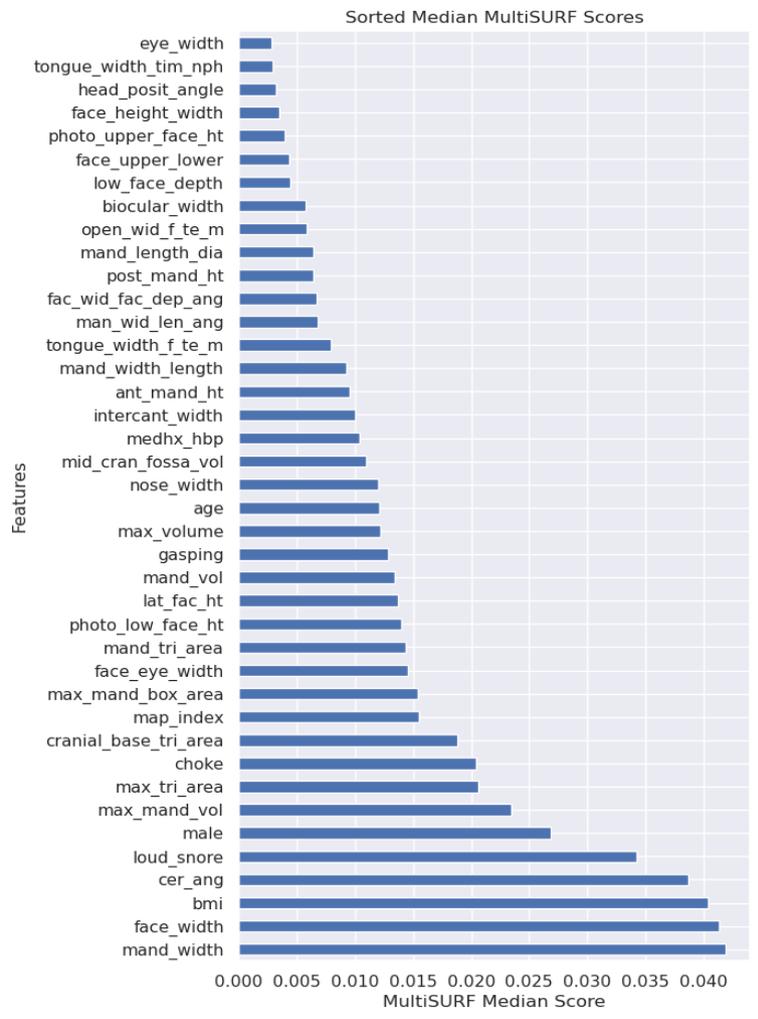

## Composite Feature Importance Plot (Normalized and Performance Weighted)

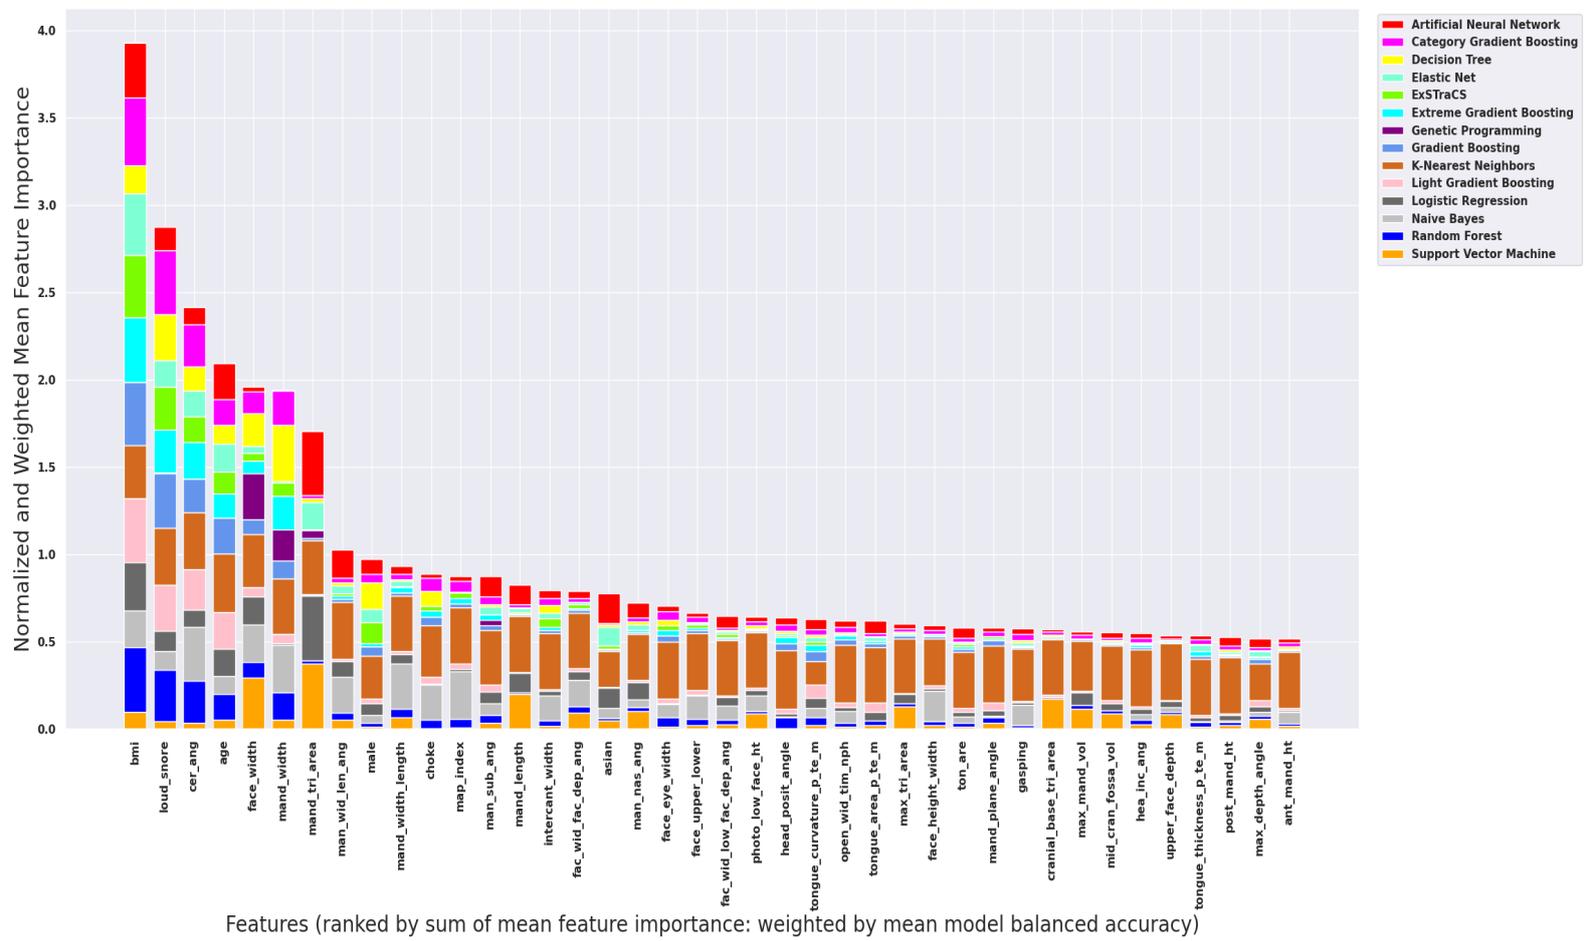

# Feature Importance Summary: D11 = K\_GE5\_DEM

Sorted Median Mutual Information Scores

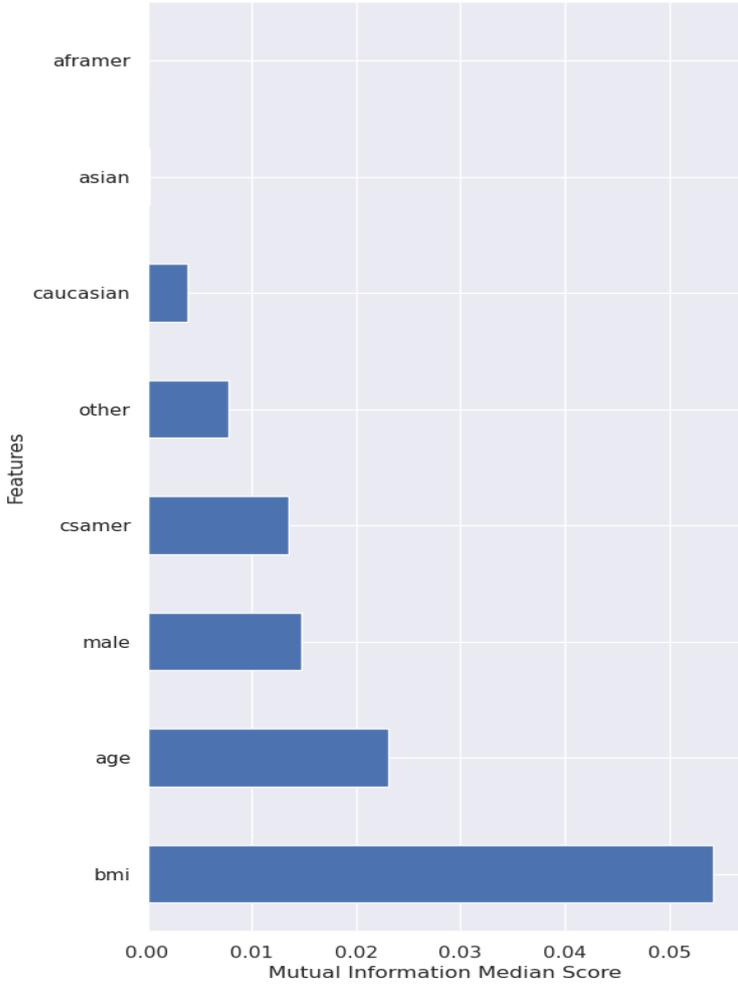

Sorted Median MultiSURF Scores

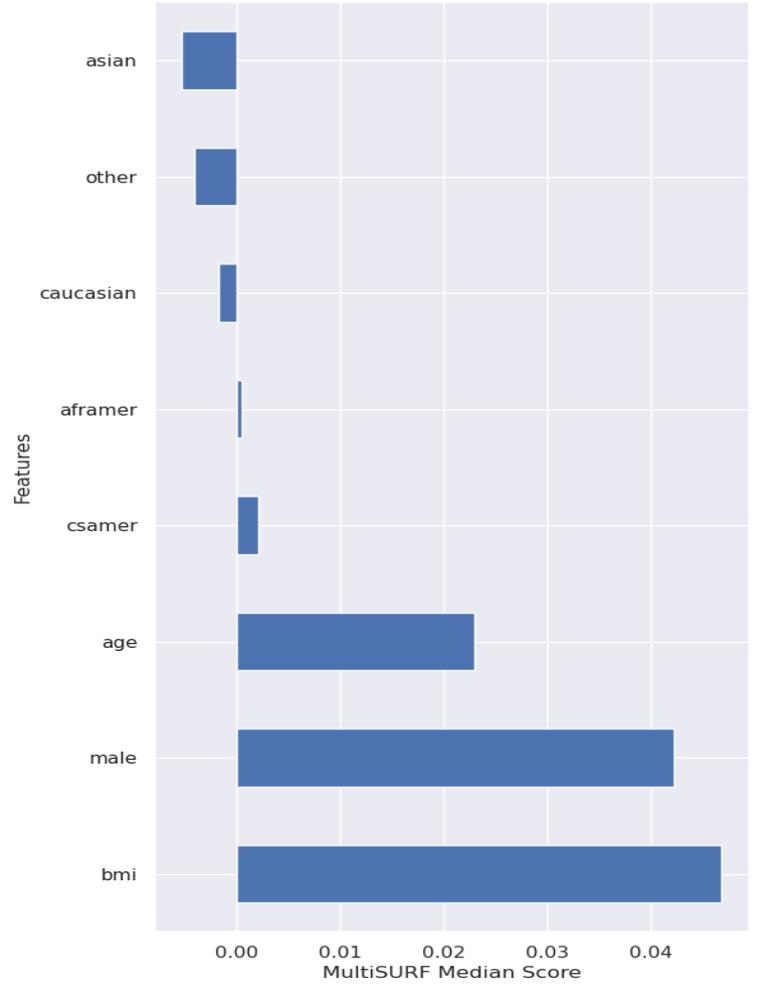

## Composite Feature Importance Plot (Normalized and Performance Weighted)

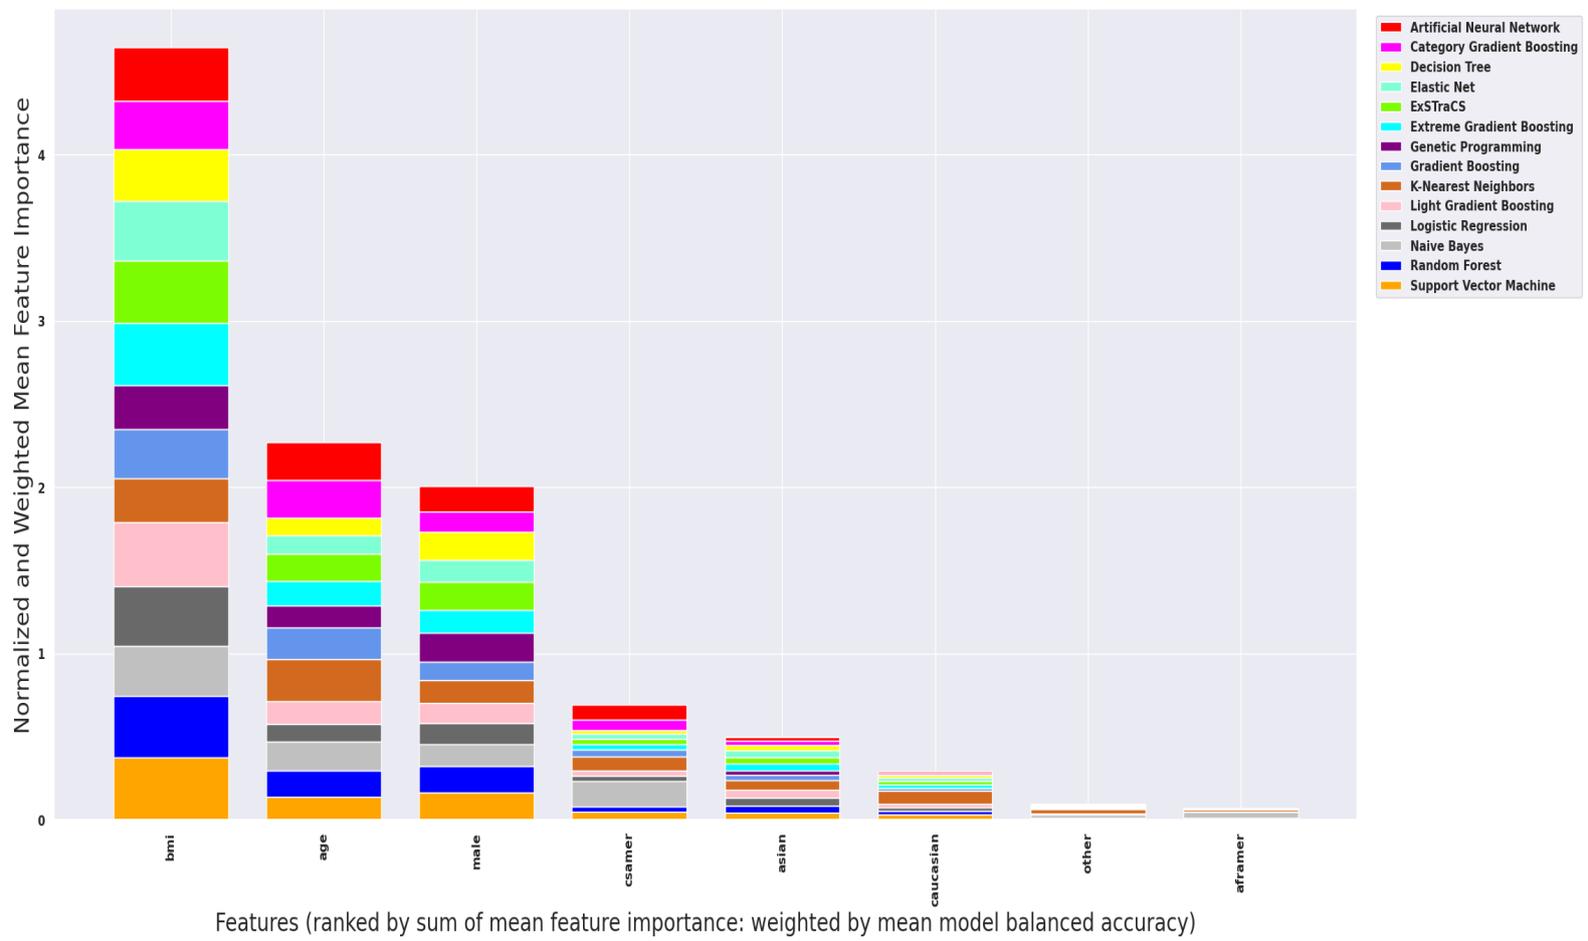

# Feature Importance Summary: D12 = L\_GE5\_DX

Sorted Median Mutual Information Scores

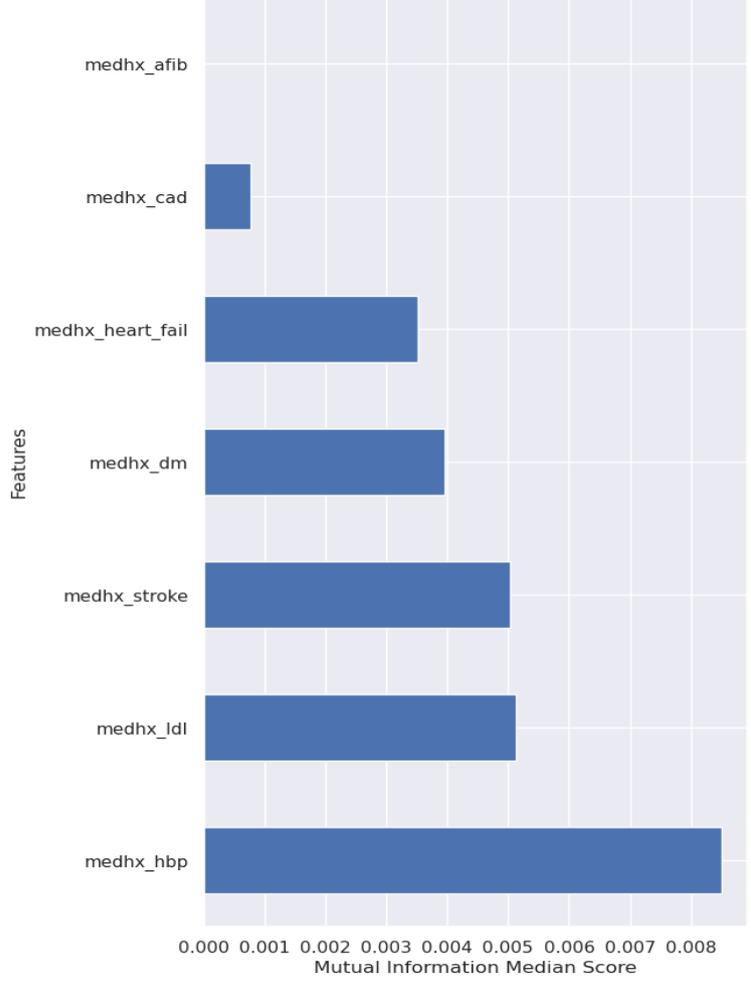

Sorted Median MultiSURF Scores

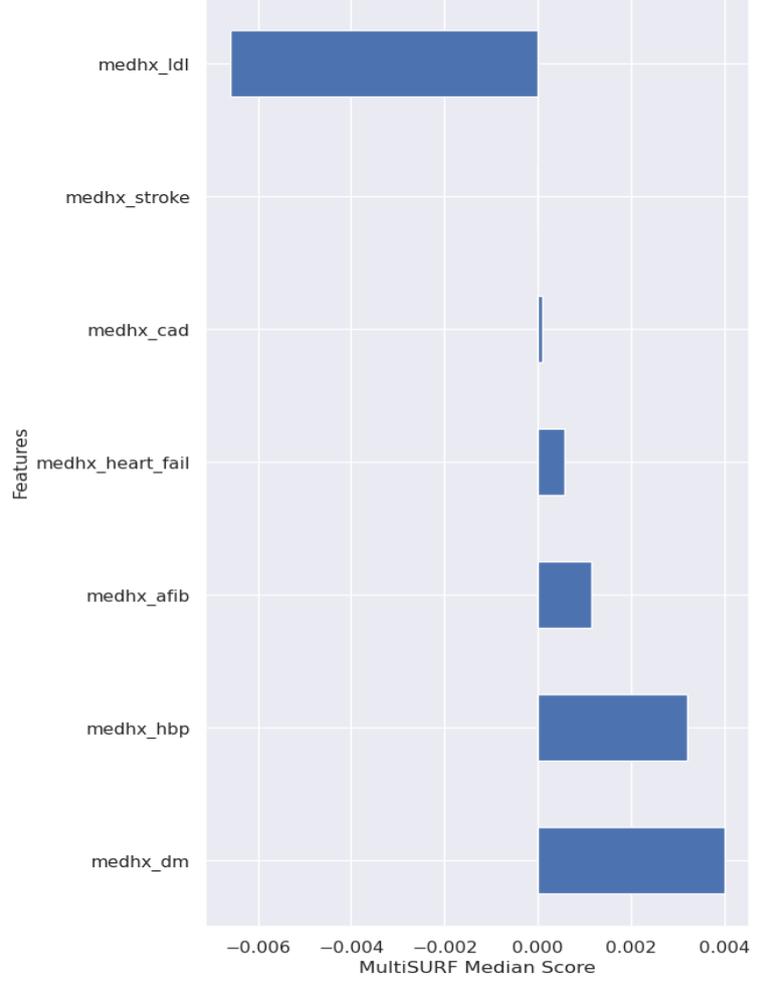

## Composite Feature Importance Plot (Normalized and Performance Weighted)

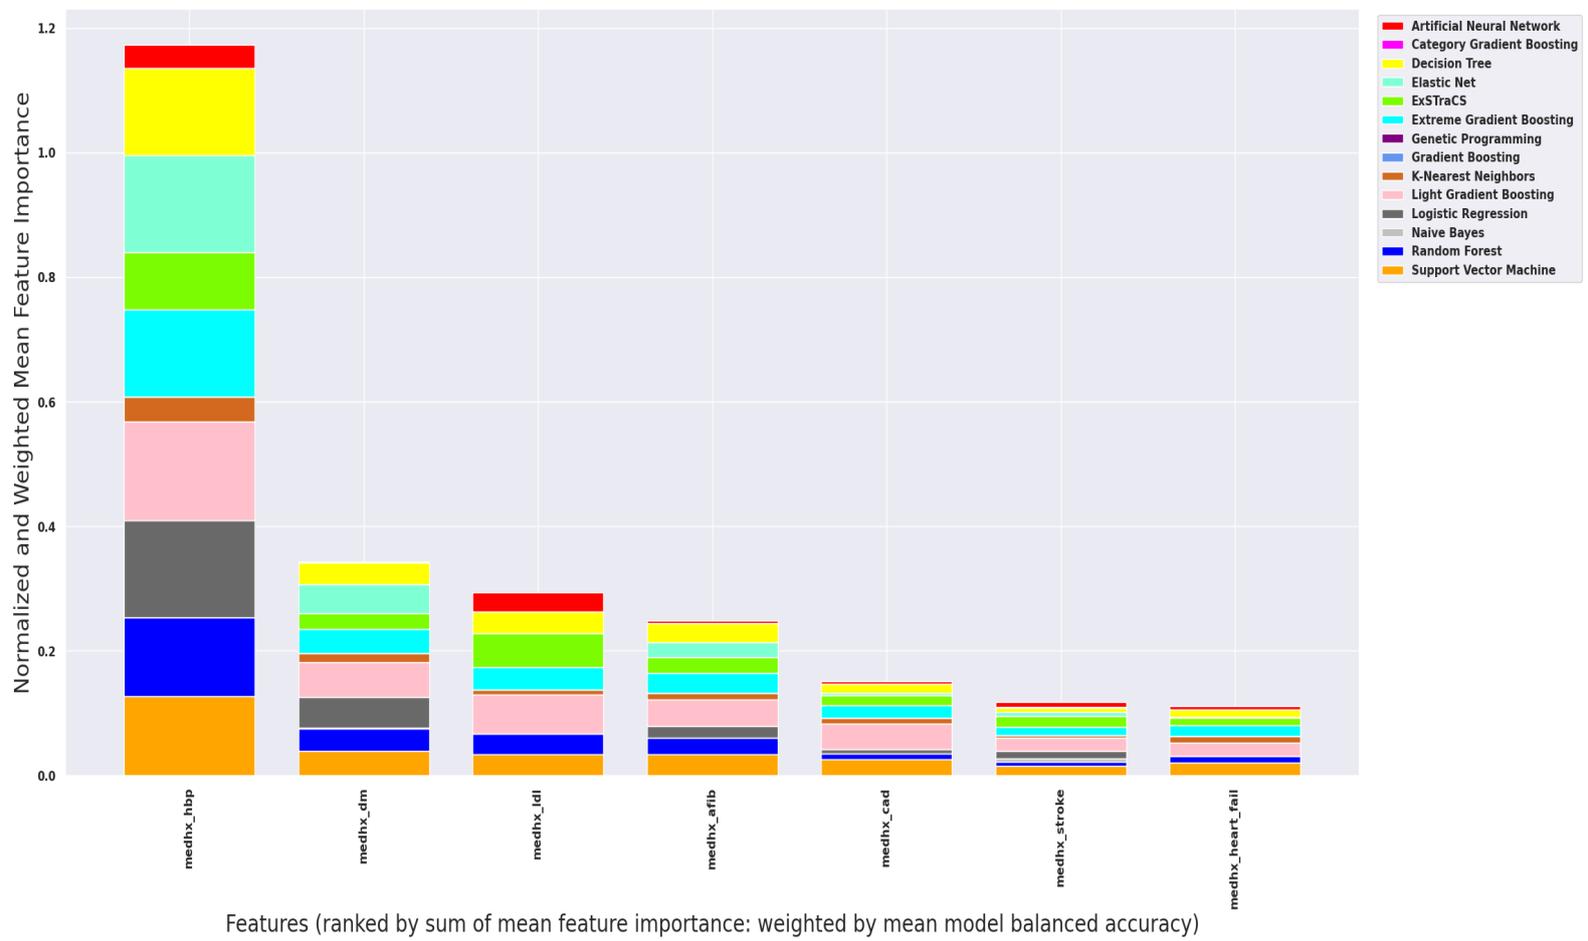

# Feature Importance Summary: D13 = M\_GE5\_SYM

Sorted Median Mutual Information Scores

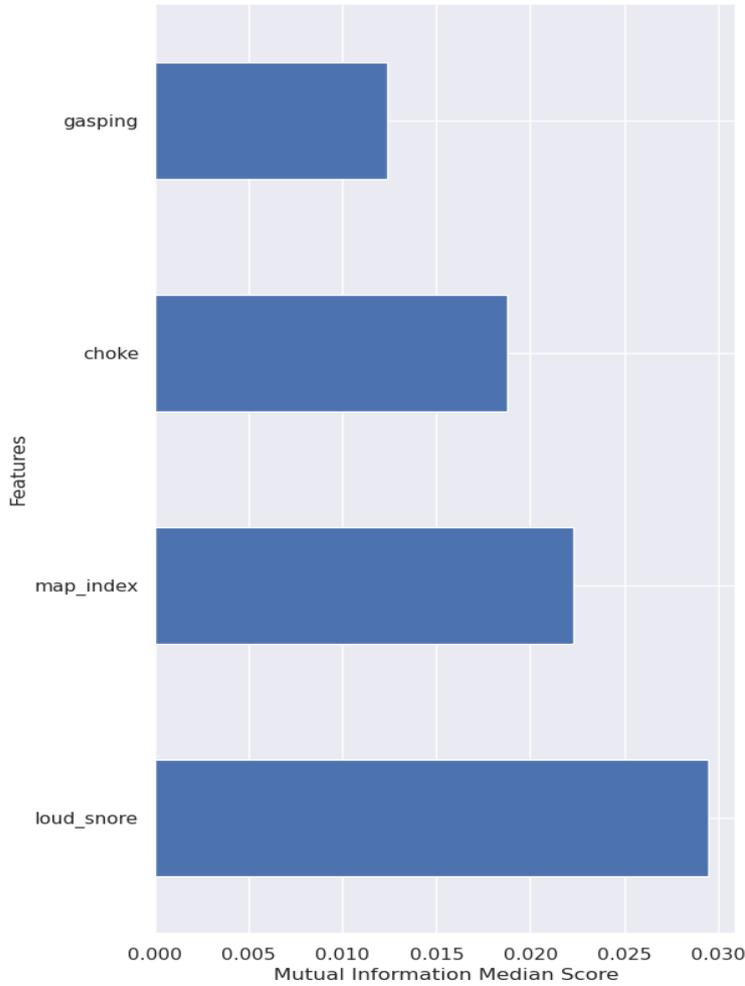

Sorted Median MultiSURF Scores

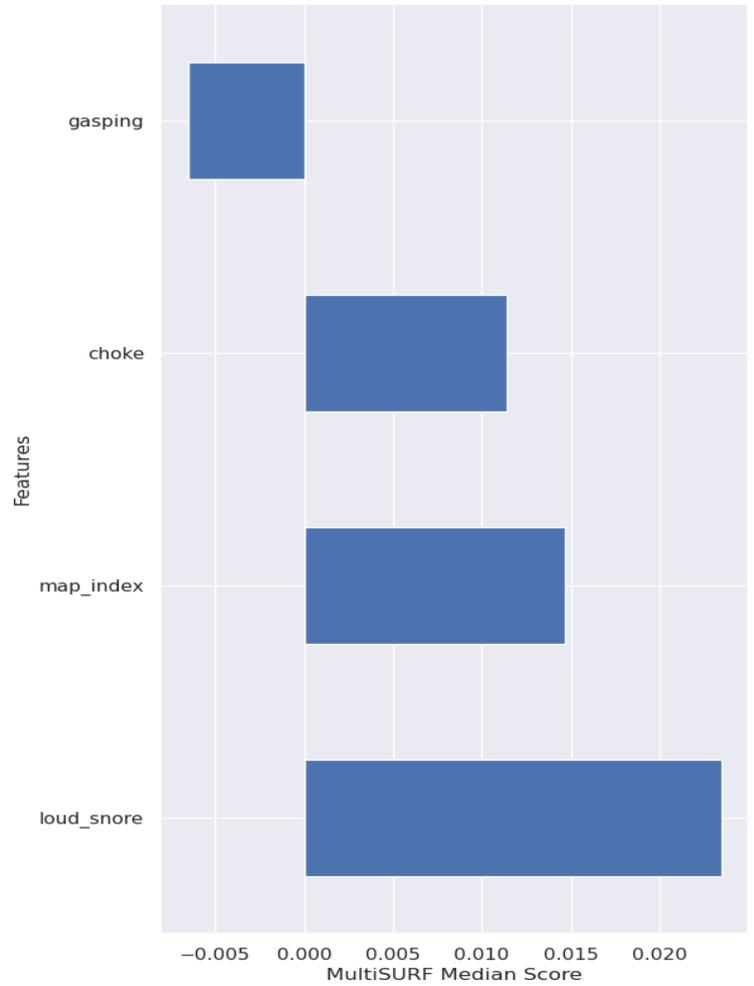

## Composite Feature Importance Plot (Normalized and Performance Weighted)

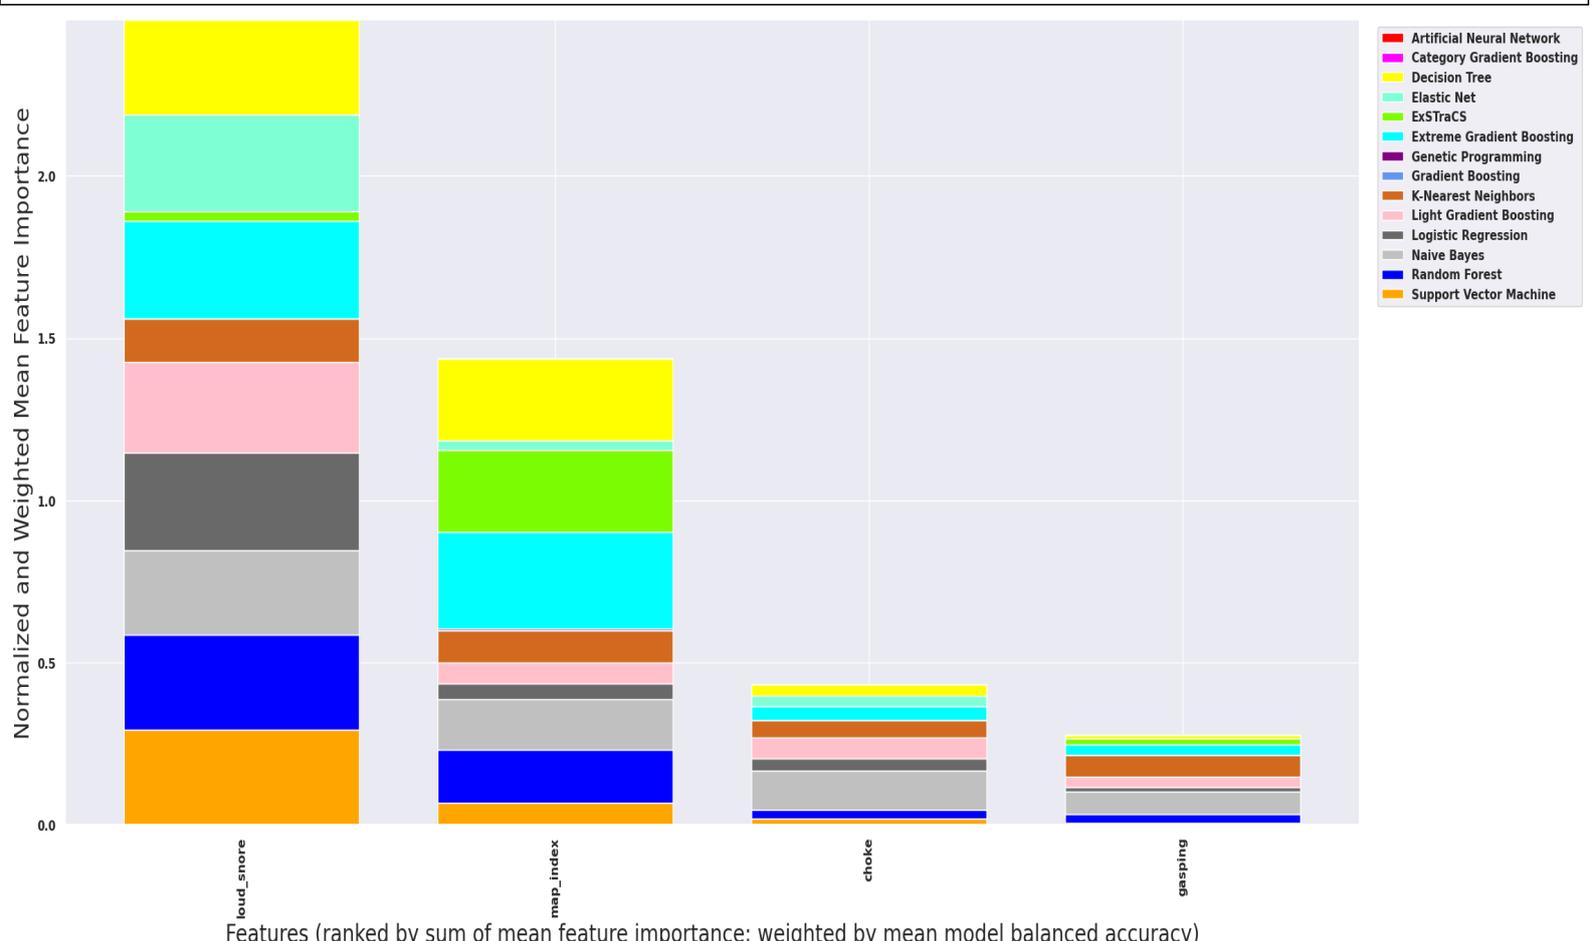

- Artificial Neural Network
- Category Gradient Boosting
- Decision Tree
- Elastic Net
- ExSTraCS
- Extreme Gradient Boosting
- Genetic Programming
- Gradient Boosting
- K-Nearest Neighbors
- Light Gradient Boosting
- Logistic Regression
- Naive Bayes
- Random Forest
- Support Vector Machine

# Feature Importance Summary: D14 = N\_GE5\_CF

Sorted Median Mutual Information Scores

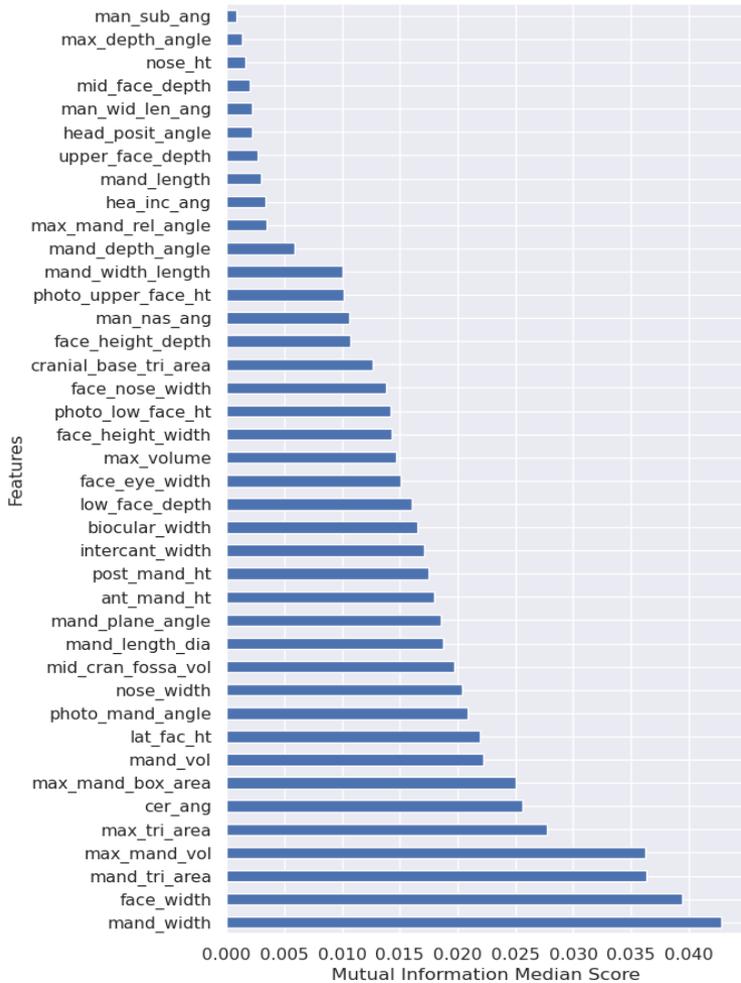

Sorted Median MultiSURF Scores

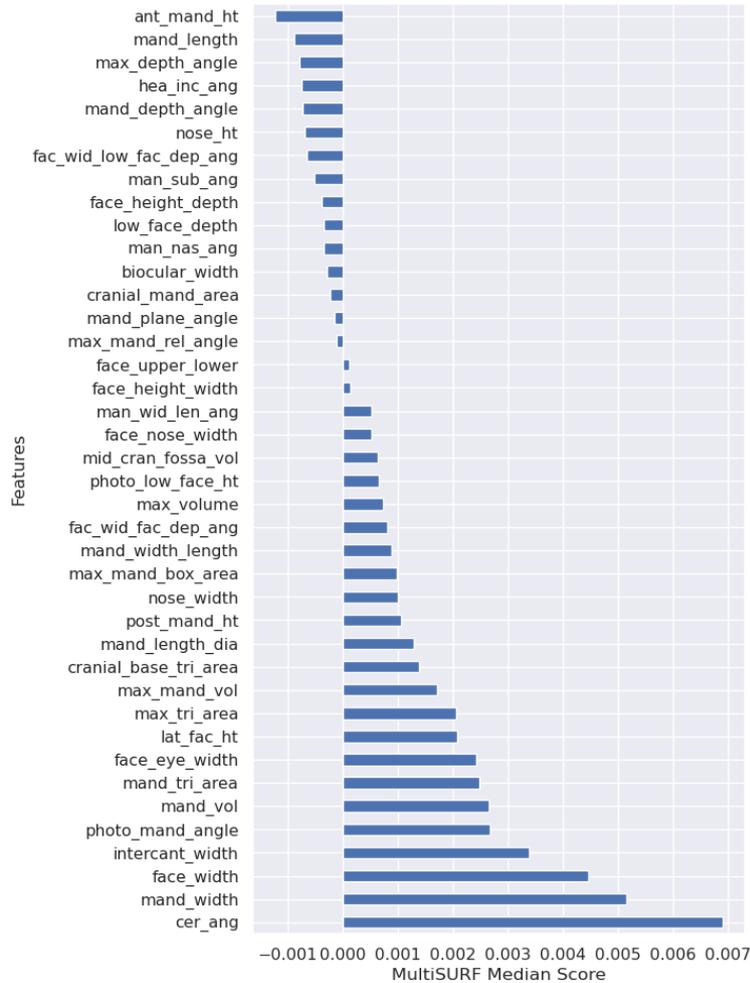

Composite Feature Importance Plot (Normalized and Performance Weighted)

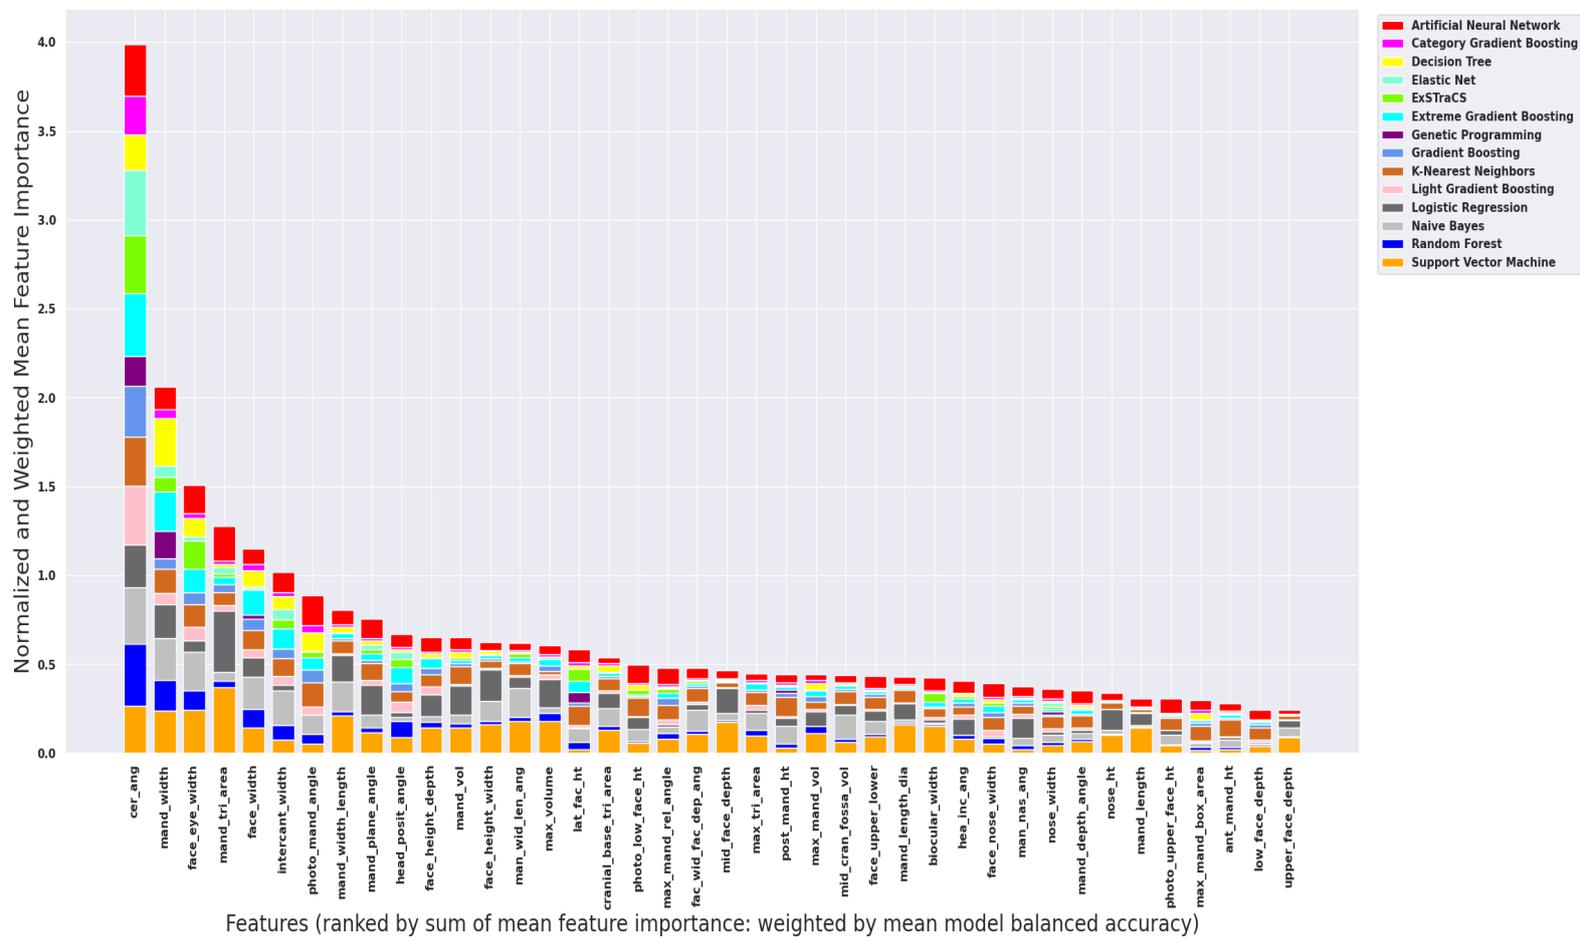

# Feature Importance Summary: D15 = O\_GE5\_IO

Sorted Median Mutual Information Scores

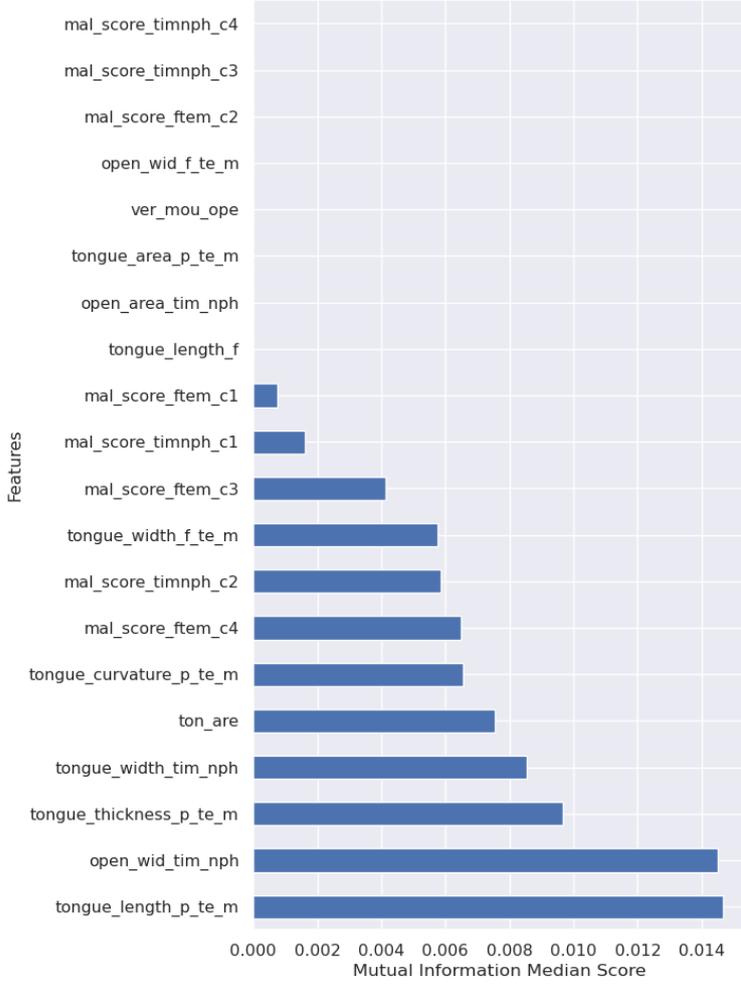

Sorted Median MultiSURF Scores

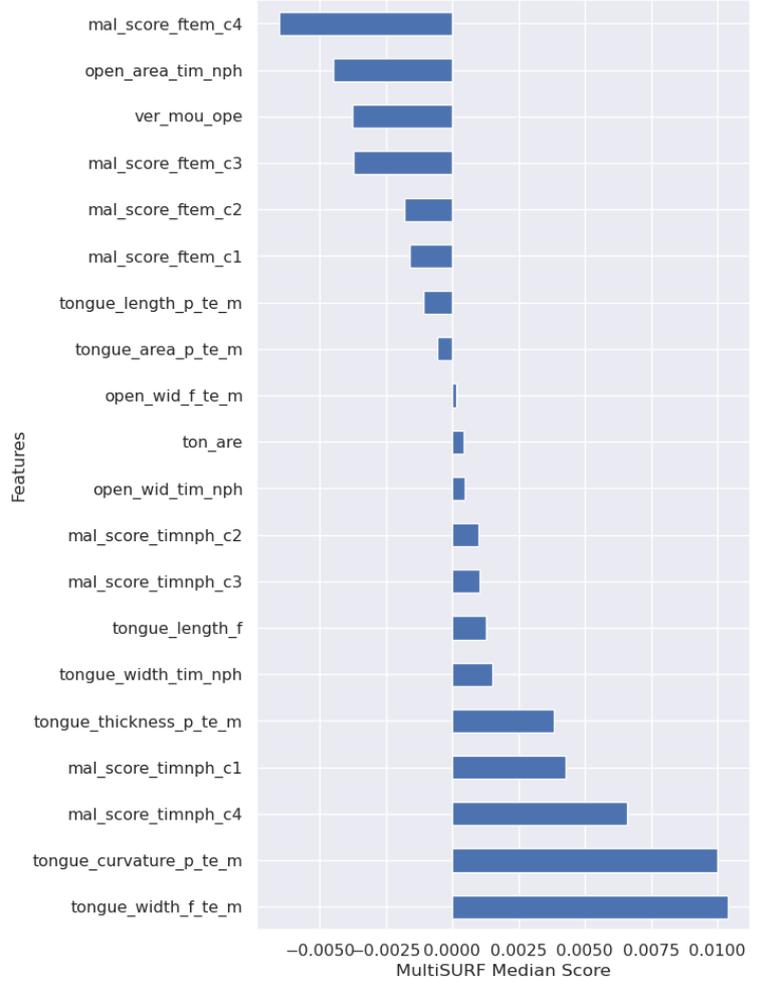

## Composite Feature Importance Plot (Normalized and Performance Weighted)

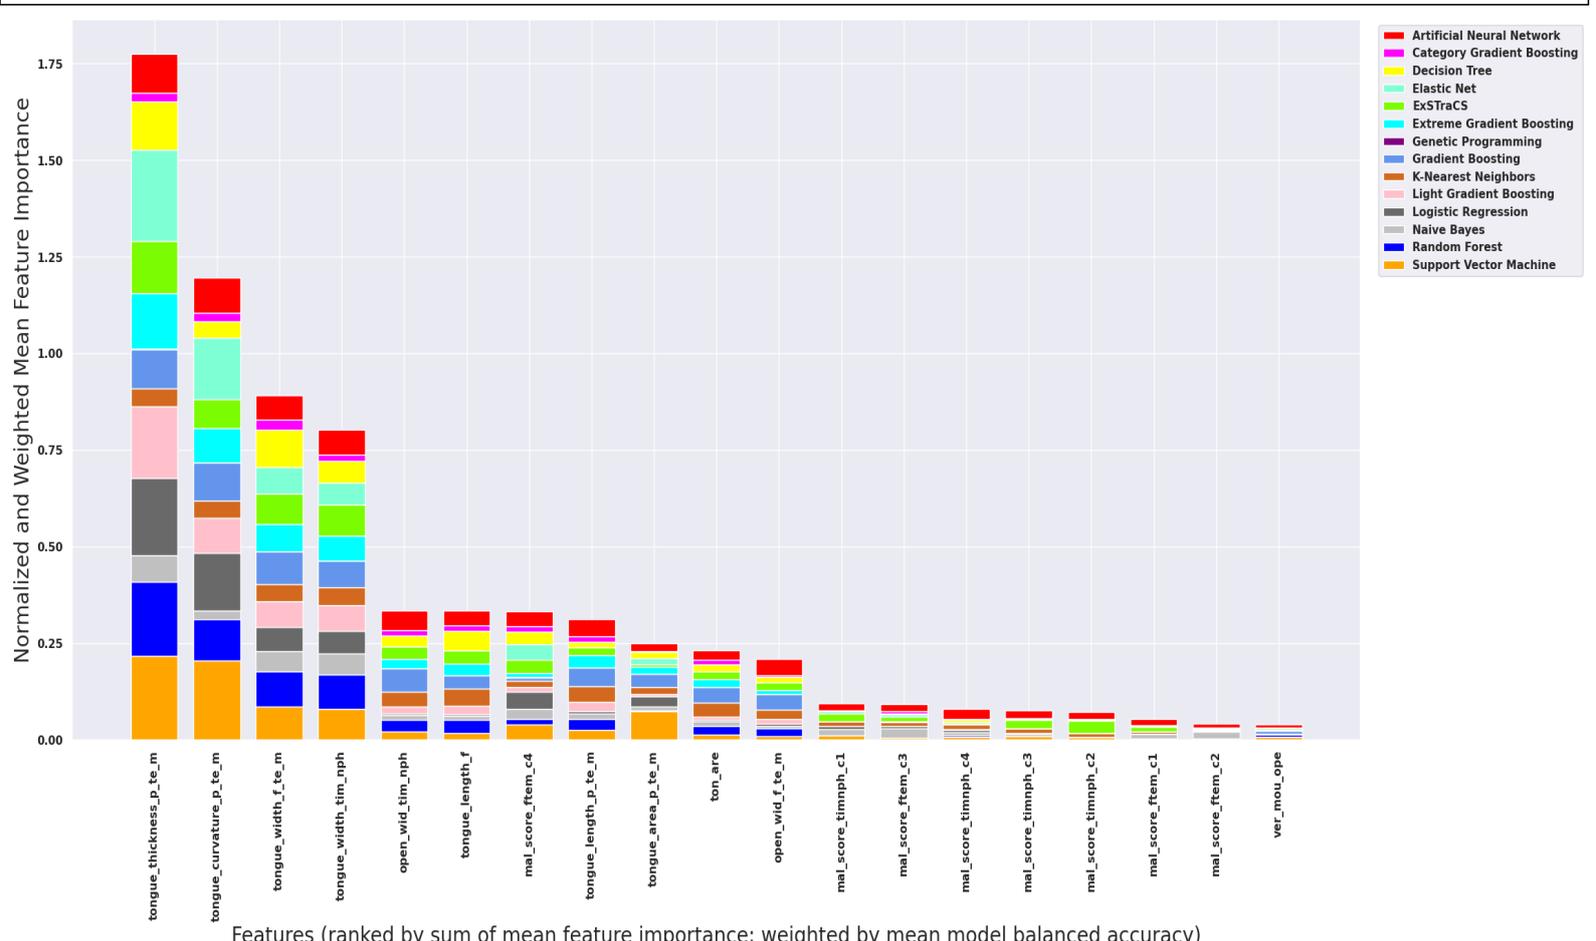

Features (ranked by sum of mean feature importance: weighted by mean model balanced accuracy)

# Feature Importance Summary: D16 = P\_GE5\_DEMDX

Sorted Median Mutual Information Scores

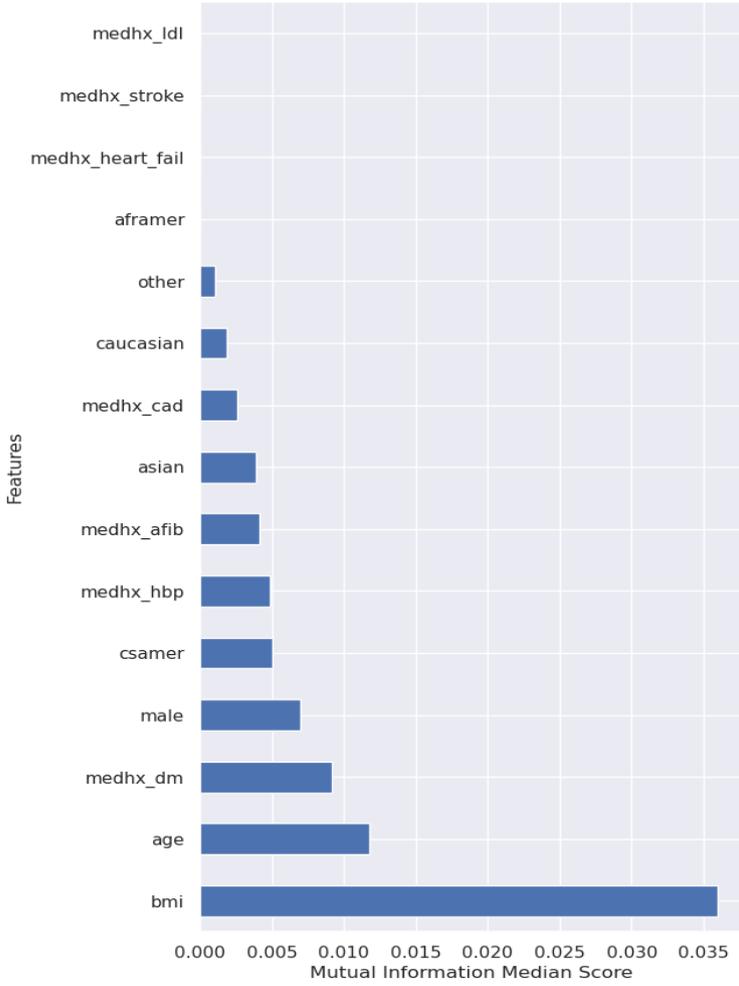

Sorted Median MultiSURF Scores

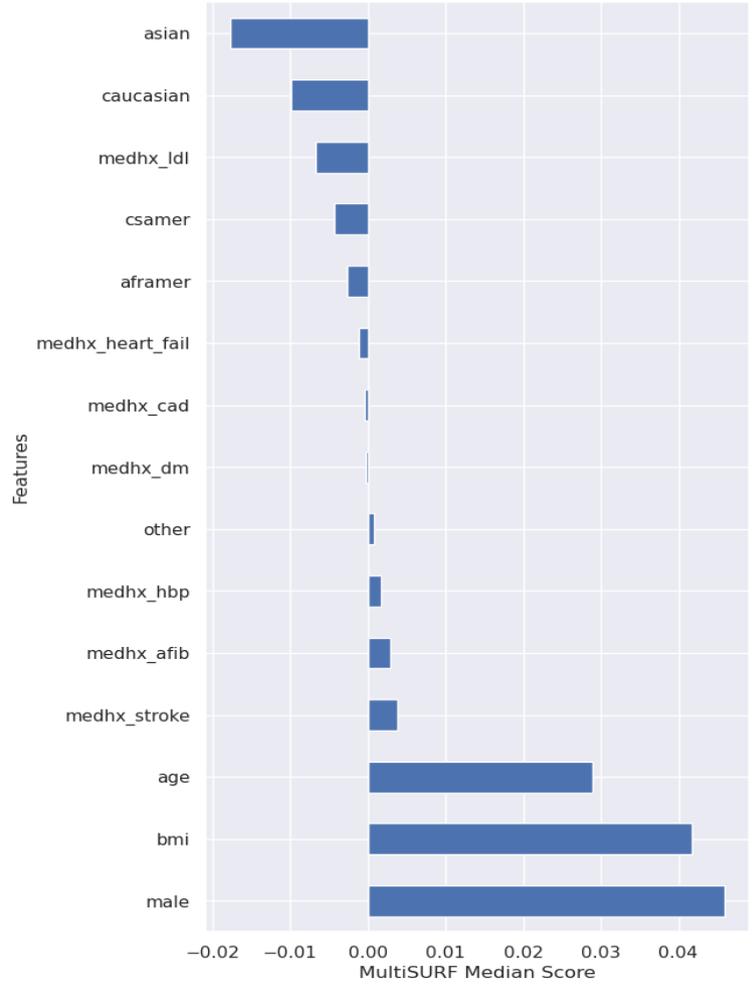

## Composite Feature Importance Plot (Normalized and Performance Weighted)

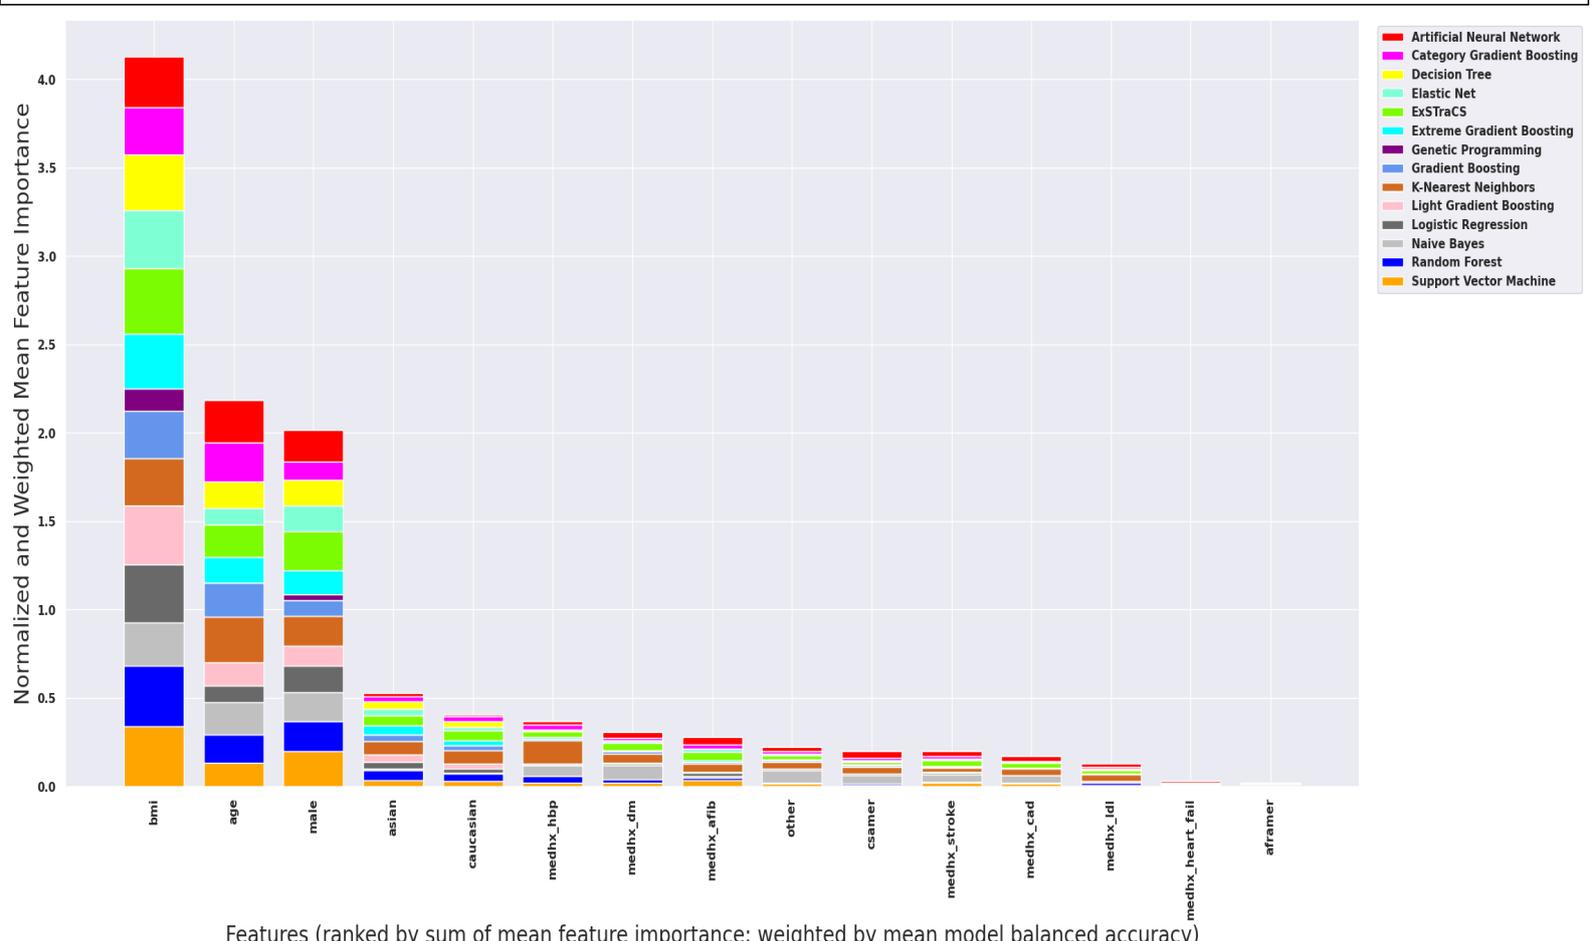

# Feature Importance Summary: D17 = Q\_GE5\_DEMDXSYM

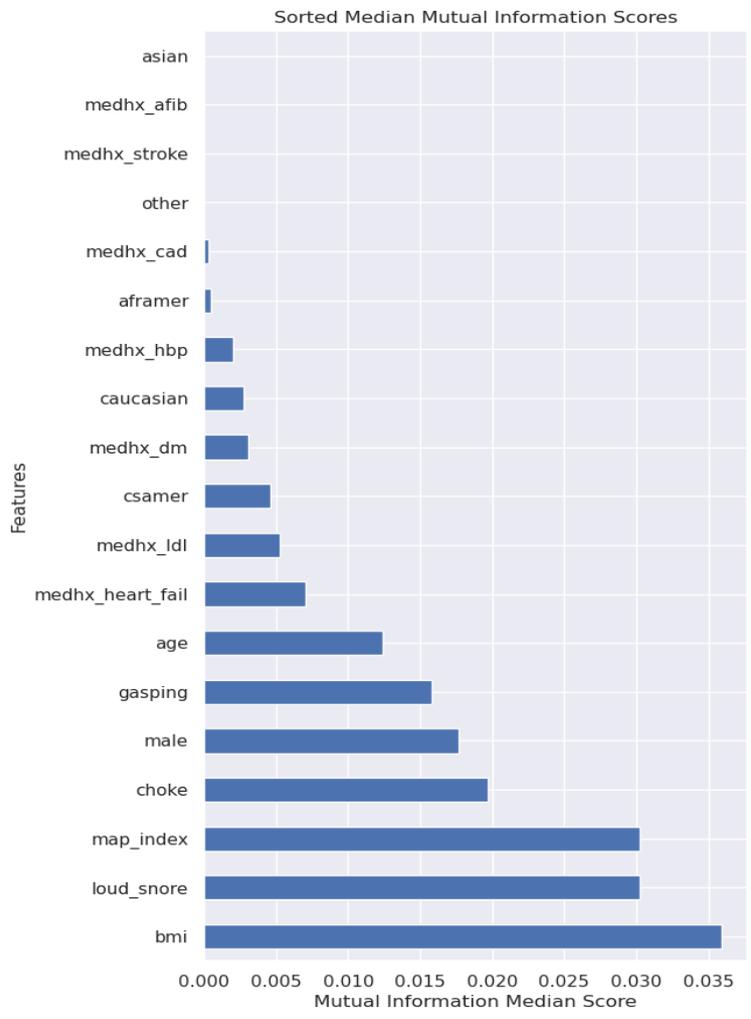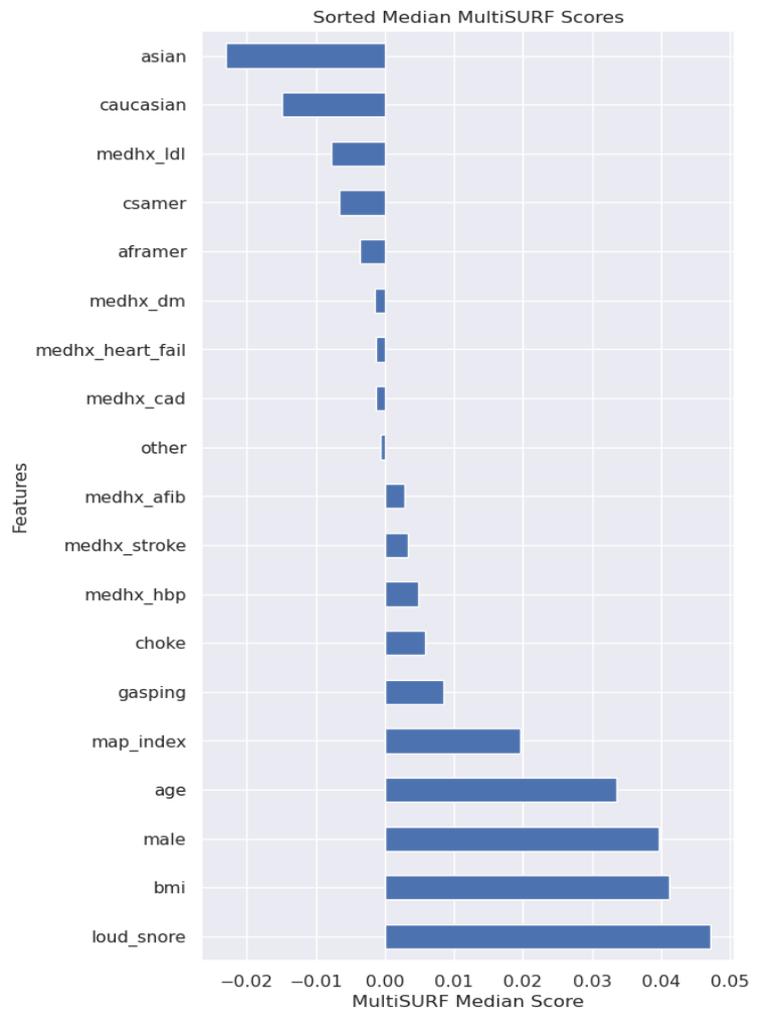

## Composite Feature Importance Plot (Normalized and Performance Weighted)

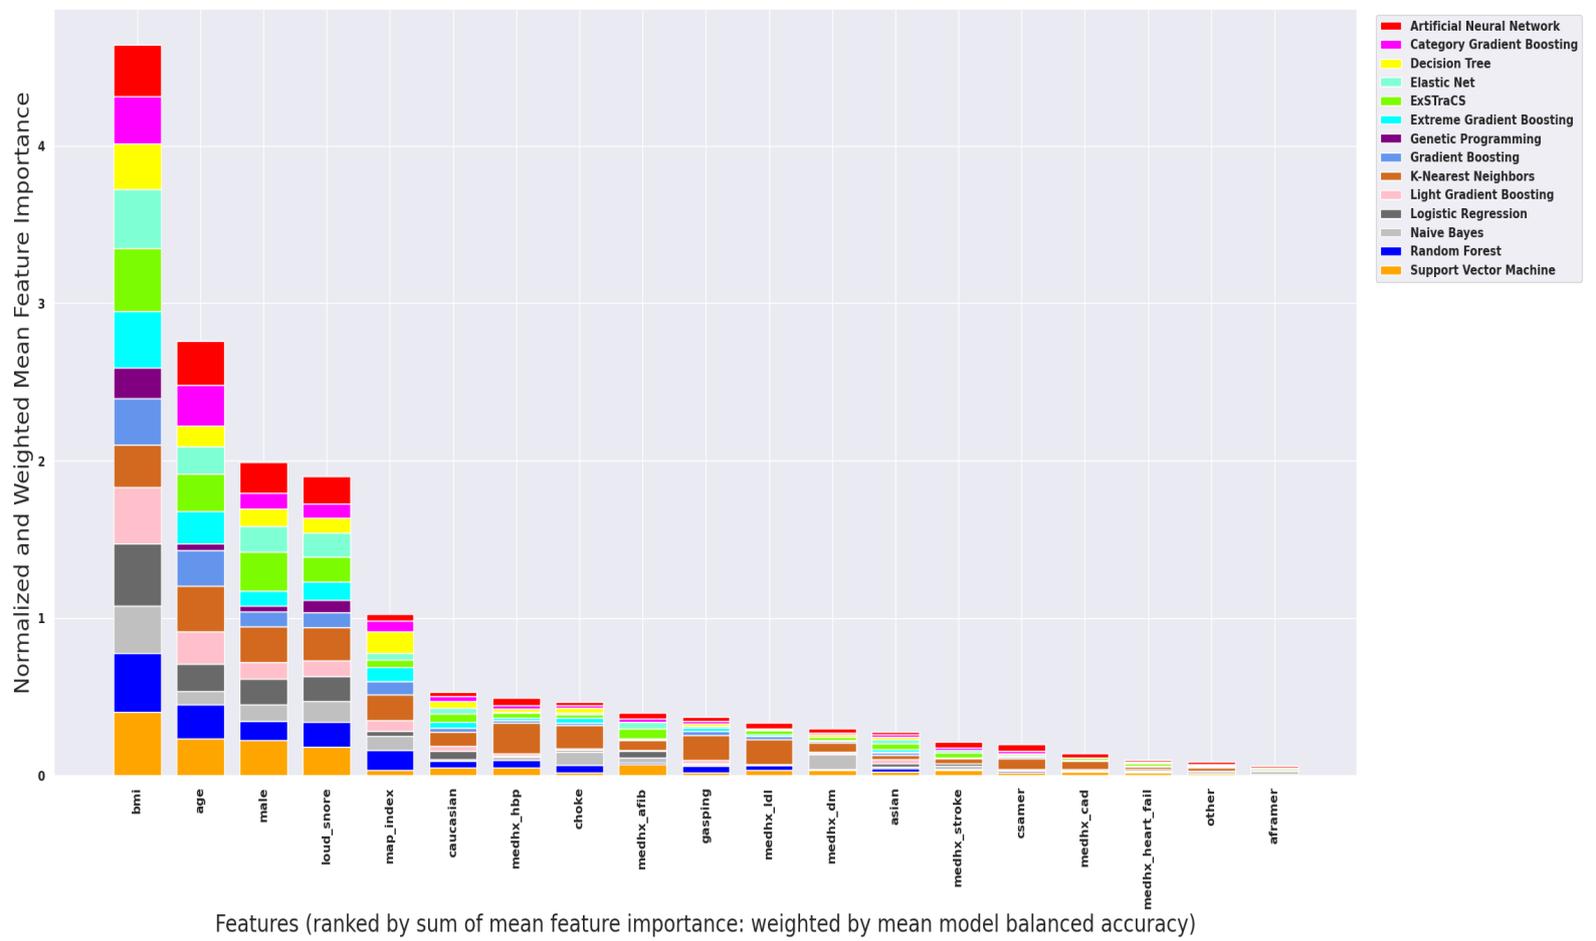

# Feature Importance Summary: D18 = R\_GE5\_DEMDXSYMCF

Sorted Median Mutual Information Scores

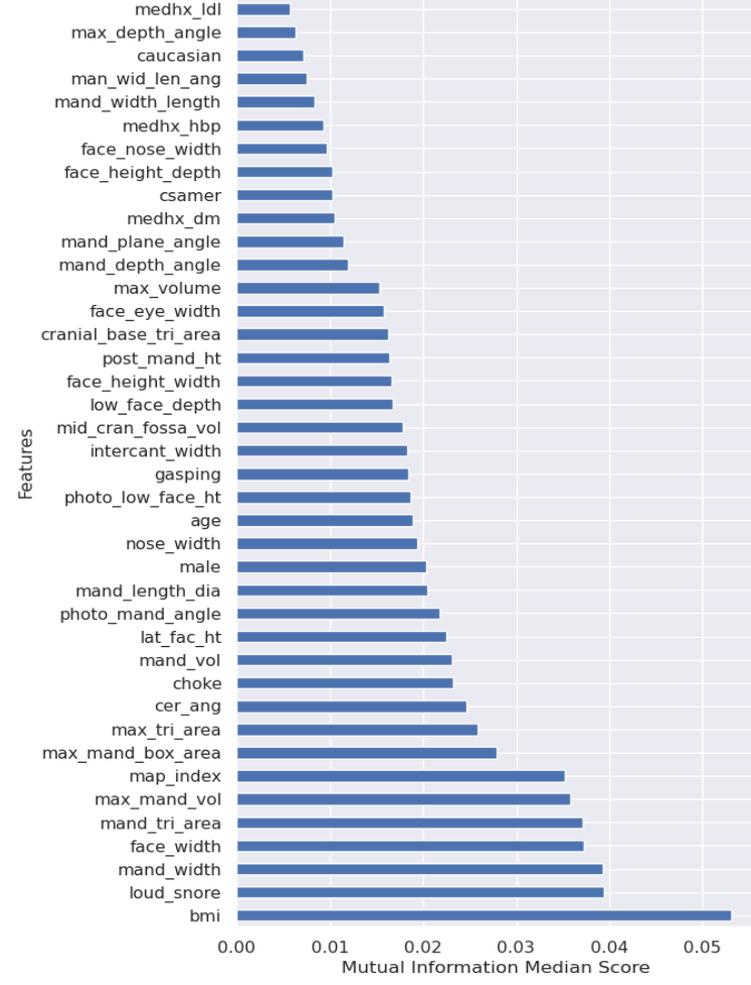

Sorted Median MultiSURF Scores

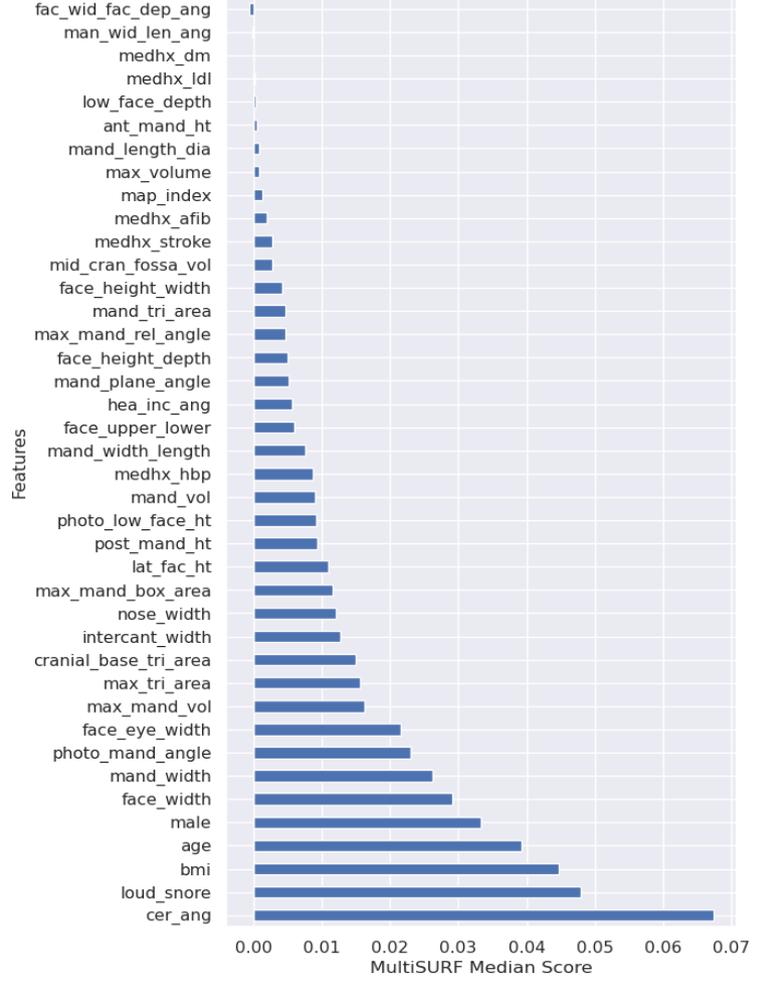

Composite Feature Importance Plot (Normalized and Performance Weighted)

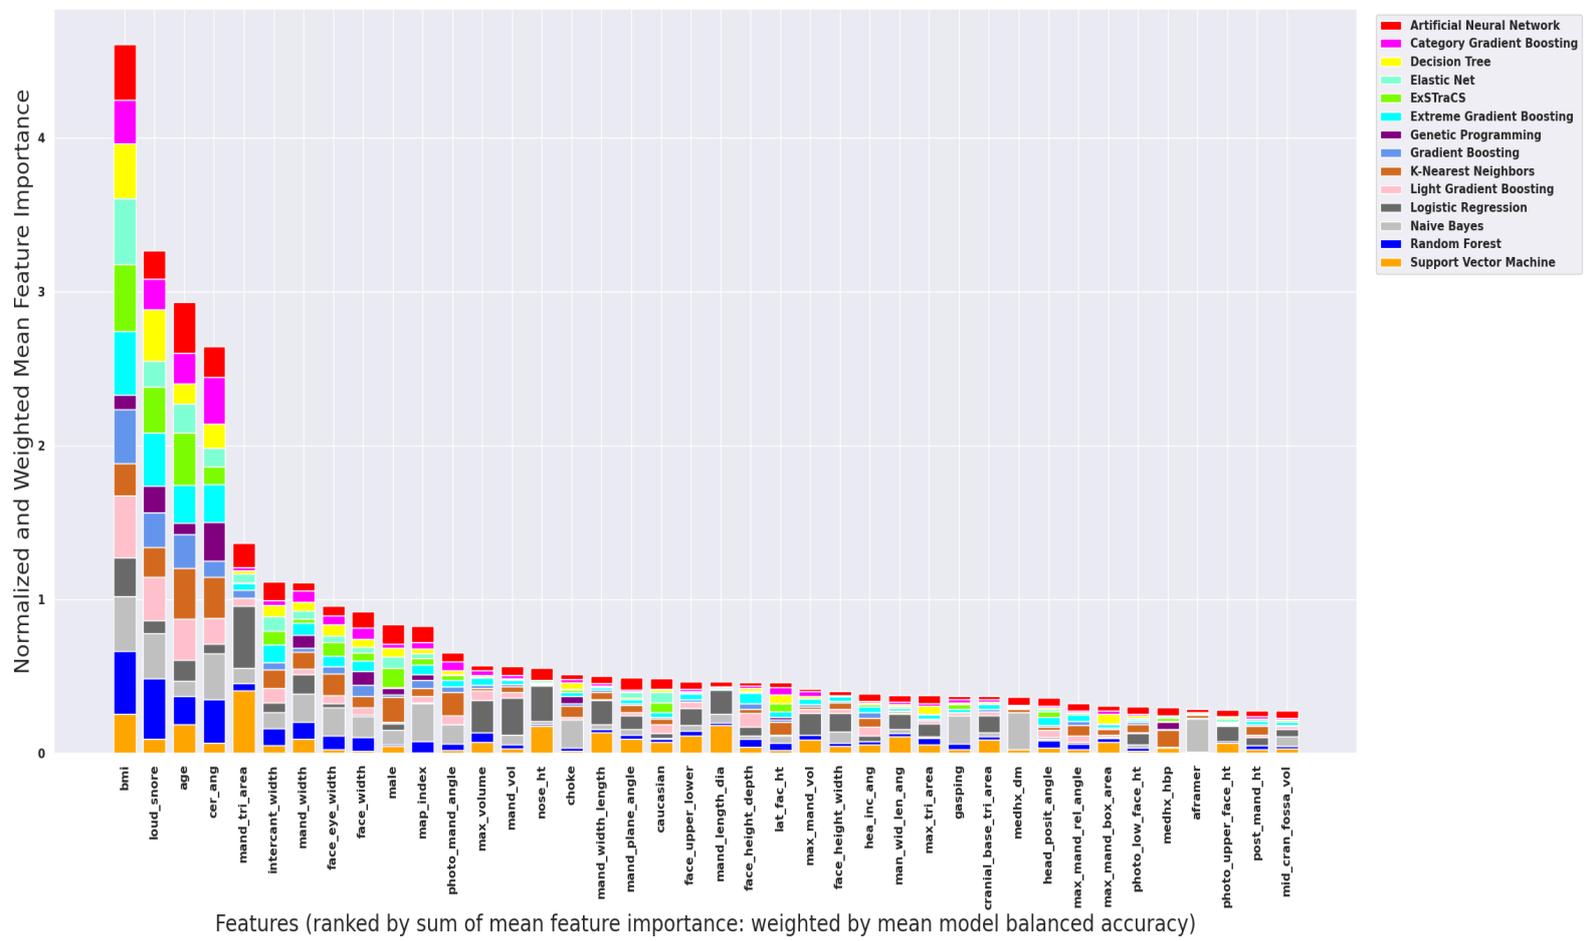

Features (ranked by sum of mean feature importance: weighted by mean model balanced accuracy)

# Feature Importance Summary: D19 = S\_GE5\_DEMDXSYMIO

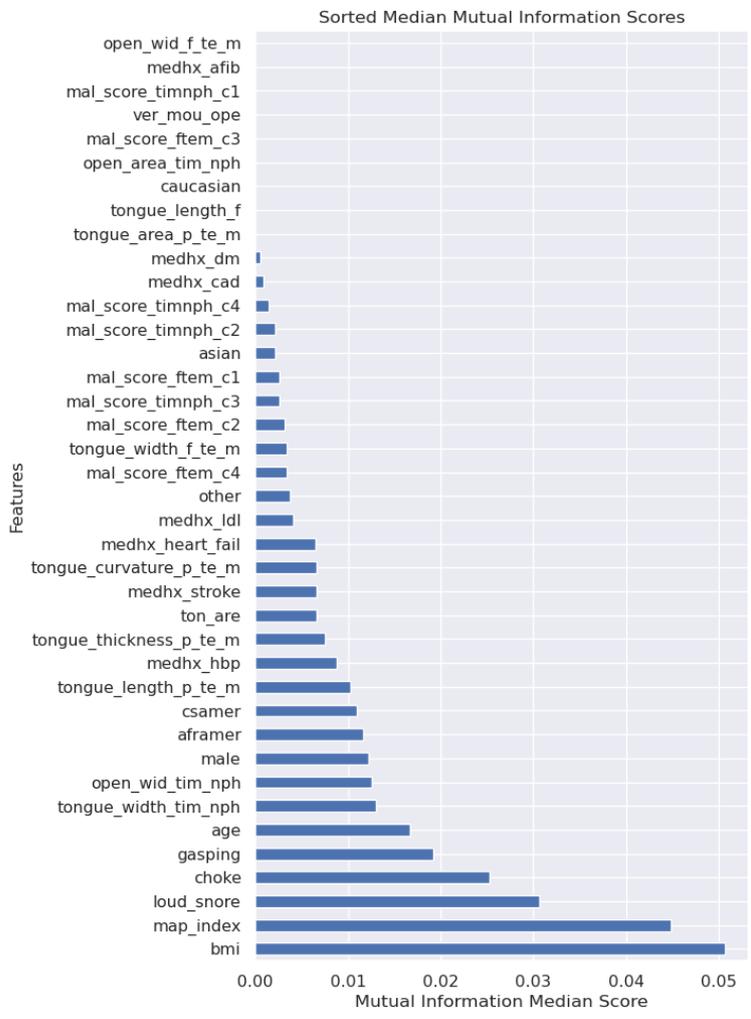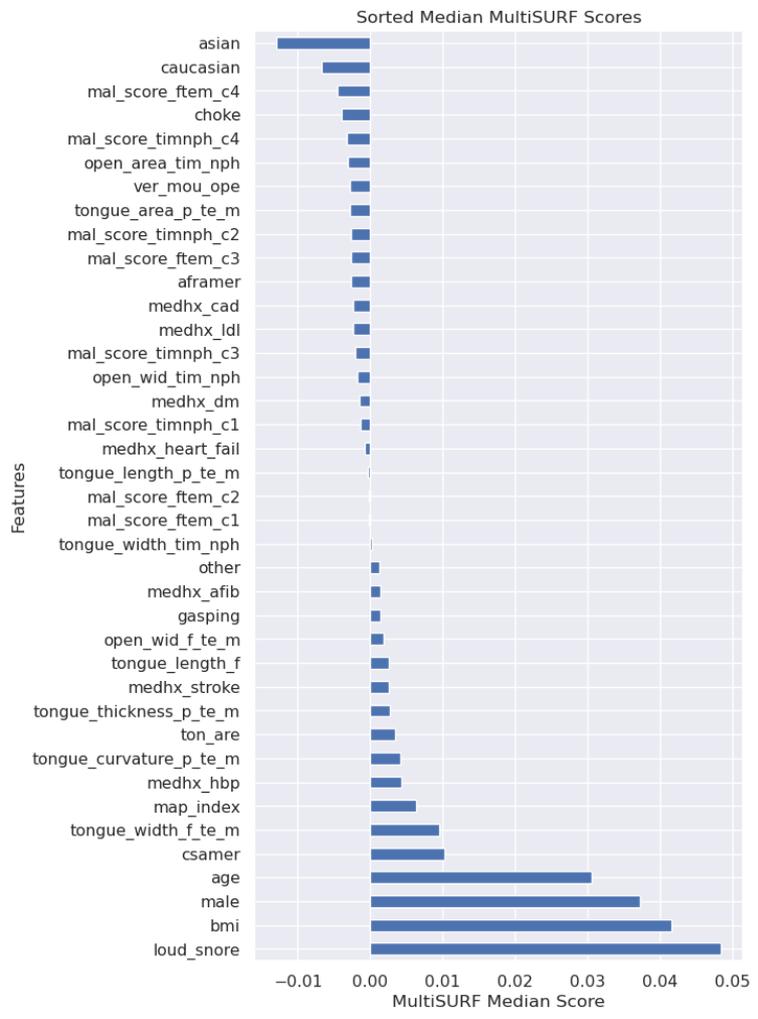

## Composite Feature Importance Plot (Normalized and Performance Weighted)

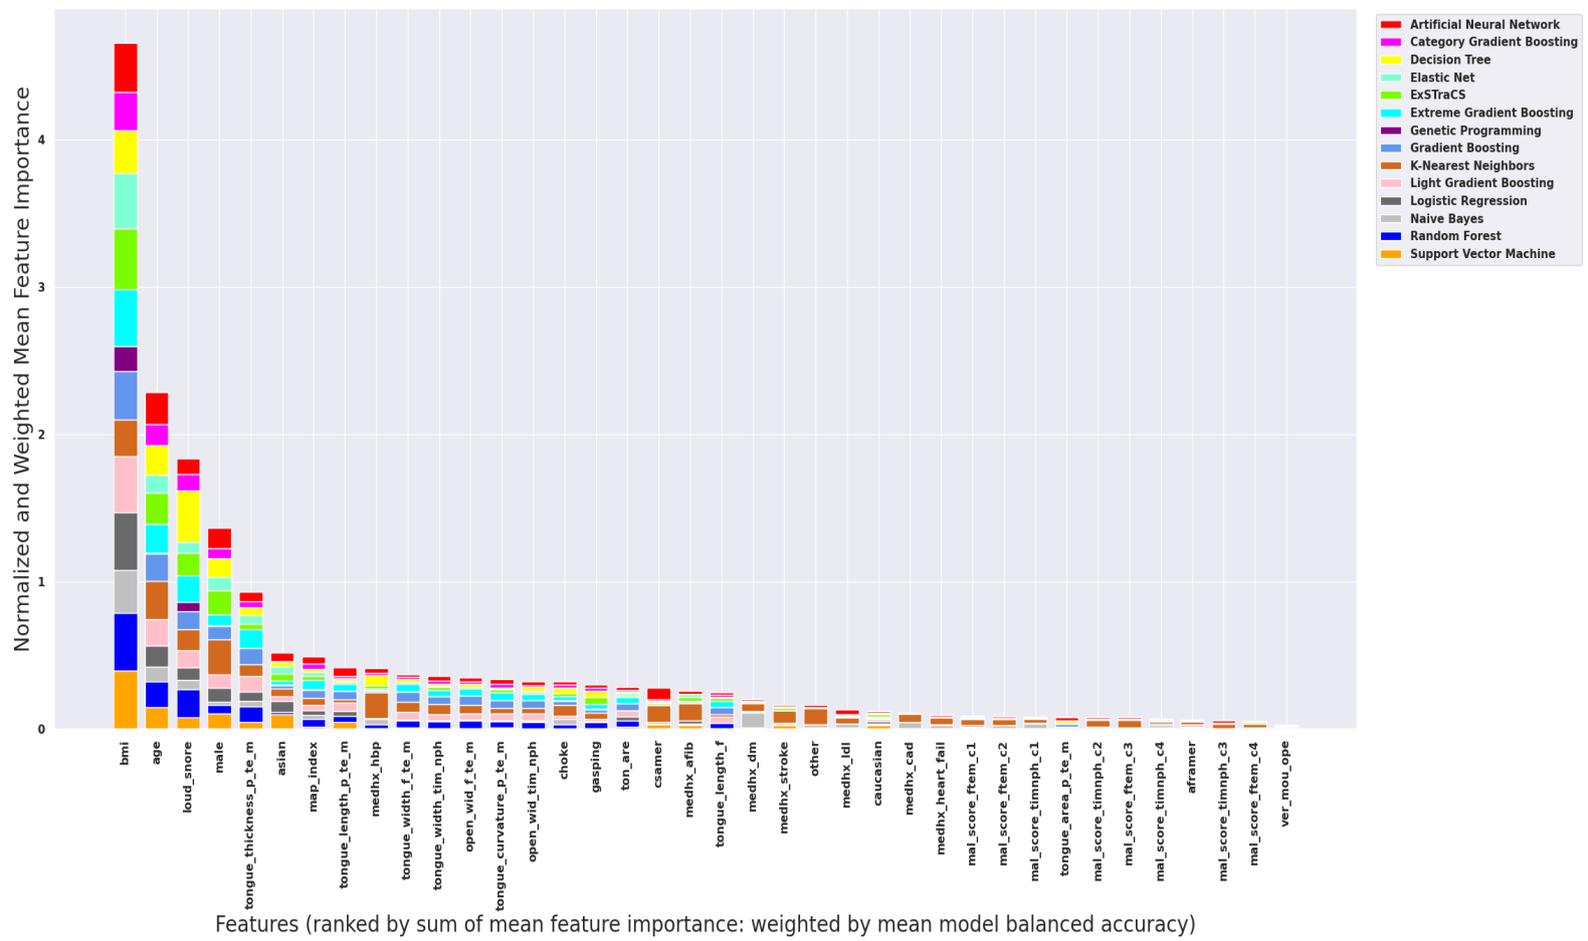

# Feature Importance Summary: D20 = T\_GE5\_DEMDXSYMCFIO

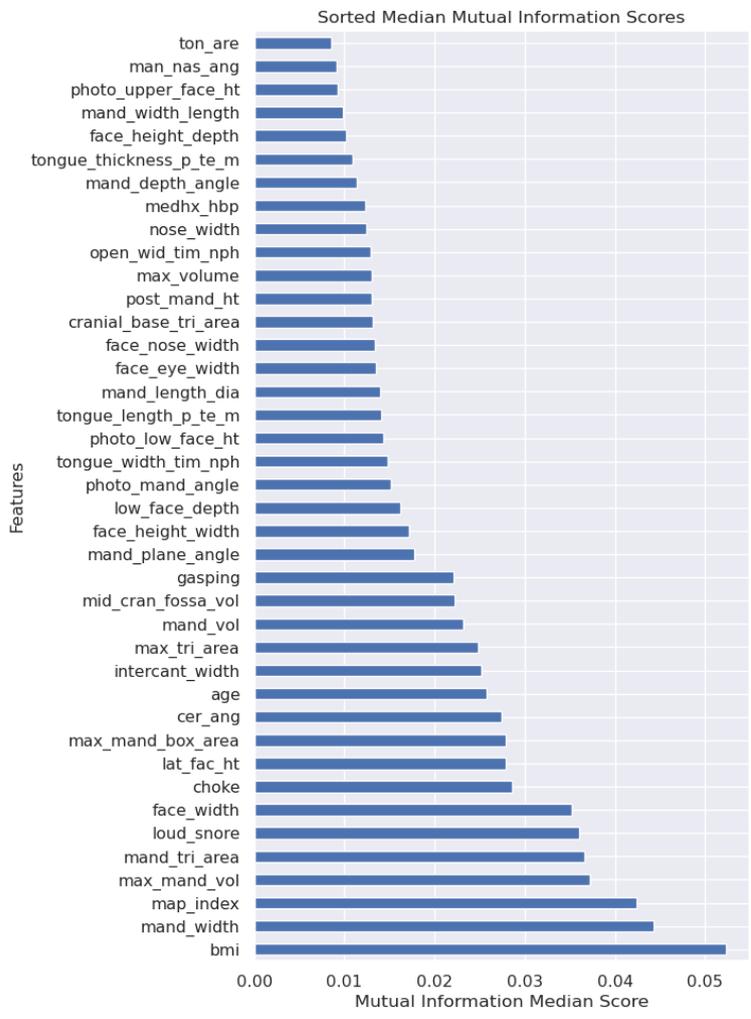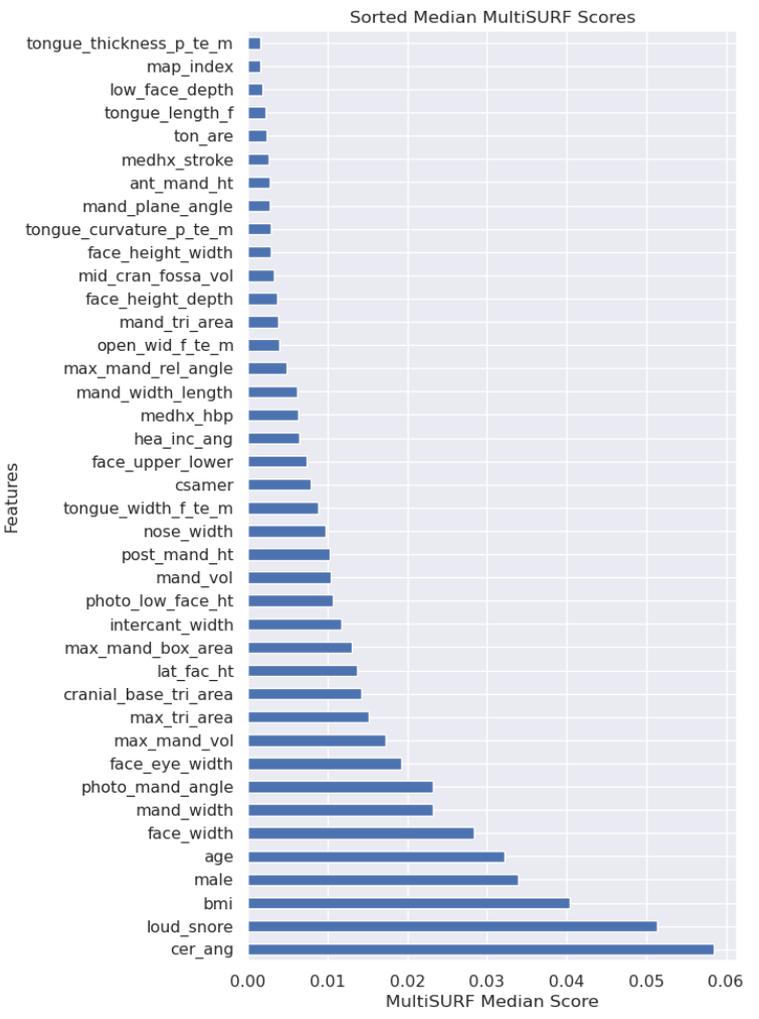

## Composite Feature Importance Plot (Normalized and Performance Weighted)

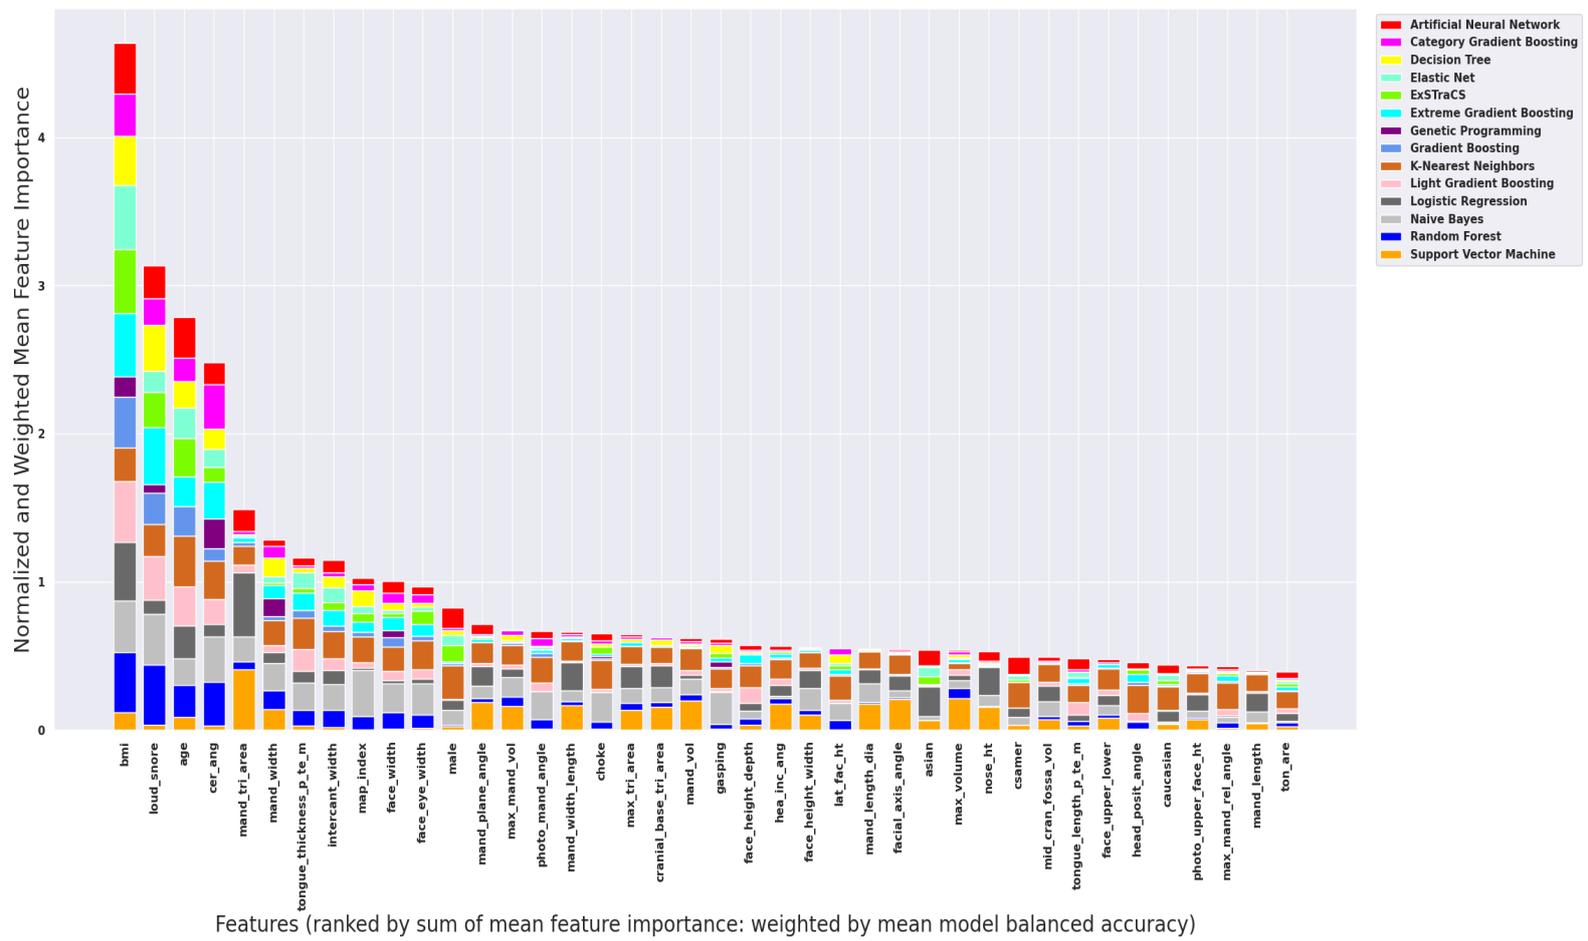

# Compare ML Performance Across Datasets

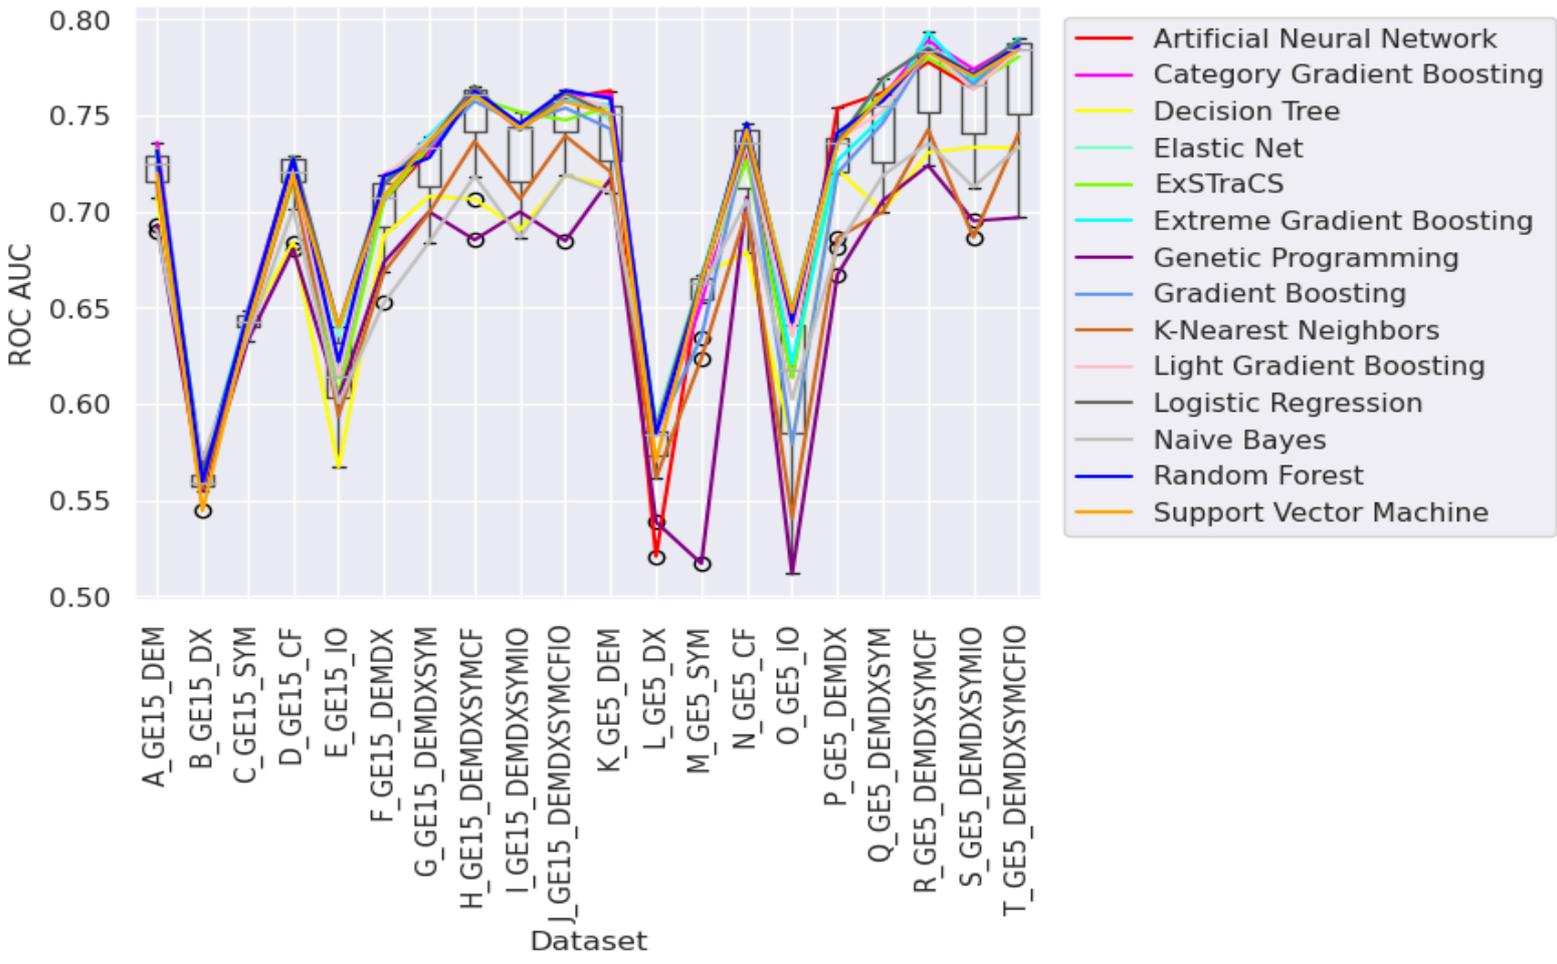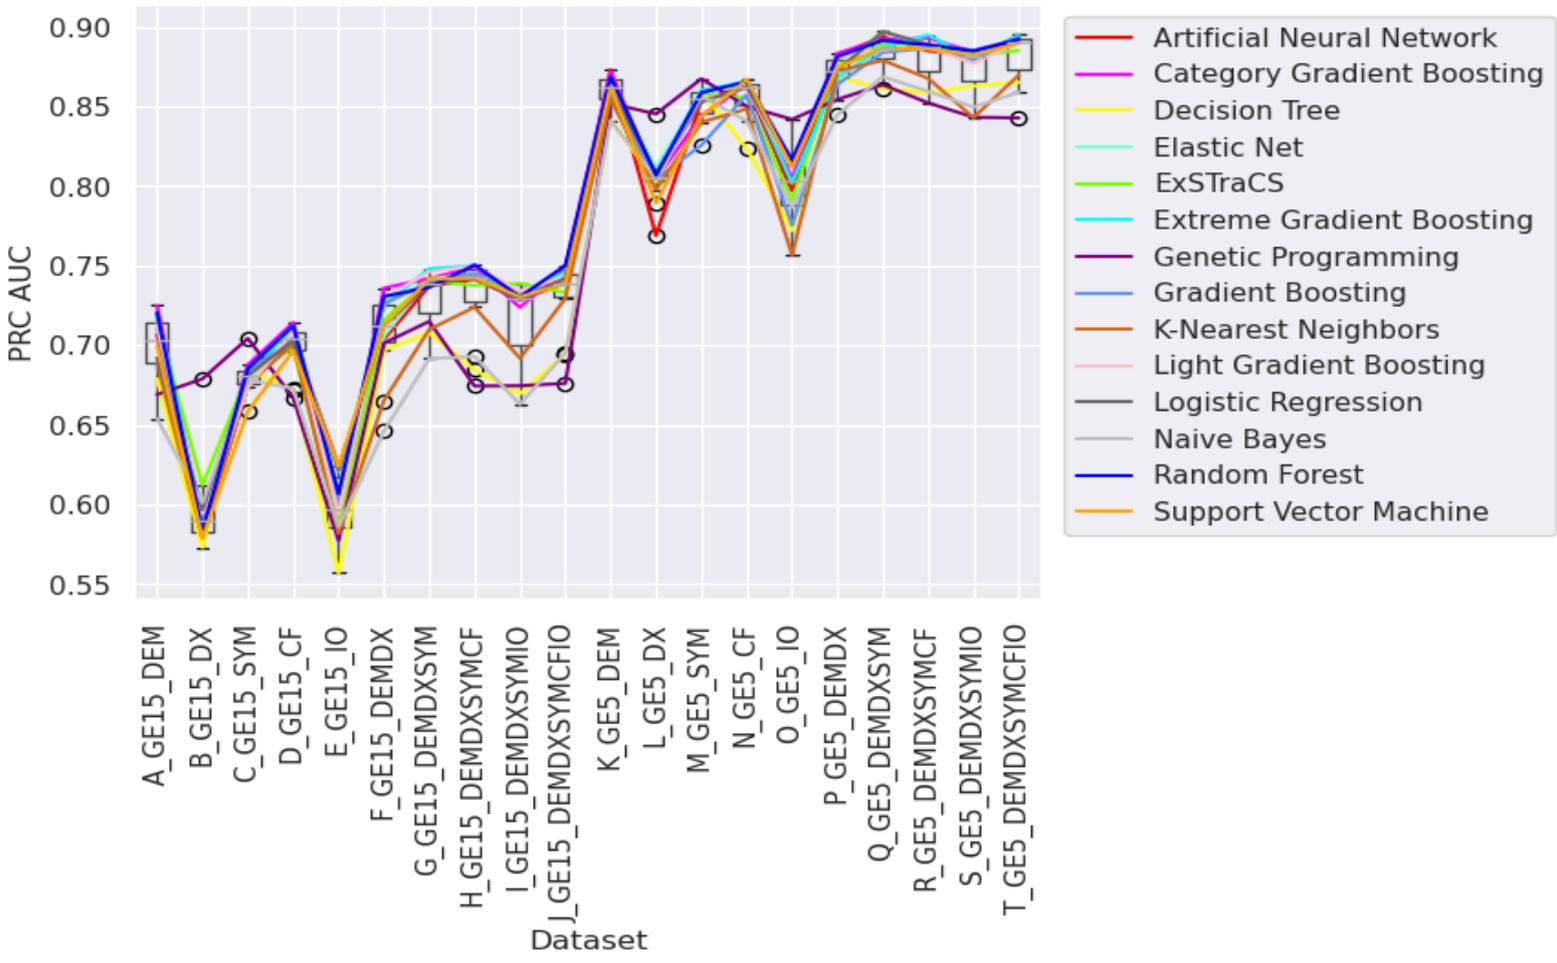

# Using Best Performing Algorithms (Kruskall Wallis Compare Datasets): Page 1

| Metrics              | P-Value | Best Alg D1                | Median D1 | Best Alg D2               | Median D2 | Best Alg D3                | Median D3 |
|----------------------|---------|----------------------------|-----------|---------------------------|-----------|----------------------------|-----------|
| Balanced Accuracy    | 0.0     | Category Gradient Boosting | 0.6749    | Genetic Programming       | 0.5588    | Light Gradient Boosting    | 0.6238    |
| Accuracy             | 0.0     | Category Gradient Boosting | 0.6751    | Extreme Gradient Boosting | 0.5559    | Artificial Neural Network  | 0.6215    |
| F1 Score             | 0.0     | Support Vector Machine     | 0.6797    | Extreme Gradient Boosting | 0.5891    | Gradient Boosting          | 0.6352    |
| Sensitivity (Recall) | 0.0     | ExSTraCS                   | 0.7315    | Extreme Gradient Boosting | 0.5737    | K-Nearest Neighbors        | 0.6178    |
| Specificity          | 0.0     | Extreme Gradient Boosting  | 0.6727    | K-Nearest Neighbors       | 0.7381    | ExSTraCS                   | 0.7603    |
| Precision (PPV)      | 0.0     | Category Gradient Boosting | 0.6652    | K-Nearest Neighbors       | 0.604     | ExSTraCS                   | 0.6742    |
| TP                   | 0.0     | ExSTraCS                   | 79.0      | Extreme Gradient Boosting | 54.5      | Category Gradient Boosting | 59.0      |
| TN                   | 0.0     | Extreme Gradient Boosting  | 74.0      | K-Nearest Neighbors       | 62.0      | ExSTraCS                   | 65.0      |
| FP                   | 0.0     | Support Vector Machine     | 44.5      | ExSTraCS                  | 40.0      | Elastic Net                | 36.0      |
| FN                   | 0.0     | Genetic Programming        | 38.0      | K-Nearest Neighbors       | 60.5      | ExSTraCS                   | 55.5      |
| NPV                  | 0.0     | Support Vector Machine     | 0.6901    | Naive Bayes               | 0.533     | Artificial Neural Network  | 0.5967    |
| LR+                  | 0.0     | Category Gradient Boosting | 2.0052    | K-Nearest Neighbors       | 1.3423    | ExSTraCS                   | 1.8553    |
| LR-                  | 0.0     | Genetic Programming        | 0.5665    | K-Nearest Neighbors       | 0.9432    | ExSTraCS                   | 0.7543    |
| ROC AUC              | 0.0     | ExSTraCS                   | 0.7387    | Light Gradient Boosting   | 0.5616    | Gradient Boosting          | 0.66      |
| PRC AUC              | 0.0     | Category Gradient Boosting | 0.7269    | Genetic Programming       | 0.6781    | Genetic Programming        | 0.7085    |
| PRC APS              | 0.0     | Category Gradient Boosting | 0.729     | Decision Tree             | 0.575     | Extreme Gradient Boosting  | 0.6749    |

| Metrics              | P-Value | Best Alg D4                | Median D4 | Best Alg D5            | Median D5 | Best Alg D6                | Median D6 |
|----------------------|---------|----------------------------|-----------|------------------------|-----------|----------------------------|-----------|
| Balanced Accuracy    | 0.0     | Logistic Regression        | 0.6784    | Logistic Regression    | 0.6017    | Extreme Gradient Boosting  | 0.662     |
| Accuracy             | 0.0     | Logistic Regression        | 0.6782    | Logistic Regression    | 0.6019    | Extreme Gradient Boosting  | 0.6657    |
| F1 Score             | 0.0     | Logistic Regression        | 0.679     | Naive Bayes            | 0.6022    | Extreme Gradient Boosting  | 0.7027    |
| Sensitivity (Recall) | 0.0     | Artificial Neural Network  | 0.6991    | Naive Bayes            | 0.6238    | Gradient Boosting          | 0.7448    |
| Specificity          | 0.0     | Category Gradient Boosting | 0.7078    | K-Nearest Neighbors    | 0.6468    | ExSTraCS                   | 0.6235    |
| Precision (PPV)      | 0.0     | Category Gradient Boosting | 0.6761    | Logistic Regression    | 0.5934    | Extreme Gradient Boosting  | 0.6714    |
| TP                   | 0.0     | Artificial Neural Network  | 75.5      | Naive Bayes            | 65.5      | Gradient Boosting          | 71.5      |
| TN                   | 0.0     | Category Gradient Boosting | 77.5      | K-Nearest Neighbors    | 70.5      | ExSTraCS                   | 53.0      |
| FP                   | 0.0     | Decision Tree              | 42.5      | Decision Tree          | 50.0      | Category Gradient Boosting | 41.0      |
| FN                   | 0.0     | Naive Bayes                | 43.0      | K-Nearest Neighbors    | 54.5      | ExSTraCS                   | 32.0      |
| NPV                  | 0.0     | Elastic Net                | 0.6862    | Logistic Regression    | 0.6122    | Extreme Gradient Boosting  | 0.6665    |
| LR+                  | 0.0     | Category Gradient Boosting | 2.1067    | Logistic Regression    | 1.5228    | Extreme Gradient Boosting  | 1.8099    |
| LR-                  | 0.0     | Genetic Programming        | 0.6084    | Decision Tree          | 0.8035    | Naive Bayes                | 0.5876    |
| ROC AUC              | 0.0     | Random Forest              | 0.7343    | Support Vector Machine | 0.6405    | Light Gradient Boosting    | 0.7205    |
| PRC AUC              | 0.0     | Extreme Gradient Boosting  | 0.7196    | Elastic Net            | 0.626     | Random Forest              | 0.7359    |
| PRC APS              | 0.0     | Extreme Gradient Boosting  | 0.7218    | Elastic Net            | 0.6292    | Random Forest              | 0.7393    |

| Metrics              | P-Value | Best Alg D7             | Median D7 | Best Alg D8                | Median D8 | Best Alg D9               | Median D9 |
|----------------------|---------|-------------------------|-----------|----------------------------|-----------|---------------------------|-----------|
| Balanced Accuracy    | 0.0     | ExSTraCS                | 0.6908    | ExSTraCS                   | 0.6943    | ExSTraCS                  | 0.6855    |
| Accuracy             | 0.0     | Gradient Boosting       | 0.6921    | ExSTraCS                   | 0.6942    | Elastic Net               | 0.6852    |
| F1 Score             | 0.0     | Gradient Boosting       | 0.719     | ExSTraCS                   | 0.7032    | ExSTraCS                  | 0.6922    |
| Sensitivity (Recall) | 0.0     | Support Vector Machine  | 0.768     | ExSTraCS                   | 0.7407    | ExSTraCS                  | 0.729     |
| Specificity          | 0.0     | Naive Bayes             | 0.6437    | K-Nearest Neighbors        | 0.7182    | Naive Bayes               | 0.6972    |
| Precision (PPV)      | 0.0     | Light Gradient Boosting | 0.6848    | Artificial Neural Network  | 0.6867    | Elastic Net               | 0.6748    |
| TP                   | 0.0     | Support Vector Machine  | 74.5      | ExSTraCS                   | 80.0      | ExSTraCS                  | 78.0      |
| TN                   | 0.0     | Naive Bayes             | 56.0      | K-Nearest Neighbors        | 79.0      | Naive Bayes               | 76.0      |
| FP                   | 0.0     | K-Nearest Neighbors     | 38.0      | Decision Tree              | 40.0      | Decision Tree             | 41.0      |
| FN                   | 0.0     | Naive Bayes             | 37.5      | K-Nearest Neighbors        | 40.0      | Naive Bayes               | 48.5      |
| NPV                  | 0.0     | Gradient Boosting       | 0.6912    | ExSTraCS                   | 0.7172    | ExSTraCS                  | 0.6991    |
| LR+                  | 0.0     | Gradient Boosting       | 1.9539    | Artificial Neural Network  | 2.2363    | Extreme Gradient Boosting | 2.1084    |
| LR-                  | 0.0     | Naive Bayes             | 0.6089    | Genetic Programming        | 0.556     | Naive Bayes               | 0.6738    |
| ROC AUC              | 0.0     | Light Gradient Boosting | 0.7421    | Artificial Neural Network  | 0.7668    | Light Gradient Boosting   | 0.7554    |
| PRC AUC              | 0.0     | Light Gradient Boosting | 0.7499    | Category Gradient Boosting | 0.7525    | Extreme Gradient Boosting | 0.7326    |
| PRC APS              | 0.0     | Light Gradient Boosting | 0.7518    | Category Gradient Boosting | 0.7545    | Extreme Gradient Boosting | 0.7344    |

| Metrics              | P-Value | Best Alg D10               | Median D10 | Best Alg D11               | Median D11 | Best Alg D12               | Median D12 |
|----------------------|---------|----------------------------|------------|----------------------------|------------|----------------------------|------------|
| Balanced Accuracy    | 0.0     | Category Gradient Boosting | 0.6929     | Extreme Gradient Boosting  | 0.7028     | Extreme Gradient Boosting  | 0.5796     |
| Accuracy             | 0.0     | Category Gradient Boosting | 0.6927     | Artificial Neural Network  | 0.7834     | Category Gradient Boosting | 0.75       |
| F1 Score             | 0.0     | Category Gradient Boosting | 0.6985     | Artificial Neural Network  | 0.8638     | Category Gradient Boosting | 0.8571     |
| Sensitivity (Recall) | 0.0     | ExSTraCS                   | 0.7222     | Artificial Neural Network  | 0.949      | Category Gradient Boosting | 1.0        |
| Specificity          | 0.0     | K-Nearest Neighbors        | 0.7227     | Elastic Net                | 0.6943     | Elastic Net                | 0.6629     |
| Precision (PPV)      | 0.0     | Category Gradient Boosting | 0.6917     | Elastic Net                | 0.8511     | Logistic Regression        | 0.8149     |
| TP                   | 0.0     | ExSTraCS                   | 78.0       | Artificial Neural Network  | 149.0      | Category Gradient Boosting | 135.0      |
| TN                   | 0.0     | K-Nearest Neighbors        | 79.5       | Elastic Net                | 42.0       | Elastic Net                | 29.5       |
| FP                   | 0.0     | Decision Tree              | 41.0       | Category Gradient Boosting | 40.0       | Genetic Programming        | 45.0       |
| FN                   | 0.0     | Genetic Programming        | 43.0       | Elastic Net                | 50.0       | Elastic Net                | 67.5       |
| NPV                  | 0.0     | Category Gradient Boosting | 0.7047     | Artificial Neural Network  | 0.7225     | Light Gradient Boosting    | 0.3087     |
| LR+                  | 0.0     | Category Gradient Boosting | 2.2849     | Elastic Net                | 2.1868     | Logistic Regression        | 1.4673     |
| LR-                  | 0.0     | Genetic Programming        | 0.6011     | Logistic Regression        | 0.4794     | Artificial Neural Network  | 0.7984     |
| ROC AUC              | 0.0     | Artificial Neural Network  | 0.7608     | Random Forest              | 0.7684     | Light Gradient Boosting    | 0.5846     |
| PRC AUC              | 0.0     | Random Forest              | 0.7564     | Category Gradient Boosting | 0.8732     | Genetic Programming        | 0.8386     |
| PRC APS              | 0.0     | Random Forest              | 0.7585     | Category Gradient Boosting | 0.8741     | Decision Tree              | 0.7942     |

| Metrics              | P-Value | Best Alg D13              | Median D13 | Best Alg D14               | Median D14 | Best Alg D15               | Median D15 |
|----------------------|---------|---------------------------|------------|----------------------------|------------|----------------------------|------------|
| Balanced Accuracy    | 0.0     | Extreme Gradient Boosting | 0.6546     | Extreme Gradient Boosting  | 0.6934     | Elastic Net                | 0.6122     |
| Accuracy             | 0.0     | Artificial Neural Network | 0.7527     | Gradient Boosting          | 0.7615     | Category Gradient Boosting | 0.719      |
| F1 Score             | 0.0     | Artificial Neural Network | 0.8589     | Category Gradient Boosting | 0.8494     | Category Gradient Boosting | 0.8365     |
| Sensitivity (Recall) | 0.0     | Artificial Neural Network | 1.0        | Category Gradient Boosting | 0.946      | Category Gradient Boosting | 1.0        |
| Specificity          | 0.0     | Decision Tree             | 0.6889     | Elastic Net                | 0.7131     | Elastic Net                | 0.625      |
| Precision (PPV)      | 0.0     | Decision Tree             | 0.8581     | Elastic Net                | 0.8521     | Elastic Net                | 0.7991     |
| TP                   | 0.0     | Artificial Neural Network | 137.0      | Category Gradient Boosting | 149.0      | Category Gradient Boosting | 153.0      |
| TN                   | 0.0     | Decision Tree             | 31.0       | Elastic Net                | 43.5       | Elastic Net                | 37.5       |
| FP                   | 0.0     | Artificial Neural Network | 45.0       | Genetic Programming        | 46.5       | Category Gradient Boosting | 60.0       |
| FN                   | 0.0     | Decision Tree             | 55.5       | Naive Bayes                | 56.5       | Decision Tree              | 66.5       |
| NPV                  | 0.0     | Logistic Regression       | 0.3774     | Category Gradient Boosting | 0.6629     | Artificial Neural Network  | 0.45       |
| LR+                  | 0.0     | Decision Tree             | 1.9882     | Elastic Net                | 2.2404     | Elastic Net                | 1.5601     |
| LR-                  | 0.0     | K-Nearest Neighbors       | 0.6898     | Decision Tree              | 0.5789     | Decision Tree              | 0.7855     |
| ROC AUC              | 0.0     | Elastic Net               | 0.6796     | Extreme Gradient Boosting  | 0.7673     | Random Forest              | 0.6538     |
| PRC AUC              | 0.0     | Genetic Programming       | 0.8764     | Random Forest              | 0.8753     | Genetic Programming        | 0.8592     |
| PRC APS              | 0.0     | Light Gradient Boosting   | 0.8495     | Random Forest              | 0.8769     | Random Forest              | 0.817      |

| Metrics              | P-Value | Best Alg D16               | Median D16 | Best Alg D17              | Median D17 | Best Alg D18               | Median D18 |
|----------------------|---------|----------------------------|------------|---------------------------|------------|----------------------------|------------|
| Balanced Accuracy    | 0.0     | Support Vector Machine     | 0.6885     | ExSTraCS                  | 0.6957     | ExSTraCS                   | 0.7187     |
| Accuracy             | 0.0     | Artificial Neural Network  | 0.7956     | Artificial Neural Network | 0.8016     | Category Gradient Boosting | 0.789      |
| F1 Score             | 0.0     | Artificial Neural Network  | 0.875      | Artificial Neural Network | 0.8781     | Category Gradient Boosting | 0.8686     |
| Sensitivity (Recall) | 0.0     | Genetic Programming        | 0.9485     | Artificial Neural Network | 0.942      | Category Gradient Boosting | 0.962      |
| Specificity          | 0.0     | Elastic Net                | 0.6667     | Support Vector Machine    | 0.6667     | Elastic Net                | 0.7049     |
| Precision (PPV)      | 0.0     | Elastic Net                | 0.8636     | Support Vector Machine    | 0.8703     | Elastic Net                | 0.8632     |
| TP                   | 0.0     | Genetic Programming        | 129.0      | Artificial Neural Network | 130.0      | Category Gradient Boosting | 152.0      |
| TN                   | 0.0     | Elastic Net                | 30.0       | Support Vector Machine    | 30.0       | Elastic Net                | 43.0       |
| FP                   | 0.0     | Genetic Programming        | 36.0       | Genetic Programming       | 33.5       | Genetic Programming        | 42.0       |
| FN                   | 0.0     | Decision Tree              | 46.5       | Decision Tree             | 46.5       | Naive Bayes                | 52.5       |
| NPV                  | 0.0     | Artificial Neural Network  | 0.6726     | Artificial Neural Network | 0.6809     | Category Gradient Boosting | 0.7596     |
| LR+                  | 0.0     | Elastic Net                | 2.095      | Support Vector Machine    | 2.1766     | Elastic Net                | 2.4391     |
| LR-                  | 0.0     | Decision Tree              | 0.5089     | Decision Tree             | 0.5316     | Naive Bayes                | 0.488      |
| ROC AUC              | 0.0     | Artificial Neural Network  | 0.7619     | Elastic Net               | 0.762      | Extreme Gradient Boosting  | 0.793      |
| PRC AUC              | 0.0     | Category Gradient Boosting | 0.8898     | Elastic Net               | 0.894      | Extreme Gradient Boosting  | 0.8949     |
| PRC APS              | 0.0     | Category Gradient Boosting | 0.8913     | Elastic Net               | 0.8952     | Extreme Gradient Boosting  | 0.8957     |

## Using Best Performing Algorithms (Kruskall Wallis Compare Datasets): Page 2

| Metrics              | P-Value | Best Alg_D19               | Median_D19 | Best Alg_D20               | Median_D20 |
|----------------------|---------|----------------------------|------------|----------------------------|------------|
| Balanced Accuracy    | 0.0     | ExSTraCS                   | 0.7094     | Elastic Net                | 0.7189     |
| Accuracy             | 0.0     | Artificial Neural Network  | 0.7765     | Category Gradient Boosting | 0.7936     |
| F1 Score             | 0.0     | Category Gradient Boosting | 0.8612     | Category Gradient Boosting | 0.8714     |
| Sensitivity (Recall) | 0.0     | Category Gradient Boosting | 0.9618     | Category Gradient Boosting | 0.9651     |
| Specificity          | 0.0     | Logistic Regression        | 0.6833     | Logistic Regression        | 0.7049     |
| Precision (PPV)      | 0.0     | Logistic Regression        | 0.8571     | Logistic Regression        | 0.8645     |
| TP                   | 0.0     | Category Gradient Boosting | 151.0      | Category Gradient Boosting | 152.0      |
| TN                   | 0.0     | Logistic Regression        | 41.0       | Logistic Regression        | 43.0       |
| FP                   | 0.0     | Category Gradient Boosting | 42.5       | Genetic Programming        | 43.0       |
| FN                   | 0.0     | Naive Bayes                | 52.0       | Naive Bayes                | 55.0       |
| NPV                  | 0.0     | Category Gradient Boosting | 0.735      | Category Gradient Boosting | 0.7894     |
| LR+                  | 0.0     | Logistic Regression        | 2.2992     | Logistic Regression        | 2.4896     |
| LR-                  | 0.0     | Naive Bayes                | 0.5018     | Naive Bayes                | 0.5078     |
| ROC AUC              | 0.0     | Category Gradient Boosting | 0.779      | Gradient Boosting          | 0.7929     |
| PRC AUC              | 0.0     | Support Vector Machine     | 0.8924     | Elastic Net                | 0.8966     |
| PRC APS              | 0.0     | Support Vector Machine     | 0.8929     | Elastic Net                | 0.8972     |

# Pipeline Runtime Summary: Page 1

## A\_GE15\_DEM

| Pipeline Component                      | Phase | Time (sec)         |
|-----------------------------------------|-------|--------------------|
| Exploratory Analysis                    | 1     | 2.736199140548706  |
| Scale and Impute                        | 2     | 0.5808000564575195 |
| Mutual Information (Feature Importance) | 3     | 0.6648447513580322 |
| MultiSURF (Feature Importance)          | 3     | 131.99613165855408 |
| Feature Selection                       | 4     | 0.7935709953308105 |
| Artificial Neural Network(Modeling)     | 5     | 3708.1571187973022 |
| Category Gradient Boosting(Modeling)    | 5     | 9529.533482789991  |
| Decision Tree(Modeling)                 | 5     | 25.564898252487183 |
| Elastic Net(Modeling)                   | 5     | 29.126837730407715 |
| ExSTraCS(Modeling)                      | 5     | 62569.96095848084  |
| Extreme Gradient Boosting(Modeling)     | 5     | 6398.502605438232  |
| Genetic Programming(Modeling)           | 5     | 10367.453958034515 |
| Gradient Boosting(Modeling)             | 5     | 4790.504416704178  |
| K-Nearest Neighbors(Modeling)           | 5     | 407.98421001434326 |
| Light Gradient Boosting(Modeling)       | 5     | 315.812863111496   |
| Logistic Regression(Modeling)           | 5     | 36.70223426818848  |
| Naive Bayes(Modeling)                   | 5     | 0.8935542106628418 |
| Random Forest(Modeling)                 | 5     | 6211.194876194     |
| Support Vector Machine(Modeling)        | 5     | 5699.444601774216  |
| Stats Summary                           | 6     | 27.12745213508606  |

## B\_GE15\_DX

| Pipeline Component                      | Phase | Time (sec)         |
|-----------------------------------------|-------|--------------------|
| Exploratory Analysis                    | 1     | 2.4778053760528564 |
| Scale and Impute                        | 2     | 0.7988710403442383 |
| Mutual Information (Feature Importance) | 3     | 0.5441083908081055 |
| MultiSURF (Feature Importance)          | 3     | 70.17340803146362  |
| Feature Selection                       | 4     | 0.8237946033477783 |
| Artificial Neural Network(Modeling)     | 5     | 1329.291328907013  |
| Category Gradient Boosting(Modeling)    | 5     | 9363.329277515411  |
| Decision Tree(Modeling)                 | 5     | 21.403674602508545 |
| Elastic Net(Modeling)                   | 5     | 28.816012620925903 |
| ExSTraCS(Modeling)                      | 5     | 17781.627497911453 |
| Extreme Gradient Boosting(Modeling)     | 5     | 5056.750956058502  |
| Genetic Programming(Modeling)           | 5     | 11580.340677022934 |
| Gradient Boosting(Modeling)             | 5     | 2102.121607065201  |
| K-Nearest Neighbors(Modeling)           | 5     | 474.8917410373688  |
| Light Gradient Boosting(Modeling)       | 5     | 505.1450881958008  |
| Logistic Regression(Modeling)           | 5     | 33.89331293106079  |
| Naive Bayes(Modeling)                   | 5     | 0.7515935897827148 |
| Random Forest(Modeling)                 | 5     | 3916.4958379268646 |
| Support Vector Machine(Modeling)        | 5     | 10139.609081745148 |
| Stats Summary                           | 6     | 27.251802682876587 |

## C\_GE15\_SYM

| Pipeline Component                      | Phase | Time (sec)         |
|-----------------------------------------|-------|--------------------|
| Exploratory Analysis                    | 1     | 2.351451873779297  |
| Scale and Impute                        | 2     | 0.714827299118042  |
| Mutual Information (Feature Importance) | 3     | 0.3655650615692138 |
| MultiSURF (Feature Importance)          | 3     | 59.95705556869507  |
| Feature Selection                       | 4     | 0.723142147064209  |
| Artificial Neural Network(Modeling)     | 5     | 1991.5963234901428 |
| Category Gradient Boosting(Modeling)    | 5     | 9463.100090026855  |
| Decision Tree(Modeling)                 | 5     | 23.38175940513611  |
| Elastic Net(Modeling)                   | 5     | 27.0253484249115   |
| ExSTraCS(Modeling)                      | 5     | 49164.19173336029  |
| Extreme Gradient Boosting(Modeling)     | 5     | 5568.8841145038605 |
| Genetic Programming(Modeling)           | 5     | 12134.772771120071 |
| Gradient Boosting(Modeling)             | 5     | 2973.687061786652  |
| K-Nearest Neighbors(Modeling)           | 5     | 305.31446862220764 |
| Light Gradient Boosting(Modeling)       | 5     | 262.7659912109375  |
| Logistic Regression(Modeling)           | 5     | 36.314871311187744 |
| Naive Bayes(Modeling)                   | 5     | 0.6484284400939941 |
| Random Forest(Modeling)                 | 5     | 5074.207618713379  |
| Support Vector Machine(Modeling)        | 5     | 8911.37706041336   |
| Stats Summary                           | 6     | 27.942686796188354 |

## D\_GE15\_CF

| Pipeline Component                      | Phase | Time (sec)         |
|-----------------------------------------|-------|--------------------|
| Exploratory Analysis                    | 1     | 9.99558973312378   |
| Scale and Impute                        | 2     | 63.53515529632568  |
| Mutual Information (Feature Importance) | 3     | 3.200991630554199  |
| MultiSURF (Feature Importance)          | 3     | 794.5921676158905  |
| Feature Selection                       | 4     | 1.740147352218628  |
| Artificial Neural Network(Modeling)     | 5     | 6443.804703950882  |
| Category Gradient Boosting(Modeling)    | 5     | 13429.509245872498 |
| Decision Tree(Modeling)                 | 5     | 54.54532337188721  |
| Elastic Net(Modeling)                   | 5     | 69.70918607711792  |
| ExSTraCS(Modeling)                      | 5     | 108419.95375442503 |
| Extreme Gradient Boosting(Modeling)     | 5     | 9288.579190969467  |
| Genetic Programming(Modeling)           | 5     | 13149.608915805817 |
| Gradient Boosting(Modeling)             | 5     | 9539.089315891266  |
| K-Nearest Neighbors(Modeling)           | 5     | 22244.26331615448  |
| Light Gradient Boosting(Modeling)       | 5     | 584.0369462966919  |
| Logistic Regression(Modeling)           | 5     | 324.0871162414551  |
| Naive Bayes(Modeling)                   | 5     | 5.151625156402588  |
| Random Forest(Modeling)                 | 5     | 9344.169716835022  |
| Support Vector Machine(Modeling)        | 5     | 11340.881962060928 |
| Stats Summary                           | 6     | 38.16250395774841  |

## E\_GE15\_IO

| Pipeline Component                      | Phase | Time (sec)         |
|-----------------------------------------|-------|--------------------|
| Exploratory Analysis                    | 1     | 4.113210678100586  |
| Scale and Impute                        | 2     | 12.957643985748293 |
| Mutual Information (Feature Importance) | 3     | 1.4939005374908447 |
| MultiSURF (Feature Importance)          | 3     | 392.2613925933838  |
| Feature Selection                       | 4     | 1.1527338027954102 |
| Artificial Neural Network(Modeling)     | 5     | 3296.1173374652863 |
| Category Gradient Boosting(Modeling)    | 5     | 11171.047201156616 |
| Decision Tree(Modeling)                 | 5     | 50.97388195991516  |
| Elastic Net(Modeling)                   | 5     | 44.032020568847656 |
| ExSTraCS(Modeling)                      | 5     | 89819.82364273071  |
| Extreme Gradient Boosting(Modeling)     | 5     | 8705.768526792526  |
| Genetic Programming(Modeling)           | 5     | 13250.99503350258  |
| Gradient Boosting(Modeling)             | 5     | 9168.55330491066   |
| K-Nearest Neighbors(Modeling)           | 5     | 4746.95511507988   |
| Light Gradient Boosting(Modeling)       | 5     | 542.7813186645508  |
| Logistic Regression(Modeling)           | 5     | 67.07617092132568  |
| Naive Bayes(Modeling)                   | 5     | 2.3079776763916016 |
| Random Forest(Modeling)                 | 5     | 8648.693257570267  |
| Support Vector Machine(Modeling)        | 5     | 8395.923493146896  |
| Stats Summary                           | 6     | 33.0876841545105   |

## F\_GE15\_DEMDX

| Pipeline Component                      | Phase | Time (sec)         |
|-----------------------------------------|-------|--------------------|
| Exploratory Analysis                    | 1     | 3.2148666381835938 |
| Scale and Impute                        | 2     | 1.1499619483947754 |
| Mutual Information (Feature Importance) | 3     | 1.030620574951172  |
| MultiSURF (Feature Importance)          | 3     | 151.34648084640503 |
| Feature Selection                       | 4     | 0.981947422027588  |
| Artificial Neural Network(Modeling)     | 5     | 3088.033630132675  |
| Category Gradient Boosting(Modeling)    | 5     | 10721.229006767271 |
| Decision Tree(Modeling)                 | 5     | 29.826025253601078 |
| Elastic Net(Modeling)                   | 5     | 39.33396363258362  |
| ExSTraCS(Modeling)                      | 5     | 71628.76627469063  |
| Extreme Gradient Boosting(Modeling)     | 5     | 7321.496260881424  |
| Genetic Programming(Modeling)           | 5     | 12485.08402442932  |
| Gradient Boosting(Modeling)             | 5     | 5878.918683052063  |
| K-Nearest Neighbors(Modeling)           | 5     | 811.7625603675842  |
| Light Gradient Boosting(Modeling)       | 5     | 410.2245268821716  |
| Logistic Regression(Modeling)           | 5     | 45.56774830818176  |
| Naive Bayes(Modeling)                   | 5     | 1.6519339084625244 |
| Random Forest(Modeling)                 | 5     | 6634.867425441742  |
| Support Vector Machine(Modeling)        | 5     | 7776.370207071304  |
| Stats Summary                           | 6     | 29.264193773269653 |

## Pipeline Runtime Summary: Page 2

### G\_GE15\_DEMDXSYM

| Pipeline Component                      | Phase | Time (sec)         |
|-----------------------------------------|-------|--------------------|
| Exploratory Analysis                    | 1     | 3.666923761367798  |
| Scale and Impute                        | 2     | 1.6598670482635498 |
| Mutual Information (Feature Importance) | 3     | 1.2556984424591064 |
| MultiSURF (Feature Importance)          | 3     | 197.9333963394165  |
| Feature Selection                       | 4     | 0.978212833404541  |
| Artificial Neural Network(Modeling)     | 5     | 2790.062906265259  |
| Category Gradient Boosting(Modeling)    | 5     | 10453.57788991928  |
| Decision Tree(Modeling)                 | 5     | 31.939983129501343 |
| Elastic Net(Modeling)                   | 5     | 40.2475049495697   |
| ExSTraCS(Modeling)                      | 5     | 81166.38758635521  |
| Extreme Gradient Boosting(Modeling)     | 5     | 8492.647159814835  |
| Genetic Programming(Modeling)           | 5     | 12400.067398786545 |
| Gradient Boosting(Modeling)             | 5     | 5354.769142866135  |
| K-Nearest Neighbors(Modeling)           | 5     | 977.6632361412048  |
| Light Gradient Boosting(Modeling)       | 5     | 393.1347811222077  |
| Logistic Regression(Modeling)           | 5     | 47.08355379104614  |
| Naive Bayes(Modeling)                   | 5     | 1.9624443054199217 |
| Random Forest(Modeling)                 | 5     | 8702.394047260284  |
| Support Vector Machine(Modeling)        | 5     | 5557.184834480286  |
| Stats Summary                           | 6     | 30.378585815429688 |

### H\_GE15\_DEMDXSYMCF

| Pipeline Component                      | Phase | Time (sec)         |
|-----------------------------------------|-------|--------------------|
| Exploratory Analysis                    | 1     | 11.368979454040527 |
| Scale and Impute                        | 2     | 139.65527820587158 |
| Mutual Information (Feature Importance) | 3     | 4.421320915222168  |
| MultiSURF (Feature Importance)          | 3     | 1001.7658998966216 |
| Feature Selection                       | 4     | 2.0576705932617188 |
| Artificial Neural Network(Modeling)     | 5     | 6672.881328821182  |
| Category Gradient Boosting(Modeling)    | 5     | 12060.14352798462  |
| Decision Tree(Modeling)                 | 5     | 50.65711331367493  |
| Elastic Net(Modeling)                   | 5     | 118.44589257240295 |
| ExSTraCS(Modeling)                      | 5     | 122748.9160554409  |
| Extreme Gradient Boosting(Modeling)     | 5     | 9436.533944368362  |
| Genetic Programming(Modeling)           | 5     | 11935.05197095871  |
| Gradient Boosting(Modeling)             | 5     | 9531.837909460068  |
| K-Nearest Neighbors(Modeling)           | 5     | 2793.845855951309  |
| Light Gradient Boosting(Modeling)       | 5     | 1095.2793900966644 |
| Logistic Regression(Modeling)           | 5     | 430.2276036739349  |
| Naive Bayes(Modeling)                   | 5     | 9.56229305267334   |
| Random Forest(Modeling)                 | 5     | 9594.420408964155  |
| Support Vector Machine(Modeling)        | 5     | 19348.0153298378   |
| Stats Summary                           | 6     | 36.04674243927002  |

### I\_GE15\_DEMDXSYMIO

| Pipeline Component                      | Phase | Time (sec)         |
|-----------------------------------------|-------|--------------------|
| Exploratory Analysis                    | 1     | 6.940638780593872  |
| Scale and Impute                        | 2     | 37.81039762496948  |
| Mutual Information (Feature Importance) | 3     | 2.768164157867432  |
| MultiSURF (Feature Importance)          | 3     | 565.8541371822357  |
| Feature Selection                       | 4     | 1.780963897705078  |
| Artificial Neural Network(Modeling)     | 5     | 5102.498142004013  |
| Category Gradient Boosting(Modeling)    | 5     | 11476.19186925888  |
| Decision Tree(Modeling)                 | 5     | 57.67974519729614  |
| Elastic Net(Modeling)                   | 5     | 55.80314421653748  |
| ExSTraCS(Modeling)                      | 5     | 95548.56536316872  |
| Extreme Gradient Boosting(Modeling)     | 5     | 9121.256692409515  |
| Genetic Programming(Modeling)           | 5     | 11405.31778550148  |
| Gradient Boosting(Modeling)             | 5     | 9099.361944198608  |
| K-Nearest Neighbors(Modeling)           | 5     | 957.814840078354   |
| Light Gradient Boosting(Modeling)       | 5     | 676.647675037384   |
| Logistic Regression(Modeling)           | 5     | 65.81187224388123  |
| Naive Bayes(Modeling)                   | 5     | 4.252352476119995  |
| Random Forest(Modeling)                 | 5     | 8897.513707637787  |
| Support Vector Machine(Modeling)        | 5     | 12645.113326311111 |
| Stats Summary                           | 6     | 34.52153754234314  |

### J\_GE15\_DEMDXSYMCFIO

| Pipeline Component                      | Phase | Time (sec)         |
|-----------------------------------------|-------|--------------------|
| Exploratory Analysis                    | 1     | 12.391699314117432 |
| Scale and Impute                        | 2     | 245.2783389091492  |
| Mutual Information (Feature Importance) | 3     | 5.640100479125977  |
| MultiSURF (Feature Importance)          | 3     | 1285.842236995697  |
| Feature Selection                       | 4     | 2.444354772567749  |
| Artificial Neural Network(Modeling)     | 5     | 5793.202986001968  |
| Category Gradient Boosting(Modeling)    | 5     | 13200.718185901642 |
| Decision Tree(Modeling)                 | 5     | 72.8807852268219   |
| Elastic Net(Modeling)                   | 5     | 164.36100149154663 |
| ExSTraCS(Modeling)                      | 5     | 133321.0840716362  |
| Extreme Gradient Boosting(Modeling)     | 5     | 9844.894379377363  |
| Genetic Programming(Modeling)           | 5     | 12379.732833862305 |
| Gradient Boosting(Modeling)             | 5     | 9881.044662475586  |
| K-Nearest Neighbors(Modeling)           | 5     | 14668.23715686798  |
| Light Gradient Boosting(Modeling)       | 5     | 988.7148814201356  |
| Logistic Regression(Modeling)           | 5     | 536.0783994197845  |
| Naive Bayes(Modeling)                   | 5     | 12.585328578948976 |
| Random Forest(Modeling)                 | 5     | 10348.637086391447 |
| Support Vector Machine(Modeling)        | 5     | 18154.73348236084  |
| Stats Summary                           | 6     | 36.67437124252319  |

### K\_GE5\_DEM

| Pipeline Component                      | Phase | Time (sec)         |
|-----------------------------------------|-------|--------------------|
| Exploratory Analysis                    | 1     | 2.738342761993408  |
| Scale and Impute                        | 2     | 0.4294099807739258 |
| Mutual Information (Feature Importance) | 3     | 0.6721868515014648 |
| MultiSURF (Feature Importance)          | 3     | 131.19042897224426 |
| Feature Selection                       | 4     | 0.7913060188293457 |
| Artificial Neural Network(Modeling)     | 5     | 4479.830198526382  |
| Category Gradient Boosting(Modeling)    | 5     | 9313.724751710892  |
| Decision Tree(Modeling)                 | 5     | 30.51618504524231  |
| Elastic Net(Modeling)                   | 5     | 35.77742123603821  |
| ExSTraCS(Modeling)                      | 5     | 60222.08992314339  |
| Extreme Gradient Boosting(Modeling)     | 5     | 6381.247848033905  |
| Genetic Programming(Modeling)           | 5     | 11081.37850356102  |
| Gradient Boosting(Modeling)             | 5     | 5198.188378334045  |
| K-Nearest Neighbors(Modeling)           | 5     | 276.2680141925812  |
| Light Gradient Boosting(Modeling)       | 5     | 485.11595129966736 |
| Logistic Regression(Modeling)           | 5     | 40.2816436290741   |
| Naive Bayes(Modeling)                   | 5     | 1.05806565284729   |
| Random Forest(Modeling)                 | 5     | 5925.115648508072  |
| Support Vector Machine(Modeling)        | 5     | 5603.331168889999  |
| Stats Summary                           | 6     | 29.02877831459045  |

### L\_GE5\_DX

| Pipeline Component                      | Phase | Time (sec)         |
|-----------------------------------------|-------|--------------------|
| Exploratory Analysis                    | 1     | 2.2770259380340576 |
| Scale and Impute                        | 2     | 0.7675566673278809 |
| Mutual Information (Feature Importance) | 3     | 0.5571210384368896 |
| MultiSURF (Feature Importance)          | 3     | 68.36309742927551  |
| Feature Selection                       | 4     | 0.7683730125427246 |
| Artificial Neural Network(Modeling)     | 5     | 2019.4962491989136 |
| Category Gradient Boosting(Modeling)    | 5     | 9036.509687423706  |
| Decision Tree(Modeling)                 | 5     | 25.56378149986267  |
| Elastic Net(Modeling)                   | 5     | 31.36198902130127  |
| ExSTraCS(Modeling)                      | 5     | 24079.49163532257  |
| Extreme Gradient Boosting(Modeling)     | 5     | 6406.604341745377  |
| Genetic Programming(Modeling)           | 5     | 12644.980162858965 |
| Gradient Boosting(Modeling)             | 5     | 3010.084730863571  |
| K-Nearest Neighbors(Modeling)           | 5     | 351.2051818370819  |
| Light Gradient Boosting(Modeling)       | 5     | 663.7972512245178  |
| Logistic Regression(Modeling)           | 5     | 36.42190456390381  |
| Naive Bayes(Modeling)                   | 5     | 0.9104824066162108 |
| Random Forest(Modeling)                 | 5     | 4655.819127559662  |
| Support Vector Machine(Modeling)        | 5     | 7971.84702706337   |
| Stats Summary                           | 6     | 26.856804609298703 |

## Pipeline Runtime Summary: Page 3

### M\_GE5\_SYM

| Pipeline Component                      | Phase | Time (sec)         |
|-----------------------------------------|-------|--------------------|
| Exploratory Analysis                    | 1     | 2.299518585205078  |
| Scale and Impute                        | 2     | 0.7066469192504883 |
| Mutual Information (Feature Importance) | 3     | 0.4284877777099609 |
| MultiSURF (Feature Importance)          | 3     | 60.67499351501465  |
| Feature Selection                       | 4     | 0.6837139129638672 |
| Artificial Neural Network(Modeling)     | 5     | 3345.0420231819157 |
| Category Gradient Boosting(Modeling)    | 5     | 8599.303049087524  |
| Decision Tree(Modeling)                 | 5     | 25.2120578289032   |
| Elastic Net(Modeling)                   | 5     | 31.464089393615723 |
| ExSTraCS(Modeling)                      | 5     | 46537.3706407547   |
| Extreme Gradient Boosting(Modeling)     | 5     | 6045.448290348053  |
| Genetic Programming(Modeling)           | 5     | 12791.123330831528 |
| Gradient Boosting(Modeling)             | 5     | 4435.598383903503  |
| K-Nearest Neighbors(Modeling)           | 5     | 183.33197331428528 |
| Light Gradient Boosting(Modeling)       | 5     | 552.2008409500122  |
| Logistic Regression(Modeling)           | 5     | 39.161131381988525 |
| Naive Bayes(Modeling)                   | 5     | 0.7575957775115967 |
| Random Forest(Modeling)                 | 5     | 5721.906391382217  |
| Support Vector Machine(Modeling)        | 5     | 2305.4584381580357 |
| Stats Summary                           | 6     | 26.27703285217285  |

### N\_GE5\_CF

| Pipeline Component                      | Phase | Time (sec)         |
|-----------------------------------------|-------|--------------------|
| Exploratory Analysis                    | 1     | 8.499229669570923  |
| Scale and Impute                        | 2     | 22.49206113815308  |
| Mutual Information (Feature Importance) | 3     | 3.345311164855957  |
| MultiSURF (Feature Importance)          | 3     | 806.9920718669891  |
| Feature Selection                       | 4     | 2.0349338054656982 |
| Artificial Neural Network(Modeling)     | 5     | 7876.607294082642  |
| Category Gradient Boosting(Modeling)    | 5     | 14245.46318101883  |
| Decision Tree(Modeling)                 | 5     | 68.7890260219574   |
| Elastic Net(Modeling)                   | 5     | 73.82219696044922  |
| ExSTraCS(Modeling)                      | 5     | 106966.28651213646 |
| Extreme Gradient Boosting(Modeling)     | 5     | 9331.2950527668    |
| Genetic Programming(Modeling)           | 5     | 12417.905377149582 |
| Gradient Boosting(Modeling)             | 5     | 9849.24455165863   |
| K-Nearest Neighbors(Modeling)           | 5     | 26087.822072029117 |
| Light Gradient Boosting(Modeling)       | 5     | 1055.870061635971  |
| Logistic Regression(Modeling)           | 5     | 305.77005887031555 |
| Naive Bayes(Modeling)                   | 5     | 6.147997617721558  |
| Random Forest(Modeling)                 | 5     | 9434.799124002457  |
| Support Vector Machine(Modeling)        | 5     | 6841.207145929337  |
| Stats Summary                           | 6     | 35.944570779800415 |

### O\_GE5\_IO

| Pipeline Component                      | Phase | Time (sec)         |
|-----------------------------------------|-------|--------------------|
| Exploratory Analysis                    | 1     | 3.71018648147583   |
| Scale and Impute                        | 2     | 12.774019002914429 |
| Mutual Information (Feature Importance) | 3     | 1.5110681056976318 |
| MultiSURF (Feature Importance)          | 3     | 394.39750599861145 |
| Feature Selection                       | 4     | 1.1929571628570557 |
| Artificial Neural Network(Modeling)     | 5     | 5262.633613348007  |
| Category Gradient Boosting(Modeling)    | 5     | 10553.43864274025  |
| Decision Tree(Modeling)                 | 5     | 37.08332943916321  |
| Elastic Net(Modeling)                   | 5     | 45.09104990959168  |
| ExSTraCS(Modeling)                      | 5     | 79939.6334066391   |
| Extreme Gradient Boosting(Modeling)     | 5     | 7482.444770812988  |
| Genetic Programming(Modeling)           | 5     | 12619.506680488586 |
| Gradient Boosting(Modeling)             | 5     | 9240.272183418274  |
| K-Nearest Neighbors(Modeling)           | 5     | 1800.7040603160858 |
| Light Gradient Boosting(Modeling)       | 5     | 711.9019055366516  |
| Logistic Regression(Modeling)           | 5     | 52.352970123291016 |
| Naive Bayes(Modeling)                   | 5     | 2.097081184387207  |
| Random Forest(Modeling)                 | 5     | 8496.992241382599  |
| Support Vector Machine(Modeling)        | 5     | 14503.108617067335 |
| Stats Summary                           | 6     | 33.019352197647095 |

### P\_GE5\_DEMDX

| Pipeline Component                      | Phase | Time (sec)         |
|-----------------------------------------|-------|--------------------|
| Exploratory Analysis                    | 1     | 3.5429255962371826 |
| Scale and Impute                        | 2     | 1.0639572143554688 |
| Mutual Information (Feature Importance) | 3     | 0.9986371994018556 |
| MultiSURF (Feature Importance)          | 3     | 154.72269368171692 |
| Feature Selection                       | 4     | 0.9235823154449464 |
| Artificial Neural Network(Modeling)     | 5     | 3864.9913918972015 |
| Category Gradient Boosting(Modeling)    | 5     | 9520.709733009338  |
| Decision Tree(Modeling)                 | 5     | 32.978456020355225 |
| Elastic Net(Modeling)                   | 5     | 37.15324068069458  |
| ExSTraCS(Modeling)                      | 5     | 64373.92537951469  |
| Extreme Gradient Boosting(Modeling)     | 5     | 6819.847410440445  |
| Genetic Programming(Modeling)           | 5     | 11442.709577798843 |
| Gradient Boosting(Modeling)             | 5     | 7797.969977855682  |
| K-Nearest Neighbors(Modeling)           | 5     | 300.92607855796814 |
| Light Gradient Boosting(Modeling)       | 5     | 549.3834645748138  |
| Logistic Regression(Modeling)           | 5     | 57.23288059234619  |
| Naive Bayes(Modeling)                   | 5     | 1.524719476699829  |
| Random Forest(Modeling)                 | 5     | 6110.774478435516  |
| Support Vector Machine(Modeling)        | 5     | 5824.41738653183   |
| Stats Summary                           | 6     | 27.61832022666931  |

### Q\_GE5\_DEMDXSYM

| Pipeline Component                      | Phase | Time (sec)         |
|-----------------------------------------|-------|--------------------|
| Exploratory Analysis                    | 1     | 3.978061437606812  |
| Scale and Impute                        | 2     | 1.6132757663726809 |
| Mutual Information (Feature Importance) | 3     | 1.2964074611663818 |
| MultiSURF (Feature Importance)          | 3     | 201.34130096435547 |
| Feature Selection                       | 4     | 1.1063811779022217 |
| Artificial Neural Network(Modeling)     | 5     | 4687.17145895958   |
| Category Gradient Boosting(Modeling)    | 5     | 9558.452844142914  |
| Decision Tree(Modeling)                 | 5     | 34.67382097244263  |
| Elastic Net(Modeling)                   | 5     | 42.04599070549011  |
| ExSTraCS(Modeling)                      | 5     | 71456.9042096138   |
| Extreme Gradient Boosting(Modeling)     | 5     | 7875.315236091614  |
| Genetic Programming(Modeling)           | 5     | 11849.325545310974 |
| Gradient Boosting(Modeling)             | 5     | 6467.702733755112  |
| K-Nearest Neighbors(Modeling)           | 5     | 1321.207248210907  |
| Light Gradient Boosting(Modeling)       | 5     | 564.9719412326813  |
| Logistic Regression(Modeling)           | 5     | 51.067782402038574 |
| Naive Bayes(Modeling)                   | 5     | 2.084380626678467  |
| Random Forest(Modeling)                 | 5     | 6168.620606184006  |
| Support Vector Machine(Modeling)        | 5     | 5712.158212423325  |
| Stats Summary                           | 6     | 29.41591739654541  |

### R\_GE5\_DEMDXSYMCF

| Pipeline Component                      | Phase | Time (sec)         |
|-----------------------------------------|-------|--------------------|
| Exploratory Analysis                    | 1     | 11.319032430648804 |
| Scale and Impute                        | 2     | 54.96133041381836  |
| Mutual Information (Feature Importance) | 3     | 4.649731636047363  |
| MultiSURF (Feature Importance)          | 3     | 1021.7614789009094 |
| Feature Selection                       | 4     | 2.1531765460968018 |
| Artificial Neural Network(Modeling)     | 5     | 7238.746876239777  |
| Category Gradient Boosting(Modeling)    | 5     | 11713.577274084091 |
| Decision Tree(Modeling)                 | 5     | 105.3693528175354  |
| Elastic Net(Modeling)                   | 5     | 108.03834533691406 |
| ExSTraCS(Modeling)                      | 5     | 113557.26822257042 |
| Extreme Gradient Boosting(Modeling)     | 5     | 9361.169572353365  |
| Genetic Programming(Modeling)           | 5     | 12642.829085350037 |
| Gradient Boosting(Modeling)             | 5     | 9528.912678480148  |
| K-Nearest Neighbors(Modeling)           | 5     | 1980.5813300609589 |
| Light Gradient Boosting(Modeling)       | 5     | 1156.6040470600128 |
| Logistic Regression(Modeling)           | 5     | 325.7730679512024  |
| Naive Bayes(Modeling)                   | 5     | 9.47347092628479   |
| Random Forest(Modeling)                 | 5     | 9685.304824829102  |
| Support Vector Machine(Modeling)        | 5     | 11397.061574459076 |
| Stats Summary                           | 6     | 35.34916138648987  |

## Pipeline Runtime Summary: Page 4

### S\_GE5\_DEMDXSYMIO

| Pipeline Component                      | Phase | Time (sec)         |
|-----------------------------------------|-------|--------------------|
| Exploratory Analysis                    | 1     | 6.842856168746948  |
| Scale and Impute                        | 2     | 40.97619986534119  |
| Mutual Information (Feature Importance) | 3     | 2.7698090076446533 |
| MultiSURF (Feature Importance)          | 3     | 565.3565111160278  |
| Feature Selection                       | 4     | 1.704500675201416  |
| Artificial Neural Network(Modeling)     | 5     | 5933.380658626556  |
| Category Gradient Boosting(Modeling)    | 5     | 10789.813467741013 |
| Decision Tree(Modeling)                 | 5     | 68.80575776100159  |
| Elastic Net(Modeling)                   | 5     | 67.19651436805725  |
| ExSTraCS(Modeling)                      | 5     | 89347.71777367592  |
| Extreme Gradient Boosting(Modeling)     | 5     | 9241.673788785934  |
| Genetic Programming(Modeling)           | 5     | 10618.93819475174  |
| Gradient Boosting(Modeling)             | 5     | 9237.427114725111  |
| K-Nearest Neighbors(Modeling)           | 5     | 1122.401423454285  |
| Light Gradient Boosting(Modeling)       | 5     | 1015.3675396442412 |
| Logistic Regression(Modeling)           | 5     | 74.9745082852246   |
| Naive Bayes(Modeling)                   | 5     | 4.522921085357666  |
| Random Forest(Modeling)                 | 5     | 8625.576086044312  |
| Support Vector Machine(Modeling)        | 5     | 8549.789148807526  |
| Stats Summary                           | 6     | 37.79141807556152  |

### T\_GE5\_DEMDXSYMCFIO

| Pipeline Component                      | Phase | Time (sec)         |
|-----------------------------------------|-------|--------------------|
| Exploratory Analysis                    | 1     | 12.254991054534912 |
| Scale and Impute                        | 2     | 100.09028244018556 |
| Mutual Information (Feature Importance) | 3     | 6.65814995765686   |
| MultiSURF (Feature Importance)          | 3     | 1338.3030951023102 |
| Feature Selection                       | 4     | 3.347966432571411  |
| Artificial Neural Network(Modeling)     | 5     | 5848.371684074402  |
| Category Gradient Boosting(Modeling)    | 5     | 13419.847387075424 |
| Decision Tree(Modeling)                 | 5     | 66.41126346588135  |
| Elastic Net(Modeling)                   | 5     | 108.08236122131348 |
| ExSTraCS(Modeling)                      | 5     | 132024.3506913185  |
| Extreme Gradient Boosting(Modeling)     | 5     | 9537.53766298294   |
| Genetic Programming(Modeling)           | 5     | 12163.415115833282 |
| Gradient Boosting(Modeling)             | 5     | 9586.512859106064  |
| K-Nearest Neighbors(Modeling)           | 5     | 2716.985781431198  |
| Light Gradient Boosting(Modeling)       | 5     | 1236.759967803955  |
| Logistic Regression(Modeling)           | 5     | 908.5430879592896  |
| Naive Bayes(Modeling)                   | 5     | 9.7320396900177    |
| Random Forest(Modeling)                 | 5     | 10117.3725836277   |
| Support Vector Machine(Modeling)        | 5     | 21266.101005792618 |
| Stats Summary                           | 6     | 38.429627656936646 |
