# Supplementary material for: STREAMLINE: An Automated Machine Learning Pipeline for Biomedicine Applied to Examine the Utility of Photography-Based Phenotypes for OSA Prediction Across International Sleep Centers
Source: arXiv:2312.05461 ancillary file (2023-12-09)
Supplement: Supplementary file 7 [file xor_exp_STREAMLINE_Report.pdf]

# STREAMLINE Testing Data Evaluation Report: 2023-09-30 18:57:24.427470

## General Pipeline Settings:

CV Partitions: 10  
Partition Method: Stratified  
Categorical Cutoff: 2  
Statistical Significance Cutoff: 0.05  
Random Seed: 42  
Run From Notebook: False

## Feature Importance/Selection Settings:

Use Mutual Information: True  
Use MultiSURF: True  
Use TURF: False  
TURF Cutoff: 0.5  
MultiSURF Instance Subset: 2000  
Max Features to Keep: 2000  
Filter Poor Features: True  
Top Features to Display: 40  
Export Feature Importance Plot: True

## ML Modeling Algorithms:

Artificial Neural Network: True  
Category Gradient Boosting: True  
Decision Tree: True  
Elastic Net: True  
ExSTraCS: True  
Extreme Gradient Boosting: True  
Genetic Programming: True  
Gradient Boosting: True  
K-Nearest Neighbors: True  
Light Gradient Boosting: True  
Logistic Regression: True  
Naive Bayes: True  
Random Forest: True  
Support Vector Machine: True  
XCS: False  
eLCS: False

## Modeling Settings:

Primary Metric: balanced\_accuracy  
Training Subsample for KNN,ANN,SVM,and XGB: 0  
Uniform Feature Importance Estimation (Models): True  
Hyperparameter Sweep Number of Trials: 200  
Hyperparameter Timeout: 900  
Export Hyperparameter Sweep Plots: False

## LCS Settings (eLCS,XCS,ExSTraCS):

Do LCS Hyperparameter Sweep: False  
nu: 1  
Training Iterations: 200000  
N (Rule Population Size): 2000  
LCS Hyperparameter Sweep Timeout: 1200

## Stats and Figure Settings:

Export ROC Plot: True  
Export PRC Plot: True  
Export Metric Boxplots: True  
Export Feature Importance Boxplots: True  
Metric Weighting Composite FI Plots: balanced\_accuracy  
Top Model Features To Display: 40

## EDA and Processing Settings:

Engineering Missingness Cutoff: 0.5  
Cleaning Missingness Cutoff: 0.5  
Correlation Removal Threshold: 1.0  
List of Exploratory Analysis Ran: ['Describe', 'Univariate Analysis', 'Feature Correlation']  
List of Exploratory Plots Saved: ['Describe', 'Univariate Analysis', 'Feature Correlation']  
Use Data Scaling: True  
Use Data Imputation: True  
Use Multivariate Imputation: True  
Overwrite CV Datasets: True

## Target Dataset(s):

D1 = xor\_2\_a\_20s\_1600\_EDM-1\_01  
D2 = xor\_3\_a\_20s\_1600\_EDM-1\_01  
D3 = xor\_4\_a\_20s\_1600\_EDM-1\_01  
D4 = xor\_5\_a\_20s\_1600\_EDM-1\_01

## Target Data Settings:

Data Path: /home/ryanurb/idata/datasets/xor\_set  
Output Path: /home/ryanurb/idata/output  
Experiment Name: xor\_exp  
Class Label: Class  
Instance Label: None  
Match Label: None  
Ignored Features: None  
Specified Categorical Features: None  
Specified Quantitative Features: None

## Univariate Analysis of Each Dataset (Top 10 Features for Each)

### D1 = xor\_2\_a\_20s\_1600\_EDM-1\_01

| Feature | p-value            | Test-statistic | Test-name           |
|---------|--------------------|----------------|---------------------|
| N10     | 0.2008159114176192 | 329187.5       | Mann-Whitney U Test |
| N16     | 0.2161131395026099 | 330469.0       | Mann-Whitney U Test |
| N14     | 0.2177044748605101 | 330157.5       | Mann-Whitney U Test |
| N12     | 0.219701376834725  | 309757.0       | Mann-Whitney U Test |
| M0P2    | 0.2247856260437952 | 309727.0       | Mann-Whitney U Test |
| N6      | 0.3325323994182377 | 311781.5       | Mann-Whitney U Test |
| N17     | 0.4024957721639753 | 326097.0       | Mann-Whitney U Test |
| N5      | 0.4049861226590078 | 326404.5       | Mann-Whitney U Test |
| N13     | 0.4220032930197887 | 314864.0       | Mann-Whitney U Test |
| N0      | 0.523664179550604  | 315495.0       | Mann-Whitney U Test |

### D2 = xor\_3\_a\_20s\_1600\_EDM-1\_01

| Feature | p-value            | Test-statistic | Test-name           |
|---------|--------------------|----------------|---------------------|
| N1      | 0.0627337878366858 | 304417.0       | Mann-Whitney U Test |
| N0      | 0.0910751126707113 | 334260.5       | Mann-Whitney U Test |
| N6      | 0.1328817197220447 | 307911.5       | Mann-Whitney U Test |
| N9      | 0.1705225466340459 | 308678.0       | Mann-Whitney U Test |
| M0P1    | 0.1959159346687257 | 330938.5       | Mann-Whitney U Test |
| N7      | 0.3618337703410067 | 312358.0       | Mann-Whitney U Test |
| N15     | 0.4519178816847056 | 315966.0       | Mann-Whitney U Test |
| N12     | 0.6283966964155301 | 315956.0       | Mann-Whitney U Test |
| M0P3    | 0.637291337012047  | 316016.0       | Mann-Whitney U Test |
| N2      | 0.6658888818546207 | 316331.0       | Mann-Whitney U Test |

### D3 = xor\_4\_a\_20s\_1600\_EDM-1\_01

| Feature | p-value            | Test-statistic | Test-name           |
|---------|--------------------|----------------|---------------------|
| M0P2    | 0.0398778601679427 | 337466.0       | Mann-Whitney U Test |
| N9      | 0.1159345401469505 | 332276.0       | Mann-Whitney U Test |
| N11     | 0.2467408986646957 | 327160.0       | Mann-Whitney U Test |
| M0P4    | 0.2562882495187207 | 310373.5       | Mann-Whitney U Test |
| N1      | 0.4123734834476052 | 313408.5       | Mann-Whitney U Test |
| N8      | 0.4533372546131419 | 314808.5       | Mann-Whitney U Test |
| N2      | 0.4538014359208079 | 313690.5       | Mann-Whitney U Test |
| N6      | 0.4975936546344156 | 314324.0       | Mann-Whitney U Test |
| N7      | 0.5099863357899403 | 325557.5       | Mann-Whitney U Test |
| N13     | 0.5245440373971155 | 314878.0       | Mann-Whitney U Test |

### D4 = xor\_5\_a\_20s\_1600\_EDM-1\_01

| Feature | p-value            | Test-statistic | Test-name           |
|---------|--------------------|----------------|---------------------|
| N13     | 0.0213637537754956 | 338747.5       | Mann-Whitney U Test |
| N5      | 0.030316904724263  | 301642.5       | Mann-Whitney U Test |
| N14     | 0.1689647199913863 | 309932.0       | Mann-Whitney U Test |
| M0P1    | 0.1718939792980206 | 331622.0       | Mann-Whitney U Test |
| N10     | 0.2440534842431895 | 329083.5       | Mann-Whitney U Test |
| M0P5    | 0.2975384753029626 | 311206.0       | Mann-Whitney U Test |
| N4      | 0.299435231416699  | 311249.5       | Mann-Whitney U Test |
| N9      | 0.3198095781608477 | 313902.5       | Mann-Whitney U Test |
| N7      | 0.3486654469538642 | 312163.5       | Mann-Whitney U Test |
| M0P4    | 0.3629442966393856 | 312361.0       | Mann-Whitney U Test |

# Dataset and Model Prediction Summary: D1 = xor\_2\_a\_20s\_1600\_EDM-1\_01

## Data Processing/Counts Summary

|           | Instances | Total Features | Categorical Features | Quantitative Features | Missing Values | Missing Percent | Class 0 | Class 1 |
|-----------|-----------|----------------|----------------------|-----------------------|----------------|-----------------|---------|---------|
| Original  | 1600      | 20             | 0                    | 20                    | 0              | 0.0             | 800     | 800     |
| C1        | 1600      | 20             | 0                    | 20                    | 0              | 0.0             | 800     | 800     |
| E1        | 1600      | 20             | 0                    | 20                    | 0              | 0.0             | 800     | 800     |
| C2        | 1600      | 20             | 0                    | 20                    | 0              | 0.0             | 800     | 800     |
| C3        | 1600      | 20             | 0                    | 20                    | 0              | 0.0             | 800     | 800     |
| E2        | 1600      | 20             | 0                    | 20                    | 0              | 0.0             | 800     | 800     |
| C4        | 1600      | 20             | 0                    | 20                    | 0              | 0.0             | 800     | 800     |
| Processed | 1600      | 20             | 0                    | 20                    | 0              | 0.0             | 800     | 800     |

## Cleaning (C) and Engineering (E) Elements

- \* C1 - Remove instances with no outcome and features to ignore
- \* E1 - Add missingness features
- \* C2 - Remove features with invariance or high missingness
- \* C3 - Remove instances with high missingness
- \* E2 - Add one-hot-encoding of categorical features
- \* C4 - Remove highly correlated features

## Class Balance (Processed)

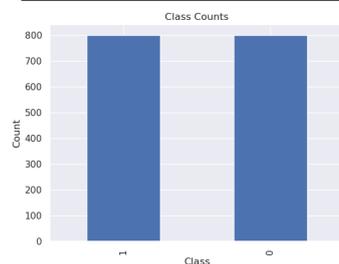

## Feature Correlations (Pearson)

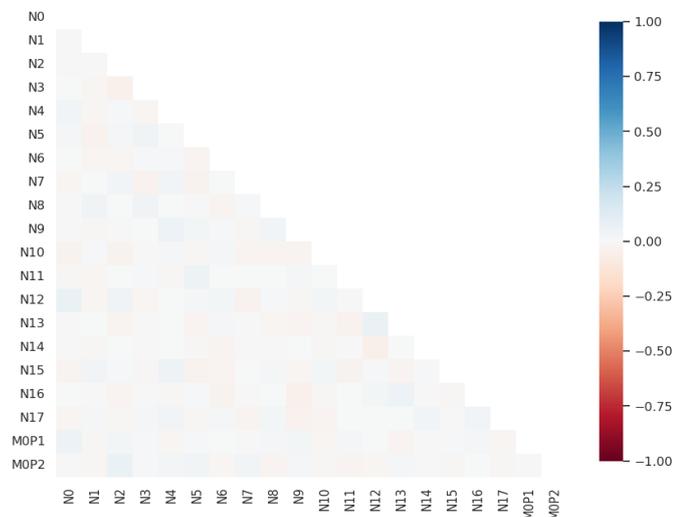

## Top ML Algorithm Results (Averaged Over CV Runs):

|                                                                |
|----------------------------------------------------------------|
| Best (ROC_AUC): Category Gradient Boosting (TIE) = 1.000       |
| Best (Balanced Acc.): Category Gradient Boosting (TIE) = 1.000 |
| Best (F1 Score): Category Gradient Boosting (TIE) = 1.000      |
| Best (PRC AUC): Category Gradient Boosting (TIE) = 1.000       |
| Best (PRC APS): Category Gradient Boosting (TIE) = 1.000       |

## ROC

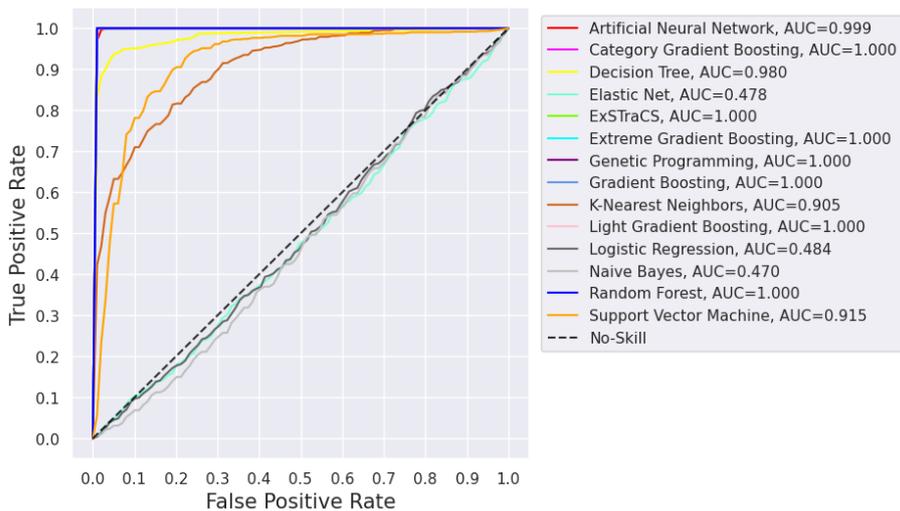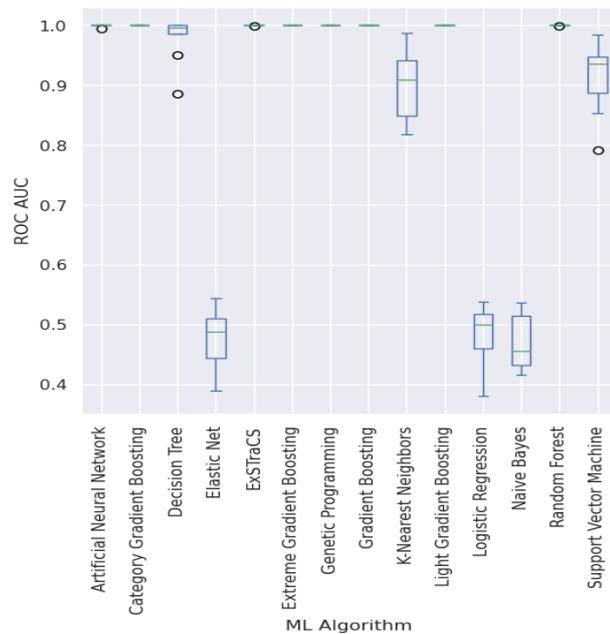

## PRC

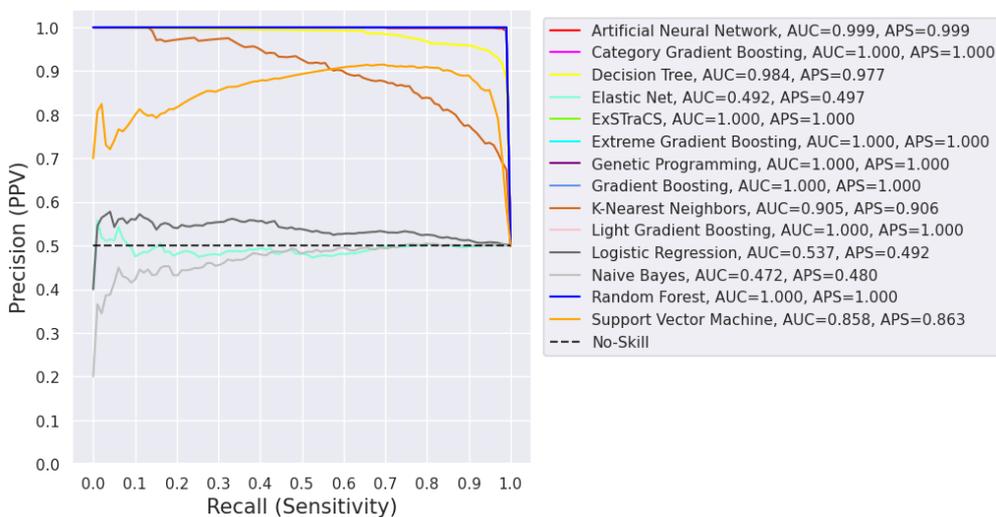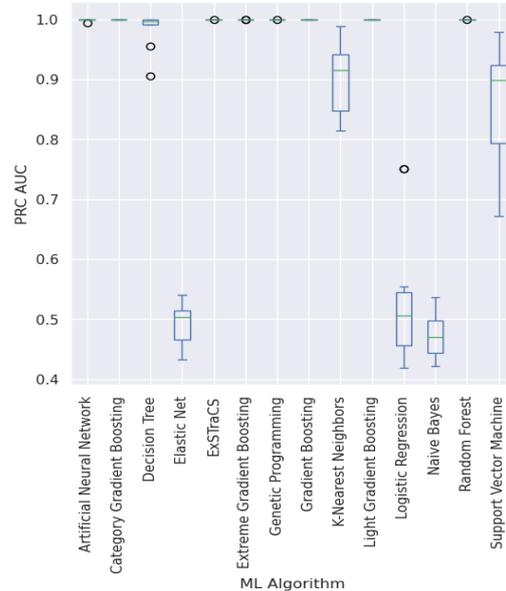

# Dataset and Model Prediction Summary: D2 = xor\_3\_a\_20s\_1600\_EDM-1\_01

## Data Processing/Counts Summary

|           | Instances | Total Features | Categorical Features | Quantitative Features | Missing Values | Missing Percent | Class 0 | Class 1 |
|-----------|-----------|----------------|----------------------|-----------------------|----------------|-----------------|---------|---------|
| Original  | 1600      | 20             | 0                    | 20                    | 0              | 0.0             | 800     | 800     |
| C1        | 1600      | 20             | 0                    | 20                    | 0              | 0.0             | 800     | 800     |
| E1        | 1600      | 20             | 0                    | 20                    | 0              | 0.0             | 800     | 800     |
| C2        | 1600      | 20             | 0                    | 20                    | 0              | 0.0             | 800     | 800     |
| C3        | 1600      | 20             | 0                    | 20                    | 0              | 0.0             | 800     | 800     |
| E2        | 1600      | 20             | 0                    | 20                    | 0              | 0.0             | 800     | 800     |
| C4        | 1600      | 20             | 0                    | 20                    | 0              | 0.0             | 800     | 800     |
| Processed | 1600      | 20             | 0                    | 20                    | 0              | 0.0             | 800     | 800     |

## Cleaning (C) and Engineering (E) Elements

- \* C1 - Remove instances with no outcome and features to ignore
- \* E1 - Add missingness features
- \* C2 - Remove features with invariance or high missingness
- \* C3 - Remove instances with high missingness
- \* E2 - Add one-hot-encoding of categorical features
- \* C4 - Remove highly correlated features

## Class Balance (Processed)

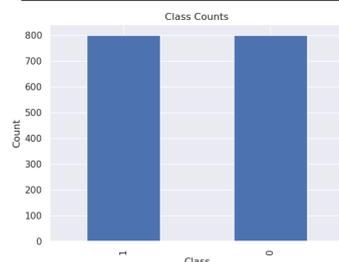

## Feature Correlations (Pearson)

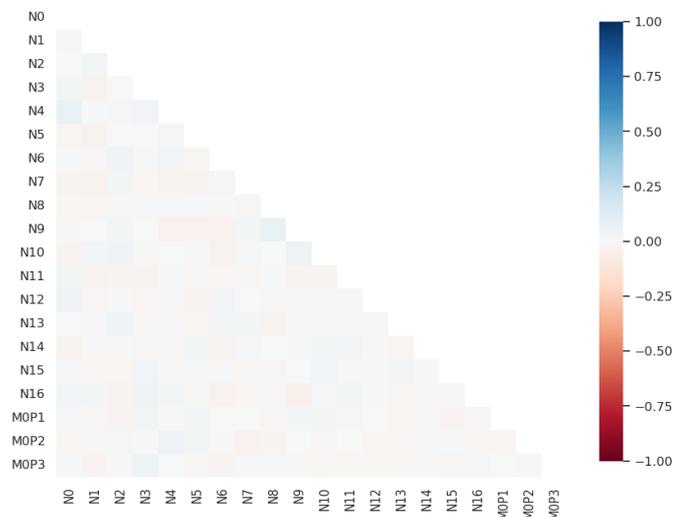

## Top ML Algorithm Results (Averaged Over CV Runs):

|                                                                |
|----------------------------------------------------------------|
| Best (ROC_AUC): Category Gradient Boosting (TIE) = 1.000       |
| Best (Balanced Acc.): Category Gradient Boosting (TIE) = 1.000 |
| Best (F1 Score): Category Gradient Boosting (TIE) = 1.000      |
| Best (PRC AUC): Category Gradient Boosting (TIE) = 1.000       |
| Best (PRC APS): Category Gradient Boosting (TIE) = 1.000       |

## ROC

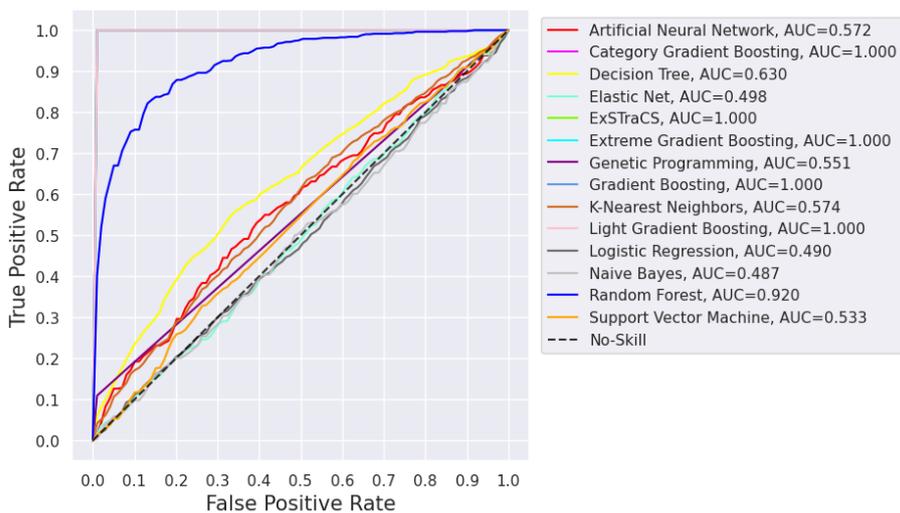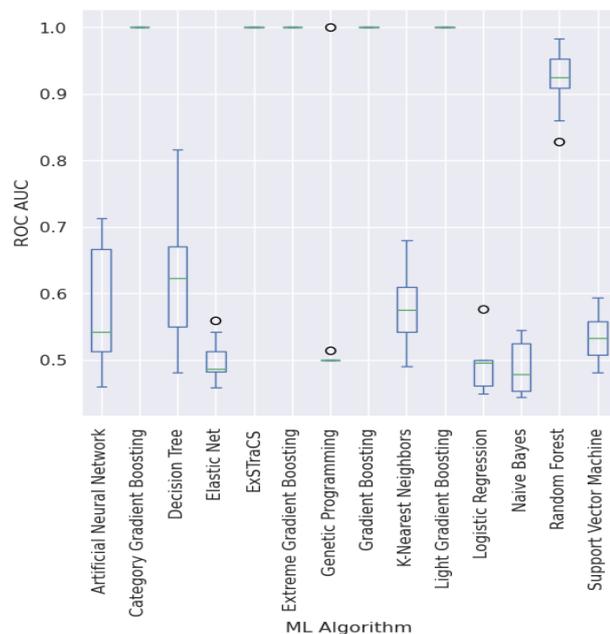

## PRC

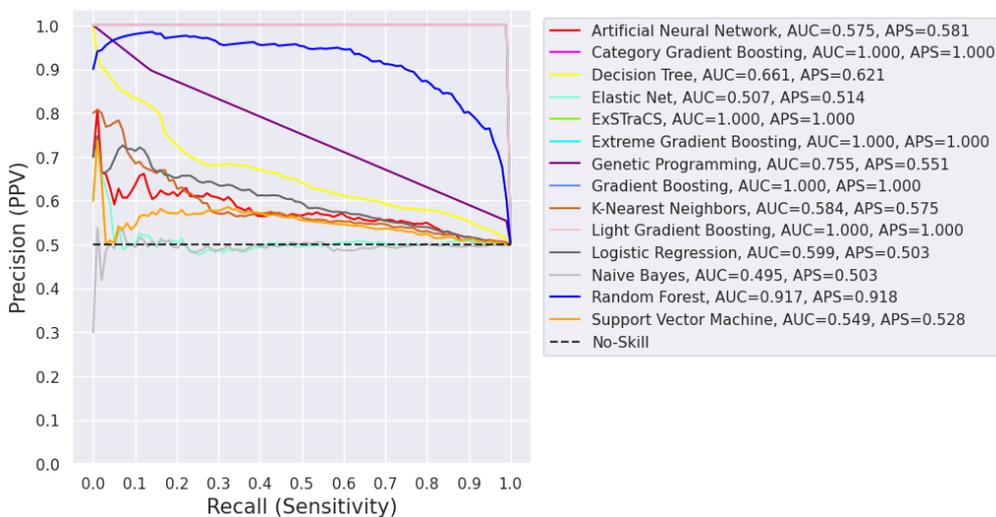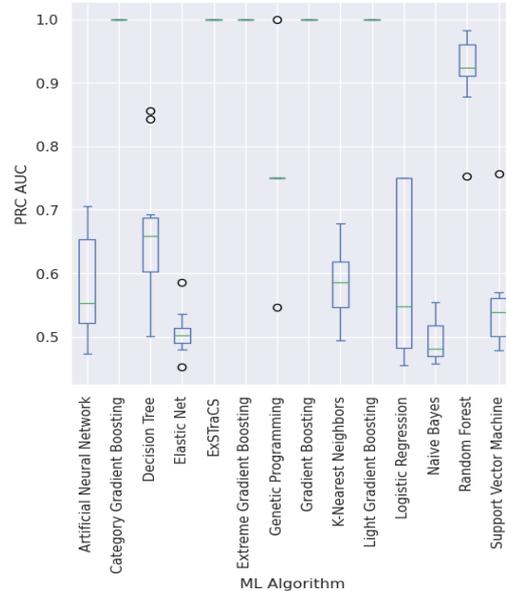

# Dataset and Model Prediction Summary: D3 = xor\_4\_a\_20s\_1600\_EDM-1\_01

## Data Processing/Counts Summary

|           | Instances | Total Features | Categorical Features | Quantitative Features | Missing Values | Missing Percent | Class 0 | Class 1 |
|-----------|-----------|----------------|----------------------|-----------------------|----------------|-----------------|---------|---------|
| Original  | 1600      | 20             | 0                    | 20                    | 0              | 0.0             | 800     | 800     |
| C1        | 1600      | 20             | 0                    | 20                    | 0              | 0.0             | 800     | 800     |
| E1        | 1600      | 20             | 0                    | 20                    | 0              | 0.0             | 800     | 800     |
| C2        | 1600      | 20             | 0                    | 20                    | 0              | 0.0             | 800     | 800     |
| C3        | 1600      | 20             | 0                    | 20                    | 0              | 0.0             | 800     | 800     |
| E2        | 1600      | 20             | 0                    | 20                    | 0              | 0.0             | 800     | 800     |
| C4        | 1600      | 20             | 0                    | 20                    | 0              | 0.0             | 800     | 800     |
| Processed | 1600      | 20             | 0                    | 20                    | 0              | 0.0             | 800     | 800     |

## Cleaning (C) and Engineering (E) Elements

- \* C1 - Remove instances with no outcome and features to ignore
- \* E1 - Add missingness features
- \* C2 - Remove features with invariance or high missingness
- \* C3 - Remove instances with high missingness
- \* E2 - Add one-hot-encoding of categorical features
- \* C4 - Remove highly correlated features

## Class Balance (Processed)

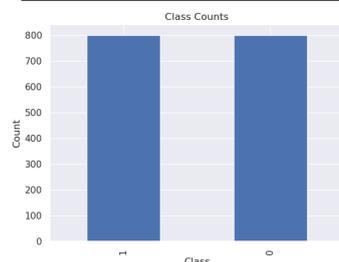

## Feature Correlations (Pearson)

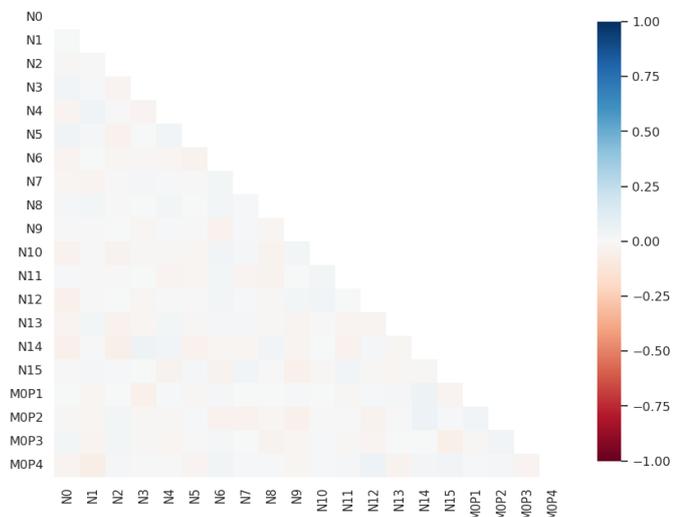

## Top ML Algorithm Results (Averaged Over CV Runs):

|                                                    |
|----------------------------------------------------|
| Best (ROC_AUC): Decision Tree = 0.517              |
| Best (Balanced Acc.): Decision Tree = 0.508        |
| Best (F1 Score): Artificial Neural Network = 0.548 |
| Best (PRC AUC): Genetic Programming = 0.733        |
| Best (PRC APS): Decision Tree = 0.527              |

## ROC

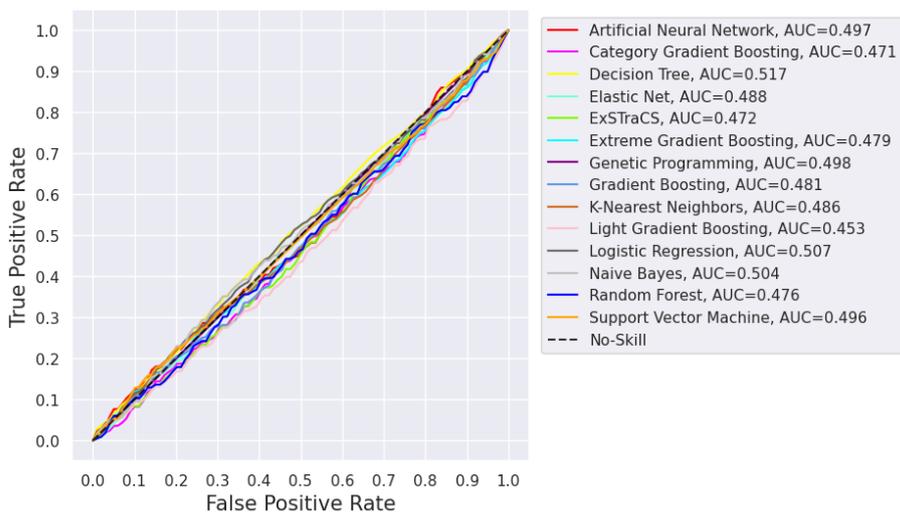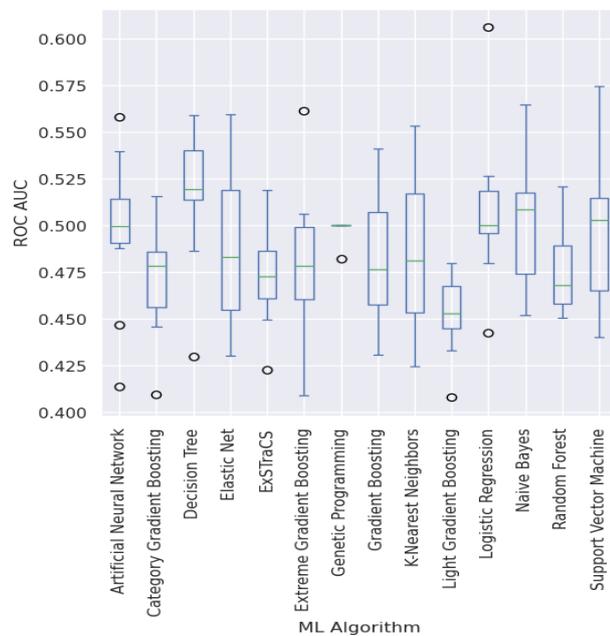

## PRC

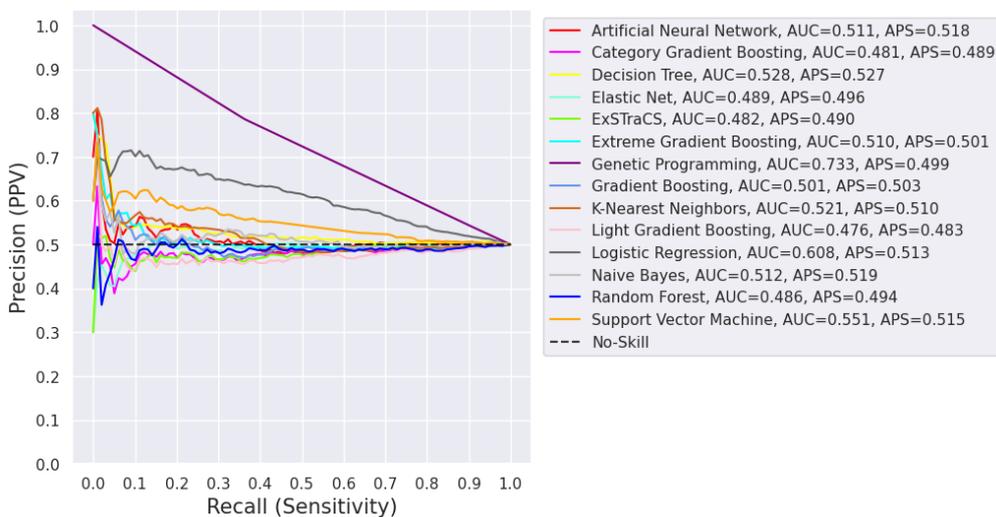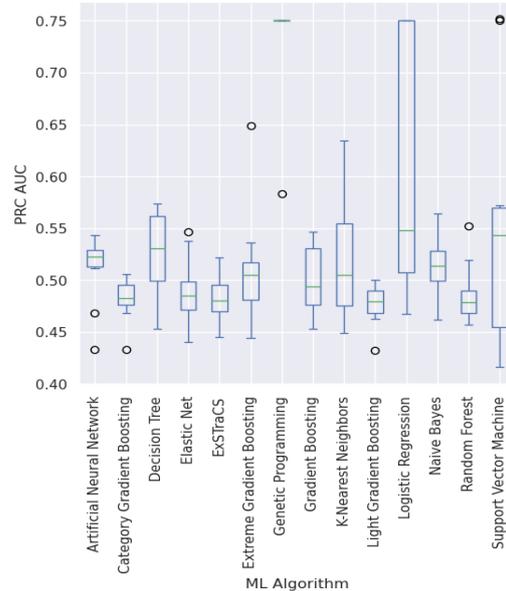

# Dataset and Model Prediction Summary: D4 = xor\_5\_a\_20s\_1600\_EDM-1\_01

## Data Processing/Counts Summary

|           | Instances | Total Features | Categorical Features | Quantitative Features | Missing Values | Missing Percent | Class 0 | Class 1 |
|-----------|-----------|----------------|----------------------|-----------------------|----------------|-----------------|---------|---------|
| Original  | 1600      | 20             | 0                    | 20                    | 0              | 0.0             | 800     | 800     |
| C1        | 1600      | 20             | 0                    | 20                    | 0              | 0.0             | 800     | 800     |
| E1        | 1600      | 20             | 0                    | 20                    | 0              | 0.0             | 800     | 800     |
| C2        | 1600      | 20             | 0                    | 20                    | 0              | 0.0             | 800     | 800     |
| C3        | 1600      | 20             | 0                    | 20                    | 0              | 0.0             | 800     | 800     |
| E2        | 1600      | 20             | 0                    | 20                    | 0              | 0.0             | 800     | 800     |
| C4        | 1600      | 20             | 0                    | 20                    | 0              | 0.0             | 800     | 800     |
| Processed | 1600      | 20             | 0                    | 20                    | 0              | 0.0             | 800     | 800     |

## Cleaning (C) and Engineering (E) Elements

- \* C1 - Remove instances with no outcome and features to ignore
- \* E1 - Add missingness features
- \* C2 - Remove features with invariance or high missingness
- \* C3 - Remove instances with high missingness
- \* E2 - Add one-hot-encoding of categorical features
- \* C4 - Remove highly correlated features

## Class Balance (Processed)

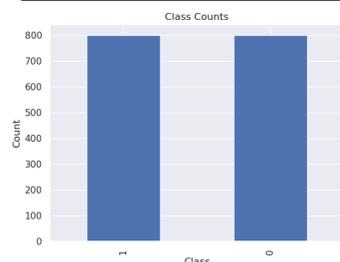

## Feature Correlations (Pearson)

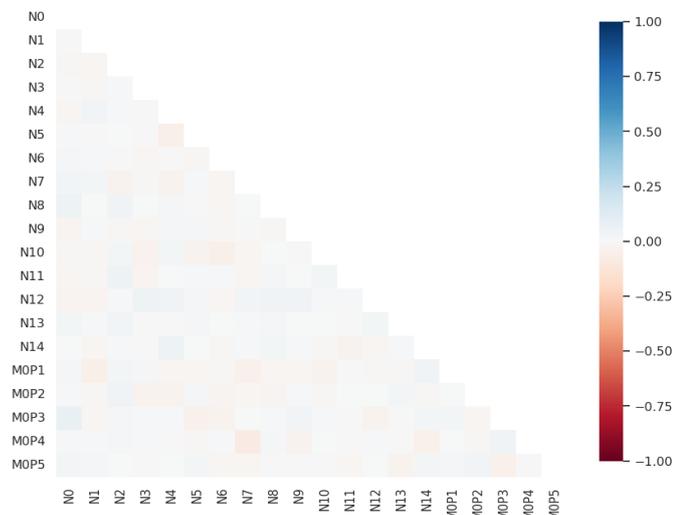

## Top ML Algorithm Results (Averaged Over CV Runs):

|                                                          |
|----------------------------------------------------------|
| Best (ROC_AUC): Elastic Net = 0.529                      |
| Best (Balanced Acc.): Category Gradient Boosting = 0.528 |
| Best (F1 Score): Gradient Boosting = 0.532               |
| Best (PRC AUC): Genetic Programming = 0.734              |
| Best (PRC APS): Category Gradient Boosting = 0.546       |

## ROC

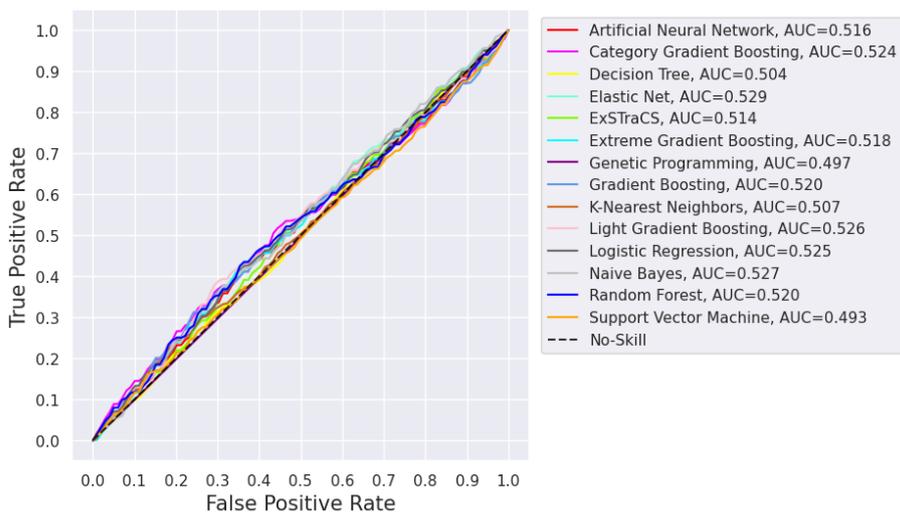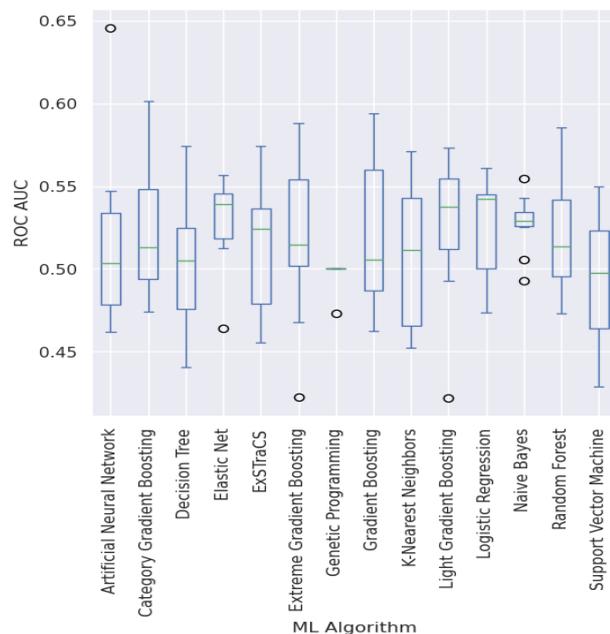

## PRC

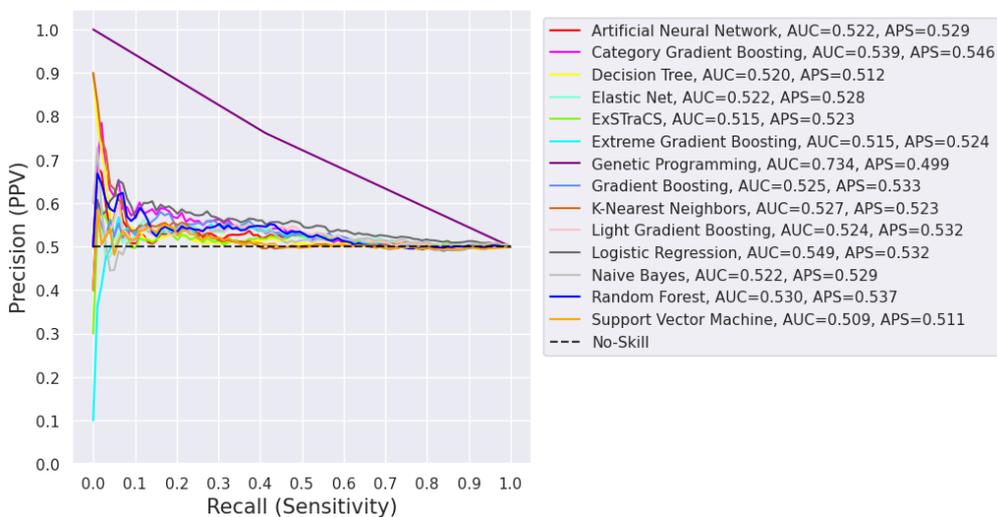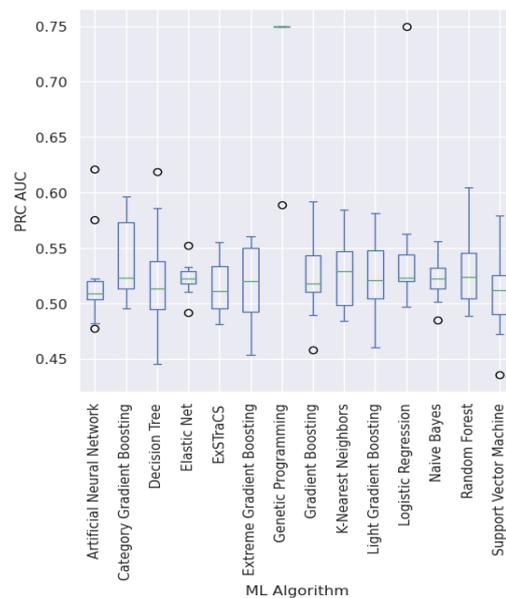

# Average Model Prediction Statistics (Rounded to 3 Decimal Points)

## D1 = xor\_2\_a\_20s\_1600\_EDM-1\_01

| ML Algorithm               | Balanced Accuracy | Accuracy | F1 Score | Sensitivity (Recall) | Specificity | Precision (PPV) | TP   | TN   | FP   | FN   | NPV   | LR+    | LR-   | ROC AUC | PRC AUC | PRC APS |
|----------------------------|-------------------|----------|----------|----------------------|-------------|-----------------|------|------|------|------|-------|--------|-------|---------|---------|---------|
| Artificial Neural Network  | 0.992             | 0.992    | 0.993    | 0.996                | 0.989       | 0.989           | 79.7 | 79.1 | 0.9  | 0.3  | 0.996 | 12.247 | 0.004 | 1.0     | 0.999   | 0.999   |
| Category Gradient Boosting | 1.0               | 1.0      | 1.0      | 1.0                  | 1.0         | 1.0             | 80.0 | 80.0 | 0.0  | 0.0  | 1.0   | 0.0    | 0.0   | 1.0     | 1.0     | 1.0     |
| Decision Tree              | 0.961             | 0.961    | 0.959    | 0.949                | 0.974       | 0.972           | 75.9 | 77.9 | 2.1  | 4.1  | 0.953 | 24.961 | 0.056 | 0.98    | 0.984   | 0.977   |
| Elastic Net                | 0.473             | 0.473    | 0.492    | 0.512                | 0.434       | 0.475           | 41.0 | 34.7 | 45.3 | 39.0 | 0.47  | 0.91   | 1.138 | 0.478   | 0.492   | 0.497   |
| ExSTraCS                   | 1.0               | 1.0      | 1.0      | 1.0                  | 1.0         | 1.0             | 80.0 | 80.0 | 0.0  | 0.0  | 1.0   | 0.0    | 0.0   | 1.0     | 1.0     | 1.0     |
| Extreme Gradient Boosting  | 1.0               | 1.0      | 1.0      | 1.0                  | 1.0         | 1.0             | 80.0 | 80.0 | 0.0  | 0.0  | 1.0   | 0.0    | 0.0   | 1.0     | 1.0     | 1.0     |
| Genetic Programming        | 1.0               | 1.0      | 1.0      | 1.0                  | 1.0         | 1.0             | 80.0 | 80.0 | 0.0  | 0.0  | 1.0   | 0.0    | 0.0   | 1.0     | 1.0     | 1.0     |
| Gradient Boosting          | 1.0               | 1.0      | 1.0      | 1.0                  | 1.0         | 1.0             | 80.0 | 80.0 | 0.0  | 0.0  | 1.0   | 0.0    | 0.0   | 1.0     | 1.0     | 1.0     |
| K-Nearest Neighbors        | 0.817             | 0.817    | 0.818    | 0.824                | 0.81        | 0.814           | 65.9 | 64.8 | 15.2 | 14.1 | 0.822 | 5.861  | 0.225 | 0.905   | 0.905   | 0.906   |
| Light Gradient Boosting    | 1.0               | 1.0      | 1.0      | 1.0                  | 1.0         | 1.0             | 80.0 | 80.0 | 0.0  | 0.0  | 1.0   | 0.0    | 0.0   | 1.0     | 1.0     | 1.0     |
| Logistic Regression        | 0.485             | 0.485    | 0.37     | 0.361                | 0.609       | 0.386           | 28.9 | 48.7 | 31.3 | 51.1 | 0.484 | 0.754  | 1.073 | 0.484   | 0.537   | 0.492   |
| Naive Bayes                | 0.476             | 0.476    | 0.482    | 0.491                | 0.46        | 0.475           | 39.3 | 36.8 | 43.2 | 40.7 | 0.476 | 0.919  | 1.124 | 0.47    | 0.472   | 0.48    |
| Random Forest              | 1.0               | 1.0      | 1.0      | 1.0                  | 1.0         | 1.0             | 80.0 | 80.0 | 0.0  | 0.0  | 1.0   | 0.0    | 0.0   | 1.0     | 1.0     | 1.0     |
| Support Vector Machine     | 0.889             | 0.889    | 0.891    | 0.904                | 0.874       | 0.879           | 72.3 | 69.9 | 10.1 | 7.7  | 0.901 | 9.739  | 0.115 | 0.915   | 0.858   | 0.863   |

## D2 = xor\_3\_a\_20s\_1600\_EDM-1\_01

| ML Algorithm               | Balanced Accuracy | Accuracy | F1 Score | Sensitivity (Recall) | Specificity | Precision (PPV) | TP   | TN   | FP   | FN   | NPV   | LR+   | LR-   | ROC AUC | PRC AUC | PRC APS |
|----------------------------|-------------------|----------|----------|----------------------|-------------|-----------------|------|------|------|------|-------|-------|-------|---------|---------|---------|
| Artificial Neural Network  | 0.561             | 0.561    | 0.563    | 0.571                | 0.55        | 0.558           | 45.7 | 44.0 | 36.0 | 34.3 | 0.564 | 1.345 | 0.811 | 0.572   | 0.575   | 0.581   |
| Category Gradient Boosting | 1.0               | 1.0      | 1.0      | 1.0                  | 1.0         | 1.0             | 80.0 | 80.0 | 0.0  | 0.0  | 1.0   | 0.0   | 0.0   | 1.0     | 1.0     | 1.0     |
| Decision Tree              | 0.598             | 0.598    | 0.593    | 0.588                | 0.609       | 0.601           | 47.0 | 48.7 | 31.3 | 33.0 | 0.596 | 1.724 | 0.709 | 0.63    | 0.661   | 0.621   |
| Elastic Net                | 0.492             | 0.492    | 0.476    | 0.461                | 0.524       | 0.493           | 36.9 | 41.9 | 38.1 | 43.1 | 0.492 | 0.98  | 1.04  | 0.498   | 0.507   | 0.514   |
| ExSTraCS                   | 1.0               | 1.0      | 1.0      | 1.0                  | 1.0         | 1.0             | 80.0 | 80.0 | 0.0  | 0.0  | 1.0   | 0.0   | 0.0   | 1.0     | 1.0     | 1.0     |
| Extreme Gradient Boosting  | 1.0               | 1.0      | 1.0      | 1.0                  | 1.0         | 1.0             | 80.0 | 80.0 | 0.0  | 0.0  | 1.0   | 0.0   | 0.0   | 1.0     | 1.0     | 1.0     |
| Genetic Programming        | 0.551             | 0.551    | 0.588    | 0.814                | 0.288       | 0.502           | 65.1 | 23.0 | 57.0 | 14.9 | 0.2   | 0.81  | 0.199 | 0.551   | 0.755   | 0.551   |
| Gradient Boosting          | 1.0               | 1.0      | 1.0      | 1.0                  | 1.0         | 1.0             | 80.0 | 80.0 | 0.0  | 0.0  | 1.0   | 0.0   | 0.0   | 1.0     | 1.0     | 1.0     |
| K-Nearest Neighbors        | 0.556             | 0.556    | 0.527    | 0.51                 | 0.601       | 0.56            | 40.8 | 48.1 | 31.9 | 39.2 | 0.555 | 1.293 | 0.813 | 0.574   | 0.584   | 0.575   |
| Light Gradient Boosting    | 1.0               | 1.0      | 1.0      | 1.0                  | 1.0         | 1.0             | 80.0 | 80.0 | 0.0  | 0.0  | 1.0   | 0.0   | 0.0   | 1.0     | 1.0     | 1.0     |
| Logistic Regression        | 0.494             | 0.494    | 0.289    | 0.286                | 0.701       | 0.295           | 22.9 | 56.1 | 23.9 | 57.1 | 0.492 | 0.589 | 1.038 | 0.49    | 0.599   | 0.503   |
| Naive Bayes                | 0.499             | 0.499    | 0.519    | 0.542                | 0.456       | 0.5             | 43.4 | 36.5 | 43.5 | 36.6 | 0.499 | 1.007 | 1.021 | 0.487   | 0.495   | 0.503   |
| Random Forest              | 0.85              | 0.85     | 0.849    | 0.846                | 0.854       | 0.854           | 67.7 | 68.3 | 11.7 | 12.3 | 0.848 | 7.18  | 0.184 | 0.92    | 0.917   | 0.918   |
| Support Vector Machine     | 0.529             | 0.529    | 0.51     | 0.499                | 0.56        | 0.532           | 39.9 | 44.8 | 35.2 | 40.1 | 0.53  | 1.155 | 0.899 | 0.533   | 0.549   | 0.528   |

## D3 = xor\_4\_a\_20s\_1600\_EDM-1\_01

| ML Algorithm               | Balanced Accuracy | Accuracy | F1 Score | Sensitivity (Recall) | Specificity | Precision (PPV) | TP   | TN   | FP   | FN   | NPV   | LR+   | LR-   | ROC AUC | PRC AUC | PRC APS |
|----------------------------|-------------------|----------|----------|----------------------|-------------|-----------------|------|------|------|------|-------|-------|-------|---------|---------|---------|
| Artificial Neural Network  | 0.502             | 0.502    | 0.548    | 0.626                | 0.379       | 0.501           | 50.1 | 30.3 | 49.7 | 29.9 | 0.458 | 1.01  | 0.886 | 0.497   | 0.511   | 0.518   |
| Category Gradient Boosting | 0.483             | 0.483    | 0.471    | 0.461                | 0.505       | 0.482           | 36.9 | 40.4 | 39.6 | 43.1 | 0.484 | 0.938 | 1.074 | 0.471   | 0.481   | 0.489   |
| Decision Tree              | 0.508             | 0.508    | 0.468    | 0.445                | 0.571       | 0.505           | 35.6 | 45.7 | 34.3 | 44.4 | 0.509 | 1.03  | 0.967 | 0.517   | 0.528   | 0.527   |
| Elastic Net                | 0.489             | 0.489    | 0.494    | 0.502                | 0.476       | 0.489           | 40.2 | 38.1 | 41.9 | 39.8 | 0.489 | 0.962 | 1.049 | 0.488   | 0.489   | 0.496   |
| ExSTraCS                   | 0.479             | 0.479    | 0.459    | 0.456                | 0.503       | 0.478           | 36.5 | 40.2 | 39.8 | 43.5 | 0.478 | 0.922 | 1.095 | 0.472   | 0.482   | 0.49    |
| Extreme Gradient Boosting  | 0.489             | 0.489    | 0.368    | 0.334                | 0.644       | 0.499           | 26.7 | 51.5 | 28.5 | 53.3 | 0.486 | 1.057 | 1.071 | 0.479   | 0.51    | 0.501   |
| Genetic Programming        | 0.498             | 0.498    | 0.464    | 0.691                | 0.305       | 0.349           | 55.3 | 24.4 | 55.6 | 24.7 | 0.186 | 0.696 | 0.475 | 0.498   | 0.733   | 0.499   |
| Gradient Boosting          | 0.488             | 0.488    | 0.489    | 0.491                | 0.485       | 0.488           | 39.3 | 38.8 | 41.2 | 40.7 | 0.488 | 0.958 | 1.053 | 0.481   | 0.501   | 0.503   |
| K-Nearest Neighbors        | 0.487             | 0.487    | 0.455    | 0.43                 | 0.544       | 0.489           | 34.4 | 43.5 | 36.5 | 45.6 | 0.485 | 0.974 | 1.074 | 0.486   | 0.521   | 0.51    |
| Light Gradient Boosting    | 0.469             | 0.469    | 0.439    | 0.424                | 0.514       | 0.465           | 33.9 | 41.1 | 38.9 | 46.1 | 0.471 | 0.872 | 1.128 | 0.453   | 0.476   | 0.483   |
| Logistic Regression        | 0.504             | 0.504    | 0.293    | 0.291                | 0.716       | 0.301           | 23.3 | 57.3 | 22.7 | 56.7 | 0.508 | 0.613 | 0.984 | 0.507   | 0.608   | 0.513   |
| Naive Bayes                | 0.506             | 0.506    | 0.533    | 0.565                | 0.446       | 0.505           | 45.2 | 35.7 | 44.3 | 34.8 | 0.506 | 1.025 | 0.982 | 0.504   | 0.512   | 0.519   |
| Random Forest              | 0.485             | 0.485    | 0.479    | 0.478                | 0.492       | 0.484           | 38.2 | 39.4 | 40.6 | 41.8 | 0.486 | 0.942 | 1.064 | 0.476   | 0.486   | 0.494   |
| Support Vector Machine     | 0.486             | 0.486    | 0.474    | 0.465                | 0.506       | 0.486           | 37.2 | 40.5 | 39.5 | 42.8 | 0.485 | 0.953 | 1.069 | 0.496   | 0.551   | 0.515   |

## D4 = xor\_5\_a\_20s\_1600\_EDM-1\_01

| ML Algorithm               | Balanced Accuracy | Accuracy | F1 Score | Sensitivity (Recall) | Specificity | Precision (PPV) | TP   | TN   | FP   | FN   | NPV   | LR+   | LR-   | ROC AUC | PRC AUC | PRC APS |
|----------------------------|-------------------|----------|----------|----------------------|-------------|-----------------|------|------|------|------|-------|-------|-------|---------|---------|---------|
| Artificial Neural Network  | 0.523             | 0.523    | 0.519    | 0.518                | 0.529       | 0.523           | 41.4 | 42.3 | 37.7 | 38.6 | 0.524 | 1.121 | 0.926 | 0.516   | 0.522   | 0.529   |
| Category Gradient Boosting | 0.528             | 0.528    | 0.526    | 0.525                | 0.531       | 0.529           | 42.0 | 42.5 | 37.5 | 38.0 | 0.528 | 1.134 | 0.904 | 0.524   | 0.539   | 0.546   |
| Decision Tree              | 0.498             | 0.498    | 0.491    | 0.486                | 0.51        | 0.499           | 38.9 | 40.8 | 39.2 | 41.1 | 0.497 | 1.01  | 1.023 | 0.504   | 0.52    | 0.512   |
| Elastic Net                | 0.524             | 0.524    | 0.495    | 0.47                 | 0.579       | 0.528           | 37.6 | 46.3 | 33.7 | 42.4 | 0.522 | 1.128 | 0.919 | 0.529   | 0.522   | 0.528   |
| ExSTraCS                   | 0.518             | 0.518    | 0.495    | 0.481                | 0.555       | 0.52            | 38.5 | 44.4 | 35.6 | 41.5 | 0.517 | 1.098 | 0.942 | 0.514   | 0.515   | 0.523   |
| Extreme Gradient Boosting  | 0.513             | 0.513    | 0.519    | 0.528                | 0.499       | 0.513           | 42.2 | 39.9 | 40.1 | 37.8 | 0.514 | 1.059 | 0.955 | 0.518   | 0.515   | 0.524   |
| Genetic Programming        | 0.499             | 0.499    | 0.532    | 0.794                | 0.205       | 0.4             | 63.5 | 16.4 | 63.6 | 16.5 | 0.144 | 0.799 | 0.325 | 0.497   | 0.734   | 0.499   |
| Gradient Boosting          | 0.523             | 0.523    | 0.532    | 0.544                | 0.502       | 0.522           | 43.5 | 40.2 | 39.8 | 36.5 | 0.525 | 1.103 | 0.914 | 0.52    | 0.525   | 0.533   |
| K-Nearest Neighbors        | 0.489             | 0.489    | 0.471    | 0.462                | 0.516       | 0.486           | 37.0 | 41.3 | 38.7 | 43.0 | 0.492 | 0.96  | 1.053 | 0.507   | 0.527   | 0.523   |
| Light Gradient Boosting    | 0.519             | 0.519    | 0.53     | 0.548                | 0.49        | 0.517           | 43.8 | 39.2 | 40.8 | 36.2 | 0.522 | 1.076 | 0.922 | 0.526   | 0.524   | 0.532   |
| Logistic Regression        | 0.522             | 0.522    | 0.474    | 0.476                | 0.569       | 0.472           | 38.1 | 45.5 | 34.5 | 41.9 | 0.523 | 1.005 | 0.923 | 0.525   | 0.549   | 0.532   |
| Naive Bayes                | 0.513             | 0.512    | 0.509    | 0.506                | 0.519       | 0.513           | 40.5 | 41.5 | 38.5 | 39.5 | 0.513 | 1.055 | 0.954 | 0.527   | 0.522   | 0.529   |
| Random Forest              | 0.522             | 0.522    | 0.513    | 0.506                | 0.539       | 0.522           | 40.5 | 43.1 | 36.9 | 39.5 | 0.523 | 1.1   | 0.917 | 0.52    | 0.53    | 0.537   |
| Support Vector Machine     | 0.501             | 0.501    | 0.505    | 0.516                | 0.485       | 0.498           | 41.3 | 38.8 | 41.2 | 38.7 | 0.504 | 1.003 | 0.998 | 0.493   | 0.509   | 0.511   |

# Median Model Prediction Statistics (Rounded to 3 Decimal Points)

## D1 = xor\_2\_a\_20s\_1600\_EDM-1\_01

| ML Algorithm               | Balanced Accuracy | Accuracy | F1 Score | Sensitivity (Recall) | Specificity | Precision (PPV) | TP   | TN   | FP   | FN   | NPV   | LR+   | LR-   | ROC AUC | PRC AUC | PRC APS |
|----------------------------|-------------------|----------|----------|----------------------|-------------|-----------------|------|------|------|------|-------|-------|-------|---------|---------|---------|
| Artificial Neural Network  | 0.997             | 0.997    | 0.997    | 1.0                  | 1.0         | 1.0             | 80.0 | 80.0 | 0.0  | 0.0  | 1.0   | 0.0   | 0.0   | 1.0     | 1.0     | 1.0     |
| Category Gradient Boosting | 1.0               | 1.0      | 1.0      | 1.0                  | 1.0         | 1.0             | 80.0 | 80.0 | 0.0  | 0.0  | 1.0   | 0.0   | 0.0   | 1.0     | 1.0     | 1.0     |
| Decision Tree              | 0.991             | 0.991    | 0.991    | 0.994                | 0.994       | 0.994           | 79.5 | 79.5 | 0.5  | 0.5  | 0.994 | 3.091 | 0.006 | 0.996   | 0.996   | 0.993   |
| Elastic Net                | 0.469             | 0.469    | 0.503    | 0.519                | 0.438       | 0.474           | 41.5 | 35.0 | 45.0 | 38.5 | 0.465 | 0.902 | 1.149 | 0.488   | 0.502   | 0.503   |
| ExSTraCS                   | 1.0               | 1.0      | 1.0      | 1.0                  | 1.0         | 1.0             | 80.0 | 80.0 | 0.0  | 0.0  | 1.0   | 0.0   | 0.0   | 1.0     | 1.0     | 1.0     |
| Extreme Gradient Boosting  | 1.0               | 1.0      | 1.0      | 1.0                  | 1.0         | 1.0             | 80.0 | 80.0 | 0.0  | 0.0  | 1.0   | 0.0   | 0.0   | 1.0     | 1.0     | 1.0     |
| Genetic Programming        | 1.0               | 1.0      | 1.0      | 1.0                  | 1.0         | 1.0             | 80.0 | 80.0 | 0.0  | 0.0  | 1.0   | 0.0   | 0.0   | 1.0     | 1.0     | 1.0     |
| Gradient Boosting          | 1.0               | 1.0      | 1.0      | 1.0                  | 1.0         | 1.0             | 80.0 | 80.0 | 0.0  | 0.0  | 1.0   | 0.0   | 0.0   | 1.0     | 1.0     | 1.0     |
| K-Nearest Neighbors        | 0.809             | 0.809    | 0.817    | 0.825                | 0.794       | 0.791           | 66.0 | 63.5 | 16.5 | 14.0 | 0.814 | 3.798 | 0.228 | 0.91    | 0.915   | 0.915   |
| Light Gradient Boosting    | 1.0               | 1.0      | 1.0      | 1.0                  | 1.0         | 1.0             | 80.0 | 80.0 | 0.0  | 0.0  | 1.0   | 0.0   | 0.0   | 1.0     | 1.0     | 1.0     |
| Logistic Regression        | 0.494             | 0.494    | 0.476    | 0.469                | 0.506       | 0.473           | 37.5 | 40.5 | 39.5 | 42.5 | 0.494 | 0.899 | 1.026 | 0.5     | 0.506   | 0.5     |
| Naive Bayes                | 0.484             | 0.484    | 0.482    | 0.488                | 0.475       | 0.484           | 39.0 | 38.0 | 42.0 | 41.0 | 0.485 | 0.94  | 1.066 | 0.456   | 0.47    | 0.478   |
| Random Forest              | 1.0               | 1.0      | 1.0      | 1.0                  | 1.0         | 1.0             | 80.0 | 80.0 | 0.0  | 0.0  | 1.0   | 0.0   | 0.0   | 1.0     | 1.0     | 1.0     |
| Support Vector Machine     | 0.919             | 0.919    | 0.917    | 0.919                | 0.9         | 0.905           | 73.5 | 72.0 | 8.0  | 6.5  | 0.916 | 9.651 | 0.092 | 0.936   | 0.899   | 0.901   |

## D2 = xor\_3\_a\_20s\_1600\_EDM-1\_01

| ML Algorithm               | Balanced Accuracy | Accuracy | F1 Score | Sensitivity (Recall) | Specificity | Precision (PPV) | TP   | TN   | FP   | FN   | NPV   | LR+   | LR-   | ROC AUC | PRC AUC | PRC APS |
|----------------------------|-------------------|----------|----------|----------------------|-------------|-----------------|------|------|------|------|-------|-------|-------|---------|---------|---------|
| Artificial Neural Network  | 0.531             | 0.531    | 0.547    | 0.562                | 0.544       | 0.528           | 45.0 | 43.5 | 36.5 | 35.0 | 0.537 | 1.121 | 0.868 | 0.542   | 0.553   | 0.558   |
| Category Gradient Boosting | 1.0               | 1.0      | 1.0      | 1.0                  | 1.0         | 1.0             | 80.0 | 80.0 | 0.0  | 0.0  | 1.0   | 0.0   | 0.0   | 1.0     | 1.0     | 1.0     |
| Decision Tree              | 0.572             | 0.572    | 0.582    | 0.575                | 0.594       | 0.568           | 46.0 | 47.5 | 32.5 | 34.0 | 0.577 | 1.314 | 0.732 | 0.623   | 0.659   | 0.613   |
| Elastic Net                | 0.484             | 0.484    | 0.467    | 0.456                | 0.525       | 0.482           | 36.5 | 42.0 | 38.0 | 43.5 | 0.486 | 0.931 | 1.057 | 0.486   | 0.502   | 0.508   |
| ExSTraCS                   | 1.0               | 1.0      | 1.0      | 1.0                  | 1.0         | 1.0             | 80.0 | 80.0 | 0.0  | 0.0  | 1.0   | 0.0   | 0.0   | 1.0     | 1.0     | 1.0     |
| Extreme Gradient Boosting  | 1.0               | 1.0      | 1.0      | 1.0                  | 1.0         | 1.0             | 80.0 | 80.0 | 0.0  | 0.0  | 1.0   | 0.0   | 0.0   | 1.0     | 1.0     | 1.0     |
| Genetic Programming        | 0.5               | 0.5      | 0.667    | 1.0                  | 0.0         | 0.5             | 80.0 | 0.0  | 80.0 | 0.0  | 0.0   | 1.0   | 0.0   | 0.5     | 0.75    | 0.5     |
| Gradient Boosting          | 1.0               | 1.0      | 1.0      | 1.0                  | 1.0         | 1.0             | 80.0 | 80.0 | 0.0  | 0.0  | 1.0   | 0.0   | 0.0   | 1.0     | 1.0     | 1.0     |
| K-Nearest Neighbors        | 0.553             | 0.553    | 0.545    | 0.525                | 0.594       | 0.557           | 42.0 | 47.5 | 32.5 | 38.0 | 0.554 | 1.259 | 0.805 | 0.575   | 0.585   | 0.566   |
| Light Gradient Boosting    | 1.0               | 1.0      | 1.0      | 1.0                  | 1.0         | 1.0             | 80.0 | 80.0 | 0.0  | 0.0  | 1.0   | 0.0   | 0.0   | 1.0     | 1.0     | 1.0     |
| Logistic Regression        | 0.5               | 0.5      | 0.436    | 0.412                | 0.606       | 0.459           | 33.0 | 48.5 | 31.5 | 47.0 | 0.5   | 0.849 | 1.0   | 0.495   | 0.547   | 0.5     |
| Naive Bayes                | 0.506             | 0.506    | 0.527    | 0.544                | 0.469       | 0.507           | 43.5 | 37.5 | 42.5 | 36.5 | 0.505 | 1.029 | 0.984 | 0.478   | 0.481   | 0.49    |
| Random Forest              | 0.834             | 0.834    | 0.836    | 0.831                | 0.844       | 0.84            | 66.5 | 67.5 | 12.5 | 13.5 | 0.831 | 5.25  | 0.203 | 0.924   | 0.924   | 0.924   |
| Support Vector Machine     | 0.516             | 0.516    | 0.487    | 0.475                | 0.531       | 0.516           | 38.0 | 42.5 | 37.5 | 42.0 | 0.515 | 1.065 | 0.941 | 0.532   | 0.539   | 0.525   |

## D3 = xor\_4\_a\_20s\_1600\_EDM-1\_01

| ML Algorithm               | Balanced Accuracy | Accuracy | F1 Score | Sensitivity (Recall) | Specificity | Precision (PPV) | TP   | TN   | FP   | FN   | NPV   | LR+   | LR-   | ROC AUC | PRC AUC | PRC APS |
|----------------------------|-------------------|----------|----------|----------------------|-------------|-----------------|------|------|------|------|-------|-------|-------|---------|---------|---------|
| Artificial Neural Network  | 0.5               | 0.5      | 0.537    | 0.581                | 0.4         | 0.5             | 46.5 | 32.0 | 48.0 | 33.5 | 0.5   | 1.0   | 0.95  | 0.5     | 0.523   | 0.529   |
| Category Gradient Boosting | 0.488             | 0.488    | 0.474    | 0.462                | 0.506       | 0.487           | 37.0 | 40.5 | 39.5 | 43.0 | 0.488 | 0.948 | 1.049 | 0.478   | 0.483   | 0.49    |
| Decision Tree              | 0.509             | 0.509    | 0.498    | 0.481                | 0.562       | 0.508           | 38.5 | 45.0 | 35.0 | 41.5 | 0.509 | 1.034 | 0.964 | 0.519   | 0.531   | 0.528   |
| Elastic Net                | 0.491             | 0.491    | 0.5      | 0.506                | 0.462       | 0.491           | 40.5 | 37.0 | 43.0 | 39.5 | 0.49  | 0.966 | 1.041 | 0.483   | 0.485   | 0.498   |
| ExSTraCS                   | 0.481             | 0.481    | 0.458    | 0.444                | 0.494       | 0.478           | 35.5 | 39.5 | 40.5 | 44.5 | 0.476 | 0.915 | 1.099 | 0.473   | 0.48    | 0.488   |
| Extreme Gradient Boosting  | 0.484             | 0.484    | 0.433    | 0.388                | 0.6         | 0.482           | 31.0 | 48.0 | 32.0 | 49.0 | 0.49  | 0.93  | 1.042 | 0.478   | 0.505   | 0.504   |
| Genetic Programming        | 0.5               | 0.5      | 0.667    | 1.0                  | 0.0         | 0.5             | 80.0 | 0.0  | 80.0 | 0.0  | 0.0   | 1.0   | 0.0   | 0.5     | 0.75    | 0.5     |
| Gradient Boosting          | 0.481             | 0.481    | 0.481    | 0.488                | 0.481       | 0.481           | 39.0 | 38.5 | 41.5 | 41.0 | 0.481 | 0.927 | 1.079 | 0.476   | 0.493   | 0.503   |
| K-Nearest Neighbors        | 0.475             | 0.475    | 0.465    | 0.425                | 0.55        | 0.476           | 34.0 | 44.0 | 36.0 | 46.0 | 0.478 | 0.907 | 1.093 | 0.481   | 0.505   | 0.507   |
| Light Gradient Boosting    | 0.478             | 0.478    | 0.43     | 0.425                | 0.494       | 0.473           | 34.0 | 39.5 | 40.5 | 46.0 | 0.477 | 0.899 | 1.095 | 0.453   | 0.48    | 0.487   |
| Logistic Regression        | 0.5               | 0.5      | 0.412    | 0.369                | 0.619       | 0.452           | 29.5 | 49.5 | 30.5 | 50.5 | 0.5   | 0.831 | 1.0   | 0.5     | 0.548   | 0.504   |
| Naive Bayes                | 0.497             | 0.497    | 0.528    | 0.569                | 0.444       | 0.497           | 45.5 | 35.5 | 44.5 | 34.5 | 0.497 | 0.989 | 1.014 | 0.509   | 0.514   | 0.522   |
| Random Forest              | 0.481             | 0.481    | 0.49     | 0.481                | 0.488       | 0.48            | 38.5 | 39.0 | 41.0 | 41.5 | 0.482 | 0.924 | 1.075 | 0.468   | 0.479   | 0.487   |
| Support Vector Machine     | 0.491             | 0.491    | 0.473    | 0.462                | 0.506       | 0.49            | 37.0 | 40.5 | 39.5 | 43.0 | 0.491 | 0.961 | 1.036 | 0.503   | 0.544   | 0.503   |

## D4 = xor\_5\_a\_20s\_1600\_EDM-1\_01

| ML Algorithm               | Balanced Accuracy | Accuracy | F1 Score | Sensitivity (Recall) | Specificity | Precision (PPV) | TP   | TN   | FP   | FN   | NPV   | LR+   | LR-   | ROC AUC | PRC AUC | PRC APS |
|----------------------------|-------------------|----------|----------|----------------------|-------------|-----------------|------|------|------|------|-------|-------|-------|---------|---------|---------|
| Artificial Neural Network  | 0.512             | 0.512    | 0.523    | 0.5                  | 0.506       | 0.514           | 40.0 | 40.5 | 39.5 | 40.0 | 0.512 | 1.057 | 0.954 | 0.504   | 0.509   | 0.518   |
| Category Gradient Boosting | 0.525             | 0.525    | 0.513    | 0.512                | 0.544       | 0.524           | 41.0 | 43.5 | 36.5 | 39.0 | 0.524 | 1.103 | 0.91  | 0.513   | 0.523   | 0.531   |
| Decision Tree              | 0.488             | 0.488    | 0.481    | 0.475                | 0.506       | 0.489           | 38.0 | 40.5 | 39.5 | 42.0 | 0.486 | 0.955 | 1.059 | 0.505   | 0.513   | 0.514   |
| Elastic Net                | 0.534             | 0.534    | 0.479    | 0.438                | 0.562       | 0.536           | 35.0 | 45.0 | 35.0 | 45.0 | 0.532 | 1.154 | 0.878 | 0.539   | 0.522   | 0.53    |
| ExSTraCS                   | 0.522             | 0.522    | 0.506    | 0.488                | 0.519       | 0.53            | 39.0 | 41.5 | 38.5 | 41.0 | 0.519 | 1.126 | 0.929 | 0.524   | 0.511   | 0.52    |
| Extreme Gradient Boosting  | 0.512             | 0.512    | 0.517    | 0.519                | 0.488       | 0.512           | 41.5 | 39.0 | 41.0 | 38.5 | 0.513 | 1.05  | 0.95  | 0.515   | 0.52    | 0.529   |
| Genetic Programming        | 0.5               | 0.5      | 0.667    | 1.0                  | 0.0         | 0.5             | 80.0 | 0.0  | 80.0 | 0.0  | 0.0   | 1.0   | 0.0   | 0.5     | 0.75    | 0.5     |
| Gradient Boosting          | 0.525             | 0.525    | 0.535    | 0.55                 | 0.5         | 0.524           | 44.0 | 40.0 | 40.0 | 36.0 | 0.527 | 1.101 | 0.901 | 0.505   | 0.518   | 0.526   |
| K-Nearest Neighbors        | 0.481             | 0.481    | 0.447    | 0.438                | 0.512       | 0.482           | 35.0 | 41.0 | 39.0 | 45.0 | 0.48  | 0.932 | 1.086 | 0.511   | 0.529   | 0.526   |
| Light Gradient Boosting    | 0.531             | 0.531    | 0.537    | 0.569                | 0.481       | 0.528           | 45.5 | 38.5 | 41.5 | 34.5 | 0.528 | 1.118 | 0.895 | 0.537   | 0.521   | 0.529   |
| Logistic Regression        | 0.525             | 0.525    | 0.525    | 0.525                | 0.531       | 0.525           | 42.0 | 42.5 | 37.5 | 38.0 | 0.525 | 1.105 | 0.904 | 0.542   | 0.523   | 0.53    |
| Naive Bayes                | 0.519             | 0.519    | 0.515    | 0.5                  | 0.519       | 0.519           | 40.0 | 41.5 | 38.5 | 40.0 | 0.518 | 1.077 | 0.931 | 0.529   | 0.523   | 0.53    |
| Random Forest              | 0.525             | 0.525    | 0.511    | 0.494                | 0.538       | 0.525           | 39.5 | 43.0 | 37.0 | 40.5 | 0.523 | 1.105 | 0.911 | 0.514   | 0.524   | 0.531   |
| Support Vector Machine     | 0.494             | 0.494    | 0.512    | 0.531                | 0.469       | 0.494           | 42.5 | 37.5 | 42.5 | 37.5 | 0.493 | 0.977 | 1.027 | 0.497   | 0.512   | 0.504   |

# Feature Importance Summary: D1 = xor\_2\_a\_20s\_1600\_EDM-1\_01

Sorted Median Mutual Information Scores

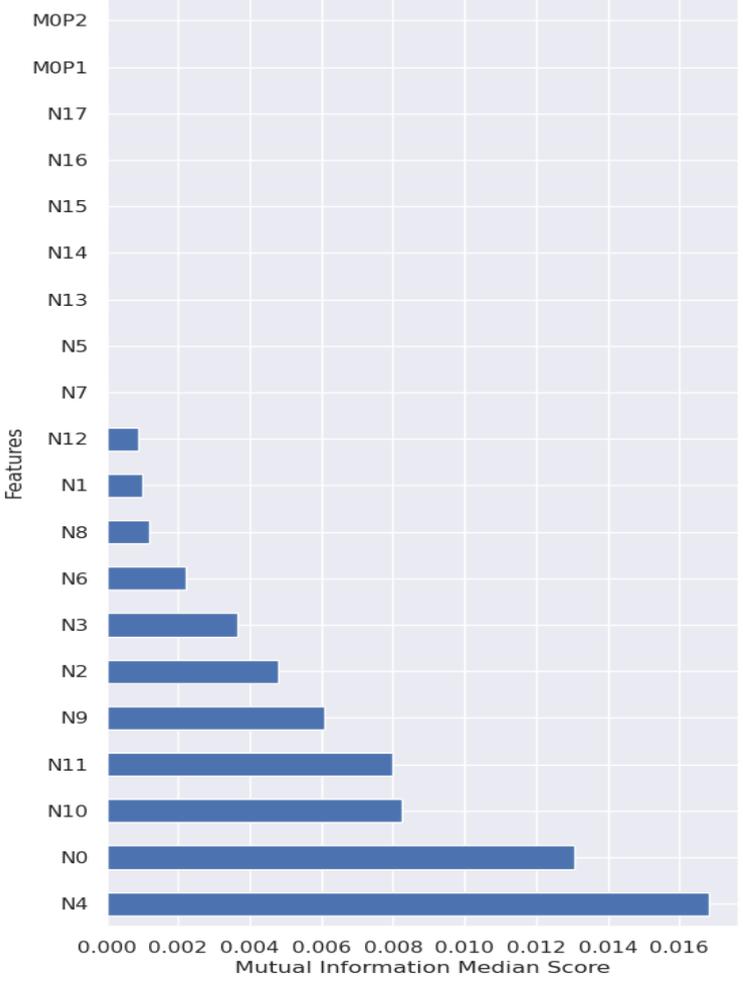

Sorted Median MultiSURF Scores

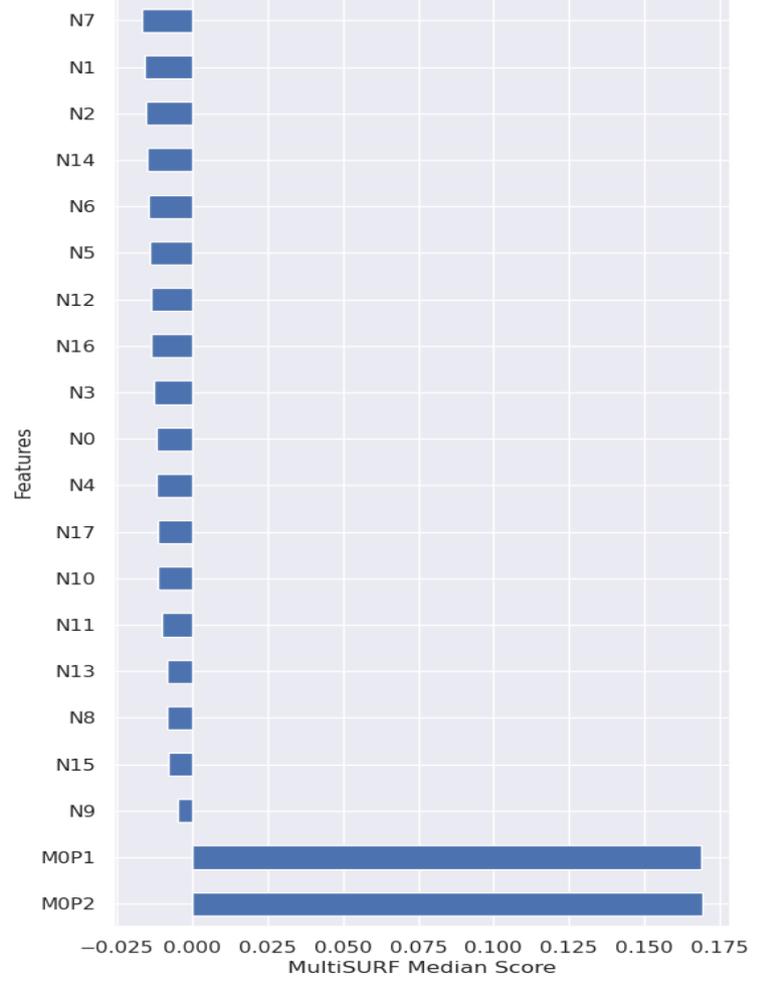

## Composite Feature Importance Plot (Normalized and Performance Weighted)

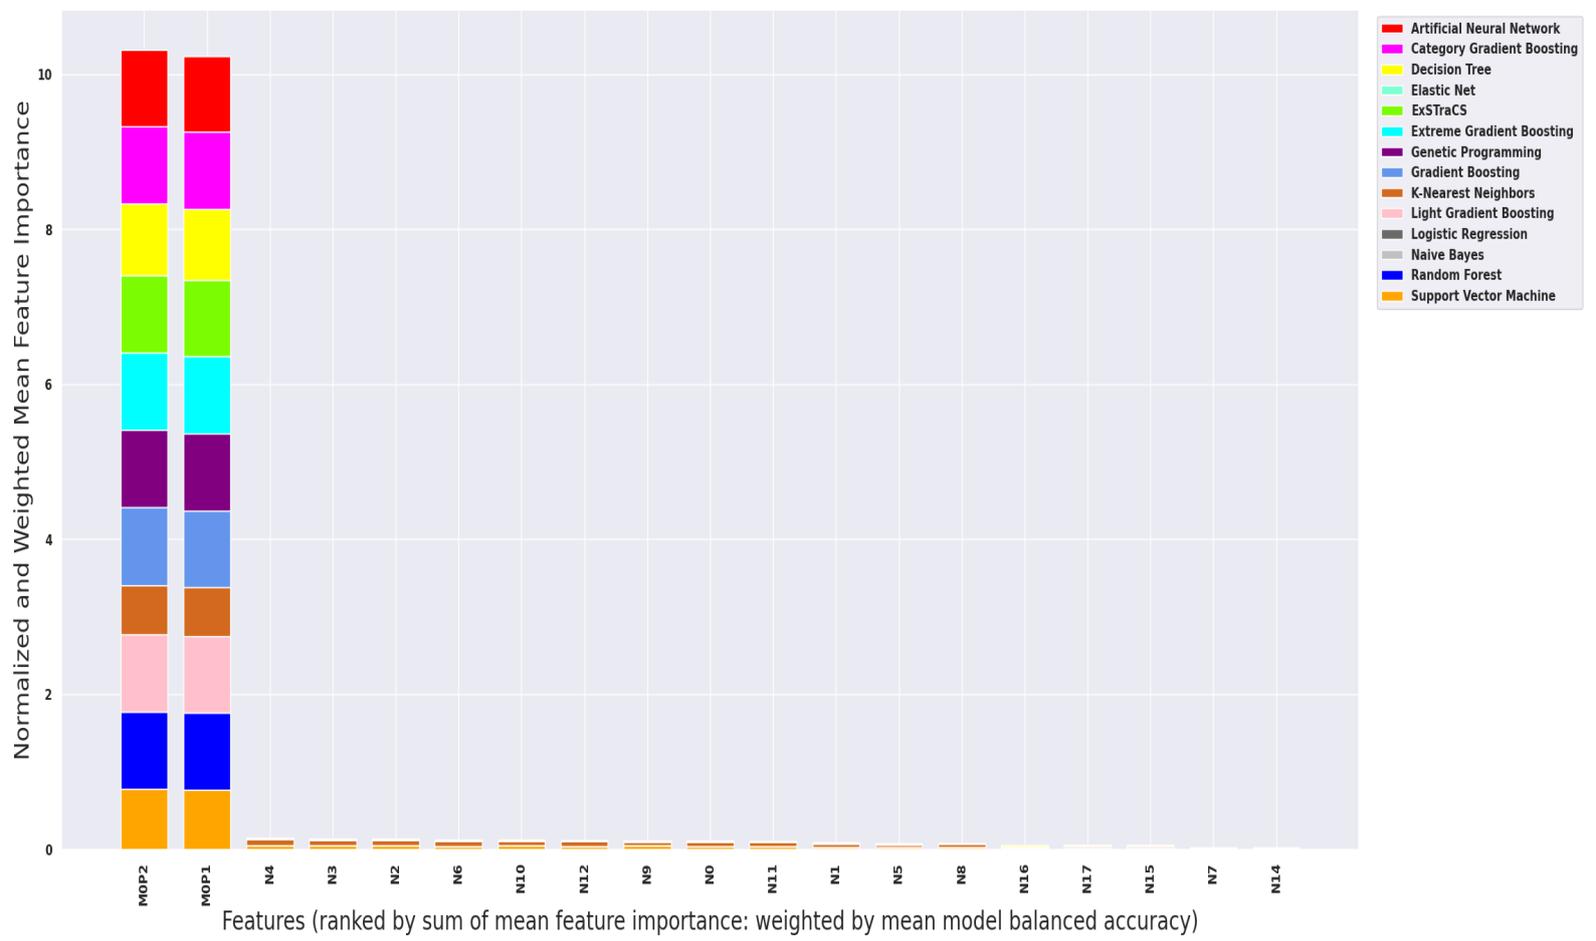

# Feature Importance Summary: D2 = xor\_3\_a\_20s\_1600\_EDM-1\_01

Sorted Median Mutual Information Scores

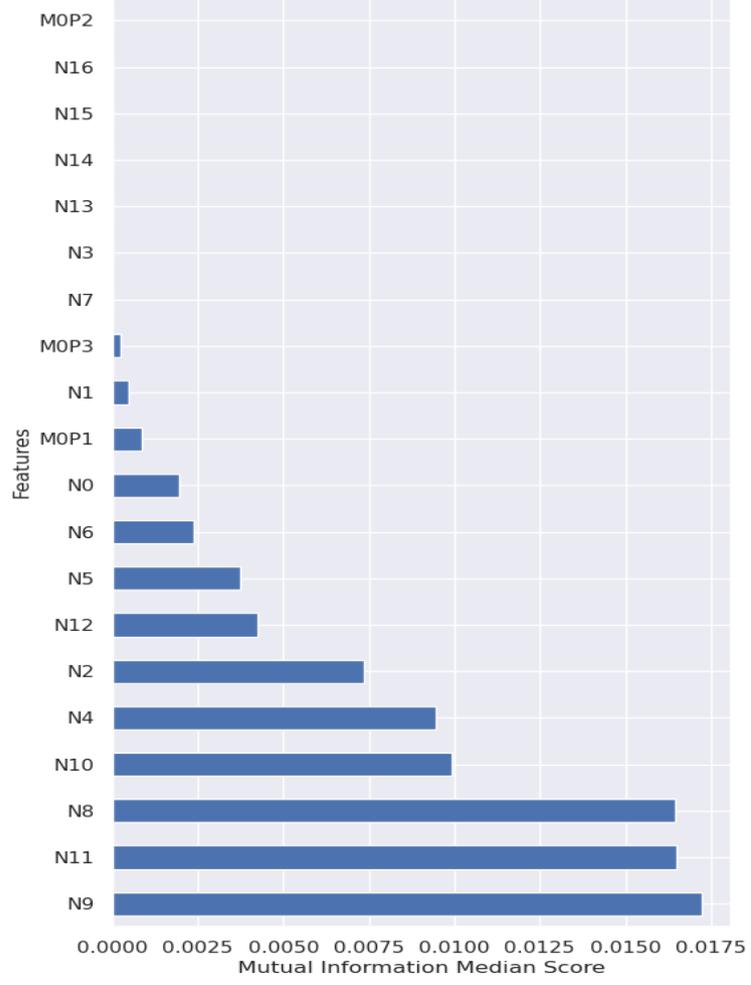

Sorted Median MultiSURF Scores

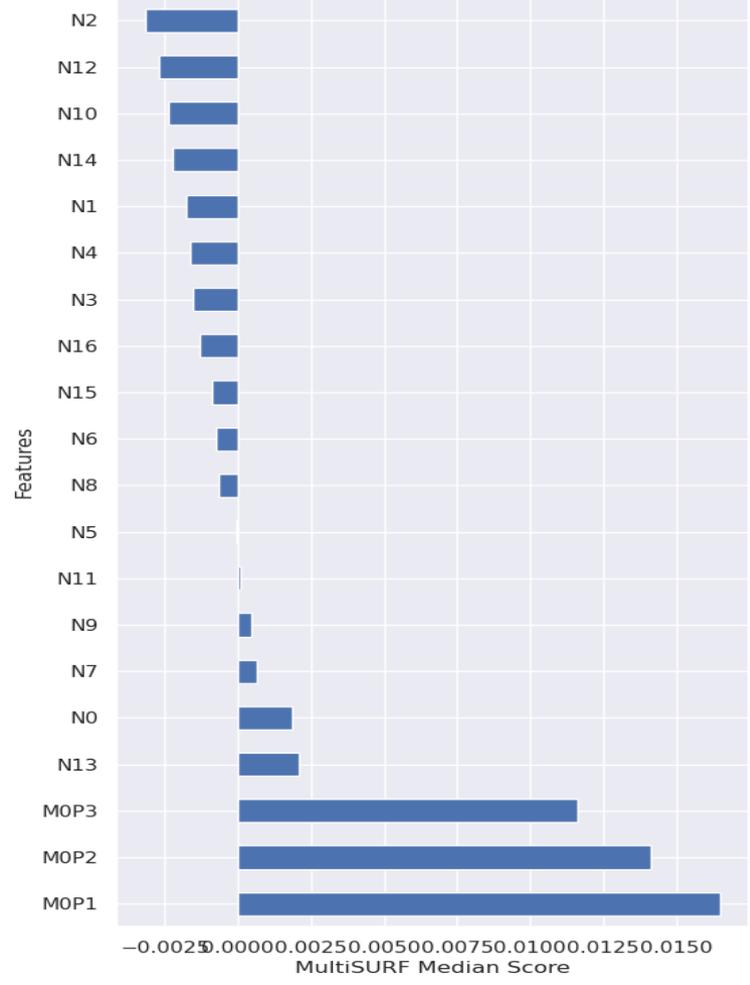

## Composite Feature Importance Plot (Normalized and Performance Weighted)

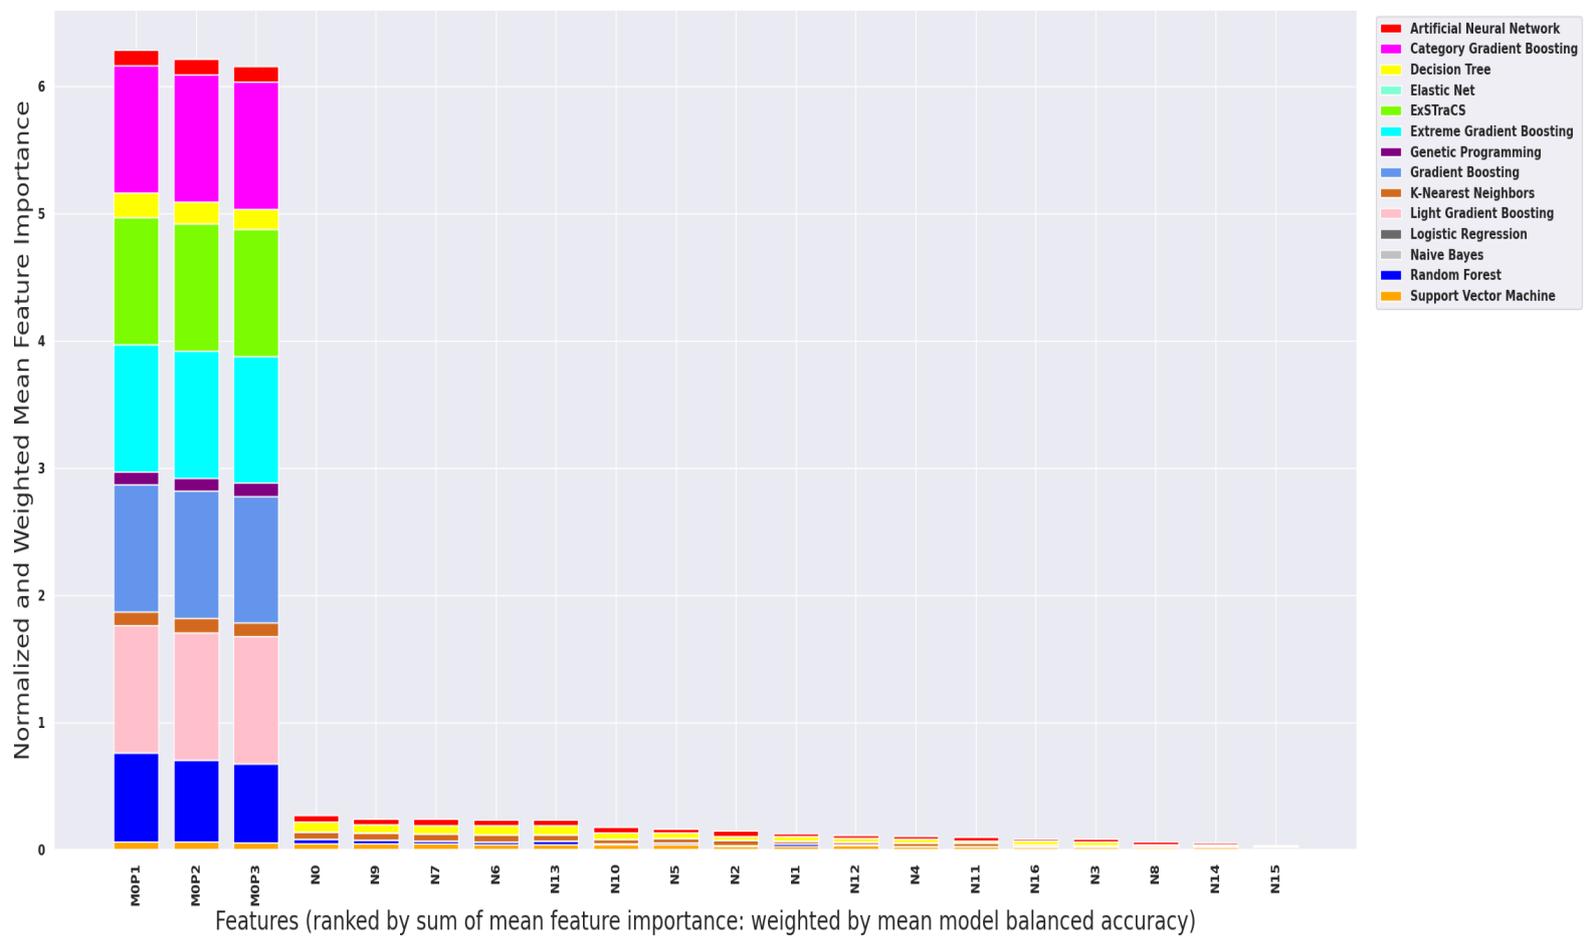

# Feature Importance Summary: D3 = xor\_4\_a\_20s\_1600\_EDM-1\_01

Sorted Median Mutual Information Scores

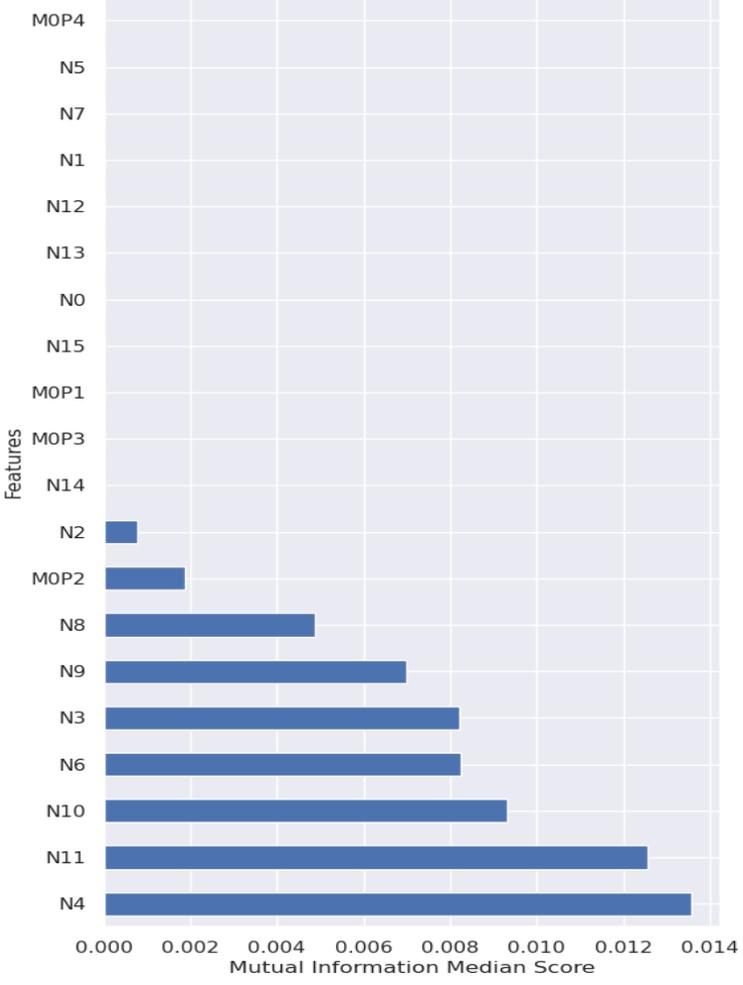

Sorted Median MultiSURF Scores

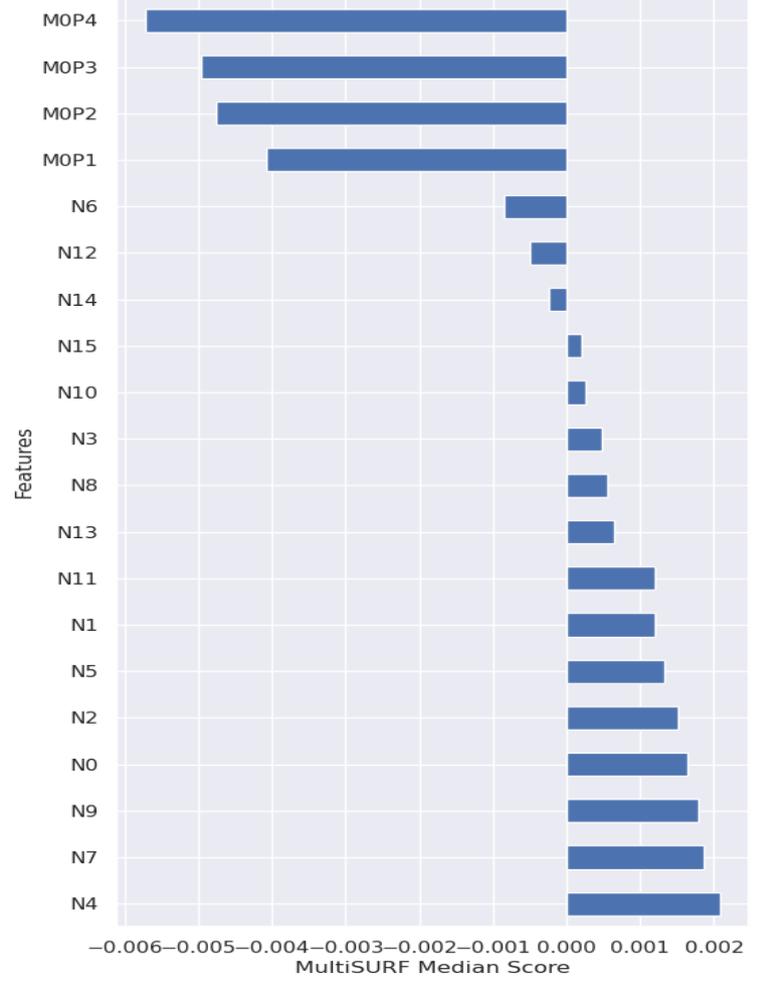

## Composite Feature Importance Plot (Normalized and Performance Weighted)

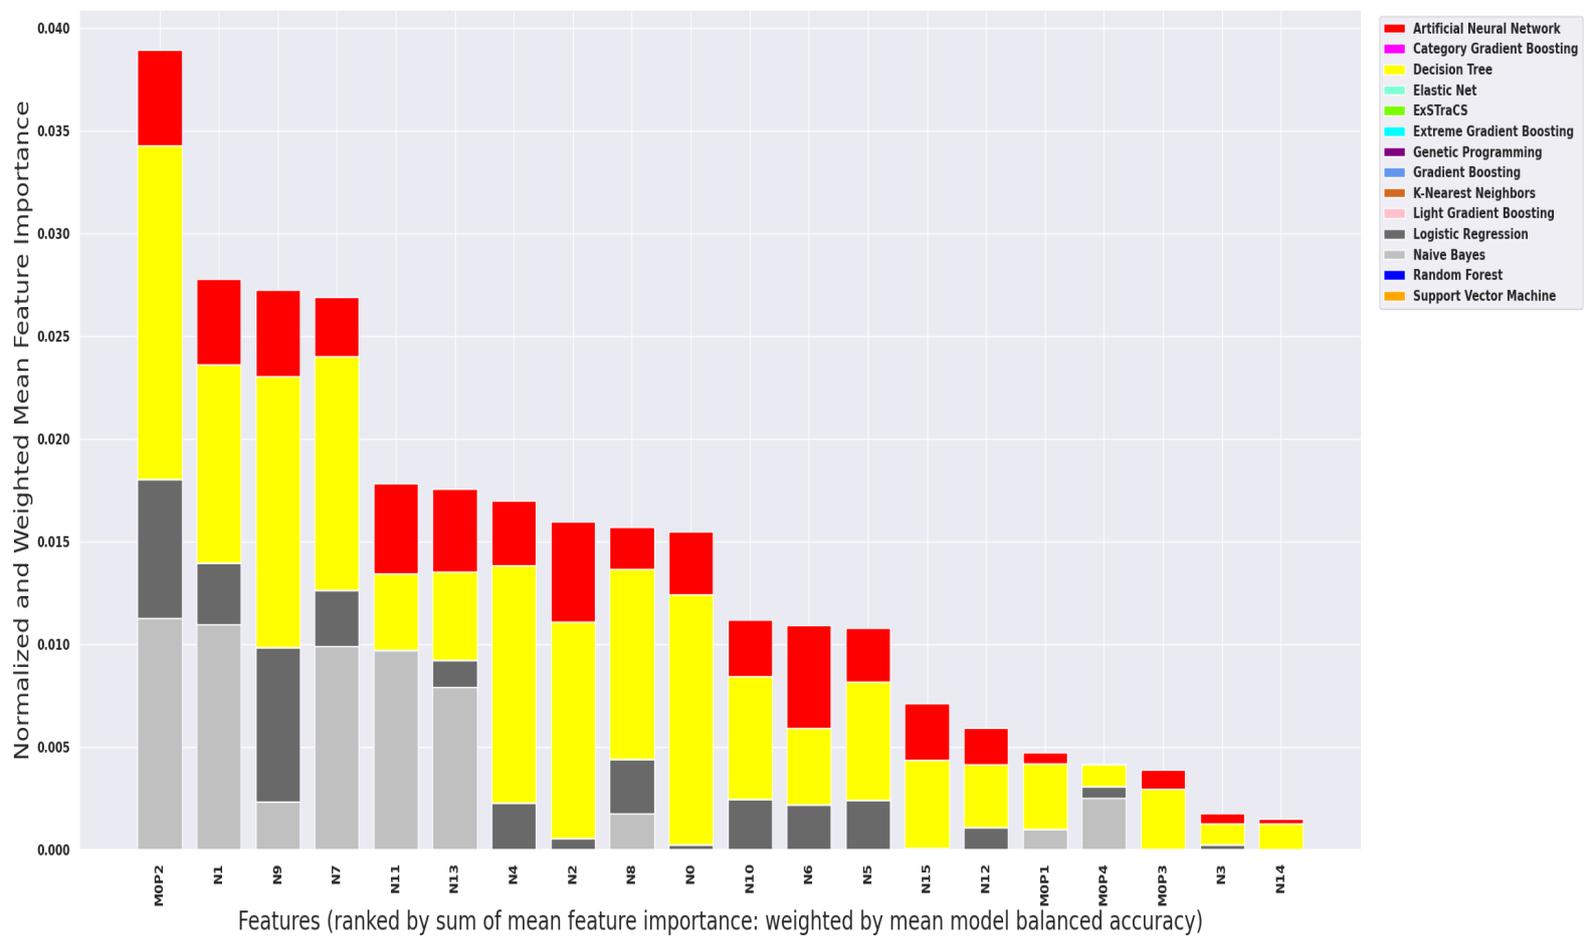

# Feature Importance Summary: D4 = xor\_5\_a\_20s\_1600\_EDM-1\_01

Sorted Median Mutual Information Scores

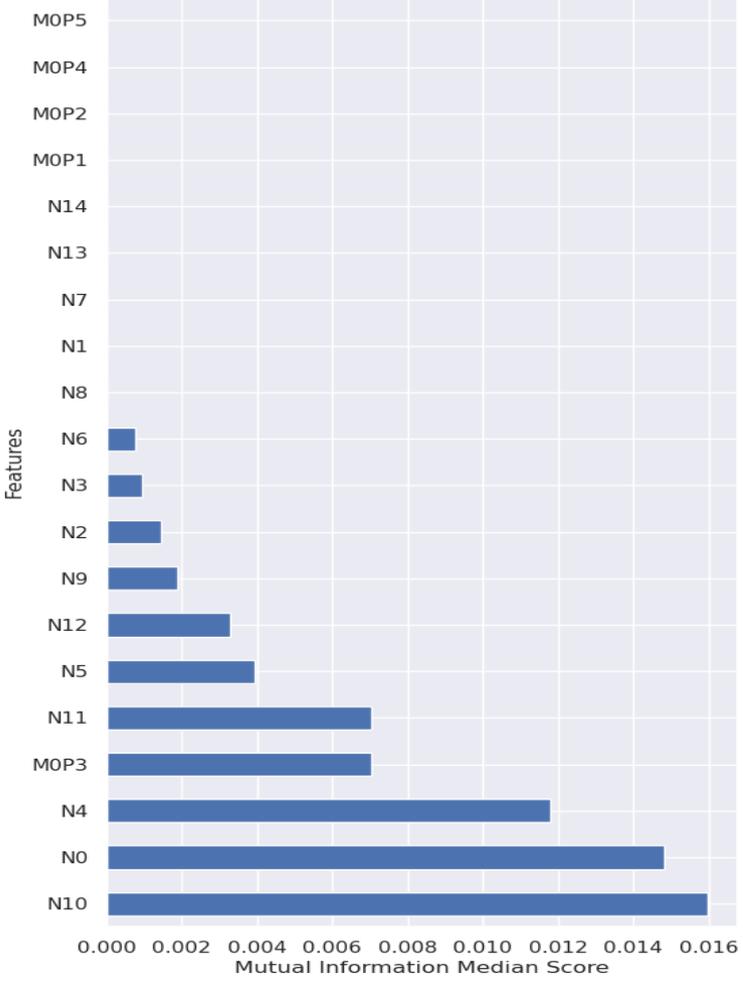

Sorted Median MultiSURF Scores

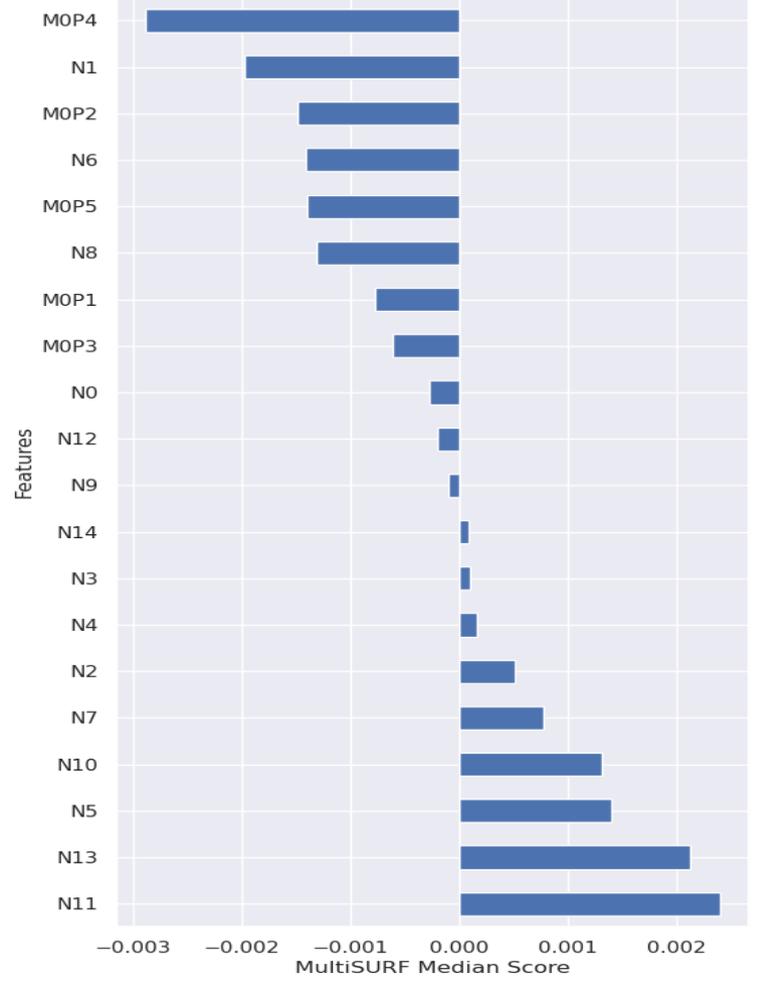

## Composite Feature Importance Plot (Normalized and Performance Weighted)

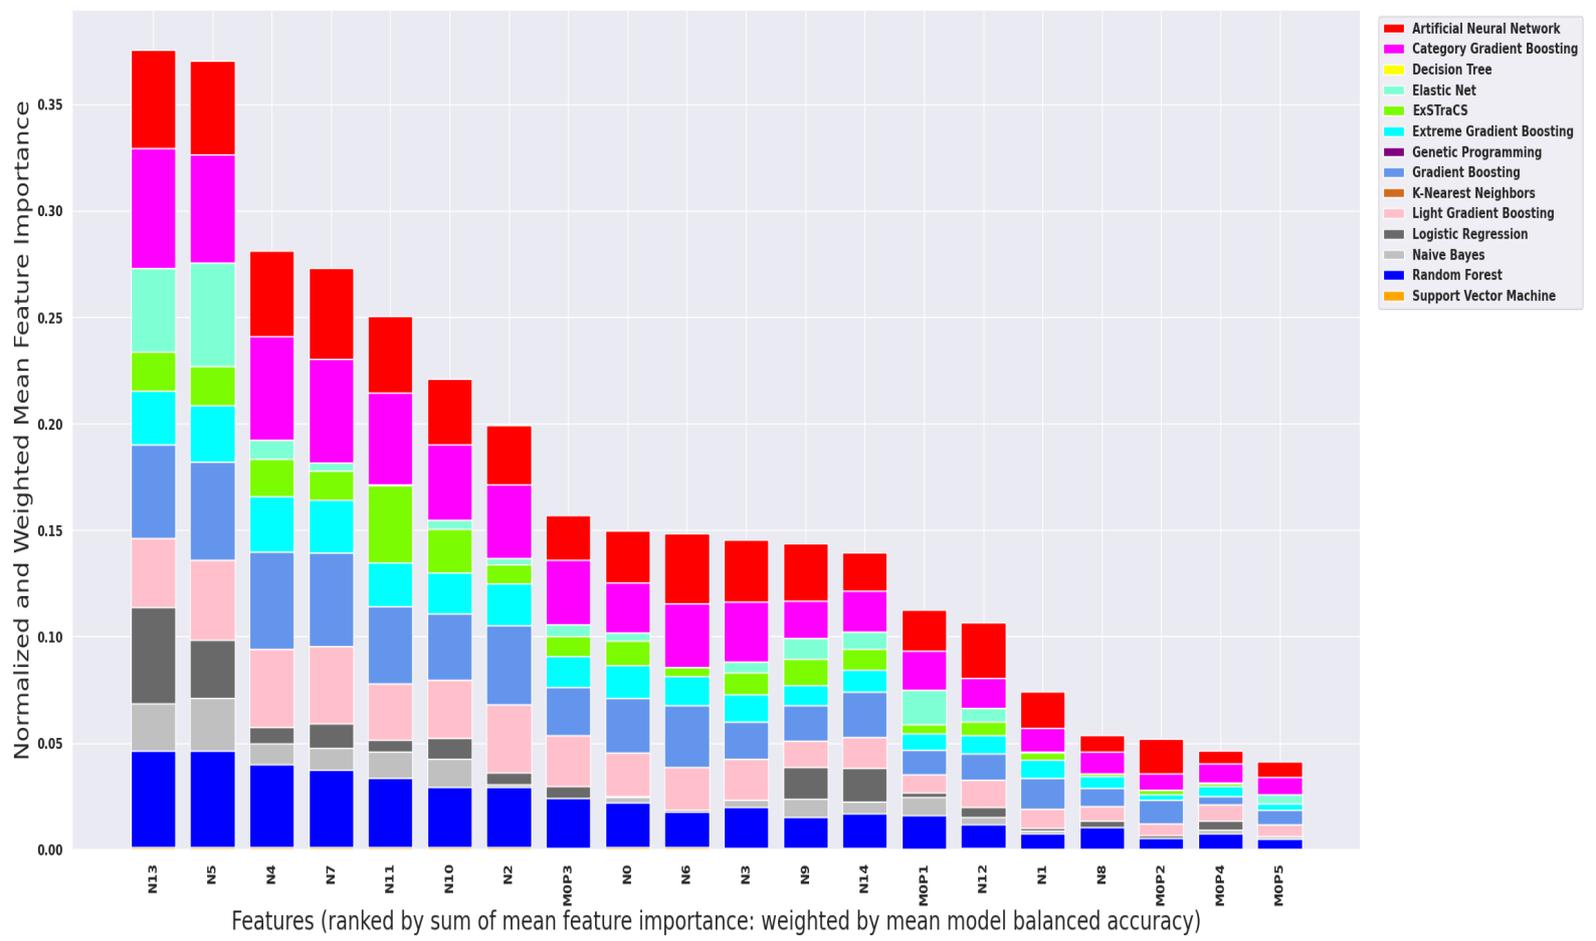

# Compare ML Performance Across Datasets

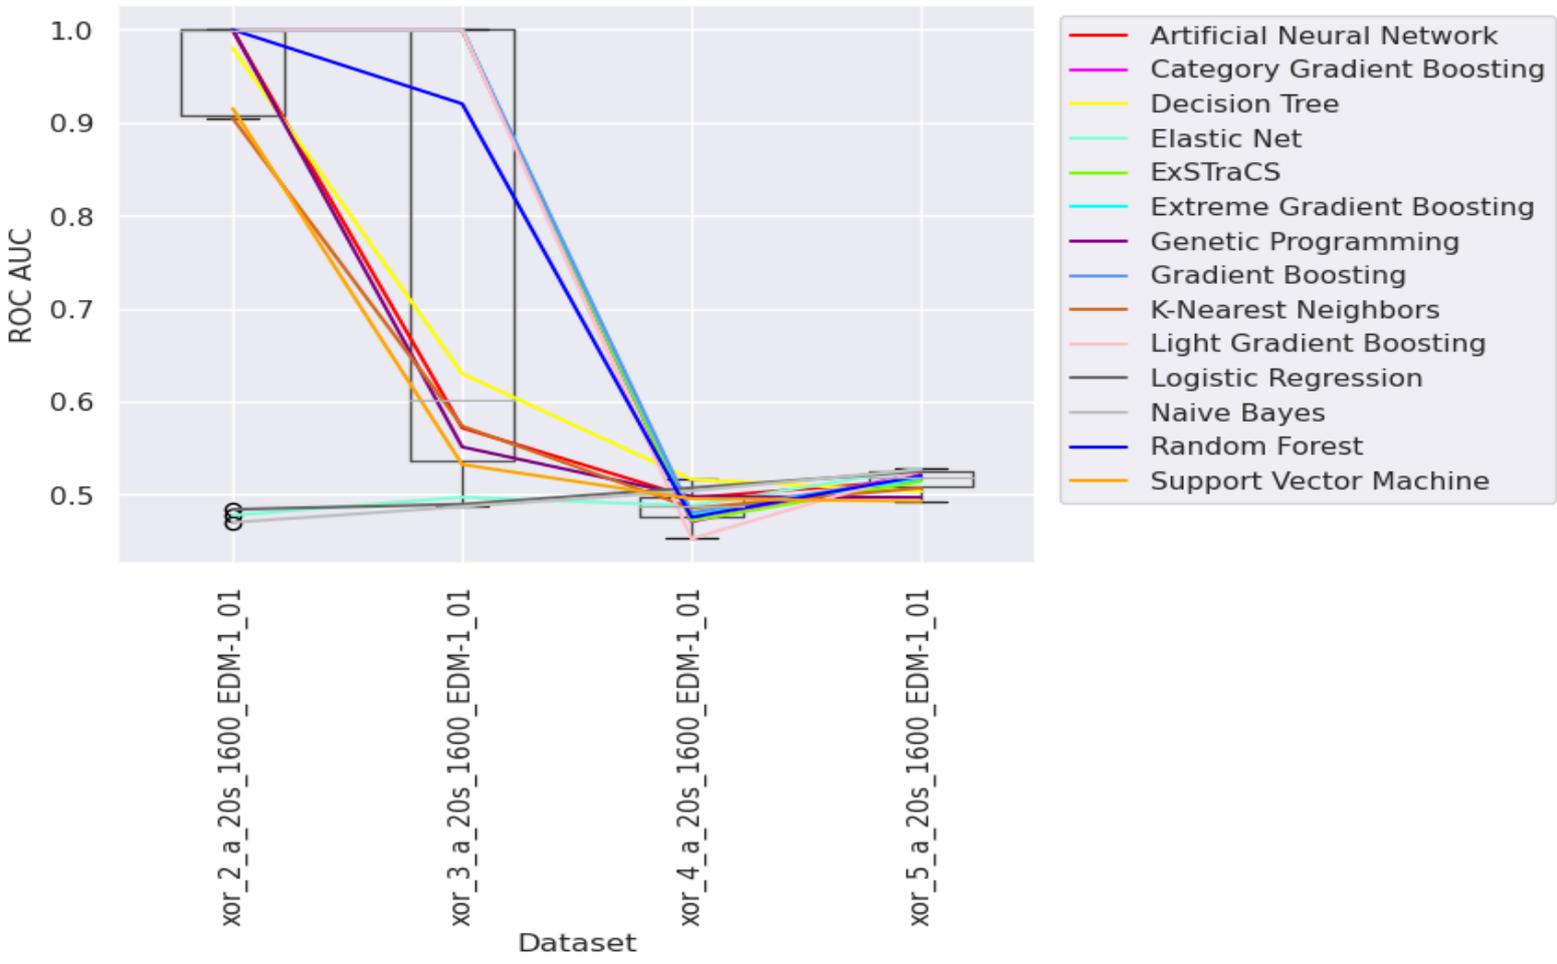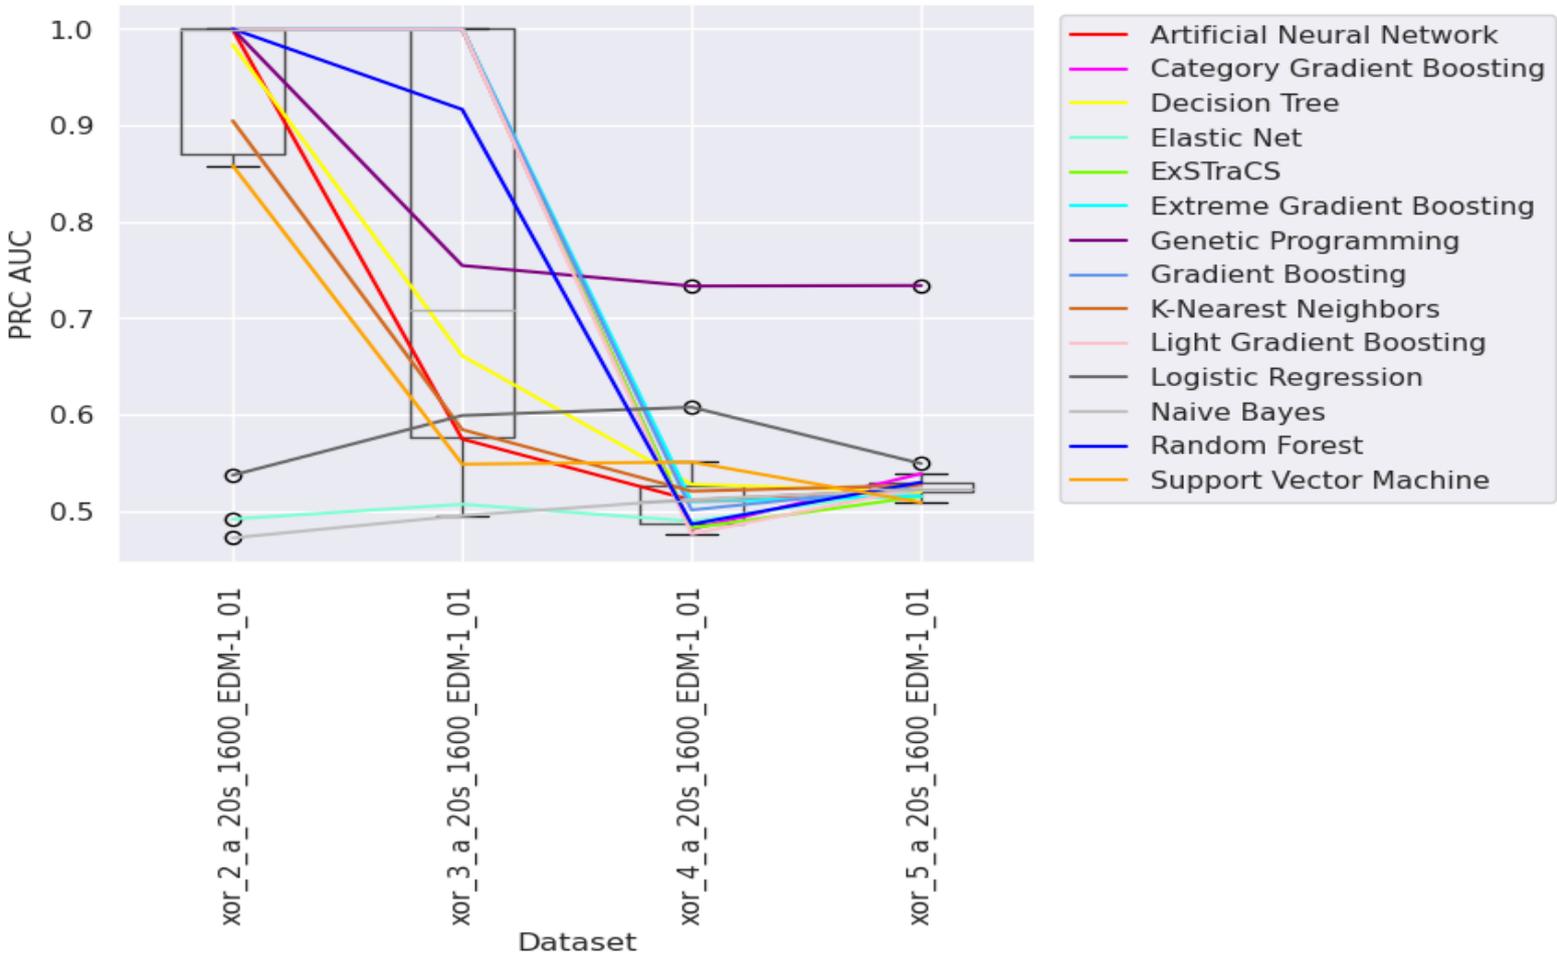

## Using Best Performing Algorithms (Kruskall Wallis Compare Datasets)

| Metrics              | P-Value | Best Alg_D1                | Median_D1 | Best Alg_D2                | Median_D2 | Best Alg_D3               | Median_D3 |
|----------------------|---------|----------------------------|-----------|----------------------------|-----------|---------------------------|-----------|
| Balanced Accuracy    | 0.0     | Category Gradient Boosting | 1.0       | Category Gradient Boosting | 1.0       | Decision Tree             | 0.5094    |
| Accuracy             | 0.0     | Category Gradient Boosting | 1.0       | Category Gradient Boosting | 1.0       | Decision Tree             | 0.5094    |
| F1 Score             | 0.0     | Category Gradient Boosting | 1.0       | Category Gradient Boosting | 1.0       | Genetic Programming       | 0.6667    |
| Sensitivity (Recall) | 0.1614  | Artificial Neural Network  | 1.0       | Category Gradient Boosting | 1.0       | Genetic Programming       | 1.0       |
| Specificity          | 0.0001  | Artificial Neural Network  | 1.0       | Category Gradient Boosting | 1.0       | Logistic Regression       | 0.6188    |
| Precision (PPV)      | 0.0     | Artificial Neural Network  | 1.0       | Category Gradient Boosting | 1.0       | Decision Tree             | 0.5083    |
| TP                   | 0.1614  | Artificial Neural Network  | 80.0      | Category Gradient Boosting | 80.0      | Genetic Programming       | 80.0      |
| TN                   | 0.0001  | Artificial Neural Network  | 80.0      | Category Gradient Boosting | 80.0      | Logistic Regression       | 49.5      |
| FP                   | 0.1221  | Elastic Net                | 45.0      | Genetic Programming        | 80.0      | Genetic Programming       | 80.0      |
| FN                   | 0.338   | Logistic Regression        | 42.5      | Logistic Regression        | 47.0      | Logistic Regression       | 50.5      |
| NPV                  | 0.0     | Artificial Neural Network  | 1.0       | Category Gradient Boosting | 1.0       | Decision Tree             | 0.5091    |
| LR+                  | 0.0     | Support Vector Machine     | 9.6508    | Random Forest              | 5.25      | Decision Tree             | 1.0336    |
| LR-                  | 0.4471  | Elastic Net                | 1.1488    | Elastic Net                | 1.0571    | ExSTraCS                  | 1.0994    |
| ROC AUC              | 0.0     | Artificial Neural Network  | 1.0       | Category Gradient Boosting | 1.0       | Decision Tree             | 0.5194    |
| PRC AUC              | 0.0     | Artificial Neural Network  | 1.0       | Category Gradient Boosting | 1.0       | Genetic Programming       | 0.75      |
| PRC APS              | 0.0     | Category Gradient Boosting | 1.0       | Category Gradient Boosting | 1.0       | Artificial Neural Network | 0.5287    |

| Metrics              | P-Value | Best Alg_D4                | Median_D4 |
|----------------------|---------|----------------------------|-----------|
| Balanced Accuracy    | 0.0     | Elastic Net                | 0.5344    |
| Accuracy             | 0.0     | Elastic Net                | 0.5344    |
| F1 Score             | 0.0     | Genetic Programming        | 0.6667    |
| Sensitivity (Recall) | 0.1614  | Genetic Programming        | 1.0       |
| Specificity          | 0.0001  | Elastic Net                | 0.5625    |
| Precision (PPV)      | 0.0     | Elastic Net                | 0.5358    |
| TP                   | 0.1614  | Genetic Programming        | 80.0      |
| TN                   | 0.0001  | Elastic Net                | 45.0      |
| FP                   | 0.1221  | Genetic Programming        | 80.0      |
| FN                   | 0.338   | Elastic Net                | 45.0      |
| NPV                  | 0.0     | Elastic Net                | 0.5324    |
| LR+                  | 0.0     | Elastic Net                | 1.1543    |
| LR-                  | 0.4471  | K-Nearest Neighbors        | 1.0859    |
| ROC AUC              | 0.0     | Logistic Regression        | 0.5423    |
| PRC AUC              | 0.0     | Genetic Programming        | 0.75      |
| PRC APS              | 0.0     | Category Gradient Boosting | 0.531     |

## Pipeline Runtime Summary

### xor\_2\_a\_20s\_1600\_EDM-1\_01

| Pipeline Component                      | Phase | Time (sec)         |
|-----------------------------------------|-------|--------------------|
| Exploratory Analysis                    | 1     | 3.145313262939453  |
| Scale and Impute                        | 2     | 0.6574831008911133 |
| Mutual Information (Feature Importance) | 3     | 1.3483061790466309 |
| MultiSURF (Feature Importance)          | 3     | 145.609313249588   |
| Feature Selection                       | 4     | 1.3617405891418457 |
| Artificial Neural Network(Modeling)     | 5     | 3195.1384270191197 |
| Category Gradient Boosting(Modeling)    | 5     | 9461.663464069366  |
| Decision Tree(Modeling)                 | 5     | 22.22918462753296  |
| Elastic Net(Modeling)                   | 5     | 31.828819274902344 |
| ExSTraCS(Modeling)                      | 5     | 17171.630984783173 |
| Extreme Gradient Boosting(Modeling)     | 5     | 6485.944395780563  |
| Genetic Programming(Modeling)           | 5     | 10761.848734378817 |
| Gradient Boosting(Modeling)             | 5     | 2851.1358003616333 |
| K-Nearest Neighbors(Modeling)           | 5     | 198.48015809059143 |
| Light Gradient Boosting(Modeling)       | 5     | 638.7833018302917  |
| Logistic Regression(Modeling)           | 5     | 25.598609685897827 |
| Naive Bayes(Modeling)                   | 5     | 1.25596022605896   |
| Random Forest(Modeling)                 | 5     | 5262.394448518753  |
| Support Vector Machine(Modeling)        | 5     | 7251.915402412415  |
| Stats Summary                           | 6     | 32.52580666542053  |

### xor\_3\_a\_20s\_1600\_EDM-1\_01

| Pipeline Component                      | Phase | Time (sec)         |
|-----------------------------------------|-------|--------------------|
| Exploratory Analysis                    | 1     | 2.576210260391236  |
| Scale and Impute                        | 2     | 0.5576777458190918 |
| Mutual Information (Feature Importance) | 3     | 1.1732399463653564 |
| MultiSURF (Feature Importance)          | 3     | 145.8568000793457  |
| Feature Selection                       | 4     | 1.1193673610687256 |
| Artificial Neural Network(Modeling)     | 5     | 3341.891882181168  |
| Category Gradient Boosting(Modeling)    | 5     | 9430.814992904665  |
| Decision Tree(Modeling)                 | 5     | 26.315868139266968 |
| Elastic Net(Modeling)                   | 5     | 35.87022829055786  |
| ExSTraCS(Modeling)                      | 5     | 21987.367011785507 |
| Extreme Gradient Boosting(Modeling)     | 5     | 8511.398111343384  |
| Genetic Programming(Modeling)           | 5     | 12497.989577531816 |
| Gradient Boosting(Modeling)             | 5     | 5599.801402807236  |
| K-Nearest Neighbors(Modeling)           | 5     | 354.5848412513733  |
| Light Gradient Boosting(Modeling)       | 5     | 1345.3816685676577 |
| Logistic Regression(Modeling)           | 5     | 28.244282007217407 |
| Naive Bayes(Modeling)                   | 5     | 1.772735357284546  |
| Random Forest(Modeling)                 | 5     | 8100.918696403503  |
| Support Vector Machine(Modeling)        | 5     | 5004.429639339447  |
| Stats Summary                           | 6     | 36.44613432884216  |

### xor\_4\_a\_20s\_1600\_EDM-1\_01

| Pipeline Component                      | Phase | Time (sec)         |
|-----------------------------------------|-------|--------------------|
| Exploratory Analysis                    | 1     | 2.5925300121307373 |
| Scale and Impute                        | 2     | 0.5919315814971924 |
| Mutual Information (Feature Importance) | 3     | 1.215752363204956  |
| MultiSURF (Feature Importance)          | 3     | 145.2647740840912  |
| Feature Selection                       | 4     | 1.129136323928833  |
| Artificial Neural Network(Modeling)     | 5     | 1559.968222141266  |
| Category Gradient Boosting(Modeling)    | 5     | 8251.8798828125    |
| Decision Tree(Modeling)                 | 5     | 24.51191997528076  |
| Elastic Net(Modeling)                   | 5     | 36.1223030090332   |
| ExSTraCS(Modeling)                      | 5     | 40393.85705780983  |
| Extreme Gradient Boosting(Modeling)     | 5     | 3431.322578191757  |
| Genetic Programming(Modeling)           | 5     | 11621.343264102936 |
| Gradient Boosting(Modeling)             | 5     | 5961.704326629639  |
| K-Nearest Neighbors(Modeling)           | 5     | 1800.2933955192566 |
| Light Gradient Boosting(Modeling)       | 5     | 641.5503857135773  |
| Logistic Regression(Modeling)           | 5     | 55.14080047607422  |
| Naive Bayes(Modeling)                   | 5     | 1.904062271118164  |
| Random Forest(Modeling)                 | 5     | 5058.18715429306   |
| Support Vector Machine(Modeling)        | 5     | 6449.941166162491  |
| Stats Summary                           | 6     | 33.2203209400177   |

### xor\_5\_a\_20s\_1600\_EDM-1\_01

| Pipeline Component                      | Phase | Time (sec)         |
|-----------------------------------------|-------|--------------------|
| Exploratory Analysis                    | 1     | 3.118624210357666  |
| Scale and Impute                        | 2     | 0.5569663047790527 |
| Mutual Information (Feature Importance) | 3     | 1.167409896850586  |
| MultiSURF (Feature Importance)          | 3     | 143.57500457763672 |
| Feature Selection                       | 4     | 1.3206396102905271 |
| Artificial Neural Network(Modeling)     | 5     | 3860.554863929749  |
| Category Gradient Boosting(Modeling)    | 5     | 8903.73549079895   |
| Decision Tree(Modeling)                 | 5     | 27.224817991256717 |
| Elastic Net(Modeling)                   | 5     | 37.27079224586487  |
| ExSTraCS(Modeling)                      | 5     | 38740.87343645096  |
| Extreme Gradient Boosting(Modeling)     | 5     | 7037.292566776276  |
| Genetic Programming(Modeling)           | 5     | 11410.549880743029 |
| Gradient Boosting(Modeling)             | 5     | 5077.902999639511  |
| K-Nearest Neighbors(Modeling)           | 5     | 814.6629889011383  |
| Light Gradient Boosting(Modeling)       | 5     | 1764.252518415451  |
| Logistic Regression(Modeling)           | 5     | 35.97503304481506  |
| Naive Bayes(Modeling)                   | 5     | 1.643091917037964  |
| Random Forest(Modeling)                 | 5     | 5280.75880074501   |
| Support Vector Machine(Modeling)        | 5     | 5337.419611930847  |
| Stats Summary                           | 6     | 37.68315410614014  |
