# Supplementary material for: STREAMLINE: An Automated Machine Learning Pipeline for Biomedicine Applied to Examine the Utility of Photography-Based Phenotypes for OSA Prediction Across International Sleep Centers
Source: arXiv:2312.05461 ancillary file (2023-12-09)
Supplement: Supplementary file 8 [file xor_nofs_exp_STREAMLINE_Report.pdf]

# STREAMLINE Testing Data Evaluation Report: 2023-10-01 20:28:19.662910

## General Pipeline Settings:

CV Partitions: 10  
Partition Method: Stratified  
Categorical Cutoff: 2  
Statistical Significance Cutoff: 0.05  
Random Seed: 42  
Run From Notebook: False

## Feature Importance/Selection Settings:

Use Mutual Information: True  
Use MultiSURF: True  
Use TURF: False  
TURF Cutoff: 0.5  
MultiSURF Instance Subset: 2000  
Max Features to Keep: 2000  
Filter Poor Features: False  
Top Features to Display: 40  
Export Feature Importance Plot: True

## ML Modeling Algorithms:

Artificial Neural Network: True  
Category Gradient Boosting: True  
Decision Tree: True  
Elastic Net: True  
ExSTraCS: True  
Extreme Gradient Boosting: True  
Genetic Programming: True  
Gradient Boosting: True  
K-Nearest Neighbors: True  
Light Gradient Boosting: True  
Logistic Regression: True  
Naive Bayes: True  
Random Forest: True  
Support Vector Machine: True  
XCS: False  
eLCS: False

## Modeling Settings:

Primary Metric: balanced\_accuracy  
Training Subsample for KNN,ANN,SVM,and XGB: 0  
Uniform Feature Importance Estimation (Models): True  
Hyperparameter Sweep Number of Trials: 200  
Hyperparameter Timeout: 900  
Export Hyperparameter Sweep Plots: False

## LCS Settings (eLCS,XCS,ExSTraCS):

Do LCS Hyperparameter Sweep: False  
nu: 1  
Training Iterations: 200000  
N (Rule Population Size): 2000  
LCS Hyperparameter Sweep Timeout: 1200

## Stats and Figure Settings:

Export ROC Plot: True  
Export PRC Plot: True  
Export Metric Boxplots: True  
Export Feature Importance Boxplots: True  
Metric Weighting Composite FI Plots: balanced\_accuracy  
Top Model Features To Display: 40

## EDA and Processing Settings:

Engineering Missingness Cutoff: 0.5  
Cleaning Missingness Cutoff: 0.5  
Correlation Removal Threshold: 1.0  
List of Exploratory Analysis Ran: ['Describe', 'Univariate Analysis', 'Feature Correlation']  
List of Exploratory Plots Saved: ['Describe', 'Univariate Analysis', 'Feature Correlation']  
Use Data Scaling: True  
Use Data Imputation: True  
Use Multivariate Imputation: True  
Overwrite CV Datasets: True

## Target Dataset(s):

D1 = xor\_2\_a\_20s\_1600\_EDM-1\_01  
D2 = xor\_3\_a\_20s\_1600\_EDM-1\_01  
D3 = xor\_4\_a\_20s\_1600\_EDM-1\_01  
D4 = xor\_5\_a\_20s\_1600\_EDM-1\_01

## Target Data Settings:

Data Path: /home/ryanurb/idata/datasets/xor\_set  
Output Path: /home/ryanurb/idata/output  
Experiment Name: xor\_nofs\_exp  
Class Label: Class  
Instance Label: None  
Match Label: None  
Ignored Features: None  
Specified Categorical Features: None  
Specified Quantitative Features: None

## Univariate Analysis of Each Dataset (Top 10 Features for Each)

### D1 = xor\_2\_a\_20s\_1600\_EDM-1\_01

| Feature | p-value            | Test-statistic | Test-name           |
|---------|--------------------|----------------|---------------------|
| N10     | 0.2008159114176192 | 329187.5       | Mann-Whitney U Test |
| N16     | 0.2161131395026099 | 330469.0       | Mann-Whitney U Test |
| N14     | 0.2177044748605101 | 330157.5       | Mann-Whitney U Test |
| N12     | 0.219701376834725  | 309757.0       | Mann-Whitney U Test |
| M0P2    | 0.2247856260437952 | 309727.0       | Mann-Whitney U Test |
| N6      | 0.3325323994182377 | 311781.5       | Mann-Whitney U Test |
| N17     | 0.4024957721639753 | 326097.0       | Mann-Whitney U Test |
| N5      | 0.4049861226590078 | 326404.5       | Mann-Whitney U Test |
| N13     | 0.4220032930197887 | 314864.0       | Mann-Whitney U Test |
| N0      | 0.523664179550604  | 315495.0       | Mann-Whitney U Test |

### D2 = xor\_3\_a\_20s\_1600\_EDM-1\_01

| Feature | p-value            | Test-statistic | Test-name           |
|---------|--------------------|----------------|---------------------|
| N1      | 0.0627337878366858 | 304417.0       | Mann-Whitney U Test |
| N0      | 0.0910751126707113 | 334260.5       | Mann-Whitney U Test |
| N6      | 0.1328817197220447 | 307911.5       | Mann-Whitney U Test |
| N9      | 0.1705225466340459 | 308678.0       | Mann-Whitney U Test |
| M0P1    | 0.1959159346687257 | 330938.5       | Mann-Whitney U Test |
| N7      | 0.3618337703410067 | 312358.0       | Mann-Whitney U Test |
| N15     | 0.4519178816847056 | 315966.0       | Mann-Whitney U Test |
| N12     | 0.6283966964155301 | 315956.0       | Mann-Whitney U Test |
| M0P3    | 0.637291337012047  | 316016.0       | Mann-Whitney U Test |
| N2      | 0.6658888818546207 | 316331.0       | Mann-Whitney U Test |

### D3 = xor\_4\_a\_20s\_1600\_EDM-1\_01

| Feature | p-value            | Test-statistic | Test-name           |
|---------|--------------------|----------------|---------------------|
| M0P2    | 0.0398778601679427 | 337466.0       | Mann-Whitney U Test |
| N9      | 0.1159345401469505 | 332276.0       | Mann-Whitney U Test |
| N11     | 0.2467408986646957 | 327160.0       | Mann-Whitney U Test |
| M0P4    | 0.2562882495187207 | 310373.5       | Mann-Whitney U Test |
| N1      | 0.4123734834476052 | 313408.5       | Mann-Whitney U Test |
| N8      | 0.4533372546131419 | 314808.5       | Mann-Whitney U Test |
| N2      | 0.4538014359208079 | 313690.5       | Mann-Whitney U Test |
| N6      | 0.4975936546344156 | 314324.0       | Mann-Whitney U Test |
| N7      | 0.5099863357899403 | 325557.5       | Mann-Whitney U Test |
| N13     | 0.5245440373971155 | 314878.0       | Mann-Whitney U Test |

### D4 = xor\_5\_a\_20s\_1600\_EDM-1\_01

| Feature | p-value            | Test-statistic | Test-name           |
|---------|--------------------|----------------|---------------------|
| N13     | 0.0213637537754956 | 338747.5       | Mann-Whitney U Test |
| N5      | 0.030316904724263  | 301642.5       | Mann-Whitney U Test |
| N14     | 0.1689647199913863 | 309932.0       | Mann-Whitney U Test |
| M0P1    | 0.1718939792980206 | 331622.0       | Mann-Whitney U Test |
| N10     | 0.2440534842431895 | 329083.5       | Mann-Whitney U Test |
| M0P5    | 0.2975384753029626 | 311206.0       | Mann-Whitney U Test |
| N4      | 0.299435231416699  | 311249.5       | Mann-Whitney U Test |
| N9      | 0.3198095781608477 | 313902.5       | Mann-Whitney U Test |
| N7      | 0.3486654469538642 | 312163.5       | Mann-Whitney U Test |
| M0P4    | 0.3629442966393856 | 312361.0       | Mann-Whitney U Test |

# Dataset and Model Prediction Summary: D1 = xor\_2\_a\_20s\_1600\_EDM-1\_01

## Data Processing/Counts Summary

|           | Instances | Total Features | Categorical Features | Quantitative Features | Missing Values | Missing Percent | Class 0 | Class 1 |
|-----------|-----------|----------------|----------------------|-----------------------|----------------|-----------------|---------|---------|
| Original  | 1600      | 20             | 0                    | 20                    | 0              | 0.0             | 800     | 800     |
| C1        | 1600      | 20             | 0                    | 20                    | 0              | 0.0             | 800     | 800     |
| E1        | 1600      | 20             | 0                    | 20                    | 0              | 0.0             | 800     | 800     |
| C2        | 1600      | 20             | 0                    | 20                    | 0              | 0.0             | 800     | 800     |
| C3        | 1600      | 20             | 0                    | 20                    | 0              | 0.0             | 800     | 800     |
| E2        | 1600      | 20             | 0                    | 20                    | 0              | 0.0             | 800     | 800     |
| C4        | 1600      | 20             | 0                    | 20                    | 0              | 0.0             | 800     | 800     |
| Processed | 1600      | 20             | 0                    | 20                    | 0              | 0.0             | 800     | 800     |

## Cleaning (C) and Engineering (E) Elements

- \* C1 - Remove instances with no outcome and features to ignore
- \* E1 - Add missingness features
- \* C2 - Remove features with invariance or high missingness
- \* C3 - Remove instances with high missingness
- \* E2 - Add one-hot-encoding of categorical features
- \* C4 - Remove highly correlated features

## Class Balance (Processed)

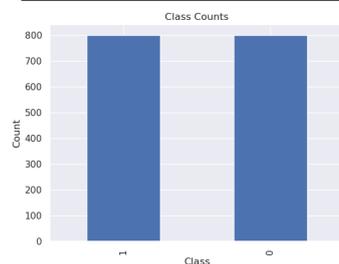

## Feature Correlations (Pearson)

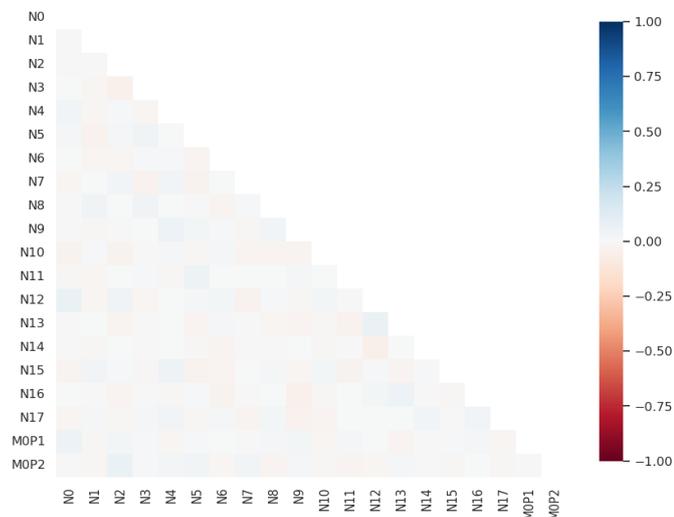

## Top ML Algorithm Results (Averaged Over CV Runs):

|                                                                |
|----------------------------------------------------------------|
| Best (ROC_AUC): Category Gradient Boosting (TIE) = 1.000       |
| Best (Balanced Acc.): Category Gradient Boosting (TIE) = 1.000 |
| Best (F1 Score): Category Gradient Boosting (TIE) = 1.000      |
| Best (PRC AUC): Category Gradient Boosting (TIE) = 1.000       |
| Best (PRC APS): Category Gradient Boosting (TIE) = 1.000       |

## ROC

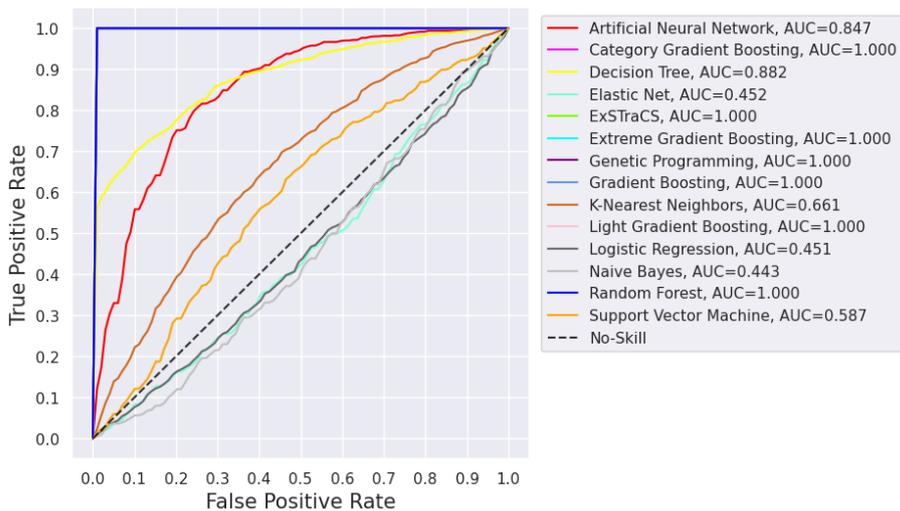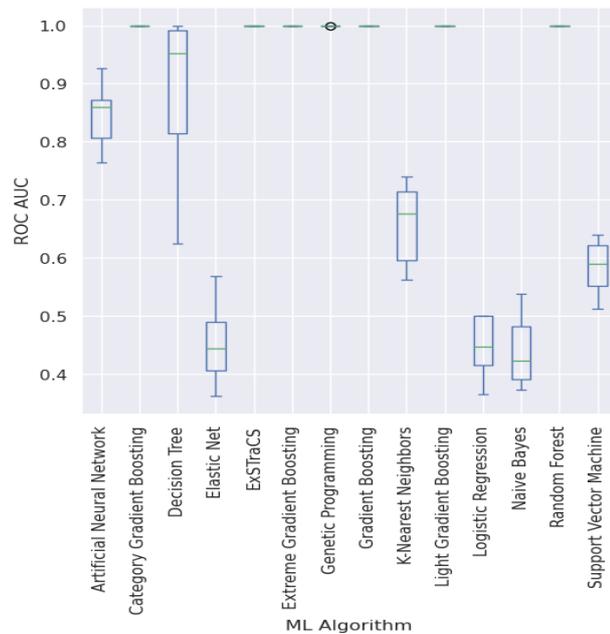

## PRC

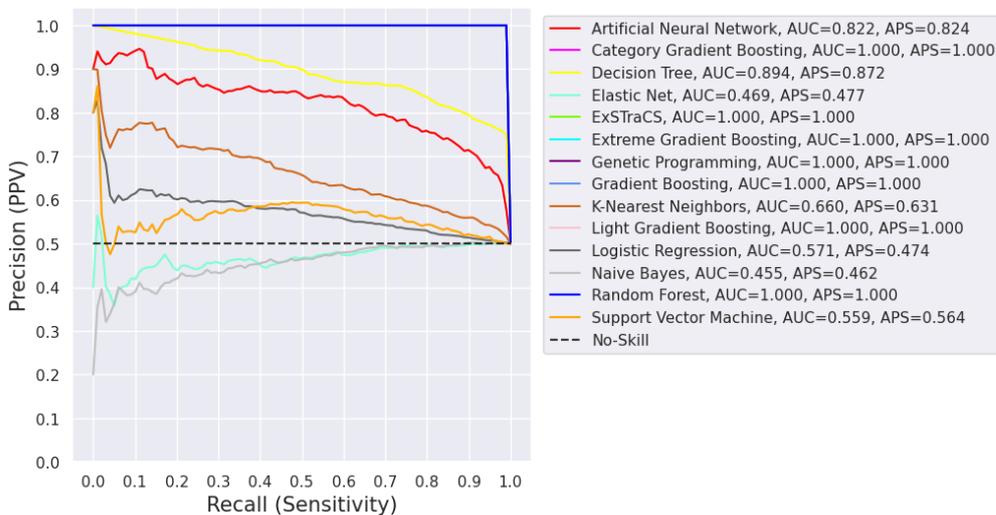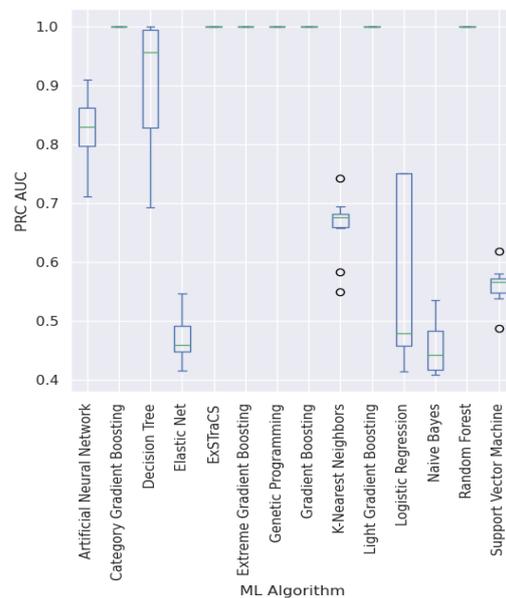

# Dataset and Model Prediction Summary: D2 = xor\_3\_a\_20s\_1600\_EDM-1\_01

## Data Processing/Counts Summary

|           | Instances | Total Features | Categorical Features | Quantitative Features | Missing Values | Missing Percent | Class 0 | Class 1 |
|-----------|-----------|----------------|----------------------|-----------------------|----------------|-----------------|---------|---------|
| Original  | 1600      | 20             | 0                    | 20                    | 0              | 0.0             | 800     | 800     |
| C1        | 1600      | 20             | 0                    | 20                    | 0              | 0.0             | 800     | 800     |
| E1        | 1600      | 20             | 0                    | 20                    | 0              | 0.0             | 800     | 800     |
| C2        | 1600      | 20             | 0                    | 20                    | 0              | 0.0             | 800     | 800     |
| C3        | 1600      | 20             | 0                    | 20                    | 0              | 0.0             | 800     | 800     |
| E2        | 1600      | 20             | 0                    | 20                    | 0              | 0.0             | 800     | 800     |
| C4        | 1600      | 20             | 0                    | 20                    | 0              | 0.0             | 800     | 800     |
| Processed | 1600      | 20             | 0                    | 20                    | 0              | 0.0             | 800     | 800     |

## Cleaning (C) and Engineering (E) Elements

- \* C1 - Remove instances with no outcome and features to ignore
- \* E1 - Add missingness features
- \* C2 - Remove features with invariance or high missingness
- \* C3 - Remove instances with high missingness
- \* E2 - Add one-hot-encoding of categorical features
- \* C4 - Remove highly correlated features

## Class Balance (Processed)

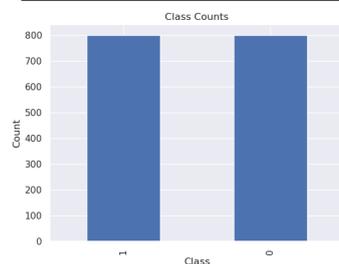

## Feature Correlations (Pearson)

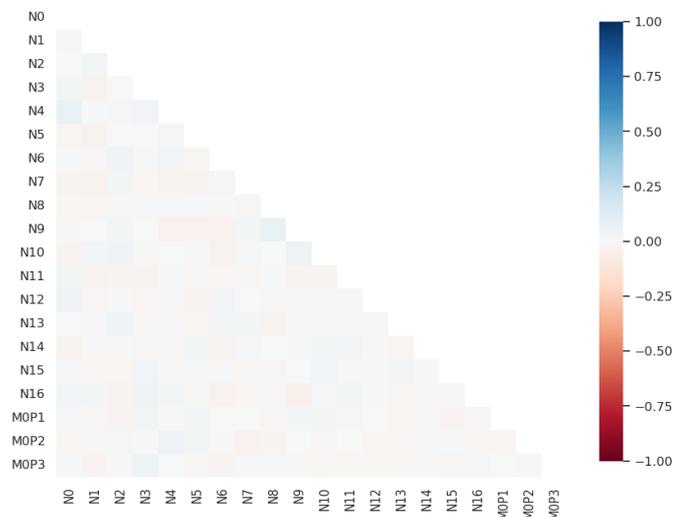

## Top ML Algorithm Results (Averaged Over CV Runs):

|                                                                |
|----------------------------------------------------------------|
| Best (ROC_AUC): Category Gradient Boosting (TIE) = 1.000       |
| Best (Balanced Acc.): Category Gradient Boosting (TIE) = 1.000 |
| Best (F1 Score): Category Gradient Boosting (TIE) = 1.000      |
| Best (PRC AUC): Category Gradient Boosting (TIE) = 1.000       |
| Best (PRC APS): Category Gradient Boosting (TIE) = 1.000       |

## ROC

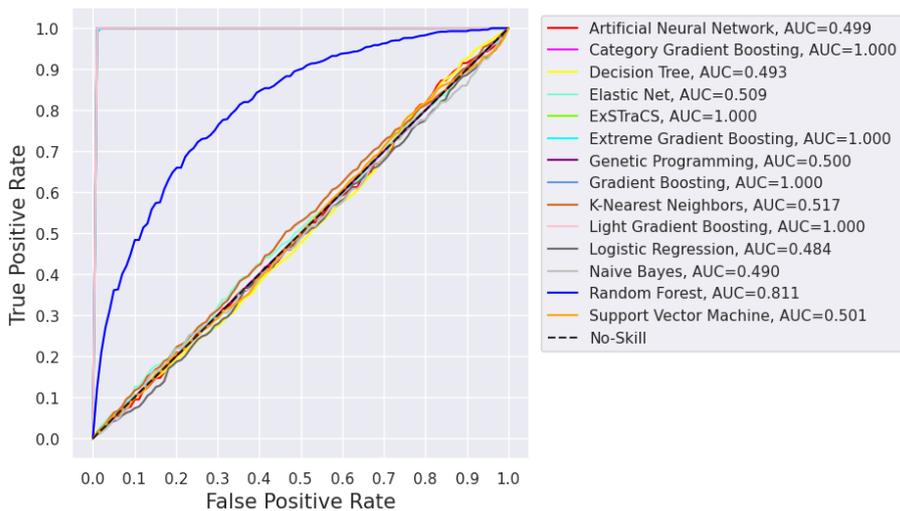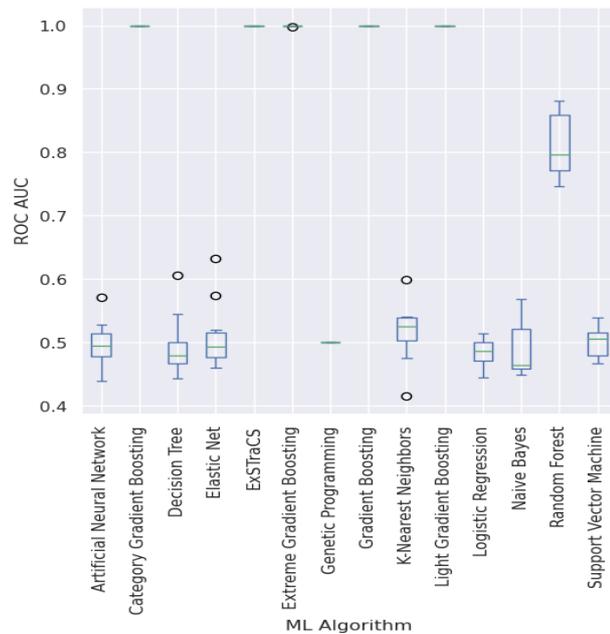

## PRC

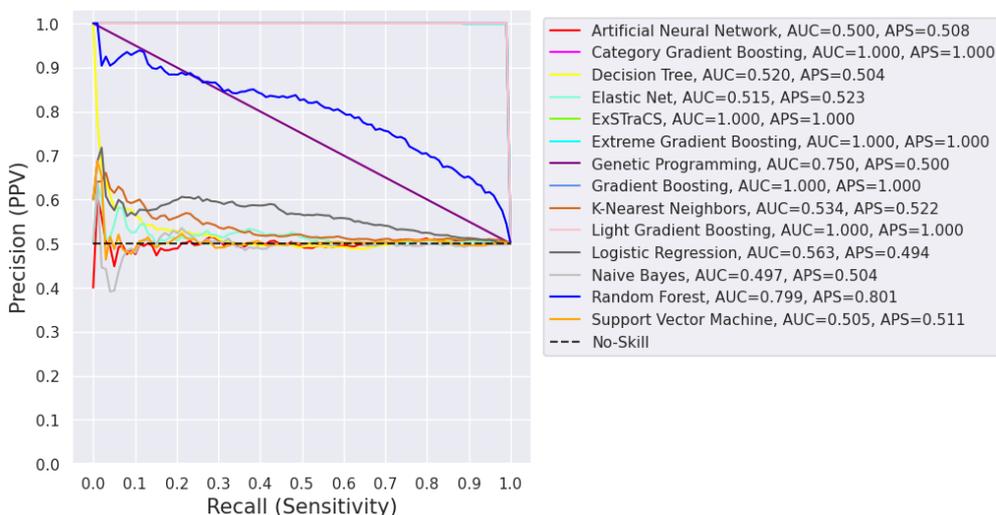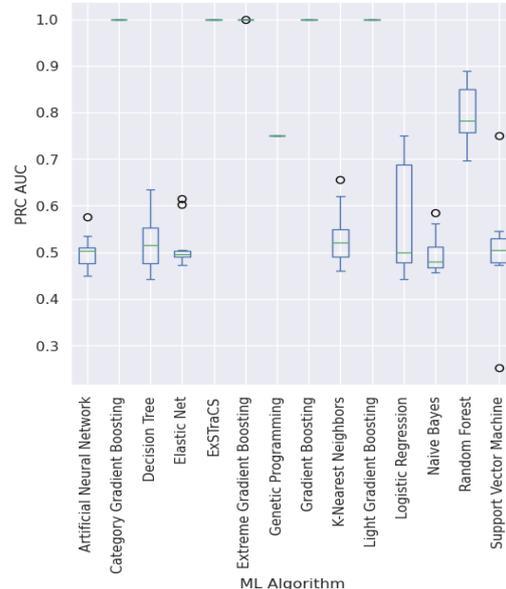

# Dataset and Model Prediction Summary: D3 = xor\_4\_a\_20s\_1600\_EDM-1\_01

## Data Processing/Counts Summary

|           | Instances | Total Features | Categorical Features | Quantitative Features | Missing Values | Missing Percent | Class 0 | Class 1 |
|-----------|-----------|----------------|----------------------|-----------------------|----------------|-----------------|---------|---------|
| Original  | 1600      | 20             | 0                    | 20                    | 0              | 0.0             | 800     | 800     |
| C1        | 1600      | 20             | 0                    | 20                    | 0              | 0.0             | 800     | 800     |
| E1        | 1600      | 20             | 0                    | 20                    | 0              | 0.0             | 800     | 800     |
| C2        | 1600      | 20             | 0                    | 20                    | 0              | 0.0             | 800     | 800     |
| C3        | 1600      | 20             | 0                    | 20                    | 0              | 0.0             | 800     | 800     |
| E2        | 1600      | 20             | 0                    | 20                    | 0              | 0.0             | 800     | 800     |
| C4        | 1600      | 20             | 0                    | 20                    | 0              | 0.0             | 800     | 800     |
| Processed | 1600      | 20             | 0                    | 20                    | 0              | 0.0             | 800     | 800     |

## Cleaning (C) and Engineering (E) Elements

- \* C1 - Remove instances with no outcome and features to ignore
- \* E1 - Add missingness features
- \* C2 - Remove features with invariance or high missingness
- \* C3 - Remove instances with high missingness
- \* E2 - Add one-hot-encoding of categorical features
- \* C4 - Remove highly correlated features

## Class Balance (Processed)

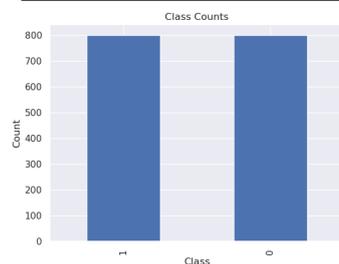

## Feature Correlations (Pearson)

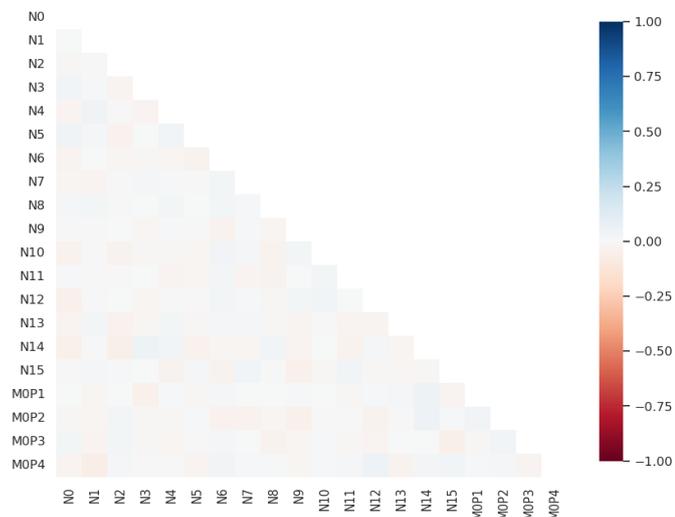

## Top ML Algorithm Results (Averaged Over CV Runs):

- Best (ROC\_AUC): ExSTraCS = 0.980
- Best (Balanced Acc.): ExSTraCS = 0.922
- Best (F1 Score): ExSTraCS = 0.919
- Best (PRC AUC): ExSTraCS = 0.981
- Best (PRC APS): ExSTraCS = 0.981

## ROC

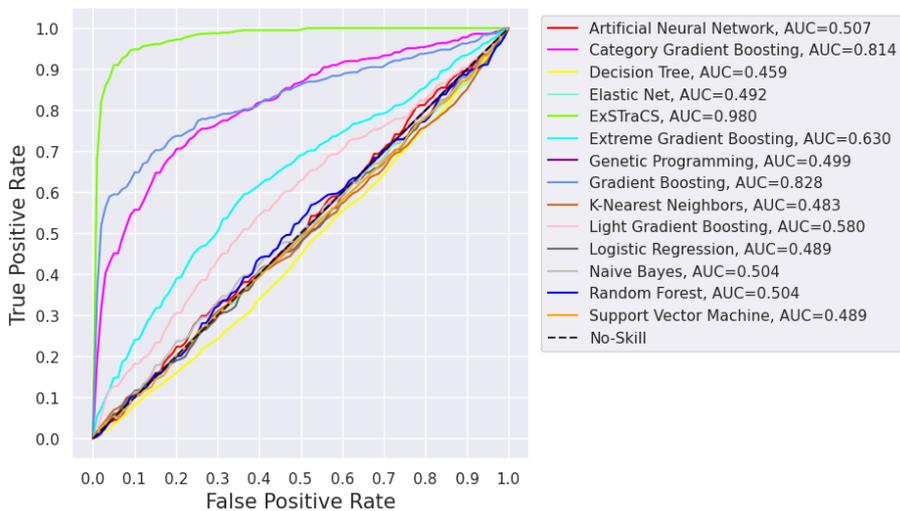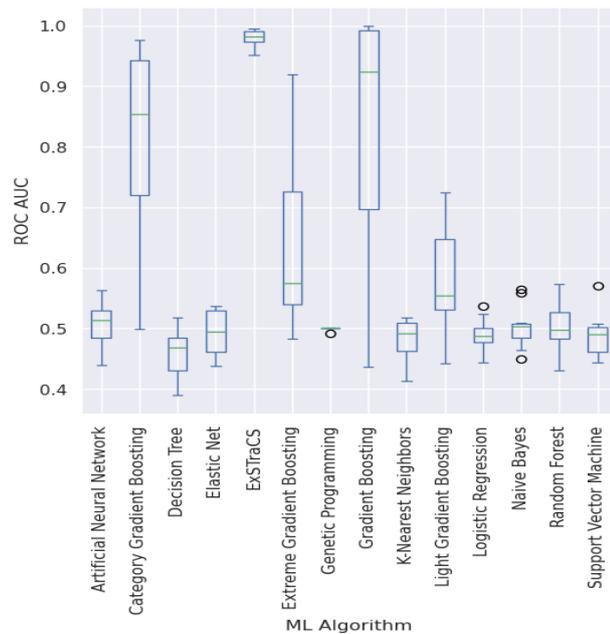

## PRC

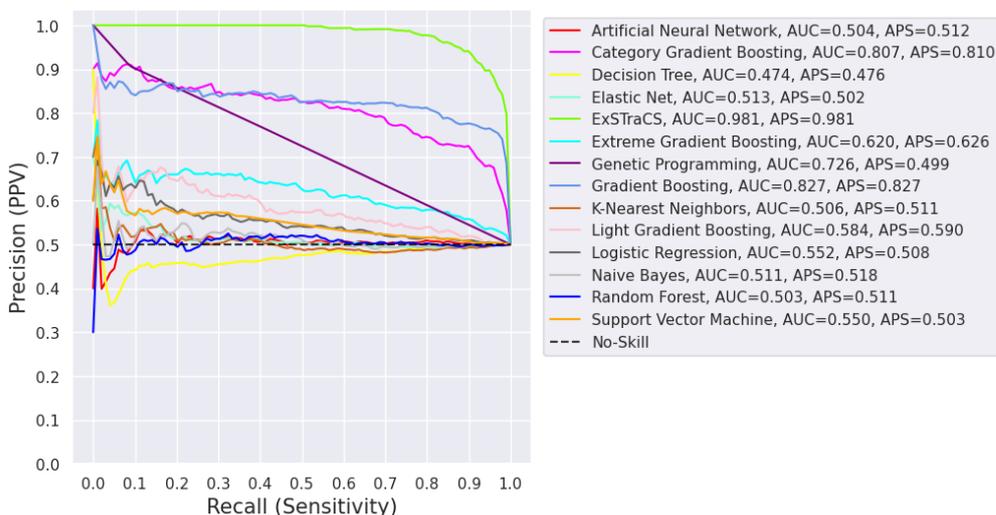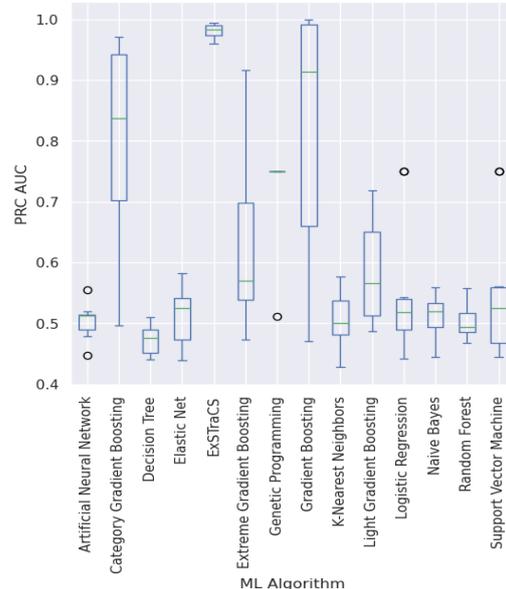

# Dataset and Model Prediction Summary: D4 = xor\_5\_a\_20s\_1600\_EDM-1\_01

## Data Processing/Counts Summary

|           | Instances | Total Features | Categorical Features | Quantitative Features | Missing Values | Missing Percent | Class 0 | Class 1 |
|-----------|-----------|----------------|----------------------|-----------------------|----------------|-----------------|---------|---------|
| Original  | 1600      | 20             | 0                    | 20                    | 0              | 0.0             | 800     | 800     |
| C1        | 1600      | 20             | 0                    | 20                    | 0              | 0.0             | 800     | 800     |
| E1        | 1600      | 20             | 0                    | 20                    | 0              | 0.0             | 800     | 800     |
| C2        | 1600      | 20             | 0                    | 20                    | 0              | 0.0             | 800     | 800     |
| C3        | 1600      | 20             | 0                    | 20                    | 0              | 0.0             | 800     | 800     |
| E2        | 1600      | 20             | 0                    | 20                    | 0              | 0.0             | 800     | 800     |
| C4        | 1600      | 20             | 0                    | 20                    | 0              | 0.0             | 800     | 800     |
| Processed | 1600      | 20             | 0                    | 20                    | 0              | 0.0             | 800     | 800     |

## Cleaning (C) and Engineering (E) Elements

- \* C1 - Remove instances with no outcome and features to ignore
- \* E1 - Add missingness features
- \* C2 - Remove features with invariance or high missingness
- \* C3 - Remove instances with high missingness
- \* E2 - Add one-hot-encoding of categorical features
- \* C4 - Remove highly correlated features

## Class Balance (Processed)

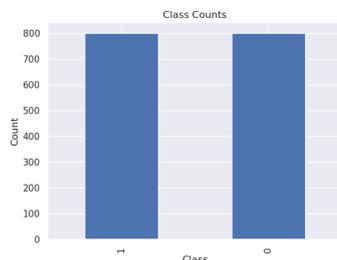

## Feature Correlations (Pearson)

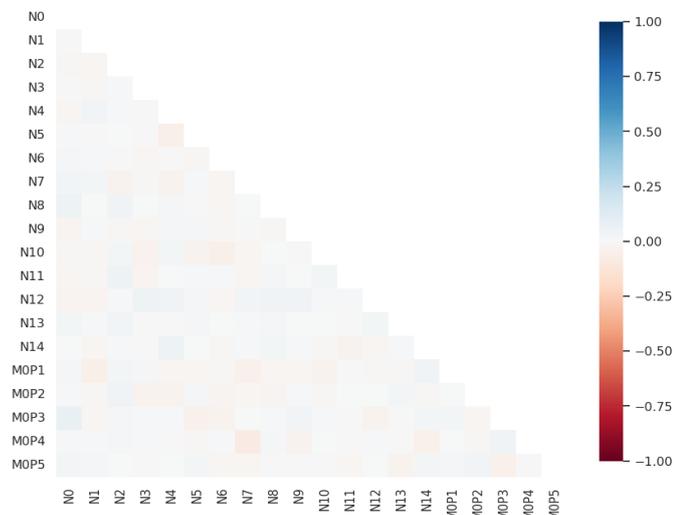

## Top ML Algorithm Results (Averaged Over CV Runs):

|                                             |
|---------------------------------------------|
| Best (ROC_AUC): ExSTraCS = 0.522            |
| Best (Balanced Acc.): ExSTraCS = 0.519      |
| Best (F1 Score): Naive Bayes = 0.510        |
| Best (PRC AUC): Genetic Programming = 0.716 |
| Best (PRC APS): Random Forest = 0.529       |

## ROC

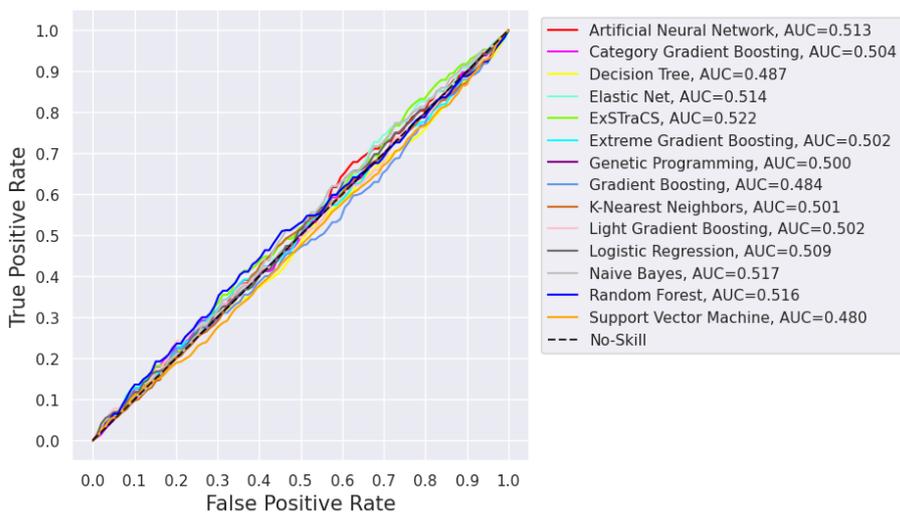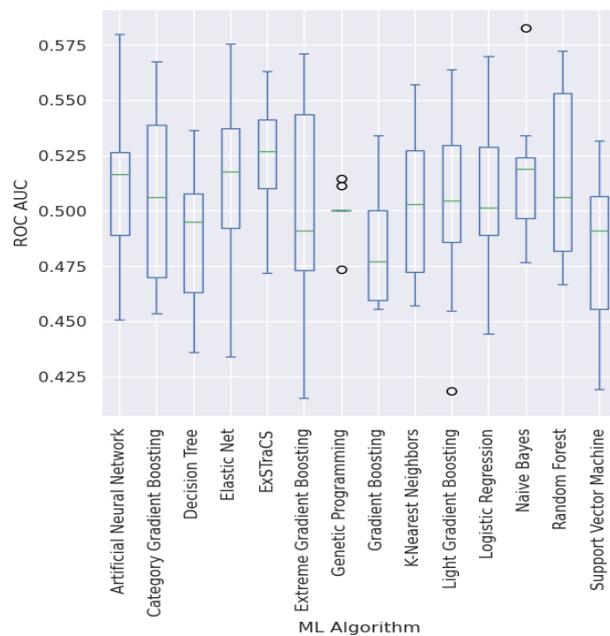

## PRC

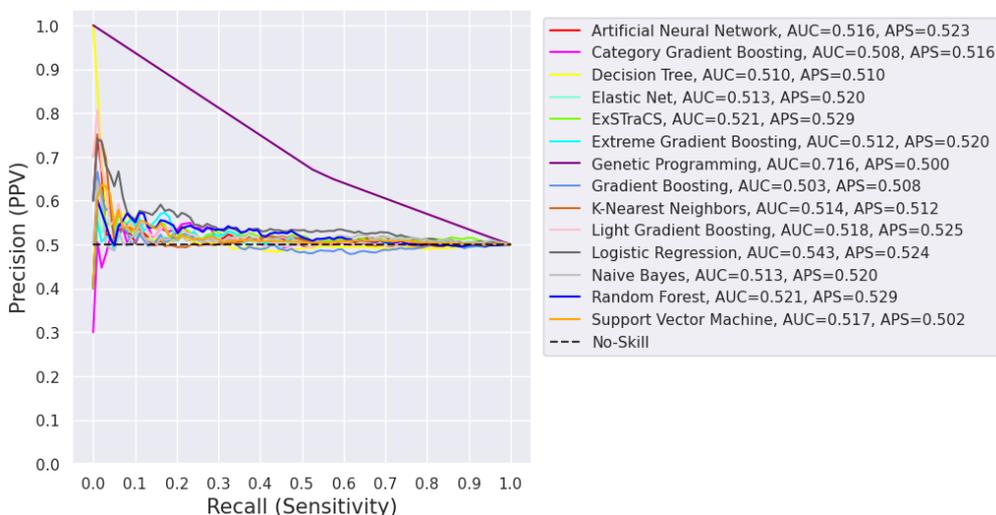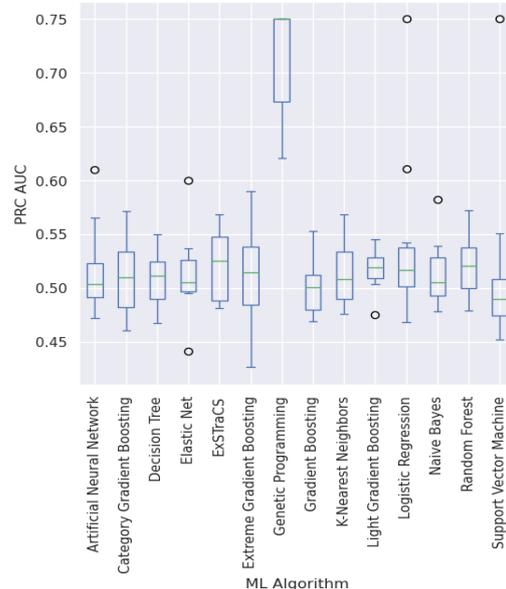

# Average Model Prediction Statistics (Rounded to 3 Decimal Points)

## D1 = xor\_2\_a\_20s\_1600\_EDM-1\_01

| ML Algorithm               | Balanced Accuracy | Accuracy | F1 Score | Sensitivity (Recall) | Specificity | Precision (PPV) | TP   | TN   | FP   | FN   | NPV   | LR+   | LR-   | ROC AUC | PRC AUC | PRC APS |
|----------------------------|-------------------|----------|----------|----------------------|-------------|-----------------|------|------|------|------|-------|-------|-------|---------|---------|---------|
| Artificial Neural Network  | 0.771             | 0.771    | 0.775    | 0.796                | 0.745       | 0.757           | 63.7 | 59.6 | 20.4 | 16.3 | 0.788 | 3.266 | 0.278 | 0.847   | 0.822   | 0.824   |
| Category Gradient Boosting | 1.0               | 1.0      | 1.0      | 1.0                  | 1.0         | 1.0             | 80.0 | 80.0 | 0.0  | 0.0  | 1.0   | 0.0   | 0.0   | 1.0     | 1.0     | 1.0     |
| Decision Tree              | 0.826             | 0.826    | 0.821    | 0.814                | 0.838       | 0.832           | 65.1 | 67.0 | 13.0 | 14.9 | 0.822 | 3.027 | 0.263 | 0.882   | 0.894   | 0.872   |
| Elastic Net                | 0.458             | 0.458    | 0.461    | 0.472                | 0.442       | 0.457           | 37.8 | 35.4 | 44.6 | 42.2 | 0.458 | 0.856 | 1.216 | 0.452   | 0.469   | 0.477   |
| ExSTraCS                   | 1.0               | 1.0      | 1.0      | 1.0                  | 1.0         | 1.0             | 80.0 | 80.0 | 0.0  | 0.0  | 1.0   | 0.0   | 0.0   | 1.0     | 1.0     | 1.0     |
| Extreme Gradient Boosting  | 1.0               | 1.0      | 1.0      | 1.0                  | 1.0         | 1.0             | 80.0 | 80.0 | 0.0  | 0.0  | 1.0   | 0.0   | 0.0   | 1.0     | 1.0     | 1.0     |
| Genetic Programming        | 1.0               | 1.0      | 1.0      | 1.0                  | 1.0         | 1.0             | 80.0 | 80.0 | 0.0  | 0.0  | 1.0   | 0.0   | 0.0   | 1.0     | 1.0     | 1.0     |
| Gradient Boosting          | 1.0               | 1.0      | 1.0      | 1.0                  | 1.0         | 1.0             | 80.0 | 80.0 | 0.0  | 0.0  | 1.0   | 0.0   | 0.0   | 1.0     | 1.0     | 1.0     |
| K-Nearest Neighbors        | 0.618             | 0.618    | 0.615    | 0.612                | 0.624       | 0.619           | 49.0 | 49.9 | 30.1 | 31.0 | 0.618 | 1.678 | 0.631 | 0.661   | 0.66    | 0.631   |
| Light Gradient Boosting    | 1.0               | 1.0      | 1.0      | 1.0                  | 1.0         | 1.0             | 80.0 | 80.0 | 0.0  | 0.0  | 1.0   | 0.0   | 0.0   | 1.0     | 1.0     | 1.0     |
| Logistic Regression        | 0.458             | 0.458    | 0.259    | 0.262                | 0.654       | 0.258           | 21.0 | 52.3 | 27.7 | 59.0 | 0.458 | 0.455 | 1.205 | 0.451   | 0.571   | 0.474   |
| Naive Bayes                | 0.451             | 0.451    | 0.465    | 0.485                | 0.416       | 0.452           | 38.8 | 33.3 | 46.7 | 41.2 | 0.448 | 0.841 | 1.261 | 0.443   | 0.455   | 0.462   |
| Random Forest              | 1.0               | 1.0      | 1.0      | 1.0                  | 1.0         | 1.0             | 80.0 | 80.0 | 0.0  | 0.0  | 1.0   | 0.0   | 0.0   | 1.0     | 1.0     | 1.0     |
| Support Vector Machine     | 0.579             | 0.579    | 0.573    | 0.568                | 0.59        | 0.581           | 45.4 | 47.2 | 32.8 | 34.6 | 0.578 | 1.401 | 0.736 | 0.587   | 0.559   | 0.564   |

## D2 = xor\_3\_a\_20s\_1600\_EDM-1\_01

| ML Algorithm               | Balanced Accuracy | Accuracy | F1 Score | Sensitivity (Recall) | Specificity | Precision (PPV) | TP   | TN   | FP   | FN   | NPV   | LR+   | LR-   | ROC AUC | PRC AUC | PRC APS |
|----------------------------|-------------------|----------|----------|----------------------|-------------|-----------------|------|------|------|------|-------|-------|-------|---------|---------|---------|
| Artificial Neural Network  | 0.494             | 0.494    | 0.541    | 0.622                | 0.366       | 0.492           | 49.8 | 29.3 | 50.7 | 30.2 | 0.51  | 0.971 | 0.98  | 0.499   | 0.5     | 0.508   |
| Category Gradient Boosting | 1.0               | 1.0      | 1.0      | 1.0                  | 1.0         | 1.0             | 80.0 | 80.0 | 0.0  | 0.0  | 1.0   | 0.0   | 0.0   | 1.0     | 1.0     | 1.0     |
| Decision Tree              | 0.492             | 0.492    | 0.478    | 0.468                | 0.516       | 0.492           | 37.4 | 41.3 | 38.7 | 42.6 | 0.492 | 0.98  | 1.044 | 0.493   | 0.52    | 0.504   |
| Elastic Net                | 0.509             | 0.509    | 0.501    | 0.494                | 0.525       | 0.511           | 39.5 | 42.0 | 38.0 | 40.5 | 0.508 | 1.058 | 0.978 | 0.509   | 0.515   | 0.523   |
| ExSTraCS                   | 1.0               | 1.0      | 1.0      | 1.0                  | 1.0         | 1.0             | 80.0 | 80.0 | 0.0  | 0.0  | 1.0   | 0.0   | 0.0   | 1.0     | 1.0     | 1.0     |
| Extreme Gradient Boosting  | 0.999             | 0.999    | 0.999    | 1.0                  | 0.998       | 0.998           | 80.0 | 79.8 | 0.2  | 0.0  | 1.0   | 16.0  | 0.0   | 1.0     | 1.0     | 1.0     |
| Genetic Programming        | 0.5               | 0.5      | 0.0      | 0.0                  | 1.0         | 0.0             | 0.0  | 80.0 | 0.0  | 80.0 | 0.5   | 0.0   | 1.0   | 0.5     | 0.75    | 0.5     |
| Gradient Boosting          | 1.0               | 1.0      | 1.0      | 1.0                  | 1.0         | 1.0             | 80.0 | 80.0 | 0.0  | 0.0  | 1.0   | 0.0   | 0.0   | 1.0     | 1.0     | 1.0     |
| K-Nearest Neighbors        | 0.516             | 0.516    | 0.509    | 0.501                | 0.53        | 0.517           | 40.1 | 42.4 | 37.6 | 39.9 | 0.514 | 1.091 | 0.959 | 0.517   | 0.534   | 0.522   |
| Light Gradient Boosting    | 1.0               | 1.0      | 1.0      | 1.0                  | 1.0         | 1.0             | 80.0 | 80.0 | 0.0  | 0.0  | 1.0   | 0.0   | 0.0   | 1.0     | 1.0     | 1.0     |
| Logistic Regression        | 0.493             | 0.493    | 0.348    | 0.352                | 0.634       | 0.344           | 28.2 | 50.7 | 29.3 | 51.8 | 0.492 | 0.682 | 1.041 | 0.484   | 0.563   | 0.494   |
| Naive Bayes                | 0.496             | 0.496    | 0.499    | 0.505                | 0.488       | 0.496           | 40.4 | 39.0 | 41.0 | 39.6 | 0.496 | 0.999 | 1.031 | 0.49    | 0.497   | 0.504   |
| Random Forest              | 0.735             | 0.735    | 0.734    | 0.732                | 0.738       | 0.738           | 58.6 | 59.0 | 21.0 | 21.4 | 0.735 | 2.945 | 0.366 | 0.811   | 0.799   | 0.801   |
| Support Vector Machine     | 0.512             | 0.512    | 0.479    | 0.461                | 0.562       | 0.517           | 36.9 | 45.0 | 35.0 | 43.1 | 0.51  | 1.094 | 0.966 | 0.501   | 0.505   | 0.511   |

## D3 = xor\_4\_a\_20s\_1600\_EDM-1\_01

| ML Algorithm               | Balanced Accuracy | Accuracy | F1 Score | Sensitivity (Recall) | Specificity | Precision (PPV) | TP   | TN   | FP   | FN   | NPV   | LR+    | LR-   | ROC AUC | PRC AUC | PRC APS |
|----------------------------|-------------------|----------|----------|----------------------|-------------|-----------------|------|------|------|------|-------|--------|-------|---------|---------|---------|
| Artificial Neural Network  | 0.503             | 0.503    | 0.587    | 0.719                | 0.288       | 0.501           | 57.5 | 23.0 | 57.0 | 22.5 | 0.514 | 1.008  | 0.96  | 0.507   | 0.504   | 0.512   |
| Category Gradient Boosting | 0.754             | 0.754    | 0.754    | 0.752                | 0.756       | 0.758           | 60.2 | 60.5 | 19.5 | 19.8 | 0.753 | 4.755  | 0.366 | 0.814   | 0.807   | 0.81    |
| Decision Tree              | 0.468             | 0.468    | 0.449    | 0.438                | 0.499       | 0.464           | 35.0 | 39.9 | 40.1 | 45.0 | 0.471 | 0.876  | 1.136 | 0.459   | 0.474   | 0.476   |
| Elastic Net                | 0.498             | 0.498    | 0.479    | 0.47                 | 0.525       | 0.497           | 37.6 | 42.0 | 38.0 | 42.4 | 0.498 | 0.994  | 1.013 | 0.492   | 0.513   | 0.502   |
| ExSTraCS                   | 0.922             | 0.922    | 0.919    | 0.896                | 0.948       | 0.945           | 71.7 | 75.8 | 4.2  | 8.3  | 0.905 | 21.418 | 0.109 | 0.98    | 0.981   | 0.981   |
| Extreme Gradient Boosting  | 0.608             | 0.608    | 0.593    | 0.582                | 0.632       | 0.608           | 46.6 | 50.6 | 29.4 | 33.4 | 0.608 | 1.771  | 0.685 | 0.63    | 0.62    | 0.626   |
| Genetic Programming        | 0.499             | 0.499    | 0.015    | 0.009                | 0.99        | 0.047           | 0.7  | 79.2 | 0.8  | 79.3 | 0.5   | 0.088  | 1.001 | 0.499   | 0.726   | 0.499   |
| Gradient Boosting          | 0.809             | 0.809    | 0.813    | 0.821                | 0.798       | 0.807           | 65.7 | 63.8 | 16.2 | 14.3 | 0.813 | 6.568  | 0.318 | 0.828   | 0.827   | 0.827   |
| K-Nearest Neighbors        | 0.499             | 0.499    | 0.471    | 0.448                | 0.55        | 0.501           | 35.8 | 44.0 | 36.0 | 44.2 | 0.497 | 1.008  | 1.014 | 0.483   | 0.506   | 0.511   |
| Light Gradient Boosting    | 0.562             | 0.562    | 0.566    | 0.57                 | 0.554       | 0.564           | 45.6 | 44.3 | 35.7 | 34.4 | 0.56  | 1.353  | 0.811 | 0.58    | 0.584   | 0.59    |
| Logistic Regression        | 0.491             | 0.491    | 0.396    | 0.402                | 0.579       | 0.39            | 32.2 | 46.3 | 33.7 | 47.8 | 0.491 | 0.765  | 1.041 | 0.489   | 0.552   | 0.508   |
| Naive Bayes                | 0.498             | 0.498    | 0.529    | 0.565                | 0.43        | 0.498           | 45.2 | 34.4 | 45.6 | 34.8 | 0.497 | 0.994  | 1.017 | 0.504   | 0.511   | 0.518   |
| Random Forest              | 0.522             | 0.522    | 0.54     | 0.568                | 0.478       | 0.52            | 45.4 | 38.2 | 41.8 | 34.6 | 0.528 | 1.089  | 0.901 | 0.504   | 0.503   | 0.511   |
| Support Vector Machine     | 0.474             | 0.474    | 0.445    | 0.431                | 0.518       | 0.471           | 34.5 | 41.4 | 38.6 | 45.5 | 0.476 | 0.896  | 1.109 | 0.489   | 0.55    | 0.503   |

## D4 = xor\_5\_a\_20s\_1600\_EDM-1\_01

| ML Algorithm               | Balanced Accuracy | Accuracy | F1 Score | Sensitivity (Recall) | Specificity | Precision (PPV) | TP   | TN   | FP   | FN   | NPV   | LR+   | LR-   | ROC AUC | PRC AUC | PRC APS |
|----------------------------|-------------------|----------|----------|----------------------|-------------|-----------------|------|------|------|------|-------|-------|-------|---------|---------|---------|
| Artificial Neural Network  | 0.504             | 0.504    | 0.501    | 0.501                | 0.507       | 0.504           | 40.1 | 40.6 | 39.4 | 39.9 | 0.505 | 1.033 | 0.988 | 0.513   | 0.516   | 0.523   |
| Category Gradient Boosting | 0.497             | 0.497    | 0.498    | 0.501                | 0.492       | 0.496           | 40.1 | 39.4 | 40.6 | 39.9 | 0.498 | 0.993 | 1.018 | 0.504   | 0.508   | 0.516   |
| Decision Tree              | 0.496             | 0.496    | 0.483    | 0.476                | 0.516       | 0.495           | 38.1 | 41.3 | 38.7 | 41.9 | 0.497 | 0.988 | 1.019 | 0.487   | 0.51    | 0.51    |
| Elastic Net                | 0.506             | 0.506    | 0.509    | 0.516                | 0.495       | 0.505           | 41.3 | 39.6 | 40.4 | 38.7 | 0.506 | 1.028 | 0.986 | 0.514   | 0.513   | 0.52    |
| ExSTraCS                   | 0.519             | 0.519    | 0.499    | 0.488                | 0.551       | 0.522           | 39.0 | 44.1 | 35.9 | 41.0 | 0.518 | 1.101 | 0.935 | 0.522   | 0.521   | 0.529   |
| Extreme Gradient Boosting  | 0.497             | 0.497    | 0.502    | 0.507                | 0.486       | 0.498           | 40.6 | 38.9 | 41.1 | 39.4 | 0.495 | 1.005 | 1.031 | 0.502   | 0.512   | 0.52    |
| Genetic Programming        | 0.499             | 0.499    | 0.181    | 0.241                | 0.756       | 0.149           | 19.3 | 60.5 | 19.5 | 60.7 | 0.502 | 0.295 | 1.0   | 0.5     | 0.716   | 0.5     |
| Gradient Boosting          | 0.484             | 0.484    | 0.483    | 0.482                | 0.486       | 0.486           | 38.6 | 38.9 | 41.1 | 41.4 | 0.483 | 0.95  | 1.078 | 0.484   | 0.503   | 0.508   |
| K-Nearest Neighbors        | 0.504             | 0.504    | 0.439    | 0.394                | 0.615       | 0.504           | 31.5 | 49.2 | 30.8 | 48.5 | 0.504 | 1.025 | 0.987 | 0.501   | 0.514   | 0.512   |
| Light Gradient Boosting    | 0.495             | 0.495    | 0.497    | 0.5                  | 0.49        | 0.496           | 40.0 | 39.2 | 40.8 | 40.0 | 0.494 | 0.996 | 1.038 | 0.502   | 0.518   | 0.525   |
| Logistic Regression        | 0.507             | 0.507    | 0.464    | 0.474                | 0.54        | 0.457           | 37.9 | 43.2 | 36.8 | 42.1 | 0.507 | 0.936 | 0.981 | 0.509   | 0.543   | 0.524   |
| Naive Bayes                | 0.508             | 0.508    | 0.51     | 0.514                | 0.502       | 0.508           | 41.1 | 40.2 | 39.8 | 38.9 | 0.509 | 1.042 | 0.974 | 0.517   | 0.513   | 0.52    |
| Random Forest              | 0.513             | 0.513    | 0.509    | 0.51                 | 0.516       | 0.512           | 40.8 | 41.3 | 38.7 | 39.2 | 0.515 | 1.059 | 0.952 | 0.516   | 0.521   | 0.529   |
| Support Vector Machine     | 0.497             | 0.497    | 0.504    | 0.515                | 0.479       | 0.495           | 41.2 | 38.3 | 41.7 | 38.8 | 0.499 | 0.995 | 1.022 | 0.48    | 0.517   | 0.502   |

# Median Model Prediction Statistics (Rounded to 3 Decimal Points)

## D1 = xor\_2\_a\_20s\_1600\_EDM-1\_01

| ML Algorithm               | Balanced Accuracy | Accuracy | F1 Score | Sensitivity (Recall) | Specificity | Precision (PPV) | TP   | TN   | FP   | FN   | NPV   | LR+   | LR-   | ROC AUC | PRC AUC | PRC APS |
|----------------------------|-------------------|----------|----------|----------------------|-------------|-----------------|------|------|------|------|-------|-------|-------|---------|---------|---------|
| Artificial Neural Network  | 0.775             | 0.775    | 0.784    | 0.819                | 0.75        | 0.753           | 65.5 | 60.0 | 20.0 | 14.5 | 0.801 | 3.066 | 0.249 | 0.86    | 0.829   | 0.831   |
| Category Gradient Boosting | 1.0               | 1.0      | 1.0      | 1.0                  | 1.0         | 1.0             | 80.0 | 80.0 | 0.0  | 0.0  | 1.0   | 0.0   | 0.0   | 1.0     | 1.0     | 1.0     |
| Decision Tree              | 0.859             | 0.859    | 0.859    | 0.856                | 0.838       | 0.846           | 68.5 | 67.0 | 13.0 | 11.5 | 0.857 | 2.25  | 0.167 | 0.952   | 0.956   | 0.95    |
| Elastic Net                | 0.456             | 0.456    | 0.469    | 0.462                | 0.4         | 0.461           | 37.0 | 32.0 | 48.0 | 43.0 | 0.45  | 0.856 | 1.222 | 0.444   | 0.459   | 0.465   |
| ExSTraCS                   | 1.0               | 1.0      | 1.0      | 1.0                  | 1.0         | 1.0             | 80.0 | 80.0 | 0.0  | 0.0  | 1.0   | 0.0   | 0.0   | 1.0     | 1.0     | 1.0     |
| Extreme Gradient Boosting  | 1.0               | 1.0      | 1.0      | 1.0                  | 1.0         | 1.0             | 80.0 | 80.0 | 0.0  | 0.0  | 1.0   | 0.0   | 0.0   | 1.0     | 1.0     | 1.0     |
| Genetic Programming        | 1.0               | 1.0      | 1.0      | 1.0                  | 1.0         | 1.0             | 80.0 | 80.0 | 0.0  | 0.0  | 1.0   | 0.0   | 0.0   | 1.0     | 1.0     | 1.0     |
| Gradient Boosting          | 1.0               | 1.0      | 1.0      | 1.0                  | 1.0         | 1.0             | 80.0 | 80.0 | 0.0  | 0.0  | 1.0   | 0.0   | 0.0   | 1.0     | 1.0     | 1.0     |
| K-Nearest Neighbors        | 0.625             | 0.625    | 0.628    | 0.638                | 0.612       | 0.622           | 51.0 | 49.0 | 31.0 | 29.0 | 0.626 | 1.645 | 0.598 | 0.677   | 0.676   | 0.659   |
| Light Gradient Boosting    | 1.0               | 1.0      | 1.0      | 1.0                  | 1.0         | 1.0             | 80.0 | 80.0 | 0.0  | 0.0  | 1.0   | 0.0   | 0.0   | 1.0     | 1.0     | 1.0     |
| Logistic Regression        | 0.459             | 0.459    | 0.377    | 0.362                | 0.488       | 0.394           | 29.0 | 39.0 | 41.0 | 51.0 | 0.453 | 0.653 | 1.206 | 0.448   | 0.479   | 0.477   |
| Naive Bayes                | 0.428             | 0.428    | 0.464    | 0.462                | 0.412       | 0.439           | 37.0 | 33.0 | 47.0 | 43.0 | 0.417 | 0.784 | 1.397 | 0.424   | 0.441   | 0.449   |
| Random Forest              | 1.0               | 1.0      | 1.0      | 1.0                  | 1.0         | 1.0             | 80.0 | 80.0 | 0.0  | 0.0  | 1.0   | 0.0   | 0.0   | 1.0     | 1.0     | 1.0     |
| Support Vector Machine     | 0.572             | 0.572    | 0.576    | 0.575                | 0.581       | 0.571           | 46.0 | 46.5 | 33.5 | 34.0 | 0.573 | 1.329 | 0.744 | 0.591   | 0.566   | 0.573   |

## D2 = xor\_3\_a\_20s\_1600\_EDM-1\_01

| ML Algorithm               | Balanced Accuracy | Accuracy | F1 Score | Sensitivity (Recall) | Specificity | Precision (PPV) | TP   | TN   | FP   | FN   | NPV   | LR+   | LR-   | ROC AUC | PRC AUC | PRC APS |
|----------------------------|-------------------|----------|----------|----------------------|-------------|-----------------|------|------|------|------|-------|-------|-------|---------|---------|---------|
| Artificial Neural Network  | 0.497             | 0.497    | 0.494    | 0.5                  | 0.431       | 0.497           | 40.0 | 34.5 | 45.5 | 40.0 | 0.497 | 0.987 | 1.012 | 0.494   | 0.504   | 0.51    |
| Category Gradient Boosting | 1.0               | 1.0      | 1.0      | 1.0                  | 1.0         | 1.0             | 80.0 | 80.0 | 0.0  | 0.0  | 1.0   | 0.0   | 0.0   | 1.0     | 1.0     | 1.0     |
| Decision Tree              | 0.481             | 0.481    | 0.469    | 0.469                | 0.5         | 0.48            | 37.5 | 40.0 | 40.0 | 42.5 | 0.482 | 0.922 | 1.073 | 0.48    | 0.515   | 0.485   |
| Elastic Net                | 0.512             | 0.512    | 0.511    | 0.506                | 0.525       | 0.513           | 40.5 | 42.0 | 38.0 | 39.5 | 0.512 | 1.053 | 0.953 | 0.493   | 0.497   | 0.504   |
| ExSTraCS                   | 1.0               | 1.0      | 1.0      | 1.0                  | 1.0         | 1.0             | 80.0 | 80.0 | 0.0  | 0.0  | 1.0   | 0.0   | 0.0   | 1.0     | 1.0     | 1.0     |
| Extreme Gradient Boosting  | 1.0               | 1.0      | 1.0      | 1.0                  | 1.0         | 1.0             | 80.0 | 80.0 | 0.0  | 0.0  | 1.0   | 0.0   | 0.0   | 1.0     | 1.0     | 1.0     |
| Genetic Programming        | 0.5               | 0.5      | 0.0      | 0.0                  | 1.0         | 0.0             | 0.0  | 80.0 | 0.0  | 80.0 | 0.5   | 0.0   | 1.0   | 0.5     | 0.75    | 0.5     |
| Gradient Boosting          | 1.0               | 1.0      | 1.0      | 1.0                  | 1.0         | 1.0             | 80.0 | 80.0 | 0.0  | 0.0  | 1.0   | 0.0   | 0.0   | 1.0     | 1.0     | 1.0     |
| K-Nearest Neighbors        | 0.516             | 0.516    | 0.508    | 0.5                  | 0.525       | 0.516           | 40.0 | 42.0 | 38.0 | 40.0 | 0.515 | 1.067 | 0.941 | 0.525   | 0.521   | 0.52    |
| Light Gradient Boosting    | 1.0               | 1.0      | 1.0      | 1.0                  | 1.0         | 1.0             | 80.0 | 80.0 | 0.0  | 0.0  | 1.0   | 0.0   | 0.0   | 1.0     | 1.0     | 1.0     |
| Logistic Regression        | 0.494             | 0.494    | 0.468    | 0.456                | 0.525       | 0.462           | 36.5 | 42.0 | 38.0 | 43.5 | 0.494 | 0.859 | 1.024 | 0.487   | 0.499   | 0.5     |
| Naive Bayes                | 0.481             | 0.481    | 0.5      | 0.5                  | 0.481       | 0.483           | 40.0 | 38.5 | 41.5 | 40.0 | 0.48  | 0.933 | 1.085 | 0.464   | 0.479   | 0.488   |
| Random Forest              | 0.734             | 0.734    | 0.733    | 0.744                | 0.738       | 0.735           | 59.5 | 59.0 | 21.0 | 20.5 | 0.736 | 2.792 | 0.359 | 0.796   | 0.782   | 0.784   |
| Support Vector Machine     | 0.506             | 0.506    | 0.517    | 0.506                | 0.506       | 0.506           | 40.5 | 40.5 | 39.5 | 39.5 | 0.507 | 1.024 | 0.974 | 0.506   | 0.505   | 0.507   |

## D3 = xor\_4\_a\_20s\_1600\_EDM-1\_01

| ML Algorithm               | Balanced Accuracy | Accuracy | F1 Score | Sensitivity (Recall) | Specificity | Precision (PPV) | TP   | TN   | FP   | FN   | NPV   | LR+    | LR-   | ROC AUC | PRC AUC | PRC APS |
|----------------------------|-------------------|----------|----------|----------------------|-------------|-----------------|------|------|------|------|-------|--------|-------|---------|---------|---------|
| Artificial Neural Network  | 0.512             | 0.512    | 0.608    | 0.762                | 0.238       | 0.508           | 61.0 | 19.0 | 61.0 | 19.0 | 0.526 | 1.033  | 0.9   | 0.514   | 0.513   | 0.52    |
| Category Gradient Boosting | 0.769             | 0.769    | 0.772    | 0.762                | 0.769       | 0.763           | 61.0 | 61.5 | 18.5 | 19.0 | 0.77  | 3.336  | 0.3   | 0.854   | 0.837   | 0.839   |
| Decision Tree              | 0.481             | 0.481    | 0.461    | 0.444                | 0.512       | 0.48            | 35.5 | 41.0 | 39.0 | 44.5 | 0.482 | 0.925  | 1.076 | 0.469   | 0.476   | 0.473   |
| Elastic Net                | 0.494             | 0.494    | 0.501    | 0.5                  | 0.512       | 0.495           | 40.0 | 41.0 | 39.0 | 40.0 | 0.493 | 0.978  | 1.03  | 0.495   | 0.526   | 0.51    |
| ExSTraCS                   | 0.931             | 0.931    | 0.932    | 0.925                | 0.95        | 0.945           | 74.0 | 76.0 | 4.0  | 6.0  | 0.929 | 17.275 | 0.077 | 0.982   | 0.983   | 0.983   |
| Extreme Gradient Boosting  | 0.556             | 0.556    | 0.556    | 0.562                | 0.625       | 0.564           | 45.0 | 50.0 | 30.0 | 35.0 | 0.551 | 1.296  | 0.815 | 0.574   | 0.57    | 0.575   |
| Genetic Programming        | 0.5               | 0.5      | 0.0      | 0.0                  | 1.0         | 0.0             | 0.0  | 80.0 | 0.0  | 80.0 | 0.5   | 0.0    | 1.0   | 0.5     | 0.75    | 0.5     |
| Gradient Boosting          | 0.875             | 0.875    | 0.874    | 0.869                | 0.875       | 0.875           | 69.5 | 70.0 | 10.0 | 10.5 | 0.87  | 2.514  | 1.156 | 0.924   | 0.914   | 0.916   |
| K-Nearest Neighbors        | 0.494             | 0.494    | 0.464    | 0.45                 | 0.55        | 0.494           | 36.0 | 44.0 | 36.0 | 44.0 | 0.494 | 0.975  | 1.023 | 0.492   | 0.501   | 0.502   |
| Light Gradient Boosting    | 0.566             | 0.566    | 0.578    | 0.581                | 0.544       | 0.562           | 46.5 | 43.5 | 36.5 | 33.5 | 0.569 | 1.285  | 0.756 | 0.555   | 0.565   | 0.573   |
| Logistic Regression        | 0.494             | 0.494    | 0.483    | 0.494                | 0.5         | 0.478           | 39.5 | 40.0 | 40.0 | 40.5 | 0.494 | 0.916  | 1.026 | 0.487   | 0.518   | 0.508   |
| Naive Bayes                | 0.497             | 0.497    | 0.532    | 0.569                | 0.438       | 0.497           | 45.5 | 35.0 | 45.0 | 34.5 | 0.496 | 0.989  | 1.014 | 0.504   | 0.519   | 0.527   |
| Random Forest              | 0.531             | 0.531    | 0.546    | 0.556                | 0.512       | 0.529           | 44.5 | 41.0 | 39.0 | 35.5 | 0.534 | 1.123  | 0.873 | 0.497   | 0.493   | 0.503   |
| Support Vector Machine     | 0.478             | 0.478    | 0.464    | 0.456                | 0.494       | 0.472           | 36.5 | 39.5 | 40.5 | 43.5 | 0.482 | 0.893  | 1.073 | 0.49    | 0.524   | 0.501   |

## D4 = xor\_5\_a\_20s\_1600\_EDM-1\_01

| ML Algorithm               | Balanced Accuracy | Accuracy | F1 Score | Sensitivity (Recall) | Specificity | Precision (PPV) | TP   | TN   | FP   | FN   | NPV   | LR+   | LR-   | ROC AUC | PRC AUC | PRC APS |
|----------------------------|-------------------|----------|----------|----------------------|-------------|-----------------|------|------|------|------|-------|-------|-------|---------|---------|---------|
| Artificial Neural Network  | 0.506             | 0.506    | 0.493    | 0.462                | 0.488       | 0.505           | 37.0 | 39.0 | 41.0 | 43.0 | 0.508 | 1.02  | 0.969 | 0.516   | 0.503   | 0.513   |
| Category Gradient Boosting | 0.491             | 0.491    | 0.483    | 0.481                | 0.488       | 0.491           | 38.5 | 39.0 | 41.0 | 41.5 | 0.491 | 0.965 | 1.038 | 0.506   | 0.51    | 0.519   |
| Decision Tree              | 0.503             | 0.503    | 0.479    | 0.462                | 0.519       | 0.504           | 37.0 | 41.5 | 38.5 | 43.0 | 0.502 | 1.017 | 0.992 | 0.495   | 0.511   | 0.511   |
| Elastic Net                | 0.516             | 0.516    | 0.526    | 0.538                | 0.494       | 0.514           | 43.0 | 39.5 | 40.5 | 37.0 | 0.516 | 1.056 | 0.937 | 0.518   | 0.505   | 0.514   |
| ExSTraCS                   | 0.522             | 0.522    | 0.506    | 0.506                | 0.55        | 0.52            | 40.5 | 44.0 | 36.0 | 39.5 | 0.521 | 1.083 | 0.92  | 0.527   | 0.525   | 0.532   |
| Extreme Gradient Boosting  | 0.497             | 0.497    | 0.5      | 0.519                | 0.481       | 0.496           | 41.5 | 38.5 | 41.5 | 38.5 | 0.497 | 0.986 | 1.012 | 0.491   | 0.514   | 0.52    |
| Genetic Programming        | 0.5               | 0.5      | 0.0      | 0.0                  | 1.0         | 0.0             | 0.0  | 80.0 | 0.0  | 80.0 | 0.5   | 0.0   | 1.0   | 0.5     | 0.75    | 0.5     |
| Gradient Boosting          | 0.478             | 0.478    | 0.476    | 0.488                | 0.481       | 0.477           | 39.0 | 38.5 | 41.5 | 41.0 | 0.479 | 0.913 | 1.087 | 0.477   | 0.5     | 0.507   |
| K-Nearest Neighbors        | 0.503             | 0.503    | 0.44     | 0.4                  | 0.606       | 0.503           | 32.0 | 48.5 | 31.5 | 48.0 | 0.503 | 1.014 | 0.989 | 0.503   | 0.508   | 0.506   |
| Light Gradient Boosting    | 0.491             | 0.491    | 0.5      | 0.494                | 0.494       | 0.492           | 39.5 | 39.5 | 40.5 | 40.5 | 0.491 | 0.968 | 1.039 | 0.504   | 0.52    | 0.526   |
| Logistic Regression        | 0.509             | 0.509    | 0.516    | 0.525                | 0.481       | 0.505           | 42.0 | 38.5 | 41.5 | 38.0 | 0.51  | 1.022 | 0.962 | 0.501   | 0.517   | 0.518   |
| Naive Bayes                | 0.5               | 0.5      | 0.499    | 0.494                | 0.488       | 0.5             | 39.5 | 39.0 | 41.0 | 40.5 | 0.5   | 1.0   | 1.0   | 0.519   | 0.505   | 0.512   |
| Random Forest              | 0.506             | 0.506    | 0.503    | 0.512                | 0.519       | 0.507           | 41.0 | 41.5 | 38.5 | 39.0 | 0.506 | 1.029 | 0.978 | 0.506   | 0.521   | 0.527   |
| Support Vector Machine     | 0.516             | 0.516    | 0.52     | 0.544                | 0.475       | 0.516           | 43.5 | 38.0 | 42.0 | 36.5 | 0.515 | 1.068 | 0.94  | 0.491   | 0.49    | 0.503   |

# Feature Importance Summary: D1 = xor\_2\_a\_20s\_1600\_EDM-1\_01

Sorted Median Mutual Information Scores

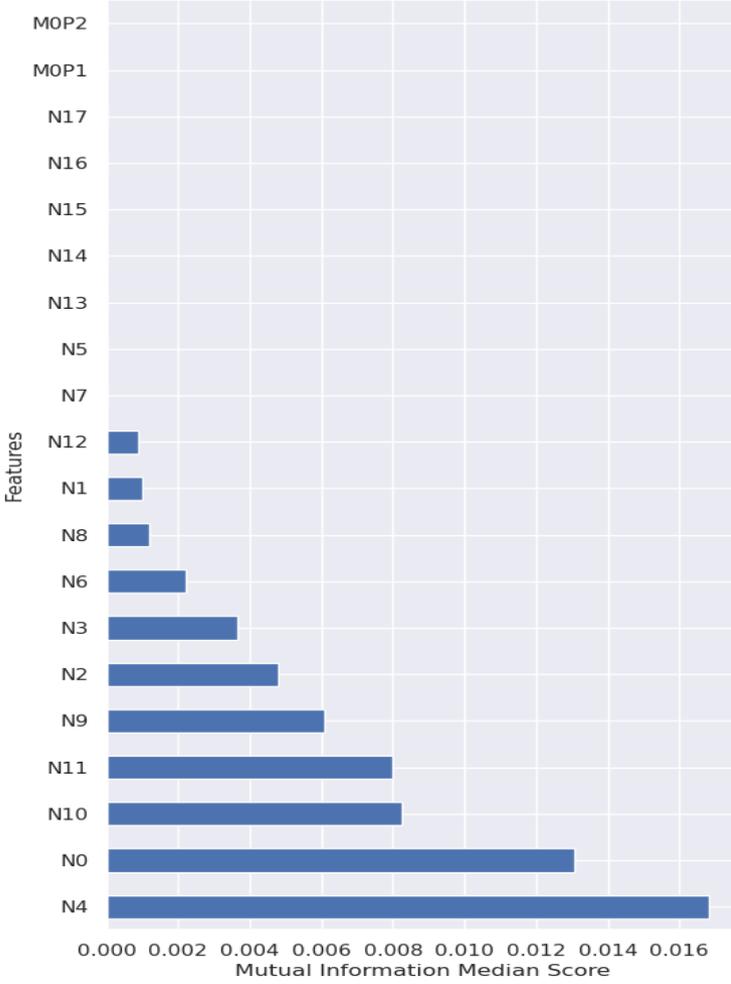

Sorted Median MultiSURF Scores

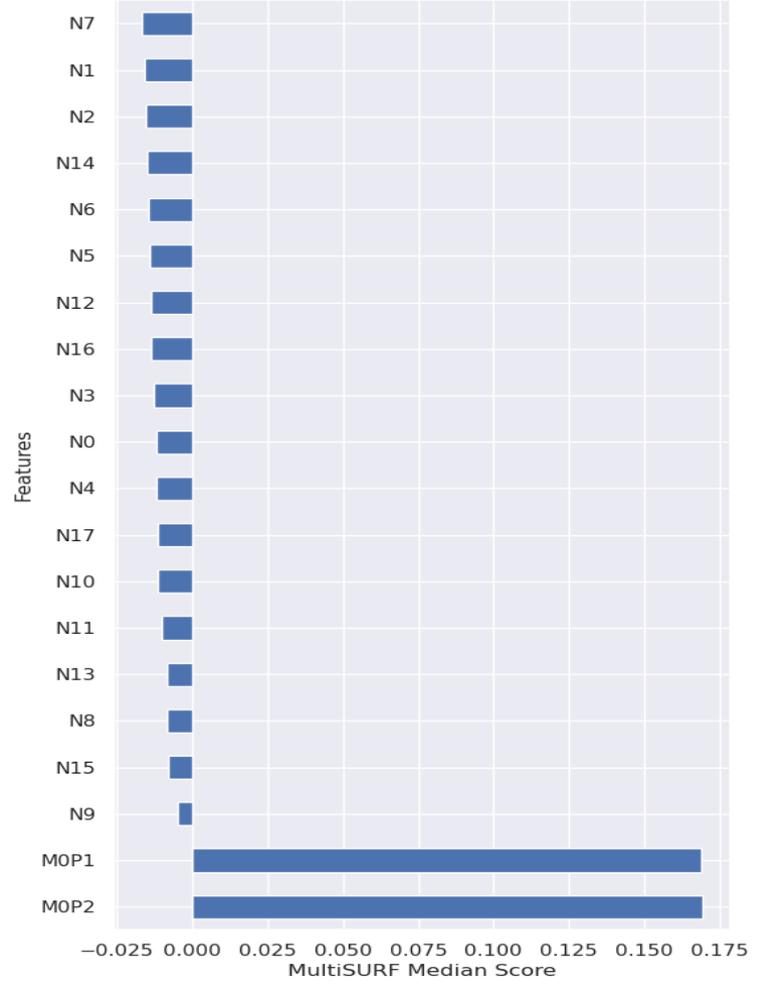

## Composite Feature Importance Plot (Normalized and Performance Weighted)

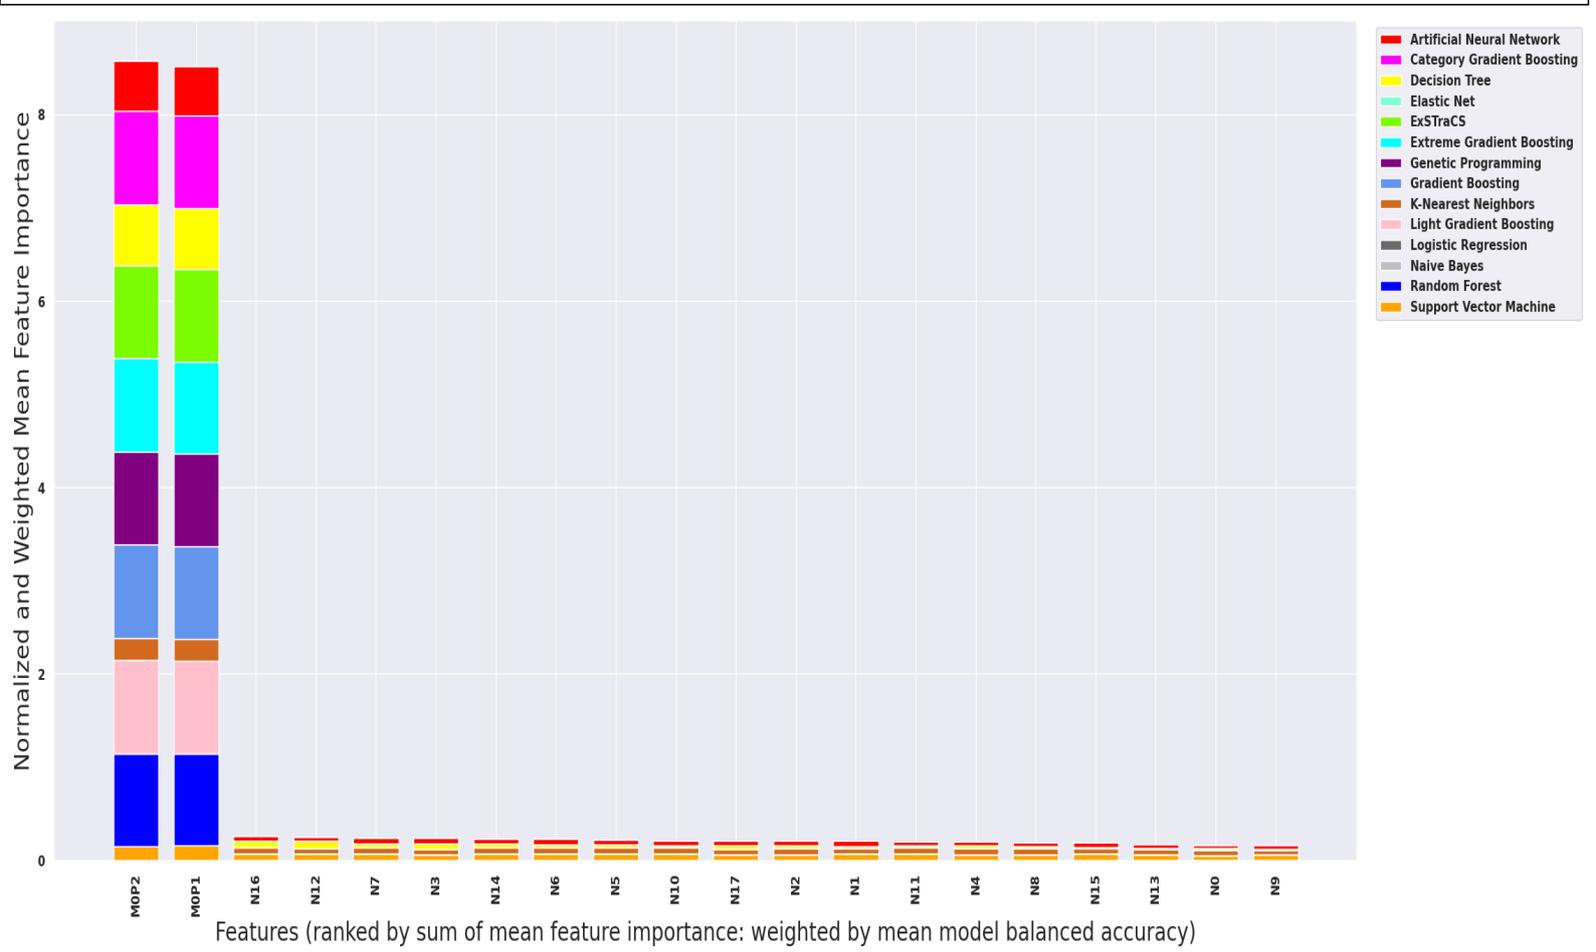

# Feature Importance Summary: D2 = xor\_3\_a\_20s\_1600\_EDM-1\_01

Sorted Median Mutual Information Scores

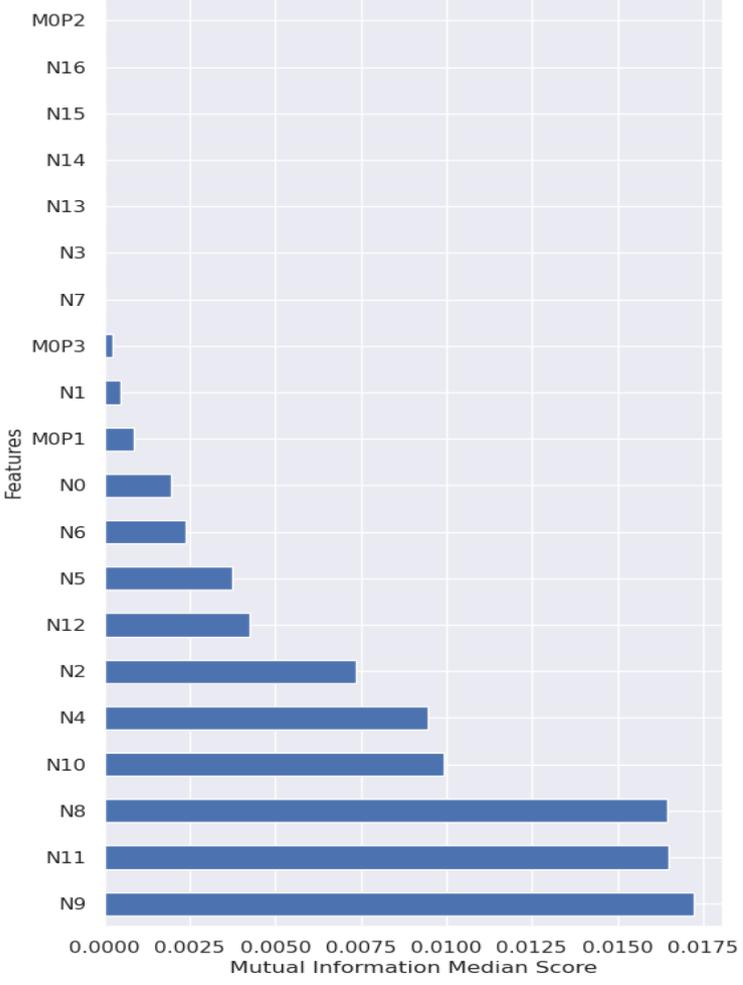

Sorted Median MultiSURF Scores

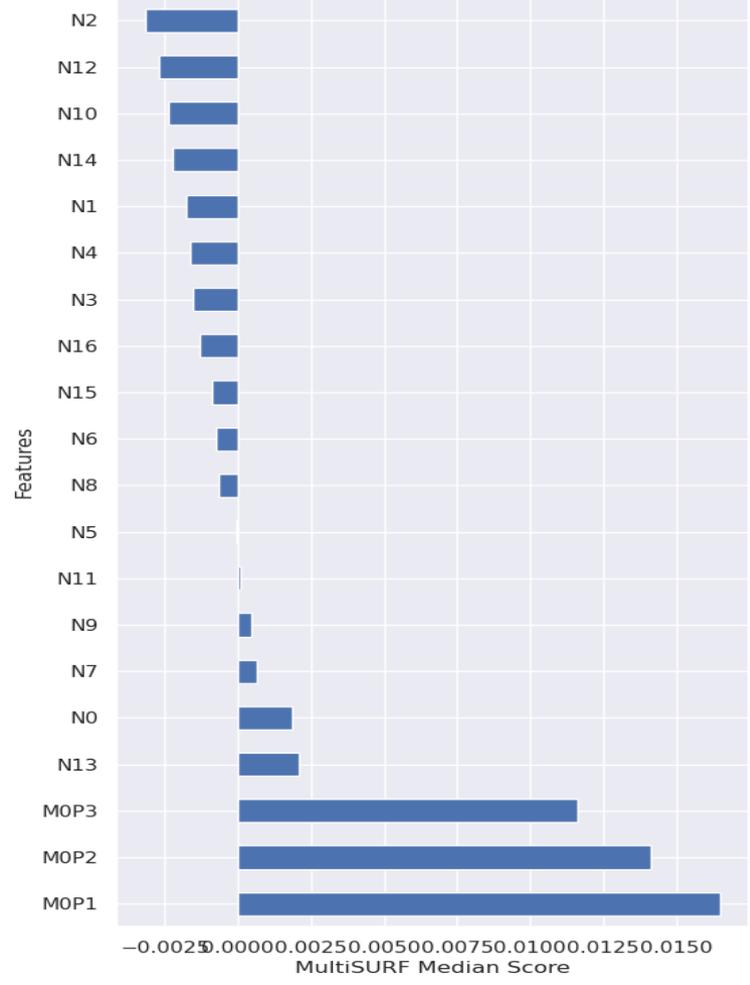

## Composite Feature Importance Plot (Normalized and Performance Weighted)

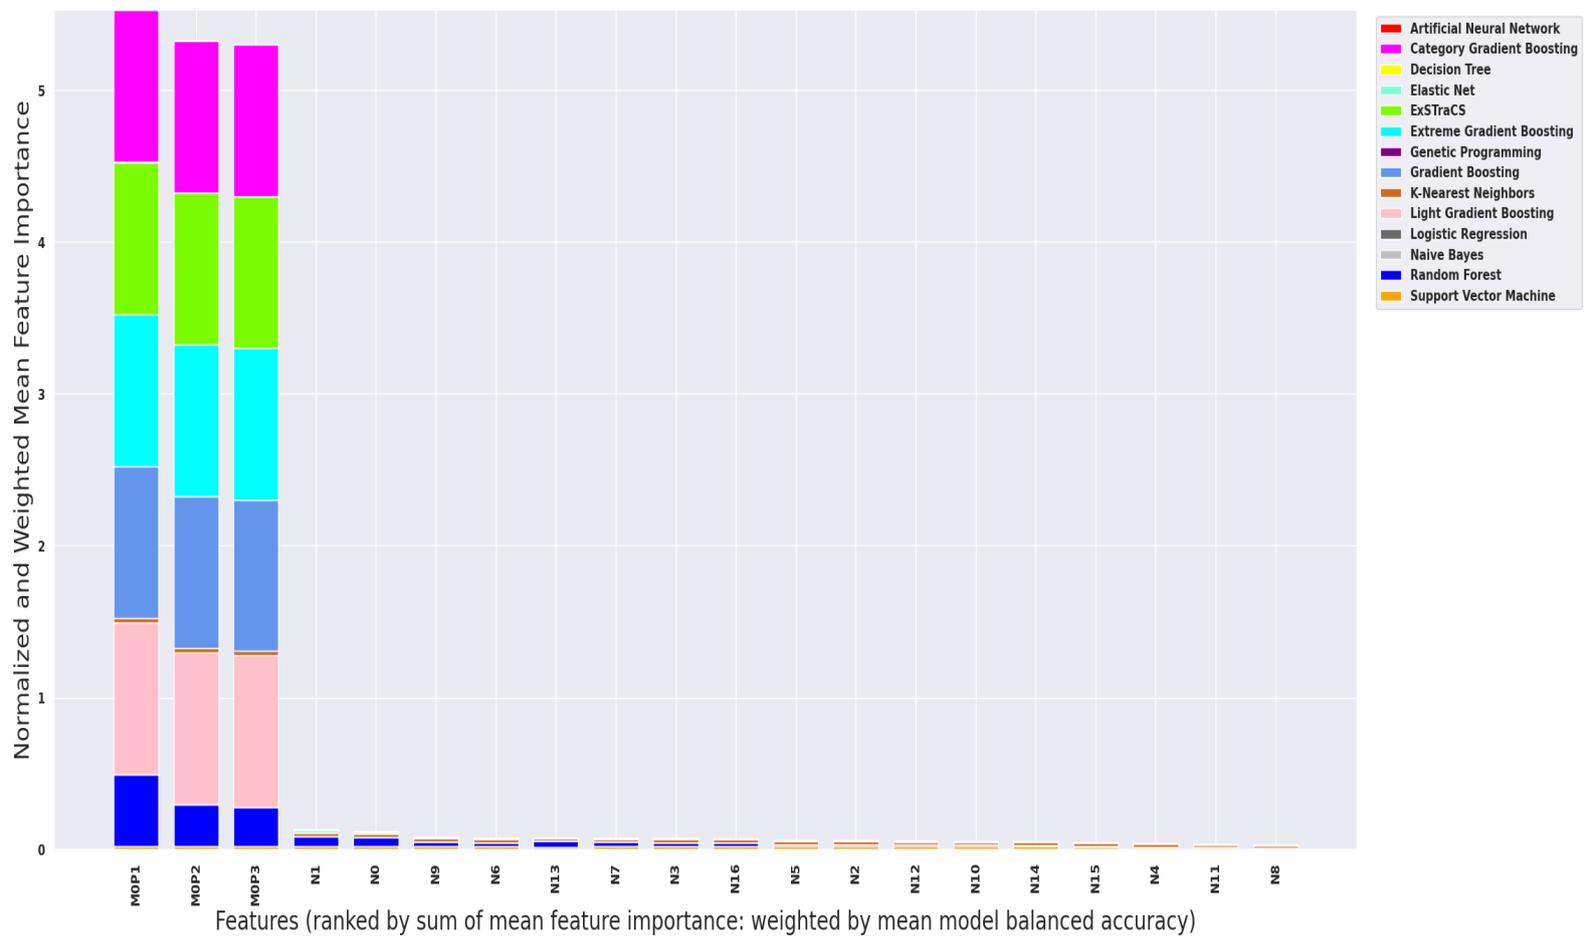

# Feature Importance Summary: D3 = xor\_4\_a\_20s\_1600\_EDM-1\_01

Sorted Median Mutual Information Scores

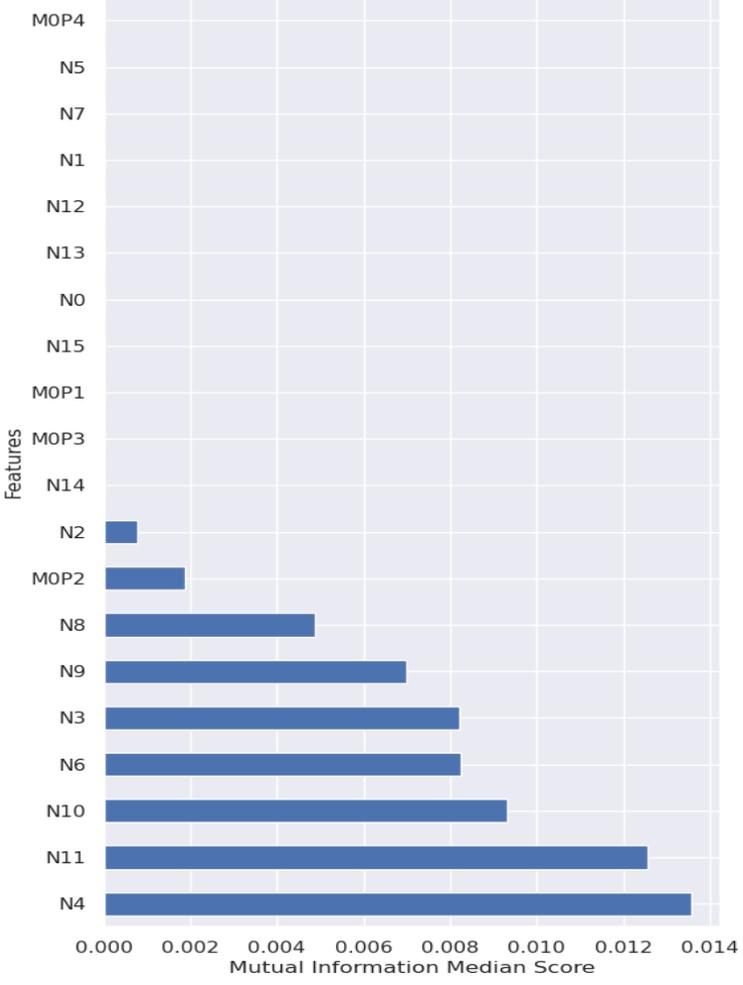

Sorted Median MultiSURF Scores

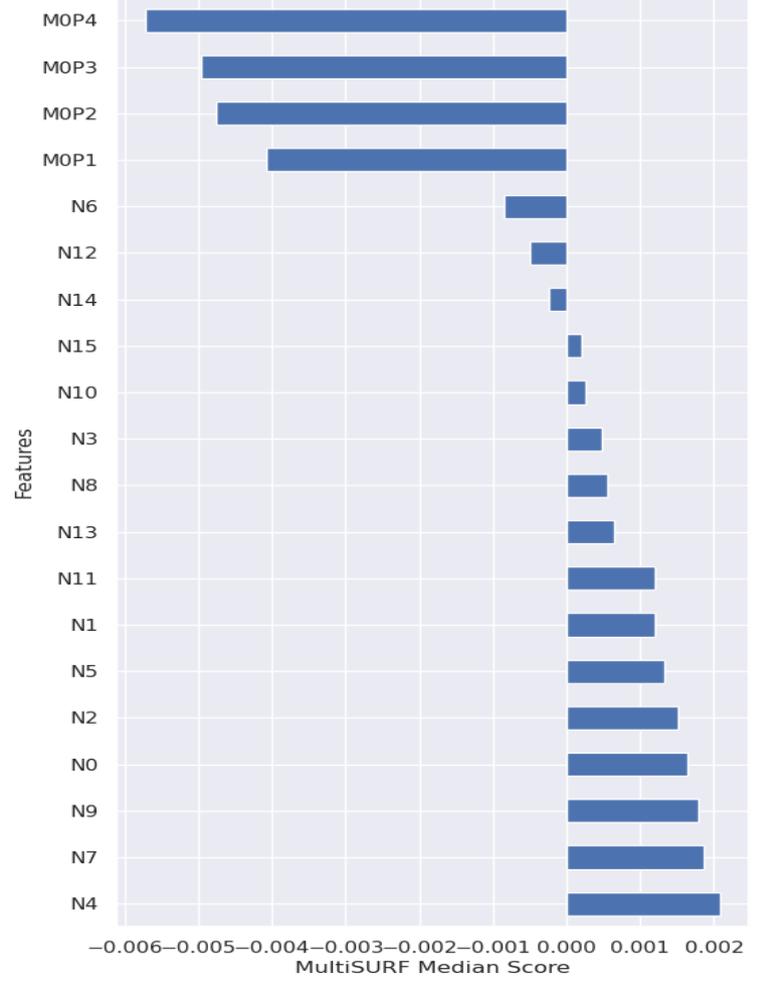

## Composite Feature Importance Plot (Normalized and Performance Weighted)

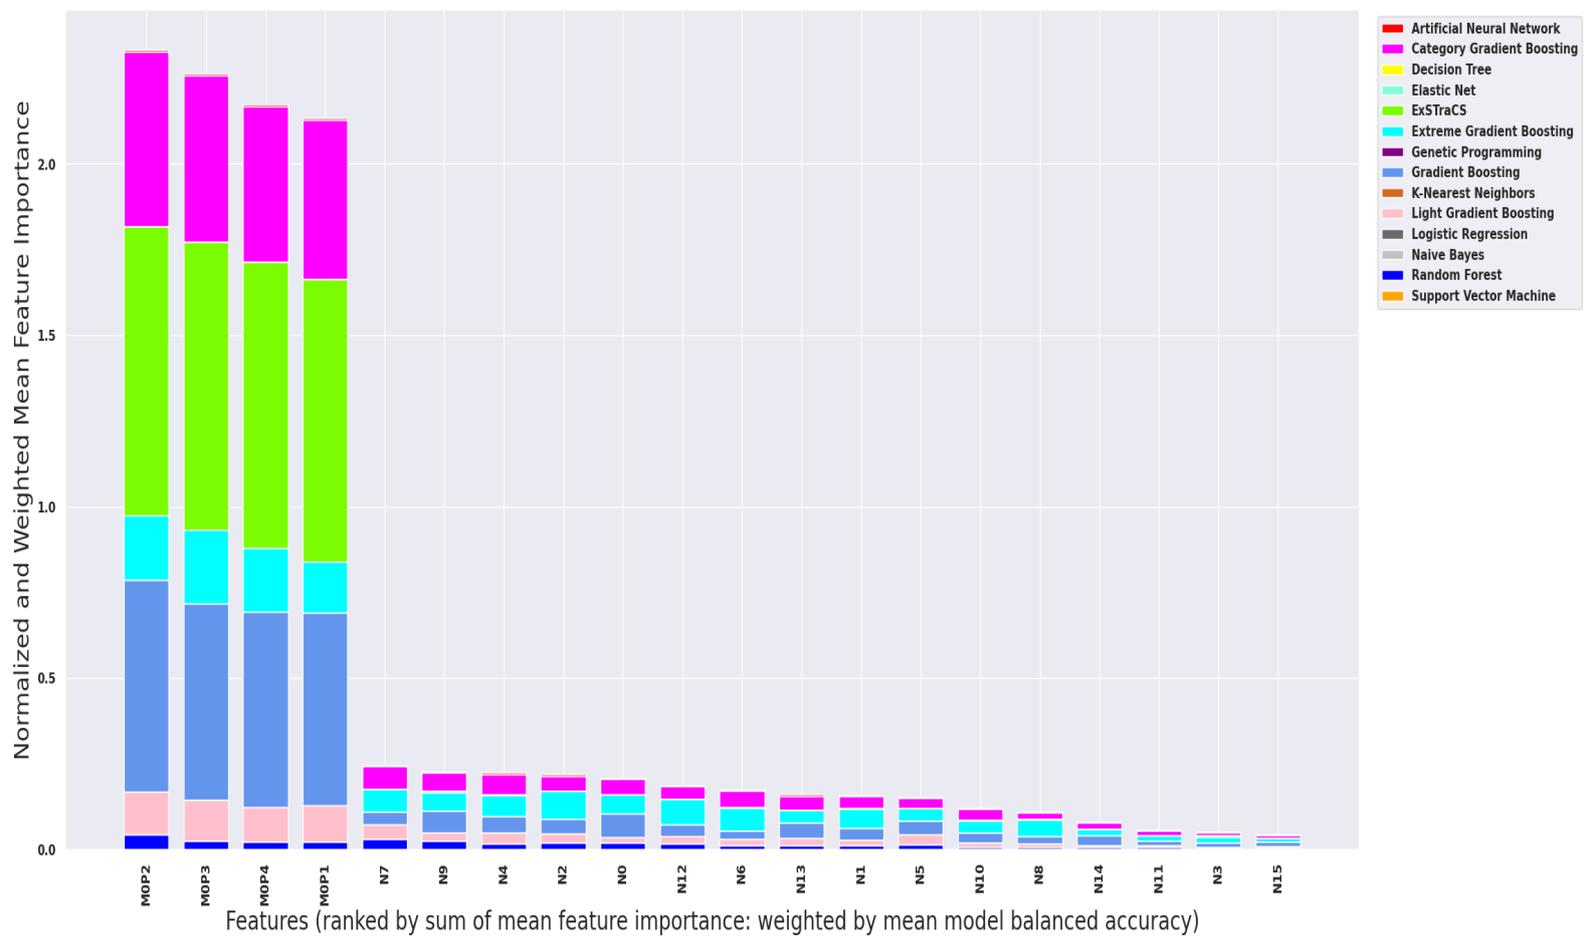

# Feature Importance Summary: D4 = xor\_5\_a\_20s\_1600\_EDM-1\_01

Sorted Median Mutual Information Scores

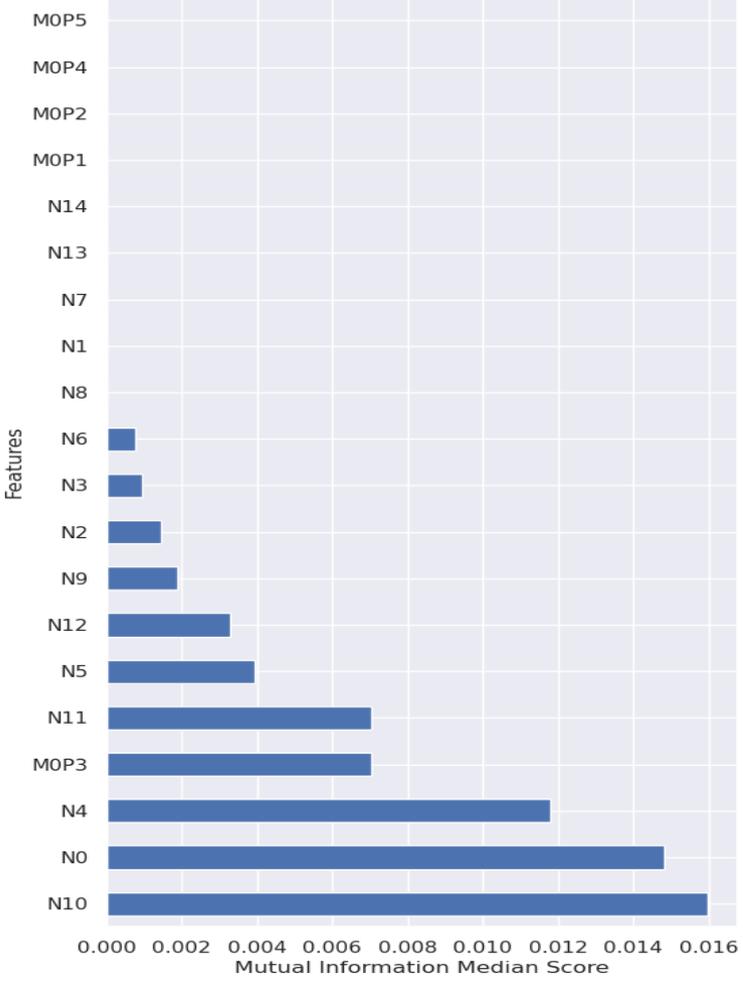

Sorted Median MultiSURF Scores

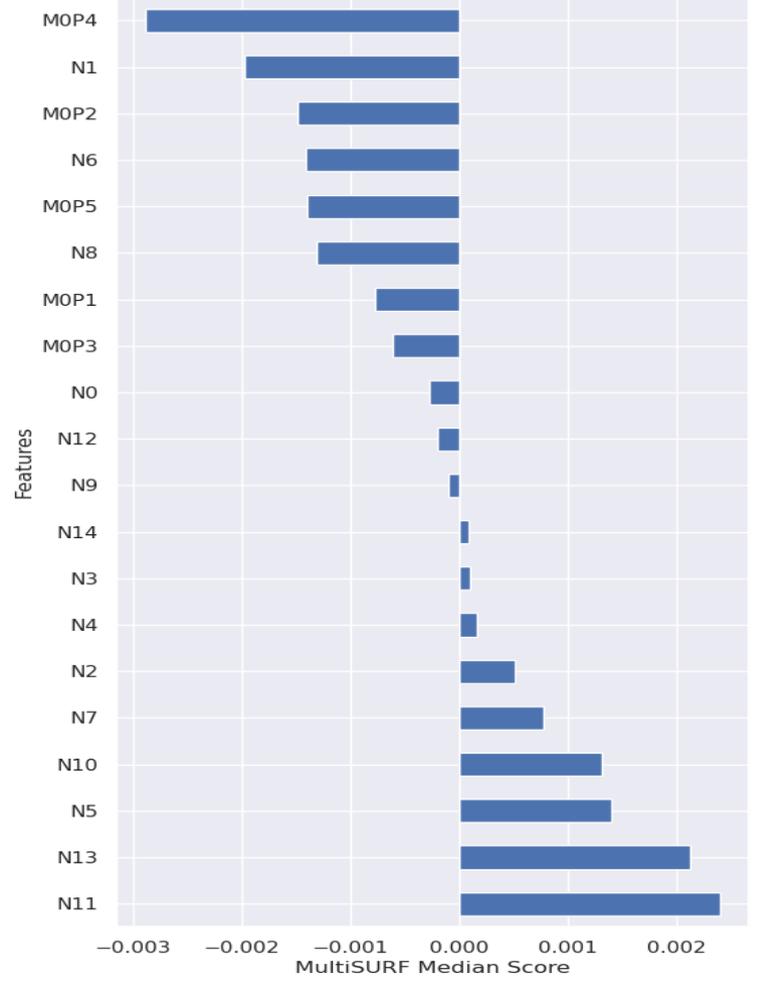

## Composite Feature Importance Plot (Normalized and Performance Weighted)

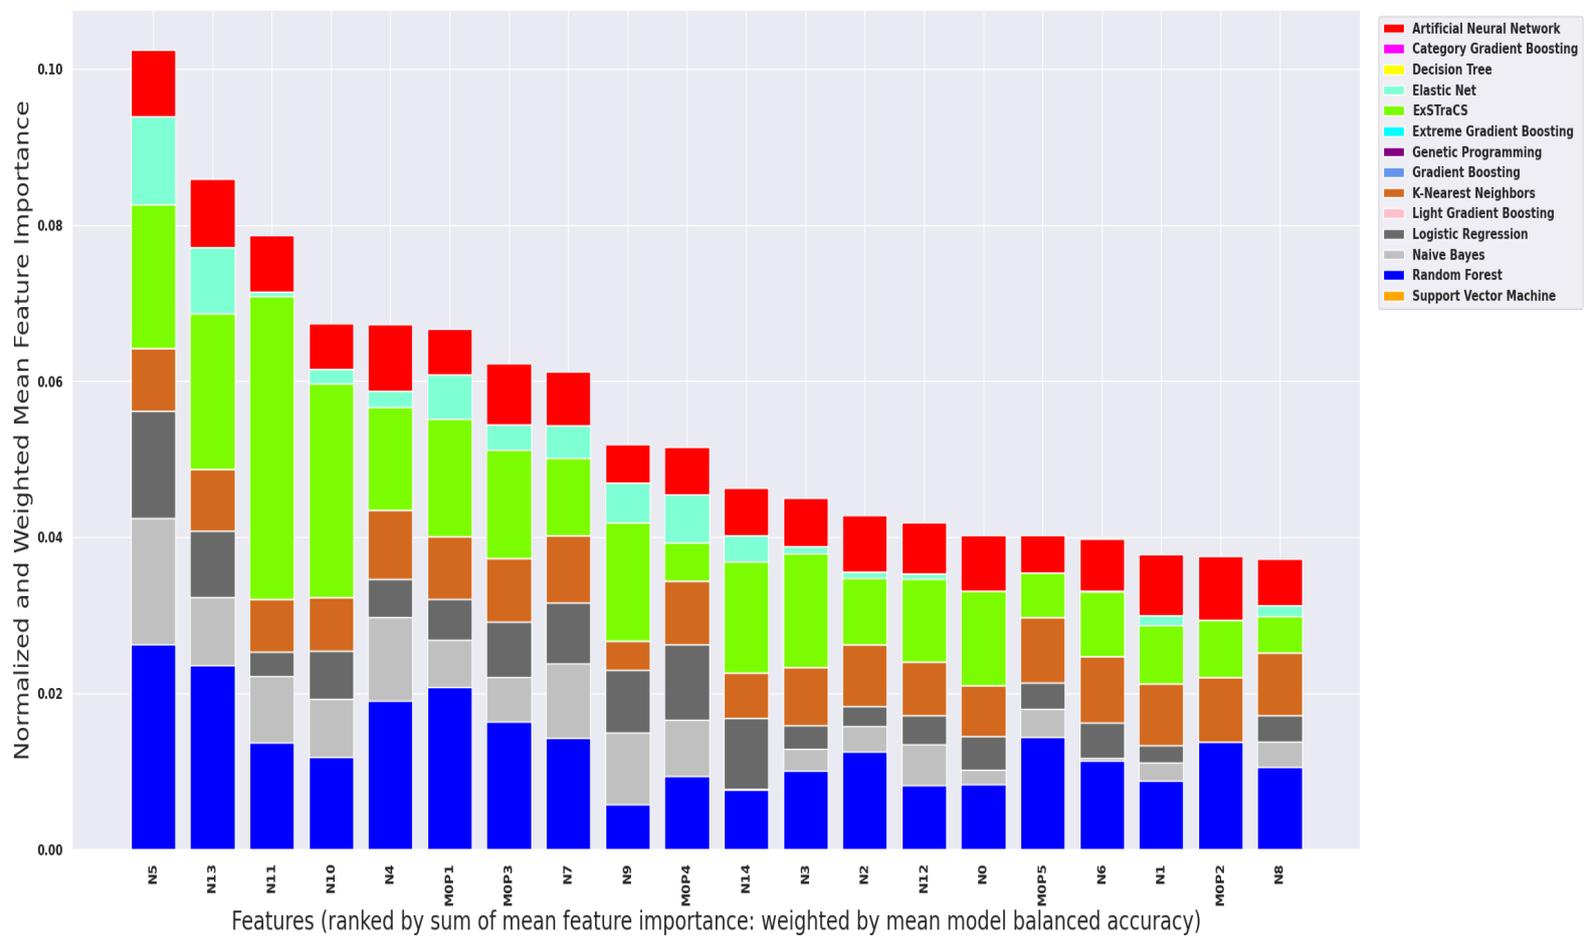

# Compare ML Performance Across Datasets

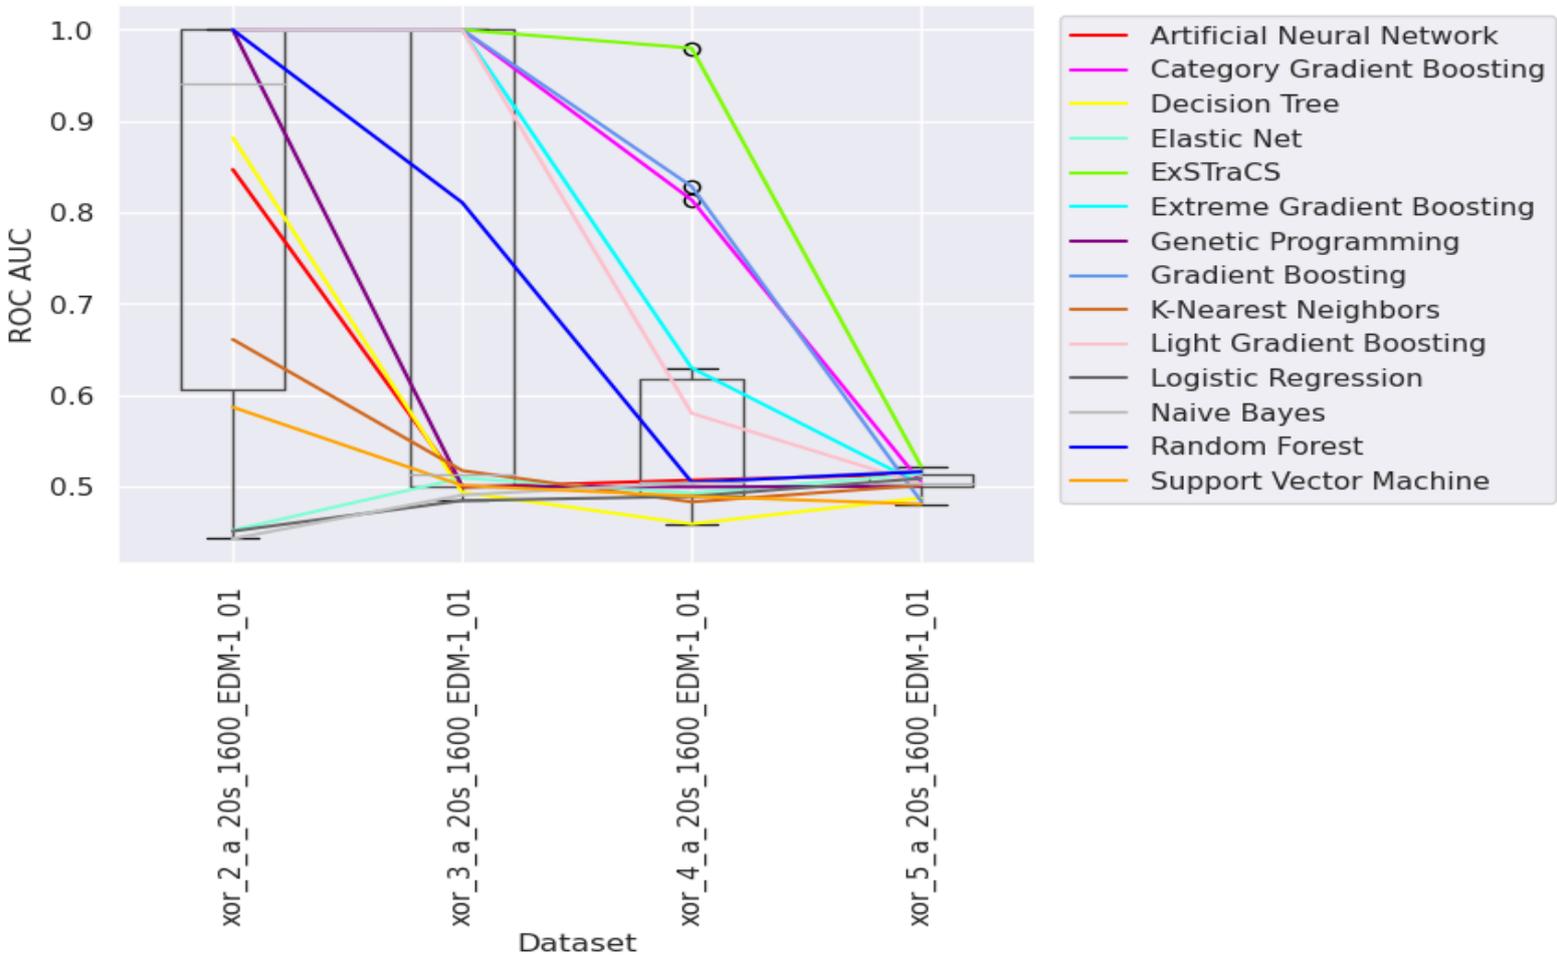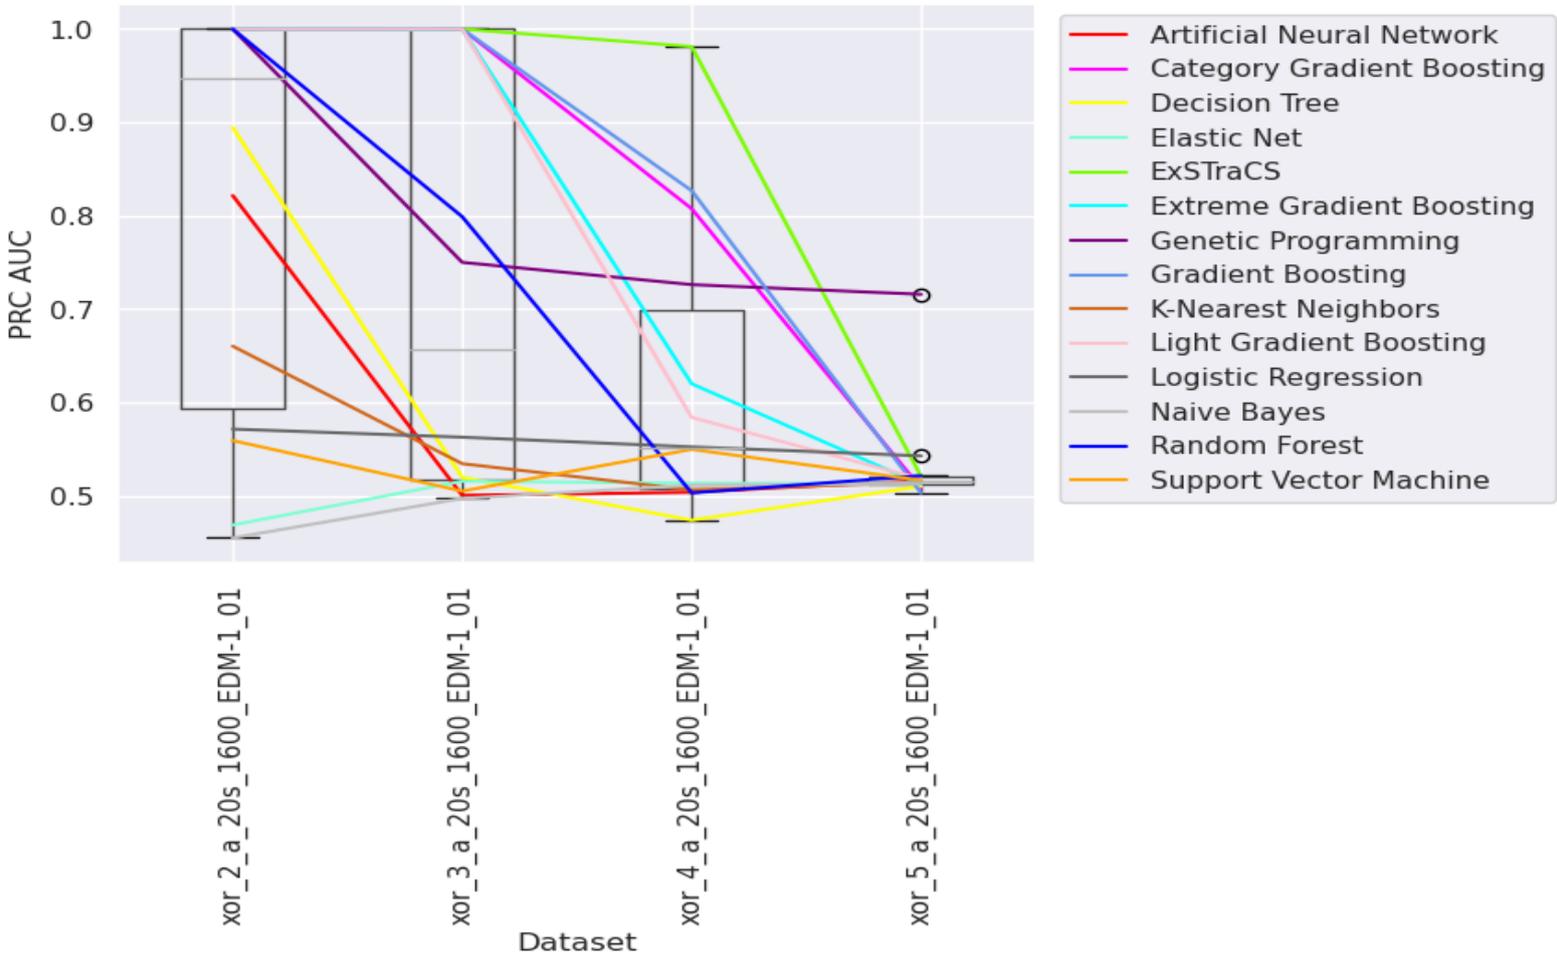

## Using Best Performing Algorithms (Kruskall Wallis Compare Datasets)

| Metrics              | P-Value | Best Alg_D1                | Median_D1 | Best Alg_D2                | Median_D2 | Best Alg_D3               | Median_D3 |
|----------------------|---------|----------------------------|-----------|----------------------------|-----------|---------------------------|-----------|
| Balanced Accuracy    | 0.0     | Category Gradient Boosting | 1.0       | Category Gradient Boosting | 1.0       | ExSTraCS                  | 0.9312    |
| Accuracy             | 0.0     | Category Gradient Boosting | 1.0       | Category Gradient Boosting | 1.0       | ExSTraCS                  | 0.9312    |
| F1 Score             | 0.0     | Category Gradient Boosting | 1.0       | Category Gradient Boosting | 1.0       | ExSTraCS                  | 0.9318    |
| Sensitivity (Recall) | 0.0     | Category Gradient Boosting | 1.0       | Category Gradient Boosting | 1.0       | ExSTraCS                  | 0.925     |
| Specificity          | 0.0781  | Category Gradient Boosting | 1.0       | Category Gradient Boosting | 1.0       | Genetic Programming       | 1.0       |
| Precision (PPV)      | 0.0     | Category Gradient Boosting | 1.0       | Category Gradient Boosting | 1.0       | ExSTraCS                  | 0.9449    |
| TP                   | 0.0     | Category Gradient Boosting | 80.0      | Category Gradient Boosting | 80.0      | ExSTraCS                  | 74.0      |
| TN                   | 0.0781  | Category Gradient Boosting | 80.0      | Category Gradient Boosting | 80.0      | Genetic Programming       | 80.0      |
| FP                   | 0.0097  | Elastic Net                | 48.0      | Artificial Neural Network  | 45.5      | Artificial Neural Network | 61.0      |
| FN                   | 0.0148  | Logistic Regression        | 51.0      | Genetic Programming        | 80.0      | Genetic Programming       | 80.0      |
| NPV                  | 0.0     | Category Gradient Boosting | 1.0       | Category Gradient Boosting | 1.0       | ExSTraCS                  | 0.9286    |
| LR+                  | 0.0     | Artificial Neural Network  | 3.0663    | Random Forest              | 2.7917    | ExSTraCS                  | 17.275    |
| LR-                  | 0.15    | Naive Bayes                | 1.3974    | Naive Bayes                | 1.0847    | Decision Tree             | 1.0763    |
| ROC AUC              | 0.0     | Category Gradient Boosting | 1.0       | Category Gradient Boosting | 1.0       | ExSTraCS                  | 0.9818    |
| PRC AUC              | 0.0     | Category Gradient Boosting | 1.0       | Category Gradient Boosting | 1.0       | ExSTraCS                  | 0.983     |
| PRC APS              | 0.0     | Category Gradient Boosting | 1.0       | Category Gradient Boosting | 1.0       | ExSTraCS                  | 0.9831    |

| Metrics              | P-Value | Best Alg_D4            | Median_D4 |
|----------------------|---------|------------------------|-----------|
| Balanced Accuracy    | 0.0     | ExSTraCS               | 0.5219    |
| Accuracy             | 0.0     | ExSTraCS               | 0.5219    |
| F1 Score             | 0.0     | Elastic Net            | 0.5259    |
| Sensitivity (Recall) | 0.0     | Support Vector Machine | 0.5438    |
| Specificity          | 0.0781  | Genetic Programming    | 1.0       |
| Precision (PPV)      | 0.0     | ExSTraCS               | 0.5198    |
| TP                   | 0.0     | Support Vector Machine | 43.5      |
| TN                   | 0.0781  | Genetic Programming    | 80.0      |
| FP                   | 0.0097  | Support Vector Machine | 42.0      |
| FN                   | 0.0148  | Genetic Programming    | 80.0      |
| NPV                  | 0.0     | ExSTraCS               | 0.5207    |
| LR+                  | 0.0     | ExSTraCS               | 1.0829    |
| LR-                  | 0.15    | Gradient Boosting      | 1.0868    |
| ROC AUC              | 0.0     | ExSTraCS               | 0.527     |
| PRC AUC              | 0.0     | Genetic Programming    | 0.75      |
| PRC APS              | 0.0     | ExSTraCS               | 0.5324    |

## Pipeline Runtime Summary

### xor\_2\_a\_20s\_1600\_EDM-1\_01

| Pipeline Component                      | Phase | Time (sec)         |
|-----------------------------------------|-------|--------------------|
| Exploratory Analysis                    | 1     | 3.0641753673553467 |
| Scale and Impute                        | 2     | 0.5761666297912598 |
| Mutual Information (Feature Importance) | 3     | 1.2682886123657229 |
| MultiSURF (Feature Importance)          | 3     | 145.02469658851624 |
| Feature Selection                       | 4     | 0.6764473915100098 |
| Artificial Neural Network(Modeling)     | 5     | 3130.707916736603  |
| Category Gradient Boosting(Modeling)    | 5     | 9690.398255586624  |
| Decision Tree(Modeling)                 | 5     | 27.0238299369812   |
| Elastic Net(Modeling)                   | 5     | 39.38248324394226  |
| ExSTraCS(Modeling)                      | 5     | 18330.742682933807 |
| Extreme Gradient Boosting(Modeling)     | 5     | 7293.579026222229  |
| Genetic Programming(Modeling)           | 5     | 11647.765572547913 |
| Gradient Boosting(Modeling)             | 5     | 3307.247713804245  |
| K-Nearest Neighbors(Modeling)           | 5     | 389.5638744831085  |
| Light Gradient Boosting(Modeling)       | 5     | 792.0739045143127  |
| Logistic Regression(Modeling)           | 5     | 30.819337844848636 |
| Naive Bayes(Modeling)                   | 5     | 2.143057346343994  |
| Random Forest(Modeling)                 | 5     | 7364.39542222023   |
| Support Vector Machine(Modeling)        | 5     | 6726.231264829636  |
| Stats Summary                           | 6     | 27.392427682876587 |

### xor\_3\_a\_20s\_1600\_EDM-1\_01

| Pipeline Component                      | Phase | Time (sec)         |
|-----------------------------------------|-------|--------------------|
| Exploratory Analysis                    | 1     | 2.5221493244171143 |
| Scale and Impute                        | 2     | 0.568861722946167  |
| Mutual Information (Feature Importance) | 3     | 1.2114510536193848 |
| MultiSURF (Feature Importance)          | 3     | 144.6504111289978  |
| Feature Selection                       | 4     | 0.7352635860443115 |
| Artificial Neural Network(Modeling)     | 5     | 2047.5548272132876 |
| Category Gradient Boosting(Modeling)    | 5     | 9570.083825588226  |
| Decision Tree(Modeling)                 | 5     | 26.238165616989136 |
| Elastic Net(Modeling)                   | 5     | 36.95730662345886  |
| ExSTraCS(Modeling)                      | 5     | 22486.603338956837 |
| Extreme Gradient Boosting(Modeling)     | 5     | 8834.424510717392  |
| Genetic Programming(Modeling)           | 5     | 11283.093751192093 |
| Gradient Boosting(Modeling)             | 5     | 5698.811798095703  |
| K-Nearest Neighbors(Modeling)           | 5     | 1550.8836629390717 |
| Light Gradient Boosting(Modeling)       | 5     | 1651.2995171546936 |
| Logistic Regression(Modeling)           | 5     | 35.38793110847473  |
| Naive Bayes(Modeling)                   | 5     | 2.1282293796539307 |
| Random Forest(Modeling)                 | 5     | 8980.076310157776  |
| Support Vector Machine(Modeling)        | 5     | 5477.692789554596  |
| Stats Summary                           | 6     | 35.92071866989136  |

### xor\_4\_a\_20s\_1600\_EDM-1\_01

| Pipeline Component                      | Phase | Time (sec)         |
|-----------------------------------------|-------|--------------------|
| Exploratory Analysis                    | 1     | 2.571923017501831  |
| Scale and Impute                        | 2     | 0.5517351627349854 |
| Mutual Information (Feature Importance) | 3     | 1.1954491138458252 |
| MultiSURF (Feature Importance)          | 3     | 144.2349021434784  |
| Feature Selection                       | 4     | 0.9309043884277344 |
| Artificial Neural Network(Modeling)     | 5     | 1220.663622379303  |
| Category Gradient Boosting(Modeling)    | 5     | 9693.93657040596   |
| Decision Tree(Modeling)                 | 5     | 25.483894109725952 |
| Elastic Net(Modeling)                   | 5     | 40.83524131774902  |
| ExSTraCS(Modeling)                      | 5     | 35908.66883325577  |
| Extreme Gradient Boosting(Modeling)     | 5     | 6187.943474054337  |
| Genetic Programming(Modeling)           | 5     | 10896.477407455444 |
| Gradient Boosting(Modeling)             | 5     | 9037.12207865715   |
| K-Nearest Neighbors(Modeling)           | 5     | 3650.027170658112  |
| Light Gradient Boosting(Modeling)       | 5     | 2109.323344707489  |
| Logistic Regression(Modeling)           | 5     | 37.49015116691589  |
| Naive Bayes(Modeling)                   | 5     | 2.330973625183105  |
| Random Forest(Modeling)                 | 5     | 4867.79810667038   |
| Support Vector Machine(Modeling)        | 5     | 5666.484535217285  |
| Stats Summary                           | 6     | 32.07957887649536  |

### xor\_5\_a\_20s\_1600\_EDM-1\_01

| Pipeline Component                      | Phase | Time (sec)         |
|-----------------------------------------|-------|--------------------|
| Exploratory Analysis                    | 1     | 3.0902271270751958 |
| Scale and Impute                        | 2     | 0.5537581443786621 |
| Mutual Information (Feature Importance) | 3     | 1.1895241737365725 |
| MultiSURF (Feature Importance)          | 3     | 143.6202838420868  |
| Feature Selection                       | 4     | 0.8595414161682129 |
| Artificial Neural Network(Modeling)     | 5     | 3243.3570375442505 |
| Category Gradient Boosting(Modeling)    | 5     | 9251.708213329315  |
| Decision Tree(Modeling)                 | 5     | 27.77396583557129  |
| Elastic Net(Modeling)                   | 5     | 44.86685919761658  |
| ExSTraCS(Modeling)                      | 5     | 40980.76172685623  |
| Extreme Gradient Boosting(Modeling)     | 5     | 6289.808042526245  |
| Genetic Programming(Modeling)           | 5     | 10805.960580348969 |
| Gradient Boosting(Modeling)             | 5     | 7488.537938117981  |
| K-Nearest Neighbors(Modeling)           | 5     | 2781.982298135757  |
| Light Gradient Boosting(Modeling)       | 5     | 1410.9272165298462 |
| Logistic Regression(Modeling)           | 5     | 38.25356483459473  |
| Naive Bayes(Modeling)                   | 5     | 2.3054206371307373 |
| Random Forest(Modeling)                 | 5     | 4442.682507514954  |
| Support Vector Machine(Modeling)        | 5     | 4996.406463861465  |
| Stats Summary                           | 6     | 35.730658531188965 |
